# Supplementary material for: Symmetry Principles in Quantum Systems Theory
Source: arXiv:1012.5256 ancillary file (2011-07-21)
Supplement: Supplementary file 1 [file supplement.pdf]

# Electronic Supplementary Material for
# “Symmetry Principles in Quantum Systems Theory”

Robert Zeier, Thomas Schulte-Herbrüggen
Department of Chemistry, Technical University of Munich (TUM)
Lichtenbergstrasse 4, 85747 Garching, Germany
E-mail: robert.zeier@ch.tum.de; tosh@ch.tum.de

Received: March 4, 2011 / Accepted: date

**Abstract**

This is the electronic supplementary material to our work “Symmetry Principles in Quantum Systems Theory”. We tabulate the irreducible simple subalgebras of $\mathfrak{su}(N)$ for $2 \leq N \leq 2^{15}$ excluding certain trivial cases.

## 1 Introduction

This is the electronic supplementary material to our work “Symmetry Principles in Quantum Systems Theory”. We tabulate the irreducible simple subalgebras of $\mathfrak{su}(N)$ for $2 \leq N \leq 2^{15}$ excluding certain trivial cases. In addition, we present sufficient information in order to determine the (equivalence classes of) representations corresponding to the subalgebras.

### 1.1 Notation

Later, we list two pieces of information for certain non-trivial cases of $\mathfrak{su}(N)$, where $2 \leq N \leq 2^{15}$. First, we present a tree of all irreducible simple subalgebras of $\mathfrak{su}(N)$, e.g.:

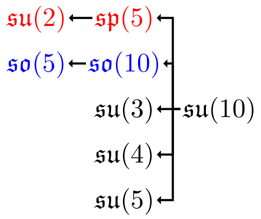


The symplectic subalgebras [i.e. subalgebras of $\mathfrak{sp}(N/2)$] are given in red, the orthogonal subalgebras [i.e. subalgebras of $\mathfrak{so}(N)$] are given in blue, and the unitary subalgebras [i.e. the rest] are given in black. The algebra $\mathfrak{su}(N)$ is the root of the tree. A directed edge of the tree connects [in the set of irreducible simple subalgebras of $\mathfrak{su}(N)$] an algebra with one of its maximal subalgebras.

Next, a comma-separated sequence of comma-separated lists of highest weights is given, e.g.:

$$[\{\langle 1,1\rangle\},\{\langle 9,1\rangle\}],[(1,0,0,0,0)],[(9)],[(1,0,0,0,0)],[(0,2)],[(3,0),(0,3)],[(2,0,0),(0,0,2)],[(0,1,0,0),(0,0,1,0)]$$

Each list of highest weights is enclosed in square brackets and identifies representations corresponding to the same irreducible simple subalgebra, where the representations are equivalent under outer automorphisms of the subalgebra. Each highest weight is given as a vector (with round brackets) if the rank $\ell \leq 5$.[1] Otherwise, the highest weight is given as a set of pairs corresponding to non-zero entries of the vector, where a pair determines the position and the value (in that order) of a non-zero element. We remark that the comma-separated sequence is ordered depth-first, e.g.:

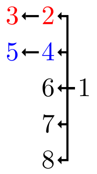


[1]Recall that the rank $\ell$ is determined by the Lie algebra: $\mathfrak{su}(\ell+1)$, $\mathfrak{so}(2\ell+1)$, $\mathfrak{sp}(2\ell)$, $\mathfrak{so}(2\ell)$, $\mathfrak{e}_\ell$, $\mathfrak{f}_\ell$, and $\mathfrak{g}_\ell$.

## 1.2 Trivial cases

In order to save space, we will not list two types of trivial cases, even more so as the presented information can be readily determined as discussed now:

First, if $N \geq 5$ is *even* and if $\mathfrak{sp}(N/2)$, $\mathfrak{so}(N)$, as well as $\mathfrak{su}(2) \subset \mathfrak{sp}(N/2)$ are the only proper irreducible simple subalgebras, then we say the case is trivial. An example is given by $\mathfrak{su}(12)$:

$$\begin{array}{l} \mathfrak{su}(2) \leftarrow \mathfrak{sp}(6) \leftarrow \\ \qquad\qquad \mathfrak{so}(12) \leftarrow \end{array} \Big] \mathfrak{su}(12)$$

We remark that also the corresponding highest weights can be easily determined: For $\mathfrak{su}(N)$ $[N > 2]$, we get two vectors: the only non-zero entry is, respectively, the first one and the last one, and its value is equal to one. For $\mathfrak{so}(2\ell)$ $[\ell \neq 4]$ and $\mathfrak{sp}(\ell)$, we get the vector whose only non-zero entry is the first one, which in both cases is equal to one. For $\mathfrak{su}(2)$, we get the vector $(N-1)$ of length one. In the example of $\mathfrak{su}(12)$, we have the following highest weights:

$$[\{\langle 1,1\rangle\},\{\langle 11,1\rangle\}],[\{\langle 1,1\rangle\}],[(11)],[\{\langle 1,1\rangle\}]$$

Second, if $N \geq 5$ is *odd* and if $\mathfrak{so}(N)$ as well as $\mathfrak{su}(2) \subset \mathfrak{so}(N)$ are the only proper irreducible simple subalgebras, then we also say the case is trivial. An example is given by $\mathfrak{su}(5)$:

$$\mathfrak{su}(2) \leftarrow \mathfrak{so}(5) \leftarrow \mathfrak{su}(5)$$

We remark that the corresponding highest weights can be determined along the same lines as for even $N$. In the example of $\mathfrak{su}(5)$, we have the following highest weights:

$$[(1,0,0,0),(0,0,0,1)],[(1,0)],[(4)]$$

# 2 Table

The complete table listing all the irreducible simple subalgebras of $\mathfrak{su}(N)$ for $2 \leq N \leq 2^{15}$ (only excluding the trivial cases) starts on the next page.

$\mathfrak{su}(2)$

[(1)]

---

$\mathfrak{su}(2) \leftarrow \mathfrak{su}(3)$

[(1,0),(0,1)],[(2)]

---

$\mathfrak{su}(2) \leftarrow \mathfrak{sp}(2) \leftarrow \mathfrak{su}(4)$

[(1,0,0),(0,0,1)],[(1,0)],[(3)]

---

$\mathfrak{su}(2) \leftarrow \mathfrak{sp}(3)$, $\mathfrak{so}(6)$, $\mathfrak{su}(3)$ $\leftarrow \mathfrak{su}(6)$

[(1,0,0,0,0),(0,0,0,0,1)], [(1,0,0)], [(5)], [(1,0,0)], [(2,0),(0,2)]

---

$\mathfrak{su}(2) \leftarrow \mathfrak{g}_2 \leftarrow \mathfrak{so}(7) \leftarrow \mathfrak{su}(7)$

[{⟨1,1⟩},{⟨6,1⟩}],[(1,0,0)],[(1,0)],[(6)]

---

$\mathfrak{su}(2) \leftarrow \mathfrak{sp}(4)$; $\mathfrak{su}(3)$, $\mathfrak{so}(7)$ $\leftarrow \mathfrak{so}(8)$; $\mathfrak{sp}(4)$, $\mathfrak{so}(8)$ $\leftarrow \mathfrak{su}(8)$

[{⟨1,1⟩},{⟨7,1⟩}], [(1,0,0,0)], [(7)], [(1,0,0,0),(0,0,1,0),(0,0,0,1)],[(1,1)],[(0,0,1)]

---

$\mathfrak{su}(2) \leftarrow \mathfrak{sp}(5)$; $\mathfrak{so}(5) \leftarrow \mathfrak{so}(10)$; $\mathfrak{sp}(5)$, $\mathfrak{so}(10)$, $\mathfrak{su}(3)$, $\mathfrak{su}(4)$, $\mathfrak{su}(5)$ $\leftarrow \mathfrak{su}(10)$

[{⟨1,1⟩},{⟨9,1⟩}], [(1,0,0,0,0)], [(9)], [(1,0,0,0,0)], [(0,2)], [(3,0),(0,3)], [(2,0,0),(0,0,2)], [(0,1,0,0),(0,0,1,0)]

---

$\mathfrak{su}(2)$, $\mathfrak{sp}(3)$ $\leftarrow \mathfrak{sp}(7)$; $\mathfrak{so}(5)$, $\mathfrak{sp}(3)$, $\mathfrak{g}_2$ $\leftarrow \mathfrak{so}(14)$; $\mathfrak{sp}(7)$, $\mathfrak{so}(14)$ $\leftarrow \mathfrak{su}(14)$

[{⟨1,1⟩},{⟨13,1⟩}], [{⟨1,1⟩}], [(13)], [(0,0,1)], [{⟨1,1⟩}],[(2,0)],[(0,1,0)],[(0,1)]

---

$\mathfrak{su}(2)$, $\mathfrak{so}(6)$ $\leftarrow \mathfrak{so}(15)$; $\mathfrak{su}(3) \leftarrow \mathfrak{su}(6)$; $\mathfrak{so}(15)$, $\mathfrak{su}(3)$, $\mathfrak{su}(5)$, $\mathfrak{su}(6)$ $\leftarrow \mathfrak{su}(15)$

[{⟨1,1⟩},{⟨14,1⟩}], [{⟨1,1⟩}], [(14)], [(0,1,1)], [(4,0),(0,4)], [(2,0,0,0),(0,0,0,2)], [(0,1,0,0,0),(0,0,0,1,0)],[(2,1),(1,2)]

---

$\mathfrak{su}(2)$, $\mathfrak{sp}(2)$ $\leftarrow \mathfrak{sp}(8)$; $\mathfrak{so}(9) \leftarrow \mathfrak{so}(16)$; $\mathfrak{sp}(8)$, $\mathfrak{so}(16)$, $\mathfrak{so}(10)$ $\leftarrow \mathfrak{su}(16)$

[{⟨1,1⟩},{⟨15,1⟩}],[{⟨1,1⟩}],[(15)],[(1,1)],[{⟨1,1⟩}],[(0,0,0,1)],[(0,0,0,1,0),(0,0,0,0,1)]

---

$\mathfrak{su}(2)$, $\mathfrak{su}(6)$, $\mathfrak{sp}(2)$ $\leftarrow \mathfrak{sp}(10)$; $\mathfrak{so}(6) \leftarrow \mathfrak{so}(20)$; $\mathfrak{sp}(10)$, $\mathfrak{so}(20)$, $\mathfrak{su}(4)$, $\mathfrak{su}(4)$ $\leftarrow \mathfrak{su}(20)$

[{⟨1,1⟩},{⟨19,1⟩}], [{⟨1,1⟩}], [(19)], [(0,0,1,0,0)], [(3,0)], [{⟨1,1⟩}], [(2,0,0)], [(1,1,0),(0,1,1)], [(3,0),(0,0,3)]

---

$\mathfrak{su}(2)$, $\mathfrak{sp}(3)$ $\leftarrow \mathfrak{so}(7) \leftarrow \mathfrak{so}(21)$; $\mathfrak{so}(21)$, $\mathfrak{su}(3)$, $\mathfrak{su}(6)$, $\mathfrak{su}(7)$ $\leftarrow \mathfrak{su}(21)$

[{⟨1,1⟩},{⟨20,1⟩}], [{⟨1,1⟩}], [(20)], [(0,1,0)], [(2,0,0)],[(5,0),(0,5)],[(2,0,0,0,0),(0,0,0,0,2)],[{⟨2,1⟩},{⟨5,1⟩}]

---

$\mathfrak{su}(2) \leftarrow \mathfrak{sp}(12)$; $\mathfrak{so}(5) \leftarrow \mathfrak{so}(24)$; $\mathfrak{sp}(12)$, $\mathfrak{so}(24)$, $\mathfrak{su}(3)$ $\leftarrow \mathfrak{su}(24)$

[{⟨1,1⟩},{⟨23,1⟩}], [{⟨1,1⟩}], [(23)], [{⟨1,1⟩}], [(1,0,0,1)],[(3,1),(1,3)]

---

$\mathfrak{su}(2) \leftarrow \mathfrak{sp}(13)$; $\mathfrak{f}_4 \leftarrow \mathfrak{so}(26)$; $\mathfrak{sp}(13)$, $\mathfrak{so}(26)$ $\leftarrow \mathfrak{su}(26)$

[{⟨1,1⟩},{⟨25,1⟩}], [{⟨1,1⟩}], [(25)], [{⟨1,1⟩}], [(0,0,0,1)]

---

$\mathfrak{su}(2)$, $\mathfrak{su}(3)$, $\mathfrak{so}(7)$, $\mathfrak{sp}(4)$ $\leftarrow \mathfrak{so}(27)$; $\mathfrak{g}_2 \leftarrow \mathfrak{so}(7)$; $\mathfrak{so}(27)$, $\mathfrak{e}_6$ $\leftarrow \mathfrak{su}(27)$

[{⟨1,1⟩},{⟨26,1⟩}],[{⟨1,1⟩}],[(26)],[(2,2)],[(2,0,0)],[(2,0)],[(0,1,0,0)],[{⟨1,1⟩},{⟨6,1⟩}]

---

$\mathfrak{su}(2) \leftarrow \mathfrak{sp}(14)$; $\mathfrak{so}(8) \leftarrow \mathfrak{so}(28)$; $\mathfrak{sp}(14)$, $\mathfrak{so}(28)$, $\mathfrak{su}(3)$, $\mathfrak{su}(7)$, $\mathfrak{su}(8)$ $\leftarrow \mathfrak{su}(28)$

[{⟨1,1⟩},{⟨27,1⟩}], [{⟨1,1⟩}], [(27)], [{⟨1,1⟩}], [(0,1,0,0)], [(6,0),(0,6)], [{⟨1,2⟩},{⟨6,2⟩}], [{⟨2,1⟩},{⟨6,1⟩}]

---

$\mathfrak{su}(2) \leftarrow \mathfrak{sp}(15)$; $\mathfrak{so}(5) \leftarrow \mathfrak{so}(30)$; $\mathfrak{sp}(15)$, $\mathfrak{so}(30)$ $\leftarrow \mathfrak{su}(30)$

[{⟨1,1⟩},{⟨29,1⟩}],[{⟨1,1⟩}],[(29)],[{⟨1,1⟩}],[(3,0)]

---

$\mathfrak{so}(11) \leftarrow \mathfrak{so}(12)$; $\mathfrak{su}(2)$, $\mathfrak{so}(12)$ $\leftarrow \mathfrak{sp}(16)$; $\mathfrak{sp}(16)$, $\mathfrak{so}(32)$ $\leftarrow \mathfrak{su}(32)$

[{⟨1,1⟩},{⟨31,1⟩}], [{⟨1,1⟩}], [(31)], [{⟨5,1⟩},{⟨6,1⟩}],[(0,0,0,0,1)],[{⟨1,1⟩}]

---

$\mathfrak{so}(7) \leftarrow \mathfrak{so}(8)$; $\mathfrak{su}(2)$, $\mathfrak{su}(6)$, $\mathfrak{so}(5)$, $\mathfrak{so}(5)$, $\mathfrak{so}(8)$ $\leftarrow \mathfrak{so}(35)$; $\mathfrak{so}(35)$, $\mathfrak{su}(3)$, $\mathfrak{su}(4)$, $\mathfrak{su}(5)$, $\mathfrak{su}(7)$ $\leftarrow \mathfrak{su}(35)$

[{⟨1,1⟩},{⟨34,1⟩}], [{⟨1,1⟩}], [(34)], [(1,0,0,0,1)], [(0,4)], [(1,2)], [(2,0,0,0),(0,0,2,0),(0,0,0,2)], [(0,2)], [(4,1),(1,4)], [(4,0,0),(0,0,4)], [(3,0,0,0),(0,0,0,3)],[{⟨3,1⟩},{⟨4,1⟩}]

---

$\mathfrak{su}(2) \leftarrow \mathfrak{sp}(18)$; $\mathfrak{so}(9)$, $\mathfrak{sp}(4)$ $\leftarrow \mathfrak{so}(36)$; $\mathfrak{sp}(18)$, $\mathfrak{so}(36)$, $\mathfrak{su}(3)$, $\mathfrak{su}(4)$, $\mathfrak{su}(8)$, $\mathfrak{su}(9)$ $\leftarrow \mathfrak{su}(36)$

[{⟨1,1⟩},{⟨35,1⟩}], [{⟨1,1⟩}], [(35)], [{⟨1,1⟩}], [(0,1,0,0)], [(2,0,0,0)], [(7,0),(0,7)], [(2,0,1),(1,0,2)], [{⟨1,2⟩},{⟨7,2⟩}],[{⟨2,1⟩},{⟨7,1⟩}]

---

$\mathfrak{su}(2)$, $\mathfrak{sp}(2)$ $\leftarrow \mathfrak{sp}(20)$; $\mathfrak{sp}(20)$, $\mathfrak{so}(40)$, $\mathfrak{su}(5)$ $\leftarrow \mathfrak{su}(40)$

[{⟨1,1⟩},{⟨39,1⟩}],[{⟨1,1⟩}],[(39)],[(1,2)],[{⟨1,1⟩}],[(1,1,0,0),(0,0,1,1)]

---

$\mathfrak{su}(2) \leftarrow \mathfrak{sp}(21)$; $\mathfrak{sp}(4) \leftarrow \mathfrak{so}(42)$; $\mathfrak{sp}(21)$, $\mathfrak{so}(42)$, $\mathfrak{su}(3)$ $\leftarrow \mathfrak{su}(42)$

[{⟨1,1⟩},{⟨41,1⟩}], [{⟨1,1⟩}], [(41)], [{⟨1,1⟩}], [(0,0,0,1)],[(3,2),(2,3)]

---

$\mathfrak{su}(2) \leftarrow \mathfrak{sp}(22)$; $\mathfrak{so}(9)$, $\mathfrak{sp}(5)$ $\leftarrow \mathfrak{so}(44)$; $\mathfrak{sp}(22)$, $\mathfrak{so}(44)$ $\leftarrow \mathfrak{su}(44)$

[{⟨1,1⟩},{⟨43,1⟩}], [{⟨1,1⟩}], [(43)], [{⟨1,1⟩}], [(2,0,0)],[(0,1,0,0,0)]

---

$\mathfrak{su}(2)$, $\mathfrak{so}(10)$ $\leftarrow \mathfrak{so}(45)$; $\mathfrak{su}(4)$, $\mathfrak{su}(5)$ $\leftarrow \mathfrak{su}(10)$; $\mathfrak{so}(45)$, $\mathfrak{su}(3)$, $\mathfrak{su}(9)$, $\mathfrak{su}(10)$ $\leftarrow \mathfrak{su}(45)$

[{⟨1,1⟩},{⟨44,1⟩}], [{⟨1,1⟩}], [(44)], [(0,1,0,0,0)], [(8,0),(0,8)], [{⟨1,2⟩},{⟨8,2⟩}], [{⟨2,1⟩},{⟨8,1⟩}], [(2,1,0),(0,1,2)],[(1,0,1,0),(0,1,0,1)]

---

$\mathfrak{su}(2)$, $\mathfrak{sp}(4)$ $\leftarrow \mathfrak{sp}(24)$; $\mathfrak{su}(7)$, $\mathfrak{so}(7)$ $\leftarrow \mathfrak{so}(48)$; $\mathfrak{sp}(24)$, $\mathfrak{so}(48)$, $\mathfrak{su}(3)$ $\leftarrow \mathfrak{su}(48)$

[{⟨1,1⟩},{⟨47,1⟩}], [{⟨1,1⟩}], [(47)], [(0,0,1,0)], [{⟨1,1⟩}],[{⟨1,1⟩, ⟨6,1⟩}],[(1,0,1)],[(5,1),(1,5)]

---

$\mathfrak{su}(2) \leftarrow \mathfrak{sp}(25)$; $\mathfrak{so}(6) \leftarrow \mathfrak{so}(50)$; $\mathfrak{sp}(25)$, $\mathfrak{so}(50)$, $\mathfrak{su}(5)$ $\leftarrow \mathfrak{su}(50)$

[{⟨1,1⟩},{⟨49,1⟩}], [{⟨1,1⟩}], [(49)], [{⟨1,1⟩}], [(3,0,0)],[(0,2,0,0),(0,0,2,0)]

---

$\mathfrak{su}(2) \leftarrow \mathfrak{sp}(26)$; $\mathfrak{f}_4 \leftarrow \mathfrak{so}(52)$; $\mathfrak{sp}(26)$, $\mathfrak{so}(52)$ $\leftarrow \mathfrak{su}(52)$

[{⟨1,1⟩},{⟨51,1⟩}], [{⟨1,1⟩}], [(51)], [{⟨1,1⟩}], [(1,0,0)]

---

$\mathfrak{su}(2) \leftarrow \mathfrak{sp}(27)$; $\mathfrak{so}(10) \leftarrow \mathfrak{so}(54)$; $\mathfrak{sp}(27)$, $\mathfrak{so}(54)$ $\leftarrow \mathfrak{su}(54)$

[{⟨1,1⟩},{⟨53,1⟩}], [{⟨1,1⟩}], [(53)], [{⟨1,1⟩}], [(2,0,0,0)]

---

$\mathfrak{su}(2)$, $\mathfrak{so}(5)$, $\mathfrak{so}(11)$, $\mathfrak{sp}(5)$ $\leftarrow \mathfrak{so}(55)$; $\mathfrak{so}(55)$, $\mathfrak{su}(3)$, $\mathfrak{su}(10)$, $\mathfrak{su}(11)$ $\leftarrow \mathfrak{su}(55)$

[{⟨1,1⟩},{⟨54,1⟩}], [{⟨1,1⟩}], [(54)], [(4,0)], [(0,1,0,0,0)], [(2,0,0,0,0)], [(9,0),(0,9)], [{⟨1,2⟩},{⟨9,2⟩}], [{⟨2,1⟩},{⟨9,1⟩}]

---

$\mathfrak{su}(2)$, $\mathfrak{sp}(2)$, $\mathfrak{sp}(3)$, $\mathfrak{e}_7$ $\leftarrow \mathfrak{sp}(28)$; $\mathfrak{so}(8) \leftarrow \mathfrak{so}(56)$; $\mathfrak{sp}(28)$, $\mathfrak{so}(56)$, $\mathfrak{su}(4)$, $\mathfrak{su}(6)$, $\mathfrak{su}(8)$ $\leftarrow \mathfrak{su}(56)$

[{⟨1, 1⟩},{⟨55, 1⟩}],[{⟨1, 1⟩}],[(55)],[(5, 0)],[(3, 0, 0)], [{⟨7, 1⟩}],[{⟨1, 1⟩}],[(1, 0, 1, 0),(1, 0, 0, 1),(0, 0, 1, 1)], [(5, 0, 0),(0, 0, 5)], [(3, 0, 0, 0, 0),(0, 0, 0, 0, 3)], [{⟨3, 1⟩},{⟨5, 1⟩}]

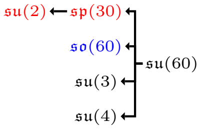


[{⟨1, 1⟩},{⟨59, 1⟩}],[{⟨1, 1⟩}],[(59)],[{⟨1, 1⟩}],[(4, 2),(2, 4)],[(1, 2, 0),(0, 2, 1)]

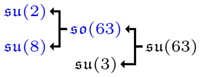


[{⟨1, 1⟩},{⟨62, 1⟩}],[{⟨1, 1⟩}],[(62)],[{⟨1, 1⟩, ⟨7, 1⟩}],[(6, 1),(1, 6)]

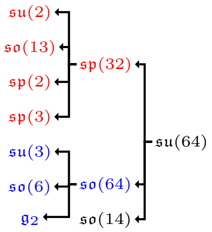


[{⟨1, 1⟩},{⟨63, 1⟩}],[{⟨1, 1⟩}],[(63)],[{⟨6, 1⟩}],[(3, 1)],[(1, 1, 0)],[{⟨1, 1⟩}],[(3, 3)],[(1, 1, 1)],[(1, 1)],[{⟨6, 1⟩},{⟨7, 1⟩}]

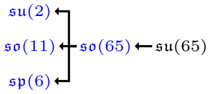


[{⟨1, 1⟩},{⟨64, 1⟩}], [{⟨1, 1⟩}], [(64)], [(2, 0, 0, 0, 0)], [{⟨2, 1⟩}]

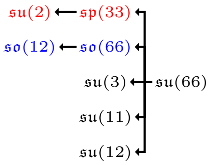


[{⟨1, 1⟩},{⟨65, 1⟩}], [{⟨1, 1⟩}], [(65)], [{⟨1, 1⟩}], [{⟨2, 1⟩}], [(10, 0),(0, 10)], [{⟨1, 2⟩},{⟨10, 2⟩}], [{⟨2, 1⟩},{⟨10, 1⟩}]

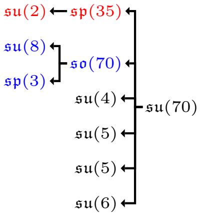


[{⟨1, 1⟩},{⟨69, 1⟩}], [{⟨1, 1⟩}], [(69)], [{⟨1, 1⟩}], [{⟨4, 1⟩}], [(1, 0, 1)], [(3, 0, 1),(1, 0, 3)], [(2, 0, 0, 1),(1, 0, 0, 2)], [(4, 0, 0, 0),(0, 0, 0, 4)], [(1, 1, 0, 0, 0),(0, 0, 0, 1, 1)]

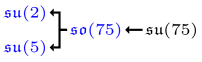


[{⟨1, 1⟩},{⟨74, 1⟩}],[{⟨1, 1⟩}],[(74)],[(0, 1, 1, 0)]

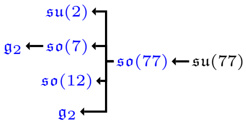


[{⟨1, 1⟩},{⟨76, 1⟩}],[{⟨1, 1⟩}],[(76)],[(3, 0, 0)],[(3, 0)],[{⟨1, 2⟩}],[(0, 2)]

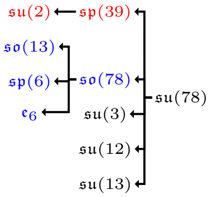


[{⟨1, 1⟩},{⟨77, 1⟩}], [{⟨1, 1⟩}], [(77)], [{⟨1, 1⟩}], [{⟨2, 1⟩}], [{⟨1, 2⟩}], [{⟨2, 1⟩}], [(11, 0),(0, 11)], [{⟨1, 2⟩},{⟨11, 2⟩}],[{⟨2, 1⟩},{⟨11, 1⟩}]

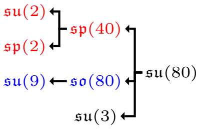


[{⟨1, 1⟩},{⟨79, 1⟩}],[{⟨1, 1⟩}],[(79)],[(1, 3)],[{⟨1, 1⟩}],[{⟨1, 1⟩, ⟨8, 1⟩}],[(7, 1),(1, 7)]

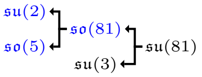


[{⟨1, 1⟩},{⟨80, 1⟩}],[{⟨1, 1⟩}],[(80)],[(2, 2)],[(5, 2),(2, 5)]

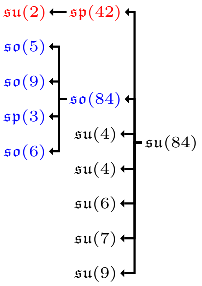


[{⟨1, 1⟩},{⟨83, 1⟩}],[{⟨1, 1⟩}],[(83)],[{⟨1, 1⟩}],[(0, 6)],[(0, 0, 1, 0)],[(0, 0, 2)],[(0, 2, 2)],[(3, 1, 0),(0, 1, 3)],[(6, 0, 0),(0, 0, 6)], [(1, 0, 0, 1, 0),(0, 1, 0, 0, 1)], [{⟨1, 3⟩},{⟨6, 3⟩}],[{⟨3, 1⟩},{⟨6, 1⟩}]

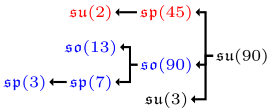


[{⟨1, 1⟩},{⟨89, 1⟩}], [{⟨1, 1⟩}], [(89)], [{⟨1, 1⟩}], [{⟨1, 2⟩}],[{⟨2, 1⟩}],[(0, 2, 0)],[(4, 3),(3, 4)]

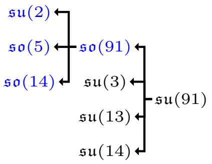


[{⟨1, 1⟩},{⟨90, 1⟩}],[{⟨1, 1⟩}],[(90)],[(5, 0)],[{⟨2, 1⟩}], [(12, 0),(0, 12)], [{⟨1, 2⟩},{⟨12, 2⟩}], [{⟨2, 1⟩}, {⟨12, 1⟩}]

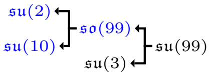


[{⟨1, 1⟩},{⟨98, 1⟩}],[{⟨1, 1⟩}],[(98)],[{⟨1, 1⟩, ⟨9, 1⟩}], [(8, 1),(1, 8)]

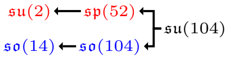


[{⟨1, 1⟩},{⟨103, 1⟩}], [{⟨1, 1⟩}], [(103)], [{⟨1, 1⟩}], [{⟨1, 2⟩}]

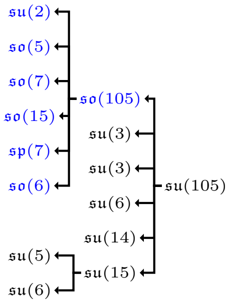


[{⟨1, 1⟩},{⟨104, 1⟩}], [{⟨1, 1⟩}], [(104)], [(1, 4)], [(1, 1, 0)], [{⟨2, 1⟩}], [{⟨1, 2⟩}], [(4, 0, 0)], [(6, 2),(2, 6)], [(13, 0),(0, 13)], [(0, 2, 0, 0, 0),(0, 0, 0, 2, 0)], [{⟨1, 2⟩}, {⟨13, 2⟩}],[{⟨2, 1⟩},{⟨13, 1⟩}],[(2, 1, 0, 0),(0, 0, 1, 2)], [(1, 0, 1, 0, 0),(0, 0, 1, 0, 1)]

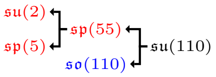


[{⟨1, 1⟩},{⟨109, 1⟩}],[{⟨1, 1⟩}],[(109)],[(0, 0, 1, 0, 0)], [{⟨1, 1⟩}]

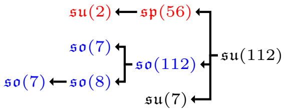


[{⟨1, 1⟩},{⟨111, 1⟩}], [{⟨1, 1⟩}], [(111)], [{⟨1, 1⟩}], [(0, 1, 1)], [(3, 0, 0, 0),(0, 0, 3, 0),(0, 0, 0, 3)], [(0, 0, 3)], [{⟨1, 1⟩, ⟨2, 1⟩},{⟨5, 1⟩, ⟨6, 1⟩}]

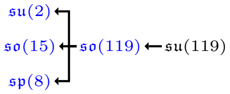


[{⟨1, 1⟩},{⟨118, 1⟩}], [{⟨1, 1⟩}], [(118)], [{⟨1, 2⟩}], [{⟨2, 1⟩}]

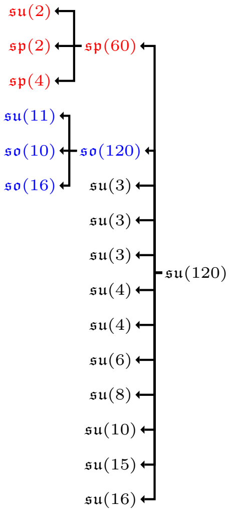


[{⟨1, 1⟩},{⟨119, 1⟩}], [{⟨1, 1⟩}], [(119)], [(7, 0)], [(3, 0, 0)], [{⟨1, 1⟩}], [{⟨1, 1⟩, ⟨10, 1⟩}], [(0, 0, 1, 0, 0)], [{⟨2, 1⟩}],[(5, 3),(3, 5)],[(9, 1),(1, 9)],[(14, 0),(0, 14)], [(4, 0, 1),(1, 0, 4)], [(7, 0, 0),(0, 0, 7)], [(2, 0, 0, 0, 1),(1, 0, 0, 0, 2)], [{⟨1, 3⟩},{⟨7, 3⟩}], [{⟨3, 1⟩},{⟨7, 1⟩}], [{⟨1, 2⟩},{⟨14, 2⟩}],[{⟨2, 1⟩},{⟨14, 1⟩}]

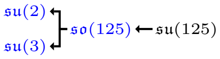


[{⟨1, 1⟩},{⟨124, 1⟩}],[{⟨1, 1⟩}],[(124)],[(4, 4)]

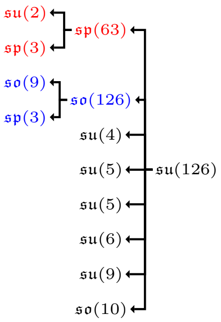


[{⟨1, 1⟩},{⟨125, 1⟩}], [{⟨1, 1⟩}], [(125)], [(0, 1, 1)], [{⟨1, 1⟩}],[(0, 0, 0, 2)],[(4, 0, 0)],[(2, 2, 0),(0, 2, 2)],[(2, 0, 1, 0),(0, 1, 0, 2)], [(5, 0, 0, 0),(0, 0, 0, 5)], [(4, 0, 0, 0, 0),(0, 0, 0, 0, 4)], [{⟨4, 1⟩},{⟨5, 1⟩}], [(0, 0, 0, 2, 0),(0, 0, 0, 0, 2)]

---

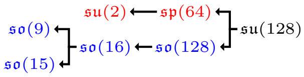


[{⟨1, 1⟩},{⟨127, 1⟩}], [{⟨1, 1⟩}], [(127)], [{⟨1, 1⟩}], [{⟨7, 1⟩},{⟨8, 1⟩}],[(1, 0, 0, 1)],[{⟨7, 1⟩}]

---

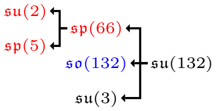


[{⟨1, 1⟩},{⟨131, 1⟩}],[{⟨1, 1⟩}],[(131)],[(0, 0, 0, 0, 1)],[{⟨1, 1⟩}],[(7, 2),(2, 7)]

---

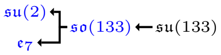


[{⟨1, 1⟩},{⟨132, 1⟩}],[{⟨1, 1⟩}],[(132)],[{⟨1, 1⟩}]

---

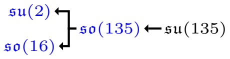


[{⟨1, 1⟩},{⟨134, 1⟩}],[{⟨1, 1⟩}],[(134)],[{⟨1, 2⟩}]

---

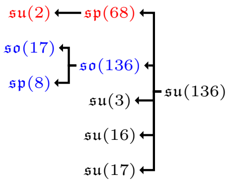


[{⟨1, 1⟩},{⟨135, 1⟩}], [{⟨1, 1⟩}], [(135)], [{⟨1, 1⟩}], [{⟨2, 1⟩}], [{⟨1, 2⟩}], [(15, 0),(0, 15)], [{⟨1, 2⟩},{⟨15, 2⟩}],[{⟨2, 1⟩},{⟨15, 1⟩}]

---

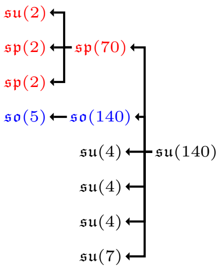


[{⟨1, 1⟩},{⟨139, 1⟩}],[{⟨1, 1⟩}],[(139)],[(1, 4)],[(3, 2)],[{⟨1, 1⟩}],[(6, 0)],[(1, 3, 0),(0, 3, 1)],[(2, 1, 1),(1, 1, 2)],[(4, 1, 0),(0, 1, 4)],[{⟨1, 1⟩, ⟨5, 1⟩},{⟨2, 1⟩, ⟨6, 1⟩}]

---

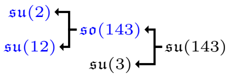


[{⟨1, 1⟩},{⟨142, 1⟩}], [{⟨1, 1⟩}], [(142)], [{⟨1, 1⟩, ⟨11, 1⟩}],[(10, 1),(1, 10)]

---

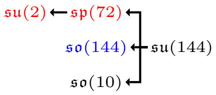


[{⟨1, 1⟩},{⟨143, 1⟩}], [{⟨1, 1⟩}], [(143)], [{⟨1, 1⟩}], [(1, 0, 0, 1, 0),(1, 0, 0, 0, 1)]

---

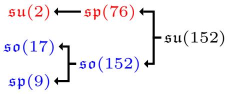


[{⟨1, 1⟩},{⟨151, 1⟩}], [{⟨1, 1⟩}], [(151)], [{⟨1, 1⟩}], [{⟨1, 2⟩}],[{⟨2, 1⟩}]

---

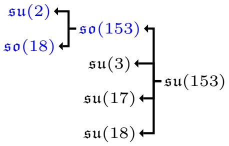


[{⟨1, 1⟩},{⟨152, 1⟩}],[{⟨1, 1⟩}],[(152)],[{⟨2, 1⟩}],[(16, 0),(0, 16)],[{⟨1, 2⟩},{⟨16, 2⟩}],[{⟨2, 1⟩},{⟨16, 1⟩}]

---

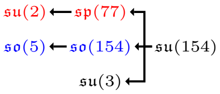


[{⟨1, 1⟩},{⟨153, 1⟩}], [{⟨1, 1⟩}], [(153)], [{⟨1, 1⟩}], [(3, 2)],[(6, 3),(3, 6)]

---

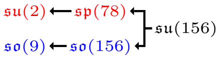


[{⟨1, 1⟩},{⟨155, 1⟩}], [{⟨1, 1⟩}], [(155)], [{⟨1, 1⟩}], [(3, 0, 0, 0)]

---

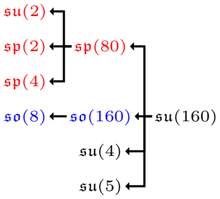


[{⟨1, 1⟩},{⟨159, 1⟩}], [{⟨1, 1⟩}], [(159)], [(5, 1)], [(1, 1, 0, 0)], [{⟨1, 1⟩}], [(1, 1, 0, 0),(0, 1, 1, 0),(0, 1, 0, 1)], [(3, 0, 2),(2, 0, 3)],[(3, 0, 0, 1),(1, 0, 0, 3)]

---

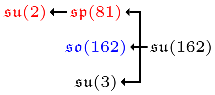


[{⟨1, 1⟩},{⟨161, 1⟩}], [{⟨1, 1⟩}], [(161)], [{⟨1, 1⟩}], [(8, 2),(2, 8)]

---

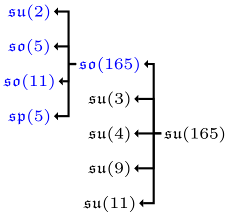


[{⟨1, 1⟩},{⟨164, 1⟩}], [{⟨1, 1⟩}], [(164)], [(0, 8)], [(0, 0, 1, 0, 0)], [(0, 0, 0, 1, 0)], [(5, 4),(4, 5)], [(8, 0, 0),(0, 0, 8)],[{⟨1, 3⟩},{⟨8, 3⟩}],[{⟨3, 1⟩},{⟨8, 1⟩}]

---

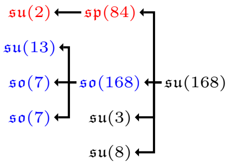


[{⟨1, 1⟩},{⟨167, 1⟩}], [{⟨1, 1⟩}], [(167)], [{⟨1, 1⟩}], [{⟨1, 1⟩, ⟨12, 1⟩}],[(0, 2, 0)],[(2, 0, 1)],[(11, 1),(1, 11)],[{⟨1, 1⟩, ⟨2, 1⟩},{⟨6, 1⟩, ⟨7, 1⟩}]

---

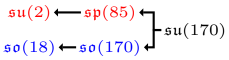


[{⟨1, 1⟩},{⟨169, 1⟩}], [{⟨1, 1⟩}], [(169)], [{⟨1, 1⟩}], [{⟨1, 2⟩}]

---

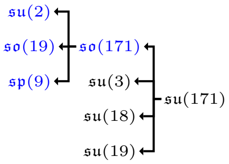


[{⟨1, 1⟩},{⟨170, 1⟩}], [{⟨1, 1⟩}], [(170)], [{⟨2, 1⟩}], [{⟨1, 2⟩}], [(17, 0),(0, 17)], [{⟨1, 2⟩},{⟨17, 2⟩}], [{⟨2, 1⟩},{⟨17, 1⟩}]

---

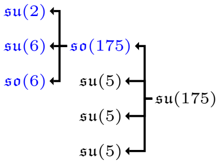


[{⟨1, 1⟩},{⟨174, 1⟩}],[{⟨1, 1⟩}],[(174)],[(0, 0, 2, 0, 0)],[(2, 1, 1)], [(0, 3, 0, 0),(0, 0, 3, 0)], [(1, 1, 0, 1),(1, 0, 1, 1)],[(1, 2, 0, 0),(0, 0, 2, 1)]

---

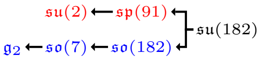


[{⟨1, 1⟩},{⟨181, 1⟩}], [{⟨1, 1⟩}], [(181)], [{⟨1, 1⟩}], [(4, 0, 0)],[(4, 0)]

---

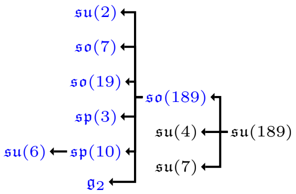


[{⟨1, 1⟩},{⟨188, 1⟩}], [{⟨1, 1⟩}], [(188)], [(1, 0, 2)], [{⟨1, 2⟩}], [(2, 1, 0)], [{⟨2, 1⟩}], [(0, 1, 0, 1, 0)], [(2, 1)], [(5, 0, 1),(1, 0, 5)],[{⟨1, 2⟩, ⟨6, 1⟩},{⟨1, 1⟩, ⟨6, 2⟩}]

---

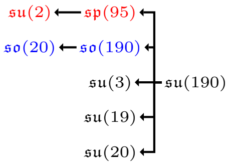


[{⟨1, 1⟩},{⟨189, 1⟩}], [{⟨1, 1⟩}], [(189)], [{⟨1, 1⟩}], [{⟨2, 1⟩}], [(18, 0),(0, 18)], [{⟨1, 2⟩},{⟨18, 2⟩}], [{⟨2, 1⟩},{⟨18, 1⟩}]

---

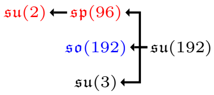


[{⟨1, 1⟩},{⟨191, 1⟩}], [{⟨1, 1⟩}], [(191)], [{⟨1, 1⟩}], [(7, 3),(3, 7)]

---

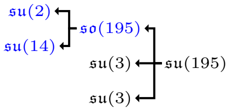


[{⟨1, 1⟩},{⟨194, 1⟩}], [{⟨1, 1⟩}], [(194)], [{⟨1, 1⟩, ⟨13, 1⟩}],[(9, 2),(2, 9)],[(12, 1),(1, 12)]

---

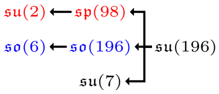


[{⟨1, 1⟩},{⟨195, 1⟩}], [{⟨1, 1⟩}], [(195)], [{⟨1, 1⟩}], [(5, 0, 0)],[{⟨2, 2⟩},{⟨5, 2⟩}]

---

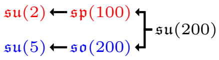


[{⟨1, 1⟩},{⟨199, 1⟩}], [{⟨1, 1⟩}], [(199)], [{⟨1, 1⟩}], [(2, 0, 0, 2)]

---

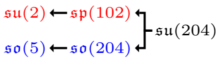


[{⟨1, 1⟩},{⟨203, 1⟩}], [{⟨1, 1⟩}], [(203)], [{⟨1, 1⟩}], [(7, 0)]

---

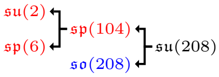


[{⟨1, 1⟩},{⟨207, 1⟩}], [{⟨1, 1⟩}], [(207)], [{⟨3, 1⟩}], [{⟨1, 1⟩}]

---

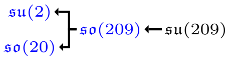

[{⟨1, 1⟩},{⟨208, 1⟩}],[{⟨1, 1⟩}],[(208)],[{⟨1, 2⟩}]

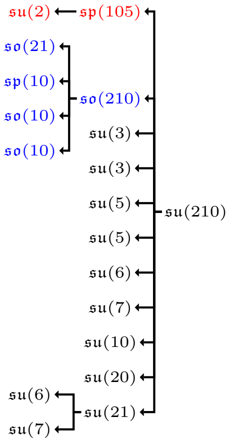


[{⟨1, 1⟩},{⟨209, 1⟩}], [{⟨1, 1⟩}], [(209)], [{⟨1, 1⟩}], [{⟨2, 1⟩}], [{⟨1, 2⟩}], [(0, 0, 0, 1, 1)], [(3, 0, 0, 0, 0)], [(6, 4),(4, 6)], [(19, 0),(0, 19)], [(1, 0, 2, 0),(0, 2, 0, 1)], [(6, 0, 0, 0),(0, 0, 0, 6)], [(0, 1, 1, 0, 0),(0, 0, 1, 1, 0)], [{⟨1, 4⟩},{⟨6, 4⟩}], [{⟨4, 1⟩},{⟨6, 1⟩}], [{⟨1, 2⟩},{⟨19, 2⟩}], [{⟨2, 1⟩},{⟨19, 1⟩}], [(2, 1, 0, 0, 0),(0, 0, 0, 1, 2)],[{⟨1, 1⟩, ⟨3, 1⟩},{⟨4, 1⟩, ⟨6, 1⟩}]

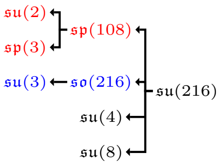


[{⟨1, 1⟩},{⟨215, 1⟩}], [{⟨1, 1⟩}], [(215)], [(2, 0, 1)], [{⟨1, 1⟩}], [(5, 5)], [(5, 1, 0),(0, 1, 5)], [{⟨1, 1⟩, ⟨6, 1⟩},{⟨2, 1⟩, ⟨7, 1⟩}]

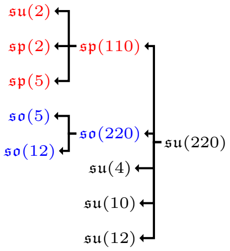


[{⟨1, 1⟩},{⟨219, 1⟩}], [{⟨1, 1⟩}], [(219)], [(9, 0)], [(3, 0, 0, 0)],[{⟨1, 1⟩}],[(2, 4)],[{⟨3, 1⟩}],[(9, 0, 0),(0, 0, 9)], [{⟨1, 3⟩},{⟨9, 3⟩}],[{⟨3, 1⟩},{⟨9, 1⟩}]

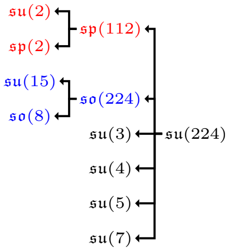


[{⟨1, 1⟩},{⟨223, 1⟩}], [{⟨1, 1⟩}], [(223)], [(1, 5)], [{⟨1, 1⟩}], [{⟨1, 1⟩, ⟨14, 1⟩}], [(2, 0, 1, 0),(2, 0, 0, 1),(1, 0, 2, 0),(1, 0, 0, 2),(0, 0, 2, 1),(0, 0, 1, 2)], [(13, 1),(1, 13)],[(3, 2, 0),(0, 2, 3)],[(3, 1, 0, 0),(0, 0, 1, 3)],[{⟨1, 1⟩, ⟨4, 1⟩},{⟨3, 1⟩, ⟨6, 1⟩}]

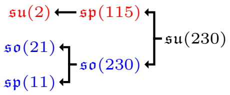


[{⟨1, 1⟩},{⟨229, 1⟩}], [{⟨1, 1⟩}], [(229)], [{⟨1, 1⟩}], [{⟨1, 2⟩}],[{⟨2, 1⟩}]

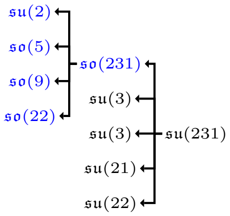


[{⟨1, 1⟩},{⟨230, 1⟩}], [{⟨1, 1⟩}], [(230)], [(1, 6)], [(1, 1, 0, 0)], [{⟨2, 1⟩}], [(10, 2),(2, 10)], [(20, 0),(0, 20)], [{⟨1, 2⟩},{⟨20, 2⟩}],[{⟨2, 1⟩},{⟨20, 1⟩}]

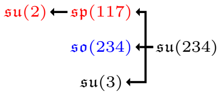


[{⟨1, 1⟩},{⟨233, 1⟩}], [{⟨1, 1⟩}], [(233)], [{⟨1, 1⟩}], [(8, 3),(3, 8)]

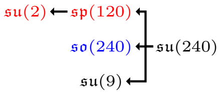


[{⟨1, 1⟩},{⟨239, 1⟩}], [{⟨1, 1⟩}], [(239)], [{⟨1, 1⟩}], [{⟨1, 1⟩, ⟨2, 1⟩},{⟨7, 1⟩, ⟨8, 1⟩}]

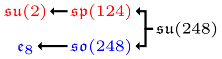


[{⟨1, 1⟩},{⟨247, 1⟩}], [{⟨1, 1⟩}], [(247)], [{⟨1, 1⟩}], [{⟨8, 1⟩}]

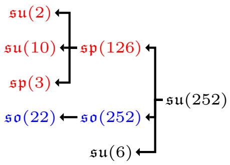


[{⟨1, 1⟩},{⟨251, 1⟩}], [{⟨1, 1⟩}], [(251)], [{⟨5, 1⟩}], [(5, 0, 0)],[{⟨1, 1⟩}],[{⟨1, 2⟩}],[(5, 0, 0, 0, 0),(0, 0, 0, 0, 5)]

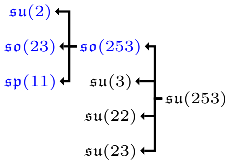


[{⟨1, 1⟩},{⟨252, 1⟩}], [{⟨1, 1⟩}], [(252)], [{⟨2, 1⟩}], [{⟨1, 2⟩}], [(21, 0),(0, 21)], [{⟨1, 2⟩},{⟨21, 2⟩}], [{⟨2, 1⟩},{⟨21, 1⟩}]

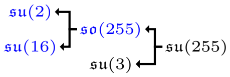


[{⟨1, 1⟩},{⟨254, 1⟩}], [{⟨1, 1⟩}], [(254)], [{⟨1, 1⟩, ⟨15, 1⟩}],[(14, 1),(1, 14)]

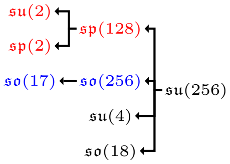


[{⟨1, 1⟩},{⟨255, 1⟩}], [{⟨1, 1⟩}], [(255)], [(3, 3)], [{⟨1, 1⟩}], [{⟨8, 1⟩}], [(3, 1, 1),(1, 1, 3)], [{⟨8, 1⟩},{⟨9, 1⟩}]

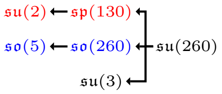


[{⟨1, 1⟩},{⟨259, 1⟩}], [{⟨1, 1⟩}], [(259)], [{⟨1, 1⟩}], [(4, 2)],[(7, 4),(4, 7)]

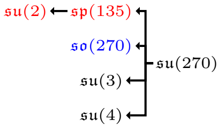


[{⟨1, 1⟩},{⟨269, 1⟩}],[{⟨1, 1⟩}],[(269)],[{⟨1, 1⟩}],[(11, 2),(2, 11)],[(4, 0, 2),(2, 0, 4)]

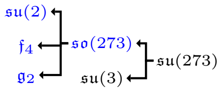


[{⟨1, 1⟩},{⟨272, 1⟩}], [{⟨1, 1⟩}], [(272)], [(0, 0, 1, 0)], [(0, 3)],[(6, 5),(5, 6)]

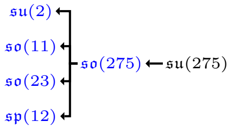


[{⟨1, 1⟩},{⟨274, 1⟩}],[{⟨1, 1⟩}],[(274)],[(3, 0, 0, 0, 0)], [{⟨1, 2⟩}],[{⟨2, 1⟩}]

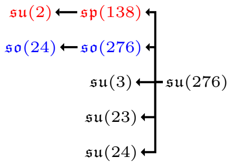


[{⟨1, 1⟩},{⟨275, 1⟩}], [{⟨1, 1⟩}], [(275)], [{⟨1, 1⟩}], [{⟨2, 1⟩}], [(22, 0),(0, 22)], [{⟨1, 2⟩},{⟨22, 2⟩}], [{⟨2, 1⟩},{⟨22, 1⟩}]

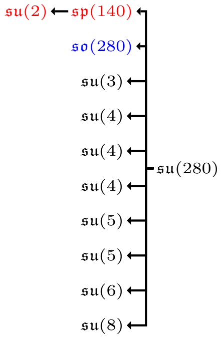


[{⟨1, 1⟩},{⟨279, 1⟩}], [{⟨1, 1⟩}], [(279)], [{⟨1, 1⟩}], [(9, 3),(3, 9)], [(1, 4, 0),(0, 4, 1)], [(2, 3, 0),(0, 3, 2)], [(6, 0, 1),(1, 0, 6)],[(1, 1, 1, 0),(0, 1, 1, 1)],[(3, 0, 1, 0),(0, 1, 0, 3)], [(2, 0, 0, 1, 0),(0, 1, 0, 0, 2)], [{⟨1, 2⟩, ⟨7, 1⟩},{⟨1, 1⟩, ⟨7, 2⟩}]

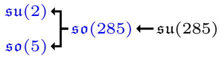


[{⟨1, 1⟩},{⟨284, 1⟩}],[{⟨1, 1⟩}],[(284)],[(8, 0)]

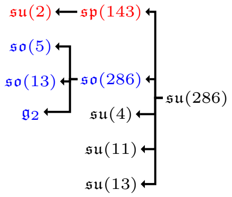


[{⟨1, 1⟩},{⟨285, 1⟩}], [{⟨1, 1⟩}], [(285)], [{⟨1, 1⟩}], [(0, 10)], [{⟨3, 1⟩}], [(1, 2)], [(10, 0, 0),(0, 0, 10)], [{⟨1, 3⟩},{⟨10, 3⟩}],[{⟨3, 1⟩},{⟨10, 1⟩}]

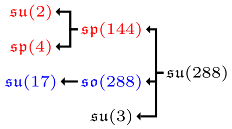


[{⟨1, 1⟩},{⟨287, 1⟩}], [{⟨1, 1⟩}], [(287)], [(1, 0, 0, 1)], [{⟨1, 1⟩}],[{⟨1, 1⟩, ⟨16, 1⟩}],[(15, 1),(1, 15)]

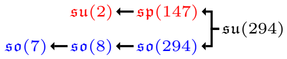


[{⟨1, 1⟩},{⟨293, 1⟩}], [{⟨1, 1⟩}], [(293)], [{⟨1, 1⟩}], [(4, 0, 0, 0),(0, 0, 4, 0),(0, 0, 0, 4)],[(0, 0, 4)]

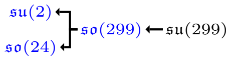

[{⟨1, 1⟩},{⟨298, 1⟩}],[{⟨1, 1⟩}],[(298)],[{⟨1, 2⟩}]

su(2) ⟵ sp(150)
so(25), sp(12), so(6), so(6), so(8) ⟵ so(300)
su(3), su(24), su(25)
sp(150), so(300), su(3), su(24), su(25) ⟵ su(300)

[{⟨1, 1⟩},{⟨299, 1⟩}], [{⟨1, 1⟩}], [(299)], [{⟨1, 1⟩}], [{⟨2, 1⟩}], [{⟨1, 2⟩}], [(0, 3, 3)], [(1, 2, 2)], [(0, 2, 0, 0)], [(23, 0),(0, 23)], [{⟨1, 2⟩},{⟨23, 2⟩}], [{⟨2, 1⟩},{⟨23, 1⟩}]

su(2) ⟵ sp(154)
sp(4) ⟵ so(308)
sp(154), so(308) ⟵ su(308)

[{⟨1, 1⟩},{⟨307, 1⟩}], [{⟨1, 1⟩}], [(307)], [{⟨1, 1⟩}], [(0, 2, 0, 0)]

su(2) ⟵ sp(156)
sp(156), so(312), su(3) ⟵ su(312)

[{⟨1, 1⟩},{⟨311, 1⟩}],[{⟨1, 1⟩}],[(311)],[{⟨1, 1⟩}],[(12, 2),(2, 12)]

su(2), sp(4) ⟵ so(315)
so(315), su(3), su(4), su(5), su(5), su(6), su(9) ⟵ su(315)

[{⟨1, 1⟩},{⟨314, 1⟩}], [{⟨1, 1⟩}], [(314)], [(1, 0, 1, 0)], [(8, 4),(4, 8)], [(6, 1, 0),(0, 1, 6)], [(0, 2, 1, 0),(0, 1, 2, 0)],[(4, 0, 0, 1),(1, 0, 0, 4)],[(3, 0, 0, 0, 1),(1, 0, 0, 0, 3)], [{⟨1, 1⟩, ⟨7, 1⟩},{⟨2, 1⟩, ⟨8, 1⟩}]

su(2), so(11), sp(2), sp(5) ⟵ sp(160)
so(10) ⟵ so(320)
sp(160), so(320) ⟵ su(320)

[{⟨1, 1⟩},{⟨319, 1⟩}],[{⟨1, 1⟩}],[(319)],[(1, 0, 0, 0, 1)], [(7, 1)],[(1, 1, 0, 0, 0)],[{⟨1, 1⟩}],[(1, 1, 0, 0, 0)]

su(2), su(18) ⟵ so(323)
so(323), su(3) ⟵ su(323)

[{⟨1, 1⟩},{⟨322, 1⟩}], [{⟨1, 1⟩}], [(322)], [{⟨1, 1⟩, ⟨17, 1⟩}],[(16, 1),(1, 16)]

su(2), sp(2) ⟵ sp(162)
so(25), sp(13), $\mathfrak{f}_4$ ⟵ so(324)
sp(162), so(324) ⟵ su(324)

[{⟨1, 1⟩},{⟨323, 1⟩}], [{⟨1, 1⟩}], [(323)], [(5, 2)], [{⟨1, 1⟩}],[{⟨1, 2⟩}],[{⟨2, 1⟩}],[(0, 0, 0, 2)]

su(2), so(26) ⟵ so(325)
so(325), su(3), su(25), su(26) ⟵ su(325)

[{⟨1, 1⟩},{⟨324, 1⟩}],[{⟨1, 1⟩}],[(324)],[{⟨2, 1⟩}],[(24, 0),(0, 24)],[{⟨1, 2⟩},{⟨24, 2⟩}],[{⟨2, 1⟩},{⟨24, 1⟩}]

su(2), sp(3) ⟵ sp(165)
so(7), so(11), sp(4) ⟵ so(330)
sp(165), so(330), su(3), su(5), su(8), su(10), su(11) ⟵ su(330)

[{⟨1, 1⟩},{⟨329, 1⟩}], [{⟨1, 1⟩}], [(329)], [(0, 0, 3)], [{⟨1, 1⟩}], [(2, 1, 0)], [(0, 0, 0, 1, 0)], [(4, 0, 0, 0)], [(10, 3),(3, 10)], [(7, 0, 0, 0),(0, 0, 0, 7)], [{⟨1, 4⟩},{⟨7, 4⟩}], [{⟨1, 1⟩, ⟨2, 1⟩},{⟨8, 1⟩, ⟨9, 1⟩}],[{⟨4, 1⟩},{⟨7, 1⟩}]

su(2), sp(2) ⟵ sp(168)
so(6) ⟵ so(336)
sp(168), so(336), su(3), su(6), su(8) ⟵ su(336)

[{⟨1, 1⟩},{⟨335, 1⟩}], [{⟨1, 1⟩}], [(335)], [(1, 6)], [{⟨1, 1⟩}], [(6, 0, 0)], [(7, 5),(5, 7)], [(2, 0, 1, 0, 0),(0, 0, 1, 0, 2)],[{⟨2, 2⟩},{⟨6, 2⟩}]

su(2), su(3) ⟵ so(343) ⟵ su(343)

[{⟨1, 1⟩},{⟨342, 1⟩}],[{⟨1, 1⟩}],[(342)],[(6, 6)]

su(2), sp(7) ⟵ sp(175); sp(3) ⟵ sp(7)
so(8), so(26) ⟵ so(350)
sp(175), so(350) ⟵ su(350)

[{⟨1, 1⟩},{⟨349, 1⟩}], [{⟨1, 1⟩}], [(349)], [{⟨3, 1⟩}], [(1, 2, 0)],[{⟨1, 1⟩}],[(1, 0, 1, 1)],[{⟨1, 2⟩}]

su(2), so(27), sp(13) ⟵ so(351)
$\mathfrak{e}_6$ ⟵ su(27)
so(351), su(3), su(26), su(27), $\mathfrak{e}_6$ ⟵ su(351)

[{⟨1, 1⟩},{⟨350, 1⟩}], [{⟨1, 1⟩}], [(350)], [{⟨2, 1⟩}], [{⟨1, 2⟩}], [(25, 0),(0, 25)], [{⟨1, 2⟩},{⟨25, 2⟩}], [{⟨2, 1⟩},{⟨25, 1⟩}], [{⟨3, 1⟩},{⟨5, 1⟩}], [{⟨1, 2⟩},{⟨6, 2⟩}]

su(2), so(12) ⟵ sp(176)
so(12) ⟵ so(352)
sp(176), so(352) ⟵ su(352)

[{⟨1, 1⟩},{⟨351, 1⟩}], [{⟨1, 1⟩}], [(351)], [{⟨1, 1⟩, ⟨5, 1⟩},{⟨1, 1⟩, ⟨6, 1⟩}],[{⟨1, 1⟩}],[{⟨1, 3⟩}]

su(2) ⟵ so(357)
so(357), su(3) ⟵ su(357)

[{⟨1, 1⟩},{⟨356, 1⟩}],[{⟨1, 1⟩}],[(356)],[(13, 2),(2, 13)]

su(2) ⟵ sp(180)
su(19) ⟵ so(360)
sp(180), so(360), su(3), su(4), su(4) ⟵ su(360)

[{⟨1, 1⟩},{⟨359, 1⟩}], [{⟨1, 1⟩}], [(359)], [{⟨1, 1⟩}], [{⟨1, 1⟩, ⟨18, 1⟩}], [(17, 1),(1, 17)], [(2, 2, 1),(1, 2, 2)], [(4, 2, 0),(0, 2, 4)]

su(2), sp(2), sp(6) ⟵ sp(182)
so(14) ⟵ so(364)
sp(182), so(364), su(4), su(12), su(14) ⟵ su(364)

[{⟨1, 1⟩},{⟨363, 1⟩}], [{⟨1, 1⟩}], [(363)], [(11, 0)], [{⟨1, 3⟩}], [{⟨1, 1⟩}], [{⟨3, 1⟩}], [(11, 0, 0),(0, 0, 11)], [{⟨1, 3⟩},{⟨11, 3⟩}],[{⟨3, 1⟩},{⟨11, 1⟩}]

su(2) ⟵ so(375)
so(375), su(3) ⟵ su(375)

[{⟨1, 1⟩},{⟨374, 1⟩}],[{⟨1, 1⟩}],[(374)],[(9, 4),(4, 9)]

su(2), so(27), sp(14) ⟵ so(377) ⟵ su(377)

[{⟨1, 1⟩},{⟨376, 1⟩}], [{⟨1, 1⟩}], [(376)], [{⟨1, 2⟩}], [{⟨2, 1⟩}]

su(2), sp(3) ⟵ sp(189)
so(7), $\mathfrak{g}_2$ ⟵ so(7), so(28) ⟵ so(378)
su(7), su(8) ⟵ su(28)
sp(189), so(378), su(3), su(27), su(28) ⟵ su(378)

[{⟨1, 1⟩},{⟨377, 1⟩}], [{⟨1, 1⟩}], [(377)], [(1, 0, 2)], [{⟨1, 1⟩}], [(0, 1, 2)], [(5, 0, 0)], [(5, 0)], [{⟨2, 1⟩}], [(26, 0),(0, 26)], [{⟨1, 2⟩},{⟨26, 2⟩}], [{⟨2, 1⟩},{⟨26, 1⟩}], [{⟨1, 2⟩, ⟨2, 1⟩},{⟨5, 1⟩, ⟨6, 2⟩}], [{⟨1, 1⟩, ⟨3, 1⟩}, {⟨5, 1⟩, ⟨7, 1⟩}]

su(2) ⟵ sp(192)
so(6) ⟵ so(384)
sp(192), so(384), su(3), su(6) ⟵ su(384)

[{⟨1, 1⟩},{⟨383, 1⟩}], [{⟨1, 1⟩}], [(383)], [{⟨1, 1⟩}], [(3, 1, 1)],[(11, 3),(3, 11)],[(1, 1, 0, 0, 1),(1, 0, 0, 1, 1)]

su(2), so(5), sp(3) ⟵ so(385) ⟵ su(385)

[{⟨1, 1⟩},{⟨384, 1⟩}], [{⟨1, 1⟩}], [(384)], [(9, 0)], [(0, 3, 0)]

su(2) ⟵ sp(195)
so(5) ⟵ so(390)
sp(195), so(390) ⟵ su(390)

[{⟨1, 1⟩},{⟨389, 1⟩}], [{⟨1, 1⟩}], [(389)], [{⟨1, 1⟩}], [(3, 4)]

su(2) ⟵ sp(196)
su(7) ⟵ so(392)
sp(196), so(392) ⟵ su(392)

[{⟨1, 1⟩},{⟨391, 1⟩}], [{⟨1, 1⟩}], [(391)], [{⟨1, 1⟩}], [{⟨2, 1⟩, ⟨5, 1⟩}]

su(2) ⟵ sp(198)
sp(198), so(396), su(4), su(9) ⟵ su(396)

[{⟨1, 1⟩},{⟨395, 1⟩}], [{⟨1, 1⟩}], [(395)], [{⟨1, 1⟩}], [(7, 0, 1),(1, 0, 7)],[{⟨1, 2⟩, ⟨8, 1⟩},{⟨1, 1⟩, ⟨8, 2⟩}]

su(2), su(20) ⟵ so(399)
so(399), su(3) ⟵ su(399)

[{⟨1, 1⟩},{⟨398, 1⟩}], [{⟨1, 1⟩}], [(398)], [{⟨1, 1⟩, ⟨19, 1⟩}],[(18, 1),(1, 18)]

su(2), su(6), so(5), so(28) ← so(405)
so(405), su(3), su(3) ← su(405)

[{⟨1, 1⟩},{⟨404, 1⟩}], [{⟨1, 1⟩}], [(404)], [(2, 0, 0, 0, 2)], [(5, 2)], [{⟨1, 2⟩}], [(8, 5),(5, 8)], [(14, 2),(2, 14)]

---

su(2) ← sp(203)
so(29), sp(14) ← so(406)
sp(203), so(406), su(3), su(28), su(29) ← su(406)

[{⟨1, 1⟩},{⟨405, 1⟩}], [{⟨1, 1⟩}], [(405)], [{⟨1, 1⟩}], [{⟨2, 1⟩}], [{⟨1, 2⟩}], [(27, 0),(0, 27)], [{⟨1, 2⟩},{⟨27, 2⟩}], [{⟨2, 1⟩},{⟨27, 1⟩}]

---

su(2), sp(2) ← sp(210)
sp(210), so(420), su(3), su(4), su(4), su(5), su(5), su(6), su(8) ← su(420)

[{⟨1, 1⟩},{⟨419, 1⟩}], [{⟨1, 1⟩}], [(419)], [(3, 4)], [{⟨1, 1⟩}], [(7, 6),(6, 7)], [(4, 1, 1),(1, 1, 4)], [(5, 0, 2),(2, 0, 5)], [(2, 2, 0, 0),(0, 0, 2, 2)], [(4, 1, 0, 0),(0, 0, 1, 4)], [(1, 2, 0, 0, 0),(0, 0, 0, 2, 1)], [{⟨1, 1⟩, ⟨5, 1⟩},{⟨3, 1⟩, ⟨7, 1⟩}]

---

su(2), so(5), so(11), sp(6), sp(6) ← so(429) ← su(429)

[{⟨1, 1⟩},{⟨428, 1⟩}], [{⟨1, 1⟩}], [(428)], [(1, 8)], [(1, 1, 0, 0, 0)], [{⟨6, 1⟩}], [{⟨4, 1⟩}]

---

su(2) ← sp(216)
so(9) ← so(432)
sp(216), so(432) ← su(432)

[{⟨1, 1⟩},{⟨431, 1⟩}], [{⟨1, 1⟩}], [(431)], [{⟨1, 1⟩}], [(0, 1, 0, 1)]

---

su(2) ← sp(217)
so(29), sp(15) ← so(434)
sp(217), so(434) ← su(434)

[{⟨1, 1⟩},{⟨433, 1⟩}], [{⟨1, 1⟩}], [(433)], [{⟨1, 1⟩}], [{⟨1, 2⟩}], [{⟨2, 1⟩}]

---

su(2), so(30) ← so(435)
so(435), su(3), su(29), su(30) ← su(435)

[{⟨1, 1⟩},{⟨434, 1⟩}], [{⟨1, 1⟩}], [(434)], [{⟨2, 1⟩}], [(28, 0),(0, 28)], [{⟨1, 2⟩},{⟨28, 2⟩}], [{⟨2, 1⟩},{⟨28, 1⟩}]

---

su(2) ← sp(220)
su(21) ← so(440)
sp(220), so(440), su(3), su(3), su(4), su(10), su(11) ← su(440)

[{⟨1, 1⟩},{⟨439, 1⟩}], [{⟨1, 1⟩}], [(439)], [{⟨1, 1⟩}], [{⟨1, 1⟩, ⟨20, 1⟩}], [(10, 4),(4, 10)], [(19, 1),(1, 19)], [(7, 1, 0),(0, 1, 7)], [{⟨1, 1⟩, ⟨8, 1⟩},{⟨2, 1⟩, ⟨9, 1⟩}], [{⟨1, 1⟩, ⟨2, 1⟩},{⟨9, 1⟩, ⟨10, 1⟩}]

---

su(2) ← sp(221)
so(13) ← so(442)
sp(221), so(442), su(3) ← su(442)

[{⟨1, 1⟩},{⟨441, 1⟩}], [{⟨1, 1⟩}], [(441)], [{⟨1, 1⟩}], [{⟨1, 3⟩}], [(12, 3),(3, 12)]

---

su(2), sp(3) ← sp(224)
so(7), g2 ← so(448)
sp(224), so(448) ← su(448)

[{⟨1, 1⟩},{⟨447, 1⟩}], [{⟨1, 1⟩}], [(447)], [(3, 1, 0)], [{⟨1, 1⟩}], [(3, 0, 1)], [(3, 1)]

---

su(2) ← sp(225)
so(9) ← so(450)
sp(225), so(450), su(5), su(5) ← su(450)

[{⟨1, 1⟩},{⟨449, 1⟩}], [{⟨1, 1⟩}], [(449)], [{⟨1, 1⟩}], [(4, 0, 0, 0)], [(2, 1, 0, 1),(1, 0, 1, 2)], [(3, 0, 0, 2),(2, 0, 0, 3)]

---

su(2), so(5), so(5), so(15) ← so(455)
so(455), su(4), su(13), su(15) ← su(455)

[{⟨1, 1⟩},{⟨454, 1⟩}], [{⟨1, 1⟩}], [(454)], [(0, 12)], [(2, 6)], [{⟨3, 1⟩}], [(12, 0, 0),(0, 0, 12)], [{⟨1, 3⟩},{⟨12, 3⟩}], [{⟨3, 1⟩},{⟨12, 1⟩}]

---

su(2) ← sp(228)
sp(228), so(456), su(3) ← su(456)

[{⟨1, 1⟩},{⟨455, 1⟩}], [{⟨1, 1⟩}], [(455)], [{⟨1, 1⟩}], [(15, 2),(2, 15)]

---

su(2) ← sp(231)
so(11) ← so(12)
sp(3), so(12) ← so(462)
sp(231), so(462), su(6), su(7), su(11) ← su(462)

[{⟨1, 1⟩},{⟨461, 1⟩}], [{⟨1, 1⟩}], [(461)], [{⟨1, 1⟩}], [(6, 0, 0)], [{⟨5, 2⟩},{⟨6, 2⟩}], [(0, 0, 0, 0, 2)], [(6, 0, 0, 0, 0),(0, 0, 0, 0, 6)], [{⟨1, 5⟩},{⟨6, 5⟩}], [{⟨5, 1⟩},{⟨6, 1⟩}]

---

su(2) ← sp(232)
so(30) ← so(464)
sp(232), so(464) ← su(464)

[{⟨1, 1⟩},{⟨463, 1⟩}], [{⟨1, 1⟩}], [(463)], [{⟨1, 1⟩}], [{⟨1, 2⟩}]

---

su(2), so(31), sp(15) ← so(465)
so(465), su(3), su(30), su(31) ← su(465)

[{⟨1, 1⟩},{⟨464, 1⟩}], [{⟨1, 1⟩}], [(464)], [{⟨2, 1⟩}], [{⟨1, 2⟩}], [(29, 0),(0, 29)], [{⟨1, 2⟩},{⟨29, 2⟩}], [{⟨2, 1⟩},{⟨29, 1⟩}]

---

su(2), sp(2) ← sp(240)
sp(240), so(480), su(3), su(4), su(5) ← su(480)

[{⟨1, 1⟩},{⟨479, 1⟩}], [{⟨1, 1⟩}], [(479)], [(1, 7)], [{⟨1, 1⟩}], [(9, 5),(5, 9)], [(3, 3, 0),(0, 3, 3)], [(2, 0, 1, 1),(1, 1, 0, 2)]

---

su(2), su(22) ← so(483)
so(483), su(3) ← su(483)

[{⟨1, 1⟩},{⟨482, 1⟩}], [{⟨1, 1⟩}], [(482)], [{⟨1, 1⟩, ⟨21, 1⟩}], [(20, 1),(1, 20)]

---

su(2) ← sp(245)
sp(245), so(490), su(5), su(6), su(7), su(7) ← su(490)

[{⟨1, 1⟩},{⟨489, 1⟩}], [{⟨1, 1⟩}], [(489)], [{⟨1, 1⟩}], [(0, 4, 0, 0),(0, 0, 4, 0)], [(0, 3, 0, 0, 0),(0, 0, 0, 3, 0)], [{⟨3, 2⟩},{⟨4, 2⟩}], [{⟨2, 1⟩, ⟨3, 1⟩},{⟨4, 1⟩, ⟨5, 1⟩}]

---

so(12) ← sp(16)
su(2), so(9), so(31), sp(16) ← so(495)
so(495), su(5), su(9), su(12) ← su(495)

[{⟨1, 1⟩},{⟨494, 1⟩}], [{⟨1, 1⟩}], [(494)], [(0, 2, 0, 0)], [{⟨1, 2⟩}], [{⟨2, 1⟩}], [{⟨4, 1⟩}], [(8, 0, 0, 0),(0, 0, 0, 8)], [{⟨1, 4⟩},{⟨8, 4⟩}], [{⟨4, 1⟩},{⟨8, 1⟩}]

---

su(2) ← sp(248)
so(32) ← so(496)
sp(248), so(496), su(3), su(31), su(32) ← su(496)

[{⟨1, 1⟩},{⟨495, 1⟩}], [{⟨1, 1⟩}], [(495)], [{⟨1, 1⟩}], [{⟨2, 1⟩}], [(30, 0),(0, 30)], [{⟨1, 2⟩},{⟨30, 2⟩}], [{⟨2, 1⟩},{⟨30, 1⟩}]

---

su(2) ← sp(250)
sp(250), so(500), su(4) ← su(500)

[{⟨1, 1⟩},{⟨499, 1⟩}], [{⟨1, 1⟩}], [(499)], [{⟨1, 1⟩}], [(4, 0, 3),(3, 0, 4)]

---

su(2) ← sp(252)
sp(252), so(504), su(3), su(3), su(4), su(6), su(8) ← su(504)

[{⟨1, 1⟩},{⟨503, 1⟩}], [{⟨1, 1⟩}], [(503)], [{⟨1, 1⟩}], [(8, 6),(6, 8)], [(13, 3),(3, 13)], [(1, 5, 0),(0, 5, 1)], [(3, 1, 0, 0, 0),(0, 0, 0, 1, 3)], [{⟨1, 1⟩, ⟨4, 1⟩},{⟨4, 1⟩, ⟨7, 1⟩}]

---

su(2) ← sp(253)
so(5) ← so(506)
sp(253), so(506) ← su(506)

[{⟨1, 1⟩},{⟨505, 1⟩}], [{⟨1, 1⟩}], [(505)], [{⟨1, 1⟩}], [(10, 0)]

---

su(2) ← sp(255)
sp(255), so(510), su(3), su(3) ← su(510)

[{⟨1, 1⟩},{⟨509, 1⟩}], [{⟨1, 1⟩}], [(509)], [{⟨1, 1⟩}], [(11, 4),(4, 11)], [(16, 2),(2, 16)]

su(2)
so(19) ⟵ so(20) sp(256)
su(3) su(512)
so(7) ⟵ so(512)
sp(3)

[{⟨1, 1⟩},{⟨511, 1⟩}], [{⟨1, 1⟩}], [(511)], [{⟨9, 1⟩}, {⟨10, 1⟩}],[{⟨9, 1⟩}],[{⟨1, 1⟩}],[(7, 7)],[(1, 1, 1)],[(1, 1, 1)]

---

su(2)
so(525) ⟵ su(525)
sp(3)

[{⟨1, 1⟩},{⟨524, 1⟩}],[{⟨1, 1⟩}],[(524)],[(3, 0, 1)]

---

su(2)
so(527) ⟵ su(527)
so(32)

[{⟨1, 1⟩},{⟨526, 1⟩}],[{⟨1, 1⟩}],[(526)],[{⟨1, 2⟩}]

---

su(2) ⟵ sp(264)
su(23)
so(33) ⟵ so(528)
sp(16) su(3) ⟵ su(528)
su(3)
su(32)
su(33)

[{⟨1, 1⟩},{⟨527, 1⟩}], [{⟨1, 1⟩}], [(527)], [{⟨1, 1⟩}], [{⟨1, 1⟩, ⟨22, 1⟩}],[{⟨2, 1⟩}],[{⟨1, 2⟩}],[(21, 1),(1, 21)], [(31, 0),(0, 31)], [{⟨1, 2⟩},{⟨31, 2⟩}], [{⟨2, 1⟩},{⟨31, 1⟩}]

---

su(2)
sp(270)
su(6)
so(6) ⟵ so(540)
su(4)
su(4)
su(4) su(540)
su(4)
su(5)
su(7)
su(9)
su(10)

[{⟨1, 1⟩},{⟨539, 1⟩}],[{⟨1, 1⟩}],[(539)],[(1, 0, 1, 0, 1)], [{⟨1, 1⟩}], [(7, 0, 0)], [(2, 4, 0),(0, 4, 2)], [(3, 1, 2),(2, 1, 3)], [(5, 2, 0),(0, 2, 5)], [(8, 0, 1),(1, 0, 8)], [(4, 0, 1, 0),(0, 1, 0, 4)], [{⟨1, 2⟩, ⟨5, 1⟩},{⟨2, 1⟩, ⟨6, 2⟩}], [{⟨2, 2⟩},{⟨7, 2⟩}],[{⟨1, 2⟩, ⟨9, 1⟩},{⟨1, 1⟩, ⟨9, 2⟩}]

---

su(2)
sp(272)
sp(8) su(544)
so(544)

[{⟨1, 1⟩},{⟨543, 1⟩}], [{⟨1, 1⟩}], [(543)], [{⟨3, 1⟩}], [{⟨1, 1⟩}]

---

su(2) ⟵ sp(273)
su(546)
so(14) ⟵ so(546)

[{⟨1, 1⟩},{⟨545, 1⟩}], [{⟨1, 1⟩}], [(545)], [{⟨1, 1⟩}], [{⟨1, 3⟩}]

---

su(2)
sp(2)
sp(2)
sp(2) sp(280)
sp(6)
sp(7)
so(7)
so(33)
sp(17) so(560)
so(12) su(4) su(560)
so(16) su(5)
su(5)
su(5)
su(6)
su(7)
su(14)
so(10) ⟵ su(16)

[{⟨1, 1⟩},{⟨559, 1⟩}],[{⟨1, 1⟩}],[(559)],[(5, 3)],[(9, 1)], [(13, 0)], [{⟨1, 1⟩, ⟨2, 1⟩}], [{⟨1, 3⟩}], [{⟨1, 1⟩}], [(1, 0, 3)], [{⟨1, 2⟩}], [{⟨2, 1⟩}], [{⟨1, 1⟩, ⟨2, 1⟩}], [{⟨3, 1⟩}], [(13, 0, 0),(0, 0, 13)], [(1, 3, 0, 0),(0, 0, 3, 1)], [(2, 0, 2, 0),(0, 2, 0, 2)],[(5, 0, 0, 1),(1, 0, 0, 5)],[(1, 0, 0, 2, 0),(0, 2, 0, 0, 1)], [{⟨1, 3⟩, ⟨6, 1⟩},{⟨1, 1⟩, ⟨6, 3⟩}], [{⟨1, 3⟩},{⟨13, 3⟩}], [{⟨3, 1⟩},{⟨13, 1⟩}], [(0, 1, 0, 1, 0),(0, 1, 0, 1, 0)]

---

su(2)
so(561)
so(34)
su(3)
su(3) ⟵ su(561)
su(33)
su(34)

[{⟨1, 1⟩},{⟨560, 1⟩}],[{⟨1, 1⟩}],[(560)],[{⟨2, 1⟩}],[(10, 5),(5, 10)], [(32, 0),(0, 32)], [{⟨1, 2⟩},{⟨32, 2⟩}], [{⟨2, 1⟩},{⟨32, 1⟩}]

---

su(2)
so(567)
so(8) su(567)
su(3)

[{⟨1, 1⟩},{⟨566, 1⟩}], [{⟨1, 1⟩}], [(566)], [(2, 1, 0, 0),(0, 1, 2, 0),(0, 1, 0, 2)],[(17, 2),(2, 17)]

---

su(2) ⟵ sp(285)
so(570) ⟵ su(570)
su(3)

[{⟨1, 1⟩},{⟨569, 1⟩}],[{⟨1, 1⟩}],[(569)],[{⟨1, 1⟩}],[(14, 3),(3, 14)]

---

su(2)
sp(286)
sp(6)
so(572) ⟵ su(572)
su(12)

[{⟨1, 1⟩},{⟨571, 1⟩}], [{⟨1, 1⟩}], [(571)], [{⟨5, 1⟩}], [{⟨1, 1⟩}],[{⟨1, 1⟩, ⟨2, 1⟩},{⟨10, 1⟩, ⟨11, 1⟩}]

---

su(2)
so(575)
su(24) su(575)
su(3)

[{⟨1, 1⟩},{⟨574, 1⟩}], [{⟨1, 1⟩}], [(574)], [{⟨1, 1⟩, ⟨23, 1⟩}],[(22, 1),(1, 22)]

---

su(2) ⟵ sp(288)
su(576)
so(9) ⟵ so(576)

[{⟨1, 1⟩},{⟨575, 1⟩}], [{⟨1, 1⟩}], [(575)], [{⟨1, 1⟩}], [(2, 0, 0, 1)]

---

su(2) ⟵ so(585)
su(585)
su(3)

[{⟨1, 1⟩},{⟨584, 1⟩}],[{⟨1, 1⟩}],[(584)],[(12, 4),(4, 12)]

---

su(2) ⟵ sp(294)
so(588) ⟵ su(588)
su(7)

[{⟨1, 1⟩},{⟨587, 1⟩}], [{⟨1, 1⟩}], [(587)], [{⟨1, 1⟩}], [{⟨2, 1⟩, ⟨4, 1⟩},{⟨3, 1⟩, ⟨5, 1⟩}]

---

su(2) ⟵ sp(297)
so(9)
sp(3) su(594)
sp(4) ⟵ so(594)
sp(4) su(4)
so(34) su(11)

[{⟨1, 1⟩},{⟨593, 1⟩}], [{⟨1, 1⟩}], [(593)], [{⟨1, 1⟩}], [(1, 0, 1, 0)], [(0, 1, 2)], [(0, 0, 0, 2)], [(2, 1, 0, 0)], [{⟨1, 2⟩}], [(8, 1, 0),(0, 1, 8)],[{⟨1, 1⟩, ⟨9, 1⟩},{⟨2, 1⟩, ⟨10, 1⟩}]

---

su(2)
so(5)
so(595)
so(35)
sp(17) su(3)
su(3) ⟵ su(595)
su(34)
su(35)

[{⟨1, 1⟩},{⟨594, 1⟩}], [{⟨1, 1⟩}], [(594)], [(6, 2)], [{⟨2, 1⟩}], [{⟨1, 2⟩}], [(9, 6),(6, 9)], [(33, 0),(0, 33)], [{⟨1, 2⟩},{⟨33, 2⟩}],[{⟨2, 1⟩},{⟨33, 1⟩}]

---

su(2) ⟵ sp(306)
so(612) ⟵ su(612)
su(3)

[{⟨1, 1⟩},{⟨611, 1⟩}], [{⟨1, 1⟩}], [(611)], [{⟨1, 1⟩}], [(8, 7),(7, 8)]

---

su(2)
sp(2) ⟵ sp(308)
sp(3) su(616)
so(7) ⟵ so(616)
su(4)

[{⟨1, 1⟩},{⟨615, 1⟩}], [{⟨1, 1⟩}], [(615)], [(7, 2)], [(0, 2, 1)],[{⟨1, 1⟩}],[(2, 0, 2)],[(6, 0, 2),(2, 0, 6)]

---

su(2) ⟵ sp(312)
su(25) ⟵ so(624) ⟵ su(624)
su(3)

[{⟨1, 1⟩},{⟨623, 1⟩}], [{⟨1, 1⟩}], [(623)], [{⟨1, 1⟩}], [{⟨1, 1⟩, ⟨24, 1⟩}],[(23, 1),(1, 23)]

---

su(2)
so(625) ⟵ su(625)
so(5)

[{⟨1, 1⟩},{⟨624, 1⟩}],[{⟨1, 1⟩}],[(624)],[(4, 4)]

---

su(2) ⟵ so(627)
su(627)
su(3)

[{⟨1, 1⟩},{⟨626, 1⟩}],[{⟨1, 1⟩}],[(626)],[(18, 2),(2, 18)]

---

su(2)
so(35) ⟵ so(629) ⟵ su(629)
sp(18)

[{⟨1, 1⟩},{⟨628, 1⟩}], [{⟨1, 1⟩}], [(628)], [{⟨1, 2⟩}], [{⟨2, 1⟩}]

---

su(2) ⟵ sp(315)
so(36) ⟵ so(630)
su(3)
su(4) su(630)
su(35)
su(8)
su(36)
su(9)

[{⟨1, 1⟩},{⟨629, 1⟩}], [{⟨1, 1⟩}], [(629)], [{⟨1, 1⟩}],

[{⟨2, 1⟩}],[(34, 0),(0, 34)],[(3, 2, 1),(1, 2, 3)],[{⟨1, 2⟩},{⟨34, 2⟩}],[{⟨2, 1⟩},{⟨34, 1⟩}],[{⟨1, 2⟩, ⟨2, 1⟩},{⟨6, 1⟩, ⟨7, 2⟩}],[{⟨1, 1⟩, ⟨3, 1⟩},{⟨6, 1⟩, ⟨8, 1⟩}]

su(2), sp(2) ← sp(320); sp(320), so(640), su(3), su(4) ← su(640)

[{⟨1, 1⟩},{⟨639, 1⟩}], [{⟨1, 1⟩}], [(639)], [(3, 5)], [{⟨1, 1⟩}],[(15, 3),(3, 15)],[(5, 1, 1),(1, 1, 5)]

su(2) ← sp(324); sp(324), so(648), su(3) ← su(648)

[{⟨1, 1⟩},{⟨647, 1⟩}],[{⟨1, 1⟩}],[(647)],[{⟨1, 1⟩}],[(11, 5),(5, 11)]

su(2) ← sp(325); so(5), e6 ← so(650); sp(325), so(650) ← su(650)

[{⟨1, 1⟩},{⟨649, 1⟩}],[{⟨1, 1⟩}],[(649)],[{⟨1, 1⟩}],[(11, 0)],[{⟨1, 1⟩, ⟨6, 1⟩}]

su(2), sp(2) ← sp(330); so(10) ← so(660); sp(330), so(660) ← su(660)

[{⟨1, 1⟩},{⟨659, 1⟩}], [{⟨1, 1⟩}], [(659)], [(1, 8)], [{⟨1, 1⟩}],[(4, 0, 0, 0, 0)]

su(2), so(15), so(36) ← so(665); so(665), su(3) ← su(665)

[{⟨1, 1⟩},{⟨664, 1⟩}], [{⟨1, 1⟩}], [(664)], [{⟨1, 3⟩}], [{⟨1, 2⟩}],[(13, 4),(4, 13)]

su(2) ← sp(333); so(37), sp(18) ← so(666); sp(333), so(666), su(3), su(36), su(37) ← su(666)

[{⟨1, 1⟩},{⟨665, 1⟩}], [{⟨1, 1⟩}], [(665)], [{⟨1, 1⟩}], [{⟨2, 1⟩}], [{⟨1, 2⟩}], [(35, 0),(0, 35)], [{⟨1, 2⟩},{⟨35, 2⟩}],[{⟨2, 1⟩},{⟨35, 1⟩}]

su(2) ← sp(336); so(7) ← so(8); so(9), so(8), so(8) ← so(672); sp(336), so(672), so(10) ← su(672)

[{⟨1, 1⟩},{⟨671, 1⟩}], [{⟨1, 1⟩}], [(671)], [{⟨1, 1⟩}], [(0, 0, 0, 3)], [(3, 0, 1, 0),(3, 0, 0, 1),(1, 0, 3, 0),(1, 0, 0, 3),(0, 0, 3, 1),(0, 0, 1, 3)], [(5, 0, 0, 0),(0, 0, 5, 0),(0, 0, 0, 5)],[(0, 0, 5)],[(0, 0, 0, 3, 0),(0, 0, 0, 0, 3)]

su(2), su(26) ← so(675); so(675), su(3) ← su(675)

[{⟨1, 1⟩},{⟨674, 1⟩}], [{⟨1, 1⟩}], [(674)], [{⟨1, 1⟩, ⟨25, 1⟩}],[(24, 1),(1, 24)]

su(2) ← sp(340); so(5), so(17) ← so(680); sp(340), so(680), su(4), su(15), su(17) ← su(680)

[{⟨1, 1⟩},{⟨679, 1⟩}], [{⟨1, 1⟩}], [(679)], [{⟨1, 1⟩}], [(0, 14)], [{⟨3, 1⟩}], [(14, 0, 0),(0, 0, 14)], [{⟨1, 3⟩},{⟨14, 3⟩}],[{⟨3, 1⟩},{⟨14, 1⟩}]

su(2) ← sp(345); sp(345), so(690), su(3) ← su(690)

[{⟨1, 1⟩},{⟨689, 1⟩}],[{⟨1, 1⟩}],[(689)],[{⟨1, 1⟩}],[(19, 2),(2, 19)]

su(2), so(7) ← so(693); so(693), su(3) ← su(693)

[{⟨1, 1⟩},{⟨692, 1⟩}],[{⟨1, 1⟩}],[(692)],[(1, 2, 0)],[(10, 6),(6, 10)]

su(2) ← sp(350); sp(350), so(700), su(5), su(5), su(6) ← su(700)

[{⟨1, 1⟩},{⟨699, 1⟩}], [{⟨1, 1⟩}], [(699)], [{⟨1, 1⟩}], [(1, 0, 3, 0),(0, 3, 0, 1)], [(2, 1, 1, 0),(0, 1, 1, 2)], [(4, 0, 0, 0, 1),(1, 0, 0, 0, 4)]

su(2) ← sp(351); so(37), sp(19) ← so(702); sp(351), so(702) ← su(702)

[{⟨1, 1⟩},{⟨701, 1⟩}], [{⟨1, 1⟩}], [(701)], [{⟨1, 1⟩}], [{⟨1, 2⟩}],[{⟨2, 1⟩}]

su(2), so(38) ← so(703); so(703), su(3), su(37), su(38) ← su(703)

[{⟨1, 1⟩},{⟨702, 1⟩}],[{⟨1, 1⟩}],[(702)],[{⟨2, 1⟩}],[(36, 0),(0, 36)],[{⟨1, 2⟩},{⟨36, 2⟩}],[{⟨2, 1⟩},{⟨36, 1⟩}]

su(2) ← sp(357); g2 ← so(7) ← so(714); sp(357), so(714), su(3) ← su(714)

[{⟨1, 1⟩},{⟨713, 1⟩}], [{⟨1, 1⟩}], [(713)], [{⟨1, 1⟩}], [(6, 0, 0)],[(6, 0)],[(16, 3),(3, 16)]

su(2), so(5), so(13), so(13), sp(5) ← so(715); so(715), su(4), su(5), su(10), su(11), su(13) ← su(715)

[{⟨1, 1⟩},{⟨714, 1⟩}], [{⟨1, 1⟩}], [(714)], [(1, 10)], [{⟨4, 1⟩}],[{⟨1, 1⟩, ⟨2, 1⟩}],[(4, 0, 0, 0, 0)],[(9, 0, 1),(1, 0, 9)], [(9, 0, 0, 0),(0, 0, 0, 9)], [{⟨1, 4⟩},{⟨9, 4⟩}],[{⟨1, 2⟩, ⟨10, 1⟩},{⟨1, 1⟩, ⟨10, 2⟩}],[{⟨4, 1⟩},{⟨9, 1⟩}]

su(2) ← sp(360); so(8), so(7) ← so(720); sp(360), so(720), su(3), su(5), su(5), su(6), su(9), so(10) ← su(720)

[{⟨1, 1⟩},{⟨719, 1⟩}], [{⟨1, 1⟩}], [(719)], [{⟨1, 1⟩}], [{⟨2, 1⟩, ⟨6, 1⟩}], [(0, 2, 1)], [(9, 7),(7, 9)], [(1, 2, 0, 1),(1, 0, 2, 1)], [(5, 1, 0, 0),(0, 0, 1, 5)], [(3, 0, 0, 1, 0),(0, 1, 0, 0, 3)],[{⟨1, 1⟩, ⟨6, 1⟩},{⟨3, 1⟩, ⟨8, 1⟩}],[(2, 0, 0, 1, 0),(2, 0, 0, 0, 1)]

su(2) ← sp(364); su(27) ← so(728); sp(364), so(728), su(3), su(13) ← su(728)

[{⟨1, 1⟩},{⟨727, 1⟩}], [{⟨1, 1⟩}], [(727)], [{⟨1, 1⟩}], [{⟨1, 1⟩, ⟨26, 1⟩}], [(25, 1),(1, 25)], [{⟨1, 1⟩, ⟨2, 1⟩},{⟨11, 1⟩, ⟨12, 1⟩}]

su(2), su(3), so(6), g2 ← so(729) ← su(729)

[{⟨1, 1⟩},{⟨728, 1⟩}], [{⟨1, 1⟩}], [(728)], [(8, 8)], [(2, 2, 2)],[(2, 2)]

su(2), su(7), so(6) ← so(735); so(735), su(7) ← su(735)

[{⟨1, 1⟩},{⟨734, 1⟩}], [{⟨1, 1⟩}], [(734)], [{⟨1, 2⟩, ⟨6, 2⟩}], [(4, 1, 1)], [{⟨1, 1⟩, ⟨2, 1⟩, ⟨6, 1⟩},{⟨1, 1⟩, ⟨5, 1⟩, ⟨6, 1⟩}]

su(2) ← sp(370); so(38) ← so(740); sp(370), so(740) ← su(740)

[{⟨1, 1⟩},{⟨739, 1⟩}], [{⟨1, 1⟩}], [(739)], [{⟨1, 1⟩}], [{⟨1, 2⟩}]

su(2), so(39), sp(19) ← so(741); so(741), su(3), su(3), su(38), su(39) ← su(741)

[{⟨1, 1⟩},{⟨740, 1⟩}], [{⟨1, 1⟩}], [(740)], [{⟨2, 1⟩}], [{⟨1, 2⟩}], [(12, 5),(5, 12)], [(37, 0),(0, 37)], [{⟨1, 2⟩},{⟨37, 2⟩}],[{⟨2, 1⟩},{⟨37, 1⟩}]

su(2) ← sp(374); g2 ← so(748); sp(374), so(748) ← su(748)

[{⟨1, 1⟩},{⟨747, 1⟩}], [{⟨1, 1⟩}], [(747)], [{⟨1, 1⟩}], [(0, 4)]

su(2) ← sp(375); sp(375), so(750), su(3), su(4) ← su(750)

[{⟨1, 1⟩},{⟨749, 1⟩}],[{⟨1, 1⟩}],[(749)],[{⟨1, 1⟩}],[(14, 4),(4, 14)],[(4, 3, 0),(0, 3, 4)]

su(2) ← sp(378); sp(378), so(756), su(3), su(4), su(7) ← su(756)

[{⟨1, 1⟩},{⟨755, 1⟩}],[{⟨1, 1⟩}],[(755)],[{⟨1, 1⟩}],[(20, 2),(2, 20)], [(2, 3, 1),(1, 3, 2)], [{⟨1, 2⟩, ⟨3, 1⟩},{⟨4, 1⟩, ⟨6, 2⟩}]

su(2), so(13) ← sp(384); so(9) ← so(768); sp(384), so(768) ← su(768)

[{⟨1, 1⟩},{⟨767, 1⟩}], [{⟨1, 1⟩}], [(767)], [{⟨1, 1⟩, ⟨6, 1⟩}],[{⟨1, 1⟩}],[(0, 0, 1, 1)]

su(2) ← sp(385); so(5), so(10) ← so(770); sp(385), so(770), su(4), su(4) ← su(770)

[{⟨1, 1⟩},{⟨769, 1⟩}], [{⟨1, 1⟩}], [(769)], [{⟨1, 1⟩}], [(3, 6)],[(0, 2, 0, 0, 0)],[(5, 0, 3),(3, 0, 5)],[(6, 2, 0),(0, 2, 6)]

su(2), so(39), sp(20) ← so(779) ← su(779)

[{⟨1, 1⟩},{⟨778, 1⟩}], [{⟨1, 1⟩}], [(778)], [{⟨1, 2⟩}], [{⟨2, 1⟩}]

su(2) ← sp(390)
sp(5), so(40) → so(780)
su(3), su(4), su(12), su(39), su(40)
→ su(780)

[{⟨1, 1⟩},{⟨779, 1⟩}], [{⟨1, 1⟩}], [(779)], [{⟨1, 1⟩}], [(0, 2, 0, 0, 0)], [{⟨2, 1⟩}], [(38, 0),(0, 38)], [(9, 1, 0),(0, 1, 9)], [{⟨1, 1⟩, ⟨10, 1⟩},{⟨2, 1⟩, ⟨11, 1⟩}], [{⟨1, 2⟩},{⟨38, 2⟩}],[{⟨2, 1⟩},{⟨38, 1⟩}]

---

su(2), su(28) → so(783)
su(3)
→ su(783)

[{⟨1, 1⟩},{⟨782, 1⟩}], [{⟨1, 1⟩}], [(782)], [{⟨1, 1⟩, ⟨27, 1⟩}],[(26, 1),(1, 26)]

---

su(2) ← sp(392)
su(7) ← so(784)
→ su(784)

[{⟨1, 1⟩},{⟨783, 1⟩}], [{⟨1, 1⟩}], [(783)], [{⟨1, 1⟩}], [{⟨3, 1⟩, ⟨4, 1⟩}]

---

su(2), sp(3), sp(4), sp(4) → sp(396)
sp(4), so(12) → so(792)
su(3), su(6), su(8), su(12)
→ su(792)

[{⟨1, 1⟩},{⟨791, 1⟩}], [{⟨1, 1⟩}], [(791)], [(7, 0, 0)], [(0, 1, 1, 0)], [(5, 0, 0, 0)], [{⟨1, 1⟩}], [(0, 1, 0, 1)], [{⟨5, 1⟩, ⟨6, 1⟩}], [(17, 3),(3, 17)], [(7, 0, 0, 0, 0),(0, 0, 0, 0, 7)], [{⟨1, 5⟩},{⟨7, 5⟩}],[{⟨5, 1⟩},{⟨7, 1⟩}]

---

su(2), sp(9) → sp(399)
so(798)
su(3)
→ su(798)

[{⟨1, 1⟩},{⟨797, 1⟩}], [{⟨1, 1⟩}], [(797)], [{⟨3, 1⟩}], [{⟨1, 1⟩}],[(11, 6),(6, 11)]

---

su(2) ← sp(400)
so(16) ← so(800)
→ su(800)

[{⟨1, 1⟩},{⟨799, 1⟩}], [{⟨1, 1⟩}], [(799)], [{⟨1, 1⟩}], [{⟨1, 3⟩}]

---

su(2) ← sp(405)
so(5) ← so(810)
→ su(810)

[{⟨1, 1⟩},{⟨809, 1⟩}], [{⟨1, 1⟩}], [(809)], [{⟨1, 1⟩}], [(2, 8)]

---

su(2), sp(2), sp(8) → sp(408)
so(18) ← so(816)
su(4), su(16), su(18)
→ su(816)

[{⟨1, 1⟩},{⟨815, 1⟩}], [{⟨1, 1⟩}], [(815)], [(15, 0)], [{⟨1, 3⟩}], [{⟨1, 1⟩}], [{⟨3, 1⟩}], [(15, 0, 0),(0, 0, 15)], [{⟨1, 3⟩},{⟨15, 3⟩}],[{⟨3, 1⟩},{⟨15, 1⟩}]

---

su(2), so(5), so(7), so(40) → so(819) ← su(819)

[{⟨1, 1⟩},{⟨818, 1⟩}], [{⟨1, 1⟩}], [(818)], [(12, 0)], [(3, 1, 0)],[{⟨1, 2⟩}]

---

su(2) ← sp(410)
so(41), sp(20) → so(820)
su(3), su(40), su(41)
→ su(820)

[{⟨1, 1⟩},{⟨819, 1⟩}], [{⟨1, 1⟩}], [(819)], [{⟨1, 1⟩}], [{⟨2, 1⟩}], [{⟨1, 2⟩}], [(39, 0),(0, 39)], [{⟨1, 2⟩},{⟨39, 2⟩}],[{⟨2, 1⟩},{⟨39, 1⟩}]

---

su(2), so(7), sp(4), so(6), so(6)
sp(4) ← so(825)
su(3) ← su(825)
su(10)
→ su(825)

[{⟨1, 1⟩},{⟨824, 1⟩}], [{⟨1, 1⟩}], [(824)], [(0, 3, 0)], [(0, 0, 2, 0)], [(0, 4, 4)], [(8, 0, 0)], [(21, 2),(2, 21)], [{⟨2, 2⟩},{⟨8, 2⟩}]

---

su(2) ← sp(416)
so(832) ← su(832)
so(14)

[{⟨1, 1⟩},{⟨831, 1⟩}], [{⟨1, 1⟩}], [(831)], [{⟨1, 1⟩}], [{⟨1, 1⟩, ⟨6, 1⟩},{⟨1, 1⟩, ⟨7, 1⟩}]

---

su(2) ← sp(418)
so(5) ← so(836) ← su(836)
su(3)

[{⟨1, 1⟩},{⟨835, 1⟩}], [{⟨1, 1⟩}], [(835)], [{⟨1, 1⟩}], [(7, 2)],[(10, 7),(7, 10)]

---

su(2) ← sp(420)
su(29), so(8), so(8) → so(840)
su(3), su(3), su(3), su(4), su(5), su(6), su(6), su(6), su(7)
→ su(840)

[{⟨1, 1⟩},{⟨839, 1⟩}], [{⟨1, 1⟩}], [(839)], [{⟨1, 1⟩}], [{⟨1, 1⟩, ⟨28, 1⟩}], [(1, 1, 1, 0),(1, 1, 0, 1),(0, 1, 1, 1)], [(2, 0, 2, 0),(2, 0, 0, 2),(0, 0, 2, 2)], [(13, 5),(5, 13)], [(15, 4),(4, 15)], [(27, 1),(1, 27)], [(1, 6, 0),(0, 6, 1)], [(3, 2, 0, 0),(0, 0, 2, 3)], [(1, 0, 2, 0, 0),(0, 0, 2, 0, 1)], [(1, 1, 0, 1, 0),(0, 1, 0, 1, 1)], [(3, 0, 1, 0, 0),(0, 0, 1, 0, 3)], [{⟨1, 2⟩, ⟨4, 1⟩},{⟨3, 1⟩, ⟨6, 2⟩}]

---

su(2) ← so(855)
su(3)
→ su(855)

[{⟨1, 1⟩},{⟨854, 1⟩}], [{⟨1, 1⟩}], [(854)], [(9, 8),(8, 9)]

---

su(2) ← sp(430)
so(41), sp(21) → so(860)
→ su(860)

[{⟨1, 1⟩},{⟨859, 1⟩}], [{⟨1, 1⟩}], [(859)], [{⟨1, 1⟩}], [{⟨1, 2⟩}],[{⟨2, 1⟩}]

---

su(2), so(42) → so(861)
su(3), su(41), su(42)
→ su(861)

[{⟨1, 1⟩},{⟨860, 1⟩}], [{⟨1, 1⟩}], [(860)], [{⟨2, 1⟩}], [(40, 0),(0, 40)], [{⟨1, 2⟩},{⟨40, 2⟩}],[{⟨2, 1⟩},{⟨40, 1⟩}]

---

su(2) ← sp(432)
so(864) ← su(864)
su(4)

[{⟨1, 1⟩},{⟨863, 1⟩}], [{⟨1, 1⟩}], [(863)], [{⟨1, 1⟩}], [(7, 0, 2),(2, 0, 7)]

---

su(2) ← sp(437)
so(874) ← su(874)
su(3)

[{⟨1, 1⟩},{⟨873, 1⟩}], [{⟨1, 1⟩}], [(873)], [{⟨1, 1⟩}], [(18, 3),(3, 18)]

---

su(2) ← so(875)
su(4) ← su(875)
su(5)

[{⟨1, 1⟩},{⟨874, 1⟩}], [{⟨1, 1⟩}], [(874)], [(4, 1, 2),(2, 1, 4)], [(4, 0, 0, 2),(2, 0, 0, 4)]

---

su(2), sp(2), sp(2)
sp(2) ← sp(440)
so(880)
→ su(880)

[{⟨1, 1⟩},{⟨879, 1⟩}], [{⟨1, 1⟩}], [(879)], [(1, 9)], [(5, 4)], [{⟨1, 1⟩}]

---

su(2) ← sp(441)
so(882) ← su(882)
su(7)

[{⟨1, 1⟩},{⟨881, 1⟩}], [{⟨1, 1⟩}], [(881)], [{⟨1, 1⟩}], [{⟨1, 1⟩, ⟨2, 2⟩},{⟨5, 2⟩, ⟨6, 1⟩}]

---

su(2), sp(5) → so(891) ← su(891)

[{⟨1, 1⟩},{⟨890, 1⟩}], [{⟨1, 1⟩}], [(890)], [(1, 0, 1, 0, 0)]

---

su(2), sp(2), sp(7)
sp(2) ← sp(448)
so(14), g2 → so(896)
su(6)
→ su(896)

[{⟨1, 1⟩},{⟨895, 1⟩}], [{⟨1, 1⟩}], [(895)], [(11, 1)], [{⟨1, 1⟩, ⟨2, 1⟩}], [{⟨1, 1⟩}], [{⟨1, 1⟩, ⟨2, 1⟩}], [(1, 3)], [(1, 1, 1, 0, 0),(0, 0, 1, 1, 1)]

---

su(2) ← so(897)
su(3)
→ su(897)

[{⟨1, 1⟩},{⟨896, 1⟩}], [{⟨1, 1⟩}], [(896)], [(22, 2),(2, 22)]

---

su(2), su(30) → so(899)
su(3)
→ su(899)

[{⟨1, 1⟩},{⟨898, 1⟩}], [{⟨1, 1⟩}], [(898)], [{⟨1, 1⟩, ⟨29, 1⟩}], [(28, 1),(1, 28)]

---

su(2) ← sp(450)
so(900) ← su(900)
su(4)

[{⟨1, 1⟩},{⟨899, 1⟩}], [{⟨1, 1⟩}], [(899)], [{⟨1, 1⟩}], [(3, 4, 0),(0, 4, 3)]

---

su(2) ← sp(451)
so(42) ← so(902)
→ su(902)

[{⟨1, 1⟩},{⟨901, 1⟩}], [{⟨1, 1⟩}], [(901)], [{⟨1, 1⟩}], [{⟨1, 2⟩}]

su(2)
so(43) ← so(903)
sp(21)
su(3)
su(42)
su(43)
su(903)

[{⟨1, 1⟩},{⟨902, 1⟩}], [{⟨1, 1⟩}], [(902)], [{⟨2, 1⟩}], [{⟨1, 2⟩}], [(41, 0),(0, 41)], [{⟨1, 2⟩},{⟨41, 2⟩}], [{⟨2, 1⟩},{⟨41, 1⟩}]

---

su(2) ← sp(455)
so(9)
sp(7)
so(910)
su(3)
su(14)
su(910)

[{⟨1, 1⟩},{⟨909, 1⟩}], [{⟨1, 1⟩}], [(909)], [{⟨1, 1⟩}], [(2, 1, 0, 0)], [{⟨4, 1⟩}], [(12, 6),(6, 12)], [{⟨1, 1⟩, ⟨2, 1⟩}, {⟨12, 1⟩, ⟨13, 1⟩}]

---

su(2)
$\mathfrak{c}_7$ ←
sp(456)
so(912)
su(912)

[{⟨1, 1⟩},{⟨911, 1⟩}], [{⟨1, 1⟩}], [(911)], [{⟨2, 1⟩}], [{⟨1, 1⟩}]

---

su(2)
sp(2)
sp(462)
su(12)
so(9)
sp(3) ← so(924)
sp(3)
$\mathfrak{g}_2$
su(4)
su(4)
su(5)
su(7)
su(8)
su(12)
su(924)

[{⟨1, 1⟩},{⟨923, 1⟩}], [{⟨1, 1⟩}], [(923)], [(3, 6)], [{⟨1, 1⟩}], [{⟨6, 1⟩}], [(1, 0, 0, 2)], [(2, 2, 0)], [(4, 1, 0)], [(4, 1)], [(6, 1, 1),(1, 1, 6)], [(10, 0, 1),(1, 0, 10)], [(6, 0, 0, 1),(1, 0, 0, 6)], [{⟨1, 6⟩},{⟨6, 6⟩}], [{⟨1, 3⟩, ⟨7, 1⟩}, {⟨1, 1⟩, ⟨7, 3⟩}],[{⟨1, 2⟩, ⟨11, 1⟩},{⟨1, 1⟩, ⟨11, 2⟩}]

---

su(2)
so(5) ← so(935)
so(11)
su(3)
su(935)

[{⟨1, 1⟩},{⟨934, 1⟩}], [{⟨1, 1⟩}], [(934)], [(5, 4)], [(4, 0, 0, 0)],[(16, 4),(4, 16)]

---

su(2)
so(43)
so(945)
sp(22)
so(10)
su(3)
su(4)
su(5)
su(5)
su(8)
su(945)

[{⟨1, 1⟩},{⟨944, 1⟩}], [{⟨1, 1⟩}], [(944)], [{⟨1, 2⟩}], [{⟨2, 1⟩}], [(1, 0, 1, 0, 0)], [(14, 5),(5, 14)], [(2, 5, 0),(0, 5, 2)], [(3, 1, 0, 1),(1, 0, 1, 3)], [(5, 0, 1, 0),(0, 1, 0, 5)], [{⟨1, 2⟩, ⟨6, 1⟩},{⟨2, 1⟩, ⟨7, 2⟩}]

---

su(2) ← sp(473)
so(44) ← so(946)
su(3)
su(43)
su(44)
su(946)

[{⟨1, 1⟩},{⟨945, 1⟩}], [{⟨1, 1⟩}], [(945)], [{⟨1, 1⟩}], [{⟨2, 1⟩}], [(42, 0),(0, 42)], [{⟨1, 2⟩},{⟨42, 2⟩}], [{⟨2, 1⟩},{⟨42, 1⟩}]

---

su(2) ← sp(476)
so(17) ← so(952)
su(952)

[{⟨1, 1⟩},{⟨951, 1⟩}], [{⟨1, 1⟩}], [(951)], [{⟨1, 1⟩}], [{⟨1, 3⟩}]

---

su(2) ← sp(480)
su(31)
so(960)
so(6)
su(3)
su(3)
su(3)
su(960)

[{⟨1, 1⟩},{⟨959, 1⟩}], [{⟨1, 1⟩}], [(959)], [{⟨1, 1⟩}], [{⟨1, 1⟩, ⟨30, 1⟩}], [(1, 3, 3)], [(11, 7),(7, 11)], [(19, 3),(3, 19)],[(29, 1),(1, 29)]

---

su(2)
so(5) ← so(969)
so(19)
su(4)
su(17)
su(19)
su(969)

[{⟨1, 1⟩},{⟨968, 1⟩}], [{⟨1, 1⟩}], [(968)], [(0, 16)], [{⟨3, 1⟩}], [(16, 0, 0),(0, 0, 16)], [{⟨1, 3⟩},{⟨16, 3⟩}], [{⟨3, 1⟩},{⟨16, 1⟩}]

---

su(2) ← sp(486)
so(972)
su(3)
su(972)

[{⟨1, 1⟩},{⟨971, 1⟩}],[{⟨1, 1⟩}],[(971)],[{⟨1, 1⟩}],[(23, 2),(2, 23)]

---

su(2)
sp(490)
su(6)
so(980)
su(5)
su(980)

[{⟨1, 1⟩},{⟨979, 1⟩}],[{⟨1, 1⟩}],[(979)],[(0, 0, 3, 0, 0)],[{⟨1, 1⟩}],[(0, 3, 1, 0),(0, 1, 3, 0)]

---

su(2)
so(989) ← su(989)
so(44)

[{⟨1, 1⟩},{⟨988, 1⟩}],[{⟨1, 1⟩}],[(988)],[{⟨1, 2⟩}]

---

su(2) ← sp(495)
so(45)
so(990)
sp(22)
su(3)
su(3)
su(44)
su(9)
su(45)
su(10)
su(990)

[{⟨1, 1⟩},{⟨989, 1⟩}], [{⟨1, 1⟩}], [(989)], [{⟨1, 1⟩}], [{⟨2, 1⟩}], [{⟨1, 2⟩}], [(10, 8),(8, 10)], [(43, 0),(0, 43)], [{⟨1, 2⟩},{⟨43, 2⟩}], [{⟨2, 1⟩},{⟨43, 1⟩}], [{⟨1, 2⟩, ⟨2, 1⟩},{⟨7, 1⟩, ⟨8, 2⟩}], [{⟨1, 1⟩, ⟨3, 1⟩},{⟨7, 1⟩, ⟨9, 1⟩}]

---

su(2) ← sp(500)
su(3)
so(1000)
su(5)
su(4)
su(1000)

[{⟨1, 1⟩},{⟨999, 1⟩}], [{⟨1, 1⟩}], [(999)], [{⟨1, 1⟩}], [(9, 9)],[(3, 0, 0, 3)],[(4, 2, 1),(1, 2, 4)]

---

su(2)
sp(3) ← so(1001)
so(14)
su(4)
su(5)
su(11)
su(13)
su(14)
su(1001)

[{⟨1, 1⟩},{⟨1000, 1⟩}], [{⟨1, 1⟩}], [(1000)], [(0, 0, 4)], [{⟨4, 1⟩}], [(10, 1, 0),(0, 1, 10)], [(10, 0, 0, 0),(0, 0, 0, 10)], [{⟨1, 4⟩},{⟨10, 4⟩}], [{⟨1, 1⟩, ⟨11, 1⟩},{⟨2, 1⟩, ⟨12, 1⟩}],[{⟨4, 1⟩},{⟨10, 1⟩}]

---

su(2) ← sp(504)
so(7)
so(1008)
so(7)
su(7)
su(8)
su(9)
su(1008)

[{⟨1, 1⟩},{⟨1007, 1⟩}], [{⟨1, 1⟩}], [(1007)], [{⟨1, 1⟩}], [(0, 1, 3)], [(4, 0, 1)], [{⟨1, 3⟩, ⟨2, 1⟩},{⟨5, 1⟩, ⟨6, 3⟩}], [{⟨2, 1⟩, ⟨3, 1⟩},{⟨5, 1⟩, ⟨6, 1⟩}], [{⟨1, 1⟩, ⟨4, 1⟩}, {⟨5, 1⟩, ⟨8, 1⟩}]

---

su(2)
so(1015) ← su(1015)
so(5)

[{⟨1, 1⟩},{⟨1014, 1⟩}],[{⟨1, 1⟩}],[(1014)],[(13, 0)]

---

su(2)
so(1023)
su(32)
su(3)
su(1023)

[{⟨1, 1⟩},{⟨1022, 1⟩}], [{⟨1, 1⟩}], [(1022)], [{⟨1, 1⟩, ⟨31, 1⟩}],[(30, 1),(1, 30)]

---

su(2)
so(21) ← sp(512)
sp(2)
su(5) ← so(1024)
so(22)
su(1024)

[{⟨1, 1⟩},{⟨1023, 1⟩}], [{⟨1, 1⟩}], [(1023)], [{⟨10, 1⟩}], [(7, 3)],[{⟨1, 1⟩}],[(1, 1, 1, 1)],[{⟨10, 1⟩},{⟨11, 1⟩}]

---

su(2) ← so(1029)
su(3)
su(1029)

[{⟨1, 1⟩},{⟨1028, 1⟩}], [{⟨1, 1⟩}], [(1028)], [(13, 6),(6, 13)]

---

su(2) ← sp(517)
so(45)
so(1034)
sp(23)
su(1034)

[{⟨1, 1⟩},{⟨1033, 1⟩}], [{⟨1, 1⟩}], [(1033)], [{⟨1, 1⟩}], [{⟨1, 2⟩}],[{⟨2, 1⟩}]

---

su(2)
so(1035)
so(46)
su(3)
su(3)
su(45)
su(46)
su(1035)

[{⟨1, 1⟩},{⟨1034, 1⟩}], [{⟨1, 1⟩}], [(1034)], [{⟨2, 1⟩}], [(17, 4),(4, 17)], [(44, 0),(0, 44)], [{⟨1, 2⟩},{⟨44, 2⟩}], [{⟨2, 1⟩},{⟨44, 1⟩}]

---

su(2)
sp(520)
sp(2)
so(1040)
su(1040)

[{⟨1, 1⟩},{⟨1039, 1⟩}], [{⟨1, 1⟩}], [(1039)], [(9, 2)], [{⟨1, 1⟩}]

---

su(2) ← sp(525)
so(1050)
su(3)
su(3)
su(5)
su(5)
su(6)
su(6)
su(6)
su(9)
so(10)
su(1050)

[{⟨1, 1⟩},{⟨1049, 1⟩}], [{⟨1, 1⟩}], [(1049)], [{⟨1, 1⟩}],

[(20, 3),(3, 20)], [(24, 2),(2, 24)], [(1, 2, 1, 0),(0, 1, 2, 1)],[(3, 0, 1, 1),(1, 1, 0, 3)],[(1, 0, 1, 1, 0),(0, 1, 1, 0, 1)],[(3, 0, 0, 0, 2),(2, 0, 0, 0, 3)], [(4, 1, 0, 0, 0),(0, 0, 0, 1, 4)], [{⟨1, 1⟩, ⟨5, 1⟩},{⟨4, 1⟩, ⟨8, 1⟩}], [(1, 0, 0, 2, 0),(1, 0, 0, 0, 2)]

---

su(2)
f4 ← so(1053) ← su(1053)
f4

[{⟨1, 1⟩},{⟨1052, 1⟩}], [{⟨1, 1⟩}], [(1052)], [(1, 0, 0, 1)], [(2, 0, 0, 0)]

---

su(2)
sp(528)
sp(4)
so(1056)
su(3) su(1056)
su(4)

[{⟨1, 1⟩},{⟨1055, 1⟩}], [{⟨1, 1⟩}], [(1055)], [(0, 0, 1, 1)], [{⟨1, 1⟩}],[(15, 5),(5, 15)],[(7, 2, 0),(0, 2, 7)]

---

su(2) ← sp(539)
su(1078)
sp(3) ← so(1078)

[{⟨1, 1⟩},{⟨1077, 1⟩}], [{⟨1, 1⟩}], [(1077)], [{⟨1, 1⟩}], [(2, 0, 2)]

---

su(2) ← sp(540)
su(1080)
so(46) ← so(1080)

[{⟨1, 1⟩},{⟨1079, 1⟩}], [{⟨1, 1⟩}], [(1079)], [{⟨1, 1⟩}], [{⟨1, 2⟩}]

---

su(2)
so(47) ← so(1081)
sp(23) su(3)
su(46) su(1081)
su(47)

[{⟨1, 1⟩},{⟨1080, 1⟩}], [{⟨1, 1⟩}], [(1080)], [{⟨2, 1⟩}], [{⟨1, 2⟩}], [(45, 0),(0, 45)], [{⟨1, 2⟩},{⟨45, 2⟩}], [{⟨2, 1⟩},{⟨45, 1⟩}]

---

su(2) ← sp(544)
su(33) ← so(1088) ← su(1088)
su(3)

[{⟨1, 1⟩},{⟨1087, 1⟩}], [{⟨1, 1⟩}], [(1087)], [{⟨1, 1⟩}], [{⟨1, 1⟩, ⟨32, 1⟩}],[(31, 1),(1, 31)]

---

su(2) ← sp(546)
so(1092) ← su(1092)
su(3)

[{⟨1, 1⟩},{⟨1091, 1⟩}], [{⟨1, 1⟩}], [(1091)], [{⟨1, 1⟩}], [(12, 7),(7, 12)]

---

su(2)
sp(550)
sp(3)
so(1100) ← su(1100)
su(4)

[{⟨1, 1⟩},{⟨1099, 1⟩}], [{⟨1, 1⟩}], [(1099)], [(4, 0, 1)], [{⟨1, 1⟩}],[(5, 3, 0),(0, 3, 5)]

---

su(2)
so(5) ← so(1105) ← su(1105)
so(15)

[{⟨1, 1⟩},{⟨1104, 1⟩}], [{⟨1, 1⟩}], [(1104)], [(1, 12)], [{⟨1, 1⟩, ⟨2, 1⟩}]

---

su(2)
sp(560)
sp(10)
so(1120)
su(4) su(1120)
su(5)
su(15)

[{⟨1, 1⟩},{⟨1119, 1⟩}], [{⟨1, 1⟩}], [(1119)], [{⟨3, 1⟩}], [{⟨1, 1⟩}], [(6, 0, 3),(3, 0, 6)], [(1, 1, 2, 0),(0, 2, 1, 1)], [{⟨1, 1⟩, ⟨2, 1⟩},{⟨13, 1⟩, ⟨14, 1⟩}]

---

su(2) ← sp(561)
so(9) su(1122)
so(1122)
so(18)

[{⟨1, 1⟩},{⟨1121, 1⟩}], [{⟨1, 1⟩}], [(1121)], [{⟨1, 1⟩}], [(5, 0, 0, 0)],[{⟨1, 3⟩}]

---

su(2)
so(47) ← so(1127) ← su(1127)
sp(24)

[{⟨1, 1⟩},{⟨1126, 1⟩}], [{⟨1, 1⟩}], [(1126)], [{⟨1, 2⟩}], [{⟨2, 1⟩}]

---

su(2) ← sp(564)
so(48) ← so(1128)
su(3) su(1128)
su(47)
su(48)

[{⟨1, 1⟩},{⟨1127, 1⟩}], [{⟨1, 1⟩}], [(1127)], [{⟨1, 1⟩}], [{⟨2, 1⟩}], [(46, 0),(0, 46)], [{⟨1, 2⟩},{⟨46, 2⟩}], [{⟨2, 1⟩},{⟨46, 1⟩}]

---

su(2) ← so(1131)
su(1131)
su(3)

[{⟨1, 1⟩},{⟨1130, 1⟩}], [{⟨1, 1⟩}], [(1130)], [(25, 2),(2, 25)]

---

su(2) ← sp(567)
so(5) ← so(1134)
su(3) su(1134)
su(6)
su(6)

[{⟨1, 1⟩},{⟨1133, 1⟩}], [{⟨1, 1⟩}], [(1133)], [{⟨1, 1⟩}], [(8, 2)], [(11, 8),(8, 11)], [(2, 1, 0, 0, 1),(1, 0, 0, 1, 2)], [(2, 2, 0, 0, 0),(0, 0, 0, 2, 2)]

---

su(2)
sp(2) sp(570)
sp(9)
so(20) ← so(1140)
su(3) su(1140)
su(4)
su(18)
su(20)

[{⟨1, 1⟩},{⟨1139, 1⟩}], [{⟨1, 1⟩}], [(1139)], [(17, 0)], [{⟨1, 3⟩}],[{⟨1, 1⟩}],[{⟨3, 1⟩}],[(18, 4),(4, 18)],[(17, 0, 0),(0, 0, 17)],[{⟨1, 3⟩},{⟨17, 3⟩}],[{⟨3, 1⟩},{⟨17, 1⟩}]

---

su(2)
sp(572)
sp(2)
so(11) ← so(1144) su(1144)
su(3)

[{⟨1, 1⟩},{⟨1143, 1⟩}], [{⟨1, 1⟩}], [(1143)], [(1, 10)], [{⟨1, 1⟩}],[(0, 2, 0, 0, 0)],[(21, 3),(3, 21)]

---

su(2)
su(34)
so(1155)
sp(4)
sp(5)
su(3)
su(3) su(1155)
su(3)
su(5)
su(10)

[{⟨1, 1⟩},{⟨1154, 1⟩}], [{⟨1, 1⟩}], [(1154)], [{⟨1, 1⟩, ⟨33, 1⟩}], [(2, 0, 0, 1)], [(1, 0, 0, 0, 1)], [(10, 9),(9, 10)], [(14, 6),(6, 14)], [(32, 1),(1, 32)], [(6, 1, 0, 0),(0, 0, 1, 6)],[{⟨1, 1⟩, ⟨7, 1⟩},{⟨3, 1⟩, ⟨9, 1⟩}]

---

su(2) ← sp(585)
so(1170)
su(4) su(1170)
su(4)
su(13)

[{⟨1, 1⟩},{⟨1169, 1⟩}], [{⟨1, 1⟩}], [(1169)], [{⟨1, 1⟩}], [(8, 0, 2),(2, 0, 8)], [(11, 0, 1),(1, 0, 11)], [{⟨1, 2⟩, ⟨12, 1⟩},{⟨1, 1⟩, ⟨12, 2⟩}]

---

su(2) ← so(1173)
su(1173)
su(3)

[{⟨1, 1⟩},{⟨1172, 1⟩}], [{⟨1, 1⟩}], [(1172)], [(16, 5),(5, 16)]

---

su(2)
so(1175) ← su(1175)
so(48)

[{⟨1, 1⟩},{⟨1174, 1⟩}],[{⟨1, 1⟩}],[(1174)],[{⟨1, 2⟩}]

---

su(2) ← sp(588)
su(5)
so(49) ← so(1176)
sp(24) su(3)
su(5)
su(6) su(1176)
su(6)
su(7)
su(8)
su(48)
su(49)

[{⟨1, 1⟩},{⟨1175, 1⟩}], [{⟨1, 1⟩}], [(1175)], [{⟨1, 1⟩}], [(0, 2, 2, 0)],[{⟨2, 1⟩}],[{⟨1, 2⟩}],[(47, 0),(0, 47)],[(0, 5, 0, 0),(0, 0, 5, 0)], [(0, 2, 0, 1, 0),(0, 1, 0, 2, 0)], [(0, 2, 1, 0, 0),(0, 0, 1, 2, 0)], [{⟨2, 3⟩},{⟨5, 3⟩}], [{⟨3, 2⟩},{⟨5, 2⟩}],[{⟨1, 2⟩},{⟨47, 2⟩}],[{⟨2, 1⟩},{⟨47, 1⟩}]

---

su(2) ← sp(595)
su(1190)
so(5) ← so(1190)

[{⟨1, 1⟩},{⟨1189, 1⟩}], [{⟨1, 1⟩}], [(1189)], [{⟨1, 1⟩}], [(4, 6)]

---

su(2) ← sp(600)
so(1200)
su(1200)
su(5)
so(10)

[{⟨1, 1⟩},{⟨1199, 1⟩}], [{⟨1, 1⟩}], [(1199)], [{⟨1, 1⟩}], [(3, 0, 2, 0),(0, 2, 0, 3)],[(0, 0, 1, 1, 0),(0, 0, 1, 0, 1)]

---

su(2) ← sp(605)
so(6) ← so(1210) ← su(1210)
su(11)

[{⟨1, 1⟩},{⟨1209, 1⟩}], [{⟨1, 1⟩}], [(1209)], [{⟨1, 1⟩}], [(9, 0, 0)],[{⟨2, 2⟩},{⟨9, 2⟩}]

---

su(2)
so(1215)
su(9)
su(3) ← su(1215)
su(5)

[{⟨1, 1⟩},{⟨1214, 1⟩}], [{⟨1, 1⟩}], [(1214)], [{⟨2, 1⟩, ⟨7, 1⟩}],[(26, 2),(2, 26)],[(2, 1, 0, 2),(2, 0, 1, 2)]

---

su(2) ← sp(612)
su(35) su(1224)
so(49) ← so(1224)
sp(25) su(3)

[{⟨1, 1⟩},{⟨1223, 1⟩}], [{⟨1, 1⟩}], [(1223)], [{⟨1, 1⟩}], [{⟨1, 1⟩, ⟨34, 1⟩}],[{⟨1, 2⟩}],[{⟨2, 1⟩}],[(33, 1),(1, 33)]

su(1225) → so(1225), su(3), su(49), su(50); so(1225) → su(2), so(50)

[{⟨1, 1⟩},{⟨1224, 1⟩}], [{⟨1, 1⟩}], [(1224)], [{⟨2, 1⟩}], [(48, 0),(0, 48)], [{⟨1, 2⟩},{⟨48, 2⟩}], [{⟨2, 1⟩},{⟨48, 1⟩}]

---

su(1232) → sp(616), so(1232), su(3); sp(616) → su(2), sp(4); so(1232) → su(8)

[{⟨1, 1⟩},{⟨1231, 1⟩}],[{⟨1, 1⟩}],[(1231)],[(2, 0, 1, 0)],[{⟨1, 1⟩}],[{⟨1, 2⟩, ⟨7, 2⟩}],[(13, 7),(7, 13)]

---

su(1240) → sp(620), so(1240); sp(620) → su(2); so(1240) → so(5)

[{⟨1, 1⟩},{⟨1239, 1⟩}], [{⟨1, 1⟩}], [(1239)], [{⟨1, 1⟩}], [(14, 0)]

---

su(1242) → sp(621), so(1242), su(3); sp(621) → su(2)

[{⟨1, 1⟩},{⟨1241, 1⟩}], [{⟨1, 1⟩}], [(1241)], [{⟨1, 1⟩}], [(22, 3),(3, 22)]

---

su(1250) → sp(625), so(1250), su(3); sp(625) → su(2)

[{⟨1, 1⟩},{⟨1249, 1⟩}], [{⟨1, 1⟩}], [(1249)], [{⟨1, 1⟩}], [(19, 4),(4, 19)]

---

su(1254) → sp(627), so(1254); sp(627) → su(2); so(1254) → so(7) → g2

[{⟨1, 1⟩},{⟨1253, 1⟩}], [{⟨1, 1⟩}], [(1253)], [{⟨1, 1⟩}], [(7, 0, 0)],[(7, 0)]

---

su(1260) → sp(630), so(1260), su(4), su(4), su(4), su(5), su(6), su(7), su(14); sp(630) → su(2)

[{⟨1, 1⟩},{⟨1259, 1⟩}], [{⟨1, 1⟩}], [(1259)], [{⟨1, 1⟩}], [(3, 2, 2),(2, 2, 3)], [(5, 0, 4),(4, 0, 5)], [(11, 1, 0),(0, 1, 11)], [(2, 3, 0, 0),(0, 0, 3, 2)], [(2, 0, 0, 1, 1),(1, 1, 0, 0, 2)], [{⟨1, 1⟩, ⟨5, 2⟩},{⟨2, 2⟩, ⟨6, 1⟩}], [{⟨1, 1⟩, ⟨12, 1⟩},{⟨2, 1⟩, ⟨13, 1⟩}]

---

su(1274) → sp(637), so(1274); sp(637) → su(2); so(1274) → sp(3), so(50), f4

[{⟨1, 1⟩},{⟨1273, 1⟩}], [{⟨1, 1⟩}], [(1273)], [{⟨1, 1⟩}], [(0, 4, 0)],[{⟨1, 2⟩}],[(0, 1, 0, 0)]

---

su(1275) → so(1275), su(3), su(50), su(51); so(1275) → su(2), so(51), sp(25)

[{⟨1, 1⟩},{⟨1274, 1⟩}], [{⟨1, 1⟩}], [(1274)], [{⟨2, 1⟩}], [{⟨1, 2⟩}], [(49, 0),(0, 49)], [{⟨1, 2⟩},{⟨49, 2⟩}], [{⟨2, 1⟩},{⟨49, 1⟩}]

---

su(1280) → sp(640), so(1280), su(4), su(4), su(8); sp(640) → su(2), sp(2); so(1280) → so(6)

[{⟨1, 1⟩},{⟨1279, 1⟩}], [{⟨1, 1⟩}], [(1279)], [(3, 7)], [{⟨1, 1⟩}], [(5, 1, 1)], [(3, 3, 1),(1, 3, 3)], [(7, 1, 1),(1, 1, 7)],[{⟨1, 1⟩, ⟨2, 1⟩, ⟨7, 1⟩},{⟨1, 1⟩, ⟨6, 1⟩, ⟨7, 1⟩}]

---

su(1287) → so(1287), su(3), su(6), su(9), su(13); so(1287) → su(2), so(13), sp(3), so(12)

[{⟨1, 1⟩},{⟨1286, 1⟩}], [{⟨1, 1⟩}], [(1286)], [{⟨5, 1⟩}], [(8, 0, 0)], [{⟨1, 4⟩}], [(12, 8),(8, 12)], [(8, 0, 0, 0, 0),(0, 0, 0, 0, 8)],[{⟨1, 5⟩},{⟨8, 5⟩}],[{⟨5, 1⟩},{⟨8, 1⟩}]

---

su(1288) → sp(644), so(1288), su(3); sp(644) → su(2)

[{⟨1, 1⟩},{⟨1287, 1⟩}], [{⟨1, 1⟩}], [(1287)], [{⟨1, 1⟩}], [(15, 6),(6, 15)]

---

su(1295) → so(1295), su(3); so(1295) → su(2), su(36)

[{⟨1, 1⟩},{⟨1294, 1⟩}], [{⟨1, 1⟩}], [(1294)], [{⟨1, 1⟩, ⟨35, 1⟩}],[(34, 1),(1, 34)]

---

su(1296) → sp(648), so(1296), su(3); sp(648) → su(2), sp(2); so(1296) → so(8)

[{⟨1, 1⟩},{⟨1295, 1⟩}], [{⟨1, 1⟩}], [(1295)], [(5, 5)], [{⟨1, 1⟩}], [(2, 0, 1, 1),(1, 0, 2, 1),(1, 0, 1, 2)], [(17, 5),(5, 17)]

---

su(1302) → sp(651), so(1302), su(3); sp(651) → su(2)

[{⟨1, 1⟩},{⟨1301, 1⟩}], [{⟨1, 1⟩}], [(1301)], [{⟨1, 1⟩}], [(27, 2),(2, 27)]

---

su(1309) → so(1309) → su(2), so(5)

[{⟨1, 1⟩},{⟨1308, 1⟩}],[{⟨1, 1⟩}],[(1308)],[(2, 10)]

---

su(1311) → so(1311) → su(2), so(19)

[{⟨1, 1⟩},{⟨1310, 1⟩}],[{⟨1, 1⟩}],[(1310)],[{⟨1, 3⟩}]

---

su(1320) → sp(660), so(1320), su(3), su(4), su(4); sp(660) → su(2)

[{⟨1, 1⟩},{⟨1319, 1⟩}], [{⟨1, 1⟩}], [(1319)], [{⟨1, 1⟩}], [(11, 9),(9, 11)],[(1, 7, 0),(0, 7, 1)],[(5, 1, 2),(2, 1, 5)]

---

su(1323) → so(1323), su(7); so(1323) → su(2)

[{⟨1, 1⟩},{⟨1322, 1⟩}], [{⟨1, 1⟩}], [(1322)], [{⟨1, 1⟩, ⟨3, 1⟩, ⟨6, 1⟩},{⟨1, 1⟩, ⟨4, 1⟩, ⟨6, 1⟩}]

---

su(1325) → so(1325) → su(2), so(51), sp(26)

[{⟨1, 1⟩},{⟨1324, 1⟩}], [{⟨1, 1⟩}], [(1324)], [{⟨1, 2⟩}], [{⟨2, 1⟩}]

---

su(1326) → sp(663), so(1326), su(3), su(51), su(52); sp(663) → su(2); so(1326) → so(5), so(52)

[{⟨1, 1⟩},{⟨1325, 1⟩}], [{⟨1, 1⟩}], [(1325)], [{⟨1, 1⟩}], [(3, 8)],[{⟨2, 1⟩}],[(50, 0),(0, 50)],[{⟨1, 2⟩},{⟨50, 2⟩}],[{⟨2, 1⟩},{⟨50, 1⟩}]

---

su(1330) → sp(665), so(1330), su(4), su(19), su(21); sp(665) → su(2); so(1330) → so(5), so(5), so(21)

[{⟨1, 1⟩},{⟨1329, 1⟩}], [{⟨1, 1⟩}], [(1329)], [{⟨1, 1⟩}], [(0, 18)], [(6, 4)], [{⟨3, 1⟩}], [(18, 0, 0),(0, 0, 18)], [{⟨1, 3⟩},{⟨18, 3⟩}],[{⟨3, 1⟩},{⟨18, 1⟩}]

---

su(1331) → so(1331) → su(2), su(3)

[{⟨1, 1⟩},{⟨1330, 1⟩}],[{⟨1, 1⟩}],[(1330)],[(10, 10)]

---

su(1344) → sp(672), so(1344), su(3), su(8); sp(672) → su(2), sp(2), sp(3), sp(8); so(1344) → so(16)

[{⟨1, 1⟩},{⟨1343, 1⟩}],[{⟨1, 1⟩}],[(1343)],[(13, 1)],[(1, 3, 0)],[{⟨1, 1⟩, ⟨2, 1⟩}],[{⟨1, 1⟩}],[{⟨1, 1⟩, ⟨2, 1⟩}],[(23, 3),(3, 23)],[{⟨2, 1⟩, ⟨5, 1⟩},{⟨3, 1⟩, ⟨6, 1⟩}]

---

su(1360) → sp(680), so(1360), su(16); sp(680) → su(2)

[{⟨1, 1⟩},{⟨1359, 1⟩}], [{⟨1, 1⟩}], [(1359)], [{⟨1, 1⟩}], [{⟨1, 1⟩, ⟨2, 1⟩},{⟨14, 1⟩, ⟨15, 1⟩}]

---

su(1365) → so(1365), su(3), su(5), su(12), su(15); so(1365) → su(2), so(15), sp(6)

[{⟨1, 1⟩},{⟨1364, 1⟩}], [{⟨1, 1⟩}], [(1364)], [{⟨4, 1⟩}], [{⟨1, 4⟩}], [(20, 4),(4, 20)], [(11, 0, 0, 0),(0, 0, 0, 11)], [{⟨1, 4⟩},{⟨11, 4⟩}],[{⟨4, 1⟩},{⟨11, 1⟩}]

---

su(1368) → sp(684), so(1368), su(3); sp(684) → su(2); so(1368) → su(37)

[{⟨1, 1⟩},{⟨1367, 1⟩}], [{⟨1, 1⟩}], [(1367)], [{⟨1, 1⟩}], [{⟨1, 1⟩, ⟨36, 1⟩}],[(35, 1),(1, 35)]

---

su(1375) → so(1375), su(4); so(1375) → su(2)

[{⟨1, 1⟩},{⟨1374, 1⟩}], [{⟨1, 1⟩}], [(1374)], [(4, 4, 0),(0, 4, 4)]

---

su(1377) → so(1377) → su(2), so(52)

[{⟨1, 1⟩},{⟨1376, 1⟩}],[{⟨1, 1⟩}],[(1376)],[{⟨1, 2⟩}]

su(2) ← sp(689) ← su(1378)
so(53), sp(26) ← so(1378) ← su(1378)
su(3), su(52), su(53) ← su(1378)

[{⟨1, 1⟩},{⟨1377, 1⟩}], [{⟨1, 1⟩}], [(1377)], [{⟨1, 1⟩}], [{⟨2, 1⟩}], [{⟨1, 2⟩}], [(51, 0),(0, 51)], [{⟨1, 2⟩},{⟨51, 2⟩}],[{⟨2, 1⟩},{⟨51, 1⟩}]

---

su(2) ← sp(690) ← su(1380)
so(1380) ← su(1380)
su(3) ← su(1380)

[{⟨1, 1⟩},{⟨1379, 1⟩}], [{⟨1, 1⟩}], [(1379)], [{⟨1, 1⟩}], [(14, 7),(7, 14)]

---

su(2), sp(3) ← sp(693) ← su(1386)
so(7), sp(3), so(8) ← so(7), so(10) ← so(1386) ← su(1386)
su(6), su(7) ← su(1386)

[{⟨1, 1⟩},{⟨1385, 1⟩}], [{⟨1, 1⟩}], [(1385)], [(2, 1, 1)], [{⟨1, 1⟩}], [(1, 0, 4)], [(1, 0, 3)], [(6, 0, 0, 0),(0, 0, 6, 0),(0, 0, 0, 6)], [(0, 0, 6)], [(2, 1, 0, 0, 0)], [(5, 0, 0, 0, 1),(1, 0, 0, 0, 5)],[{⟨1, 4⟩, ⟨6, 1⟩},{⟨1, 1⟩, ⟨6, 4⟩}]

---

su(2) ← sp(696) ← su(1392)
so(1392) ← su(1392)
su(3) ← su(1392)

[{⟨1, 1⟩},{⟨1391, 1⟩}], [{⟨1, 1⟩}], [(1391)], [{⟨1, 1⟩}], [(28, 2),(2, 28)]

---

su(2) ← sp(700) ← su(1400)
so(8) ← so(1400) ← su(1400)
su(4) ← su(1400)

[{⟨1, 1⟩},{⟨1399, 1⟩}], [{⟨1, 1⟩}], [(1399)], [{⟨1, 1⟩}], [(1, 2, 0, 0),(0, 2, 1, 0),(0, 2, 0, 1)],[(2, 4, 1),(1, 4, 2)]

---

su(2) ← sp(702) ← su(1404)
so(1404) ← su(1404)
su(4) ← su(1404)

[{⟨1, 1⟩},{⟨1403, 1⟩}], [{⟨1, 1⟩}], [(1403)], [{⟨1, 1⟩}], [(8, 2, 0),(0, 2, 8)]

---

su(2), so(11) ← sp(704) ← su(1408)
so(11), sp(5) ← so(1408) ← su(1408)

[{⟨1, 1⟩},{⟨1407, 1⟩}], [{⟨1, 1⟩}], [(1407)], [(0, 1, 0, 0, 1)],[(1, 0, 0, 1, 0)],[{⟨1, 1⟩}]

---

su(2) ← so(1425) ← su(1425)
su(3) ← su(1425)

[{⟨1, 1⟩},{⟨1424, 1⟩}], [{⟨1, 1⟩}], [(1424)], [(18, 5),(5, 18)]

---

su(2) ← sp(714) ← su(1428)
so(1428) ← su(1428)
su(3) ← su(1428)

[{⟨1, 1⟩},{⟨1427, 1⟩}], [{⟨1, 1⟩}], [(1427)], [{⟨1, 1⟩}], [(16, 6),(6, 16)]

---

su(2), sp(7) ← sp(715) ← su(1430)
so(11), so(53), sp(5), sp(27) ← so(1430) ← su(1430)

[{⟨1, 1⟩},{⟨1429, 1⟩}], [{⟨1, 1⟩}], [(1429)], [{⟨7, 1⟩}], [{⟨1, 1⟩}], [(1, 0, 1, 0, 0)], [{⟨1, 2⟩}], [(2, 1, 0, 0, 0)], [{⟨2, 1⟩}]

---

su(2), so(54) ← so(1431) ← su(1431)
su(3), su(53), su(54) ← su(1431)

[{⟨1, 1⟩},{⟨1430, 1⟩}], [{⟨1, 1⟩}], [(1430)], [{⟨2, 1⟩}], [(52, 0),(0, 52)], [{⟨1, 2⟩},{⟨52, 2⟩}], [{⟨2, 1⟩},{⟨52, 1⟩}]

---

su(2) ← sp(720) ← su(1440)
so(1440) ← su(1440)
su(5), su(5), su(9), so(10) ← su(1440)

[{⟨1, 1⟩},{⟨1439, 1⟩}], [{⟨1, 1⟩}], [(1439)], [{⟨1, 1⟩}], [(3, 1, 1, 0),(0, 1, 1, 3)],[(7, 0, 0, 1),(1, 0, 0, 7)],[{⟨1, 3⟩, ⟨8, 1⟩},{⟨1, 1⟩, ⟨8, 3⟩}],[(0, 0, 0, 2, 1),(0, 0, 0, 1, 2)]

---

su(2), su(38) ← so(1443) ← su(1443)
su(3) ← su(1443)

[{⟨1, 1⟩},{⟨1442, 1⟩}], [{⟨1, 1⟩}], [(1442)], [{⟨1, 1⟩, ⟨37, 1⟩}],[(36, 1),(1, 36)]

---

su(2) ← so(1449) ← su(1449)
su(3) ← su(1449)

[{⟨1, 1⟩},{⟨1448, 1⟩}], [{⟨1, 1⟩}], [(1448)], [(13, 8),(8, 13)]

---

su(2) ← sp(725) ← su(1450)
so(1450) ← su(1450)
su(3) ← su(1450)

[{⟨1, 1⟩},{⟨1449, 1⟩}], [{⟨1, 1⟩}], [(1449)], [{⟨1, 1⟩}], [(24, 3),(3, 24)]

---

su(2), sp(2) ← sp(728) ← su(1456)
so(1456) ← su(1456)
su(4), su(14) ← su(1456)

[{⟨1, 1⟩},{⟨1455, 1⟩}], [{⟨1, 1⟩}], [(1455)], [(1, 11)], [{⟨1, 1⟩}], [(12, 0, 1),(1, 0, 12)], [{⟨1, 2⟩, ⟨13, 1⟩},{⟨1, 1⟩, ⟨13, 2⟩}]

---

su(2), $\mathfrak{e}_7$ ← so(1463) ← su(1463)

[{⟨1, 1⟩},{⟨1462, 1⟩}],[{⟨1, 1⟩}],[(1462)],[{⟨7, 2⟩}]

---

su(2) ← sp(735) ← su(1470)
so(6) ← so(1470) ← su(1470)
su(5), su(6) ← su(1470)

[{⟨1, 1⟩},{⟨1469, 1⟩}], [{⟨1, 1⟩}], [(1469)], [{⟨1, 1⟩}], [(3, 2, 2)],[(1, 4, 0, 0),(0, 0, 4, 1)],[(0, 1, 2, 0, 0),(0, 0, 2, 1, 0)]

---

su(2) ← sp(742) ← su(1484)
so(54) ← so(1484) ← su(1484)

[{⟨1, 1⟩},{⟨1483, 1⟩}], [{⟨1, 1⟩}], [(1483)], [{⟨1, 1⟩}], [{⟨1, 2⟩}]

---

su(2), so(55), sp(27) ← so(1485) ← su(1485)
su(3), su(3), su(3), su(4), su(54) ← su(1485)
su(10), su(11) ← su(55) ← su(1485)

[{⟨1, 1⟩},{⟨1484, 1⟩}], [{⟨1, 1⟩}], [(1484)], [{⟨2, 1⟩}], [{⟨1, 2⟩}], [(21, 4),(4, 21)], [(29, 2),(2, 29)], [(53, 0),(0, 53)], [(5, 2, 1),(1, 2, 5)], [{⟨1, 2⟩},{⟨53, 2⟩}], [{⟨2, 1⟩},{⟨53, 1⟩}], [{⟨1, 2⟩, ⟨2, 1⟩},{⟨8, 1⟩, ⟨9, 2⟩}], [{⟨1, 1⟩, ⟨3, 1⟩},{⟨8, 1⟩, ⟨10, 1⟩}]

---

su(2), so(5) ← so(1495) ← su(1495)
su(3) ← su(1495)

[{⟨1, 1⟩},{⟨1494, 1⟩}],[{⟨1, 1⟩}],[(1494)],[(9, 2)],[(12, 9),(9, 12)]

---

su(2) ← sp(748) ← su(1496)
so(5) ← so(1496) ← su(1496)

[{⟨1, 1⟩},{⟨1495, 1⟩}], [{⟨1, 1⟩}], [(1495)], [{⟨1, 1⟩}], [(15, 0)]

---

su(2) ← sp(750) ← su(1500)
so(1500) ← su(1500)
su(5) ← su(1500)

[{⟨1, 1⟩},{⟨1499, 1⟩}], [{⟨1, 1⟩}], [(1499)], [{⟨1, 1⟩}], [(4, 2, 0, 0),(0, 0, 2, 4)]

---

su(2), sp(4) ← sp(756) ← su(1512)
so(7) ← so(1512) ← su(1512)
su(8), su(8) ← su(1512)

[{⟨1, 1⟩},{⟨1511, 1⟩}],[{⟨1, 1⟩}],[(1511)],[(1, 2, 0, 0)], [{⟨1, 1⟩}], [(2, 1, 1)], [{⟨2, 1⟩, ⟨4, 1⟩},{⟨4, 1⟩, ⟨6, 1⟩}], [{⟨1, 2⟩, ⟨3, 1⟩},{⟨5, 1⟩, ⟨7, 2⟩}]

---

su(2), sp(11) ← sp(759) ← su(1518)
so(1518) ← su(1518)
su(3) ← su(1518)

[{⟨1, 1⟩},{⟨1517, 1⟩}], [{⟨1, 1⟩}], [(1517)], [{⟨3, 1⟩}], [{⟨1, 1⟩}],[(11, 10),(10, 11)]

---

su(2) ← sp(760) ← su(1520)
su(39), so(20) ← so(1520) ← su(1520)
su(3) ← su(1520)

[{⟨1, 1⟩},{⟨1519, 1⟩}], [{⟨1, 1⟩}], [(1519)], [{⟨1, 1⟩}], [{⟨1, 1⟩, ⟨38, 1⟩}],[{⟨1, 3⟩}],[(37, 1),(1, 37)]

---

su(2) ← sp(768) ← su(1536)
so(1536) ← su(1536)
su(3) ← su(1536)

[{⟨1, 1⟩},{⟨1535, 1⟩}], [{⟨1, 1⟩}], [(1535)], [{⟨1, 1⟩}], [(15, 7),(7, 15)]

---

su(2), so(55) ← so(1539) ← su(1539)
$\mathfrak{e}_7$ ← sp(28) ← so(1539)

[{⟨1, 1⟩},{⟨1538, 1⟩}], [{⟨1, 1⟩}], [(1538)], [{⟨1, 2⟩}], [{⟨2, 1⟩}],[{⟨6, 1⟩}]

su(1540) ← sp(770) ← su(2), sp(2), sp(10); su(1540) ← so(1540) ← so(22), so(56); su(1540) ← su(3), su(4), su(4), su(4), su(4), su(4), su(4), su(5), su(5), su(9), su(20), su(22), su(55), su(56)

[{⟨1, 1⟩},{⟨1539, 1⟩}], [{⟨1, 1⟩}], [(1539)], [(19, 0)], [{⟨1, 3⟩}], [{⟨1, 1⟩}], [{⟨3, 1⟩}], [{⟨2, 1⟩}], [(54, 0),(0, 54)], [(2, 6, 0),(0, 6, 2)], [(3, 5, 0),(0, 5, 3)], [(4, 1, 3),(3, 1, 4)], [(6, 3, 0),(0, 3, 6)], [(9, 0, 2),(2, 0, 9)], [(19, 0, 0),(0, 0, 19)], [(5, 0, 0, 2),(2, 0, 0, 5)], [(6, 0, 1, 0),(0, 1, 0, 6)], [{⟨1, 2⟩, ⟨7, 1⟩},{⟨2, 1⟩, ⟨8, 2⟩}], [{⟨1, 3⟩},{⟨19, 3⟩}], [{⟨3, 1⟩},{⟨19, 1⟩}], [{⟨1, 2⟩},{⟨54, 2⟩}], [{⟨2, 1⟩},{⟨54, 1⟩}]

---

su(1547) ← so(1547) ← su(2), $\mathfrak{g}_2$

[{⟨1, 1⟩},{⟨1546, 1⟩}],[{⟨1, 1⟩}],[(1546)],[(3, 2)]

---

su(1560) ← sp(780) ← su(2), sp(2); su(1560) ← so(1560) ← so(7); su(1560) ← su(3), su(3), su(4), su(4), su(15)

[{⟨1, 1⟩},{⟨1559, 1⟩}], [{⟨1, 1⟩}], [(1559)], [(7, 4)], [{⟨1, 1⟩}], [(3, 0, 2)], [(19, 5),(5, 19)], [(25, 3),(3, 25)], [(7, 0, 3),(3, 0, 7)], [(12, 1, 0),(0, 1, 12)], [{⟨1, 1⟩, ⟨13, 1⟩},{⟨2, 1⟩, ⟨14, 1⟩}]

---

su(1568) ← sp(784) ← su(2); su(1568) ← so(1568) ← so(8)

[{⟨1, 1⟩},{⟨1567, 1⟩}], [{⟨1, 1⟩}], [(1567)], [{⟨1, 1⟩}], [(3, 1, 0, 0),(0, 1, 3, 0),(0, 1, 0, 3)]

---

su(1575) ← so(1575) ← su(2); su(1575) ← su(3), su(6), su(7)

[{⟨1, 1⟩},{⟨1574, 1⟩}], [{⟨1, 1⟩}], [(1574)], [(17, 6),(6, 17)], [(4, 0, 0, 1, 0),(0, 1, 0, 0, 4)], [{⟨1, 3⟩, ⟨5, 1⟩},{⟨2, 1⟩, ⟨6, 3⟩}]

---

su(1581) ← so(1581) ← su(2); su(1581) ← su(3)

[{⟨1, 1⟩},{⟨1580, 1⟩}], [{⟨1, 1⟩}], [(1580)], [(30, 2),(2, 30)]

---

su(1595) ← so(1595) ← su(2), so(56)

[{⟨1, 1⟩},{⟨1594, 1⟩}],[{⟨1, 1⟩}],[(1594)],[{⟨1, 2⟩}]

---

su(1596) ← sp(798) ← su(2); su(1596) ← so(1596) ← so(57), sp(28); su(1596) ← su(3), su(56), su(57)

[{⟨1, 1⟩},{⟨1595, 1⟩}], [{⟨1, 1⟩}], [(1595)], [{⟨1, 1⟩}], [{⟨2, 1⟩}], [{⟨1, 2⟩}], [(55, 0),(0, 55)], [{⟨1, 2⟩},{⟨55, 2⟩}],[{⟨2, 1⟩},{⟨55, 1⟩}]

---

su(1599) ← so(1599) ← su(2), su(40); su(1599) ← su(3)

[{⟨1, 1⟩},{⟨1598, 1⟩}], [{⟨1, 1⟩}], [(1598)], [{⟨1, 1⟩, ⟨39, 1⟩}],[(38, 1),(1, 38)]

---

su(1610) ← sp(805) ← su(2); su(1610) ← so(1610); su(1610) ← su(3)

[{⟨1, 1⟩},{⟨1609, 1⟩}], [{⟨1, 1⟩}], [(1609)], [{⟨1, 1⟩}], [(22, 4),(4, 22)]

---

su(1615) ← so(1615) ← su(2), so(5), so(17)

[{⟨1, 1⟩},{⟨1614, 1⟩}], [{⟨1, 1⟩}], [(1614)], [(1, 14)], [{⟨1, 1⟩, ⟨2, 1⟩}]

---

su(1617) ← so(1617) ← su(2), so(7)

[{⟨1, 1⟩},{⟨1616, 1⟩}],[{⟨1, 1⟩}],[(1616)],[(1, 1, 2)]

---

su(1620) ← sp(810) ← su(2), sp(2); su(1620) ← so(1620); su(1620) ← su(3)

[{⟨1, 1⟩},{⟨1619, 1⟩}], [{⟨1, 1⟩}], [(1619)], [(11, 2)], [{⟨1, 1⟩}],[(14, 8),(8, 14)]

---

su(1632) ← sp(816) ← su(2); su(1632) ← so(1632); su(1632) ← su(17)

[{⟨1, 1⟩},{⟨1631, 1⟩}], [{⟨1, 1⟩}], [(1631)], [{⟨1, 1⟩}], [{⟨1, 1⟩, ⟨2, 1⟩},{⟨15, 1⟩, ⟨16, 1⟩}]

---

su(1638) ← sp(819) ← su(2), sp(7); su(1638) ← so(1638) ← so(12)

[{⟨1, 1⟩},{⟨1637, 1⟩}], [{⟨1, 1⟩}], [(1637)], [{⟨5, 1⟩}], [{⟨1, 1⟩}],[{⟨2, 2⟩}]

---

su(1650) ← sp(825) ← su(2); su(1650) ← so(1650) ← so(9), sp(6)

[{⟨1, 1⟩},{⟨1649, 1⟩}], [{⟨1, 1⟩}], [(1649)], [{⟨1, 1⟩}], [(0, 1, 1, 0)],[{⟨2, 2⟩}]

---

su(1652) ← sp(826) ← su(2); su(1652) ← so(1652) ← so(57), sp(29)

[{⟨1, 1⟩},{⟨1651, 1⟩}], [{⟨1, 1⟩}], [(1651)], [{⟨1, 1⟩}], [{⟨1, 2⟩}],[{⟨2, 1⟩}]

---

su(1653) ← so(1653) ← su(2), so(58); su(1653) ← su(3), su(57), su(58)

[{⟨1, 1⟩},{⟨1652, 1⟩}], [{⟨1, 1⟩}], [(1652)], [{⟨2, 1⟩}], [(56, 0),(0, 56)], [{⟨1, 2⟩},{⟨56, 2⟩}], [{⟨2, 1⟩},{⟨56, 1⟩}]

---

su(1674) ← sp(837) ← su(2); su(1674) ← so(1674); su(1674) ← su(3)

[{⟨1, 1⟩},{⟨1673, 1⟩}], [{⟨1, 1⟩}], [(1673)], [{⟨1, 1⟩}], [(26, 3),(3, 26)]

---

su(1680) ← sp(840) ← su(2), sp(2); su(1680) ← so(1680) ← su(41), so(8); su(1680) ← su(3), su(3), su(3), su(8)

[{⟨1, 1⟩},{⟨1679, 1⟩}], [{⟨1, 1⟩}], [(1679)], [(9, 3)], [{⟨1, 1⟩}], [{⟨1, 1⟩, ⟨40, 1⟩}], [(4, 0, 1, 0),(4, 0, 0, 1),(1, 0, 4, 0),(1, 0, 0, 4),(0, 0, 4, 1),(0, 0, 1, 4)], [(13, 9),(9, 13)], [(31, 2),(2, 31)], [(39, 1),(1, 39)], [{⟨1, 1⟩, ⟨2, 2⟩},{⟨6, 2⟩, ⟨7, 1⟩}]

---

su(1700) ← sp(850) ← su(2); su(1700) ← so(1700) ← sp(8); su(1700) ← su(3)

[{⟨1, 1⟩},{⟨1699, 1⟩}], [{⟨1, 1⟩}], [(1699)], [{⟨1, 1⟩}], [{⟨4, 1⟩}],[(16, 7),(7, 16)]

---

su(1701) ← so(1701) ← su(2); su(1701) ← su(3), su(5), su(6)

[{⟨1, 1⟩},{⟨1700, 1⟩}], [{⟨1, 1⟩}], [(1700)], [(20, 5),(5, 20)], [(2, 2, 0, 1),(1, 0, 2, 2)], [(2, 0, 1, 0, 1),(1, 0, 1, 0, 2)]

---

su(1710) ← sp(855) ← su(2); su(1710) ← so(1710) ← so(58)

[{⟨1, 1⟩},{⟨1709, 1⟩}], [{⟨1, 1⟩}], [(1709)], [{⟨1, 1⟩}], [{⟨1, 2⟩}]

---

su(1711) ← so(1711) ← su(2), so(59), sp(29); su(1711) ← su(3), su(58), su(59)

[{⟨1, 1⟩},{⟨1710, 1⟩}], [{⟨1, 1⟩}], [(1710)], [{⟨2, 1⟩}], [{⟨1, 2⟩}], [(57, 0),(0, 57)], [{⟨1, 2⟩},{⟨57, 2⟩}], [{⟨2, 1⟩},{⟨57, 1⟩}]

---

su(1716) ← sp(858) ← su(2), sp(2); su(1716) ← so(1716) ← so(13), sp(4), so(6); su(1716) ← su(3), su(4), su(7), su(8), su(12), su(13), so(14)

[{⟨1, 1⟩},{⟨1715, 1⟩}], [{⟨1, 1⟩}], [(1715)], [(3, 8)], [{⟨1, 1⟩}], [{⟨6, 2⟩}], [(6, 0, 0, 0)], [(10, 0, 0)], [(12, 10),(10, 12)], [(8, 1, 1),(1, 1, 8)], [{⟨1, 7⟩},{⟨6, 7⟩}], [{⟨1, 6⟩},{⟨7, 6⟩}], [{⟨2, 2⟩},{⟨10, 2⟩}], [{⟨6, 1⟩},{⟨7, 1⟩}],[{⟨6, 2⟩},{⟨7, 2⟩}]

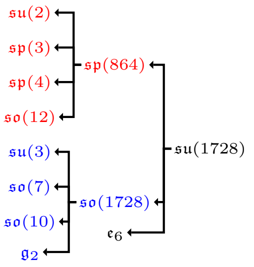


[{⟨1, 1⟩},{⟨1727, 1⟩}], [{⟨1, 1⟩}], [(1727)], [(5, 1, 0)], [(3, 1, 0, 0)], [{⟨2, 1⟩, ⟨5, 1⟩},{⟨2, 1⟩, ⟨6, 1⟩}], [{⟨1, 1⟩}], [(11, 11)], [(2, 0, 3)], [(1, 0, 0, 1, 1)], [(5, 1)], [{⟨1, 1⟩, ⟨2, 1⟩},{⟨2, 1⟩, ⟨6, 1⟩}]

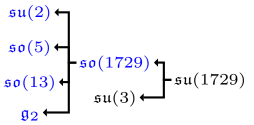


[{⟨1, 1⟩},{⟨1728, 1⟩}], [{⟨1, 1⟩}], [(1728)], [(5, 6)], [{⟨1, 4⟩}],[(0, 5)],[(18, 6),(6, 18)]

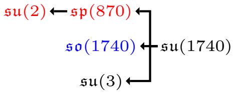


[{⟨1, 1⟩},{⟨1739, 1⟩}], [{⟨1, 1⟩}], [(1739)], [{⟨1, 1⟩}], [(23, 4),(4, 23)]

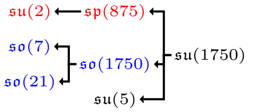


[{⟨1, 1⟩},{⟨1749, 1⟩}], [{⟨1, 1⟩}], [(1749)], [{⟨1, 1⟩}], [(4, 1, 0)],[{⟨1, 3⟩}],[(4, 1, 0, 1),(1, 0, 1, 4)]

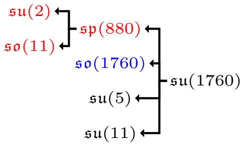


[{⟨1, 1⟩},{⟨1759, 1⟩}], [{⟨1, 1⟩}], [(1759)], [(2, 0, 0, 0, 1)], [{⟨1, 1⟩}], [(7, 1, 0, 0),(0, 0, 1, 7)], [{⟨1, 1⟩, ⟨8, 1⟩},{⟨3, 1⟩, ⟨10, 1⟩}]

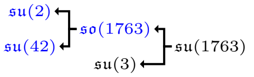


[{⟨1, 1⟩},{⟨1762, 1⟩}], [{⟨1, 1⟩}], [(1762)], [{⟨1, 1⟩, ⟨41, 1⟩}],[(40, 1),(1, 40)]

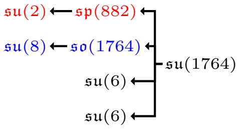


[{⟨1, 1⟩},{⟨1763, 1⟩}], [{⟨1, 1⟩}], [(1763)], [{⟨1, 1⟩}], [{⟨4, 2⟩}], [(0, 4, 0, 0, 0),(0, 0, 0, 4, 0)], [(1, 3, 0, 0, 0),(0, 0, 0, 3, 1)]

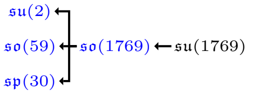


[{⟨1, 1⟩},{⟨1768, 1⟩}], [{⟨1, 1⟩}], [(1768)], [{⟨1, 2⟩}], [{⟨2, 1⟩}]

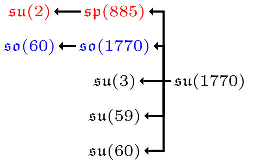


[{⟨1, 1⟩},{⟨1769, 1⟩}], [{⟨1, 1⟩}], [(1769)], [{⟨1, 1⟩}], [{⟨2, 1⟩}], [(58, 0),(0, 58)], [{⟨1, 2⟩},{⟨58, 2⟩}], [{⟨2, 1⟩},{⟨58, 1⟩}]

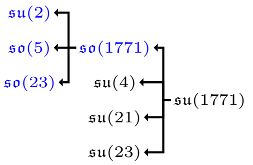


[{⟨1, 1⟩},{⟨1770, 1⟩}], [{⟨1, 1⟩}], [(1770)], [(0, 20)], [{⟨3, 1⟩}], [(20, 0, 0),(0, 0, 20)], [{⟨1, 3⟩},{⟨20, 3⟩}], [{⟨3, 1⟩},{⟨20, 1⟩}]

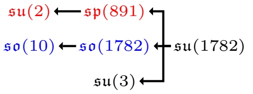


[{⟨1, 1⟩},{⟨1781, 1⟩}], [{⟨1, 1⟩}], [(1781)], [{⟨1, 1⟩}], [(5, 0, 0, 0, 0)],[(32, 2),(2, 32)]

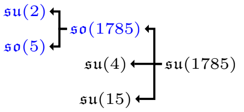


[{⟨1, 1⟩},{⟨1784, 1⟩}], [{⟨1, 1⟩}], [(1784)], [(16, 0)], [(13, 0, 1),(1, 0, 13)], [{⟨1, 2⟩, ⟨14, 1⟩},{⟨1, 1⟩, ⟨14, 2⟩}]

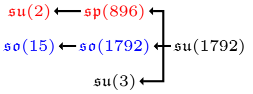


[{⟨1, 1⟩},{⟨1791, 1⟩}], [{⟨1, 1⟩}], [(1791)], [{⟨1, 1⟩}], [{⟨1, 1⟩, ⟨7, 1⟩}],[(27, 3),(3, 27)]

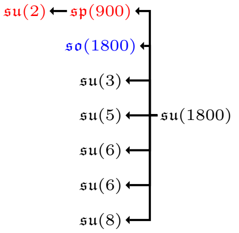


[{⟨1, 1⟩},{⟨1799, 1⟩}], [{⟨1, 1⟩}], [(1799)], [{⟨1, 1⟩}], [(15, 8),(8, 15)], [(2, 0, 3, 0),(0, 3, 0, 2)], [(2, 0, 0, 2, 0),(0, 2, 0, 0, 2)], [(4, 0, 1, 0, 0),(0, 0, 1, 0, 4)], [{⟨1, 2⟩, ⟨5, 1⟩},{⟨3, 1⟩, ⟨7, 2⟩}]

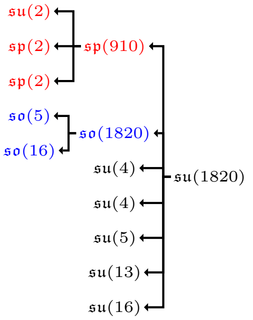


[{⟨1, 1⟩},{⟨1819, 1⟩}],[{⟨1, 1⟩}],[(1819)],[(1, 12)],[(5, 6)],[{⟨1, 1⟩}],[(7, 4)],[{⟨4, 1⟩}],[(6, 0, 4),(4, 0, 6)],[(9, 2, 0),(0, 2, 9)], [(12, 0, 0, 0),(0, 0, 0, 12)], [{⟨1, 4⟩},{⟨12, 4⟩}],[{⟨4, 1⟩},{⟨12, 1⟩}]

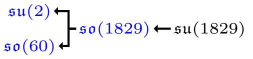


[{⟨1, 1⟩},{⟨1828, 1⟩}],[{⟨1, 1⟩}],[(1828)],[{⟨1, 2⟩}]

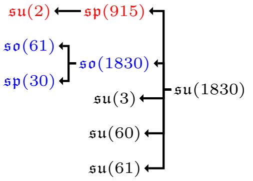


[{⟨1, 1⟩},{⟨1829, 1⟩}], [{⟨1, 1⟩}], [(1829)], [{⟨1, 1⟩}], [{⟨2, 1⟩}], [{⟨1, 2⟩}], [(59, 0),(0, 59)], [{⟨1, 2⟩},{⟨59, 2⟩}],[{⟨2, 1⟩},{⟨59, 1⟩}]

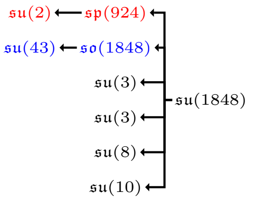


[{⟨1, 1⟩},{⟨1847, 1⟩}], [{⟨1, 1⟩}], [(1847)], [{⟨1, 1⟩}], [{⟨1, 1⟩, ⟨42, 1⟩}], [(21, 5),(5, 21)], [(41, 1),(1, 41)], [{⟨1, 3⟩, ⟨2, 1⟩},{⟨6, 1⟩, ⟨7, 3⟩}], [{⟨1, 1⟩, ⟨4, 1⟩},{⟨6, 1⟩, ⟨9, 1⟩}]

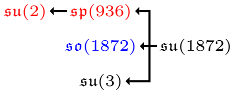


[{⟨1, 1⟩},{⟨1871, 1⟩}], [{⟨1, 1⟩}], [(1871)], [{⟨1, 1⟩}], [(17, 7),(7, 17)]

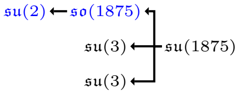


[{⟨1, 1⟩},{⟨1874, 1⟩}], [{⟨1, 1⟩}], [(1874)], [(14, 9),(9, 14)],[(24, 4),(4, 24)]

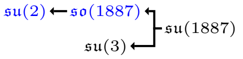


[{⟨1, 1⟩},{⟨1886, 1⟩}], [{⟨1, 1⟩}], [(1886)], [(33, 2),(2, 33)]

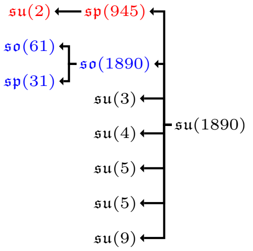


[{⟨1, 1⟩},{⟨1889, 1⟩}], [{⟨1, 1⟩}], [(1889)], [{⟨1, 1⟩}], [{⟨1, 2⟩}], [{⟨2, 1⟩}], [(19, 6),(6, 19)], [(6, 1, 2),(2, 1, 6)], [(1, 0, 4, 0),(0, 4, 0, 1)], [(2, 0, 2, 1),(1, 2, 0, 2)], [{⟨2, 1⟩, ⟨3, 1⟩},{⟨6, 1⟩, ⟨7, 1⟩}]

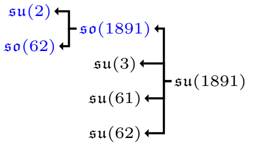


[{⟨1, 1⟩},{⟨1890, 1⟩}], [{⟨1, 1⟩}], [(1890)], [{⟨2, 1⟩}], [(60, 0),(0, 60)], [{⟨1, 2⟩},{⟨60, 2⟩}], [{⟨2, 1⟩},{⟨60, 1⟩}]

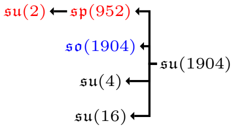


[{⟨1, 1⟩},{⟨1903, 1⟩}], [{⟨1, 1⟩}], [(1903)], [{⟨1, 1⟩}], [(13, 1, 0),(0, 1, 13)], [{⟨1, 1⟩, ⟨14, 1⟩},{⟨2, 1⟩, ⟨15, 1⟩}]

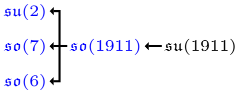


[{⟨1, 1⟩},{⟨1910, 1⟩}], [{⟨1, 1⟩}], [(1910)], [(2, 2, 0)], [(0, 5, 5)]

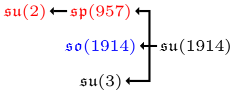


[{⟨1, 1⟩},{⟨1913, 1⟩}], [{⟨1, 1⟩}], [(1913)], [{⟨1, 1⟩}], [(28, 3),(3, 28)]

- su(1920)
  - sp(960): su(2), sp(2), sp(9)
  - so(1920): so(9), so(16), so(18)

[{⟨1, 1⟩},{⟨1919, 1⟩}], [{⟨1, 1⟩}], [(1919)], [(15, 1)], [{⟨1, 1⟩, ⟨2, 1⟩}], [{⟨1, 1⟩}], [(3, 0, 0, 1)], [{⟨1, 1⟩, ⟨7, 1⟩},{⟨1, 1⟩, ⟨8, 1⟩}],[{⟨1, 1⟩, ⟨2, 1⟩}]

- su(1925)
  - so(1925): su(2), su(10), so(5), so(8)
  - su(3)
  - su(5)

[{⟨1, 1⟩},{⟨1924, 1⟩}], [{⟨1, 1⟩}], [(1924)], [{⟨2, 1⟩, ⟨8, 1⟩}], [(10, 2)], [(0, 3, 0, 0)], [(13, 10),(10, 13)], [(4, 0, 0, 3),(3, 0, 0, 4)]

- su(1935)
  - so(1935): su(2), su(44)
  - su(3)

[{⟨1, 1⟩},{⟨1934, 1⟩}], [{⟨1, 1⟩}], [(1934)], [{⟨1, 1⟩, ⟨43, 1⟩}],[(42, 1),(1, 42)]

- su(1938)
  - sp(969): su(2)
  - so(1938)
  - su(18)

[{⟨1, 1⟩},{⟨1937, 1⟩}], [{⟨1, 1⟩}], [(1937)], [{⟨1, 1⟩}], [{⟨1, 1⟩, ⟨2, 1⟩},{⟨16, 1⟩, ⟨17, 1⟩}]

- su(1944)
  - sp(972): su(2)
  - so(1944): su(9)

[{⟨1, 1⟩},{⟨1943, 1⟩}], [{⟨1, 1⟩}], [(1943)], [{⟨1, 1⟩}], [{⟨1, 2⟩, ⟨8, 2⟩}]

- su(1950)
  - sp(975): su(2)
  - so(1950)
  - su(3)

[{⟨1, 1⟩},{⟨1949, 1⟩}], [{⟨1, 1⟩}], [(1949)], [{⟨1, 1⟩}], [(12, 11),(11, 12)]

- su(1952)
  - sp(976): su(2)
  - so(1952): so(62)

[{⟨1, 1⟩},{⟨1951, 1⟩}], [{⟨1, 1⟩}], [(1951)], [{⟨1, 1⟩}], [{⟨1, 2⟩}]

- su(1953)
  - so(1953): su(2), so(63), sp(31)
  - su(3)
  - su(62)
  - su(63)

[{⟨1, 1⟩},{⟨1952, 1⟩}], [{⟨1, 1⟩}], [(1952)], [{⟨2, 1⟩}], [{⟨1, 2⟩}], [(61, 0),(0, 61)], [{⟨1, 2⟩},{⟨61, 2⟩}], [{⟨2, 1⟩},{⟨61, 1⟩}]

- su(1960)
  - sp(980): su(2), su(6)
  - so(1960)

[{⟨1, 1⟩},{⟨1959, 1⟩}], [{⟨1, 1⟩}], [(1959)], [(0, 1, 1, 1, 0)],[{⟨1, 1⟩}]

- su(1976)
  - sp(988): su(2)
  - so(1976): so(5)

[{⟨1, 1⟩},{⟨1975, 1⟩}], [{⟨1, 1⟩}], [(1975)], [{⟨1, 1⟩}], [(2, 12)]

- su(1980)
  - sp(990): su(2)
  - so(1980): so(9)
  - su(4)
  - su(4)
  - su(4)
  - su(4)
  - su(4)
  - su(6)
  - su(10)

[{⟨1, 1⟩},{⟨1979, 1⟩}], [{⟨1, 1⟩}], [(1979)], [{⟨1, 1⟩}], [(0, 0, 2, 0)], [(1, 8, 0),(0, 8, 1)], [(4, 2, 2),(2, 2, 4)], [(4, 3, 1),(1, 3, 4)], [(5, 4, 0),(0, 4, 5)], [(10, 0, 2),(2, 0, 10)], [(5, 1, 0, 0, 0),(0, 0, 0, 1, 5)], [{⟨1, 1⟩, ⟨6, 1⟩},{⟨4, 1⟩, ⟨9, 1⟩}]

- su(1989)
  - so(1989): su(2)
  - su(3)

[{⟨1, 1⟩},{⟨1988, 1⟩}], [{⟨1, 1⟩}], [(1988)], [(16, 8),(8, 16)]

- su(1995)
  - so(1995): su(2), so(5)
  - su(3)

[{⟨1, 1⟩},{⟨1994, 1⟩}],[{⟨1, 1⟩}],[(1994)],[(4, 8)],[(34, 2),(2, 34)]

- su(2000)
  - sp(1000): su(2), sp(12)
  - so(2000)
  - su(5)

[{⟨1, 1⟩},{⟨1999, 1⟩}], [{⟨1, 1⟩}], [(1999)], [{⟨3, 1⟩}], [{⟨1, 1⟩}],[(4, 0, 1, 1),(1, 1, 0, 4)]

- su(2001)
  - so(2001): su(2)
  - su(3)

[{⟨1, 1⟩},{⟨2000, 1⟩}], [{⟨1, 1⟩}], [(2000)], [(22, 5),(5, 22)]

- su(2002)
  - sp(1001): su(2), sp(3), sp(3), sp(5)
  - so(2002): sp(6), sp(7), so(14), so(22)
  - su(6)
  - su(10)
  - su(14)

[{⟨1, 1⟩},{⟨2001, 1⟩}], [{⟨1, 1⟩}], [(2001)], [(0, 1, 3)], [(9, 0, 0)], [(5, 0, 0, 0, 0)], [{⟨1, 1⟩}], [{⟨1, 1⟩, ⟨3, 1⟩}], [{⟨6, 1⟩}],[{⟨5, 1⟩}],[{⟨1, 3⟩}],[(9, 0, 0, 0, 0),(0, 0, 0, 0, 9)],[{⟨1, 5⟩},{⟨9, 5⟩}],[{⟨5, 1⟩},{⟨9, 1⟩}]

- su(2015)
  - so(2015): su(2), so(63), sp(32)
  - su(3)

[{⟨1, 1⟩},{⟨2014, 1⟩}], [{⟨1, 1⟩}], [(2014)], [{⟨1, 2⟩}], [{⟨2, 1⟩}],[(25, 4),(4, 25)]

- su(2016)
  - sp(1008): su(2), sp(3)
  - so(2016): so(7), so(64)
  - su(3)
  - su(7)
  - su(63)
  - su(64)

[{⟨1, 1⟩},{⟨2015, 1⟩}], [{⟨1, 1⟩}], [(2015)], [(3, 2, 0)], [{⟨1, 1⟩}],[(5, 0, 1)],[{⟨2, 1⟩}],[(62, 0),(0, 62)],[{⟨1, 1⟩, ⟨2, 1⟩, ⟨5, 1⟩},{⟨2, 1⟩, ⟨5, 1⟩, ⟨6, 1⟩}], [{⟨1, 2⟩},{⟨62, 2⟩}],[{⟨2, 1⟩},{⟨62, 1⟩}]

- su(2024)
  - sp(1012): su(2), sp(2), sp(11)
  - so(2024): su(45), so(24)
  - su(3)
  - su(4)
  - su(22)
  - su(24)

[{⟨1, 1⟩},{⟨2023, 1⟩}], [{⟨1, 1⟩}], [(2023)], [(21, 0)], [{⟨1, 3⟩}], [{⟨1, 1⟩}], [{⟨1, 1⟩, ⟨44, 1⟩}], [{⟨3, 1⟩}], [(43, 1),(1, 43)], [(21, 0, 0),(0, 0, 21)], [{⟨1, 3⟩},{⟨21, 3⟩}], [{⟨3, 1⟩},{⟨21, 1⟩}]

- su(2025)
  - so(2025): su(2), so(11)

[{⟨1, 1⟩},{⟨2024, 1⟩}], [{⟨1, 1⟩}], [(2024)], [(2, 1, 0, 0, 0)]

- su(2040)
  - sp(1020): su(2)
  - so(2040)
  - su(3)

[{⟨1, 1⟩},{⟨2039, 1⟩}], [{⟨1, 1⟩}], [(2039)], [{⟨1, 1⟩}], [(29, 3),(3, 29)]

- su(2048)
  - sp(1024): su(2)
  - so(2048): so(24): so(23)

[{⟨1, 1⟩},{⟨2047, 1⟩}], [{⟨1, 1⟩}], [(2047)], [{⟨1, 1⟩}], [{⟨11, 1⟩},{⟨12, 1⟩}],[{⟨11, 1⟩}]

- su(2052)
  - sp(1026): su(2)
  - so(2052)
  - su(3)

[{⟨1, 1⟩},{⟨2051, 1⟩}], [{⟨1, 1⟩}], [(2051)], [{⟨1, 1⟩}], [(18, 7),(7, 18)]

- su(2058)
  - sp(1029): su(2)
  - so(2058)
  - su(3)

[{⟨1, 1⟩},{⟨2057, 1⟩}], [{⟨1, 1⟩}], [(2057)], [{⟨1, 1⟩}], [(20, 6),(6, 20)]

- su(2079)
  - so(2079): su(2), so(7), so(7) (: g2), sp(3), so(6), so(12), so(64), g2
  - su(9)

[{⟨1, 1⟩},{⟨2078, 1⟩}], [{⟨1, 1⟩}], [(2078)], [(0, 2, 2)], [(8, 0, 0)],[(8, 0)],[(5, 0, 1)],[(6, 1, 1)],[{⟨1, 1⟩, ⟨3, 1⟩}], [{⟨1, 2⟩}], [(2, 3)], [{⟨1, 1⟩, ⟨2, 1⟩, ⟨8, 1⟩},{⟨1, 1⟩, ⟨7, 1⟩, ⟨8, 1⟩}]

- su(2080)
  - sp(1040): su(2)
  - so(2080): so(65), sp(32)
  - su(3)
  - su(3)
  - su(4)
  - su(64)
  - su(65)

[{⟨1, 1⟩},{⟨2079, 1⟩}], [{⟨1, 1⟩}], [(2079)], [{⟨1, 1⟩}], [{⟨2, 1⟩}], [{⟨1, 2⟩}], [(15, 9),(9, 15)], [(63, 0),(0, 63)], [(7, 3, 0),(0, 3, 7)], [{⟨1, 2⟩},{⟨63, 2⟩}], [{⟨2, 1⟩}, {⟨63, 1⟩}]

- su(2090)
  - sp(1045): su(2)
  - so(2090): so(5)

[{⟨1, 1⟩},{⟨2089, 1⟩}], [{⟨1, 1⟩}], [(2089)], [{⟨1, 1⟩}], [(3, 10)]

---

su(2) ⟵ sp(1050) ←
so(2100) ←
su(4) ←
su(4) ← su(2100)
su(7) ←
su(8) ←

[{⟨1, 1⟩},{⟨2099, 1⟩}], [{⟨1, 1⟩}], [(2099)], [{⟨1, 1⟩}], [(6, 2, 1),(1, 2, 6)], [(8, 0, 3),(3, 0, 8)], [{⟨1, 3⟩, ⟨3, 1⟩},{⟨4, 1⟩, ⟨6, 3⟩}],[{⟨1, 2⟩, ⟨4, 1⟩},{⟨4, 1⟩, ⟨7, 2⟩}]

---

su(2) ⟵ sp(1053) ←
so(2106) ← su(2106)
su(3) ←

[{⟨1, 1⟩},{⟨2105, 1⟩}], [{⟨1, 1⟩}], [(2105)], [{⟨1, 1⟩}], [(35, 2),(2, 35)]

---

su(2) ←
so(2109) ⟵ su(2109)
so(5) ←

[{⟨1, 1⟩},{⟨2108, 1⟩}],[{⟨1, 1⟩}],[(2108)],[(17, 0)]

---

su(2) ←
sp(1056) ←
so(12) ← su(2112)
so(2112) ←

[{⟨1, 1⟩},{⟨2111, 1⟩}], [{⟨1, 1⟩}], [(2111)], [{⟨1, 2⟩, ⟨5, 1⟩},{⟨1, 2⟩, ⟨6, 1⟩}],[{⟨1, 1⟩}]

---

su(2) ←
so(2115) ←
su(46) ← su(2115)
su(3) ←

[{⟨1, 1⟩},{⟨2114, 1⟩}], [{⟨1, 1⟩}], [(2114)], [{⟨1, 1⟩, ⟨45, 1⟩}],[(44, 1),(1, 44)]

---

su(2) ⟵ sp(1072) ←
su(2144)
so(65) ←
so(2144) ←
sp(33) ←

[{⟨1, 1⟩},{⟨2143, 1⟩}], [{⟨1, 1⟩}], [(2143)], [{⟨1, 1⟩}], [{⟨1, 2⟩}],[{⟨2, 1⟩}]

---

su(2) ←
so(2145) ←
so(66) ←
su(3) ←
su(3) ←
su(5) ← su(2145)
su(10) ←
su(65) ←
su(11) ←
su(66) ←
su(12) ←

[{⟨1, 1⟩},{⟨2144, 1⟩}], [{⟨1, 1⟩}], [(2144)], [{⟨2, 1⟩}], [(14, 10),(10, 14)], [(64, 0),(0, 64)], [(8, 0, 0, 1),(1, 0, 0, 8)], [{⟨1, 3⟩, ⟨9, 1⟩},{⟨1, 1⟩, ⟨9, 3⟩}], [{⟨1, 2⟩},{⟨64, 2⟩}],[{⟨2, 1⟩},{⟨64, 1⟩}],[{⟨1, 2⟩, ⟨2, 1⟩},{⟨9, 1⟩, ⟨10, 2⟩}],[{⟨1, 1⟩, ⟨3, 1⟩},{⟨9, 1⟩, ⟨11, 1⟩}]

---

su(2) ⟵ sp(1078) ←
so(6) ⟵ so(2156) ← su(2156)
su(7) ←

[{⟨1, 1⟩},{⟨2155, 1⟩}], [{⟨1, 1⟩}], [(2155)], [{⟨1, 1⟩}], [(2, 3, 3)],[{⟨1, 3⟩, ⟨6, 2⟩},{⟨1, 2⟩, ⟨6, 3⟩}]

---

su(2) ⟵ sp(1080) ←
so(2160) ←
su(3) ←
su(3) ← su(2160)
su(4) ←
su(16) ←

[{⟨1, 1⟩},{⟨2159, 1⟩}], [{⟨1, 1⟩}], [(2159)], [{⟨1, 1⟩}], [(23, 5),(5, 23)], [(26, 4),(4, 26)], [(14, 0, 1),(1, 0, 14)], [{⟨1, 2⟩, ⟨15, 1⟩},{⟨1, 1⟩, ⟨15, 2⟩}]

---

su(2) ⟵ sp(1085) ←
so(2170) ← su(2170)
su(3) ←

[{⟨1, 1⟩},{⟨2169, 1⟩}], [{⟨1, 1⟩}], [(2169)], [{⟨1, 1⟩}], [(30, 3),(3, 30)]

---

su(2) ←
sp(1092) ←
sp(3) ←
sp(4) ⟵ so(2184) ← su(2184)
su(3) ←

[{⟨1, 1⟩},{⟨2183, 1⟩}], [{⟨1, 1⟩}], [(2183)], [(0, 3, 1)], [{⟨1, 1⟩}],[(0, 3, 0, 0)],[(13, 11),(11, 13)]

---

su(2) ⟵ so(2187) ←
su(2187)
su(3) ←

[{⟨1, 1⟩},{⟨2186, 1⟩}], [{⟨1, 1⟩}], [(2186)], [(17, 8),(8, 17)]

---

su(2) ←
so(2197) ⟵ su(2197)
su(3) ←

[{⟨1, 1⟩},{⟨2196, 1⟩}],[{⟨1, 1⟩}],[(2196)],[(12, 12)]

---

su(2) ←
so(2205) ←
sp(3) ←
su(5) ← su(2205)
su(6) ←

[{⟨1, 1⟩},{⟨2204, 1⟩}], [{⟨1, 1⟩}], [(2204)], [(1, 2, 1)], [(1, 3, 0, 1),(1, 0, 3, 1)],[(1, 2, 0, 0, 1),(1, 0, 0, 2, 1)]

---

su(2) ⟵ sp(1104) ←
su(47) ⟵ so(2208) ← su(2208)
su(3) ←

[{⟨1, 1⟩},{⟨2207, 1⟩}], [{⟨1, 1⟩}], [(2207)], [{⟨1, 1⟩}], [{⟨1, 1⟩, ⟨46, 1⟩}],[(45, 1),(1, 45)]

---

su(2) ⟵ sp(1105) ←
su(2210)
so(66) ⟵ so(2210) ←

[{⟨1, 1⟩},{⟨2209, 1⟩}], [{⟨1, 1⟩}], [(2209)], [{⟨1, 1⟩}], [{⟨1, 2⟩}]

---

su(2) ←
so(67) ← so(2211) ←
sp(33) ←
su(3) ←
su(2211)
su(66) ←
su(67) ←

[{⟨1, 1⟩},{⟨2210, 1⟩}], [{⟨1, 1⟩}], [(2210)], [{⟨2, 1⟩}], [{⟨1, 2⟩}], [(65, 0),(0, 65)], [{⟨1, 2⟩},{⟨65, 2⟩}], [{⟨2, 1⟩},{⟨65, 1⟩}]

---

su(2) ⟵ sp(1110) ←
so(2220) ← su(2220)
su(3) ←

[{⟨1, 1⟩},{⟨2219, 1⟩}], [{⟨1, 1⟩}], [(2219)], [{⟨1, 1⟩}], [(36, 2),(2, 36)]

---

su(2) ⟵ so(2233) ←
su(2233)
su(3) ←

[{⟨1, 1⟩},{⟨2232, 1⟩}], [{⟨1, 1⟩}], [(2232)], [(21, 6),(6, 21)]

---

su(2) ←
sp(2) ←
sp(2) ← sp(1120) ←
sp(2) ← so(2240) ←
su(2240)
sp(3) ← su(3) ←
su(4) ←

[{⟨1, 1⟩},{⟨2239, 1⟩}],[{⟨1, 1⟩}],[(2239)],[(1, 13)],[(3, 9)], [(7, 5)], [(1, 1, 2)], [{⟨1, 1⟩}], [(19, 7),(7, 19)], [(9, 1, 1),(1, 1, 9)]

---

su(2) ⟵ sp(1125) ←
so(2250) ← su(2250)
su(5) ←

[{⟨1, 1⟩},{⟨2249, 1⟩}], [{⟨1, 1⟩}], [(2249)], [{⟨1, 1⟩}], [(4, 0, 2, 0),(0, 2, 0, 4)]

---

su(2) ←
so(5) ←
so(2261) ⟵ su(2261)
so(19) ←
g2 ←

[{⟨1, 1⟩},{⟨2260, 1⟩}], [{⟨1, 1⟩}], [(2260)], [(1, 16)], [{⟨1, 1⟩, ⟨2, 1⟩}],[(1, 4)]

---

su(2) ←
so(13) ← so(2275) ⟵ su(2275)
so(14) ←

[{⟨1, 1⟩},{⟨2274, 1⟩}], [{⟨1, 1⟩}], [(2274)], [{⟨2, 2⟩}], [{⟨1, 4⟩}]

---

su(2) ←
so(23) ←
so(2277) ⟵ su(2277)
so(67) ←
sp(34) ←

[{⟨1, 1⟩},{⟨2276, 1⟩}], [{⟨1, 1⟩}], [(2276)], [{⟨1, 3⟩}], [{⟨1, 2⟩}],[{⟨2, 1⟩}]

---

su(2) ⟵ sp(1139) ←
so(68) ⟵ so(2278) ←
su(3) ← su(2278)
su(67) ←
su(68) ←

[{⟨1, 1⟩},{⟨2277, 1⟩}], [{⟨1, 1⟩}], [(2277)], [{⟨1, 1⟩}], [{⟨2, 1⟩}], [(66, 0),(0, 66)], [{⟨1, 2⟩},{⟨66, 2⟩}], [{⟨2, 1⟩},{⟨66, 1⟩}]

---

su(2) ⟵ sp(1140) ←
so(2280) ← su(2280)
su(19) ←

[{⟨1, 1⟩},{⟨2279, 1⟩}], [{⟨1, 1⟩}], [(2279)], [{⟨1, 1⟩}], [{⟨1, 1⟩, ⟨2, 1⟩},{⟨17, 1⟩, ⟨18, 1⟩}]

---

su(2) ⟵ so(2295) ←
su(3) ←
su(2295)
su(4) ←
su(17) ←

[{⟨1, 1⟩},{⟨2294, 1⟩}], [{⟨1, 1⟩}], [(2294)], [(16, 9),(9, 16)], [(14, 1, 0),(0, 1, 14)], [{⟨1, 1⟩, ⟨15, 1⟩},{⟨2, 1⟩, ⟨16, 1⟩}]

---

su(2) ⟵ sp(1150) ←
so(5) ←
so(2300) ←
so(25) ←
su(4) ← su(2300)
su(23) ←
su(25) ←

[{⟨1, 1⟩},{⟨2299, 1⟩}], [{⟨1, 1⟩}], [(2299)], [{⟨1, 1⟩}], [(0, 22)], [{⟨3, 1⟩}], [(22, 0, 0),(0, 0, 22)], [{⟨1, 3⟩},{⟨22, 3⟩}],[{⟨3, 1⟩},{⟨22, 1⟩}]

---

su(2) ←
so(2303) ←
su(48) ← su(2303)
su(3) ←

[{⟨1, 1⟩},{⟨2302, 1⟩}], [{⟨1, 1⟩}], [(2302)], [{⟨1, 1⟩, ⟨47, 1⟩}],[(46, 1),(1, 46)]

---

su(2) ⟵ sp(1152) ←
so(2304) ←
su(2304)
su(3) ←
su(4) ←

[{⟨1, 1⟩},{⟨2303, 1⟩}], [{⟨1, 1⟩}], [(2303)], [{⟨1, 1⟩}], [(31, 3),(3, 31)],[(5, 1, 3),(3, 1, 5)]

su(2) ← sp(1155)
so(7) ← so(2310)
su(3)
su(4)
su(4) ← su(2310)
su(4)
su(6)
su(7)
su(10)

[{⟨1, 1⟩},{⟨2309, 1⟩}], [{⟨1, 1⟩}], [(2309)], [{⟨1, 1⟩}], [(0, 1, 4)], [(27, 4),(4, 27)], [(3, 4, 1),(1, 4, 3)], [(4, 5, 0),(0, 5, 4)], [(10, 2, 0),(0, 2, 10)], [(4, 0, 0, 0, 2),(2, 0, 0, 0, 4)], [{⟨1, 4⟩, ⟨2, 1⟩},{⟨5, 1⟩, ⟨6, 4⟩}], [{⟨1, 1⟩, ⟨5, 1⟩},{⟨5, 1⟩, ⟨9, 1⟩}]

---

su(2) ← so(2325) ← su(2325)
su(3)

[{⟨1, 1⟩},{⟨2324, 1⟩}], [{⟨1, 1⟩}], [(2324)], [(24, 5),(5, 24)]

---

su(2) ← so(2337) ← su(2337)
su(3)

[{⟨1, 1⟩},{⟨2336, 1⟩}], [{⟨1, 1⟩}], [(2336)], [(37, 2),(2, 37)]

---

su(2)
so(68) ← so(2345) ← su(2345)

[{⟨1, 1⟩},{⟨2344, 1⟩}],[{⟨1, 1⟩}],[(2344)],[{⟨1, 2⟩}]

---

su(2) ← sp(1173)
so(69)
sp(34) ← so(2346)
su(3) ← su(2346)
su(68)
su(69)

[{⟨1, 1⟩},{⟨2345, 1⟩}], [{⟨1, 1⟩}], [(2345)], [{⟨1, 1⟩}], [{⟨2, 1⟩}], [{⟨1, 2⟩}], [(67, 0),(0, 67)], [{⟨1, 2⟩},{⟨67, 2⟩}],[{⟨2, 1⟩},{⟨67, 1⟩}]

---

su(2) ← sp(1176)
su(8) ← so(2352)
su(7) ← su(2352)
su(8)

[{⟨1, 1⟩},{⟨2351, 1⟩}], [{⟨1, 1⟩}], [(2351)], [{⟨1, 1⟩}], [{⟨3, 1⟩, ⟨5, 1⟩}], [{⟨1, 1⟩, ⟨2, 1⟩, ⟨3, 1⟩},{⟨4, 1⟩, ⟨5, 1⟩, ⟨6, 1⟩}],[{⟨3, 1⟩, ⟨4, 1⟩},{⟨4, 1⟩, ⟨5, 1⟩}]

---

su(2) ← sp(1183)
so(6) ← so(2366) ← su(2366)
su(13)

[{⟨1, 1⟩},{⟨2365, 1⟩}], [{⟨1, 1⟩}], [(2365)], [{⟨1, 1⟩}], [(11, 0, 0)],[{⟨2, 2⟩},{⟨11, 2⟩}]

---

su(2) ← sp(1188)
so(2376)
su(3)
su(4) ← su(2376)
su(4)
su(5)
su(10)

[{⟨1, 1⟩},{⟨2375, 1⟩}], [{⟨1, 1⟩}], [(2375)], [{⟨1, 1⟩}], [(15, 10),(10, 15)], [(2, 5, 1),(1, 5, 2)], [(2, 7, 0),(0, 7, 2)], [(7, 0, 1, 0),(0, 1, 0, 7)], [{⟨1, 2⟩, ⟨8, 1⟩},{⟨2, 1⟩, ⟨9, 2⟩}]

---

su(2)
sp(2) ← sp(1190)
so(17)
sp(7) ← so(2380)
su(5) ← su(2380)
su(14)
su(17)

[{⟨1, 1⟩},{⟨2379, 1⟩}], [{⟨1, 1⟩}], [(2379)], [(13, 2)], [{⟨1, 1⟩}], [{⟨4, 1⟩}], [{⟨1, 4⟩}], [(13, 0, 0, 0),(0, 0, 0, 13)],[{⟨1, 4⟩},{⟨13, 4⟩}],[{⟨4, 1⟩},{⟨13, 1⟩}]

---

su(2) ← sp(1197)
so(2394) ← su(2394)
su(3)

[{⟨1, 1⟩},{⟨2393, 1⟩}], [{⟨1, 1⟩}], [(2393)], [{⟨1, 1⟩}], [(18, 8),(8, 18)]

---

su(2) ← sp(1200)
su(49)
so(8) ← so(2400)
su(3) ← su(2400)
su(5)
su(7)

[{⟨1, 1⟩},{⟨2399, 1⟩}], [{⟨1, 1⟩}], [(2399)], [{⟨1, 1⟩}], [{⟨1, 1⟩, ⟨48, 1⟩}], [(3, 0, 2, 0),(3, 0, 0, 2),(2, 0, 3, 0),(2, 0, 0, 3),(0, 0, 3, 2),(0, 0, 2, 3)],[(47, 1),(1, 47)],[(3, 3, 0, 0),(0, 0, 3, 3)],[{⟨1, 3⟩, ⟨4, 1⟩},{⟨3, 1⟩, ⟨6, 3⟩}]

---

su(2)
so(5) ← so(2401) ← su(2401)

[{⟨1, 1⟩},{⟨2400, 1⟩}],[{⟨1, 1⟩}],[(2400)],[(6, 6)]

---

su(2) ← sp(1207) ← su(2414)
so(69)
sp(35) ← so(2414)

[{⟨1, 1⟩},{⟨2413, 1⟩}], [{⟨1, 1⟩}], [(2413)], [{⟨1, 1⟩}], [{⟨1, 2⟩}],[{⟨2, 1⟩}]

---

su(2)
so(5) ← so(2415)
so(70)
su(3)
su(3) ← su(2415)
su(69)
su(70)

[{⟨1, 1⟩},{⟨2414, 1⟩}], [{⟨1, 1⟩}], [(2414)], [(8, 4)], [{⟨2, 1⟩}], [(22, 6),(6, 22)], [(68, 0),(0, 68)], [{⟨1, 2⟩},{⟨68, 2⟩}],[{⟨2, 1⟩},{⟨68, 1⟩}]

---

su(2) ← sp(1215)
so(5)
$\mathfrak{e}_6$ ← so(2430)
su(3) ← su(2430)
su(5)
su(6)

[{⟨1, 1⟩},{⟨2429, 1⟩}], [{⟨1, 1⟩}], [(2429)], [{⟨1, 1⟩}], [(11, 2)],[{⟨2, 2⟩}],[(14, 11),(11, 14)],[(2, 2, 1, 0),(0, 1, 2, 2)],[(2, 1, 0, 1, 0),(0, 1, 0, 1, 2)]

---

su(2) ← sp(1218)
so(2436) ← su(2436)
su(3)

[{⟨1, 1⟩},{⟨2435, 1⟩}], [{⟨1, 1⟩}], [(2435)], [{⟨1, 1⟩}], [(20, 7),(7, 20)]

---

su(2) ← sp(1221)
so(2442) ← su(2442)
su(3)

[{⟨1, 1⟩},{⟨2441, 1⟩}], [{⟨1, 1⟩}], [(2441)], [{⟨1, 1⟩}], [(32, 3),(3, 32)]

---

su(2) ← sp(1225)
so(6) ← so(2450) ← su(2450)
su(7)

[{⟨1, 1⟩},{⟨2449, 1⟩}], [{⟨1, 1⟩}], [(2449)], [{⟨1, 1⟩}], [(1, 4, 4)], [{⟨1, 2⟩, ⟨2, 1⟩, ⟨6, 1⟩},{⟨1, 1⟩, ⟨5, 1⟩, ⟨6, 2⟩}]

---

su(2)
so(9) ← so(2457)
sp(3)
su(3) ← su(2457)
su(3)

[{⟨1, 1⟩},{⟨2456, 1⟩}],[{⟨1, 1⟩}],[(2456)],[(2, 0, 1, 0)],[(0, 2, 2)],[(13, 12),(12, 13)],[(38, 2),(2, 38)]

---

su(2)
sp(2) ← sp(1232)
sp(3) ← so(2464)
su(4) ← su(2464)
su(4)

[{⟨1, 1⟩},{⟨2463, 1⟩}], [{⟨1, 1⟩}], [(2463)], [(5, 7)], [(3, 0, 2)],[{⟨1, 1⟩}],[(3, 3, 2),(2, 3, 3)],[(3, 6, 0),(0, 6, 3)]

---

su(2) ← so(2465) ← su(2465)
su(3)

[{⟨1, 1⟩},{⟨2464, 1⟩}], [{⟨1, 1⟩}], [(2464)], [(28, 4),(4, 28)]

---

su(2) ← sp(1235) ← su(2470)
so(5) ← so(2470)

[{⟨1, 1⟩},{⟨2469, 1⟩}], [{⟨1, 1⟩}], [(2469)], [{⟨1, 1⟩}], [(18, 0)]

---

su(2) ← so(2475) ← su(2475)
su(5)

[{⟨1, 1⟩},{⟨2474, 1⟩}], [{⟨1, 1⟩}], [(2474)], [(5, 2, 0, 0),(0, 0, 2, 5)]

---

su(2) ← sp(1242) ← su(2484)
so(70) ← so(2484)

[{⟨1, 1⟩},{⟨2483, 1⟩}], [{⟨1, 1⟩}], [(2483)], [{⟨1, 1⟩}], [{⟨1, 2⟩}]

---

su(2)
so(71) ← so(2485)
sp(35)
su(3) ← su(2485)
su(70)
su(71)

[{⟨1, 1⟩},{⟨2484, 1⟩}], [{⟨1, 1⟩}], [(2484)], [{⟨2, 1⟩}], [{⟨1, 2⟩}], [(69, 0),(0, 69)], [{⟨1, 2⟩},{⟨69, 2⟩}], [{⟨2, 1⟩},{⟨69, 1⟩}]

---

su(2) ← sp(1248)
so(2496) ← su(2496)
su(3)
su(4)

[{⟨1, 1⟩},{⟨2495, 1⟩}], [{⟨1, 1⟩}], [(2495)], [{⟨1, 1⟩}], [(25, 5),(5, 25)],[(11, 0, 2),(2, 0, 11)]

---

su(2)
su(50) ← so(2499) ← su(2499)
su(3)

[{⟨1, 1⟩},{⟨2498, 1⟩}], [{⟨1, 1⟩}], [(2498)], [{⟨1, 1⟩, ⟨49, 1⟩}],[(48, 1),(1, 48)]

---

su(2)
sp(2) ← sp(1250) ← su(2500)
so(2500)

[{⟨1, 1⟩},{⟨2499, 1⟩}], [{⟨1, 1⟩}], [(2499)], [(9, 4)], [{⟨1, 1⟩}]

---

su(2) ← sp(1254) ← su(2508)
so(9) ← so(2508)

[{⟨1, 1⟩},{⟨2507, 1⟩}], [{⟨1, 1⟩}], [(2507)], [{⟨1, 1⟩}],

[(6, 0, 0, 0)]

---

su(2) ← sp(1260)
so(2520)
su(3)
su(4)
su(5)
su(5)
su(5)
su(5)
su(5)
su(6)
su(6)
su(6)
su(6)
su(6)
su(8)
su(8)
su(8)
su(9) — su(2520)

[{⟨1, 1⟩},{⟨2519, 1⟩}], [{⟨1, 1⟩}], [(2519)], [{⟨1, 1⟩}], [(17, 9),(9, 17)], [(7, 0, 4),(4, 0, 7)], [(0, 4, 1, 0),(0, 1, 4, 0)], [(0, 6, 0, 0),(0, 0, 6, 0)], [(2, 1, 1, 1),(1, 1, 1, 2)], [(3, 1, 0, 2),(2, 0, 1, 3)], [(6, 0, 0, 2),(2, 0, 0, 6)], [(1, 0, 0, 3, 0),(0, 3, 0, 0, 1)], [(2, 0, 2, 0, 0),(0, 0, 2, 0, 2)], [(2, 1, 1, 0, 0),(0, 0, 1, 1, 2)], [(3, 2, 0, 0, 0),(0, 0, 0, 2, 3)], [(6, 0, 0, 0, 1),(1, 0, 0, 0, 6)], [{⟨2, 3⟩},{⟨6, 3⟩}], [{⟨1, 1⟩, ⟨6, 2⟩},{⟨2, 2⟩, ⟨7, 1⟩}], [{⟨1, 4⟩, ⟨7, 1⟩},{⟨1, 1⟩, ⟨7, 4⟩}],[{⟨3, 2⟩},{⟨6, 2⟩}]

---

su(2), sp(3) — sp(1274)
so(2548) — su(2548)

[{⟨1, 1⟩},{⟨2547, 1⟩}], [{⟨1, 1⟩}], [(2547)], [(0, 0, 5)], [{⟨1, 1⟩}]

---

su(2), so(71), sp(36) — so(2555) ← su(2555)

[{⟨1, 1⟩},{⟨2554, 1⟩}], [{⟨1, 1⟩}], [(2554)], [{⟨1, 2⟩}], [{⟨2, 1⟩}]

---

su(2) ← sp(1278)
so(72) ← so(2556)
su(3)
su(71)
su(72) — su(2556)

[{⟨1, 1⟩},{⟨2555, 1⟩}], [{⟨1, 1⟩}], [(2555)], [{⟨1, 1⟩}], [{⟨2, 1⟩}], [(70, 0),(0, 70)], [{⟨1, 2⟩},{⟨70, 2⟩}], [{⟨2, 1⟩},{⟨70, 1⟩}]

---

su(2), sp(2) — sp(1280)
so(9) ← so(2560) — su(2560)

[{⟨1, 1⟩},{⟨2559, 1⟩}], [{⟨1, 1⟩}], [(2559)], [(11, 3)], [{⟨1, 1⟩}],[(1, 1, 0, 1)]

---

su(2), sp(13) — sp(1287)
so(9) ← so(2574)
su(5)
su(12) — su(2574)

[{⟨1, 1⟩},{⟨2573, 1⟩}], [{⟨1, 1⟩}], [(2573)], [{⟨3, 1⟩}], [{⟨1, 1⟩}], [(1, 2, 0, 0)], [(8, 1, 0, 0),(0, 0, 1, 8)], [{⟨1, 1⟩, ⟨9, 1⟩},{⟨3, 1⟩, ⟨11, 1⟩}]

---

su(2) ← sp(1288)
so(24) ← so(2576) — su(2576)

[{⟨1, 1⟩},{⟨2575, 1⟩}], [{⟨1, 1⟩}], [(2575)], [{⟨1, 1⟩}],

[{⟨1, 3⟩}]

---

su(2) ← sp(1290)
so(2580)
su(3) — su(2580)

[{⟨1, 1⟩},{⟨2579, 1⟩}], [{⟨1, 1⟩}], [(2579)], [{⟨1, 1⟩}], [(39, 2),(2, 39)]

---

su(2) ← sp(1292)
so(2584)
su(3)
su(4)
su(17) — su(2584)

[{⟨1, 1⟩},{⟨2583, 1⟩}], [{⟨1, 1⟩}], [(2583)], [{⟨1, 1⟩}], [(33, 3),(3, 33)],[(15, 0, 1),(1, 0, 15)],[{⟨1, 2⟩, ⟨16, 1⟩},{⟨1, 1⟩, ⟨16, 2⟩}]

---

su(2), sp(2), sp(12) — sp(1300)
su(51), so(26) — so(2600)
su(3)
su(4)
su(4)
su(24)
su(26) — su(2600)

[{⟨1, 1⟩},{⟨2599, 1⟩}], [{⟨1, 1⟩}], [(2599)], [(23, 0)], [{⟨1, 3⟩}], [{⟨1, 1⟩}], [{⟨1, 1⟩, ⟨50, 1⟩}], [{⟨3, 1⟩}], [(49, 1),(1, 49)], [(7, 1, 2),(2, 1, 7)], [(23, 0, 0),(0, 0, 23)], [{⟨1, 3⟩},{⟨23, 3⟩}],[{⟨3, 1⟩},{⟨23, 1⟩}]

---

su(2) ← sp(1302)
so(2604)
su(3) — su(2604)

[{⟨1, 1⟩},{⟨2603, 1⟩}], [{⟨1, 1⟩}], [(2603)], [{⟨1, 1⟩}], [(23, 6),(6, 23)]

---

su(2) ← sp(1305)
so(2610)
su(3) — su(2610)

[{⟨1, 1⟩},{⟨2609, 1⟩}], [{⟨1, 1⟩}], [(2609)], [{⟨1, 1⟩}], [(19, 8),(8, 19)]

---

su(2) ← sp(1309)
so(2618)
su(3) — su(2618)

[{⟨1, 1⟩},{⟨2617, 1⟩}], [{⟨1, 1⟩}], [(2617)], [{⟨1, 1⟩}], [(16, 10),(10, 16)]

---

su(2) ← so(2625)
su(3)
su(5)
su(5) — su(2625)

[{⟨1, 1⟩},{⟨2624, 1⟩}], [{⟨1, 1⟩}], [(2624)], [(29, 4),(4, 29)],[(3, 0, 1, 2),(2, 1, 0, 3)],[(4, 1, 1, 0),(0, 1, 1, 4)]

---

su(2), so(72) — so(2627) ← su(2627)

[{⟨1, 1⟩},{⟨2626, 1⟩}],[{⟨1, 1⟩}],[(2626)],[{⟨1, 2⟩}]

---

su(2) ← sp(1314)
so(73), sp(36) — so(2628)
su(3)
su(72)
su(73) — su(2628)

[{⟨1, 1⟩},{⟨2627, 1⟩}], [{⟨1, 1⟩}], [(2627)], [{⟨1, 1⟩}], [{⟨2, 1⟩}], [{⟨1, 2⟩}], [(71, 0),(0, 71)], [{⟨1, 2⟩},{⟨71, 2⟩}],[{⟨2, 1⟩},{⟨71, 1⟩}]

---

su(2), sp(2), sp(10) — sp(1320)
so(6)
so(7) ← so(8) — so(2640)
so(20)
su(3)
so(10) — su(2640)

[{⟨1, 1⟩},{⟨2639, 1⟩}], [{⟨1, 1⟩}], [(2639)], [(17, 1)], [{⟨1, 1⟩, ⟨2, 1⟩}], [{⟨1, 1⟩}], [(4, 2, 2)], [(7, 0, 0, 0),(0, 0, 7, 0),(0, 0, 0, 7)],[(0, 0, 7)],[{⟨1, 1⟩, ⟨2, 1⟩}],[(21, 7),(7, 21)],[(3, 0, 0, 1, 0),(3, 0, 0, 0, 1)]

---

su(2) ← sp(1323)
so(2646)
su(7)
su(7) — su(2646)

[{⟨1, 1⟩},{⟨2645, 1⟩}], [{⟨1, 1⟩}], [(2645)], [{⟨1, 1⟩}], [{⟨1, 1⟩, ⟨3, 2⟩},{⟨4, 2⟩, ⟨6, 1⟩}], [{⟨1, 2⟩, ⟨2, 2⟩},{⟨5, 2⟩, ⟨6, 2⟩}]

---

su(2) ← sp(1326)
f4 ← so(2652) — su(2652)

[{⟨1, 1⟩},{⟨2651, 1⟩}], [{⟨1, 1⟩}], [(2651)], [{⟨1, 1⟩}], [(0, 0, 0, 3)]

---

su(2) ← sp(1330)
so(2660)
su(20) — su(2660)

[{⟨1, 1⟩},{⟨2659, 1⟩}], [{⟨1, 1⟩}], [(2659)], [{⟨1, 1⟩}], [{⟨1, 1⟩, ⟨2, 1⟩},{⟨18, 1⟩, ⟨19, 1⟩}]

---

su(2) ← so(2673)
su(3) — su(2673)

[{⟨1, 1⟩},{⟨2672, 1⟩}], [{⟨1, 1⟩}], [(2672)], [(26, 5),(5, 26)]

---

su(2) ← sp(1344)
so(2688)
su(3)
su(6) — su(2688)

[{⟨1, 1⟩},{⟨2687, 1⟩}], [{⟨1, 1⟩}], [(2687)], [{⟨1, 1⟩}], [(15, 11),(11, 15)],[(3, 1, 0, 0, 1),(1, 0, 0, 1, 3)]

---

su(2), su(6) — so(2695) ← su(2695)

[{⟨1, 1⟩},{⟨2694, 1⟩}], [{⟨1, 1⟩}], [(2694)], [(3, 0, 0, 0, 3)]

---

su(2) ← sp(1350)
so(73), sp(37) — so(2700)
su(5)
su(9) — su(2700)

[{⟨1, 1⟩},{⟨2699, 1⟩}], [{⟨1, 1⟩}], [(2699)], [{⟨1, 1⟩}], [{⟨1, 2⟩}], [{⟨2, 1⟩}], [(2, 1, 2, 0),(0, 2, 1, 2)], [{⟨2, 1⟩, ⟨6, 1⟩},{⟨3, 1⟩, ⟨7, 1⟩}]

---

su(2), so(74) — so(2701)
su(3)
su(73)
su(74) — su(2701)

[{⟨1, 1⟩},{⟨2700, 1⟩}], [{⟨1, 1⟩}], [(2700)], [{⟨2, 1⟩}], [(72, 0),(0, 72)], [{⟨1, 2⟩},{⟨72, 2⟩}], [{⟨2, 1⟩},{⟨72, 1⟩}]

---

su(2), su(52) — so(2703)
su(3) — su(2703)

[{⟨1, 1⟩},{⟨2702, 1⟩}], [{⟨1, 1⟩}], [(2702)], [{⟨1, 1⟩, ⟨51, 1⟩}],[(50, 1),(1, 50)]

su(2) ← sp(1353)
so(2706) ← su(2706)
su(3)

[{⟨1, 1⟩},{⟨2705, 1⟩}], [{⟨1, 1⟩}], [(2705)], [{⟨1, 1⟩}], [(40, 2),(2, 40)]

---

su(2)
so(2717) ← su(2717)
so(11)

[{⟨1, 1⟩},{⟨2716, 1⟩}], [{⟨1, 1⟩}], [(2716)], [(5, 0, 0, 0, 0)]

---

su(2)
sp(1360)
sp(2) su(2720)
so(2720)

[{⟨1, 1⟩},{⟨2719, 1⟩}], [{⟨1, 1⟩}], [(2719)], [(1, 14)], [{⟨1, 1⟩}]

---

su(2) ← sp(1365)
so(2730)
su(3)
su(3) su(2730)
su(4)
su(4)

[{⟨1, 1⟩},{⟨2729, 1⟩}], [{⟨1, 1⟩}], [(2729)], [{⟨1, 1⟩}], [(14, 12),(12, 14)], [(34, 3),(3, 34)], [(6, 4, 0),(0, 4, 6)], [(8, 3, 0),(0, 3, 8)]

---

su(2) ← sp(1368)
so(2736)
su(4) su(2736)
su(18)

[{⟨1, 1⟩},{⟨2735, 1⟩}], [{⟨1, 1⟩}], [(2735)], [{⟨1, 1⟩}], [(15, 1, 0),(0, 1, 15)], [{⟨1, 1⟩, ⟨16, 1⟩},{⟨2, 1⟩, ⟨17, 1⟩}]

---

su(2) ← sp(1372)
su(3) ← so(2744) ← su(2744)
su(4)

[{⟨1, 1⟩},{⟨2743, 1⟩}], [{⟨1, 1⟩}], [(2743)], [{⟨1, 1⟩}], [(13, 13)],[(6, 0, 5),(5, 0, 6)]

---

su(2) ← sp(1375)
so(2750) ← su(2750)
su(4)

[{⟨1, 1⟩},{⟨2749, 1⟩}], [{⟨1, 1⟩}], [(2749)], [{⟨1, 1⟩}], [(9, 0, 3),(3, 0, 9)]

---

su(2) ← so(2755)
su(3) su(2755)

[{⟨1, 1⟩},{⟨2754, 1⟩}], [{⟨1, 1⟩}], [(2754)], [(18, 9),(9, 18)]

---

su(2) ← sp(1386)
so(9)
so(9) so(2772) ← su(2772)
so(9) su(9)
so(10)

[{⟨1, 1⟩},{⟨2771, 1⟩}], [{⟨1, 1⟩}], [(2771)], [{⟨1, 1⟩}], [(0, 0, 0, 4)], [(0, 1, 0, 2)], [(3, 1, 0, 0)], [{⟨1, 2⟩, ⟨3, 1⟩},{⟨6, 1⟩, ⟨8, 2⟩}],[(0, 0, 0, 4, 0),(0, 0, 0, 0, 4)]

---

su(2) ← sp(1387)
su(2774)
so(74) ← so(2774)

[{⟨1, 1⟩},{⟨2773, 1⟩}], [{⟨1, 1⟩}], [(2773)], [{⟨1, 1⟩}], [{⟨1, 2⟩}]

---

su(2)
so(75) so(2775)
sp(37) su(3)
su(2775)
su(74)
su(75)

[{⟨1, 1⟩},{⟨2774, 1⟩}], [{⟨1, 1⟩}], [(2774)], [{⟨2, 1⟩}], [{⟨1, 2⟩}], [(73, 0),(0, 73)], [{⟨1, 2⟩},{⟨73, 2⟩}], [{⟨2, 1⟩},{⟨73, 1⟩}]

---

su(2) ← sp(1395)
so(2790) ← su(2790)
su(3)

[{⟨1, 1⟩},{⟨2789, 1⟩}], [{⟨1, 1⟩}], [(2789)], [{⟨1, 1⟩}], [(30, 4),(4, 30)]

---

su(2) ← sp(1400)
so(7)
so(2800)
so(8)
su(3) su(2800)
su(7)
su(8)

[{⟨1, 1⟩},{⟨2799, 1⟩}], [{⟨1, 1⟩}], [(2799)], [{⟨1, 1⟩}], [(1, 2, 1)], [(2, 1, 1, 0),(2, 1, 0, 1),(1, 1, 2, 0),(1, 1, 0, 2),(0, 1, 2, 1),(0, 1, 1, 2)], [(24, 6),(6, 24)], [{⟨1, 2⟩, ⟨5, 1⟩, ⟨6, 1⟩},{⟨1, 1⟩, ⟨2, 1⟩, ⟨6, 2⟩}], [{⟨1, 1⟩, ⟨3, 1⟩, ⟨7, 1⟩},{⟨1, 1⟩, ⟨5, 1⟩, ⟨7, 1⟩}]

---

su(2) ← sp(1404)
su(53) ← so(2808) ← su(2808)
su(3)

[{⟨1, 1⟩},{⟨2807, 1⟩}], [{⟨1, 1⟩}], [(2807)], [{⟨1, 1⟩}], [{⟨1, 1⟩, ⟨52, 1⟩}],[(51, 1),(1, 51)]

---

su(2)
so(5) so(2835)
so(5) su(3) su(2835)
su(3)

[{⟨1, 1⟩},{⟨2834, 1⟩}],[{⟨1, 1⟩}],[(2834)],[(2, 14)],[(5, 8)],[(20, 8),(8, 20)],[(41, 2),(2, 41)]

---

su(2)
so(75) so(2849) ← su(2849)
sp(38)

[{⟨1, 1⟩},{⟨2848, 1⟩}], [{⟨1, 1⟩}], [(2848)], [{⟨1, 2⟩}], [{⟨2, 1⟩}]

---

su(2) ← sp(1425)
so(76) ← so(2850)
su(3) su(2850)
su(75)
su(76)

[{⟨1, 1⟩},{⟨2849, 1⟩}], [{⟨1, 1⟩}], [(2849)], [{⟨1, 1⟩}], [{⟨2, 1⟩}], [(74, 0),(0, 74)], [{⟨1, 2⟩},{⟨74, 2⟩}], [{⟨2, 1⟩},{⟨74, 1⟩}]

---

su(2) ← sp(1426)
so(2852) ← su(2852)
su(3)

[{⟨1, 1⟩},{⟨2851, 1⟩}], [{⟨1, 1⟩}], [(2851)], [{⟨1, 1⟩}], [(22, 7),(7, 22)]

---

su(2) ← sp(1428)
so(2856) ← su(2856)
su(3)

[{⟨1, 1⟩},{⟨2855, 1⟩}], [{⟨1, 1⟩}], [(2855)], [{⟨1, 1⟩}], [(27, 5),(5, 27)]

---

su(2)
sp(2) sp(1430)
sp(5)
so(12) ← so(2860) su(2860)
su(4)
su(4)
su(4)

[{⟨1, 1⟩},{⟨2859, 1⟩}],[{⟨1, 1⟩}],[(2859)],[(3, 10)],[(0, 1, 1, 0, 0)], [{⟨1, 1⟩}], [{⟨1, 2⟩, ⟨2, 1⟩}], [(1, 9, 0),(0, 9, 1)],[(7, 2, 1),(1, 2, 7)],[(10, 1, 1),(1, 1, 10)]

---

su(2) ← sp(1435)
su(2870)
so(5) ← so(2870)

[{⟨1, 1⟩},{⟨2869, 1⟩}], [{⟨1, 1⟩}], [(2869)], [{⟨1, 1⟩}], [(19, 0)]

---

su(2) ← so(2871)
su(2871)
su(3)

[{⟨1, 1⟩},{⟨2870, 1⟩}], [{⟨1, 1⟩}], [(2870)], [(17, 10),(10, 17)]

---

su(2) ← sp(1440)
so(2880)
su(3) su(2880)
su(4)
su(4)

[{⟨1, 1⟩},{⟨2879, 1⟩}], [{⟨1, 1⟩}], [(2879)], [{⟨1, 1⟩}], [(35, 3),(3, 35)],[(5, 3, 1),(1, 3, 5)],[(11, 2, 0),(0, 2, 11)]

---

su(2) ← sp(1450)
su(2900)
so(25) ← so(2900)

[{⟨1, 1⟩},{⟨2899, 1⟩}], [{⟨1, 1⟩}], [(2899)], [{⟨1, 1⟩}], [{⟨1, 3⟩}]

---

su(2) ← sp(1452)
su(2904)
su(11) ← so(2904)

[{⟨1, 1⟩},{⟨2903, 1⟩}], [{⟨1, 1⟩}], [(2903)], [{⟨1, 1⟩}], [{⟨2, 1⟩, ⟨9, 1⟩}]

---

su(2)
so(2907) ← su(2907)
sp(9)

[{⟨1, 1⟩},{⟨2906, 1⟩}],[{⟨1, 1⟩}],[(2906)],[{⟨4, 1⟩}]

---

su(2)
so(2915)
su(54) su(2915)
su(3)

[{⟨1, 1⟩},{⟨2914, 1⟩}], [{⟨1, 1⟩}], [(2914)], [{⟨1, 1⟩, ⟨53, 1⟩}],[(52, 1),(1, 52)]

---

su(2) ← sp(1458)
so(2916) ← su(2916)
su(4)

[{⟨1, 1⟩},{⟨2915, 1⟩}], [{⟨1, 1⟩}], [(2915)], [{⟨1, 1⟩}], [(5, 2, 2),(2, 2, 5)]

---

su(2)
su(10)
so(5)
so(13)
so(2925)
so(27)
su(4)
sp(6) su(2925)
su(25)
so(76)
su(27)
$\mathfrak{e}_6$

[{⟨1, 1⟩},{⟨2924, 1⟩}], [{⟨1, 1⟩}], [(2924)], [{⟨1, 2⟩, ⟨9, 2⟩}], [(0, 24)], [{⟨1, 1⟩, ⟨3, 1⟩}], [{⟨3, 1⟩}], [{⟨1, 2⟩, ⟨2, 1⟩}], [{⟨1, 2⟩}], [{⟨4, 1⟩}], [(24, 0, 0),(0, 0, 24)], [{⟨1, 3⟩},{⟨24, 3⟩}],[{⟨3, 1⟩},{⟨24, 1⟩}]

---

su(2) ← sp(1463)
so(77)
sp(38) so(2926)
su(2926)
$\mathfrak{g}_2$ su(3)
su(76)
su(77)

[{⟨1, 1⟩},{⟨2925, 1⟩}], [{⟨1, 1⟩}], [(2925)], [{⟨1, 1⟩}], [{⟨2, 1⟩}], [{⟨1, 2⟩}], [(4, 2)], [(75, 0),(0, 75)], [{⟨1, 2⟩},{⟨75, 2⟩}],[{⟨2, 1⟩},{⟨75, 1⟩}]

su(2) ← sp(1470)
so(15) ← so(2940)
su(7)
su(7)
su(2940)

[{⟨1, 1⟩},{⟨2939, 1⟩}], [{⟨1, 1⟩}], [(2939)], [{⟨1, 1⟩}], [{⟨1, 4⟩}], [{⟨1, 1⟩, ⟨4, 2⟩},{⟨3, 2⟩, ⟨6, 1⟩}], [{⟨1, 1⟩, ⟨2, 1⟩, ⟨4, 1⟩},{⟨3, 1⟩, ⟨5, 1⟩, ⟨6, 1⟩}]

---

su(2) ← sp(1479)
so(2958)
su(3)
su(2958)

[{⟨1, 1⟩},{⟨2957, 1⟩}], [{⟨1, 1⟩}], [(2957)], [{⟨1, 1⟩}], [(16, 11),(11, 16)]

---

su(2) ← sp(1480)
so(2960)
su(3)
su(2960)

[{⟨1, 1⟩},{⟨2959, 1⟩}], [{⟨1, 1⟩}], [(2959)], [{⟨1, 1⟩}], [(31, 4),(4, 31)]

---

su(2) ← so(2967)
su(3)
su(2967)

[{⟨1, 1⟩},{⟨2966, 1⟩}], [{⟨1, 1⟩}], [(2966)], [(42, 2),(2, 42)]

---

su(2) ← sp(1485)
so(10) ← so(2970)
su(5)
su(9)
su(2970)

[{⟨1, 1⟩},{⟨2969, 1⟩}], [{⟨1, 1⟩}], [(2969)], [{⟨1, 1⟩}], [(0, 1, 1, 0, 0)], [(5, 1, 0, 1),(1, 0, 1, 5)], [{⟨1, 1⟩, ⟨2, 2⟩},{⟨7, 2⟩, ⟨8, 1⟩}]

---

su(2) ← sp(1500)
so(3000)
su(3)
su(3000)

[{⟨1, 1⟩},{⟨2999, 1⟩}], [{⟨1, 1⟩}], [(2999)], [{⟨1, 1⟩}], [(19, 9),(9, 19)]

---

su(2) ← sp(1501)
so(77)
so(3002)
sp(39)
su(3002)

[{⟨1, 1⟩},{⟨3001, 1⟩}], [{⟨1, 1⟩}], [(3001)], [{⟨1, 1⟩}], [{⟨1, 2⟩}],[{⟨2, 1⟩}]

---

su(2)
so(7)
so(7)
so(11)
so(15)
so(3003)
sp(3)
sp(3)
so(14)
so(78)
g2
su(3)
su(3)
su(6)
su(7)
su(9)
su(11)
su(14)
su(15)
su(77)
su(12)
su(78)
su(13)
e6
su(3003)

[{⟨1, 1⟩},{⟨3002, 1⟩}], [{⟨1, 1⟩}], [(3002)], [(0, 4, 0)], [(1, 3, 0)], [(1, 0, 0, 1, 0)], [{⟨5, 1⟩}], [(6, 1, 0)], [(10, 0, 0)],[{⟨6, 1⟩, ⟨7, 1⟩}],[{⟨2, 1⟩}],[(6, 1)],[(25, 6),(6, 25)], [(76, 0),(0, 76)], [(10, 0, 0, 0, 0),(0, 0, 0, 0, 10)], [{⟨1, 8⟩},{⟨6, 8⟩}], [{⟨1, 6⟩},{⟨8, 6⟩}], [{⟨1, 5⟩},{⟨10, 5⟩}], [{⟨6, 1⟩},{⟨8, 1⟩}], [{⟨5, 1⟩},{⟨10, 1⟩}], [{⟨1, 2⟩},{⟨76, 2⟩}], [{⟨2, 1⟩},{⟨76, 1⟩}], [{⟨1, 2⟩, ⟨2, 1⟩},{⟨10, 1⟩, ⟨11, 2⟩}], [{⟨1, 1⟩, ⟨3, 1⟩},{⟨10, 1⟩, ⟨12, 1⟩}],[{⟨1, 3⟩},{⟨6, 3⟩}]

---

su(2) ← sp(1508)
so(5) ← so(3016)
su(3)
su(3016)

[{⟨1, 1⟩},{⟨3015, 1⟩}], [{⟨1, 1⟩}], [(3015)], [{⟨1, 1⟩}], [(12, 2)],[(15, 12),(12, 15)]

---

su(2) ← sp(1512)
su(55)
so(3024)
so(7)
su(3)
su(5)
su(7)
su(7)
su(3024)

[{⟨1, 1⟩},{⟨3023, 1⟩}], [{⟨1, 1⟩}], [(3023)], [{⟨1, 1⟩}], [{⟨1, 1⟩, ⟨54, 1⟩}], [(1, 0, 5)], [(53, 1),(1, 53)], [(1, 3, 1, 0),(0, 1, 3, 1)], [{⟨1, 1⟩, ⟨4, 1⟩, ⟨5, 1⟩},{⟨2, 1⟩, ⟨3, 1⟩, ⟨6, 1⟩}],[{⟨1, 5⟩, ⟨6, 1⟩},{⟨1, 1⟩, ⟨6, 5⟩}]

---

su(2) ← sp(1517)
so(3034)
su(3)
su(3034)

[{⟨1, 1⟩},{⟨3033, 1⟩}], [{⟨1, 1⟩}], [(3033)], [{⟨1, 1⟩}], [(36, 3),(3, 36)]

---

su(2) ← so(3045)
su(3)
su(3)
su(3045)

[{⟨1, 1⟩},{⟨3044, 1⟩}], [{⟨1, 1⟩}], [(3044)], [(14, 13),(13, 14)],[(28, 5),(5, 28)]

---

su(2)
so(5)
so(3059) ← su(3059)
so(21)

[{⟨1, 1⟩},{⟨3058, 1⟩}], [{⟨1, 1⟩}], [(3058)], [(1, 18)], [{⟨1, 1⟩, ⟨2, 1⟩}]

---

su(2) ← sp(1530)
so(18) ← so(3060)
su(4)
su(5)
su(15)
su(18)
su(18)
su(3060)

[{⟨1, 1⟩},{⟨3059, 1⟩}], [{⟨1, 1⟩}], [(3059)], [{⟨1, 1⟩}], [{⟨4, 1⟩}], [(16, 0, 1),(1, 0, 16)], [(14, 0, 0, 0),(0, 0, 0, 14)], [{⟨1, 4⟩},{⟨14, 4⟩}], [{⟨4, 1⟩},{⟨14, 1⟩}], [{⟨1, 2⟩, ⟨17, 1⟩},{⟨1, 1⟩, ⟨17, 2⟩}]

---

su(2) ← so(3069)
su(3)
su(3069)

[{⟨1, 1⟩},{⟨3068, 1⟩}], [{⟨1, 1⟩}], [(3068)], [(21, 8),(8, 21)]

---

su(2) ← sp(1536)
sp(3) ← so(3072)
su(3)
su(3072)

[{⟨1, 1⟩},{⟨3071, 1⟩}], [{⟨1, 1⟩}], [(3071)], [{⟨1, 1⟩}], [(3, 1, 1)],[(23, 7),(7, 23)]

---

su(2)
sp(1540)
sp(2)
so(5)
so(7)
so(3080)
so(14)
so(78)
su(5)
su(6)
su(8)
su(11)
su(21)
su(3080)

[{⟨1, 1⟩},{⟨3079, 1⟩}], [{⟨1, 1⟩}], [(3079)], [(7, 6)], [{⟨1, 1⟩}], [(4, 10)], [(0, 3, 1)], [{⟨2, 2⟩}], [{⟨1, 2⟩}], [(9, 0, 0, 1),(1, 0, 0, 9)], [(5, 0, 0, 1, 0),(0, 1, 0, 0, 5)], [{⟨1, 3⟩, ⟨6, 1⟩},{⟨2, 1⟩, ⟨7, 3⟩}], [{⟨1, 3⟩, ⟨10, 1⟩},{⟨1, 1⟩, ⟨10, 3⟩}],[{⟨1, 1⟩, ⟨2, 1⟩},{⟨19, 1⟩, ⟨20, 1⟩}]

---

su(2)
so(79)
so(3081)
sp(39)
su(3)
su(78)
su(79)
su(3081)

[{⟨1, 1⟩},{⟨3080, 1⟩}], [{⟨1, 1⟩}], [(3080)], [{⟨2, 1⟩}], [{⟨1, 2⟩}], [(77, 0),(0, 77)], [{⟨1, 2⟩},{⟨77, 2⟩}], [{⟨2, 1⟩},{⟨77, 1⟩}]

---

su(2) ← sp(1547)
so(5)
so(3094)
sp(7)
su(4)
su(3094)

[{⟨1, 1⟩},{⟨3093, 1⟩}], [{⟨1, 1⟩}], [(3093)], [{⟨1, 1⟩}], [(3, 12)],[{⟨2, 2⟩}],[(12, 0, 2),(2, 0, 12)]

---

su(2) ← sp(1551)
so(3102)
su(3)
su(3102)

[{⟨1, 1⟩},{⟨3101, 1⟩}], [{⟨1, 1⟩}], [(3101)], [{⟨1, 1⟩}], [(43, 2),(2, 43)]

---

su(2)
so(3125) ← su(3125)
so(5)

[{⟨1, 1⟩},{⟨3124, 1⟩}],[{⟨1, 1⟩}],[(3124)],[(9, 4)]

---

su(2)
so(3135)
su(56)
su(3)
su(3)
su(3)
su(3135)

[{⟨1, 1⟩},{⟨3134, 1⟩}], [{⟨1, 1⟩}], [(3134)], [{⟨1, 1⟩, ⟨55, 1⟩}], [(18, 10),(10, 18)], [(32, 4),(4, 32)], [(54, 1),(1, 54)]

---

su(2) ← sp(1575)
so(3150)
su(5)
su(3150)

[{⟨1, 1⟩},{⟨3149, 1⟩}], [{⟨1, 1⟩}], [(3149)], [{⟨1, 1⟩}], [(2, 4, 0, 0),(0, 0, 4, 2)]

---

su(2)
so(79)
so(3159) ← su(3159)
sp(40)

[{⟨1, 1⟩},{⟨3158, 1⟩}], [{⟨1, 1⟩}], [(3158)], [{⟨1, 2⟩}], [{⟨2, 1⟩}]

---

su(2) ← sp(1580)
so(80) ← so(3160)
su(3)
su(79)
su(80)
su(3160)

[{⟨1, 1⟩},{⟨3159, 1⟩}], [{⟨1, 1⟩}], [(3159)], [{⟨1, 1⟩}], [{⟨2, 1⟩}], [(78, 0),(0, 78)], [{⟨1, 2⟩},{⟨78, 2⟩}], [{⟨2, 1⟩},{⟨78, 1⟩}]

su(2) ← sp(1584)
so(3168)
su(9)
su(11)
su(3168)

[{⟨1, 1⟩},{⟨3167, 1⟩}], [{⟨1, 1⟩}], [(3167)], [{⟨1, 1⟩}], [{⟨1, 3⟩, ⟨2, 1⟩},{⟨7, 1⟩, ⟨8, 3⟩}], [{⟨1, 1⟩, ⟨4, 1⟩},{⟨7, 1⟩, ⟨10, 1⟩}]

su(2), so(6)
so(3185)
su(14)
su(3185)

[{⟨1, 1⟩},{⟨3184, 1⟩}], [{⟨1, 1⟩}], [(3184)], [(12, 0, 0)], [{⟨2, 2⟩},{⟨12, 2⟩}]

su(2) ← sp(1596)
so(3192)
su(3)
su(3192)

[{⟨1, 1⟩},{⟨3191, 1⟩}], [{⟨1, 1⟩}], [(3191)], [{⟨1, 1⟩}], [(37, 3),(3, 37)]

su(2) ← sp(1600)
so(6) ← so(3200)
su(6)
su(10)
su(3200)

[{⟨1, 1⟩},{⟨3199, 1⟩}], [{⟨1, 1⟩}], [(3199)], [{⟨1, 1⟩}], [(7, 1, 1)], [(3, 0, 0, 1, 1),(1, 1, 0, 0, 3)], [{⟨1, 1⟩, ⟨2, 1⟩, ⟨9, 1⟩},{⟨1, 1⟩, ⟨8, 1⟩, ⟨9, 1⟩}]

su(2) ← so(3213)
su(3)
su(3213)

[{⟨1, 1⟩},{⟨3212, 1⟩}], [{⟨1, 1⟩}], [(3212)], [(26, 6),(6, 26)]

su(2) ← sp(1610)
so(5) ← so(3220)
su(3220)

[{⟨1, 1⟩},{⟨3219, 1⟩}], [{⟨1, 1⟩}], [(3219)], [{⟨1, 1⟩}], [(7, 6)]

su(2) ← sp(1615)
so(3230)
su(4)
su(19)
su(3230)

[{⟨1, 1⟩},{⟨3229, 1⟩}], [{⟨1, 1⟩}], [(3229)], [{⟨1, 1⟩}], [(16, 1, 0),(0, 1, 16)], [{⟨1, 1⟩, ⟨17, 1⟩},{⟨2, 1⟩, ⟨18, 1⟩}]

su(2), so(80)
so(3239) ← su(3239)

[{⟨1, 1⟩},{⟨3238, 1⟩}],[{⟨1, 1⟩}],[(3238)],[{⟨1, 2⟩}]

su(2), sp(2)
sp(1620)
so(81), sp(40)
so(3240)
su(3)
su(3)
su(3)
su(3)
su(6)
su(80)
su(81)
su(3240)

[{⟨1, 1⟩},{⟨3239, 1⟩}], [{⟨1, 1⟩}], [(3239)], [(5, 8)], [{⟨1, 1⟩}], [{⟨2, 1⟩}], [{⟨1, 2⟩}], [(17, 11),(11, 17)], [(29, 5),(5, 29)], [(44, 2),(2, 44)], [(79, 0),(0, 79)], [(2, 0, 1, 1, 0),(0, 1, 1, 0, 2)], [{⟨1, 2⟩},{⟨79, 2⟩}], [{⟨2, 1⟩},{⟨79, 1⟩}]

su(2), sp(14)
sp(1624)
su(57) ← so(3248)
su(3)
su(3248)

[{⟨1, 1⟩},{⟨3247, 1⟩}], [{⟨1, 1⟩}], [(3247)], [{⟨3, 1⟩}], [{⟨1, 1⟩}],[{⟨1, 1⟩, ⟨56, 1⟩}],[(55, 1),(1, 55)]

su(2) ← sp(1625)
so(26) ← so(3250)
su(3250)

[{⟨1, 1⟩},{⟨3249, 1⟩}], [{⟨1, 1⟩}], [(3249)], [{⟨1, 1⟩}], [{⟨1, 3⟩}]

su(2) ← so(3255)
su(3)
su(3255)

[{⟨1, 1⟩},{⟨3254, 1⟩}], [{⟨1, 1⟩}], [(3254)], [(20, 9),(9, 20)]

su(2), sp(2)
sp(1632)
so(3264)
su(3264)

[{⟨1, 1⟩},{⟨3263, 1⟩}], [{⟨1, 1⟩}], [(3263)], [(1, 15)], [{⟨1, 1⟩}]

su(2), sp(2), sp(13)
sp(1638)
sp(3), so(28)
so(3276)
su(4)
su(4)
su(4)
su(26)
su(28)
su(3276)

[{⟨1, 1⟩},{⟨3275, 1⟩}], [{⟨1, 1⟩}], [(3275)], [(25, 0)], [{⟨1, 3⟩}], [{⟨1, 1⟩}], [(2, 3, 0)], [{⟨3, 1⟩}], [(5, 5, 0),(0, 5, 5)],[(6, 1, 3),(3, 1, 6)],[(25, 0, 0),(0, 0, 25)],[{⟨1, 3⟩},{⟨25, 3⟩}],[{⟨3, 1⟩},{⟨25, 1⟩}]

su(2), $g_2$ ← so(7)
so(3289) ← su(3289)

[{⟨1, 1⟩},{⟨3288, 1⟩}], [{⟨1, 1⟩}], [(3288)], [(9, 0, 0)], [(9, 0)]

su(2) ← sp(1650)
so(3300)
su(3)
su(10)
su(3300)

[{⟨1, 1⟩},{⟨3299, 1⟩}], [{⟨1, 1⟩}], [(3299)], [{⟨1, 1⟩}], [(24, 7),(7, 24)],[{⟨2, 1⟩, ⟨3, 1⟩},{⟨7, 1⟩, ⟨8, 1⟩}]

su(2), so(5)
so(3311) ← su(3311)

[{⟨1, 1⟩},{⟨3310, 1⟩}],[{⟨1, 1⟩}],[(3310)],[(20, 0)]

su(2) ← sp(1656)
so(3312)
su(3)
su(3312)

[{⟨1, 1⟩},{⟨3311, 1⟩}], [{⟨1, 1⟩}], [(3311)], [{⟨1, 1⟩}], [(22, 8),(8, 22)]

su(2) ← so(3315)
su(3)
su(3)
su(3315)

[{⟨1, 1⟩},{⟨3314, 1⟩}], [{⟨1, 1⟩}], [(3314)], [(16, 12),(12, 16)],[(33, 4),(4, 33)]

su(2) ← sp(1660)
so(81), sp(41)
so(3320)
su(3320)

[{⟨1, 1⟩},{⟨3319, 1⟩}], [{⟨1, 1⟩}], [(3319)], [{⟨1, 1⟩}], [{⟨1, 2⟩}],[{⟨2, 1⟩}]

su(2), so(82)
so(3321)
su(3)
su(81)
su(82)
su(3321)

[{⟨1, 1⟩},{⟨3320, 1⟩}], [{⟨1, 1⟩}], [(3320)], [{⟨2, 1⟩}], [(80, 0),(0, 80)], [{⟨1, 2⟩},{⟨80, 2⟩}], [{⟨2, 1⟩},{⟨80, 1⟩}]

su(2), sp(2)
sp(1672)
so(3344)
su(3344)

[{⟨1, 1⟩},{⟨3343, 1⟩}], [{⟨1, 1⟩}], [(3343)], [(15, 2)], [{⟨1, 1⟩}]

su(2) ← sp(1677)
so(3354)
su(3)
su(3354)

[{⟨1, 1⟩},{⟨3353, 1⟩}], [{⟨1, 1⟩}], [(3353)], [{⟨1, 1⟩}], [(38, 3),(3, 38)]

su(2) ← sp(1680)
so(3360)
su(3)
su(4)
su(5)
su(5)
su(5)
su(5)
su(5)
su(7)
su(3360)

[{⟨1, 1⟩},{⟨3359, 1⟩}], [{⟨1, 1⟩}], [(3359)], [{⟨1, 1⟩}], [(15, 13),(13, 15)], [(4, 2, 3),(3, 2, 4)], [(0, 3, 2, 0),(0, 2, 3, 0)], [(1, 1, 3, 0),(0, 3, 1, 1)], [(1, 5, 0, 0),(0, 0, 5, 1)], [(3, 2, 0, 1),(1, 0, 2, 3)],[(5, 0, 0, 3),(3, 0, 0, 5)],[{⟨2, 2⟩, ⟨5, 1⟩},{⟨2, 1⟩, ⟨5, 2⟩}]

su(2), su(58)
so(3363)
su(3)
su(3363)

[{⟨1, 1⟩},{⟨3362, 1⟩}], [{⟨1, 1⟩}], [(3362)], [{⟨1, 1⟩, ⟨57, 1⟩}],[(56, 1),(1, 56)]

su(2) ← sp(1683)
so(7) ← so(3366)
su(3366)

[{⟨1, 1⟩},{⟨3365, 1⟩}], [{⟨1, 1⟩}], [(3365)], [{⟨1, 1⟩}], [(5, 1, 0)]

su(2), su(3), so(7)
so(3375)
su(4)
su(3375)

[{⟨1, 1⟩},{⟨3374, 1⟩}], [{⟨1, 1⟩}], [(3374)], [(14, 14)], [(4, 0, 2)],[(8, 0, 4),(4, 0, 8)]

su(2) ← so(3381)
su(3)
su(3381)

[{⟨1, 1⟩},{⟨3380, 1⟩}], [{⟨1, 1⟩}], [(3380)], [(45, 2),(2, 45)]

su(2) ← sp(1701)
so(82) ← so(3402)
su(7)
su(9)
su(3402)

[{⟨1, 1⟩},{⟨3401, 1⟩}], [{⟨1, 1⟩}], [(3401)], [{⟨1, 1⟩}], [{⟨1, 2⟩}], [{⟨1, 1⟩, ⟨3, 1⟩, ⟨5, 1⟩},{⟨2, 1⟩, ⟨4, 1⟩, ⟨6, 1⟩}],[{⟨2, 1⟩, ⟨4, 1⟩},{⟨5, 1⟩, ⟨7, 1⟩}]

su(2), sp(41)
so(83)
so(3403)
su(3)
su(82)
su(83)
su(3403)

[{⟨1, 1⟩},{⟨3402, 1⟩}], [{⟨1, 1⟩}], [(3402)], [{⟨2, 1⟩}], [{⟨1, 2⟩}], [(81, 0),(0, 81)], [{⟨1, 2⟩},{⟨81, 2⟩}], [{⟨2, 1⟩},{⟨81, 1⟩}]

su(2) ← sp(1705)
so(3410) ← su(3410)
su(3)

[{⟨1, 1⟩},{⟨3409, 1⟩}], [{⟨1, 1⟩}], [(3409)], [{⟨1, 1⟩}], [(19, 10),(10, 19)]

---

su(2) ← sp(1715)
so(3430) ← su(3430)
su(3)

[{⟨1, 1⟩},{⟨3429, 1⟩}], [{⟨1, 1⟩}], [(3429)], [{⟨1, 1⟩}], [(27, 6),(6, 27)]

---

su(2), su(14), sp(4) ← sp(1716)
sp(1716), so(3432) ← su(3432)
su(8)

[{⟨1, 1⟩},{⟨3431, 1⟩}], [{⟨1, 1⟩}], [(3431)], [{⟨7, 1⟩}], [(7, 0, 0, 0)],[{⟨1, 1⟩}],[{⟨1, 7⟩},{⟨7, 7⟩}]

---

su(2) ← so(3441) ← su(3441)
su(3)

[{⟨1, 1⟩},{⟨3440, 1⟩}], [{⟨1, 1⟩}], [(3440)], [(30, 5),(5, 30)]

---

su(2) ← so(3465) ← su(3465)
su(4)
su(5)
su(6)
su(6)
su(9)
su(11)

[{⟨1, 1⟩},{⟨3464, 1⟩}], [{⟨1, 1⟩}], [(3464)], [(8, 1, 2),(2, 1, 8)], [(5, 0, 1, 1),(1, 1, 0, 5)], [(5, 0, 1, 0, 0),(0, 0, 1, 0, 5)], [(6, 1, 0, 0, 0),(0, 0, 0, 1, 6)], [{⟨1, 2⟩, ⟨6, 1⟩},{⟨3, 1⟩, ⟨8, 2⟩}],[{⟨1, 1⟩, ⟨7, 1⟩},{⟨4, 1⟩, ⟨10, 1⟩}]

---

su(2) ← sp(1740)
su(59) ← so(3480) ← su(3480)
su(3)

[{⟨1, 1⟩},{⟨3479, 1⟩}], [{⟨1, 1⟩}], [(3479)], [{⟨1, 1⟩}], [{⟨1, 1⟩, ⟨58, 1⟩}],[(57, 1),(1, 57)]

---

su(2), so(83), sp(42) ← so(3485) ← su(3485)

[{⟨1, 1⟩},{⟨3484, 1⟩}], [{⟨1, 1⟩}], [(3484)], [{⟨1, 2⟩}], [{⟨2, 1⟩}]

---

su(2) ← sp(1743)
so(84) ← so(3486)
su(3) ← su(3486)
su(83)
su(84)

[{⟨1, 1⟩},{⟨3485, 1⟩}], [{⟨1, 1⟩}], [(3485)], [{⟨1, 1⟩}], [{⟨2, 1⟩}], [(82, 0),(0, 82)], [{⟨1, 2⟩},{⟨82, 2⟩}], [{⟨2, 1⟩},{⟨82, 1⟩}]

---

su(2) ← sp(1750)
so(3500)
su(3) ← su(3500)
su(4)
su(4)

[{⟨1, 1⟩},{⟨3499, 1⟩}], [{⟨1, 1⟩}], [(3499)], [{⟨1, 1⟩}], [(34, 4),(4, 34)],[(4, 4, 1),(1, 4, 4)],[(9, 3, 0),(0, 3, 9)]

---

su(2) ← sp(1755)
so(3510)
su(4) ← su(3510)
su(5)
su(11)

[{⟨1, 1⟩},{⟨3509, 1⟩}], [{⟨1, 1⟩}], [(3509)], [{⟨1, 1⟩}], [(2, 8, 0),(0, 8, 2)], [(8, 0, 1, 0),(0, 1, 0, 8)], [{⟨1, 2⟩, ⟨9, 1⟩},{⟨2, 1⟩, ⟨10, 2⟩}]

---

su(2), so(11), sp(2), sp(2), sp(4), sp(11) ← sp(1760)
sp(1760) ← su(3520)
so(22) ← so(3520)
su(3)
su(3)
su(4)

[{⟨1, 1⟩},{⟨3519, 1⟩}], [{⟨1, 1⟩}], [(3519)], [(0, 0, 1, 0, 1)], [(9, 5)], [(19, 1)], [(3, 0, 0, 1)], [{⟨1, 1⟩, ⟨2, 1⟩}], [{⟨1, 1⟩}],[{⟨1, 1⟩, ⟨2, 1⟩}],[(21, 9),(9, 21)],[(39, 3),(3, 39)],[(10, 0, 3),(3, 0, 10)]

---

su(2) ← so(3525) ← su(3525)
su(3)

[{⟨1, 1⟩},{⟨3524, 1⟩}], [{⟨1, 1⟩}], [(3524)], [(46, 2),(2, 46)]

---

su(2) ← sp(1764)
sp(3) ← so(3528) ← su(3528)
su(7)

[{⟨1, 1⟩},{⟨3527, 1⟩}], [{⟨1, 1⟩}], [(3527)], [{⟨1, 1⟩}], [(0, 5, 0)],[{⟨2, 2⟩, ⟨3, 1⟩},{⟨4, 1⟩, ⟨5, 2⟩}]

---

su(2) ← sp(1767)
so(3534) ← su(3534)
su(3)

[{⟨1, 1⟩},{⟨3533, 1⟩}], [{⟨1, 1⟩}], [(3533)], [{⟨1, 1⟩}], [(18, 11),(11, 18)]

---

su(2) ← sp(1768)
so(3536) ← su(3536)
su(3)
su(4)

[{⟨1, 1⟩},{⟨3535, 1⟩}], [{⟨1, 1⟩}], [(3535)], [{⟨1, 1⟩}], [(25, 7),(7, 25)],[(12, 2, 0),(0, 2, 12)]

---

su(2) ← sp(1771)
$\mathfrak{g}_2$ ← so(3542) ← su(3542)
su(22)

[{⟨1, 1⟩},{⟨3541, 1⟩}], [{⟨1, 1⟩}], [(3541)], [{⟨1, 1⟩}], [(0, 6)],[{⟨1, 1⟩, ⟨2, 1⟩},{⟨20, 1⟩, ⟨21, 1⟩}]

---

su(2) ← sp(1782)
so(3564) ← su(3564)
su(3)

[{⟨1, 1⟩},{⟨3563, 1⟩}], [{⟨1, 1⟩}], [(3563)], [{⟨1, 1⟩}], [(23, 8),(8, 23)]

---

su(2), so(84) ← so(3569) ← su(3569)

[{⟨1, 1⟩},{⟨3568, 1⟩}],[{⟨1, 1⟩}],[(3568)],[{⟨1, 2⟩}]

---

su(2) ← sp(1785)
so(85), sp(42) ← so(3570)
so(3570) ← su(3570)
su(3)
su(84)
su(85)

[{⟨1, 1⟩},{⟨3569, 1⟩}], [{⟨1, 1⟩}], [(3569)], [{⟨1, 1⟩}], [{⟨2, 1⟩}], [{⟨1, 2⟩}], [(83, 0),(0, 83)], [{⟨1, 2⟩},{⟨83, 2⟩}],[{⟨2, 1⟩},{⟨83, 1⟩}]

---

su(2), sp(2) ← sp(1792)
su(8), so(7) ← so(3584)
sp(1792), so(3584) ← su(3584)
su(4)

[{⟨1, 1⟩},{⟨3583, 1⟩}], [{⟨1, 1⟩}], [(3583)], [(3, 11)], [{⟨1, 1⟩}],[{⟨1, 1⟩, ⟨4, 1⟩, ⟨7, 1⟩}],[(3, 1, 1)],[(11, 1, 1),(1, 1, 11)]

---

su(2) ← so(3591)
su(4) ← su(3591)
su(19)

[{⟨1, 1⟩},{⟨3590, 1⟩}], [{⟨1, 1⟩}], [(3590)], [(17, 0, 1),(1, 0, 17)],[{⟨1, 2⟩, ⟨18, 1⟩},{⟨1, 1⟩, ⟨18, 2⟩}]

---

su(2), su(60) ← so(3599) ← su(3599)
su(3)

[{⟨1, 1⟩},{⟨3598, 1⟩}], [{⟨1, 1⟩}], [(3598)], [{⟨1, 1⟩, ⟨59, 1⟩}],[(58, 1),(1, 58)]

---

su(2), so(27) ← so(3627) ← su(3627)
su(3)

[{⟨1, 1⟩},{⟨3626, 1⟩}], [{⟨1, 1⟩}], [(3626)], [{⟨1, 3⟩}], [(17, 12),(12, 17)]

---

su(2), sp(3) ← sp(1820)
so(3640)
su(4)
su(4) ← su(3640)
su(4)
su(5)
su(13)

[{⟨1, 1⟩},{⟨3639, 1⟩}], [{⟨1, 1⟩}], [(3639)], [(6, 0, 1)], [{⟨1, 1⟩}], [(4, 6, 0),(0, 6, 4)], [(5, 1, 4),(4, 1, 5)], [(7, 4, 0),(0, 4, 7)], [(9, 1, 0, 0),(0, 0, 1, 9)], [{⟨1, 1⟩, ⟨10, 1⟩},{⟨3, 1⟩, ⟨12, 1⟩}]

---

su(2) ← sp(1824)
so(3648) ← su(3648)
su(3)

[{⟨1, 1⟩},{⟨3647, 1⟩}], [{⟨1, 1⟩}], [(3647)], [{⟨1, 1⟩}], [(31, 5),(5, 31)]

---

su(2) ← sp(1827)
so(5), so(29), so(85), sp(43) ← so(3654)
so(3654) ← su(3654)
su(3)
su(4)
su(27)
su(29)

[{⟨1, 1⟩},{⟨3653, 1⟩}], [{⟨1, 1⟩}], [(3653)], [{⟨1, 1⟩}], [(0, 26)], [{⟨3, 1⟩}], [{⟨1, 2⟩}], [{⟨2, 1⟩}], [(28, 6),(6, 28)], [(26, 0, 0),(0, 0, 26)], [{⟨1, 3⟩},{⟨26, 3⟩}], [{⟨3, 1⟩},{⟨26, 1⟩}]

---

su(2), so(86) ← so(3655)
so(3655) ← su(3655)
su(3)
su(85)
su(86)

[{⟨1, 1⟩},{⟨3654, 1⟩}], [{⟨1, 1⟩}], [(3654)], [{⟨2, 1⟩}], [(84, 0),(0, 84)], [{⟨1, 2⟩},{⟨84, 2⟩}], [{⟨2, 1⟩},{⟨84, 1⟩}]

---

su(2) ← sp(1836)
so(3672) ← su(3672)
su(3)

[{⟨1, 1⟩},{⟨3671, 1⟩}], [{⟨1, 1⟩}], [(3671)], [{⟨1, 1⟩}], [(47, 2),(2, 47)]

su(2)
su(5)
so(3675)
su(6)
su(5) su(3675)
so(8)
su(6)

[{⟨1, 1⟩},{⟨3674, 1⟩}], [{⟨1, 1⟩}], [(3674)], [(4, 0, 0, 4)], [(1, 1, 0, 1, 1)], [(3, 0, 1, 1),(1, 0, 3, 1),(1, 0, 1, 3)], [(1, 2, 1, 1),(1, 1, 2, 1)], [(2, 1, 0, 0, 2),(2, 0, 0, 1, 2)]

---

su(2)
so(3689)
so(5) su(3689)
su(3)

[{⟨1, 1⟩},{⟨3688, 1⟩}], [{⟨1, 1⟩}], [(3688)], [(13, 2)], [(16, 13),(13, 16)]

---

su(2) ⟵ sp(1845)
so(3690) su(3690)
su(3)
su(3)

[{⟨1, 1⟩},{⟨3689, 1⟩}], [{⟨1, 1⟩}], [(3689)], [{⟨1, 1⟩}], [(35, 4),(4, 35)],[(40, 3),(3, 40)]

---

su(2)
sp(2) sp(1848)
sp(4)
so(7)
sp(4) su(3696)
so(3696)
so(8)
su(3)
so(8)
so(10)
so(10)

[{⟨1, 1⟩},{⟨3695, 1⟩}], [{⟨1, 1⟩}], [(3695)], [(13, 3)], [(1, 0, 0, 2)], [{⟨1, 1⟩}], [(6, 0, 1)], [(3, 0, 1, 0)], [(4, 1, 0, 0), (0, 1, 4, 0),(0, 1, 0, 4)], [(5, 0, 1, 0),(5, 0, 0, 1),(1, 0, 5, 0),(1, 0, 0, 5),(0, 0, 5, 1),(0, 0, 1, 5)], [(20, 10),(10, 20)], [(0, 1, 0, 2, 0),(0, 1, 0, 0, 2)], [(1, 1, 0, 1, 0),(1, 1, 0, 0, 1)]

---

su(2) ⟵ sp(1860)
su(61) ⟵ so(3720) su(3720)
su(3)
su(3)

[{⟨1, 1⟩},{⟨3719, 1⟩}], [{⟨1, 1⟩}], [(3719)], [{⟨1, 1⟩}], [{⟨1, 1⟩, ⟨60, 1⟩}],[(15, 14),(14, 15)],[(59, 1),(1, 59)]

---

su(2)
sp(1870)
sp(2) su(3740)
so(16)
so(3740)
so(86)

[{⟨1, 1⟩},{⟨3739, 1⟩}], [{⟨1, 1⟩}], [(3739)], [(11, 4)], [{⟨1, 1⟩}],[{⟨1, 4⟩}],[{⟨1, 2⟩}]

---

su(2)
so(87) so(3741)
sp(43) su(3)
su(3741)
su(86)
su(87)

[{⟨1, 1⟩},{⟨3740, 1⟩}], [{⟨1, 1⟩}], [(3740)], [{⟨2, 1⟩}], [{⟨1, 2⟩}], [(85, 0),(0, 85)], [{⟨1, 2⟩},{⟨85, 2⟩}], [{⟨2, 1⟩},{⟨85, 1⟩}]

---

su(2)
sp(1872)
sp(3)
so(3744) su(3744)
su(4)

[{⟨1, 1⟩},{⟨3743, 1⟩}], [{⟨1, 1⟩}], [(3743)], [(2, 0, 3)], [{⟨1, 1⟩}],[(3, 7, 0),(0, 7, 3)]

---

su(2) ⟵ sp(1875)
so(3750) su(3750)
su(5)

[{⟨1, 1⟩},{⟨3749, 1⟩}], [{⟨1, 1⟩}], [(3749)], [{⟨1, 1⟩}], [(3, 0, 3, 0),(0, 3, 0, 3)]

---

su(2) ⟵ sp(1890)
so(3780)
su(3)
su(4)
su(4)
su(4)
su(4) su(3780)
su(4)
su(4)
su(5)
su(9)
su(20)

[{⟨1, 1⟩},{⟨3779, 1⟩}], [{⟨1, 1⟩}], [(3779)], [{⟨1, 1⟩}], [(26, 7),(7, 26)], [(2, 6, 1),(1, 6, 2)], [(4, 3, 2),(2, 3, 4)], [(7, 0, 5),(5, 0, 7)], [(8, 2, 1),(1, 2, 8)], [(13, 0, 2),(2, 0, 13)], [(17, 1, 0),(0, 1, 17)], [(1, 2, 2, 0),(0, 2, 2, 1)], [{⟨2, 1⟩, ⟨5, 1⟩},{⟨4, 1⟩, ⟨7, 1⟩}], [{⟨1, 1⟩, ⟨18, 1⟩}, {⟨2, 1⟩, ⟨19, 1⟩}]

---

su(2)
so(3795)
so(5) su(3795)
su(3)

[{⟨1, 1⟩},{⟨3794, 1⟩}], [{⟨1, 1⟩}], [(3794)], [(21, 0)], [(22, 9),(9, 22)]

---

su(2)
sp(1904)
sp(8) su(3808)
so(3808)

[{⟨1, 1⟩},{⟨3807, 1⟩}], [{⟨1, 1⟩}], [(3807)], [{⟨5, 1⟩}], [{⟨1, 1⟩}]

---

su(2) ⟵ sp(1911)
so(3822) su(3822)
su(3)

[{⟨1, 1⟩},{⟨3821, 1⟩}], [{⟨1, 1⟩}], [(3821)], [{⟨1, 1⟩}], [(48, 2),(2, 48)]

---

su(2) ⟵ so(3825)
su(3825)
su(3)

[{⟨1, 1⟩},{⟨3824, 1⟩}], [{⟨1, 1⟩}], [(3824)], [(24, 8),(8, 24)]

---

su(2)
so(87) so(3827) ⟵ su(3827)
sp(44)

[{⟨1, 1⟩},{⟨3826, 1⟩}], [{⟨1, 1⟩}], [(3826)], [{⟨1, 2⟩}], [{⟨2, 1⟩}]

---

su(2) ⟵ sp(1914)
so(88) ⟵ so(3828)
su(3) su(3828)
su(87)
su(88)

[{⟨1, 1⟩},{⟨3827, 1⟩}], [{⟨1, 1⟩}], [(3827)], [{⟨1, 1⟩}], [{⟨2, 1⟩}], [(86, 0),(0, 86)], [{⟨1, 2⟩},{⟨86, 2⟩}], [{⟨2, 1⟩},{⟨86, 1⟩}]

---

su(2) ⟵ sp(1920)
so(3840)
su(3) su(3840)
su(4)

[{⟨1, 1⟩},{⟨3839, 1⟩}], [{⟨1, 1⟩}], [(3839)], [{⟨1, 1⟩}], [(19, 11),(11, 19)],[(3, 5, 1),(1, 5, 3)]

---

su(2)
so(3843)
su(62) su(3843)
su(3)

[{⟨1, 1⟩},{⟨3842, 1⟩}], [{⟨1, 1⟩}], [(3842)], [{⟨1, 1⟩, ⟨61, 1⟩}],[(60, 1),(1, 60)]

---

su(2) ⟵ sp(1925)
so(3850)
su(5) su(3850)
su(5)
su(7)

[{⟨1, 1⟩},{⟨3849, 1⟩}], [{⟨1, 1⟩}], [(3849)], [{⟨1, 1⟩}], [(5, 0, 2, 0),(0, 2, 0, 5)],[(6, 2, 0, 0),(0, 0, 2, 6)],[{⟨1, 4⟩, ⟨5, 1⟩},{⟨2, 1⟩, ⟨6, 4⟩}]

---

su(2) ⟵ so(3861)
su(3861)
su(3)

[{⟨1, 1⟩},{⟨3860, 1⟩}], [{⟨1, 1⟩}], [(3860)], [(32, 5),(5, 32)]

---

su(2) ⟵ sp(1932)
so(5) ⟵ so(3864) su(3864)
su(3)

[{⟨1, 1⟩},{⟨3863, 1⟩}], [{⟨1, 1⟩}], [(3863)], [{⟨1, 1⟩}], [(6, 8)],[(41, 3),(3, 41)]

---

su(2)
so(3875) ⟵ su(3875)
$\mathfrak{e}_8$

[{⟨1, 1⟩},{⟨3874, 1⟩}],[{⟨1, 1⟩}],[(3874)],[{⟨1, 1⟩}]

---

su(2)
sp(1938)
sp(2)
so(19)
so(3876)
sp(8) su(3876)
su(5)
su(16)
su(19)

[{⟨1, 1⟩},{⟨3875, 1⟩}], [{⟨1, 1⟩}], [(3875)], [(1, 16)], [{⟨1, 1⟩}], [{⟨4, 1⟩}], [{⟨1, 4⟩}], [(15, 0, 0, 0),(0, 0, 0, 15)],[{⟨1, 4⟩},{⟨15, 4⟩}],[{⟨4, 1⟩},{⟨15, 1⟩}]

---

su(2) ⟵ so(3885)
su(3) su(3885)
su(3)

[{⟨1, 1⟩},{⟨3884, 1⟩}], [{⟨1, 1⟩}], [(3884)], [(29, 6),(6, 29)],[(36, 4),(4, 36)]

---

su(2) ⟵ sp(1950)
so(9) su(3900)
sp(3) so(3900)
sp(7) su(5)

[{⟨1, 1⟩},{⟨3899, 1⟩}], [{⟨1, 1⟩}], [(3899)], [{⟨1, 1⟩}], [(2, 0, 0, 2)], [(4, 2, 0)], [{⟨1, 1⟩, ⟨3, 1⟩}], [(7, 0, 0, 2),(2, 0, 0, 7)]

---

su(2) ⟵ sp(1955)
su(3910)
so(5) ⟵ so(3910)

[{⟨1, 1⟩},{⟨3909, 1⟩}], [{⟨1, 1⟩}], [(3909)], [{⟨1, 1⟩}], [(2, 16)]

---

su(2)
so(3915) ⟵ su(3915)
so(88)

[{⟨1, 1⟩},{⟨3914, 1⟩}],[{⟨1, 1⟩}],[(3914)],[{⟨1, 2⟩}]

---

su(2) ⟵ sp(1958)
so(89)
so(3916)
sp(44) su(3916)
su(3)
su(88)
su(89)

[{⟨1, 1⟩},{⟨3915, 1⟩}], [{⟨1, 1⟩}], [(3915)], [{⟨1, 1⟩}], [{⟨2, 1⟩}], [{⟨1, 2⟩}], [(87, 0),(0, 87)], [{⟨1, 2⟩},{⟨87, 2⟩}],[{⟨2, 1⟩},{⟨87, 1⟩}]

---

su(2) ⟵ sp(1960)
su(3920)
so(6) ⟵ so(3920)

[{⟨1, 1⟩},{⟨3919, 1⟩}], [{⟨1, 1⟩}], [(3919)], [{⟨1, 1⟩}],

[(0, 6, 6)]

---

su(3927) → so(3927) → su(2), so(13)

[{⟨1, 1⟩},{⟨3926, 1⟩}], [{⟨1, 1⟩}], [(3926)], [{⟨1, 2⟩, ⟨2, 1⟩}]

---

su(3952) → sp(1976) → su(2); su(3952) → so(3952); su(3952) → su(3)

[{⟨1, 1⟩},{⟨3951, 1⟩}], [{⟨1, 1⟩}], [(3951)], [{⟨1, 1⟩}], [(18, 12),(12, 18)]

---

su(3960) → sp(1980) → su(2); su(3960) → so(3960) → so(5)

[{⟨1, 1⟩},{⟨3959, 1⟩}], [{⟨1, 1⟩}], [(3959)], [{⟨1, 1⟩}], [(10, 4)]

---

su(3968) → sp(1984) → su(2); su(3968) → so(3968) → su(63); su(3968) → su(3)

[{⟨1, 1⟩},{⟨3967, 1⟩}], [{⟨1, 1⟩}], [(3967)], [{⟨1, 1⟩}], [{⟨1, 1⟩, ⟨62, 1⟩}],[(61, 1),(1, 61)]

---

su(3969) → so(3969) → su(2), su(6)

[{⟨1, 1⟩},{⟨3968, 1⟩}], [{⟨1, 1⟩}], [(3968)], [(1, 0, 2, 0, 1)]

---

su(3975) → so(3975) → su(2); su(3975) → su(3)

[{⟨1, 1⟩},{⟨3974, 1⟩}], [{⟨1, 1⟩}], [(3974)], [(49, 2),(2, 49)]

---

su(3993) → so(3993) → su(2); su(3993) → su(3)

[{⟨1, 1⟩},{⟨3992, 1⟩}], [{⟨1, 1⟩}], [(3992)], [(21, 10), (10, 21)]

---

su(4000) → sp(2000) → su(2); su(4000) → so(4000); su(4000) → su(5)

[{⟨1, 1⟩},{⟨3999, 1⟩}], [{⟨1, 1⟩}], [(3999)], [{⟨1, 1⟩}], [(3, 0, 2, 1),(1, 2, 0, 3)]

---

su(4004) → sp(2002) → su(2), sp(3); su(4004) → so(4004) → so(9), so(89), sp(5), sp(45), so(12), so(14); su(4004) → su(4); su(4004) → su(4)

[{⟨1, 1⟩},{⟨4003, 1⟩}], [{⟨1, 1⟩}], [(4003)], [(1, 0, 4)], [{⟨1, 1⟩}], [(0, 3, 0, 0)], [{⟨1, 2⟩}], [(0, 0, 2, 0, 0)], [{⟨2, 1⟩}],[{⟨1, 5⟩}],[{⟨1, 1⟩, ⟨3, 1⟩}],[(1, 10, 0),(0, 10, 1)],[(6, 3, 1),(1, 3, 6)]

---

su(4005) → so(4005) → su(2), so(90); su(4005) → su(3); su(4005) → su(89); su(4005) → su(90)

[{⟨1, 1⟩},{⟨4004, 1⟩}], [{⟨1, 1⟩}], [(4004)], [{⟨2, 1⟩}], [(88, 0),(0, 88)], [{⟨1, 2⟩},{⟨88, 2⟩}], [{⟨2, 1⟩},{⟨88, 1⟩}]

---

su(4025) → so(4025) → su(2), so(5), so(23)

[{⟨1, 1⟩},{⟨4024, 1⟩}], [{⟨1, 1⟩}], [(4024)], [(1, 20)], [{⟨1, 1⟩, ⟨2, 1⟩}]

---

su(4030) → sp(2015) → su(2), sp(15); su(4030) → so(4030)

[{⟨1, 1⟩},{⟨4029, 1⟩}], [{⟨1, 1⟩}], [(4029)], [{⟨3, 1⟩}], [{⟨1, 1⟩}]

---

su(4032) → sp(2016) → su(2); su(4032) → so(4032) → so(28); su(4032) → su(3); su(4032) → su(3); su(4032) → su(8)

[{⟨1, 1⟩},{⟨4031, 1⟩}], [{⟨1, 1⟩}], [(4031)], [{⟨1, 1⟩}], [{⟨1, 3⟩}], [(17, 13),(13, 17)], [(27, 7),(7, 27)], [{⟨1, 3⟩, ⟨7, 2⟩},{⟨1, 2⟩, ⟨7, 3⟩}]

---

su(4042) → sp(2021) → su(2); su(4042) → so(4042); su(4042) → su(3)

[{⟨1, 1⟩},{⟨4041, 1⟩}], [{⟨1, 1⟩}], [(4041)], [{⟨1, 1⟩}], [(42, 3),(3, 42)]

---

su(4048) → sp(2024) → su(2); su(4048) → so(4048); su(4048) → su(23)

[{⟨1, 1⟩},{⟨4047, 1⟩}], [{⟨1, 1⟩}], [(4047)], [{⟨1, 1⟩}], [{⟨1, 1⟩, ⟨2, 1⟩},{⟨21, 1⟩, ⟨22, 1⟩}]

---

su(4060) → sp(2030) → su(2), sp(2), sp(14); su(4060) → so(4060) → so(30); su(4060) → su(4); su(4060) → su(28); su(4060) → su(30)

[{⟨1, 1⟩},{⟨4059, 1⟩}], [{⟨1, 1⟩}], [(4059)], [(27, 0)], [{⟨1, 3⟩}], [{⟨1, 1⟩}], [{⟨3, 1⟩}], [(27, 0, 0),(0, 0, 27)], [{⟨1, 3⟩},{⟨27, 3⟩}],[{⟨3, 1⟩},{⟨27, 1⟩}]

---

su(4080) → sp(2040) → su(2); su(4080) → so(4080) → so(15); su(4080) → su(3); su(4080) → su(3); su(4080) → su(3)

[{⟨1, 1⟩},{⟨4079, 1⟩}], [{⟨1, 1⟩}], [(4079)], [{⟨1, 1⟩}], [{⟨2, 2⟩}], [(16, 14),(14, 16)], [(23, 9),(9, 23)], [(33, 5),(5, 33)]

---

su(4085) → so(4085) → su(2); su(4085) → su(3)

[{⟨1, 1⟩},{⟨4084, 1⟩}], [{⟨1, 1⟩}], [(4084)], [(37, 4),(4, 37)]

---

su(4094) → sp(2047) → su(2); su(4094) → so(4094) → so(90)

[{⟨1, 1⟩},{⟨4093, 1⟩}], [{⟨1, 1⟩}], [(4093)], [{⟨1, 1⟩}], [{⟨1, 2⟩}]

---

su(4095) → so(4095) → su(2), su(64), so(7), so(91), sp(45); su(4095) → su(3); su(4095) → su(3); su(4095) → su(3); su(4095) → su(4); su(4095) → su(90); su(4095) → su(91) → su(13), su(14)

[{⟨1, 1⟩},{⟨4094, 1⟩}], [{⟨1, 1⟩}], [(4094)], [{⟨1, 1⟩, ⟨63, 1⟩}], [(2, 0, 4)], [{⟨2, 1⟩}], [{⟨1, 2⟩}], [(25, 8),(8, 25)], [(62, 1),(1, 62)], [(89, 0),(0, 89)], [(6, 2, 2),(2, 2, 6)], [{⟨1, 2⟩},{⟨89, 2⟩}], [{⟨2, 1⟩},{⟨89, 1⟩}], [{⟨1, 2⟩, ⟨2, 1⟩},{⟨11, 1⟩, ⟨12, 2⟩}], [{⟨1, 1⟩, ⟨3, 1⟩},{⟨11, 1⟩, ⟨13, 1⟩}]

---

su(4096) → sp(2048) → su(2), sp(2); su(4096) → so(4096) → su(3), so(7), so(17), so(25), sp(4), so(6), so(8), f4, g2; su(4096) → so(26)

[{⟨1, 1⟩},{⟨4095, 1⟩}], [{⟨1, 1⟩}], [(4095)], [(7, 7)], [{⟨1, 1⟩}], [(15, 15)], [(1, 1, 3)], [{⟨1, 1⟩, ⟨8, 1⟩}], [{⟨12, 1⟩}],[(1, 1, 1, 0)],[(3, 3, 3)],[(1, 1, 1, 1)],[(0, 0, 1, 1)],[(3, 3)],[{⟨12, 1⟩},{⟨13, 1⟩}]

---

su(4116) → sp(2058) → su(2), sp(3); su(4116) → so(4116) → su(6); su(4116) → su(7)

[{⟨1, 1⟩},{⟨4115, 1⟩}], [{⟨1, 1⟩}], [(4115)], [(1, 4, 0)], [{⟨1, 1⟩}],[(0, 0, 4, 0, 0)],[{⟨3, 3⟩},{⟨4, 3⟩}]

---

su(4123) → so(4123) → su(2); su(4123) → su(3)

[{⟨1, 1⟩},{⟨4122, 1⟩}], [{⟨1, 1⟩}], [(4122)], [(30, 6),(6, 30)]

---

su(4125) → so(4125) → su(2), so(10); su(4125) → su(5)

[{⟨1, 1⟩},{⟨4124, 1⟩}], [{⟨1, 1⟩}], [(4124)], [(0, 0, 2, 0, 0)],[(4, 3, 0, 0),(0, 0, 3, 4)]

---

su(4131) → so(4131) → su(2); su(4131) → su(3)

[{⟨1, 1⟩},{⟨4130, 1⟩}], [{⟨1, 1⟩}], [(4130)], [(50, 2),(2, 50)]

---

su(4158) → sp(2079) → su(2); su(4158) → so(4158) → so(9); su(4158) → su(3)

[{⟨1, 1⟩},{⟨4157, 1⟩}], [{⟨1, 1⟩}], [(4157)], [{⟨1, 1⟩}], [(0, 0, 1, 2)],[(20, 11),(11, 20)]

---

su(4160) → sp(2080) → su(2), so(13), sp(2); su(4160) → so(4160)

[{⟨1, 1⟩},{⟨4159, 1⟩}], [{⟨1, 1⟩}], [(4159)], [{⟨2, 1⟩, ⟨6, 1⟩}],[(5, 9)],[{⟨1, 1⟩}]

---

su(4180) → sp(2090) → su(2); su(4180) → so(4180); su(4180) → su(4); su(4180) → su(20)

[{⟨1, 1⟩},{⟨4179, 1⟩}], [{⟨1, 1⟩}], [(4179)], [{⟨1, 1⟩}], [(18, 0, 1),(1, 0, 18)], [{⟨1, 2⟩, ⟨19, 1⟩},{⟨1, 1⟩, ⟨19, 2⟩}]

---

su(4185) → so(4185) → su(2), so(91), sp(46)

[{⟨1, 1⟩},{⟨4184, 1⟩}], [{⟨1, 1⟩}], [(4184)], [{⟨1, 2⟩}], [{⟨2, 1⟩}]

---

su(2) ← sp(2093)
so(92) ← so(4186)
su(3), su(91), su(92)
→ su(4186)

[{⟨1, 1⟩},{⟨4185, 1⟩}], [{⟨1, 1⟩}], [(4185)], [{⟨1, 1⟩}], [{⟨2, 1⟩}], [(90, 0),(0, 90)], [{⟨1, 2⟩},{⟨90, 2⟩}], [{⟨2, 1⟩},{⟨90, 1⟩}]

---

su(2), sp(4) → sp(2100)
so(5), so(7), so(6) → so(4200)
su(6), su(8), su(15)
→ su(4200)

[{⟨1, 1⟩},{⟨4199, 1⟩}], [{⟨1, 1⟩}], [(4199)], [(1, 1, 0, 1)], [{⟨1, 1⟩}], [(8, 6)], [(3, 0, 3)], [(13, 0, 0)], [(3, 0, 1, 0, 1),(1, 0, 1, 0, 3)], [{⟨1, 1⟩, ⟨2, 1⟩, ⟨6, 1⟩},{⟨2, 1⟩, ⟨6, 1⟩, ⟨7, 1⟩}],[{⟨2, 2⟩},{⟨13, 2⟩}]

---

su(2), sp(5) → sp(2106)
su(12) ← so(4212)
→ su(4212)

[{⟨1, 1⟩},{⟨4211, 1⟩}], [{⟨1, 1⟩}], [(4211)], [(2, 0, 1, 0, 0)],[{⟨1, 1⟩}],[{⟨2, 1⟩, ⟨10, 1⟩}]

---

su(2), so(11) ← so(12) → sp(2112)
su(65) ← so(4224)
su(3), su(3)
→ su(4224)

[{⟨1, 1⟩},{⟨4223, 1⟩}], [{⟨1, 1⟩}], [(4223)], [{⟨5, 3⟩},{⟨6, 3⟩}], [(0, 0, 0, 0, 3)], [{⟨1, 1⟩}], [{⟨1, 1⟩, ⟨64, 1⟩}], [(43, 3),(3, 43)],[(63, 1),(1, 63)]

---

su(2), su(11) → so(4235) ← su(4235)

[{⟨1, 1⟩},{⟨4234, 1⟩}], [{⟨1, 1⟩}], [(4234)], [{⟨1, 2⟩, ⟨10, 2⟩}]

---

su(2), so(92) → so(4277) ← su(4277)

[{⟨1, 1⟩},{⟨4276, 1⟩}],[{⟨1, 1⟩}],[(4276)],[{⟨1, 2⟩}]

---

su(2) ← sp(2139)
so(93), sp(46) → so(4278)
su(3), su(92), su(93)
→ su(4278)

[{⟨1, 1⟩},{⟨4277, 1⟩}], [{⟨1, 1⟩}], [(4277)], [{⟨1, 1⟩}], [{⟨2, 1⟩}], [{⟨1, 2⟩}], [(91, 0),(0, 91)], [{⟨1, 2⟩},{⟨91, 2⟩}],[{⟨2, 1⟩},{⟨91, 1⟩}]

---

su(2) ← sp(2142)
so(4284)
su(4)
→ su(4284)

[{⟨1, 1⟩},{⟨4283, 1⟩}], [{⟨1, 1⟩}], [(4283)], [{⟨1, 1⟩}], [(13, 2, 0),(0, 2, 13)]

---

su(2), sp(5) → sp(2145)
so(11), sp(4), so(10) → so(4290)
su(3), su(3), su(3), su(5), su(6), su(9), su(12)
→ su(4290)

[{⟨1, 1⟩},{⟨4289, 1⟩}], [{⟨1, 1⟩}], [(4289)], [(0, 1, 0, 0, 1)], [{⟨1, 1⟩}], [(1, 0, 0, 0, 2)], [(4, 1, 0, 0)], [(6, 0, 0, 0)], [(19, 12),(12, 19)], [(38, 4),(4, 38)], [(51, 2),(2, 51)], [(10, 0, 0, 1),(1, 0, 0, 10)], [(7, 0, 0, 0, 1),(1, 0, 0, 0, 7)], [{⟨1, 4⟩, ⟨8, 1⟩},{⟨1, 1⟩, ⟨8, 4⟩}], [{⟨1, 3⟩, ⟨11, 1⟩},{⟨1, 1⟩, ⟨11, 3⟩}]

---

su(2) ← sp(2146)
so(4292)
su(3)
→ su(4292)

[{⟨1, 1⟩},{⟨4291, 1⟩}], [{⟨1, 1⟩}], [(4291)], [{⟨1, 1⟩}], [(28, 7),(7, 28)]

---

su(2), so(5) → so(4301)
su(3)
→ su(4301)

[{⟨1, 1⟩},{⟨4300, 1⟩}], [{⟨1, 1⟩}], [(4300)], [(5, 10)], [(22, 10),(10, 22)]

---

su(2) ← so(4305)
su(3)
→ su(4305)

[{⟨1, 1⟩},{⟨4304, 1⟩}], [{⟨1, 1⟩}], [(4304)], [(34, 5),(5, 34)]

---

su(2) ← sp(2156)
so(7), so(8), so(10) → so(4312)
→ su(4312)

[{⟨1, 1⟩},{⟨4311, 1⟩}], [{⟨1, 1⟩}], [(4311)], [{⟨1, 1⟩}], [(3, 2, 0)],[(2, 2, 0, 0),(0, 2, 2, 0),(0, 2, 0, 2)],[(2, 0, 1, 0, 0)]

---

su(2) ← sp(2160)
so(4320)
su(4)
→ su(4320)

[{⟨1, 1⟩},{⟨4319, 1⟩}], [{⟨1, 1⟩}], [(4319)], [{⟨1, 1⟩}], [(3, 4, 2),(2, 4, 3)]

---

su(2) ← sp(2162)
so(5) ← so(4324)
→ su(4324)

[{⟨1, 1⟩},{⟨4323, 1⟩}], [{⟨1, 1⟩}], [(4323)], [{⟨1, 1⟩}], [(22, 0)]

---

su(2) ← sp(2176)
so(4352)
so(18)
→ su(4352)

[{⟨1, 1⟩},{⟨4351, 1⟩}], [{⟨1, 1⟩}], [(4351)], [{⟨1, 1⟩}], [{⟨1, 1⟩, ⟨8, 1⟩},{⟨1, 1⟩, ⟨9, 1⟩}]

---

su(2), su(66) → so(4355)
su(3)
→ su(4355)

[{⟨1, 1⟩},{⟨4354, 1⟩}], [{⟨1, 1⟩}], [(4354)], [{⟨1, 1⟩, ⟨65, 1⟩}],[(64, 1),(1, 64)]

---

su(2), sp(3), sp(6), sp(6) → sp(2184)
so(16) ← so(4368)
su(3), su(6), su(12), su(16)
→ su(4368)

[{⟨1, 1⟩},{⟨4367, 1⟩}], [{⟨1, 1⟩}], [(4367)], [(11, 0, 0)], [{⟨1, 1⟩, ⟨4, 1⟩}], [{⟨1, 5⟩}], [{⟨1, 1⟩}], [{⟨5, 1⟩}], [(31, 6),(6, 31)], [(11, 0, 0, 0, 0),(0, 0, 0, 0, 11)], [{⟨1, 5⟩},{⟨11, 5⟩}],[{⟨5, 1⟩},{⟨11, 1⟩}]

---

su(2) ← sp(2185)
so(5), so(93), sp(47) → so(4370)
→ su(4370)

[{⟨1, 1⟩},{⟨4369, 1⟩}], [{⟨1, 1⟩}], [(4369)], [{⟨1, 1⟩}], [(3, 14)],[{⟨1, 2⟩}],[{⟨2, 1⟩}]

---

su(2), so(94) → so(4371)
su(3), su(93), su(94)
→ su(4371)

[{⟨1, 1⟩},{⟨4370, 1⟩}], [{⟨1, 1⟩}], [(4370)], [{⟨2, 1⟩}], [(92, 0),(0, 92)], [{⟨1, 2⟩},{⟨92, 2⟩}], [{⟨2, 1⟩},{⟨92, 1⟩}]

---

su(2) ← sp(2187)
so(6) ← so(4374)
su(3)
→ su(4374)

[{⟨1, 1⟩},{⟨4373, 1⟩}], [{⟨1, 1⟩}], [(4373)], [{⟨1, 1⟩}], [(5, 2, 2)],[(26, 8),(8, 26)]

---

su(2) ← so(4375)
su(3)
→ su(4375)

[{⟨1, 1⟩},{⟨4374, 1⟩}], [{⟨1, 1⟩}], [(4374)], [(24, 9),(9, 24)]

---

su(2) ← so(4389)
su(3), su(4), su(21)
→ su(4389)

[{⟨1, 1⟩},{⟨4388, 1⟩}], [{⟨1, 1⟩}], [(4388)], [(18, 13),(13, 18)], [(18, 1, 0),(0, 1, 18)], [{⟨1, 1⟩, ⟨19, 1⟩},{⟨2, 1⟩, ⟨20, 1⟩}]

---

su(2) ← sp(2200)
so(4400)
su(4), su(4), su(5)
→ su(4400)

[{⟨1, 1⟩},{⟨4399, 1⟩}], [{⟨1, 1⟩}], [(4399)], [{⟨1, 1⟩}], [(9, 0, 4),(4, 0, 9)], [(10, 3, 0),(0, 3, 10)], [(5, 1, 1, 0),(0, 1, 1, 5)]

---

su(2) ← sp(2205)
so(10) ← so(4410)
su(3), su(5), su(5), su(6), su(6), su(6), su(6), su(7)
→ su(4410)

[{⟨1, 1⟩},{⟨4409, 1⟩}], [{⟨1, 1⟩}], [(4409)], [{⟨1, 1⟩}], [(1, 2, 0, 0, 0)], [(44, 3),(3, 44)], [(1, 0, 5, 0),(0, 5, 0, 1)], [(2, 2, 0, 2),(2, 0, 2, 2)], [(1, 0, 3, 0, 0),(0, 0, 3, 0, 1)], [(1, 1, 0, 1),(1, 0, 1, 1, 1)], [(1, 2, 1, 0, 0),(0, 0, 1, 2, 1)], [(2, 3, 0, 0, 0),(0, 0, 0, 3, 2)], [{⟨1, 1⟩, ⟨3, 1⟩, ⟨4, 1⟩}, {⟨3, 1⟩, ⟨4, 1⟩, ⟨6, 1⟩}]

---

su(2), sp(2) ← sp(2210)
sp(2210), so(4420), su(4), su(4) ← su(4420)

[{⟨1, 1⟩},{⟨4419, 1⟩}], [{⟨1, 1⟩}], [(4419)], [(3, 12)], [{⟨1, 1⟩}], [(11, 0, 3),(3, 0, 11)], [(12, 1, 1),(1, 1, 12)]

---

su(2) ← sp(2226)
sp(2226), so(4452), su(3) ← su(4452)

[{⟨1, 1⟩},{⟨4451, 1⟩}], [{⟨1, 1⟩}], [(4451)], [{⟨1, 1⟩}], [(52, 2),(2, 52)]

---

su(2), so(5) ← so(4455)
so(4455), su(3) ← su(4455)

[{⟨1, 1⟩},{⟨4454, 1⟩}], [{⟨1, 1⟩}], [(4454)], [(14, 2)], [(17, 14),(14, 17)]

---

su(2) ← so(4459)
so(4459), su(4) ← su(4459)

[{⟨1, 1⟩},{⟨4458, 1⟩}], [{⟨1, 1⟩}], [(4458)], [(6, 5, 0),(0, 5, 6)]

---

su(2) ← sp(2232)
so(94) ← so(4464)
sp(2232), so(4464) ← su(4464)

[{⟨1, 1⟩},{⟨4463, 1⟩}], [{⟨1, 1⟩}], [(4463)], [{⟨1, 1⟩}], [{⟨1, 2⟩}]

---

su(2), so(95), sp(47) ← so(4465)
so(4465), su(3), su(94), su(95) ← su(4465)

[{⟨1, 1⟩},{⟨4464, 1⟩}], [{⟨1, 1⟩}], [(4464)], [{⟨2, 1⟩}], [{⟨1, 2⟩}], [(93, 0),(0, 93)], [{⟨1, 2⟩},{⟨93, 2⟩}], [{⟨2, 1⟩},{⟨93, 1⟩}]

---

su(2) ← sp(2233)
so(29) ← so(4466)
sp(2233), so(4466) ← su(4466)

[{⟨1, 1⟩},{⟨4465, 1⟩}], [{⟨1, 1⟩}], [(4465)], [{⟨1, 1⟩}], [{⟨1, 3⟩}]

---

su(2) ← sp(2240)
sp(2240), so(4480), su(4) ← su(4480)

[{⟨1, 1⟩},{⟨4479, 1⟩}], [{⟨1, 1⟩}], [(4479)], [{⟨1, 1⟩}], [(7, 1, 3),(3, 1, 7)]

---

su(2), so(5) ← so(4485) ← su(4485)

[{⟨1, 1⟩},{⟨4484, 1⟩}], [{⟨1, 1⟩}], [(4484)], [(4, 12)]

---

su(2) ← sp(2244)
su(67) ← so(4488)
sp(2244), so(4488), su(3), su(3), su(3) ← su(4488)

[{⟨1, 1⟩},{⟨4487, 1⟩}], [{⟨1, 1⟩}], [(4487)], [{⟨1, 1⟩}], [{⟨1, 1⟩, ⟨66, 1⟩}], [(16, 15),(15, 16)], [(21, 11),(11, 21)], [(65, 1),(1, 65)]

---

su(2), so(5), so(31) ← so(4495)
so(4495), su(4), su(29), su(31) ← su(4495)

[{⟨1, 1⟩},{⟨4494, 1⟩}], [{⟨1, 1⟩}], [(4494)], [(0, 28)], [{⟨3, 1⟩}], [(28, 0, 0),(0, 0, 28)], [{⟨1, 3⟩},{⟨28, 3⟩}], [{⟨3, 1⟩},{⟨28, 1⟩}]

---

su(2) ← sp(2250)
sp(2250), so(4500), su(3), su(4), su(6) ← su(4500)

[{⟨1, 1⟩},{⟨4499, 1⟩}], [{⟨1, 1⟩}], [(4499)], [{⟨1, 1⟩}], [(39, 4),(4, 39)], [(9, 1, 2),(2, 1, 9)], [(3, 0, 0, 2, 0),(0, 2, 0, 0, 3)]

---

su(2), sp(2) ← sp(2268)
so(8) ← so(4536)
sp(2268), so(4536), su(3), su(6), su(6) ← su(4536)

[{⟨1, 1⟩},{⟨4535, 1⟩}], [{⟨1, 1⟩}], [(4535)], [(17, 2)], [{⟨1, 1⟩}], [(2, 0, 2, 1),(2, 0, 1, 2),(1, 0, 2, 2)], [(35, 5),(5, 35)], [(1, 2, 0, 1, 0),(0, 1, 0, 2, 1)], [(5, 0, 0, 0, 2),(2, 0, 0, 0, 5)]

---

su(2) ← sp(2275)
so(7) ← so(4550)
sp(2275), so(4550) ← su(4550)

[{⟨1, 1⟩},{⟨4549, 1⟩}], [{⟨1, 1⟩}], [(4549)], [{⟨1, 1⟩}], [(2, 1, 2)]

---

su(2), so(95), sp(48) ← so(4559) ← su(4559)

[{⟨1, 1⟩},{⟨4558, 1⟩}], [{⟨1, 1⟩}], [(4558)], [{⟨1, 2⟩}], [{⟨2, 1⟩}]

---

su(2), sp(2) ← sp(2280)
so(96) ← so(4560)
sp(2280), so(4560), su(3), su(3), su(4), su(95), su(96) ← su(4560)

[{⟨1, 1⟩},{⟨4559, 1⟩}], [{⟨1, 1⟩}], [(4559)], [(1, 17)], [{⟨1, 1⟩}], [{⟨2, 1⟩}], [(29, 7),(7, 29)], [(94, 0),(0, 94)], [(14, 0, 2),(2, 0, 14)], [{⟨1, 2⟩},{⟨94, 2⟩}], [{⟨2, 1⟩},{⟨94, 1⟩}]

---

su(2), sp(2), sp(6), sp(12) ← sp(2288)
so(24) ← so(4576)
sp(2288), so(4576) ← su(4576)

[{⟨1, 1⟩},{⟨4575, 1⟩}], [{⟨1, 1⟩}], [(4575)], [(21, 1)], [{⟨1, 1⟩, ⟨6, 1⟩}], [{⟨1, 1⟩, ⟨2, 1⟩}], [{⟨1, 1⟩}], [{⟨1, 1⟩, ⟨2, 1⟩}]

---

su(2) ← sp(2300)
sp(2300), so(4600), su(3), su(24) ← su(4600)

[{⟨1, 1⟩},{⟨4599, 1⟩}], [{⟨1, 1⟩}], [(4599)], [{⟨1, 1⟩}], [(45, 3),(3, 45)], [{⟨1, 1⟩, ⟨2, 1⟩},{⟨22, 1⟩, ⟨23, 1⟩}]

---

su(2) ← sp(2304)
so(9), so(10) ← so(4608)
sp(2304), so(4608) ← su(4608)

[{⟨1, 1⟩},{⟨4607, 1⟩}], [{⟨1, 1⟩}], [(4607)], [{⟨1, 1⟩}], [(1, 0, 0, 3)], [(3, 1, 0, 0, 0)]

---

su(2) ← so(4617)
so(4617), su(3) ← su(4617)

[{⟨1, 1⟩},{⟨4616, 1⟩}], [{⟨1, 1⟩}], [(4616)], [(53, 2),(2, 53)]

---

su(2), sp(5) ← sp(2310)
sp(2310), so(4620), su(3), su(3), su(5), su(8), su(8), su(9), su(9), su(11) ← su(4620)

[{⟨1, 1⟩},{⟨4619, 1⟩}], [{⟨1, 1⟩}], [(4619)], [(1, 2, 0, 0, 0)], [{⟨1, 1⟩}], [(23, 10),(10, 23)], [(32, 6),(6, 32)], [(4, 1, 0, 2),(2, 0, 1, 4)], [{⟨1, 3⟩, ⟨3, 1⟩},{⟨5, 1⟩, ⟨7, 3⟩}], [{⟨1, 4⟩, ⟨2, 1⟩},{⟨6, 1⟩, ⟨7, 4⟩}], [{⟨1, 1⟩, ⟨7, 2⟩}, {⟨2, 2⟩, ⟨8, 1⟩}], [{⟨1, 2⟩, ⟨4, 1⟩},{⟨5, 1⟩, ⟨8, 2⟩}], [{⟨1, 1⟩, ⟨5, 1⟩},{⟨6, 1⟩, ⟨10, 1⟩}]

---

su(2), su(68) ← so(4623)
so(4623), su(3) ← su(4623)

[{⟨1, 1⟩},{⟨4622, 1⟩}], [{⟨1, 1⟩}], [(4622)], [{⟨1, 1⟩, ⟨67, 1⟩}], [(66, 1),(1, 66)]

---

su(2) ← so(4641)
so(4641), su(3) ← su(4641)

[{⟨1, 1⟩},{⟨4640, 1⟩}], [{⟨1, 1⟩}], [(4640)], [(20, 12),(12, 20)]

---

su(2), sp(10), so(96) ← so(4655) ← su(4655)

[{⟨1, 1⟩},{⟨4654, 1⟩}], [{⟨1, 1⟩}], [(4654)], [{⟨4, 1⟩}], [{⟨1, 2⟩}]

---

su(2) ← sp(2328)
so(97), sp(48) ← so(4656)
sp(2328), so(4656), su(3), su(96), su(97) ← su(4656)

[{⟨1, 1⟩},{⟨4655, 1⟩}], [{⟨1, 1⟩}], [(4655)], [{⟨1, 1⟩}], [{⟨2, 1⟩}], [{⟨1, 2⟩}], [(95, 0),(0, 95)], [{⟨1, 2⟩}, {⟨95, 2⟩}], [{⟨2, 1⟩},{⟨95, 1⟩}]

---

su(2) ← sp(2331)
sp(2331), so(4662), su(3) ← su(4662)

[{⟨1, 1⟩},{⟨4661, 1⟩}], [{⟨1, 1⟩}], [(4661)], [{⟨1, 1⟩}], [(27, 8),(8, 27)]

---

su(2) ← sp(2340)
sp(2340), so(4680), su(3) ← su(4680)

[{⟨1, 1⟩},{⟨4679, 1⟩}], [{⟨1, 1⟩}], [(4679)], [{⟨1, 1⟩}], [(25, 9),(9, 25)]

---

su(2) ← sp(2346)
so(17) ← so(4692)
sp(2346), so(4692) ← su(4692)

[{⟨1, 1⟩},{⟨4691, 1⟩}], [{⟨1, 1⟩}], [(4691)], [{⟨1, 1⟩}], [{⟨1, 4⟩}]

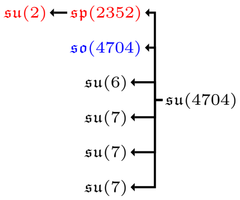


[{⟨1, 1⟩},{⟨4703, 1⟩}], [{⟨1, 1⟩}], [(4703)], [{⟨1, 1⟩}], [(0, 3, 1, 0, 0),(0, 0, 1, 3, 0)], [{⟨2, 2⟩, ⟨4, 1⟩},{⟨3, 1⟩, ⟨5, 2⟩}], [{⟨1, 1⟩, ⟨2, 3⟩},{⟨5, 3⟩, ⟨6, 1⟩}], [{⟨1, 2⟩, ⟨3, 1⟩, ⟨6, 1⟩},{⟨1, 1⟩, ⟨4, 1⟩, ⟨6, 2⟩}]

---

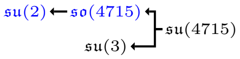


[{⟨1, 1⟩},{⟨4714, 1⟩}], [{⟨1, 1⟩}], [(4714)], [(40, 4),(4, 40)]

---

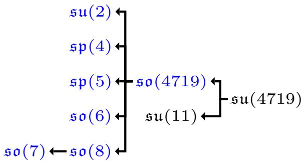


[{⟨1, 1⟩},{⟨4718, 1⟩}], [{⟨1, 1⟩}], [(4718)], [(0, 0, 0, 3)], [(0, 0, 0, 0, 2)], [(8, 1, 1)], [(8, 0, 0, 0),(0, 0, 8, 0),(0, 0, 0, 8)], [(0, 0, 8)], [{⟨1, 1⟩, ⟨2, 1⟩, ⟨10, 1⟩},{⟨1, 1⟩, ⟨9, 1⟩, ⟨10, 1⟩}]

---

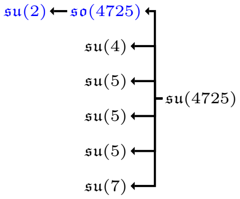


[{⟨1, 1⟩},{⟨4724, 1⟩}], [{⟨1, 1⟩}], [(4724)], [(8, 4, 0),(0, 4, 8)], [(2, 0, 4, 0),(0, 4, 0, 2)], [(3, 2, 1, 0),(0, 1, 2, 3)], [(6, 1, 0, 1),(1, 0, 1, 6)], [{⟨1, 2⟩, ⟨5, 2⟩},{⟨2, 2⟩, ⟨6, 2⟩}]

---

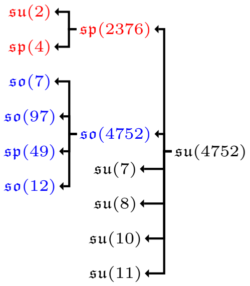


[{⟨1, 1⟩},{⟨4751, 1⟩}], [{⟨1, 1⟩}], [(4751)], [(1, 0, 2, 0)], [{⟨1, 1⟩}], [(0, 1, 5)], [{⟨1, 2⟩}], [{⟨2, 1⟩}], [{⟨1, 1⟩, ⟨5, 2⟩},{⟨1, 1⟩, ⟨6, 2⟩}], [{⟨1, 5⟩, ⟨2, 1⟩},{⟨5, 1⟩, ⟨6, 5⟩}], [{⟨1, 2⟩, ⟨2, 1⟩, ⟨7, 1⟩},{⟨1, 1⟩, ⟨6, 1⟩, ⟨7, 2⟩}], [{⟨1, 2⟩, ⟨3, 1⟩},{⟨7, 1⟩, ⟨9, 2⟩}], [{⟨1, 1⟩, ⟨6, 1⟩},{⟨5, 1⟩, ⟨10, 1⟩}]

---

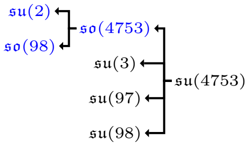


[{⟨1, 1⟩},{⟨4752, 1⟩}], [{⟨1, 1⟩}], [(4752)], [{⟨2, 1⟩}], [(96, 0),(0, 96)], [{⟨1, 2⟩},{⟨96, 2⟩}], [{⟨2, 1⟩},{⟨96, 1⟩}]

---

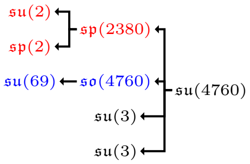


[{⟨1, 1⟩},{⟨4759, 1⟩}], [{⟨1, 1⟩}], [(4759)], [(9, 6)], [{⟨1, 1⟩}], [{⟨1, 1⟩, ⟨68, 1⟩}], [(19, 13),(13, 19)], [(67, 1),(1, 67)]

---

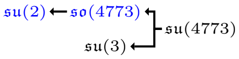


[{⟨1, 1⟩},{⟨4772, 1⟩}], [{⟨1, 1⟩}], [(4772)], [(36, 5),(5, 36)]

---

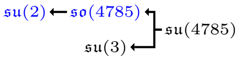


[{⟨1, 1⟩},{⟨4784, 1⟩}], [{⟨1, 1⟩}], [(4784)], [(54, 2),(2, 54)]

---

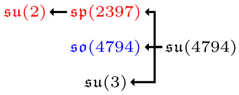


[{⟨1, 1⟩},{⟨4793, 1⟩}], [{⟨1, 1⟩}], [(4793)], [{⟨1, 1⟩}], [(46, 3),(3, 46)]

---

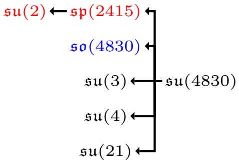


[{⟨1, 1⟩},{⟨4829, 1⟩}], [{⟨1, 1⟩}], [(4829)], [{⟨1, 1⟩}], [(22, 11),(11, 22)], [(19, 0, 1),(1, 0, 19)], [{⟨1, 2⟩, ⟨20, 1⟩},{⟨1, 1⟩, ⟨20, 2⟩}]

---

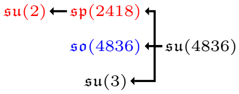


[{⟨1, 1⟩},{⟨4835, 1⟩}], [{⟨1, 1⟩}], [(4835)], [{⟨1, 1⟩}], [(30, 7),(7, 30)]

---

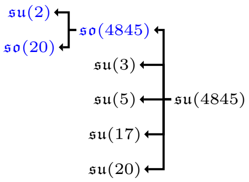


[{⟨1, 1⟩},{⟨4844, 1⟩}], [{⟨1, 1⟩}], [(4844)], [{⟨4, 1⟩}], [(18, 14),(14, 18)], [(16, 0, 0, 0),(0, 0, 0, 16)], [{⟨1, 4⟩},{⟨16, 4⟩}],[{⟨4, 1⟩},{⟨16, 1⟩}]

---

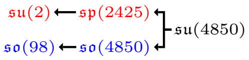


[{⟨1, 1⟩},{⟨4849, 1⟩}], [{⟨1, 1⟩}], [(4849)], [{⟨1, 1⟩}], [{⟨1, 2⟩}]

---

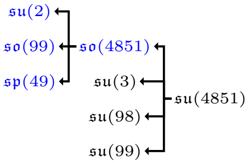


[{⟨1, 1⟩},{⟨4850, 1⟩}], [{⟨1, 1⟩}], [(4850)], [{⟨2, 1⟩}], [{⟨1, 2⟩}], [(97, 0),(0, 97)], [{⟨1, 2⟩},{⟨97, 2⟩}], [{⟨2, 1⟩},{⟨97, 1⟩}]

---

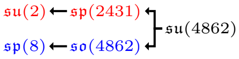


[{⟨1, 1⟩},{⟨4861, 1⟩}], [{⟨1, 1⟩}], [(4861)], [{⟨1, 1⟩}], [{⟨8, 1⟩}]

---

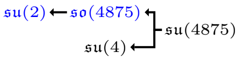


[{⟨1, 1⟩},{⟨4874, 1⟩}], [{⟨1, 1⟩}], [(4874)], [(9, 2, 1),(1, 2, 9)]

---

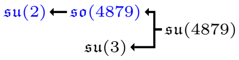


[{⟨1, 1⟩},{⟨4878, 1⟩}], [{⟨1, 1⟩}], [(4878)], [(33, 6),(6, 33)]

---

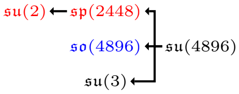


[{⟨1, 1⟩},{⟨4895, 1⟩}], [{⟨1, 1⟩}], [(4895)], [{⟨1, 1⟩}], [(17, 15),(15, 17)]

---

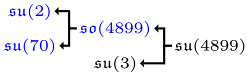


[{⟨1, 1⟩},{⟨4898, 1⟩}], [{⟨1, 1⟩}], [(4898)], [{⟨1, 1⟩, ⟨69, 1⟩}],[(68, 1),(1, 68)]

---

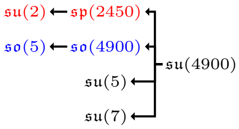


[{⟨1, 1⟩},{⟨4899, 1⟩}], [{⟨1, 1⟩}], [(4899)], [{⟨1, 1⟩}], [(23, 0)], [(2, 3, 0, 1),(1, 0, 3, 2)], [{⟨1, 2⟩, ⟨4, 1⟩, ⟨6, 1⟩},{⟨1, 1⟩, ⟨3, 1⟩, ⟨6, 2⟩}]

---

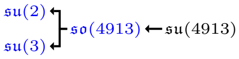


[{⟨1, 1⟩},{⟨4912, 1⟩}],[{⟨1, 1⟩}],[(4912)],[(16, 16)]

---

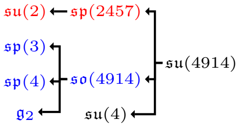


[{⟨1, 1⟩},{⟨4913, 1⟩}], [{⟨1, 1⟩}], [(4913)], [{⟨1, 1⟩}], [(4, 0, 2)],[(2, 2, 0, 0)],[(2, 4)],[(5, 2, 3),(3, 2, 5)]

---

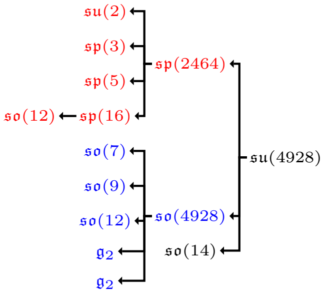


[{⟨1, 1⟩},{⟨4927, 1⟩}], [{⟨1, 1⟩}], [(4927)], [(7, 1, 0)], [(3, 1, 0, 0, 0)], [{⟨3, 1⟩}], [{⟨3, 1⟩, ⟨5, 1⟩},{⟨3, 1⟩, ⟨6, 1⟩}], [{⟨1, 1⟩}], [(0, 2, 3)], [(0, 2, 0, 1)], [{⟨1, 1⟩, ⟨4, 1⟩}], [(1, 5)], [(7, 1)], [{⟨2, 1⟩, ⟨6, 1⟩},{⟨2, 1⟩, ⟨7, 1⟩}]

---

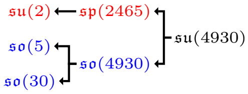


[{⟨1, 1⟩},{⟨4929, 1⟩}], [{⟨1, 1⟩}], [(4929)], [{⟨1, 1⟩}], [(11, 4)],[{⟨1, 3⟩}]

---

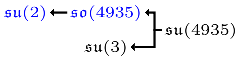


[{⟨1, 1⟩},{⟨4934, 1⟩}], [{⟨1, 1⟩}], [(4934)], [(41, 4),(4, 41)]

---

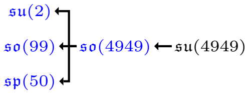


[{⟨1, 1⟩},{⟨4948, 1⟩}], [{⟨1, 1⟩}], [(4948)], [{⟨1, 2⟩}], [{⟨2, 1⟩}]

su(4950): su(2) ⟵ sp(2475); so(100) ⟵ so(4950); su(3); su(3); su(5); su(5); su(6); su(7); su(9); su(9); su(10); su(10); su(10); su(99); su(100); so(10)

[{⟨1, 1⟩},{⟨4949, 1⟩}], [{⟨1, 1⟩}], [(4949)], [{⟨1, 1⟩}], [{⟨2, 1⟩}], [(24, 10),(10, 24)], [(98, 0),(0, 98)], [(0, 7, 0, 0),(0, 0, 7, 0)],[(4, 0, 1, 2),(2, 1, 0, 4)],[(4, 2, 0, 0, 0),(0, 0, 0, 2, 4)], [{⟨1, 4⟩, ⟨3, 1⟩},{⟨4, 1⟩, ⟨6, 4⟩}], [{⟨2, 3⟩},{⟨7, 3⟩}], [{⟨1, 2⟩, ⟨5, 1⟩},{⟨4, 1⟩, ⟨8, 2⟩}], [{⟨3, 2⟩},{⟨7, 2⟩}], [{⟨2, 1⟩, ⟨7, 1⟩},{⟨3, 1⟩, ⟨8, 1⟩}], [{⟨1, 1⟩, ⟨2, 2⟩},{⟨8, 2⟩, ⟨9, 1⟩}], [{⟨1, 2⟩},{⟨98, 2⟩}], [{⟨2, 1⟩},{⟨98, 1⟩}],[(2, 0, 0, 2, 0),(2, 0, 0, 0, 2)]

---

su(4956): su(2) ⟵ sp(2478); so(4956); su(3)

[{⟨1, 1⟩},{⟨4955, 1⟩}], [{⟨1, 1⟩}], [(4955)], [{⟨1, 1⟩}], [(55, 2),(2, 55)]

---

su(4959): su(2) ⟵ so(4959); su(3)

[{⟨1, 1⟩},{⟨4958, 1⟩}], [{⟨1, 1⟩}], [(4958)], [(28, 8),(8, 28)]

---

su(4960): su(2), sp(2), sp(15) ⟵ sp(2480); so(32) ⟵ so(4960); su(4); su(30); su(32)

[{⟨1, 1⟩},{⟨4959, 1⟩}], [{⟨1, 1⟩}], [(4959)], [(29, 0)], [{⟨1, 3⟩}], [{⟨1, 1⟩}], [{⟨3, 1⟩}], [(29, 0, 0),(0, 0, 29)], [{⟨1, 3⟩},{⟨29, 3⟩}],[{⟨3, 1⟩},{⟨29, 1⟩}]

---

su(4992): su(2), so(13) ⟵ sp(2496); so(4992); su(3)

[{⟨1, 1⟩},{⟨4991, 1⟩}], [{⟨1, 1⟩}], [(4991)], [{⟨1, 2⟩, ⟨6, 1⟩}],[{⟨1, 1⟩}],[(47, 3),(3, 47)]

---

su(4995): su(2) ⟵ so(4995); su(3)

[{⟨1, 1⟩},{⟨4994, 1⟩}], [{⟨1, 1⟩}], [(4994)], [(26, 9),(9, 26)]

---

su(5005): su(2), g2 ⟵ so(7), so(11), so(15), sp(5), sp(5) ⟵ so(5005); su(3); su(4); su(4); su(5); su(5); su(7); su(10); su(12); su(14); su(15)

[{⟨1, 1⟩},{⟨5004, 1⟩}], [{⟨1, 1⟩}], [(5004)], [(10, 0, 0)], [(10, 0)],[(0, 1, 1, 0, 0)],[{⟨6, 1⟩}],[(0, 1, 0, 1, 0)],[(6, 0, 0, 0, 0)],[(21, 12),(12, 21)],[(2, 9, 0),(0, 9, 2)],[(5, 4, 1),(1, 4, 5)], [(9, 0, 1, 0),(0, 1, 0, 9)], [(10, 1, 0, 0),(0, 0, 1, 10)], [{⟨1, 9⟩},{⟨6, 9⟩}], [{⟨1, 6⟩},{⟨9, 6⟩}], [{⟨1, 2⟩, ⟨10, 1⟩},{⟨2, 1⟩, ⟨11, 2⟩}], [{⟨1, 1⟩, ⟨11, 1⟩},{⟨3, 1⟩, ⟨13, 1⟩}],[{⟨6, 1⟩},{⟨9, 1⟩}]

---

su(5016): su(2) ⟵ sp(2508); so(5016); su(3)

[{⟨1, 1⟩},{⟨5015, 1⟩}], [{⟨1, 1⟩}], [(5015)], [{⟨1, 1⟩}], [(37, 5),(5, 37)]

---

su(5040): su(2) ⟵ sp(2520); su(71), so(9) ⟵ so(5040); su(3); su(4); su(6); su(6)

[{⟨1, 1⟩},{⟨5039, 1⟩}], [{⟨1, 1⟩}], [(5039)], [{⟨1, 1⟩}], [{⟨1, 1⟩, ⟨70, 1⟩}], [(1, 0, 1, 1)], [(69, 1),(1, 69)], [(8, 0, 5),(5, 0, 8)], [(0, 3, 0, 1, 0),(0, 1, 0, 3, 0)], [(1, 1, 0, 2, 0),(0, 2, 0, 1, 1)]

---

su(5049): su(2), so(100) ⟵ so(5049)

[{⟨1, 1⟩},{⟨5048, 1⟩}],[{⟨1, 1⟩}],[(5048)],[{⟨1, 2⟩}]

---

su(5050): su(2) ⟵ sp(2525); so(101), sp(50) ⟵ so(5050); su(3); su(100); su(101)

[{⟨1, 1⟩},{⟨5049, 1⟩}], [{⟨1, 1⟩}], [(5049)], [{⟨1, 1⟩}], [{⟨2, 1⟩}], [{⟨1, 2⟩}], [(99, 0),(0, 99)], [{⟨1, 2⟩},{⟨99, 2⟩}],[{⟨2, 1⟩},{⟨99, 1⟩}]

---

su(5060): su(2) ⟵ sp(2530); so(5060); su(4); su(22)

[{⟨1, 1⟩},{⟨5059, 1⟩}], [{⟨1, 1⟩}], [(5059)], [{⟨1, 1⟩}], [(19, 1, 0),(0, 1, 19)], [{⟨1, 1⟩, ⟨20, 1⟩},{⟨2, 1⟩, ⟨21, 1⟩}]

---

su(5096): su(2) ⟵ sp(2548); so(5096); su(4)

[{⟨1, 1⟩},{⟨5095, 1⟩}], [{⟨1, 1⟩}], [(5095)], [{⟨1, 1⟩}], [(5, 6, 0),(0, 6, 5)]

---

su(5100): su(2) ⟵ sp(2550); so(5) ⟵ so(5100)

[{⟨1, 1⟩},{⟨5099, 1⟩}], [{⟨1, 1⟩}], [(5099)], [{⟨1, 1⟩}], [(7, 8)]

---

su(5103): su(2), g2 ⟵ so(5103)

[{⟨1, 1⟩},{⟨5102, 1⟩}],[{⟨1, 1⟩}],[(5102)],[(5, 2)]

---

su(5120): su(2), sp(2) ⟵ sp(2560); so(5120); su(3); su(5)

[{⟨1, 1⟩},{⟨5119, 1⟩}], [{⟨1, 1⟩}], [(5119)], [(15, 3)], [{⟨1, 1⟩}],[(31, 7),(7, 31)],[(3, 1, 1, 1),(1, 1, 1, 3)]

---

su(5130): su(2) ⟵ sp(2565); so(5130); su(3); su(4)

[{⟨1, 1⟩},{⟨5129, 1⟩}], [{⟨1, 1⟩}], [(5129)], [{⟨1, 1⟩}], [(56, 2),(2, 56)],[(14, 2, 0),(0, 2, 14)]

---

su(5145): su(2) ⟵ so(5145); su(3); su(3); su(4)

[{⟨1, 1⟩},{⟨5144, 1⟩}], [{⟨1, 1⟩}], [(5144)], [(20, 13),(13, 20)],[(34, 6),(6, 34)],[(6, 1, 4),(4, 1, 6)]

---

su(5148): su(2) ⟵ sp(2574); so(9) ⟵ so(5148); su(10); su(12)

[{⟨1, 1⟩},{⟨5147, 1⟩}], [{⟨1, 1⟩}], [(5147)], [{⟨1, 1⟩}], [(7, 0, 0, 0)], [{⟨1, 3⟩, ⟨2, 1⟩},{⟨8, 1⟩, ⟨9, 3⟩}], [{⟨1, 1⟩, ⟨4, 1⟩},{⟨8, 1⟩, ⟨11, 1⟩}]

---

su(5150): su(2) ⟵ sp(2575); su(101), sp(51) ⟵ so(5150)

[{⟨1, 1⟩},{⟨5149, 1⟩}], [{⟨1, 1⟩}], [(5149)], [{⟨1, 1⟩}], [{⟨1, 2⟩}],[{⟨2, 1⟩}]

---

su(5151): su(2), so(102) ⟵ so(5151); su(3); su(101); su(102)

[{⟨1, 1⟩},{⟨5150, 1⟩}], [{⟨1, 1⟩}], [(5150)], [{⟨2, 1⟩}], [(100, 0),(0, 100)], [{⟨1, 2⟩},{⟨100, 2⟩}], [{⟨2, 1⟩},{⟨100, 1⟩}]

---

su(5160): su(2) ⟵ sp(2580); so(5160); su(3)

[{⟨1, 1⟩},{⟨5159, 1⟩}], [{⟨1, 1⟩}], [(5159)], [{⟨1, 1⟩}], [(42, 4),(4, 42)]

---

su(5175): su(2), so(5), so(25) ⟵ so(5175)

[{⟨1, 1⟩},{⟨5174, 1⟩}], [{⟨1, 1⟩}], [(5174)], [(1, 22)], [{⟨1, 1⟩, ⟨2, 1⟩}]

---

su(5183): su(2), su(72) ⟵ so(5183); su(3)

[{⟨1, 1⟩},{⟨5182, 1⟩}], [{⟨1, 1⟩}], [(5182)], [{⟨1, 1⟩, ⟨71, 1⟩}],[(70, 1),(1, 70)]

su(2), sp(2) ← sp(2592)
sp(2592), so(5184), su(3) ← su(5184)

[{⟨1, 1⟩},{⟨5183, 1⟩}], [{⟨1, 1⟩}], [(5183)], [(11, 5)], [{⟨1, 1⟩}],[(23, 11),(11, 23)]

---

su(2) ← sp(2597)
sp(2597), so(5194), su(3) ← su(5194)

[{⟨1, 1⟩},{⟨5193, 1⟩}], [{⟨1, 1⟩}], [(5193)], [{⟨1, 1⟩}], [(48, 3),(3, 48)]

---

su(2) ← sp(2600)
so(6) ← so(5200)
sp(2600), so(5200), su(25) ← su(5200)

[{⟨1, 1⟩},{⟨5199, 1⟩}], [{⟨1, 1⟩}], [(5199)], [{⟨1, 1⟩}], [(2, 4, 4)],[{⟨1, 1⟩, ⟨2, 1⟩},{⟨23, 1⟩, ⟨24, 1⟩}]

---

su(2), so(5) ← so(5225) ← su(5225)

[{⟨1, 1⟩},{⟨5224, 1⟩}],[{⟨1, 1⟩}],[(5224)],[(2, 18)]

---

su(2), sp(2) ← sp(2618)
sp(2618), so(5236) ← su(5236)

[{⟨1, 1⟩},{⟨5235, 1⟩}], [{⟨1, 1⟩}], [(5235)], [(5, 10)], [{⟨1, 1⟩}]

---

su(2) ← sp(2625)
sp(2625), so(5250), su(3) ← su(5250)

[{⟨1, 1⟩},{⟨5249, 1⟩}], [{⟨1, 1⟩}], [(5249)], [{⟨1, 1⟩}], [(19, 14),(14, 19)]

---

su(2) ← sp(2626)
so(102) ← so(5252)
sp(2626), so(5252) ← su(5252)

[{⟨1, 1⟩},{⟨5251, 1⟩}], [{⟨1, 1⟩}], [(5251)], [{⟨1, 1⟩}], [{⟨1, 2⟩}]

---

su(2), so(103), sp(51) ← so(5253)
so(5253), su(3), su(102), su(103) ← su(5253)

[{⟨1, 1⟩},{⟨5252, 1⟩}], [{⟨1, 1⟩}], [(5252)], [{⟨2, 1⟩}], [{⟨1, 2⟩}], [(101, 0),(0, 101)], [{⟨1, 2⟩},{⟨101, 2⟩}], [{⟨2, 1⟩},{⟨101, 1⟩}]

---

su(2), so(14) ← so(5265)
so(5265), su(3), su(3) ← su(5265)

[{⟨1, 1⟩},{⟨5264, 1⟩}], [{⟨1, 1⟩}], [(5264)], [{⟨1, 2⟩, ⟨2, 1⟩}],[(29, 8),(8, 29)],[(38, 5),(5, 38)]

---

su(2), so(11) ← sp(2640)
so(9) ← so(5280)
sp(2640), so(5280), so(10) ← su(5280)

[{⟨1, 1⟩},{⟨5279, 1⟩}], [{⟨1, 1⟩}], [(5279)], [(0, 0, 0, 1, 1)],[{⟨1, 1⟩}],[(4, 0, 0, 1)],[(1, 0, 0, 3, 0),(1, 0, 0, 0, 3)]

---

su(2) ← so(5291)
so(5291), su(3) ← su(5291)

[{⟨1, 1⟩},{⟨5290, 1⟩}], [{⟨1, 1⟩}], [(5290)], [(25, 10),(10, 25)]

---

su(2), su(6) ← sp(2646)
sp(2646), so(5292), su(6), su(7), su(7), su(7), su(9) ← su(5292)

[{⟨1, 1⟩},{⟨5291, 1⟩}], [{⟨1, 1⟩}], [(5291)], [(2, 0, 1, 0, 2)], [{⟨1, 1⟩}], [(0, 5, 0, 0, 0),(0, 0, 0, 5, 0)], [{⟨2, 1⟩, ⟨3, 2⟩},{⟨4, 2⟩, ⟨5, 1⟩}], [{⟨2, 4⟩},{⟨5, 4⟩}], [{⟨1, 4⟩, ⟨6, 2⟩},{⟨1, 2⟩, ⟨6, 4⟩}],[{⟨4, 2⟩},{⟨5, 2⟩}]

---

su(2), sp(2) ← sp(2652)
so(16) ← so(5304)
sp(2652), so(5304) ← su(5304)

[{⟨1, 1⟩},{⟨5303, 1⟩}], [{⟨1, 1⟩}], [(5303)], [(7, 8)], [{⟨1, 1⟩}],[{⟨2, 2⟩}]

---

su(2) ← so(5307)
so(5307), su(3) ← su(5307)

[{⟨1, 1⟩},{⟨5306, 1⟩}], [{⟨1, 1⟩}], [(5306)], [(57, 2),(2, 57)]

---

su(2), sp(2), sp(2) ← sp(2660)
so(5), sp(8) ← so(5320)
sp(2660), so(5320), su(3), su(3) ← su(5320)

[{⟨1, 1⟩},{⟨5319, 1⟩}], [{⟨1, 1⟩}], [(5319)], [(1, 18)], [(13, 4)], [{⟨1, 1⟩}], [(15, 2)], [{⟨2, 2⟩}], [(18, 15),(15, 18)],[(27, 9),(9, 27)]

---

su(2) ← sp(2664)
su(73) ← so(5328)
sp(2664), so(5328), su(3) ← su(5328)

[{⟨1, 1⟩},{⟨5327, 1⟩}], [{⟨1, 1⟩}], [(5327)], [{⟨1, 1⟩}], [{⟨1, 1⟩, ⟨72, 1⟩}],[(71, 1),(1, 71)]

---

su(2) ← sp(2673)
sp(2673), so(5346), su(9) ← su(5346)

[{⟨1, 1⟩},{⟨5345, 1⟩}], [{⟨1, 1⟩}], [(5345)], [{⟨1, 1⟩}], [{⟨1, 1⟩, ⟨3, 1⟩, ⟨8, 1⟩},{⟨1, 1⟩, ⟨6, 1⟩, ⟨8, 1⟩}]

---

su(2), so(5), so(15), so(103), sp(7), sp(52) ← so(5355)
so(5355), su(3) ← su(5355)

[{⟨1, 1⟩},{⟨5354, 1⟩}], [{⟨1, 1⟩}], [(5354)], [(9, 6)], [{⟨1, 1⟩, ⟨3, 1⟩}],[{⟨1, 2⟩}],[{⟨1, 2⟩, ⟨2, 1⟩}],[{⟨2, 1⟩}], [(17, 16),(16, 17)]

---

su(2) ← sp(2678)
so(104) ← so(5356)
sp(2678), so(5356), su(3), su(103), su(104) ← su(5356)

[{⟨1, 1⟩},{⟨5355, 1⟩}], [{⟨1, 1⟩}], [(5355)], [{⟨1, 1⟩}], [{⟨2, 1⟩}], [(102, 0),(0, 102)], [{⟨1, 2⟩},{⟨102, 2⟩}], [{⟨2, 1⟩},{⟨102, 1⟩}]

---

su(2), sp(2) ← sp(2688)
so(6) ← so(5376)
sp(2688), so(5376), su(4), su(4), su(4), su(8) ← su(5376)

[{⟨1, 1⟩},{⟨5375, 1⟩}], [{⟨1, 1⟩}], [(5375)], [(3, 13)], [{⟨1, 1⟩}], [(1, 5, 5)], [(7, 0, 6),(6, 0, 7)], [(7, 3, 1),(1, 3, 7)], [(13, 1, 1),(1, 1, 13)], [{⟨1, 1⟩, ⟨2, 1⟩, ⟨3, 1⟩},{⟨5, 1⟩, ⟨6, 1⟩, ⟨7, 1⟩}]

---

su(2) ← sp(2691)
sp(2691), so(5382), su(3) ← su(5382)

[{⟨1, 1⟩},{⟨5381, 1⟩}], [{⟨1, 1⟩}], [(5381)], [{⟨1, 1⟩}], [(22, 12),(12, 22)]

---

su(2) ← sp(2695)
sp(2695), so(5390), su(3), su(5) ← su(5390)

[{⟨1, 1⟩},{⟨5389, 1⟩}], [{⟨1, 1⟩}], [(5389)], [{⟨1, 1⟩}], [(43, 4),(4, 43)],[(3, 1, 0, 3),(3, 0, 1, 3)]

---

su(2) ← sp(2700)
sp(2700), so(5400), su(3), su(5) ← su(5400)

[{⟨1, 1⟩},{⟨5399, 1⟩}], [{⟨1, 1⟩}], [(5399)], [{⟨1, 1⟩}], [(49, 3),(3, 49)],[(3, 1, 2, 0),(0, 2, 1, 3)]

---

su(2) ← sp(2706)
sp(2706), so(5412), su(3) ← su(5412)

[{⟨1, 1⟩},{⟨5411, 1⟩}], [{⟨1, 1⟩}], [(5411)], [{⟨1, 1⟩}], [(32, 7),(7, 32)]

---

su(2) ← sp(2709)
sp(2709), so(5418), su(3) ← su(5418)

[{⟨1, 1⟩},{⟨5417, 1⟩}], [{⟨1, 1⟩}], [(5417)], [{⟨1, 1⟩}], [(35, 6),(6, 35)]

---

su(2), so(31) ← so(5425) ← su(5425)

[{⟨1, 1⟩},{⟨5424, 1⟩}],[{⟨1, 1⟩}],[(5424)],[{⟨1, 3⟩}]

---

su(2) ← sp(2720)
so(6) ← so(5440)
sp(2720), so(5440), su(4), su(4), su(16) ← su(5440)

[{⟨1, 1⟩},{⟨5439, 1⟩}], [{⟨1, 1⟩}], [(5439)], [{⟨1, 1⟩}], [(14, 0, 0)], [(11, 3, 0),(0, 3, 11)], [(15, 0, 2),(2, 0, 15)], [{⟨2, 2⟩},{⟨14, 2⟩}]

---

su(2) ← so(5445)
so(5445), su(11) ← su(5445)

[{⟨1, 1⟩},{⟨5444, 1⟩}], [{⟨1, 1⟩}], [(5444)], [{⟨2, 1⟩, ⟨3, 1⟩},{⟨8, 1⟩, ⟨9, 1⟩}]

---

su(2) ← sp(2728)
so(5), so(33) ← so(5456)
sp(2728), so(5456), su(4), su(31), su(33) ← su(5456)

[{⟨1, 1⟩},{⟨5455, 1⟩}], [{⟨1, 1⟩}], [(5455)], [{⟨1, 1⟩}], [(0, 30)], [{⟨3, 1⟩}], [(30, 0, 0),(0, 0, 30)], [{⟨1, 3⟩},

{⟨30, 3⟩}],[{⟨3, 1⟩},{⟨30, 1⟩}]

---

su(5459) → so(5459) → su(2), so(104)

[{⟨1, 1⟩},{⟨5458, 1⟩}],[{⟨1, 1⟩}],[(5458)],[{⟨1, 2⟩}]

---

su(5460) → sp(2730) → su(2), sp(3); so(5460) → so(105), sp(3), sp(52); su(3); su(4); su(4); su(4); su(4); su(4); su(5); su(104); su(105) → su(14), su(15)

[{⟨1, 1⟩},{⟨5459, 1⟩}], [{⟨1, 1⟩}], [(5459)], [(2, 2, 1)], [{⟨1, 1⟩}], [{⟨2, 1⟩}], [(0, 1, 4)], [{⟨1, 2⟩}], [(103, 0),(0, 103)],[(1, 11, 0),(0, 11, 1)],[(3, 8, 0),(0, 8, 3)],[(4, 7, 0),(0, 7, 4)],[(5, 3, 2),(2, 3, 5)],[(12, 0, 3),(3, 0, 12)],[(6, 0, 0, 3),(3, 0, 0, 6)], [{⟨1, 2⟩},{⟨103, 2⟩}], [{⟨2, 1⟩},{⟨103, 1⟩}], [{⟨1, 2⟩, ⟨2, 1⟩},{⟨12, 1⟩, ⟨13, 2⟩}], [{⟨1, 1⟩, ⟨3, 1⟩},{⟨12, 1⟩, ⟨14, 1⟩}]

---

su(5475) → so(5475) → su(2), su(74); su(3)

[{⟨1, 1⟩},{⟨5474, 1⟩}], [{⟨1, 1⟩}], [(5474)], [{⟨1, 1⟩, ⟨73, 1⟩}],[(72, 1),(1, 72)]

---

su(5487) → so(5487) → su(2); su(3)

[{⟨1, 1⟩},{⟨5486, 1⟩}], [{⟨1, 1⟩}], [(5486)], [(58, 2),(2, 58)]

---

su(5520) → sp(2760) → su(2); so(5520); su(3)

[{⟨1, 1⟩},{⟨5519, 1⟩}], [{⟨1, 1⟩}], [(5519)], [{⟨1, 1⟩}], [(39, 5),(5, 39)]

---

su(5525) → so(5525) → su(2), so(5)

[{⟨1, 1⟩},{⟨5524, 1⟩}],[{⟨1, 1⟩}],[(5524)],[(24, 0)]

---

su(5544) → sp(2772) → su(2); so(5544); su(3); su(4); su(4); su(6); su(6); su(8); su(8); su(9); su(22)

[{⟨1, 1⟩},{⟨5543, 1⟩}], [{⟨1, 1⟩}], [(5543)], [{⟨1, 1⟩}], [(21, 13),(13, 21)], [(7, 2, 2),(2, 2, 7)], [(20, 0, 1),(1, 0, 20)],[(4, 1, 0, 0, 1),(1, 0, 0, 1, 4)],[(6, 0, 0, 1, 0),(0, 1, 0, 0, 6)], [{⟨1, 2⟩, ⟨6, 1⟩, ⟨7, 1⟩},{⟨1, 1⟩, ⟨2, 1⟩, ⟨7, 2⟩}], [{⟨1, 2⟩, ⟨2, 2⟩},{⟨6, 2⟩, ⟨7, 2⟩}], [{⟨1, 3⟩, ⟨7, 1⟩},{⟨2, 1⟩, ⟨8, 3⟩}],[{⟨1, 2⟩, ⟨21, 1⟩},{⟨1, 1⟩, ⟨21, 2⟩}]

---

su(5550) → sp(2775) → su(2); so(5550); su(3)

[{⟨1, 1⟩},{⟨5549, 1⟩}], [{⟨1, 1⟩}], [(5549)], [{⟨1, 1⟩}], [(24, 11),(11, 24)]

---

su(5564) → sp(2782) → su(2); so(5564) → so(105), sp(53)

[{⟨1, 1⟩},{⟨5563, 1⟩}], [{⟨1, 1⟩}], [(5563)], [{⟨1, 1⟩}], [{⟨1, 2⟩}],[{⟨2, 1⟩}]

---

su(5565) → so(5565) → su(2), so(106); su(3); su(105); su(106)

[{⟨1, 1⟩},{⟨5564, 1⟩}], [{⟨1, 1⟩}], [(5564)], [{⟨2, 1⟩}], [(104, 0),(0, 104)], [{⟨1, 2⟩},{⟨104, 2⟩}], [{⟨2, 1⟩},{⟨104, 1⟩}]

---

su(5580) → sp(2790) → su(2); so(5580); su(3)

[{⟨1, 1⟩},{⟨5579, 1⟩}], [{⟨1, 1⟩}], [(5579)], [{⟨1, 1⟩}], [(30, 8),(8, 30)]

---

su(5600) → sp(2800) → su(2); so(5600); su(5); su(5); su(5); su(7)

[{⟨1, 1⟩},{⟨5599, 1⟩}], [{⟨1, 1⟩}], [(5599)], [{⟨1, 1⟩}], [(1, 4, 0, 1),(1, 0, 4, 1)],[(2, 0, 3, 1),(1, 3, 0, 2)],[(6, 0, 1, 1),(1, 1, 0, 6)], [{⟨1, 1⟩, ⟨2, 2⟩, ⟨6, 1⟩},{⟨1, 1⟩, ⟨5, 2⟩, ⟨6, 1⟩}]

---

su(5610) → sp(2805) → su(2); so(5610); su(3); su(4)

[{⟨1, 1⟩},{⟨5609, 1⟩}], [{⟨1, 1⟩}], [(5609)], [{⟨1, 1⟩}], [(50, 3),(3, 50)],[(10, 0, 4),(4, 0, 10)]

---

su(5624) → sp(2812) → su(2); so(5624) → su(75); su(3)

[{⟨1, 1⟩},{⟨5623, 1⟩}], [{⟨1, 1⟩}], [(5623)], [{⟨1, 1⟩}], [{⟨1, 1⟩, ⟨74, 1⟩}],[(73, 1),(1, 73)]

---

su(5625) → so(5625) → su(2); su(3)

[{⟨1, 1⟩},{⟨5624, 1⟩}], [{⟨1, 1⟩}], [(5624)], [(44, 4),(4, 44)]

---

su(5643) → so(5643) → su(2); su(3)

[{⟨1, 1⟩},{⟨5642, 1⟩}], [{⟨1, 1⟩}], [(5642)], [(26, 10),(10, 26)]

---

su(5655) → so(5655) → su(2); su(3)

[{⟨1, 1⟩},{⟨5654, 1⟩}], [{⟨1, 1⟩}], [(5654)], [(28, 9),(9, 28)]

---

su(5670) → sp(2835) → su(2); so(5670) → so(106); su(3); su(3); su(5); su(6); su(6)

[{⟨1, 1⟩},{⟨5669, 1⟩}], [{⟨1, 1⟩}], [(5669)], [{⟨1, 1⟩}], [{⟨1, 2⟩}], [(20, 14),(14, 20)], [(59, 2),(2, 59)], [(0, 5, 1, 0),(0, 1, 5, 0)], [(1, 0, 1, 2, 0),(0, 2, 1, 0, 1)], [(3, 1, 0, 1, 0),(0, 1, 0, 1, 3)]

---

su(5671) → so(5671) → su(2), so(107), sp(53); su(3); su(106); su(107)

[{⟨1, 1⟩},{⟨5670, 1⟩}], [{⟨1, 1⟩}], [(5670)], [{⟨2, 1⟩}], [{⟨1, 2⟩}], [(105, 0),(0, 105)], [{⟨1, 2⟩},{⟨105, 2⟩}], [{⟨2, 1⟩},{⟨105, 1⟩}]

---

su(5698) → sp(2849) → su(2); so(5698); su(3)

[{⟨1, 1⟩},{⟨5697, 1⟩}], [{⟨1, 1⟩}], [(5697)], [{⟨1, 1⟩}], [(36, 6),(6, 36)]

---

su(5712) → sp(2856) → su(2); so(5712) → sp(3); su(3)

[{⟨1, 1⟩},{⟨5711, 1⟩}], [{⟨1, 1⟩}], [(5711)], [{⟨1, 1⟩}], [(0, 0, 6)],[(33, 7),(7, 33)]

---

su(5720) → sp(2860) → su(2), sp(5); so(5720) → sp(3); su(4); su(4); su(4); su(5); su(6); su(12)

[{⟨1, 1⟩},{⟨5719, 1⟩}], [{⟨1, 1⟩}], [(5719)], [(2, 0, 0, 0, 1)],[{⟨1, 1⟩}],[(2, 1, 2)],[(2, 7, 1),(1, 7, 2)],[(4, 5, 1),(1, 5, 4)], [(10, 1, 2),(2, 1, 10)], [(7, 2, 0, 0),(0, 0, 2, 7)], [(7, 1, 0, 0, 0),(0, 0, 0, 1, 7)], [{⟨1, 1⟩, ⟨8, 1⟩},{⟨4, 1⟩, ⟨11, 1⟩}]

---

su(5733) → so(5733) → su(2), so(13)

[{⟨1, 1⟩},{⟨5732, 1⟩}],[{⟨1, 1⟩}],[(5732)],[{⟨1, 5⟩}]

---

su(5760) → sp(2880) → su(2); so(5760) → su(9); su(3); su(6)

[{⟨1, 1⟩},{⟨5759, 1⟩}], [{⟨1, 1⟩}], [(5759)], [{⟨1, 1⟩}], [{⟨3, 1⟩, ⟨6, 1⟩}],[(19, 15),(15, 19)],[(3, 1, 1, 0, 0),(0, 0, 1, 1, 3)]

---

su(5772) → sp(2886) → su(2); so(5772); su(3)

[{⟨1, 1⟩},{⟨5771, 1⟩}], [{⟨1, 1⟩}], [(5771)], [{⟨1, 1⟩}], [(23, 12),(12, 23)]

---

su(5775) → so(5775) → su(2), su(76), so(5), so(8); su(3); su(5); su(5); su(7); su(8)

[{⟨1, 1⟩},{⟨5774, 1⟩}], [{⟨1, 1⟩}], [(5774)], [{⟨1, 1⟩, ⟨75, 1⟩}],[(6, 10)],[(4, 0, 2, 0),(4, 0, 0, 2),(2, 0, 4, 0),(2, 0, 0, 4),(0, 0, 4, 2),(0, 0, 2, 4)],[(74, 1),(1, 74)],[(3, 4, 0, 0),(0, 0, 4, 3)], [(8, 0, 0, 2),(2, 0, 0, 8)], [{⟨1, 4⟩, ⟨4, 1⟩},{⟨3, 1⟩, ⟨6, 4⟩}],[{⟨1, 3⟩, ⟨5, 1⟩},{⟨3, 1⟩, ⟨7, 3⟩}]

su(5777) → so(5777) → {su(2), so(107), sp(54)}

[{⟨1, 1⟩},{⟨5776, 1⟩}], [{⟨1, 1⟩}], [(5776)], [{⟨1, 2⟩}], [{⟨2, 1⟩}]

---

su(5778) → {sp(2889) → su(2), so(5778) → so(108), su(3), su(107), su(108)}

[{⟨1, 1⟩},{⟨5777, 1⟩}], [{⟨1, 1⟩}], [(5777)], [{⟨1, 1⟩}], [{⟨2, 1⟩}], [(106, 0),(0, 106)], [{⟨1, 2⟩},{⟨106, 2⟩}], [{⟨2, 1⟩},{⟨106, 1⟩}]

---

su(5781) → {so(5781) → su(2), su(3)}

[{⟨1, 1⟩},{⟨5780, 1⟩}], [{⟨1, 1⟩}], [(5780)], [(40, 5),(5, 40)]

---

su(5796) → {sp(2898) → su(2), so(5796), su(4), su(23)}

[{⟨1, 1⟩},{⟨5795, 1⟩}], [{⟨1, 1⟩}], [(5795)], [{⟨1, 1⟩}], [(20, 1, 0),(0, 1, 20)], [{⟨1, 1⟩, ⟨21, 1⟩},{⟨2, 1⟩, ⟨22, 1⟩}]

---

su(5814) → {sp(2907) → su(2), so(5814) → so(18), su(3)}

[{⟨1, 1⟩},{⟨5813, 1⟩}], [{⟨1, 1⟩}], [(5813)], [{⟨1, 1⟩}], [{⟨1, 4⟩}],[(18, 16),(16, 18)]

---

su(5824) → {sp(2912) → {su(2), sp(2), sp(13)}, so(5824) → so(26), su(3), su(5), su(13), so(14), $\mathfrak{e}_6$}

[{⟨1, 1⟩},{⟨5823, 1⟩}], [{⟨1, 1⟩}], [(5823)], [(23, 1)], [{⟨1, 1⟩, ⟨2, 1⟩}], [{⟨1, 1⟩}], [{⟨1, 1⟩, ⟨2, 1⟩}], [(51, 3),(3, 51)], [(11, 0, 0, 1),(1, 0, 0, 11)], [{⟨1, 3⟩, ⟨12, 1⟩},{⟨1, 1⟩, ⟨12, 3⟩}], [{⟨1, 2⟩, ⟨6, 1⟩},{⟨1, 2⟩, ⟨7, 1⟩}], [{⟨1, 1⟩, ⟨3, 1⟩},{⟨5, 1⟩, ⟨6, 1⟩}]

---

su(5832) → {sp(2916) → su(2), so(5832) → su(3)}

[{⟨1, 1⟩},{⟨5831, 1⟩}], [{⟨1, 1⟩}], [(5831)], [{⟨1, 1⟩}], [(17, 17)]

---

su(5850) → {sp(2925) → su(2), so(5850), su(26)}

[{⟨1, 1⟩},{⟨5849, 1⟩}], [{⟨1, 1⟩}], [(5849)], [{⟨1, 1⟩}], [{⟨1, 1⟩, ⟨2, 1⟩},{⟨24, 1⟩, ⟨25, 1⟩}]

---

su(5856) → {sp(2928) → su(2), so(5856), su(3)}

[{⟨1, 1⟩},{⟨5855, 1⟩}], [{⟨1, 1⟩}], [(5855)], [{⟨1, 1⟩}], [(60, 2),(2, 60)]

---

su(5865) → {so(5865) → su(2), su(3)}

[{⟨1, 1⟩},{⟨5864, 1⟩}], [{⟨1, 1⟩}], [(5864)], [(45, 4),(4, 45)]

---

su(5880) → {sp(2940) → su(2), so(5880), su(4), su(6), su(6), su(6), su(6)}

[{⟨1, 1⟩},{⟨5879, 1⟩}], [{⟨1, 1⟩}], [(5879)], [{⟨1, 1⟩}], [(7, 5, 0),(0, 5, 7)],[(1, 1, 2, 0, 0),(0, 0, 2, 1, 1)],[(1, 4, 0, 0, 0),(0, 0, 0, 4, 1)], [(2, 2, 0, 0, 1),(1, 0, 0, 2, 2)], [(4, 0, 0, 0, 3),(3, 0, 0, 0, 4)]

---

su(5885) → so(5885) → {su(2), so(108)}

[{⟨1, 1⟩},{⟨5884, 1⟩}],[{⟨1, 1⟩}],[(5884)],[{⟨1, 2⟩}]

---

su(5886) → {sp(2943) → su(2), so(5886) → {so(109), sp(54)}, su(3), su(108), su(109)}

[{⟨1, 1⟩},{⟨5885, 1⟩}], [{⟨1, 1⟩}], [(5885)], [{⟨1, 1⟩}], [{⟨2, 1⟩}], [{⟨1, 2⟩}], [(107, 0),(0, 107)], [{⟨1, 2⟩},{⟨107, 2⟩}],[{⟨2, 1⟩},{⟨107, 1⟩}]

---

su(5904) → {sp(2952) → su(2), so(5904), su(3)}

[{⟨1, 1⟩},{⟨5903, 1⟩}], [{⟨1, 1⟩}], [(5903)], [{⟨1, 1⟩}], [(31, 8),(8, 31)]

---

su(5915) → so(5915) → {su(2), su(13)}

[{⟨1, 1⟩},{⟨5914, 1⟩}], [{⟨1, 1⟩}], [(5914)], [{⟨2, 1⟩, ⟨11, 1⟩}]

---

su(5928) → {sp(2964) → su(2), so(5928) → su(77), su(3), su(3)}

[{⟨1, 1⟩},{⟨5927, 1⟩}], [{⟨1, 1⟩}], [(5927)], [{⟨1, 1⟩}], [{⟨1, 1⟩, ⟨76, 1⟩}],[(25, 11),(11, 25)],[(75, 1),(1, 75)]

---

su(5940) → {sp(2970) → su(2), so(5940) → {su(12), so(10)}, su(4), su(5)}

[{⟨1, 1⟩},{⟨5939, 1⟩}], [{⟨1, 1⟩}], [(5939)], [{⟨1, 1⟩}], [{⟨1, 2⟩, ⟨11, 2⟩}], [(0, 1, 0, 1, 1)], [(8, 1, 3),(3, 1, 8)], [(4, 2, 0, 1),(1, 0, 2, 4)]

---

su(5950) → {sp(2975) → {su(2), sp(17)}, so(5950) → so(5)}

[{⟨1, 1⟩},{⟨5949, 1⟩}], [{⟨1, 1⟩}], [(5949)], [{⟨3, 1⟩}], [{⟨1, 1⟩}],[(3, 16)]

---

su(5952) → {sp(2976) → su(2), so(5952) → so(32)}

[{⟨1, 1⟩},{⟨5951, 1⟩}], [{⟨1, 1⟩}], [(5951)], [{⟨1, 1⟩}], [{⟨1, 3⟩}]

---

su(5957) → {so(5957) → su(2), su(3)}

[{⟨1, 1⟩},{⟨5956, 1⟩}], [{⟨1, 1⟩}], [(5956)], [(22, 13),(13, 22)]

---

su(5980) → {sp(2990) → {su(2), sp(2)}, so(5980)}

[{⟨1, 1⟩},{⟨5979, 1⟩}], [{⟨1, 1⟩}], [(5979)], [(19, 2)], [{⟨1, 1⟩}]

---

su(5984) → {sp(2992) → {su(2), sp(2), sp(16)}, so(5984) → so(34), su(4), su(32), su(34)}

[{⟨1, 1⟩},{⟨5983, 1⟩}], [{⟨1, 1⟩}], [(5983)], [(31, 0)], [{⟨1, 3⟩}], [{⟨1, 1⟩}], [{⟨3, 1⟩}], [(31, 0, 0),(0, 0, 31)], [{⟨1, 3⟩},{⟨31, 3⟩}],[{⟨3, 1⟩},{⟨31, 1⟩}]

---

su(5985) → {so(5985) → {su(2), so(7), so(21), sp(9)}, su(3), su(5), su(18), su(21)}

[{⟨1, 1⟩},{⟨5984, 1⟩}], [{⟨1, 1⟩}], [(5984)], [(6, 1, 0)], [{⟨4, 1⟩}],[{⟨1, 4⟩}],[(37, 6),(6, 37)],[(17, 0, 0, 0),(0, 0, 0, 17)],[{⟨1, 4⟩},{⟨17, 4⟩}],[{⟨4, 1⟩},{⟨17, 1⟩}]

---

su(5994) → {sp(2997) → su(2), so(5994) → {so(109), sp(55)}}

[{⟨1, 1⟩},{⟨5993, 1⟩}], [{⟨1, 1⟩}], [(5993)], [{⟨1, 1⟩}], [{⟨1, 2⟩}],[{⟨2, 1⟩}]

---

su(5995) → {so(5995) → {su(2), so(110)}, su(3), su(109), su(110)}

[{⟨1, 1⟩},{⟨5994, 1⟩}], [{⟨1, 1⟩}], [(5994)], [{⟨2, 1⟩}], [(108, 0),(0, 108)], [{⟨1, 2⟩},{⟨108, 2⟩}], [{⟨2, 1⟩},{⟨108, 1⟩}]

---

su(6000) → {sp(3000) → su(2), so(6000), su(3), su(4), su(6)}

[{⟨1, 1⟩},{⟨5999, 1⟩}], [{⟨1, 1⟩}], [(5999)], [{⟨1, 1⟩}], [(29, 9),(9, 29)], [(9, 4, 0),(0, 4, 9)], [(3, 0, 2, 0, 0),(0, 0, 2, 0, 3)]

---

su(6006) → {sp(3003) → {su(2), sp(3)}, so(6006) → {so(7), sp(3), sp(6)}, su(3), su(4), su(7), su(8)}

[{⟨1, 1⟩},{⟨6005, 1⟩}], [{⟨1, 1⟩}], [(6005)], [(4, 1, 1)], [{⟨1, 1⟩}], [(1, 0, 6)], [(7, 0, 1)], [{⟨1, 1⟩, ⟨5, 1⟩}], [(27, 10),(10, 27)], [(3, 6, 1),(1, 6, 3)], [{⟨1, 6⟩, ⟨6, 1⟩},{⟨1, 1⟩, ⟨6, 6⟩}],[{⟨1, 5⟩, ⟨7, 1⟩},{⟨1, 1⟩, ⟨7, 5⟩}]

---

su(6020) → {sp(3010) → su(2), so(6020), su(3)}

[{⟨1, 1⟩},{⟨6019, 1⟩}], [{⟨1, 1⟩}], [(6019)], [{⟨1, 1⟩}], [(34, 7),(7, 34)]

su(2) ← sp(3021) ←
so(6042) ← su(6042)
su(3) ←

[{⟨1, 1⟩},{⟨6041, 1⟩}], [{⟨1, 1⟩}], [(6041)], [{⟨1, 1⟩}], [(52, 3),(3, 52)]

---

su(2) ←
so(6045) ←
so(5) ← su(6045)
su(3) ←

[{⟨1, 1⟩},{⟨6044, 1⟩}], [{⟨1, 1⟩}], [(6044)], [(12, 4)], [(61, 2),(2, 61)]

---

su(2) ← sp(3024) ←
so(6048) ←
su(6048)
su(3) ←
su(9) ←

[{⟨1, 1⟩},{⟨6047, 1⟩}], [{⟨1, 1⟩}], [(6047)], [{⟨1, 1⟩}], [(41, 5),(5, 41)],[{⟨3, 1⟩, ⟨4, 1⟩},{⟨5, 1⟩, ⟨6, 1⟩}]

---

su(2) ← sp(3040) ←
so(6080) ← su(6080)
su(4) ←

[{⟨1, 1⟩},{⟨6079, 1⟩}], [{⟨1, 1⟩}], [(6079)], [{⟨1, 1⟩}], [(15, 2, 0),(0, 2, 15)]

---

su(2) ←
so(6083) ←
su(78) ← su(6083)
su(3) ←

[{⟨1, 1⟩},{⟨6082, 1⟩}], [{⟨1, 1⟩}], [(6082)], [{⟨1, 1⟩, ⟨77, 1⟩}],[(76, 1),(1, 76)]

---

su(2) ← sp(3052) ←
su(6104)
so(110) ← so(6104) ←

[{⟨1, 1⟩},{⟨6103, 1⟩}], [{⟨1, 1⟩}], [(6103)], [{⟨1, 1⟩}], [{⟨1, 2⟩}]

---

su(2) ←
so(111) ← so(6105) ←
sp(55) ← su(3) ←
su(3) ← su(6105)
su(110) ←
su(111) ←

[{⟨1, 1⟩},{⟨6104, 1⟩}], [{⟨1, 1⟩}], [(6104)], [{⟨2, 1⟩}], [{⟨1, 2⟩}], [(21, 14),(14, 21)], [(109, 0),(0, 109)], [{⟨1, 2⟩},{⟨109, 2⟩}],[{⟨2, 1⟩},{⟨109, 1⟩}]

---

su(2) ← sp(3055) ←
so(6110) ← su(6110)
su(3) ←

[{⟨1, 1⟩},{⟨6109, 1⟩}], [{⟨1, 1⟩}], [(6109)], [{⟨1, 1⟩}], [(46, 4),(4, 46)]

---

su(2) ←
so(6125) ← su(6125)
su(5) ←

[{⟨1, 1⟩},{⟨6124, 1⟩}],[{⟨1, 1⟩}],[(6124)],[(2, 1, 1, 2)]

---

su(2) ←
sp(3080) ←
sp(2) ←
so(8) ← so(6160) ←
su(4) ← su(6160)
su(5) ←
su(6) ←
su(10) ←

[{⟨1, 1⟩},{⟨6159, 1⟩}], [{⟨1, 1⟩}], [(6159)], [(1, 19)], [{⟨1, 1⟩}],[(1, 2, 1, 0),(1, 2, 0, 1),(0, 2, 1, 1)],[(10, 2, 1),(1, 2, 10)], [(6, 0, 2, 0),(0, 2, 0, 6)], [(6, 0, 1, 0, 0),(0, 0, 1, 0, 6)],[{⟨1, 2⟩, ⟨7, 1⟩},{⟨3, 1⟩, ⟨9, 2⟩}]

---

su(2) ←
so(6175) ←
so(5) ← su(6175)
su(3) ←

[{⟨1, 1⟩},{⟨6174, 1⟩}], [{⟨1, 1⟩}], [(6174)], [(5, 12)], [(24, 12),(12, 24)]

---

su(2) ← sp(3094) ←
so(17) ←
sp(3) ← so(6188) ←
sp(8) ← su(6) ← su(6188)
su(13) ←
su(17) ←

[{⟨1, 1⟩},{⟨6187, 1⟩}], [{⟨1, 1⟩}], [(6187)], [{⟨1, 1⟩}], [{⟨5, 1⟩}],[(12, 0, 0)],[{⟨6, 1⟩}],[(12, 0, 0, 0, 0),(0, 0, 0, 0, 12)],[{⟨1, 5⟩},{⟨12, 5⟩}],[{⟨5, 1⟩},{⟨12, 1⟩}]

---

su(2) ←
so(6201) ← su(6201)
so(5) ←

[{⟨1, 1⟩},{⟨6200, 1⟩}],[{⟨1, 1⟩}],[(6200)],[(25, 0)]

---

su(2) ←
so(111) ← so(6215) ← su(6215)
sp(56) ←

[{⟨1, 1⟩},{⟨6214, 1⟩}], [{⟨1, 1⟩}], [(6214)], [{⟨1, 2⟩}], [{⟨2, 1⟩}]

---

su(2) ← sp(3108) ←
so(112) ← so(6216) ←
su(3) ←
su(3) ← su(6216)
su(111) ←
su(112) ←

[{⟨1, 1⟩},{⟨6215, 1⟩}], [{⟨1, 1⟩}], [(6215)], [{⟨1, 1⟩}], [{⟨2, 1⟩}], [(20, 15),(15, 20)], [(110, 0),(0, 110)], [{⟨1, 2⟩},{⟨110, 2⟩}],[{⟨2, 1⟩},{⟨110, 1⟩}]

---

su(2) ←
so(6237) ←
sp(4) ←
su(3) ← su(6237)
su(3) ←

[{⟨1, 1⟩},{⟨6236, 1⟩}],[{⟨1, 1⟩}],[(6236)],[(1, 0, 1, 1)], [(32, 8),(8, 32)],[(62, 2),(2, 62)]

---

su(2) ←
sp(3120) ←
sp(2) ←
su(79) ← so(6240) ← su(6240)
su(3) ←
su(4) ←

[{⟨1, 1⟩},{⟨6239, 1⟩}], [{⟨1, 1⟩}], [(6239)], [(9, 7)], [{⟨1, 1⟩}], [{⟨1, 1⟩, ⟨78, 1⟩}], [(77, 1),(1, 77)], [(4, 3, 3),(3, 3, 4)]

---

su(2) ← sp(3125) ←
su(6250)
so(5) ← so(6250) ←

[{⟨1, 1⟩},{⟨6249, 1⟩}], [{⟨1, 1⟩}], [(6249)], [{⟨1, 1⟩}], [(4, 14)]

---

su(2) ← sp(3132) ←
so(6264) ← su(6264)
su(3) ←

[{⟨1, 1⟩},{⟨6263, 1⟩}], [{⟨1, 1⟩}], [(6263)], [{⟨1, 1⟩}], [(53, 3),(3, 53)]

---

su(2) ← sp(3136) ←
su(6272)
su(7) ← so(6272) ←

[{⟨1, 1⟩},{⟨6271, 1⟩}], [{⟨1, 1⟩}], [(6271)], [{⟨1, 1⟩}], [{⟨1, 3⟩, ⟨6, 3⟩}]

---

su(2) ← so(6279) ←
su(6279)
su(3) ←

[{⟨1, 1⟩},{⟨6278, 1⟩}], [{⟨1, 1⟩}], [(6278)], [(38, 6),(6, 38)]

---

su(2) ← sp(3145) ←
so(5) ← so(6290) ← su(6290)
su(3) ←

[{⟨1, 1⟩},{⟨6289, 1⟩}], [{⟨1, 1⟩}], [(6289)], [{⟨1, 1⟩}], [(16, 2)],[(19, 16),(16, 19)]

---

su(2) ←
sp(3150) ←
sp(3) ← su(6300)
so(6300) ←

[{⟨1, 1⟩},{⟨6299, 1⟩}], [{⟨1, 1⟩}], [(6299)], [(0, 4, 1)], [{⟨1, 1⟩}]

---

su(2) ← sp(3159) ←
so(6318) ← su(6318)
su(3) ←

[{⟨1, 1⟩},{⟨6317, 1⟩}], [{⟨1, 1⟩}], [(6317)], [{⟨1, 1⟩}], [(26, 11),(11, 26)]

---

su(2) ← so(6321) ←
su(6321)
su(3) ←

[{⟨1, 1⟩},{⟨6320, 1⟩}], [{⟨1, 1⟩}], [(6320)], [(42, 5),(5, 42)]

---

su(2) ← so(6325) ←
su(4) ← su(6325)
su(23) ←

[{⟨1, 1⟩},{⟨6324, 1⟩}], [{⟨1, 1⟩}], [(6324)], [(21, 0, 1),(1, 0, 21)],[{⟨1, 2⟩, ⟨22, 1⟩},{⟨1, 1⟩, ⟨22, 2⟩}]

---

su(2) ←
so(6327) ←
so(112) ← su(6327)
su(3) ←

[{⟨1, 1⟩},{⟨6326, 1⟩}], [{⟨1, 1⟩}], [(6326)], [{⟨1, 2⟩}], [(18, 17),(17, 18)]

---

su(2) ← sp(3164) ←
so(113) ←
so(6328) ←
sp(56) ← su(6328)
su(3) ←
su(112) ←
su(113) ←

[{⟨1, 1⟩},{⟨6327, 1⟩}], [{⟨1, 1⟩}], [(6327)], [{⟨1, 1⟩}], [{⟨2, 1⟩}], [{⟨1, 2⟩}], [(111, 0),(0, 111)], [{⟨1, 2⟩},{⟨111, 2⟩}],[{⟨2, 1⟩},{⟨111, 1⟩}]

---

su(2) ← sp(3168) ←
so(7) ← so(6336) ← su(6336)
su(3) ←

[{⟨1, 1⟩},{⟨6335, 1⟩}], [{⟨1, 1⟩}], [(6335)], [{⟨1, 1⟩}], [(7, 0, 1)],[(35, 7),(7, 35)]

---

su(2) ← so(6355) ←
su(6355)
su(3) ←

[{⟨1, 1⟩},{⟨6354, 1⟩}], [{⟨1, 1⟩}], [(6354)], [(30, 9),(9, 30)]

---

su(2) ← sp(3180) ←
so(6360) ← su(6360)
su(3) ←

[{⟨1, 1⟩},{⟨6359, 1⟩}], [{⟨1, 1⟩}], [(6359)], [{⟨1, 1⟩}], [(47, 4),(4, 47)]

---

su(2) ← sp(3185) ←
so(6370) ← su(6370)
su(5) ←

[{⟨1, 1⟩},{⟨6369, 1⟩}], [{⟨1, 1⟩}], [(6369)], [{⟨1, 1⟩}], [(5, 0, 0, 4),(4, 0, 0, 5)]

---

su(2) ← sp(3190) ←
so(6380) ← su(6380)
su(3) ←

[{⟨1, 1⟩},{⟨6379, 1⟩}], [{⟨1, 1⟩}], [(6379)], [{⟨1, 1⟩}], [(28, 10),(10, 28)]

---

su(2) ← sp(3192) ←
so(6384) ← su(6384)
su(3) ←

[{⟨1, 1⟩},{⟨6383, 1⟩}], [{⟨1, 1⟩}], [(6383)], [{⟨1, 1⟩}], [(23, 13),(13, 23)]

---

su(6399) ← so(6399), su(3); so(6399) ← su(2), su(80)

[{⟨1, 1⟩},{⟨6398, 1⟩}], [{⟨1, 1⟩}], [(6398)], [{⟨1, 1⟩, ⟨79, 1⟩}],[(78, 1),(1, 78)]

---

su(6426) ← sp(3213), so(6426), su(4); sp(3213) ← su(2)

[{⟨1, 1⟩},{⟨6425, 1⟩}], [{⟨1, 1⟩}], [(6425)], [{⟨1, 1⟩}], [(16, 0, 2),(2, 0, 16)]

---

su(6432) ← sp(3216), so(6432), su(3); sp(3216) ← su(2)

[{⟨1, 1⟩},{⟨6431, 1⟩}], [{⟨1, 1⟩}], [(6431)], [{⟨1, 1⟩}], [(63, 2),(2, 63)]

---

su(6435) ← so(6435), su(8), su(9), su(15); so(6435) ← su(2), sp(4), so(16); so(16) ← so(15)

[{⟨1, 1⟩},{⟨6434, 1⟩}],[{⟨1, 1⟩}],[(6434)],[(8, 0, 0, 0)], [{⟨7, 2⟩},{⟨8, 2⟩}], [{⟨7, 2⟩}], [{⟨1, 8⟩},{⟨7, 8⟩}], [{⟨1, 7⟩},{⟨8, 7⟩}],[{⟨7, 1⟩},{⟨8, 1⟩}]

---

su(6440) ← sp(3220), so(6440); sp(3220) ← su(2); so(6440) ← so(113), sp(57)

[{⟨1, 1⟩},{⟨6439, 1⟩}], [{⟨1, 1⟩}], [(6439)], [{⟨1, 1⟩}], [{⟨1, 2⟩}],[{⟨2, 1⟩}]

---

su(6441) ← so(6441), su(3), su(113), su(114); so(6441) ← su(2), so(114)

[{⟨1, 1⟩},{⟨6440, 1⟩}], [{⟨1, 1⟩}], [(6440)], [{⟨2, 1⟩}], [(112, 0),(0, 112)], [{⟨1, 2⟩},{⟨112, 2⟩}], [{⟨2, 1⟩},{⟨112, 1⟩}]

---

su(6460) ← sp(3230), so(6460), su(4); sp(3230) ← su(2), sp(2)

[{⟨1, 1⟩},{⟨6459, 1⟩}], [{⟨1, 1⟩}], [(6459)], [(3, 14)], [{⟨1, 1⟩}],[(14, 1, 1),(1, 1, 14)]

---

su(6468) ← sp(3234), so(6468), su(7), su(7); sp(3234) ← su(2)

[{⟨1, 1⟩},{⟨6467, 1⟩}], [{⟨1, 1⟩}], [(6467)], [{⟨1, 1⟩}], [{⟨1, 3⟩, ⟨2, 1⟩, ⟨6, 1⟩},{⟨1, 1⟩, ⟨5, 1⟩, ⟨6, 3⟩}], [{⟨1, 3⟩, ⟨2, 2⟩},{⟨5, 2⟩, ⟨6, 3⟩}]

---

su(6480) ← sp(3240), so(6480); sp(3240) ← su(2), sp(2), $\mathfrak{e}_7$

[{⟨1, 1⟩},{⟨6479, 1⟩}], [{⟨1, 1⟩}], [(6479)], [(5, 11)], [{⟨1, 1⟩, ⟨7, 1⟩}],[{⟨1, 1⟩}]

---

su(6490) ← sp(3245), so(6490), su(3); sp(3245) ← su(2)

[{⟨1, 1⟩},{⟨6489, 1⟩}], [{⟨1, 1⟩}], [(6489)], [{⟨1, 1⟩}], [(54, 3),(3, 54)]

---

su(6500) ← sp(3250), so(6500), su(4); sp(3250) ← su(2)

[{⟨1, 1⟩},{⟨6499, 1⟩}], [{⟨1, 1⟩}], [(6499)], [{⟨1, 1⟩}], [(4, 4, 2),(2, 4, 4)]

---

su(6512) ← sp(3256), so(6512); sp(3256) ← su(2); so(6512) ← so(33)

[{⟨1, 1⟩},{⟨6511, 1⟩}], [{⟨1, 1⟩}], [(6511)], [{⟨1, 1⟩}], [{⟨1, 3⟩}]

---

su(6525) ← so(6525); so(6525) ← su(2), so(5), so(27)

[{⟨1, 1⟩},{⟨6524, 1⟩}], [{⟨1, 1⟩}], [(6524)], [(1, 24)], [{⟨1, 1⟩, ⟨2, 1⟩}]

---

su(6545) ← so(6545), su(4), su(4), su(33), su(35); so(6545) ← su(2), so(5), so(7), so(35)

[{⟨1, 1⟩},{⟨6544, 1⟩}],[{⟨1, 1⟩}],[(6544)],[(0, 32)],[(5, 0, 2)], [{⟨3, 1⟩}], [(9, 0, 5),(5, 0, 9)], [(32, 0, 0),(0, 0, 32)],[{⟨1, 3⟩},{⟨32, 3⟩}],[{⟨3, 1⟩},{⟨32, 1⟩}]

---

su(6552) ← sp(3276), so(6552), su(27); sp(3276) ← su(2), sp(4)

[{⟨1, 1⟩},{⟨6551, 1⟩}],[{⟨1, 1⟩}],[(6551)],[(0, 2, 1, 0)], [{⟨1, 1⟩}],[{⟨1, 1⟩, ⟨2, 1⟩},{⟨25, 1⟩, ⟨26, 1⟩}]

---

su(6554) ← sp(3277), so(6554); sp(3277) ← su(2); so(6554) ← so(114)

[{⟨1, 1⟩},{⟨6553, 1⟩}], [{⟨1, 1⟩}], [(6553)], [{⟨1, 1⟩}], [{⟨1, 2⟩}]

---

su(6555) ← so(6555), su(3), su(3), su(114), su(115); so(6555) ← su(2), so(115), sp(57)

[{⟨1, 1⟩},{⟨6554, 1⟩}], [{⟨1, 1⟩}], [(6554)], [{⟨2, 1⟩}], [{⟨1, 2⟩}], [(22, 14),(14, 22)], [(113, 0),(0, 113)], [{⟨1, 2⟩},{⟨113, 2⟩}],[{⟨2, 1⟩},{⟨113, 1⟩}]

---

su(6560) ← sp(3280), so(6560), su(3); sp(3280) ← su(2); so(6560) ← su(81)

[{⟨1, 1⟩},{⟨6559, 1⟩}], [{⟨1, 1⟩}], [(6559)], [{⟨1, 1⟩}], [{⟨1, 1⟩, ⟨80, 1⟩}],[(79, 1),(1, 79)]

---

su(6561) ← so(6561); so(6561) ← su(2), so(5)

[{⟨1, 1⟩},{⟨6560, 1⟩}],[{⟨1, 1⟩}],[(6560)],[(8, 8)]

---

su(6579) ← so(6579), su(3); so(6579) ← su(2)

[{⟨1, 1⟩},{⟨6578, 1⟩}], [{⟨1, 1⟩}], [(6578)], [(33, 8),(8, 33)]

---

su(6580) ← sp(3290), so(6580), su(3); sp(3290) ← su(2)

[{⟨1, 1⟩},{⟨6579, 1⟩}], [{⟨1, 1⟩}], [(6579)], [{⟨1, 1⟩}], [(39, 6),(6, 39)]

---

su(6591) ← so(6591), su(3); so(6591) ← su(2)

[{⟨1, 1⟩},{⟨6590, 1⟩}], [{⟨1, 1⟩}], [(6590)], [(25, 12),(12, 25)]

---

su(6600) ← sp(3300), so(6600), su(3), su(4), su(5), su(8), su(24); sp(3300) ← su(2); so(6600) ← so(8)

[{⟨1, 1⟩},{⟨6599, 1⟩}], [{⟨1, 1⟩}], [(6599)], [{⟨1, 1⟩}], [(3, 0, 3, 0),(3, 0, 0, 3),(0, 0, 3, 3)], [(43, 5),(5, 43)], [(21, 1, 0),(0, 1, 21)], [(5, 3, 0, 0),(0, 0, 3, 5)], [{⟨1, 3⟩, ⟨4, 1⟩},{⟨4, 1⟩, ⟨7, 3⟩}], [{⟨1, 1⟩, ⟨22, 1⟩},{⟨2, 1⟩, ⟨23, 1⟩}]

---

su(6615) ← so(6615), su(3), su(5), su(7); so(6615) ← su(2)

[{⟨1, 1⟩},{⟨6614, 1⟩}], [{⟨1, 1⟩}], [(6614)], [(48, 4),(4, 48)], [(2, 3, 1, 0),(0, 1, 3, 2)], [{⟨1, 2⟩, ⟨2, 1⟩, ⟨5, 1⟩},{⟨2, 1⟩, ⟨5, 1⟩, ⟨6, 2⟩}]

---

su(6630) ← sp(3315), so(6630), su(3), su(4); sp(3315) ← su(2); so(6630) ← $\mathfrak{g}_2$

[{⟨1, 1⟩},{⟨6629, 1⟩}], [{⟨1, 1⟩}], [(6629)], [{⟨1, 1⟩}], [(0, 7)],[(64, 2),(2, 64)],[(12, 3, 0),(0, 3, 12)]

---

su(6650) ← sp(3325), so(6650), su(4); sp(3325) ← su(2)

[{⟨1, 1⟩},{⟨6649, 1⟩}], [{⟨1, 1⟩}], [(6649)], [{⟨1, 1⟩}], [(13, 0, 3),(3, 0, 13)]

---

su(6660) ← sp(3330), so(6660), su(3); sp(3330) ← su(2)

[{⟨1, 1⟩},{⟨6659, 1⟩}], [{⟨1, 1⟩}], [(6659)], [{⟨1, 1⟩}], [(36, 7),(7, 36)]

---

su(6669) ← so(6669); so(6669) ← su(2), so(115), sp(58)

[{⟨1, 1⟩},{⟨6668, 1⟩}], [{⟨1, 1⟩}], [(6668)], [{⟨1, 2⟩}], [{⟨2, 1⟩}]

---

su(6670) ← sp(3335), so(6670), su(3), su(115), su(116); sp(3335) ← su(2); so(6670) ← so(116)

[{⟨1, 1⟩},{⟨6669, 1⟩}], [{⟨1, 1⟩}], [(6669)], [{⟨1, 1⟩}], [{⟨2, 1⟩}], [(114, 0),(0, 114)], [{⟨1, 2⟩},{⟨114, 2⟩}], [{⟨2, 1⟩},{⟨114, 1⟩}]

---

su(6688) ← sp(3344), so(6688), su(3); sp(3344) ← su(2)

[{⟨1, 1⟩},{⟨6687, 1⟩}], [{⟨1, 1⟩}], [(6687)], [{⟨1, 1⟩}], [(21, 15),(15, 21)]

---

su(6699) ← so(6699); so(6699) ← su(2), so(5)

[{⟨1, 1⟩},{⟨6698, 1⟩}],[{⟨1, 1⟩}],[(6698)],[(10, 6)]

su(2), sp(2), sp(3) ← sp(3360)
su(6), so(6) ← so(6720)
sp(3360), so(6720), su(3), su(3), su(3), su(5), su(12), su(15) ← su(6720)

[{⟨1, 1⟩},{⟨6719, 1⟩}], [{⟨1, 1⟩}], [(6719)], [(7, 9)], [(3, 3, 0)], [{⟨1, 1⟩}], [(0, 2, 0, 2, 0)], [(9, 1, 1)], [(27, 11),(11, 27)], [(31, 9),(9, 31)], [(55, 3),(3, 55)], [(11, 1, 0, 0),(0, 0, 1, 11)], [{⟨1, 1⟩, ⟨2, 1⟩, ⟨11, 1⟩},{⟨1, 1⟩, ⟨10, 1⟩, ⟨11, 1⟩}],[{⟨1, 1⟩, ⟨12, 1⟩},{⟨3, 1⟩, ⟨14, 1⟩}]

---

su(2), su(82) ← so(6723)
so(6723), su(3) ← su(6723)

[{⟨1, 1⟩},{⟨6722, 1⟩}], [{⟨1, 1⟩}], [(6722)], [{⟨1, 1⟩, ⟨81, 1⟩}],[(80, 1),(1, 80)]

---

su(2) ← so(6765)
so(6765), su(3) ← su(6765)

[{⟨1, 1⟩},{⟨6764, 1⟩}], [{⟨1, 1⟩}], [(6764)], [(29, 10),(10, 29)]

---

su(2), so(17) ← so(6783)
so(6783), su(3) ← su(6783)

[{⟨1, 1⟩},{⟨6782, 1⟩}], [{⟨1, 1⟩}], [(6782)], [{⟨2, 2⟩}], [(20, 16),(16, 20)]

---

su(2), so(116) ← so(6785) ← su(6785)

[{⟨1, 1⟩},{⟨6784, 1⟩}],[{⟨1, 1⟩}],[(6784)],[{⟨1, 2⟩}]

---

su(2) ← sp(3393)
so(117), sp(58) ← so(6786)
sp(3393), so(6786), su(3), su(116), su(117) ← su(6786)

[{⟨1, 1⟩},{⟨6785, 1⟩}], [{⟨1, 1⟩}], [(6785)], [{⟨1, 1⟩}], [{⟨2, 1⟩}], [{⟨1, 2⟩}], [(115, 0),(0, 115)], [{⟨1, 2⟩},{⟨115, 2⟩}],[{⟨2, 1⟩},{⟨115, 1⟩}]

---

su(2) ← sp(3402)
so(5) ← so(6804)
sp(3402), so(6804), su(6) ← su(6804)

[{⟨1, 1⟩},{⟨6803, 1⟩}], [{⟨1, 1⟩}], [(6803)], [{⟨1, 1⟩}], [(2, 20)],[(1, 0, 2, 1, 0),(0, 1, 2, 0, 1)]

---

su(2), so(6) ← so(6825)
so(6825), su(3) ← su(6825)

[{⟨1, 1⟩},{⟨6824, 1⟩}], [{⟨1, 1⟩}], [(6824)], [(6, 2, 2)], [(24, 13),(13, 24)]

---

su(2) ← so(6831)
so(6831), su(3) ← su(6831)

[{⟨1, 1⟩},{⟨6830, 1⟩}], [{⟨1, 1⟩}], [(6830)], [(65, 2),(2, 65)]

---

su(2) ← sp(3420)
sp(3420), so(6840), su(3) ← su(6840)

[{⟨1, 1⟩},{⟨6839, 1⟩}], [{⟨1, 1⟩}], [(6839)], [{⟨1, 1⟩}], [(19, 17),(17, 19)]

---

su(2), su(3) ← so(6859) ← su(6859)

[{⟨1, 1⟩},{⟨6858, 1⟩}],[{⟨1, 1⟩}],[(6858)],[(18, 18)]

---

su(2) ← sp(3430)
sp(3430), so(6860), su(4), su(4), su(4) ← su(6860)

[{⟨1, 1⟩},{⟨6859, 1⟩}], [{⟨1, 1⟩}], [(6859)], [{⟨1, 1⟩}], [(6, 2, 3),(3, 2, 6)],[(6, 4, 1),(1, 4, 6)],[(6, 6, 0),(0, 6, 6)]

---

su(2), sp(2) ← sp(3432)
sp(5) ← so(6864)
sp(3432), so(6864) ← su(6864)

[{⟨1, 1⟩},{⟨6863, 1⟩}], [{⟨1, 1⟩}], [(6863)], [(17, 3)], [{⟨1, 1⟩}],[(2, 0, 0, 1, 0)]

---

su(2) ← so(6875)
so(6875), su(3), su(5) ← su(6875)

[{⟨1, 1⟩},{⟨6874, 1⟩}], [{⟨1, 1⟩}], [(6874)], [(49, 4),(4, 49)],[(4, 0, 3, 0),(0, 3, 0, 4)]

---

su(2), sp(8) ← so(6885)
so(6885), su(3) ← su(6885)

[{⟨1, 1⟩},{⟨6884, 1⟩}], [{⟨1, 1⟩}], [(6884)], [{⟨1, 1⟩, ⟨3, 1⟩}],[(44, 5),(5, 44)]

---

su(2) ← sp(3444)
su(83) ← so(6888)
sp(3444), so(6888), su(3), su(3) ← su(6888)

[{⟨1, 1⟩},{⟨6887, 1⟩}], [{⟨1, 1⟩}], [(6887)], [{⟨1, 1⟩}], [{⟨1, 1⟩, ⟨82, 1⟩}],[(40, 6),(6, 40)],[(81, 1),(1, 81)]

---

su(2) ← sp(3451)
so(117), sp(59) ← so(6902)
sp(3451), so(6902) ← su(6902)

[{⟨1, 1⟩},{⟨6901, 1⟩}], [{⟨1, 1⟩}], [(6901)], [{⟨1, 1⟩}], [{⟨1, 2⟩}],[{⟨2, 1⟩}]

---

su(2), so(118) ← so(6903)
so(6903), su(3), su(117), su(118) ← su(6903)

[{⟨1, 1⟩},{⟨6902, 1⟩}], [{⟨1, 1⟩}], [(6902)], [{⟨2, 1⟩}], [(116, 0),(0, 116)], [{⟨1, 2⟩},{⟨116, 2⟩}], [{⟨2, 1⟩},{⟨116, 1⟩}]

---

su(2), sp(2) ← sp(3458)
so(15) ← so(6916)
sp(3458), so(6916) ← su(6916)

[{⟨1, 1⟩},{⟨6915, 1⟩}], [{⟨1, 1⟩}], [(6915)], [(11, 6)], [{⟨1, 1⟩}],[{⟨1, 2⟩, ⟨2, 1⟩}]

---

su(2), sp(3) ← sp(3465)
so(5) ← so(6930)
sp(3465), so(6930), su(3), su(4), su(5), su(5), su(5), su(5), su(6), su(6), su(10), su(10), su(13), so(10), so(10) ← su(6930)

[{⟨1, 1⟩},{⟨6929, 1⟩}], [{⟨1, 1⟩}], [(6929)], [(5, 2, 0)], [{⟨1, 1⟩}], [(26, 0)], [(34, 8),(8, 34)], [(2, 10, 0),(0, 10, 2)], [(1, 6, 0, 0),(0, 0, 6, 1)], [(2, 5, 0, 0),(0, 0, 5, 2)], [(6, 1, 1, 0),(0, 1, 1, 6)], [(10, 0, 1, 0),(0, 1, 0, 10)], [(4, 0, 0, 1, 1),(1, 1, 0, 0, 4)], [(8, 0, 0, 0, 1),(1, 0, 0, 0, 8)], [{⟨2, 1⟩, ⟨4, 1⟩},{⟨6, 1⟩, ⟨8, 1⟩}], [{⟨1, 4⟩, ⟨9, 1⟩},{⟨1, 1⟩, ⟨9, 4⟩}],[{⟨1, 2⟩, ⟨11, 1⟩},{⟨2, 1⟩, ⟨12, 2⟩}],[(0, 0, 0, 3, 1),(0, 0, 0, 1, 3)],[(0, 0, 1, 2, 0),(0, 0, 1, 0, 2)]

---

su(2) ← sp(3468)
so(6) ← so(6936)
sp(3468), so(6936), su(17) ← su(6936)

[{⟨1, 1⟩},{⟨6935, 1⟩}], [{⟨1, 1⟩}], [(6935)], [{⟨1, 1⟩}], [(15, 0, 0)],[{⟨2, 2⟩},{⟨15, 2⟩}]

---

su(2) ← sp(3477)
sp(3477), so(6954), su(3) ← su(6954)

[{⟨1, 1⟩},{⟨6953, 1⟩}], [{⟨1, 1⟩}], [(6953)], [{⟨1, 1⟩}], [(56, 3),(3, 56)]

---

su(2) ← sp(3496)
sp(3496), so(6992), su(3) ← su(6992)

[{⟨1, 1⟩},{⟨6991, 1⟩}], [{⟨1, 1⟩}], [(6991)], [{⟨1, 1⟩}], [(37, 7),(7, 37)]

---

su(2) ← sp(3500)
sp(3500), so(7000), su(4), su(6) ← su(7000)

[{⟨1, 1⟩},{⟨6999, 1⟩}], [{⟨1, 1⟩}], [(6999)], [{⟨1, 1⟩}], [(7, 1, 4),(4, 1, 7)],[(2, 0, 0, 2, 1),(1, 2, 0, 0, 2)]

---

su(2), so(11) ← so(7007) ← su(7007)

[{⟨1, 1⟩},{⟨7006, 1⟩}], [{⟨1, 1⟩}], [(7006)], [(6, 0, 0, 0, 0)]

---

su(2) ← sp(3510)
sp(4), so(6), so(16), so(118) ← so(7020)
sp(3510), so(7020), su(3), su(3), su(4), su(4), su(4), su(9) ← su(7020)

[{⟨1, 1⟩},{⟨7019, 1⟩}], [{⟨1, 1⟩}], [(7019)], [{⟨1, 1⟩}], [(0, 2, 0, 1)],[(4, 3, 3)],[{⟨1, 1⟩, ⟨3, 1⟩}],[{⟨1, 2⟩}],[(23,

14),(14, 23)], [(26, 12),(12, 26)], [(3, 5, 2),(2, 5, 3)], [(8, 3, 1),(1, 3, 8)], [(11, 0, 4),(4, 0, 11)], [{⟨1, 3⟩, ⟨8, 2⟩}, {⟨1, 2⟩, ⟨8, 3⟩}]

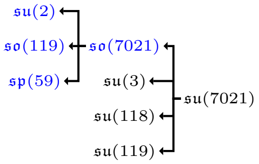


[{⟨1, 1⟩},{⟨7020, 1⟩}], [{⟨1, 1⟩}], [(7020)], [{⟨2, 1⟩}], [{⟨1, 2⟩}], [(117, 0),(0, 117)], [{⟨1, 2⟩},{⟨117, 2⟩}], [{⟨2, 1⟩},{⟨117, 1⟩}]

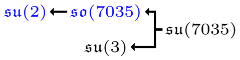


[{⟨1, 1⟩},{⟨7034, 1⟩}], [{⟨1, 1⟩}], [(7034)], [(66, 2),(2, 66)]

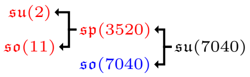


[{⟨1, 1⟩},{⟨7039, 1⟩}], [{⟨1, 1⟩}], [(7039)], [(3, 0, 0, 1)],[{⟨1, 1⟩}]

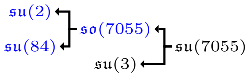


[{⟨1, 1⟩},{⟨7054, 1⟩}], [{⟨1, 1⟩}], [(7054)], [{⟨1, 1⟩, ⟨83, 1⟩}],[(82, 1),(1, 82)]

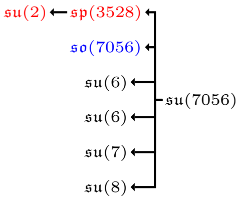


[{⟨1, 1⟩},{⟨7055, 1⟩}], [{⟨1, 1⟩}], [(7055)], [{⟨1, 1⟩}], [(0, 1, 3, 0, 0),(0, 0, 3, 1, 0)], [(0, 2, 2, 0, 0),(0, 0, 2, 2, 0)], [{⟨2, 1⟩, ⟨4, 2⟩},{⟨3, 2⟩, ⟨5, 1⟩}], [{⟨1, 1⟩, ⟨3, 2⟩},{⟨5, 2⟩, ⟨7, 1⟩}]

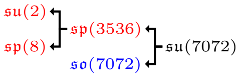


[{⟨1, 1⟩},{⟨7071, 1⟩}], [{⟨1, 1⟩}], [(7071)], [{⟨7, 1⟩}], [{⟨1, 1⟩}]

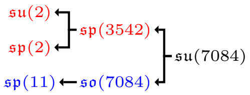


[{⟨1, 1⟩},{⟨7083, 1⟩}], [{⟨1, 1⟩}], [(7083)], [(1, 20)], [{⟨1, 1⟩}],[{⟨4, 1⟩}]

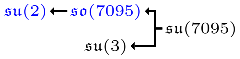


[{⟨1, 1⟩},{⟨7094, 1⟩}], [{⟨1, 1⟩}], [(7094)], [(32, 9),(9, 32)]

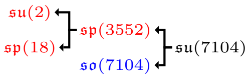


[{⟨1, 1⟩},{⟨7103, 1⟩}], [{⟨1, 1⟩}], [(7103)], [{⟨3, 1⟩}], [{⟨1, 1⟩}]

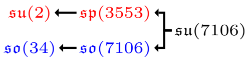


[{⟨1, 1⟩},{⟨7105, 1⟩}], [{⟨1, 1⟩}], [(7105)], [{⟨1, 1⟩}], [{⟨1, 3⟩}]

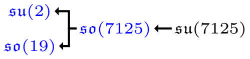


[{⟨1, 1⟩},{⟨7124, 1⟩}],[{⟨1, 1⟩}],[(7124)],[{⟨1, 4⟩}]

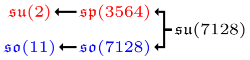


[{⟨1, 1⟩},{⟨7127, 1⟩}], [{⟨1, 1⟩}], [(7127)], [{⟨1, 1⟩}], [(2, 0, 1, 0, 0)]

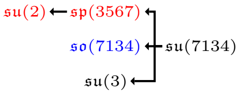


[{⟨1, 1⟩},{⟨7133, 1⟩}], [{⟨1, 1⟩}], [(7133)], [{⟨1, 1⟩}], [(28, 11),(11, 28)]

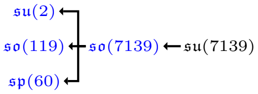


[{⟨1, 1⟩},{⟨7138, 1⟩}], [{⟨1, 1⟩}], [(7138)], [{⟨1, 2⟩}], [{⟨2, 1⟩}]

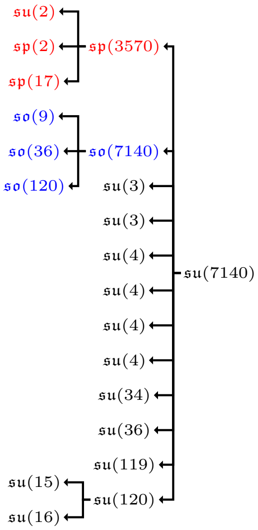


[{⟨1, 1⟩},{⟨7139, 1⟩}], [{⟨1, 1⟩}], [(7139)], [(33, 0)], [{⟨1, 3⟩}], [{⟨1, 1⟩}], [(4, 1, 0, 0)], [{⟨3, 1⟩}], [{⟨2, 1⟩}], [(50, 4),(4, 50)], [(118, 0),(0, 118)], [(8, 0, 6),(6, 0, 8)], [(11, 1, 2),(2, 1, 11)], [(16, 2, 0),(0, 2, 16)], [(33, 0, 0),(0, 0, 33)], [{⟨1, 3⟩},{⟨33, 3⟩}], [{⟨3, 1⟩},{⟨33, 1⟩}], [{⟨1, 2⟩},{⟨118, 2⟩}], [{⟨2, 1⟩},{⟨118, 1⟩}], [{⟨1, 2⟩, ⟨2, 1⟩},{⟨13, 1⟩, ⟨14, 2⟩}], [{⟨1, 1⟩, ⟨3, 1⟩},{⟨13, 1⟩, ⟨15, 1⟩}]

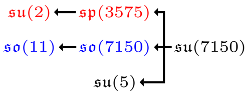


[{⟨1, 1⟩},{⟨7149, 1⟩}], [{⟨1, 1⟩}], [(7149)], [{⟨1, 1⟩}], [(1, 2, 0, 0, 0)],[(7, 1, 0, 1),(1, 0, 1, 7)]

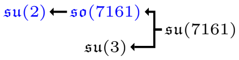


[{⟨1, 1⟩},{⟨7160, 1⟩}], [{⟨1, 1⟩}], [(7160)], [(30, 10),(10, 30)]

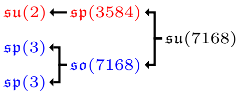


[{⟨1, 1⟩},{⟨7167, 1⟩}], [{⟨1, 1⟩}], [(7167)], [{⟨1, 1⟩}], [(1, 1, 3)],[(1, 3, 1)]

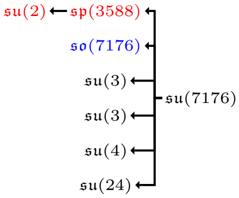


[{⟨1, 1⟩},{⟨7175, 1⟩}], [{⟨1, 1⟩}], [(7175)], [{⟨1, 1⟩}], [(22, 15),(15, 22)], [(45, 5),(5, 45)], [(22, 0, 1),(1, 0, 22)],[{⟨1, 2⟩, ⟨23, 1⟩},{⟨1, 1⟩, ⟨23, 2⟩}]

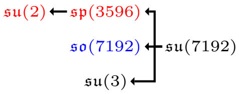


[{⟨1, 1⟩},{⟨7191, 1⟩}], [{⟨1, 1⟩}], [(7191)], [{⟨1, 1⟩}], [(57, 3),(3, 57)]

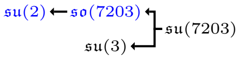


[{⟨1, 1⟩},{⟨7202, 1⟩}], [{⟨1, 1⟩}], [(7202)], [(41, 6),(6, 41)]

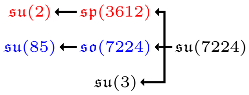


[{⟨1, 1⟩},{⟨7223, 1⟩}], [{⟨1, 1⟩}], [(7223)], [{⟨1, 1⟩}], [{⟨1, 1⟩, ⟨84, 1⟩}],[(83, 1),(1, 83)]

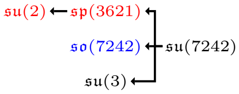


[{⟨1, 1⟩},{⟨7241, 1⟩}], [{⟨1, 1⟩}], [(7241)], [{⟨1, 1⟩}], [(67, 2),(2, 67)]

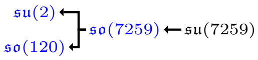


[{⟨1, 1⟩},{⟨7258, 1⟩}],[{⟨1, 1⟩}],[(7258)],[{⟨1, 2⟩}]

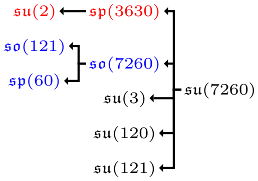


[{⟨1, 1⟩},{⟨7259, 1⟩}], [{⟨1, 1⟩}], [(7259)], [{⟨1, 1⟩}], [{⟨2, 1⟩}], [{⟨1, 2⟩}], [(119, 0),(0, 119)], [{⟨1, 2⟩},{⟨119, 2⟩}],[{⟨2, 1⟩},{⟨119, 1⟩}]

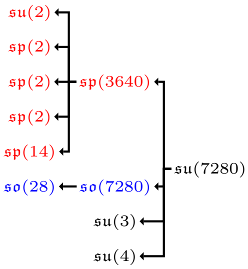


[{⟨1, 1⟩},{⟨7279, 1⟩}], [{⟨1, 1⟩}], [(7279)], [(13, 5)], [(15, 4)], [(25, 1)], [{⟨1, 1⟩, ⟨2, 1⟩}], [{⟨1, 1⟩}], [{⟨1, 1⟩, ⟨2, 1⟩}],[(25, 13),(13, 25)],[(1, 12, 0),(0, 12, 1)]

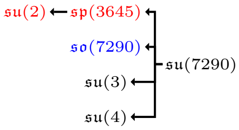


[{⟨1, 1⟩},{⟨7289, 1⟩}], [{⟨1, 1⟩}], [(7289)], [{⟨1, 1⟩}], [(35, 8),(8, 35)],[(8, 2, 2),(2, 2, 8)]

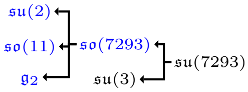


[{⟨1, 1⟩},{⟨7292, 1⟩}], [{⟨1, 1⟩}], [(7292)], [(3, 1, 0, 0, 0)],[(4, 3)],[(21, 16),(16, 21)]

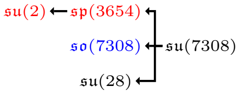


[{⟨1, 1⟩},{⟨7307, 1⟩}], [{⟨1, 1⟩}], [(7307)], [{⟨1, 1⟩}], [{⟨1, 1⟩, ⟨2, 1⟩},{⟨26, 1⟩, ⟨27, 1⟩}]

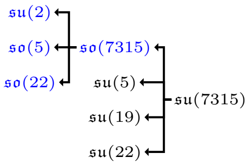

[{⟨1, 1⟩},{⟨7314, 1⟩}], [{⟨1, 1⟩}], [(7314)], [(13, 4)], [{⟨4, 1⟩}], [(18, 0, 0, 0),(0, 0, 0, 18)], [{⟨1, 4⟩},{⟨18, 4⟩}],[{⟨4, 1⟩},{⟨18, 1⟩}]

su(2) ← sp(3666)
so(7332) ← su(7332)
su(3)

[{⟨1, 1⟩},{⟨7331, 1⟩}], [{⟨1, 1⟩}], [(7331)], [{⟨1, 1⟩}], [(38, 7),(7, 38)]

su(2) ← sp(3672)
so(6) ← so(7344)
su(7344)

[{⟨1, 1⟩},{⟨7343, 1⟩}], [{⟨1, 1⟩}], [(7343)], [{⟨1, 1⟩}], [(0, 7, 7)]

su(2) ← sp(3675)
so(7350)
su(5)
su(7)
su(7)
su(8)
su(7350)

[{⟨1, 1⟩},{⟨7349, 1⟩}], [{⟨1, 1⟩}], [(7349)], [{⟨1, 1⟩}], [(1, 4, 1, 0),(0, 1, 4, 1)], [{⟨1, 1⟩, ⟨5, 3⟩},{⟨2, 3⟩, ⟨6, 1⟩}],[{⟨1, 2⟩, ⟨2, 1⟩, ⟨3, 1⟩},{⟨4, 1⟩, ⟨5, 1⟩, ⟨6, 2⟩}], [{⟨1, 1⟩, ⟨5, 1⟩, ⟨6, 1⟩},{⟨2, 1⟩, ⟨3, 1⟩, ⟨7, 1⟩}]

su(2)
so(5)
$\mathfrak{g}_2$ ← so(7)
$\mathfrak{e}_7$
so(7371)
su(3)
$\mathfrak{e}_6$
su(7371)

[{⟨1, 1⟩},{⟨7370, 1⟩}], [{⟨1, 1⟩}], [(7370)], [(17, 2)], [(11, 0, 0)], [(11, 0)], [{⟨1, 2⟩}], [(20, 17),(17, 20)], [{⟨1, 1⟩, ⟨5, 1⟩},{⟨3, 1⟩, ⟨6, 1⟩}]

su(2) ← sp(3690)
so(121)
sp(61)
so(7380)
su(7380)

[{⟨1, 1⟩},{⟨7379, 1⟩}], [{⟨1, 1⟩}], [(7379)], [{⟨1, 1⟩}], [{⟨1, 2⟩}],[{⟨2, 1⟩}]

su(2)
so(122)
so(7381)
su(3)
su(121)
su(122)
su(7381)

[{⟨1, 1⟩},{⟨7380, 1⟩}], [{⟨1, 1⟩}], [(7380)], [{⟨2, 1⟩}], [(120, 0),(0, 120)], [{⟨1, 2⟩},{⟨120, 2⟩}], [{⟨2, 1⟩},{⟨120, 1⟩}]

su(2)
sp(3)
sp(3696)
so(7)
so(7)
so(8)
so(8)
so(7392)
su(7392)

[{⟨1, 1⟩},{⟨7391, 1⟩}], [{⟨1, 1⟩}], [(7391)], [(0, 2, 3)], [{⟨1, 1⟩}], [(2, 2, 1)], [(4, 1, 1)], [(3, 1, 1, 0),(3, 1, 0, 1),(1, 1, 3, 0),(1, 1, 0, 3),(0, 1, 3, 1),(0, 1, 1, 3)], [(6, 0, 1, 0),(6, 0, 0, 1),(1, 0, 6, 0),(1, 0, 0, 6),(0, 0, 6, 1),(0, 0, 1, 6)]

su(2)
su(86)
so(7395)
su(3)
su(7395)

[{⟨1, 1⟩},{⟨7394, 1⟩}], [{⟨1, 1⟩}], [(7394)], [{⟨1, 1⟩, ⟨85, 1⟩}],[(84, 1),(1, 84)]

su(2) ← sp(3705)
so(7410)
su(3)
su(3)
su(7410)

[{⟨1, 1⟩},{⟨7409, 1⟩}], [{⟨1, 1⟩}], [(7409)], [{⟨1, 1⟩}], [(19, 18),(18, 19)],[(51, 4),(4, 51)]

su(2) ← so(7425)
su(5)
su(7425)

[{⟨1, 1⟩},{⟨7424, 1⟩}], [{⟨1, 1⟩}], [(7424)], [(4, 0, 2, 1),(1, 2, 0, 4)]

su(2) ← sp(3717)
so(7434) ← su(7434)
su(3)

[{⟨1, 1⟩},{⟨7433, 1⟩}], [{⟨1, 1⟩}], [(7433)], [{⟨1, 1⟩}], [(58, 3),(3, 58)]

su(2) ← sp(3726)
so(7452) ← su(7452)
su(3)

[{⟨1, 1⟩},{⟨7451, 1⟩}], [{⟨1, 1⟩}], [(7451)], [{⟨1, 1⟩}], [(68, 2),(2, 68)]

su(2) ← sp(3731)
so(7462) ← su(7462)
su(3)

[{⟨1, 1⟩},{⟨7461, 1⟩}], [{⟨1, 1⟩}], [(7461)], [{⟨1, 1⟩}], [(27, 12),(12, 27)]

su(2) ← so(7473)
su(3)
su(7473)

[{⟨1, 1⟩},{⟨7472, 1⟩}], [{⟨1, 1⟩}], [(7472)], [(46, 5),(5, 46)]

su(2) ← so(7475)
su(4) ← su(7475)
su(25)

[{⟨1, 1⟩},{⟨7474, 1⟩}], [{⟨1, 1⟩}], [(7474)], [(22, 1, 0),(0, 1, 22)],[{⟨1, 1⟩, ⟨23, 1⟩},{⟨2, 1⟩, ⟨24, 1⟩}]

su(2) ← sp(3740)
so(7480)
su(3)
su(4)
su(7480)

[{⟨1, 1⟩},{⟨7479, 1⟩}], [{⟨1, 1⟩}], [(7479)], [{⟨1, 1⟩}], [(33, 9),(9, 33)],[(10, 4, 0),(0, 4, 10)]

su(2) ← sp(3750)
so(7500) ← su(7500)
su(3)

[{⟨1, 1⟩},{⟨7499, 1⟩}], [{⟨1, 1⟩}], [(7499)], [{⟨1, 1⟩}], [(24, 14),(14, 24)]

su(2) ← sp(3751)
so(122) ← so(7502)
su(7502)

[{⟨1, 1⟩},{⟨7501, 1⟩}], [{⟨1, 1⟩}], [(7501)], [{⟨1, 1⟩}], [{⟨1, 2⟩}]

su(2)
so(123) ← so(7503)
sp(61)
su(3)
su(122)
su(123)
su(7503)

[{⟨1, 1⟩},{⟨7502, 1⟩}], [{⟨1, 1⟩}], [(7502)], [{⟨2, 1⟩}], [{⟨1, 2⟩}], [(121, 0),(0, 121)], [{⟨1, 2⟩},{⟨121, 2⟩}], [{⟨2, 1⟩},{⟨121, 1⟩}]

su(2) ← sp(3762)
so(5) ← so(7524) ← su(7524)
su(4)

[{⟨1, 1⟩},{⟨7523, 1⟩}], [{⟨1, 1⟩}], [(7523)], [{⟨1, 1⟩}], [(7, 10)],[(17, 0, 2),(2, 0, 17)]

su(2) ← so(7525)
su(3)
su(7525)

[{⟨1, 1⟩},{⟨7524, 1⟩}], [{⟨1, 1⟩}], [(7524)], [(42, 6),(6, 42)]

su(2) ← sp(3773)
so(7546) ← su(7546)
su(4)

[{⟨1, 1⟩},{⟨7545, 1⟩}], [{⟨1, 1⟩}], [(7545)], [{⟨1, 1⟩}], [(6, 3, 2),(2, 3, 6)]

su(2) ← sp(3780)
so(7) ← so(7560)
su(3)
su(4)
su(4) ← su(7560)
su(4)
su(4)
su(7)
su(9)

[{⟨1, 1⟩},{⟨7559, 1⟩}], [{⟨1, 1⟩}], [(7559)], [{⟨1, 1⟩}], [(2, 3, 0)], [(29, 11),(11, 29)], [(5, 2, 4),(4, 2, 5)], [(5, 7, 0),(0, 7, 5)], [(6, 1, 5),(5, 1, 6)], [(8, 5, 0),(0, 5, 8)], [{⟨2, 1⟩, ⟨3, 1⟩, ⟨5, 1⟩},{⟨2, 1⟩, ⟨4, 1⟩, ⟨5, 1⟩}], [{⟨3, 1⟩, ⟨5, 1⟩},{⟨4, 1⟩, ⟨6, 1⟩}]

su(2) ← sp(3784)
su(87) ← so(7568)
su(3)
su(3)
su(7568)

[{⟨1, 1⟩},{⟨7567, 1⟩}], [{⟨1, 1⟩}], [(7567)], [{⟨1, 1⟩}], [{⟨1, 1⟩, ⟨86, 1⟩}],[(31, 10),(10, 31)],[(85, 1),(1, 85)]

su(2)
so(123) ← so(7625) ← su(7625)
sp(62)

[{⟨1, 1⟩},{⟨7624, 1⟩}], [{⟨1, 1⟩}], [(7624)], [{⟨1, 2⟩}], [{⟨2, 1⟩}]

su(2) ← sp(3813)
so(124) ← so(7626)
su(3) ← su(7626)
su(123)
su(124)

[{⟨1, 1⟩},{⟨7625, 1⟩}], [{⟨1, 1⟩}], [(7625)], [{⟨1, 1⟩}], [{⟨2, 1⟩}], [(122, 0),(0, 122)], [{⟨1, 2⟩},{⟨122, 2⟩}], [{⟨2, 1⟩},{⟨122, 1⟩}]

su(2) ← sp(3822)
so(10) ← so(7644)
su(7644)

[{⟨1, 1⟩},{⟨7643, 1⟩}], [{⟨1, 1⟩}], [(7643)], [{⟨1, 1⟩}], [(0, 3, 0, 0, 0)]

su(2) ← sp(3825)
so(7650) ← su(7650)
su(4)

[{⟨1, 1⟩},{⟨7649, 1⟩}], [{⟨1, 1⟩}], [(7649)], [{⟨1, 1⟩}], [(11, 2, 1),(1, 2, 11)]

su(2) ← so(7659)
su(3)
su(7659)

[{⟨1, 1⟩},{⟨7658, 1⟩}], [{⟨1, 1⟩}], [(7658)], [(36, 8),(8, 36)]

su(2) ← so(7665)
su(3)
su(7665)

[{⟨1, 1⟩},{⟨7664, 1⟩}], [{⟨1, 1⟩}], [(7664)], [(69, 2),(2, 69)]

su(2), sp(2) ← sp(3840); sp(3840), so(7680), su(3), su(3), su(3), su(4), su(4), su(8) ← su(7680)

[{⟨1, 1⟩},{⟨7679, 1⟩}], [{⟨1, 1⟩}], [(7679)], [(3, 15)], [{⟨1, 1⟩}], [(23, 15),(15, 23)], [(39, 7),(7, 39)], [(59, 3),(3, 59)], [(9, 1, 3),(3, 1, 9)], [(15, 1, 1),(1, 1, 15)], [{⟨1, 1⟩, ⟨2, 1⟩, ⟨5, 1⟩},{⟨3, 1⟩, ⟨6, 1⟩, ⟨7, 1⟩}]

---

su(2) ← so(7685); so(7685), su(3) ← su(7685)

[{⟨1, 1⟩},{⟨7684, 1⟩}], [{⟨1, 1⟩}], [(7684)], [(52, 4),(4, 52)]

---

su(2), sp(2) ← sp(3850); so(9), sp(3) ← so(7700); sp(3850), so(7700), su(4) ← su(7700)

[{⟨1, 1⟩},{⟨7699, 1⟩}], [{⟨1, 1⟩}], [(7699)], [(21, 2)], [{⟨1, 1⟩}],[(3, 0, 1, 0)],[(0, 3, 2)],[(3, 9, 0),(0, 9, 3)]

---

su(2) ← sp(3857); so(5) ← so(7714); sp(3857), so(7714) ← su(7714)

[{⟨1, 1⟩},{⟨7713, 1⟩}], [{⟨1, 1⟩}], [(7713)], [{⟨1, 1⟩}], [(27, 0)]

---

su(2) ← sp(3861); so(7), so(13), sp(3), g2 ← so(7722); sp(3861), so(7722), su(11), e6 ← su(7722)

[{⟨1, 1⟩},{⟨7721, 1⟩}], [{⟨1, 1⟩}], [(7721)], [{⟨1, 1⟩}], [(1, 2, 2)], [{⟨1, 1⟩, ⟨4, 1⟩}], [(8, 1, 0)], [(8, 1)], [{⟨1, 2⟩, ⟨3, 1⟩},{⟨8, 1⟩, ⟨10, 2⟩}], [{⟨1, 2⟩, ⟨6, 1⟩},{⟨1, 1⟩, ⟨6, 2⟩}]

---

su(2), so(35) ← so(7735); so(7735), su(5), su(14) ← su(7735)

[{⟨1, 1⟩},{⟨7734, 1⟩}], [{⟨1, 1⟩}], [(7734)], [{⟨1, 3⟩}], [(12, 0, 0, 1),(1, 0, 0, 12)], [{⟨1, 3⟩, ⟨13, 1⟩},{⟨1, 1⟩, ⟨13, 3⟩}]

---

su(2), su(88) ← so(7743); so(7743), su(3) ← su(7743)

[{⟨1, 1⟩},{⟨7742, 1⟩}], [{⟨1, 1⟩}], [(7742)], [{⟨1, 1⟩, ⟨87, 1⟩}],[(86, 1),(1, 86)]

---

su(2), so(124) ← so(7749); so(7749), su(3) ← su(7749)

[{⟨1, 1⟩},{⟨7748, 1⟩}], [{⟨1, 1⟩}], [(7748)], [{⟨1, 2⟩}], [(26, 13),(13, 26)]

---

su(2) ← sp(3875); so(125), sp(62) ← so(7750); sp(3875), so(7750), su(3), su(124), su(125) ← su(7750)

[{⟨1, 1⟩},{⟨7749, 1⟩}], [{⟨1, 1⟩}], [(7749)], [{⟨1, 1⟩}], [{⟨2, 1⟩}], [{⟨1, 2⟩}], [(123, 0),(0, 123)], [{⟨1, 2⟩},{⟨123, 2⟩}],[{⟨2, 1⟩},{⟨123, 1⟩}]

---

su(2), sp(9) ← sp(3876); sp(3876), so(7752) ← su(7752)

[{⟨1, 1⟩},{⟨7751, 1⟩}], [{⟨1, 1⟩}], [(7751)], [{⟨5, 1⟩}], [{⟨1, 1⟩}]

---

su(2) ← sp(3885); so(5), so(37) ← so(7770); sp(3885), so(7770), su(4), su(35), su(37) ← su(7770)

[{⟨1, 1⟩},{⟨7769, 1⟩}], [{⟨1, 1⟩}], [(7769)], [{⟨1, 1⟩}], [(0, 34)], [{⟨3, 1⟩}], [(34, 0, 0),(0, 0, 34)], [{⟨1, 3⟩},{⟨34, 3⟩}],[{⟨3, 1⟩},{⟨34, 1⟩}]

---

su(2) ← sp(3888); so(8) ← so(7776); sp(3888), so(7776), su(3), su(5) ← su(7776)

[{⟨1, 1⟩},{⟨7775, 1⟩}], [{⟨1, 1⟩}], [(7775)], [{⟨1, 1⟩}], [(5, 1, 0, 0),(0, 1, 5, 0),(0, 1, 0, 5)], [(47, 5),(5, 47)], [(5, 1, 0, 2),(2, 0, 1, 5)]

---

su(2), sp(6) ← sp(3900); sp(3900), so(7800) ← su(7800)

[{⟨1, 1⟩},{⟨7799, 1⟩}], [{⟨1, 1⟩}], [(7799)], [{⟨2, 1⟩, ⟨3, 1⟩}],[{⟨1, 1⟩}]

---

su(2) ← sp(3910); sp(3910), so(7820), su(3) ← su(7820)

[{⟨1, 1⟩},{⟨7819, 1⟩}], [{⟨1, 1⟩}], [(7819)], [{⟨1, 1⟩}], [(22, 16),(16, 22)]

---

su(2) ← sp(3920); so(8) ← so(7840); sp(3920), so(7840) ← su(7840)

[{⟨1, 1⟩},{⟨7839, 1⟩}], [{⟨1, 1⟩}], [(7839)], [{⟨1, 1⟩}], [(1, 3, 0, 0),(0, 3, 1, 0),(0, 3, 0, 1)]

---

su(2) ← sp(3927); sp(3927), so(7854), su(3) ← su(7854)

[{⟨1, 1⟩},{⟨7853, 1⟩}], [{⟨1, 1⟩}], [(7853)], [{⟨1, 1⟩}], [(43, 6),(6, 43)]

---

su(2), so(11), sp(5) ← so(7865); so(7865), su(11) ← su(7865)

[{⟨1, 1⟩},{⟨7864, 1⟩}], [{⟨1, 1⟩}], [(7864)], [(0, 0, 2, 0, 0)],[(0, 0, 0, 2, 0)],[{⟨1, 1⟩, ⟨2, 2⟩},{⟨9, 2⟩, ⟨10, 1⟩}]

---

su(2) ← sp(3933); so(5) ← so(7866); sp(3933), so(7866) ← su(7866)

[{⟨1, 1⟩},{⟨7865, 1⟩}], [{⟨1, 1⟩}], [(7865)], [{⟨1, 1⟩}], [(3, 18)]

---

su(2) ← sp(3937); so(125), sp(63) ← so(7874); sp(3937), so(7874) ← su(7874)

[{⟨1, 1⟩},{⟨7873, 1⟩}], [{⟨1, 1⟩}], [(7873)], [{⟨1, 1⟩}], [{⟨1, 2⟩}],[{⟨2, 1⟩}]

---

su(2), so(126) ← so(7875); so(7875), su(3), su(3), su(4), su(5), su(6), su(6), su(125), su(126) ← su(7875)

[{⟨1, 1⟩},{⟨7874, 1⟩}], [{⟨1, 1⟩}], [(7874)], [{⟨2, 1⟩}], [(34, 9),(9, 34)], [(124, 0),(0, 124)], [(4, 8, 0),(0, 8, 4)], [(2, 1, 3, 0),(0, 3, 1, 2)],[(2, 0, 0, 3, 0),(0, 3, 0, 0, 2)],[(3, 0, 1, 1, 0),(0, 1, 1, 0, 3)], [{⟨1, 2⟩},{⟨124, 2⟩}], [{⟨2, 1⟩},{⟨124, 1⟩}]

---

su(2) ← so(7881); so(7881), su(3) ← su(7881)

[{⟨1, 1⟩},{⟨7880, 1⟩}], [{⟨1, 1⟩}], [(7880)], [(70, 2),(2, 70)]

---

su(2), sp(2) ← sp(3952); sp(3952), so(7904) ← su(7904)

[{⟨1, 1⟩},{⟨7903, 1⟩}], [{⟨1, 1⟩}], [(7903)], [(5, 12)], [{⟨1, 1⟩}]

---

su(2) ← so(7917); so(7917), su(3) ← su(7917)

[{⟨1, 1⟩},{⟨7916, 1⟩}], [{⟨1, 1⟩}], [(7916)], [(28, 12),(12, 28)]

---

su(2) ← sp(3960); su(89) ← so(7920); sp(3960), so(7920), su(3), su(3), su(9), su(10), so(10) ← su(7920)

[{⟨1, 1⟩},{⟨7919, 1⟩}], [{⟨1, 1⟩}], [(7919)], [{⟨1, 1⟩}], [{⟨1, 1⟩, ⟨88, 1⟩}], [(21, 17),(17, 21)], [(87, 1),(1, 87)], [{⟨1, 1⟩, ⟨2, 1⟩, ⟨7, 1⟩},{⟨2, 1⟩, ⟨7, 1⟩, ⟨8, 1⟩}], [{⟨1, 1⟩, ⟨8, 2⟩},{⟨2, 2⟩, ⟨9, 1⟩}],[(4, 0, 0, 1, 0),(4, 0, 0, 0, 1)]

---

su(2) ← sp(3965); sp(3965), so(7930), su(3) ← su(7930)

[{⟨1, 1⟩},{⟨7929, 1⟩}], [{⟨1, 1⟩}], [(7929)], [{⟨1, 1⟩}], [(60, 3),(3, 60)]

---

su(2) ← so(7965); so(7965), su(3) ← su(7965)

[{⟨1, 1⟩},{⟨7964, 1⟩}], [{⟨1, 1⟩}], [(7964)], [(53, 4),(4, 53)]

---

su(2), sp(2) ← sp(3990); sp(3990), so(7980), su(3), su(4) ← su(7980)

[{⟨1, 1⟩},{⟨7979, 1⟩}], [{⟨1, 1⟩}], [(7979)], [(9, 8)], [{⟨1, 1⟩}],[(20, 18),(18, 20)],[(13, 3, 0),(0, 3, 13)]

---

su(2) ← sp(3993); sp(3993), so(7986), su(3) ← su(7986)

[{⟨1, 1⟩},{⟨7985, 1⟩}], [{⟨1, 1⟩}], [(7985)], [{⟨1, 1⟩}], [(32, 10),(10, 32)]

---

su(2) ← so(7995); so(7995), su(3) ← su(7995)

[{⟨1, 1⟩},{⟨7994, 1⟩}], [{⟨1, 1⟩}], [(7994)], [(25, 14),

(14, 25)]

su(2) ⟵ sp(3999)
so(7998) ⟵ su(7998)
su(3)

[{⟨1, 1⟩},{⟨7997, 1⟩}], [{⟨1, 1⟩}], [(7997)], [{⟨1, 1⟩}], [(30, 11),(11, 30)]

su(2) ⟵ sp(4000)
su(3), so(126) ⟵ so(8000) ⟵ su(8000)
su(4)

[{⟨1, 1⟩},{⟨7999, 1⟩}], [{⟨1, 1⟩}], [(7999)], [{⟨1, 1⟩}], [(19, 19)],[{⟨1, 2⟩}],[(14, 0, 3),(3, 0, 14)]

su(2), so(127), sp(63) ⟵ so(8001)
su(3)
su(126) ⟵ su(8001)
su(127)

[{⟨1, 1⟩},{⟨8000, 1⟩}], [{⟨1, 1⟩}], [(8000)], [{⟨2, 1⟩}], [{⟨1, 2⟩}], [(125, 0),(0, 125)], [{⟨1, 2⟩},{⟨125, 2⟩}], [{⟨2, 1⟩},{⟨125, 1⟩}]

su(2), sp(4) ⟵ sp(4004)
so(7)
so(7) ⟵ so(8)
so(12) ⟵ so(8008)
so(14)
so(16)
su(7), su(11), su(11), su(13), su(16) ⟵ su(8008)

[{⟨1, 1⟩},{⟨8007, 1⟩}], [{⟨1, 1⟩}], [(8007)], [(0, 0, 3, 0)], [{⟨1, 1⟩}], [(0, 3, 2)], [(9, 0, 0, 0),(0, 0, 9, 0),(0, 0, 0, 9)], [(0, 0, 9)], [{⟨2, 1⟩, ⟨3, 1⟩}], [{⟨1, 5⟩}], [{⟨6, 1⟩}], [{⟨1, 10⟩},{⟨6, 10⟩}], [{⟨1, 3⟩, ⟨2, 1⟩},{⟨9, 1⟩, ⟨10, 3⟩}], [{⟨1, 6⟩},{⟨10, 6⟩}], [{⟨1, 1⟩, ⟨4, 1⟩},{⟨9, 1⟩, ⟨12, 1⟩}],[{⟨6, 1⟩},{⟨10, 1⟩}]

su(2) ⟵ sp(4018)
so(8036) ⟵ su(8036)
su(3)

[{⟨1, 1⟩},{⟨8035, 1⟩}], [{⟨1, 1⟩}], [(8035)], [{⟨1, 1⟩}], [(40, 7),(7, 40)]

su(2) ⟵ so(8037)
su(3) ⟵ su(8037)

[{⟨1, 1⟩},{⟨8036, 1⟩}], [{⟨1, 1⟩}], [(8036)], [(37, 8),(8, 37)]

su(2) ⟵ sp(4032)
so(8064)
su(4) ⟵ su(8064)
su(6)
so(10)

[{⟨1, 1⟩},{⟨8063, 1⟩}], [{⟨1, 1⟩}], [(8063)], [{⟨1, 1⟩}], [(5, 5, 1),(1, 5, 5)],[(1, 1, 1, 1, 0),(0, 1, 1, 1, 1)],[(0, 2, 0, 1, 0),(0, 2, 0, 0, 1)]

su(2), su(14), so(10), so(12) ⟵ so(8085)
su(3) ⟵ su(8085)
su(7)

[{⟨1, 1⟩},{⟨8084, 1⟩}], [{⟨1, 1⟩}], [(8084)], [{⟨2, 1⟩, ⟨12, 1⟩}], [(2, 0, 0, 1, 1)], [{⟨1, 1⟩, ⟨5, 1⟩, ⟨6, 1⟩}], [(48, 5),(5, 48)], [{⟨1, 3⟩, ⟨5, 1⟩, ⟨6, 1⟩},{⟨1, 1⟩, ⟨2, 1⟩, ⟨6, 3⟩}]

su(2), so(5), so(29) ⟵ so(8091) ⟵ su(8091)

[{⟨1, 1⟩},{⟨8090, 1⟩}], [{⟨1, 1⟩}], [(8090)], [(1, 26)], [{⟨1, 1⟩, ⟨2, 1⟩}]

su(2), sp(2) ⟵ sp(4048)
so(8096) ⟵ su(8096)

[{⟨1, 1⟩},{⟨8095, 1⟩}], [{⟨1, 1⟩}], [(8095)], [(1, 21)], [{⟨1, 1⟩}]

su(2), su(90) ⟵ so(8099)
su(3) ⟵ su(8099)

[{⟨1, 1⟩},{⟨8098, 1⟩}], [{⟨1, 1⟩}], [(8098)], [{⟨1, 1⟩, ⟨89, 1⟩}],[(88, 1),(1, 88)]

su(2) ⟵ sp(4050)
so(8100)
su(3)
su(4) ⟵ su(8100)
su(5)
su(8)
su(25)

[{⟨1, 1⟩},{⟨8099, 1⟩}], [{⟨1, 1⟩}], [(8099)], [{⟨1, 1⟩}], [(71, 2),(2, 71)], [(23, 0, 1),(1, 0, 23)], [(0, 4, 2, 0),(0, 2, 4, 0)], [{⟨2, 2⟩, ⟨6, 1⟩},{⟨2, 1⟩, ⟨6, 2⟩}], [{⟨1, 2⟩, ⟨24, 1⟩},{⟨1, 1⟩, ⟨24, 2⟩}]

su(2) ⟵ sp(4056)
su(13) ⟵ so(8112) ⟵ su(8112)

[{⟨1, 1⟩},{⟨8111, 1⟩}], [{⟨1, 1⟩}], [(8111)], [{⟨1, 1⟩}], [{⟨1, 2⟩, ⟨12, 2⟩}]

su(2) ⟵ sp(4060)
so(8120) ⟵ su(8120)
su(29)

[{⟨1, 1⟩},{⟨8119, 1⟩}], [{⟨1, 1⟩}], [(8119)], [{⟨1, 1⟩}], [{⟨1, 1⟩, ⟨2, 1⟩},{⟨27, 1⟩, ⟨28, 1⟩}]

su(2), so(127), sp(64) ⟵ so(8127) ⟵ su(8127)

[{⟨1, 1⟩},{⟨8126, 1⟩}], [{⟨1, 1⟩}], [(8126)], [{⟨1, 2⟩}], [{⟨2, 1⟩}]

su(2) ⟵ sp(4064)
so(128) ⟵ so(8128)
su(3) ⟵ su(8128)
su(127)
su(128)

[{⟨1, 1⟩},{⟨8127, 1⟩}], [{⟨1, 1⟩}], [(8127)], [{⟨1, 1⟩}], [{⟨2, 1⟩}], [(126, 0),(0, 126)], [{⟨1, 2⟩},{⟨126, 2⟩}], [{⟨2, 1⟩},{⟨126, 1⟩}]

su(2) ⟵ sp(4092)
so(8184) ⟵ su(8184)
su(3)

[{⟨1, 1⟩},{⟨8183, 1⟩}], [{⟨1, 1⟩}], [(8183)], [{⟨1, 1⟩}], [(61, 3),(3, 61)]

su(2) ⟵ sp(4095)
so(5), sp(3) ⟵ so(8190)
su(3) ⟵ su(8190)
su(5)
su(6)

[{⟨1, 1⟩},{⟨8189, 1⟩}], [{⟨1, 1⟩}], [(8189)], [{⟨1, 1⟩}], [(6, 12)], [(3, 0, 3)], [(44, 6),(6, 44)], [(8, 2, 0, 0),(0, 0, 2, 8)],[(6, 0, 0, 0, 2),(2, 0, 0, 0, 6)]

su(2) ⟵ sp(4096)
so(27) ⟵ so(28)
so(8192) ⟵ su(8192)

[{⟨1, 1⟩},{⟨8191, 1⟩}], [{⟨1, 1⟩}], [(8191)], [{⟨13, 1⟩}, {⟨14, 1⟩}],[{⟨13, 1⟩}],[{⟨1, 1⟩}]

su(2) ⟵ sp(4100)
so(8200) ⟵ su(8200)
su(3)

[{⟨1, 1⟩},{⟨8199, 1⟩}], [{⟨1, 1⟩}], [(8199)], [{⟨1, 1⟩}], [(24, 15),(15, 24)]

su(2) ⟵ sp(4116)
so(8232)
su(3) ⟵ su(8232)
su(7)

[{⟨1, 1⟩},{⟨8231, 1⟩}], [{⟨1, 1⟩}], [(8231)], [{⟨1, 1⟩}], [(27, 13),(13, 27)],[{⟨3, 2⟩, ⟨4, 1⟩},{⟨3, 1⟩, ⟨4, 2⟩}]

su(2) ⟵ sp(4123)
so(5) ⟵ so(8246) ⟵ su(8246)

[{⟨1, 1⟩},{⟨8245, 1⟩}], [{⟨1, 1⟩}], [(8245)], [{⟨1, 1⟩}], [(11, 6)]

su(2) ⟵ sp(4125)
sp(5) ⟵ so(8250)
su(3)
su(5) ⟵ su(8250)
su(5)
su(10)

[{⟨1, 1⟩},{⟨8249, 1⟩}], [{⟨1, 1⟩}], [(8249)], [{⟨1, 1⟩}], [(0, 3, 0, 0, 0)], [(54, 4),(4, 54)], [(4, 2, 1, 0),(0, 1, 2, 4)], [(9, 0, 0, 2),(2, 0, 0, 9)], [{⟨2, 1⟩, ⟨6, 1⟩},{⟨4, 1⟩, ⟨8, 1⟩}]

su(2), so(128) ⟵ so(8255) ⟵ su(8255)

[{⟨1, 1⟩},{⟨8254, 1⟩}],[{⟨1, 1⟩}],[(8254)],[{⟨1, 2⟩}]

su(2) ⟵ sp(4128)
so(129), sp(64) ⟵ so(8256)
su(3) ⟵ su(8256)
su(128)
su(129)

[{⟨1, 1⟩},{⟨8255, 1⟩}], [{⟨1, 1⟩}], [(8255)], [{⟨1, 1⟩}], [{⟨2, 1⟩}], [{⟨1, 2⟩}], [(127, 0),(0, 127)], [{⟨1, 2⟩},{⟨127, 2⟩}],[{⟨2, 1⟩},{⟨127, 1⟩}]

su(2), so(5) ⟵ so(8265) ⟵ su(8265)

[{⟨1, 1⟩},{⟨8264, 1⟩}],[{⟨1, 1⟩}],[(8264)],[(9, 8)]

su(2) ⟵ sp(4140)
su(91) ⟵ so(8280) ⟵ su(8280)
su(3)
su(3)

[{⟨1, 1⟩},{⟨8279, 1⟩}], [{⟨1, 1⟩}], [(8279)], [{⟨1, 1⟩}], [{⟨1, 1⟩, ⟨90, 1⟩}],[(35, 9),(9, 35)],[(89, 1),(1, 89)]

su(2), sp(3) ⟵ sp(4158)
so(8316)
su(4)
su(4) ⟵ su(8316)
su(4)
su(7)
su(8)
su(9)

[{⟨1, 1⟩},{⟨8315, 1⟩}], [{⟨1, 1⟩}], [(8315)], [(1, 2, 2)],

[{⟨1, 1⟩}], [(2, 8, 1),(1, 8, 2)], [(10, 0, 5),(5, 0, 10)], [(17, 2, 0),(0, 2, 17)], [{⟨1, 5⟩, ⟨5, 1⟩},{⟨2, 1⟩, ⟨6, 5⟩}], [{⟨1, 4⟩, ⟨6, 1⟩},{⟨2, 1⟩, ⟨7, 4⟩}], [{⟨1, 1⟩, ⟨4, 1⟩, ⟨8, 1⟩},{⟨1, 1⟩, ⟨5, 1⟩, ⟨8, 1⟩}]

---

su(2) ← sp(4161) ←
so(8322) ← su(8322)
su(3) ←

[{⟨1, 1⟩},{⟨8321, 1⟩}], [{⟨1, 1⟩}], [(8321)], [{⟨1, 1⟩}], [(72, 2),(2, 72)]

---

su(2), sp(2) ← sp(4180) ←
so(8360) ← su(8360)

[{⟨1, 1⟩},{⟨8359, 1⟩}], [{⟨1, 1⟩}], [(8359)], [(7, 10)], [{⟨1, 1⟩}]

---

su(2) ← sp(4182) ←
so(8364) ← su(8364)
su(3) ←

[{⟨1, 1⟩},{⟨8363, 1⟩}], [{⟨1, 1⟩}], [(8363)], [{⟨1, 1⟩}], [(23, 16),(16, 23)]

---

su(2) ← sp(4186) ←
$\mathfrak{g}_2$ ← so(8372) ← su(8372)

[{⟨1, 1⟩},{⟨8371, 1⟩}], [{⟨1, 1⟩}], [(8371)], [{⟨1, 1⟩}], [(6, 2)]

---

su(2) ← sp(4192) ←
so(129), sp(65) ← so(8384) ← su(8384)

[{⟨1, 1⟩},{⟨8383, 1⟩}], [{⟨1, 1⟩}], [(8383)], [{⟨1, 1⟩}], [{⟨1, 2⟩}],[{⟨2, 1⟩}]

---

su(2), so(130) ← so(8385) ←
su(3), su(3), su(129), su(130) ← su(8385)

[{⟨1, 1⟩},{⟨8384, 1⟩}], [{⟨1, 1⟩}], [(8384)], [{⟨2, 1⟩}], [(29, 12),(12, 29)], [(128, 0),(0, 128)], [{⟨1, 2⟩},{⟨128, 2⟩}],[{⟨2, 1⟩},{⟨128, 1⟩}]

---

su(2), sp(19) ← sp(4199) ←
so(8398) ← su(8398)

[{⟨1, 1⟩},{⟨8397, 1⟩}], [{⟨1, 1⟩}], [(8397)], [{⟨3, 1⟩}], [{⟨1, 1⟩}]

---

su(2) ← sp(4200) ←
so(36) ← so(8400) ←
su(3), su(3), su(5), su(5), su(5), su(8), su(8) ← su(8400)

[{⟨1, 1⟩},{⟨8399, 1⟩}], [{⟨1, 1⟩}], [(8399)], [{⟨1, 1⟩}], [{⟨1, 3⟩}], [(41, 7),(7, 41)], [(49, 5),(5, 49)], [(1, 1, 4, 0),(0, 4, 1, 1)], [(2, 2, 1, 1),(1, 1, 2, 2)], [(7, 0, 0, 3),(3, 0, 0, 7)], [{⟨1, 1⟩, ⟨5, 2⟩},{⟨3, 2⟩, ⟨7, 1⟩}], [{⟨1, 1⟩, ⟨2, 1⟩, ⟨4, 1⟩},{⟨4, 1⟩, ⟨6, 1⟩, ⟨7, 1⟩}]

---

su(2), so(5) ← so(8415) ←
su(3) ← su(8415)

[{⟨1, 1⟩},{⟨8414, 1⟩}], [{⟨1, 1⟩}], [(8414)], [(4, 16)], [(33, 10),(10, 33)]

---

su(2) ← sp(4212) ←
$\mathfrak{f}_4$ ← so(8424) ←
su(3), su(4), su(26) ← su(8424)

[{⟨1, 1⟩},{⟨8423, 1⟩}], [{⟨1, 1⟩}], [(8423)], [{⟨1, 1⟩}], [(1, 0, 1, 0)], [(38, 8),(8, 38)], [(23, 1, 0),(0, 1, 23)], [{⟨1, 1⟩, ⟨24, 1⟩},{⟨2, 1⟩, ⟨25, 1⟩}]

---

su(2), sp(2), sp(18) ← sp(4218) ←
so(38) ← so(8436) ←
su(4), su(36), su(38) ← su(8436)

[{⟨1, 1⟩},{⟨8435, 1⟩}], [{⟨1, 1⟩}], [(8435)], [(35, 0)], [{⟨1, 3⟩}], [{⟨1, 1⟩}], [{⟨3, 1⟩}], [(35, 0, 0),(0, 0, 35)], [{⟨1, 3⟩},{⟨35, 3⟩}],[{⟨3, 1⟩},{⟨35, 1⟩}]

---

su(2) ← sp(4221) ←
so(8442) ← su(8442)
su(3) ←

[{⟨1, 1⟩},{⟨8441, 1⟩}], [{⟨1, 1⟩}], [(8441)], [{⟨1, 1⟩}], [(62, 3),(3, 62)]

---

su(2) ← sp(4224) ←
so(8448) ← su(8448)
su(3) ←

[{⟨1, 1⟩},{⟨8447, 1⟩}], [{⟨1, 1⟩}], [(8447)], [{⟨1, 1⟩}], [(31, 11),(11, 31)]

---

su(2), su(92) ← so(8463) ←
su(3) ← su(8463)

[{⟨1, 1⟩},{⟨8462, 1⟩}], [{⟨1, 1⟩}], [(8462)], [{⟨1, 1⟩, ⟨91, 1⟩}],[(90, 1),(1, 90)]

---

su(2) ← sp(4235) ←
so(8470) ← su(8470)
su(11) ←

[{⟨1, 1⟩},{⟨8469, 1⟩}], [{⟨1, 1⟩}], [(8469)], [{⟨1, 1⟩}], [{⟨2, 1⟩, ⟨8, 1⟩},{⟨3, 1⟩, ⟨9, 1⟩}]

---

su(2) ← so(8487) ←
su(3) ← su(8487)

[{⟨1, 1⟩},{⟨8486, 1⟩}], [{⟨1, 1⟩}], [(8486)], [(22, 17),(17, 22)]

---

su(2), so(5) ← so(8505) ←
su(3), su(5), su(5), su(9) ← su(8505)

[{⟨1, 1⟩},{⟨8504, 1⟩}], [{⟨1, 1⟩}], [(8504)], [(5, 14)], [(26, 14),(14, 26)], [(2, 2, 2, 0),(0, 2, 2, 2)], [(5, 0, 1, 2),(2, 1, 0, 5)], [{⟨1, 2⟩, ⟨2, 1⟩, ⟨8, 1⟩},{⟨1, 1⟩, ⟨7, 1⟩, ⟨8, 2⟩}]

---

su(2) ← sp(4257) ←
so(130) ← so(8514) ← su(8514)

[{⟨1, 1⟩},{⟨8513, 1⟩}], [{⟨1, 1⟩}], [(8513)], [{⟨1, 1⟩}], [{⟨1, 2⟩}]

---

su(2), so(131), sp(65) ← so(8515) ←
su(3), su(130), su(131) ← su(8515)

[{⟨1, 1⟩},{⟨8514, 1⟩}], [{⟨1, 1⟩}], [(8514)], [{⟨2, 1⟩}], [{⟨1, 2⟩}], [(129, 0),(0, 129)], [{⟨1, 2⟩},{⟨129, 2⟩}], [{⟨2, 1⟩},{⟨129, 1⟩}]

---

su(2) ← so(8533) ←
su(3) ← su(8533)

[{⟨1, 1⟩},{⟨8532, 1⟩}], [{⟨1, 1⟩}], [(8532)], [(45, 6),(6, 45)]

---

su(2) ← sp(4270) ←
so(8540) ← su(8540)
su(3) ←

[{⟨1, 1⟩},{⟨8539, 1⟩}], [{⟨1, 1⟩}], [(8539)], [{⟨1, 1⟩}], [(55, 4),(4, 55)]

---

su(2) ← so(8547) ←
su(3) ← su(8547)

[{⟨1, 1⟩},{⟨8546, 1⟩}], [{⟨1, 1⟩}], [(8546)], [(73, 2),(2, 73)]

---

su(2) ← sp(4275) ←
so(18) ← so(8550) ← su(8550)

[{⟨1, 1⟩},{⟨8549, 1⟩}], [{⟨1, 1⟩}], [(8549)], [{⟨1, 1⟩}], [{⟨2, 2⟩}]

---

su(2), so(5) ← so(8555) ← su(8555)

[{⟨1, 1⟩},{⟨8554, 1⟩}],[{⟨1, 1⟩}],[(8554)],[(28, 0)]

---

su(2), sp(3), sp(7) ← sp(4284) ←
so(7), sp(3), sp(9), so(18) ← so(8568) ←
su(6), su(14), su(18) ← su(8568)

[{⟨1, 1⟩},{⟨8567, 1⟩}], [{⟨1, 1⟩}], [(8567)], [(13, 0, 0)], [{⟨1, 5⟩}], [{⟨1, 1⟩}], [(4, 2, 0)], [(0, 6, 0)], [{⟨2, 2⟩}], [{⟨5, 1⟩}], [(13, 0, 0, 0, 0),(0, 0, 0, 0, 13)], [{⟨1, 5⟩},{⟨13, 5⟩}],[{⟨5, 1⟩},{⟨13, 1⟩}]

---

su(2), so(5) ← so(8569) ←
su(3) ← su(8569)

[{⟨1, 1⟩},{⟨8568, 1⟩}], [{⟨1, 1⟩}], [(8568)], [(18, 2)], [(21, 18),(18, 21)]

---

su(2) ← sp(4290) ←
sp(5) ← so(8580) ←
su(5), su(9), su(12), su(12) ← su(8580)

[{⟨1, 1⟩},{⟨8579, 1⟩}], [{⟨1, 1⟩}], [(8579)], [{⟨1, 1⟩}], [(0, 0, 1, 0, 1)], [(7, 0, 1, 1),(1, 1, 0, 7)], [{⟨1, 4⟩, ⟨2, 1⟩},{⟨7, 1⟩, ⟨8, 4⟩}], [{⟨2, 1⟩, ⟨3, 1⟩},{⟨9, 1⟩, ⟨10, 1⟩}], [{⟨1, 1⟩, ⟨5, 1⟩},{⟨7, 1⟩, ⟨11, 1⟩}]

---

su(2) ← sp(4305) ←
so(8610) ← su(8610)
su(3) ←

[{⟨1, 1⟩},{⟨8609, 1⟩}], [{⟨1, 1⟩}], [(8609)], [{⟨1, 1⟩}], [(20, 19),(19, 20)]

---

su(2) ← sp(4312) ←
so(7) ← so(8624) ←
su(5), su(6) ← su(8624)

[{⟨1, 1⟩},{⟨8623, 1⟩}], [{⟨1, 1⟩}], [(8623)], [{⟨1, 1⟩}], [(2, 0, 5)],[(3, 2, 0, 2),(2, 0, 2, 3)],[(3, 1, 0, 0, 2),(2, 0, 0, 1, 3)]

---

su(2) ← , so(131) ← , sp(66) ← , so(20) ← , $\mathfrak{e}_7$ ← so(8645); so(8645), su(4) ← su(8645)

[{⟨1, 1⟩},{⟨8644, 1⟩}], [{⟨1, 1⟩}], [(8644)], [{⟨1, 2⟩}], [{⟨2, 1⟩}],[{⟨1, 4⟩}],[{⟨3, 1⟩}],[(12, 0, 4),(4, 0, 12)]

---

su(2) ← sp(4323); so(132) ← so(8646); sp(4323), so(8646), su(3), su(131), su(132) ← su(8646)

[{⟨1, 1⟩},{⟨8645, 1⟩}], [{⟨1, 1⟩}], [(8645)], [{⟨1, 1⟩}], [{⟨2, 1⟩}], [(130, 0),(0, 130)], [{⟨1, 2⟩},{⟨130, 2⟩}], [{⟨2, 1⟩},{⟨130, 1⟩}]

---

su(2) ← sp(4324); su(93) ← so(8648); sp(4324), so(8648), su(3) ← su(8648)

[{⟨1, 1⟩},{⟨8647, 1⟩}], [{⟨1, 1⟩}], [(8647)], [{⟨1, 1⟩}], [{⟨1, 1⟩, ⟨92, 1⟩}],[(91, 1),(1, 91)]

---

su(2), so(5) ← so(8671) ← su(8671)

[{⟨1, 1⟩},{⟨8670, 1⟩}],[{⟨1, 1⟩}],[(8670)],[(2, 22)]

---

su(2) ← so(8695); so(8695), su(3) ← su(8695)

[{⟨1, 1⟩},{⟨8694, 1⟩}], [{⟨1, 1⟩}], [(8694)], [(36, 9),(9, 36)]

---

su(2) ← sp(4352); sp(4352), so(8704), su(3) ← su(8704)

[{⟨1, 1⟩},{⟨8703, 1⟩}], [{⟨1, 1⟩}], [(8703)], [{⟨1, 1⟩}], [(63, 3),(3, 63)]

---

su(2), so(6) ← so(8721); so(8721), su(3), su(18) ← su(8721)

[{⟨1, 1⟩},{⟨8720, 1⟩}], [{⟨1, 1⟩}], [(8720)], [(16, 0, 0)], [(50, 5),(5, 50)],[{⟨2, 2⟩},{⟨16, 2⟩}]

---

su(2) ← so(8729); so(8729), su(3) ← su(8729)

[{⟨1, 1⟩},{⟨8728, 1⟩}], [{⟨1, 1⟩}], [(8728)], [(28, 13),(13, 28)]

---

su(2) ← sp(4368); sp(4368), so(8736), su(3) ← su(8736)

[{⟨1, 1⟩},{⟨8735, 1⟩}], [{⟨1, 1⟩}], [(8735)], [{⟨1, 1⟩}], [(25, 15),(15, 25)]

---

su(2) ← sp(4370); sp(4370), so(8740), su(4) ← su(8740)

[{⟨1, 1⟩},{⟨8739, 1⟩}], [{⟨1, 1⟩}], [(8739)], [{⟨1, 1⟩}], [(18, 0, 2),(2, 0, 18)]

---

su(2) ← sp(4374); so(9) ← so(8748); sp(4374), so(8748) ← su(8748)

[{⟨1, 1⟩},{⟨8747, 1⟩}], [{⟨1, 1⟩}], [(8747)], [{⟨1, 1⟩}], [(2, 2, 0, 0)]

---

su(2) ← sp(4375); so(5) ← so(8750); sp(4375), so(8750), su(5) ← su(8750)

[{⟨1, 1⟩},{⟨8749, 1⟩}], [{⟨1, 1⟩}], [(8749)], [{⟨1, 1⟩}], [(14, 4)],[(2, 1, 2, 1),(1, 2, 1, 2)]

---

su(2) ← sp(4386); sp(4386), so(8772), su(3) ← su(8772)

[{⟨1, 1⟩},{⟨8771, 1⟩}], [{⟨1, 1⟩}], [(8771)], [{⟨1, 1⟩}], [(42, 7),(7, 42)]

---

su(2) ← so(8775); so(8775), su(3), su(4) ← su(8775)

[{⟨1, 1⟩},{⟨8774, 1⟩}], [{⟨1, 1⟩}], [(8774)], [(74, 2),(2, 74)],[(12, 1, 2),(2, 1, 12)]

---

su(2), so(132) ← so(8777) ← su(8777)

[{⟨1, 1⟩},{⟨8776, 1⟩}],[{⟨1, 1⟩}],[(8776)],[{⟨1, 2⟩}]

---

su(2) ← sp(4389); so(133), sp(66) ← so(8778); sp(4389), so(8778), su(3), su(132), su(133) ← su(8778)

[{⟨1, 1⟩},{⟨8777, 1⟩}], [{⟨1, 1⟩}], [(8777)], [{⟨1, 1⟩}], [{⟨2, 1⟩}], [{⟨1, 2⟩}], [(131, 0),(0, 131)], [{⟨1, 2⟩},{⟨131, 2⟩}],[{⟨2, 1⟩},{⟨131, 1⟩}]

---

su(2), so(12) ← sp(4400); so(7), so(8) ← so(8800); sp(4400), so(8800), so(10) ← su(8800)

[{⟨1, 1⟩},{⟨8799, 1⟩}], [{⟨1, 1⟩}], [(8799)], [{⟨4, 1⟩, ⟨5, 1⟩},{⟨4, 1⟩, ⟨6, 1⟩}], [{⟨1, 1⟩}], [(4, 0, 3)], [(4, 0, 1, 1),(1, 0, 4, 1),(1, 0, 1, 4)],[(1, 0, 1, 1, 0),(1, 0, 1, 0, 1)]

---

su(2) ← sp(4410); su(9) ← so(8820); sp(4410), so(8820), su(3), su(4), su(6), su(7), su(8) ← su(8820)

[{⟨1, 1⟩},{⟨8819, 1⟩}], [{⟨1, 1⟩}], [(8819)], [{⟨1, 1⟩}], [{⟨4, 1⟩, ⟨5, 1⟩}], [(39, 8),(8, 39)], [(4, 6, 1),(1, 6, 4)], [(1, 0, 0, 4, 0),(0, 4, 0, 0, 1)], [{⟨1, 2⟩, ⟨3, 2⟩},{⟨4, 2⟩, ⟨6, 2⟩}],[{⟨1, 1⟩, ⟨3, 1⟩, ⟨6, 1⟩},{⟨2, 1⟩, ⟨5, 1⟩, ⟨7, 1⟩}]

---

su(2), su(94) ← so(8835); so(8835), su(3), su(3) ← su(8835)

[{⟨1, 1⟩},{⟨8834, 1⟩}], [{⟨1, 1⟩}], [(8834)], [{⟨1, 1⟩, ⟨93, 1⟩}],[(56, 4),(4, 56)],[(92, 1),(1, 92)]

---

su(2) ← sp(4420); sp(4420), so(8840), su(5), su(16) ← su(8840)

[{⟨1, 1⟩},{⟨8839, 1⟩}], [{⟨1, 1⟩}], [(8839)], [{⟨1, 1⟩}], [(12, 1, 0, 0),(0, 0, 1, 12)], [{⟨1, 1⟩, ⟨13, 1⟩},{⟨3, 1⟩, ⟨15, 1⟩}]

---

su(2), so(23), sp(10) ← so(8855); so(8855), su(3), su(5), su(20), su(23) ← su(8855)

[{⟨1, 1⟩},{⟨8854, 1⟩}], [{⟨1, 1⟩}], [(8854)], [{⟨4, 1⟩}], [{⟨1, 4⟩}],[(34, 10),(10, 34)],[(19, 0, 0, 0),(0, 0, 0, 19)], [{⟨1, 4⟩},{⟨19, 4⟩}],[{⟨4, 1⟩},{⟨19, 1⟩}]

---

su(2) ← sp(4433); sp(4433), so(8866), su(3) ← su(8866)

[{⟨1, 1⟩},{⟨8865, 1⟩}], [{⟨1, 1⟩}], [(8865)], [{⟨1, 1⟩}], [(30, 12),(12, 30)]

---

su(2) ← so(8883); so(8883), su(3) ← su(8883)

[{⟨1, 1⟩},{⟨8882, 1⟩}], [{⟨1, 1⟩}], [(8882)], [(46, 6),(6, 46)]

---

su(2) ← sp(4455); so(133), sp(67), so(8), so(10) ← so(8910); sp(4455), so(8910), su(3), su(6), su(6) ← su(8910)

[{⟨1, 1⟩},{⟨8909, 1⟩}], [{⟨1, 1⟩}], [(8909)], [{⟨1, 1⟩}], [{⟨1, 2⟩}],[{⟨2, 1⟩}],[(2, 1, 2, 0),(2, 1, 0, 2),(0, 1, 2, 2)], [(0, 0, 0, 2, 2)], [(32, 11),(11, 32)], [(4, 0, 1, 0, 1),(1, 0, 1, 0, 4)],[(5, 2, 0, 0, 0),(0, 0, 0, 2, 5)]

---

su(2), so(134) ← so(8911); so(8911), su(3), su(133), su(134) ← su(8911)

[{⟨1, 1⟩},{⟨8910, 1⟩}], [{⟨1, 1⟩}], [(8910)], [{⟨2, 1⟩}], [(132, 0),(0, 132)], [{⟨1, 2⟩},{⟨132, 2⟩}], [{⟨2, 1⟩},{⟨132, 1⟩}]

---

su(2), sp(3) ← sp(4459); so(7), so(8) ← so(8918); sp(4459), so(8918) ← su(8918)

[{⟨1, 1⟩},{⟨8917, 1⟩}], [{⟨1, 1⟩}], [(8917)], [(5, 0, 2)], [{⟨1, 1⟩}],[(0, 5, 0)],[(0, 4, 0, 0)]

---

su(2), so(16) ← so(8925); so(8925), su(3) ← su(8925)

[{⟨1, 1⟩},{⟨8924, 1⟩}], [{⟨1, 1⟩}], [(8924)], [{⟨1, 2⟩, ⟨2, 1⟩}],[(24, 16),(16, 24)]

---

su(2), sp(2), sp(2), sp(2), sp(15) ← sp(4480); so(30) ← so(8960); sp(4480), so(8960), su(4), su(4), su(4), su(4), su(6) ← su(8960)

[{⟨1, 1⟩},{⟨8959, 1⟩}], [{⟨1, 1⟩}], [(8959)], [(11, 7)], [(19, 3)], [(27, 1)], [{⟨1, 1⟩, ⟨2, 1⟩}], [{⟨1, 1⟩}], [{⟨1, 1⟩, ⟨2, 1⟩}],[(3, 7, 1),(1, 7, 3)],[(5, 3, 3),(3, 3, 5)],[(7, 6, 0),(0, 6, 7)], [(9, 3, 1),(1, 3, 9)], [(1, 3, 0, 0, 1),(1, 0, 0, 3, 1)]

---

su(2) ← sp(4485); sp(4485), so(8970), su(3) ← su(8970)

[{⟨1, 1⟩},{⟨8969, 1⟩}], [{⟨1, 1⟩}], [(8969)], [{⟨1, 1⟩}], [(64, 3),(3, 64)]

$\mathfrak{su}(2) \leftarrow \mathfrak{sp}(4495)$, $\mathfrak{so}(8990)$, $\mathfrak{su}(30)$ → $\mathfrak{su}(8990)$

[{⟨1,1⟩},{⟨8989,1⟩}], [{⟨1,1⟩}], [(8989)], [{⟨1,1⟩}], [{⟨1,1⟩,⟨2,1⟩},{⟨28,1⟩,⟨29,1⟩}]

---

$\mathfrak{su}(2) \leftarrow \mathfrak{sp}(4500)$, $\mathfrak{su}(5) \leftarrow \mathfrak{so}(9000)$ → $\mathfrak{su}(9000)$

[{⟨1,1⟩},{⟨8999,1⟩}], [{⟨1,1⟩}], [(8999)], [{⟨1,1⟩}], [(0,3,3,0)]

---

$\mathfrak{su}(2) \leftarrow \mathfrak{sp}(4503)$, $\mathfrak{so}(9006)$, $\mathfrak{su}(3)$ → $\mathfrak{su}(9006)$

[{⟨1,1⟩},{⟨9005,1⟩}], [{⟨1,1⟩}], [(9005)], [{⟨1,1⟩}], [(75,2),(2,75)]

---

$\mathfrak{su}(2)$, $\mathfrak{so}(7)$, $\mathfrak{so}(7)$, $\mathfrak{so}(9)$, $\mathfrak{sp}(4)$, $\mathfrak{sp}(4)$ → $\mathfrak{so}(9009)$; $\mathfrak{so}(9009)$, $\mathfrak{su}(6)$, $\mathfrak{su}(7)$, $\mathfrak{su}(12)$, $\mathfrak{su}(13)$ → $\mathfrak{su}(9009)$

[{⟨1,1⟩},{⟨9008,1⟩}], [{⟨1,1⟩}], [(9008)], [(0,1,6)], [(1,1,4)], [(1,1,1,0)], [(0,1,0,2)], [(4,0,0,1)], [(8,1,0,0,0),(0,0,0,1,8)], [{⟨1,6⟩,⟨2,1⟩},{⟨5,1⟩,⟨6,6⟩}], [{⟨1,1⟩,⟨7,1⟩},{⟨5,1⟩,⟨11,1⟩}], [{⟨1,1⟩,⟨9,1⟩},{⟨4,1⟩,⟨12,1⟩}]

---

$\mathfrak{su}(2) \leftarrow \mathfrak{sp}(4512)$, $\mathfrak{su}(95) \leftarrow \mathfrak{so}(9024)$, $\mathfrak{su}(3)$ → $\mathfrak{su}(9024)$

[{⟨1,1⟩},{⟨9023,1⟩}], [{⟨1,1⟩}], [(9023)], [{⟨1,1⟩}], [{⟨1,1⟩,⟨94,1⟩}],[(93,1),(1,93)]

---

$\mathfrak{su}(2) \leftarrow \mathfrak{sp}(4515)$, $\mathfrak{so}(9030)$, $\mathfrak{su}(3)$ → $\mathfrak{su}(9030)$

[{⟨1,1⟩},{⟨9029,1⟩}], [{⟨1,1⟩}], [(9029)], [{⟨1,1⟩}], [(27,14),(14,27)]

---

$\mathfrak{su}(2)$, $\mathfrak{sp}(2)$ → $\mathfrak{sp}(4522)$; $\mathfrak{so}(17)$, $\mathfrak{sp}(8)$, $\mathfrak{so}(134)$ → $\mathfrak{so}(9044)$; $\mathfrak{sp}(4522)$, $\mathfrak{so}(9044)$, $\mathfrak{su}(4)$ → $\mathfrak{su}(9044)$

[{⟨1,1⟩},{⟨9043,1⟩}], [{⟨1,1⟩}], [(9043)], [(3,16)], [{⟨1,1⟩}],[{⟨1,1⟩,⟨3,1⟩}],[{⟨1,2⟩,⟨2,1⟩}],[{⟨1,2⟩}], [(16,1,1),(1,1,16)]

---

$\mathfrak{su}(2)$, $\mathfrak{so}(135)$, $\mathfrak{sp}(67)$ → $\mathfrak{so}(9045)$; $\mathfrak{so}(9045)$, $\mathfrak{su}(3)$, $\mathfrak{su}(134)$, $\mathfrak{su}(135)$ → $\mathfrak{su}(9045)$

[{⟨1,1⟩},{⟨9044,1⟩}], [{⟨1,1⟩}], [(9044)], [{⟨2,1⟩}], [{⟨1,2⟩}], [(133,0),(0,133)], [{⟨1,2⟩},{⟨133,2⟩}], [{⟨2,1⟩},{⟨133,1⟩}]

---

$\mathfrak{su}(2) \leftarrow \mathfrak{sp}(4524)$, $\mathfrak{so}(9048)$, $\mathfrak{su}(3)$ → $\mathfrak{su}(9048)$

[{⟨1,1⟩},{⟨9047,1⟩}], [{⟨1,1⟩}], [(9047)], [{⟨1,1⟩}], [(51,5),(5,51)]

---

$\mathfrak{su}(2) \leftarrow \mathfrak{sp}(4536)$, $\mathfrak{so}(9072)$, $\mathfrak{su}(3)$, $\mathfrak{su}(8)$ → $\mathfrak{su}(9072)$

[{⟨1,1⟩},{⟨9071,1⟩}], [{⟨1,1⟩}], [(9071)], [{⟨1,1⟩}], [(23,17),(17,23)],[{⟨2,2⟩,⟨3,1⟩},{⟨5,1⟩,⟨6,2⟩}]

---

$\mathfrak{su}(2) \leftarrow \mathfrak{so}(9075)$, $\mathfrak{su}(5)$, $\mathfrak{su}(10)$, $\mathfrak{su}(11)$ → $\mathfrak{su}(9075)$

[{⟨1,1⟩},{⟨9074,1⟩}], [{⟨1,1⟩}], [(9074)], [(0,8,0,0),(0,0,8,0)],[{⟨2,3⟩},{⟨8,3⟩}],[{⟨3,2⟩},{⟨8,2⟩}]

---

$\mathfrak{su}(2) \leftarrow \mathfrak{sp}(4550)$, $\mathfrak{so}(9100)$, $\mathfrak{su}(4)$, $\mathfrak{su}(4)$, $\mathfrak{su}(26)$ → $\mathfrak{su}(9100)$

[{⟨1,1⟩},{⟨9099,1⟩}], [{⟨1,1⟩}], [(9099)], [{⟨1,1⟩}], [(7,4,1),(1,4,7)], [(24,0,1),(1,0,24)], [{⟨1,2⟩,⟨25,1⟩},{⟨1,1⟩,⟨25,2⟩}]

---

$\mathfrak{su}(2) \leftarrow \mathfrak{sp}(4551)$, $\mathfrak{so}(37) \leftarrow \mathfrak{so}(9102)$ → $\mathfrak{su}(9102)$

[{⟨1,1⟩},{⟨9101,1⟩}], [{⟨1,1⟩}], [(9101)], [{⟨1,1⟩}], [{⟨1,3⟩}]

---

$\mathfrak{su}(2) \leftarrow \mathfrak{sp}(4560)$, $\mathfrak{so}(9120)$, $\mathfrak{su}(3)$ → $\mathfrak{su}(9120)$

[{⟨1,1⟩},{⟨9119,1⟩}], [{⟨1,1⟩}], [(9119)], [{⟨1,1⟩}], [(37,9),(9,37)]

---

$\mathfrak{su}(2) \leftarrow \mathfrak{so}(9135)$, $\mathfrak{su}(3)$ → $\mathfrak{su}(9135)$

[{⟨1,1⟩},{⟨9134,1⟩}], [{⟨1,1⟩}], [(9134)], [(57,4),(4,57)]

---

$\mathfrak{su}(2)$, $\mathfrak{so}(5)$, $\mathfrak{so}(39)$ → $\mathfrak{so}(9139)$; $\mathfrak{so}(9139)$, $\mathfrak{su}(4)$, $\mathfrak{su}(37)$, $\mathfrak{su}(39)$ → $\mathfrak{su}(9139)$

[{⟨1,1⟩},{⟨9138,1⟩}], [{⟨1,1⟩}], [(9138)], [(0,36)], [{⟨3,1⟩}], [(36,0,0),(0,0,36)], [{⟨1,3⟩},{⟨36,3⟩}], [{⟨3,1⟩},{⟨36,1⟩}]

---

$\mathfrak{su}(2)$, $\mathfrak{sp}(5)$, $\mathfrak{so}(12)$ → $\mathfrak{sp}(4576)$, $\mathfrak{so}(9152)$; $\mathfrak{sp}(4576)$, $\mathfrak{so}(9152)$, $\mathfrak{su}(3)$ → $\mathfrak{su}(9152)$

[{⟨1,1⟩},{⟨9151,1⟩}], [{⟨1,1⟩}], [(9151)], [(0,0,1,1,0)],[{⟨1,3⟩,⟨5,1⟩},{⟨1,3⟩,⟨6,1⟩}],[{⟨1,1⟩}],[(43,7),(7,43)]

---

$\mathfrak{su}(2)$, $\mathfrak{g}_2$ → $\mathfrak{so}(9177)$; $\mathfrak{so}(9177)$, $\mathfrak{su}(3)$ → $\mathfrak{su}(9177)$

[{⟨1,1⟩},{⟨9176,1⟩}],[{⟨1,1⟩}],[(9176)],[(3,4)],[(22,18),(18,22)]

---

$\mathfrak{su}(2)$, $\mathfrak{so}(135)$, $\mathfrak{sp}(68)$ → $\mathfrak{so}(9179) \leftarrow \mathfrak{su}(9179)$

[{⟨1,1⟩},{⟨9178,1⟩}], [{⟨1,1⟩}], [(9178)], [{⟨1,2⟩}], [{⟨2,1⟩}]

---

$\mathfrak{su}(2) \leftarrow \mathfrak{sp}(4590)$, $\mathfrak{so}(136) \leftarrow \mathfrak{so}(9180)$, $\mathfrak{su}(3)$, $\mathfrak{su}(4)$, $\mathfrak{su}(135)$, $\mathfrak{su}(136)$ → $\mathfrak{su}(9180)$; $\mathfrak{su}(16)$, $\mathfrak{su}(17)$ → $\mathfrak{su}(136)$

[{⟨1,1⟩},{⟨9179,1⟩}], [{⟨1,1⟩}], [(9179)], [{⟨1,1⟩}], [{⟨2,1⟩}], [(134,0),(0,134)], [(11,4,0),(0,4,11)], [{⟨1,2⟩},{⟨134,2⟩}], [{⟨2,1⟩},{⟨134,1⟩}], [{⟨1,2⟩,⟨2,1⟩},{⟨14,1⟩,⟨15,2⟩}], [{⟨1,1⟩,⟨3,1⟩},{⟨14,1⟩,⟨16,1⟩}]

---

$\mathfrak{su}(2)$, $\mathfrak{sp}(2)$ → $\mathfrak{sp}(4600)$; $\mathfrak{sp}(4600)$, $\mathfrak{so}(9200)$ → $\mathfrak{su}(9200)$

[{⟨1,1⟩},{⟨9199,1⟩}], [{⟨1,1⟩}], [(9199)], [(1,22)], [{⟨1,1⟩}]

---

$\mathfrak{su}(2)$, $\mathfrak{su}(96)$ → $\mathfrak{so}(9215)$; $\mathfrak{so}(9215)$, $\mathfrak{su}(3)$ → $\mathfrak{su}(9215)$

[{⟨1,1⟩},{⟨9214,1⟩}], [{⟨1,1⟩}], [(9214)], [{⟨1,1⟩,⟨95,1⟩}],[(94,1),(1,94)]

---

$\mathfrak{su}(2)$, $\mathfrak{so}(19)$ → $\mathfrak{sp}(4608)$; $\mathfrak{sp}(4608)$, $\mathfrak{so}(9216)$ → $\mathfrak{su}(9216)$

[{⟨1,1⟩},{⟨9215,1⟩}], [{⟨1,1⟩}], [(9215)], [{⟨1,1⟩,⟨9,1⟩}],[{⟨1,1⟩}]

---

$\mathfrak{su}(2) \leftarrow \mathfrak{so}(9225)$, $\mathfrak{su}(3)$ → $\mathfrak{su}(9225)$

[{⟨1,1⟩},{⟨9224,1⟩}], [{⟨1,1⟩}], [(9224)], [(40,8),(8,40)]

---

$\mathfrak{su}(2) \leftarrow \mathfrak{sp}(4620)$, $\mathfrak{so}(9240)$, $\mathfrak{su}(3)$, $\mathfrak{su}(3)$, $\mathfrak{su}(3)$, $\mathfrak{su}(3)$, $\mathfrak{su}(3)$, $\mathfrak{su}(4)$, $\mathfrak{su}(4)$, $\mathfrak{su}(4)$, $\mathfrak{su}(4)$, $\mathfrak{su}(5)$, $\mathfrak{su}(5)$, $\mathfrak{su}(5)$, $\mathfrak{su}(5)$, $\mathfrak{su}(6)$, $\mathfrak{su}(6)$, $\mathfrak{su}(7)$, $\mathfrak{su}(9)$, $\mathfrak{su}(10)$, $\mathfrak{su}(10)$ → $\mathfrak{su}(9240)$

[{⟨1,1⟩},{⟨9239,1⟩}], [{⟨1,1⟩}], [(9239)], [{⟨1,1⟩}], [(21,19),(19,21)], [(29,13),(13,29)], [(47,6),(6,47)], [(65,3),(3,65)],[(76,2),(2,76)],[(5,4,2),(2,4,5)],[(7,2,3),(3,2,7)], [(8,1,4),(4,1,8)], [(9,0,6),(6,0,9)], [(1,0,6,0),(0,6,0,1)],[(3,0,2,2),(2,2,0,3)],[(3,3,0,1),(1,0,3,3)],[(4,1,1,1),(1,1,1,4)],[(3,0,0,1,2),(2,1,0,0,3)], [(3,3,0,0,0),(0,0,0,3,3)], [{⟨1,2⟩,⟨2,1⟩,⟨6,2⟩},{⟨1,2⟩,⟨5,1⟩,⟨6,2⟩}], [{⟨1,3⟩,⟨3,1⟩},{⟨6,1⟩,⟨8,3⟩}], [{⟨2,1⟩,⟨5,1⟩},{⟨5,1⟩,⟨8,1⟩}], [{⟨1,2⟩,⟨4,1⟩},{⟨6,1⟩,⟨9,2⟩}]

---

$\mathfrak{su}(2)$, $\mathfrak{su}(3)$ → $\mathfrak{so}(9261) \leftarrow \mathfrak{su}(9261)$

[{⟨1,1⟩},{⟨9260,1⟩}],[{⟨1,1⟩}],[(9260)],[(20,20)]

---

$\mathfrak{su}(2) \leftarrow \mathfrak{sp}(4644)$, $\mathfrak{so}(9288)$, $\mathfrak{su}(3)$ → $\mathfrak{su}(9288)$

[{⟨1,1⟩},{⟨9287,1⟩}], [{⟨1,1⟩}], [(9287)], [{⟨1,1⟩}], [(26,15),(15,26)]

su(2)
so(6)
so(9295)
su(13)
su(9295)

[{⟨1, 1⟩},{⟨9294, 1⟩}], [{⟨1, 1⟩}], [(9294)], [(10, 1, 1)], [{⟨1, 1⟩, ⟨2, 1⟩, ⟨12, 1⟩},{⟨1, 1⟩, ⟨11, 1⟩, ⟨12, 1⟩}]

---

su(2) ← sp(4653)
so(9306) ← su(9306)
su(3)

[{⟨1, 1⟩},{⟨9305, 1⟩}], [{⟨1, 1⟩}], [(9305)], [{⟨1, 1⟩}], [(35, 10),(10, 35)]

---

su(2)
so(136)
so(9315) ← su(9315)

[{⟨1, 1⟩},{⟨9314, 1⟩}],[{⟨1, 1⟩}],[(9314)],[{⟨1, 2⟩}]

---

su(2) ← sp(4658)
so(137)
sp(68)
so(9316)
su(3)
su(136)
su(137)
su(9316)

[{⟨1, 1⟩},{⟨9315, 1⟩}], [{⟨1, 1⟩}], [(9315)], [{⟨1, 1⟩}], [{⟨2, 1⟩}], [{⟨1, 2⟩}], [(135, 0),(0, 135)], [{⟨1, 2⟩},{⟨135, 2⟩}],[{⟨2, 1⟩},{⟨135, 1⟩}]

---

su(2)
sp(4)
sp(4680)
so(9360)
su(3)
su(4)
su(4)
su(4) ← su(9360)
su(5)
su(5)
su(6)
su(10)
su(14)

[{⟨1, 1⟩},{⟨9359, 1⟩}],[{⟨1, 1⟩}],[(9359)],[(4, 0, 1, 0)], [{⟨1, 1⟩}], [(31, 12),(12, 31)], [(2, 11, 0),(0, 11, 2)], [(9, 2, 2),(2, 2, 9)],[(12, 2, 1),(1, 2, 12)],[(7, 0, 2, 0),(0, 2, 0, 7)], [(11, 0, 1, 0),(0, 1, 0, 11)], [(7, 0, 0, 1, 0),(0, 1, 0, 0, 7)], [{⟨1, 3⟩, ⟨8, 1⟩},{⟨2, 1⟩, ⟨9, 3⟩}], [{⟨1, 2⟩, ⟨12, 1⟩},{⟨2, 1⟩, ⟨13, 2⟩}]

---

su(2) ← so(9381)
su(3)
su(9381)

[{⟨1, 1⟩},{⟨9380, 1⟩}], [{⟨1, 1⟩}], [(9380)], [(52, 5),(5, 52)]

---

su(2) ← sp(4692)
so(9384) ← su(9384)
su(3)

[{⟨1, 1⟩},{⟨9383, 1⟩}], [{⟨1, 1⟩}], [(9383)], [{⟨1, 1⟩}], [(33, 11),(11, 33)]

---

su(2)
sp(4)
sp(4704)
su(97) ← so(9408)
su(3)
su(7)
su(9408)

[{⟨1, 1⟩},{⟨9407, 1⟩}],[{⟨1, 1⟩}],[(9407)],[(1, 3, 0, 0)], [{⟨1, 1⟩}], [{⟨1, 1⟩, ⟨96, 1⟩}], [(95, 1),(1, 95)], [{⟨2, 1⟩, ⟨3, 1⟩, ⟨4, 1⟩},{⟨3, 1⟩, ⟨4, 1⟩, ⟨5, 1⟩}]

---

su(2)
sp(5)
sp(4719)
so(10) ← so(9438)
su(9438)

[{⟨1, 1⟩},{⟨9437, 1⟩}], [{⟨1, 1⟩}], [(9437)], [(0, 0, 0, 1, 1)],[{⟨1, 1⟩}],[(7, 0, 0, 0, 0)]

---

su(2) ← sp(4720)
so(9440) ← su(9440)
su(3)

[{⟨1, 1⟩},{⟨9439, 1⟩}], [{⟨1, 1⟩}], [(9439)], [{⟨1, 1⟩}], [(58, 4),(4, 58)]

---

su(2)
sp(3)
sp(4725)
sp(3)
so(6)
so(9450)
su(4) ← su(9450)
su(7)
su(10)
su(27)

[{⟨1, 1⟩},{⟨9449, 1⟩}], [{⟨1, 1⟩}], [(9449)], [(8, 0, 1)], [{⟨1, 1⟩}], [(2, 4, 0)], [(3, 4, 4)], [(24, 1, 0),(0, 1, 24)], [{⟨1, 2⟩, ⟨2, 1⟩, ⟨4, 1⟩},{⟨3, 1⟩, ⟨5, 1⟩, ⟨6, 2⟩}], [{⟨1, 1⟩, ⟨3, 1⟩, ⟨9, 1⟩},{⟨1, 1⟩, ⟨7, 1⟩, ⟨9, 1⟩}],[{⟨1, 1⟩, ⟨25, 1⟩},{⟨2, 1⟩, ⟨26, 1⟩}]

---

su(2) ← sp(4726)
so(137)
sp(69)
so(9452)
su(9452)

[{⟨1, 1⟩},{⟨9451, 1⟩}], [{⟨1, 1⟩}], [(9451)], [{⟨1, 1⟩}], [{⟨1, 2⟩}],[{⟨2, 1⟩}]

---

su(2)
so(138)
so(9453)
su(3)
su(137)
su(138)
su(9453)

[{⟨1, 1⟩},{⟨9452, 1⟩}], [{⟨1, 1⟩}], [(9452)], [{⟨2, 1⟩}], [(136, 0),(0, 136)], [{⟨1, 2⟩},{⟨136, 2⟩}], [{⟨2, 1⟩},{⟨136, 1⟩}]

---

su(2)
so(5)
so(9455) ← su(9455)

[{⟨1, 1⟩},{⟨9454, 1⟩}],[{⟨1, 1⟩}],[(9454)],[(29, 0)]

---

su(2) ← so(9477)
su(3)
su(9477)

[{⟨1, 1⟩},{⟨9476, 1⟩}], [{⟨1, 1⟩}], [(9476)], [(77, 2),(2, 77)]

---

su(2) ← sp(4750)
so(9500) ← su(9500)
su(4)

[{⟨1, 1⟩},{⟨9499, 1⟩}], [{⟨1, 1⟩}], [(9499)], [{⟨1, 1⟩}], [(14, 3, 0),(0, 3, 14)]

---

su(2) ← so(9503)
su(3)
su(9503)

[{⟨1, 1⟩},{⟨9502, 1⟩}], [{⟨1, 1⟩}], [(9502)], [(25, 16),(16, 25)]

---

su(2)
sp(4) ← sp(4752)
so(12)
so(9)
so(9)
so(9504)
so(10)
su(9504)

[{⟨1, 1⟩},{⟨9503, 1⟩}],[{⟨1, 1⟩}],[(9503)],[(5, 1, 0, 0)], [{⟨5, 2⟩, ⟨6, 1⟩},{⟨5, 1⟩, ⟨6, 2⟩}], [{⟨1, 1⟩}], [(0, 0, 0, 5)],[(2, 1, 0, 1)],[(0, 0, 0, 5, 0),(0, 0, 0, 0, 5)]

---

su(2) ← sp(4757)
so(9514) ← su(9514)
su(3)

[{⟨1, 1⟩},{⟨9513, 1⟩}], [{⟨1, 1⟩}], [(9513)], [{⟨1, 1⟩}], [(66, 3),(3, 66)]

---

su(2)
sp(2)
sp(4760)
so(9520)
su(4) ← su(9520)
su(4)
su(4)

[{⟨1, 1⟩},{⟨9519, 1⟩}], [{⟨1, 1⟩}], [(9519)], [(5, 13)], [{⟨1, 1⟩}],[(1, 13, 0),(0, 13, 1)],[(9, 5, 0),(0, 5, 9)],[(15, 0, 3),(3, 0, 15)]

---

su(2) ← sp(4770)
so(9540) ← su(9540)
su(3)

[{⟨1, 1⟩},{⟨9539, 1⟩}], [{⟨1, 1⟩}], [(9539)], [{⟨1, 1⟩}], [(44, 7),(7, 44)]

---

su(2) ← so(9555)
su(3)
su(9555)

[{⟨1, 1⟩},{⟨9554, 1⟩}], [{⟨1, 1⟩}], [(9554)], [(38, 9),(9, 38)]

---

su(2) ← sp(4785)
so(5) ← so(9570) ← su(9570)
su(3)

[{⟨1, 1⟩},{⟨9569, 1⟩}], [{⟨1, 1⟩}], [(9569)], [{⟨1, 1⟩}], [(8, 10)],[(28, 14),(14, 28)]

---

su(2) ← sp(4795)
so(138) ← so(9590)
su(9590)

[{⟨1, 1⟩},{⟨9589, 1⟩}], [{⟨1, 1⟩}], [(9589)], [{⟨1, 1⟩}], [{⟨1, 2⟩}]

---

su(2)
so(139) ← so(9591)
sp(69)
su(3)
su(138)
su(139)
su(9591)

[{⟨1, 1⟩},{⟨9590, 1⟩}], [{⟨1, 1⟩}], [(9590)], [{⟨2, 1⟩}], [{⟨1, 2⟩}], [(137, 0),(0, 137)], [{⟨1, 2⟩},{⟨137, 2⟩}], [{⟨2, 1⟩},{⟨137, 1⟩}]

---

su(2)
su(98)
so(9603)
su(3)
su(9603)

[{⟨1, 1⟩},{⟨9602, 1⟩}], [{⟨1, 1⟩}], [(9602)], [{⟨1, 1⟩, ⟨97, 1⟩}],[(96, 1),(1, 96)]

---

su(2)
sp(2)
sp(4802)
so(9604) ← su(9604)
su(3)

[{⟨1, 1⟩},{⟨9603, 1⟩}], [{⟨1, 1⟩}], [(9603)], [(13, 6)], [{⟨1, 1⟩}],[(48, 6),(6, 48)]

---

su(2) ← sp(4807)
so(9614) ← su(9614)
su(4)

[{⟨1, 1⟩},{⟨9613, 1⟩}], [{⟨1, 1⟩}], [(9613)], [{⟨1, 1⟩}], [(18, 2, 0),(0, 2, 18)]

---

su(2)
so(7)
so(9625)
su(5)
su(5) ← su(9625)
su(5)
su(6)

[{⟨1, 1⟩},{⟨9624, 1⟩}], [{⟨1, 1⟩}], [(9624)], [(3, 0, 4)], [(3, 0, 4, 0),(0, 4, 0, 3)],[(4, 1, 2, 0),(0, 2, 1, 4)],[(4, 4, 0, 0),(0, 0, 4, 4)],[(4, 0, 0, 2, 0),(0, 2, 0, 0, 4)]

---

su(2) ← so(9639)
su(3)
su(9639)

[{⟨1, 1⟩},{⟨9638, 1⟩}], [{⟨1, 1⟩}], [(9638)], [(41, 8),(8,

41)]

---

su(2), sp(2) ← sp(4830); g2 ← so(9660); sp(4830), so(9660) ← su(9660)

[{⟨1, 1⟩},{⟨9659, 1⟩}], [{⟨1, 1⟩}], [(9659)], [(17, 4)], [{⟨1, 1⟩}],[(1, 6)]

---

su(2) ← so(9675); so(9675), su(3) ← su(9675)

[{⟨1, 1⟩},{⟨9674, 1⟩}], [{⟨1, 1⟩}], [(9674)], [(24, 17),(17, 24)]

---

su(2) ← so(9717); so(9717), su(3) ← su(9717)

[{⟨1, 1⟩},{⟨9716, 1⟩}], [{⟨1, 1⟩}], [(9716)], [(78, 2),(2, 78)]

---

su(2), sp(2) ← sp(4860); sp(4860), so(9720), su(3), su(4), su(5) ← su(9720)

[{⟨1, 1⟩},{⟨9719, 1⟩}], [{⟨1, 1⟩}], [(9719)], [(23, 2)], [{⟨1, 1⟩}], [(53, 5),(5, 53)], [(8, 0, 7),(7, 0, 8)], [(5, 2, 0, 1),(1, 0, 2, 5)]

---

su(2) ← sp(4862); sp(4862), so(9724), su(4) ← su(9724)

[{⟨1, 1⟩},{⟨9723, 1⟩}], [{⟨1, 1⟩}], [(9723)], [{⟨1, 1⟩}], [(10, 1, 3),(3, 1, 10)]

---

su(2), so(20) ← sp(4864); sp(4864), so(9728) ← su(9728)

[{⟨1, 1⟩},{⟨9727, 1⟩}], [{⟨1, 1⟩}], [(9727)], [{⟨1, 1⟩, ⟨9, 1⟩},{⟨1, 1⟩, ⟨10, 1⟩}],[{⟨1, 1⟩}]

---

su(2), so(139), sp(70) ← so(9729) ← su(9729)

[{⟨1, 1⟩},{⟨9728, 1⟩}], [{⟨1, 1⟩}], [(9728)], [{⟨1, 2⟩}], [{⟨2, 1⟩}]

---

su(2) ← sp(4865); so(140) ← so(9730); sp(4865), so(9730), su(3), su(139), su(140) ← su(9730)

[{⟨1, 1⟩},{⟨9729, 1⟩}], [{⟨1, 1⟩}], [(9729)], [{⟨1, 1⟩}], [{⟨2, 1⟩}], [(138, 0),(0, 138)], [{⟨1, 2⟩},{⟨138, 2⟩}], [{⟨2, 1⟩},{⟨138, 1⟩}]

---

su(2) ← sp(4875); sp(4875), so(9750), su(3) ← su(9750)

[{⟨1, 1⟩},{⟨9749, 1⟩}], [{⟨1, 1⟩}], [(9749)], [{⟨1, 1⟩}], [(59, 4),(4, 59)]

---

su(2) ← so(9765); so(9765), su(3) ← su(9765)

[{⟨1, 1⟩},{⟨9764, 1⟩}], [{⟨1, 1⟩}], [(9764)], [(30, 13),(13, 30)]

---

su(2) ← sp(4884); sp(4884), so(9768), su(3) ← su(9768)

[{⟨1, 1⟩},{⟨9767, 1⟩}], [{⟨1, 1⟩}], [(9767)], [{⟨1, 1⟩}], [(36, 10),(10, 36)]

---

su(2) ← sp(4896); sp(4896), so(9792), su(3) ← su(9792)

[{⟨1, 1⟩},{⟨9791, 1⟩}], [{⟨1, 1⟩}], [(9791)], [{⟨1, 1⟩}], [(67, 3),(3, 67)]

---

su(2) ← sp(4900); su(99) ← so(9800); sp(4900), so(9800), su(3), su(5) ← su(9800)

[{⟨1, 1⟩},{⟨9799, 1⟩}], [{⟨1, 1⟩}], [(9799)], [{⟨1, 1⟩}], [{⟨1, 1⟩, ⟨98, 1⟩}], [(97, 1),(1, 97)], [(4, 1, 0, 3),(3, 0, 1, 4)]

---

su(2) ← sp(4902); sp(4902), so(9804), su(3) ← su(9804)

[{⟨1, 1⟩},{⟨9803, 1⟩}], [{⟨1, 1⟩}], [(9803)], [{⟨1, 1⟩}], [(23, 18),(18, 23)]

---

su(2) ← sp(4914); sp(3) ← so(9828); sp(4914), so(9828) ← su(9828)

[{⟨1, 1⟩},{⟨9827, 1⟩}], [{⟨1, 1⟩}], [(9827)], [{⟨1, 1⟩}], [(1, 0, 5)]

---

su(2), sp(20) ← sp(4920); sp(4920), so(9840) ← su(9840)

[{⟨1, 1⟩},{⟨9839, 1⟩}], [{⟨1, 1⟩}], [(9839)], [{⟨3, 1⟩}], [{⟨1, 1⟩}]

---

su(2) ← sp(4921); so(38) ← so(9842); sp(4921), so(9842) ← su(9842)

[{⟨1, 1⟩},{⟨9841, 1⟩}], [{⟨1, 1⟩}], [(9841)], [{⟨1, 1⟩}], [{⟨1, 3⟩}]

---

su(2), sp(2) ← sp(4928); sp(4928), so(9856), su(3) ← su(9856)

[{⟨1, 1⟩},{⟨9855, 1⟩}], [{⟨1, 1⟩}], [(9855)], [(15, 5)], [{⟨1, 1⟩}],[(27, 15),(15, 27)]

---

su(2), so(9) ← so(9867); so(9867), su(3) ← su(9867)

[{⟨1, 1⟩},{⟨9866, 1⟩}],[{⟨1, 1⟩}],[(9866)],[(8, 0, 0, 0)], [(32, 12),(12, 32)]

---

su(2), so(140) ← so(9869) ← su(9869)

[{⟨1, 1⟩},{⟨9868, 1⟩}],[{⟨1, 1⟩}],[(9868)],[{⟨1, 2⟩}]

---

su(2) ← sp(4935); so(141), sp(70) ← so(9870); sp(4935), so(9870), su(3), su(3), su(140), su(141) ← su(9870)

[{⟨1, 1⟩},{⟨9869, 1⟩}], [{⟨1, 1⟩}], [(9869)], [{⟨1, 1⟩}], [{⟨2, 1⟩}], [{⟨1, 2⟩}], [(34, 11),(11, 34)], [(139, 0),(0, 139)],[{⟨1, 2⟩},{⟨139, 2⟩}],[{⟨2, 1⟩},{⟨139, 1⟩}]

---

su(2), sp(2), sp(19) ← sp(4940); so(40) ← so(9880); sp(4940), so(9880), su(4), su(38), su(40) ← su(9880)

[{⟨1, 1⟩},{⟨9879, 1⟩}], [{⟨1, 1⟩}], [(9879)], [(37, 0)], [{⟨1, 3⟩}], [{⟨1, 1⟩}], [{⟨3, 1⟩}], [(37, 0, 0),(0, 0, 37)], [{⟨1, 3⟩},{⟨37, 3⟩}],[{⟨3, 1⟩},{⟨37, 1⟩}]

---

su(2), so(5), so(31) ← so(9889) ← su(9889)

[{⟨1, 1⟩},{⟨9888, 1⟩}], [{⟨1, 1⟩}], [(9888)], [(1, 28)], [{⟨1, 1⟩, ⟨2, 1⟩}]

---

su(2) ← sp(4945); so(5) ← so(9890); sp(4945), so(9890), su(3) ← su(9890)

[{⟨1, 1⟩},{⟨9889, 1⟩}], [{⟨1, 1⟩}], [(9889)], [{⟨1, 1⟩}], [(19, 2)],[(22, 19),(19, 22)]

---

su(2) ← sp(4960); sp(4960), so(9920), su(31) ← su(9920)

[{⟨1, 1⟩},{⟨9919, 1⟩}], [{⟨1, 1⟩}], [(9919)], [{⟨1, 1⟩}], [{⟨1, 1⟩, ⟨2, 1⟩},{⟨29, 1⟩, ⟨30, 1⟩}]

---

su(2) ← so(9933); so(9933), su(3) ← su(9933)

[{⟨1, 1⟩},{⟨9932, 1⟩}], [{⟨1, 1⟩}], [(9932)], [(21, 20),(20, 21)]

---

su(2) ← sp(4968); sp(4968), so(9936), su(3) ← su(9936)

[{⟨1, 1⟩},{⟨9935, 1⟩}], [{⟨1, 1⟩}], [(9935)], [{⟨1, 1⟩}], [(45, 7),(7, 45)]

---

su(2) ← sp(4980); sp(4980), so(9960), su(3) ← su(9960)

[{⟨1, 1⟩},{⟨9959, 1⟩}], [{⟨1, 1⟩}], [(9959)], [{⟨1, 1⟩}], [(79, 2),(2, 79)]

---

su(2) ← so(9975); so(9975), su(3) ← su(9975)

[{⟨1, 1⟩},{⟨9974, 1⟩}], [{⟨1, 1⟩}], [(9974)], [(49, 6),(6, 49)]

---

su(2), su(100) ← so(9999); so(9999), su(3) ← su(9999)

[{⟨1, 1⟩},{⟨9998, 1⟩}], [{⟨1, 1⟩}], [(9998)], [{⟨1, 1⟩, ⟨99, 1⟩}],[(98, 1),(1, 98)]

---

su(2), sp(2) ← sp(5000); sp(5000), so(10000), su(3) ← su(10000)

[{⟨1, 1⟩},{⟨9999, 1⟩}], [{⟨1, 1⟩}], [(9999)], [(9, 9)], [{⟨1, 1⟩}],[(39, 9),(9, 39)]

---

su(2) ← sp(5005); so(5), so(7), so(7), so(141), sp(4), sp(71) ← so(10010); sp(5005), so(10010), su(5) ← su(10010)

[{⟨1, 1⟩},{⟨10009, 1⟩}],[{⟨1, 1⟩}],[(10009)],[{⟨1, 1⟩}], [(12, 6)], [(1, 4, 0)], [(7, 1, 0)], [{⟨1, 2⟩}], [(0, 1, 2, 0)], [{⟨2, 1⟩}],[(6, 3, 0, 0),(0, 0, 3, 6)]

---

su(2), so(142) ← so(10011); so(10011), su(3), su(141), su(142) ← su(10011)

[{⟨1, 1⟩},{⟨10010, 1⟩}],[{⟨1, 1⟩}],[(10010)],[{⟨2, 1⟩}],[(140, 0),(0, 140)], [{⟨1, 2⟩},{⟨140, 2⟩}], [{⟨2, 1⟩},{⟨140, 1⟩}]

su(2) ← sp(5031) ←
so(10062) ← su(10062)
su(3) ←

[{⟨1, 1⟩},{⟨10061, 1⟩}],[{⟨1, 1⟩}],[(10061)],[{⟨1, 1⟩}],[(42, 8),(8, 42)]

su(2) ← so(10065) ←
su(3) ← su(10065)
su(3) ←

[{⟨1, 1⟩},{⟨10064, 1⟩}], [{⟨1, 1⟩}], [(10064)], [(54, 5),(5, 54)],[(60, 4),(4, 60)]

su(2) ← sp(5037) ←
so(10074) ← su(10074)
su(3) ←

[{⟨1, 1⟩},{⟨10073, 1⟩}],[{⟨1, 1⟩}],[(10073)],[{⟨1, 1⟩}],[(68, 3),(3, 68)]

su(2) ← sp(5040) ←
so(10080) ←
su(4) ←
su(4) ←
su(4) ←
su(5) ← su(10080)
su(5) ←
su(5) ←
su(6) ←
su(9) ←
su(15) ←

[{⟨1, 1⟩},{⟨10079, 1⟩}],[{⟨1, 1⟩}],[(10079)],[{⟨1, 1⟩}],[(6, 7, 0),(0, 7, 6)], [(7, 3, 2),(2, 3, 7)], [(19, 0, 2),(2, 0, 19)], [(1, 3, 2, 0),(0, 2, 3, 1)], [(4, 0, 1, 3),(3, 1, 0, 4)], [(13, 0, 0, 1),(1, 0, 0, 13)], [(0, 2, 1, 1, 0),(0, 1, 1, 2, 0)], [{⟨1, 2⟩, ⟨7, 1⟩, ⟨8, 1⟩},{⟨1, 1⟩, ⟨2, 1⟩, ⟨8, 2⟩}], [{⟨1, 3⟩, ⟨14, 1⟩},{⟨1, 1⟩, ⟨14, 3⟩}]

su(2) ← sp(5049) ←
so(10098) ← su(10098)
su(3) ←

[{⟨1, 1⟩},{⟨10097, 1⟩}],[{⟨1, 1⟩}],[(10097)],[{⟨1, 1⟩}],[(26, 16),(16, 26)]

su(2) ← so(10125) ←
su(3) ← su(10125)

[{⟨1, 1⟩},{⟨10124, 1⟩}], [{⟨1, 1⟩}], [(10124)], [(29, 14),(14, 29)]

su(2) ← sp(5075) ←
so(5) ← so(10150) ← su(10150)

[{⟨1, 1⟩},{⟨10149, 1⟩}],[{⟨1, 1⟩}],[(10149)],[{⟨1, 1⟩}],[(3, 20)]

su(2) ← sp(5076) ←
so(142) ← so(10152) ← su(10152)

[{⟨1, 1⟩},{⟨10151, 1⟩}],[{⟨1, 1⟩}],[(10151)],[{⟨1, 1⟩}],[{⟨1, 2⟩}]

su(2) ←
so(143) ← so(10153) ←
sp(71) ←
su(3) ←
su(142) ← su(10153)
su(143) ←

[{⟨1, 1⟩},{⟨10152, 1⟩}],[{⟨1, 1⟩}],[(10152)],[{⟨2, 1⟩}],[{⟨1, 2⟩}], [(141, 0),(0, 141)], [{⟨1, 2⟩},{⟨141, 2⟩}], [{⟨2, 1⟩},{⟨141, 1⟩}]

su(2) ← sp(5082) ←
so(6) ← so(10164) ← su(10164)

[{⟨1, 1⟩},{⟨10163, 1⟩}],[{⟨1, 1⟩}],[(10163)],[{⟨1, 1⟩}],[(7, 2, 2)]

su(2) ← so(10179) ←
su(4) ← su(10179)
su(27) ←

[{⟨1, 1⟩},{⟨10178, 1⟩}],[{⟨1, 1⟩}],[(10178)],[(25, 0, 1),(1, 0, 25)],[{⟨1, 2⟩, ⟨26, 1⟩},{⟨1, 1⟩, ⟨26, 2⟩}]

su(2) ← sp(5096) ←
so(7) ← so(10192) ← su(10192)

[{⟨1, 1⟩},{⟨10191, 1⟩}],[{⟨1, 1⟩}],[(10191)],[{⟨1, 1⟩}],[(0, 4, 1)]

su(2) ← sp(5100) ←
su(101) ← so(10200) ← su(10200)
su(3) ←

[{⟨1, 1⟩},{⟨10199, 1⟩}],[{⟨1, 1⟩}],[(10199)],[{⟨1, 1⟩}],[{⟨1, 1⟩, ⟨100, 1⟩}],[(99, 1),(1, 99)]

su(2) ← sp(5103) ←
g2 ← so(10206) ← su(10206)
su(3) ←

[{⟨1, 1⟩},{⟨10205, 1⟩}],[{⟨1, 1⟩}],[(10205)],[{⟨1, 1⟩}],[(2, 5)],[(80, 2),(2, 80)]

su(2) ← sp(5115) ←
so(5) ← so(10230) ← su(10230)

[{⟨1, 1⟩},{⟨10229, 1⟩}],[{⟨1, 1⟩}],[(10229)],[{⟨1, 1⟩}],[(10, 8)]

su(2) ←
so(11) ← sp(5120) ←
sp(2) ←
su(7) ← so(10240) ← su(10240)
su(4) ←
su(5) ←

[{⟨1, 1⟩},{⟨10239, 1⟩}],[{⟨1, 1⟩}],[(10239)],[(1, 1, 0, 0, 1)], [(7, 11)], [{⟨1, 1⟩}], [{⟨1, 1⟩, ⟨2, 1⟩, ⟨5, 1⟩, ⟨6, 1⟩}], [(7, 1, 5),(5, 1, 7)],[(1, 3, 1, 1),(1, 1, 3, 1)]

su(2) ← so(10241) ←
su(3) ← su(10241)

[{⟨1, 1⟩},{⟨10240, 1⟩}], [{⟨1, 1⟩}], [(10240)], [(37, 10),(10, 37)]

su(2) ← sp(5145) ←
so(10290) ← su(10290)
su(5) ←

[{⟨1, 1⟩},{⟨10289, 1⟩}],[{⟨1, 1⟩}],[(10289)],[{⟨1, 1⟩}],[(6, 0, 0, 4),(4, 0, 0, 6)]

su(2) ←
so(143) ← so(10295) ← su(10295)
sp(72) ←

[{⟨1, 1⟩},{⟨10294, 1⟩}],[{⟨1, 1⟩}],[(10294)],[{⟨1, 2⟩}],[{⟨2, 1⟩}]

su(2) ←
sp(4) ← sp(5148) ←
so(7) ←
so(7) ← so(10296) ←
so(144) ←
su(3) ←
su(3) ←
su(6) ← su(10296)
su(8) ←
su(11) ←
su(12) ←
su(143) ←
su(144) ←

[{⟨1, 1⟩},{⟨10295, 1⟩}], [{⟨1, 1⟩}], [(10295)], [(0, 0, 1, 2)], [{⟨1, 1⟩}], [(0, 2, 4)], [(8, 0, 1)], [{⟨2, 1⟩}], [(25, 17),(17, 25)], [(142, 0),(0, 142)], [(7, 0, 1, 0, 0),(0, 0, 1, 0, 7)], [{⟨1, 5⟩, ⟨2, 1⟩},{⟨6, 1⟩, ⟨7, 5⟩}], [{⟨1, 2⟩, ⟨8, 1⟩},{⟨3, 1⟩, ⟨10, 2⟩}], [{⟨1, 1⟩, ⟨6, 1⟩},{⟨6, 1⟩, ⟨11, 1⟩}], [{⟨1, 2⟩},{⟨142, 2⟩}],[{⟨2, 1⟩},{⟨142, 1⟩}]

su(2) ← sp(5152) ←
so(10304) ← su(10304)
su(3) ←

[{⟨1, 1⟩},{⟨10303, 1⟩}],[{⟨1, 1⟩}],[(10303)],[{⟨1, 1⟩}],[(31, 13),(13, 31)]

su(2) ← sp(5170) ←
so(10340) ← su(10340)
su(3) ←

[{⟨1, 1⟩},{⟨10339, 1⟩}],[{⟨1, 1⟩}],[(10339)],[{⟨1, 1⟩}],[(46, 7),(7, 46)]

su(2) ← sp(5175) ←
sp(12) ← so(10350) ← su(10350)

[{⟨1, 1⟩},{⟨10349, 1⟩}],[{⟨1, 1⟩}],[(10349)],[{⟨1, 1⟩}],[{⟨4, 1⟩}]

su(2) ← so(10353) ←
su(3) ← su(10353)

[{⟨1, 1⟩},{⟨10352, 1⟩}], [{⟨1, 1⟩}], [(10352)], [(50, 6),(6, 50)]

su(2) ← sp(5180) ←
so(5) ← so(10360) ← su(10360)
su(3) ←

[{⟨1, 1⟩},{⟨10359, 1⟩}],[{⟨1, 1⟩}],[(10359)],[{⟨1, 1⟩}],[(15, 4)],[(69, 3),(3, 69)]

su(2) ← sp(5184) ←
so(10368) ←
su(3) ← su(10368)
su(6) ←

[{⟨1, 1⟩},{⟨10367, 1⟩}],[{⟨1, 1⟩}],[(10367)],[{⟨1, 1⟩}],[(35, 11),(11, 35)],[(5, 1, 0, 0, 1),(1, 0, 0, 1, 5)]

su(2) ← sp(5187) ←
so(10374) ← su(10374)
su(4) ←

[{⟨1, 1⟩},{⟨10373, 1⟩}],[{⟨1, 1⟩}],[(10373)],[{⟨1, 1⟩}],[(11, 0, 5),(5, 0, 11)]

su(2) ← so(10385) ←
su(3) ← su(10385)

[{⟨1, 1⟩},{⟨10384, 1⟩}], [{⟨1, 1⟩}], [(10384)], [(61, 4),(4, 61)]

su(2) ← so(10387) ←
su(3) ← su(10387)

[{⟨1, 1⟩},{⟨10386, 1⟩}], [{⟨1, 1⟩}], [(10386)], [(33, 12),(12, 33)]

su(2) ←
so(7) ←
so(21) ← so(10395) ←
sp(3) ←
su(4) ←
su(5) ← su(10395)
su(7) ←
su(10) ←

[{⟨1, 1⟩},{⟨10394, 1⟩}],[{⟨1, 1⟩}],[(10394)],[(3, 1, 2)],[{⟨1, 4⟩}], [(2, 0, 4)], [(4, 5, 2),(2, 5, 4)], [(8, 1, 0, 1),(1, 0, 1, 8)], [{⟨1, 5⟩, ⟨3, 1⟩},{⟨4, 1⟩, ⟨6, 5⟩}], [{⟨1, 2⟩, ⟨6, 1⟩},{⟨4, 1⟩, ⟨9, 2⟩}]

su(2) ←
sp(2) ← sp(5200) ←
so(10400) ← su(10400)
su(5) ←

[{⟨1, 1⟩},{⟨10399, 1⟩}], [{⟨1, 1⟩}], [(10399)], [(1, 23)], [{⟨1, 1⟩}],[(7, 1, 1, 0),(0, 1, 1, 7)]

su(10403) → so(10403) → su(2), su(102); su(10403) → su(3)

[{⟨1, 1⟩},{⟨10402, 1⟩}], [{⟨1, 1⟩}], [(10402)], [{⟨1, 1⟩, ⟨101, 1⟩}],[(100, 1),(1, 100)]

su(10416) → sp(5208) → su(2); su(10416) → so(10416) → so(5); su(10416) → su(3)

[{⟨1, 1⟩},{⟨10415, 1⟩}],[{⟨1, 1⟩}],[(10415)],[{⟨1, 1⟩}],[(30, 0)],[(55, 5),(5, 55)]

su(10439) → so(10439) → su(2), so(144)

[{⟨1, 1⟩},{⟨10438, 1⟩}],[{⟨1, 1⟩}],[(10438)],[{⟨1, 2⟩}]

su(10440) → sp(5220) → su(2); su(10440) → so(10440) → so(145), sp(72); su(10440) → su(3), su(3), su(144), su(145)

[{⟨1, 1⟩},{⟨10439, 1⟩}],[{⟨1, 1⟩}],[(10439)],[{⟨1, 1⟩}],[{⟨2, 1⟩}], [{⟨1, 2⟩}], [(28, 15),(15, 28)], [(143, 0),(0, 143)],[{⟨1, 2⟩},{⟨143, 2⟩}],[{⟨2, 1⟩},{⟨143, 1⟩}]

su(10450) → sp(5225) → su(2); su(10450) → so(10450), su(3)

[{⟨1, 1⟩},{⟨10449, 1⟩}],[{⟨1, 1⟩}],[(10449)],[{⟨1, 1⟩}],[(24, 18),(18, 24)]

su(10455) → so(10455) → su(2); su(10455) → su(3), su(3)

[{⟨1, 1⟩},{⟨10454, 1⟩}], [{⟨1, 1⟩}], [(10454)], [(40, 9),(9, 40)],[(81, 2),(2, 81)]

su(10494) → sp(5247) → su(2); su(10494) → so(10494), su(3)

[{⟨1, 1⟩},{⟨10493, 1⟩}],[{⟨1, 1⟩}],[(10493)],[{⟨1, 1⟩}],[(43, 8),(8, 43)]

su(10500) → sp(5250) → su(2); su(10500) → so(10500), su(4), su(4), su(4), su(5), su(6), su(7)

[{⟨1, 1⟩},{⟨10499, 1⟩}],[{⟨1, 1⟩}],[(10499)],[{⟨1, 1⟩}],[(4, 4, 3),(3, 4, 4)], [(6, 2, 4),(4, 2, 6)], [(13, 0, 4),(4, 0, 13)], [(1, 2, 3, 0),(0, 3, 2, 1)], [(2, 1, 0, 1, 1),(1, 1, 0, 1, 2)],[{⟨1, 2⟩, ⟨4, 2⟩},{⟨3, 2⟩, ⟨6, 2⟩}]

su(10556) → sp(5278) → su(2); su(10556) → so(10556) → so(5), so(7) → g2; su(10556) → su(4), su(28)

[{⟨1, 1⟩},{⟨10555, 1⟩}],[{⟨1, 1⟩}],[(10555)],[{⟨1, 1⟩}],[(7, 12)], [(12, 0, 0)], [(12, 0)], [(25, 1, 0),(0, 1, 25)],[{⟨1, 1⟩, ⟨26, 1⟩},{⟨2, 1⟩, ⟨27, 1⟩}]

su(10560) → sp(5280) → su(2), sp(2); su(10560) → so(10560) → so(10); su(10560) → su(3), su(4), su(4)

[{⟨1, 1⟩},{⟨10559, 1⟩}], [{⟨1, 1⟩}], [(10559)], [(3, 17)], [{⟨1, 1⟩}], [(0, 0, 1, 1, 1)], [(23, 19),(19, 23)], [(3, 10, 0),(0, 10, 3)],[(17, 1, 1),(1, 1, 17)]

su(10584) → sp(5292) → su(2); su(10584) → so(10584) → so(145), sp(73), so(6); su(10584) → su(8)

[{⟨1, 1⟩},{⟨10583, 1⟩}],[{⟨1, 1⟩}],[(10583)],[{⟨1, 1⟩}],[{⟨1, 2⟩}], [{⟨2, 1⟩}], [(1, 6, 6)], [{⟨1, 1⟩, ⟨4, 1⟩, ⟨6, 1⟩},{⟨2, 1⟩, ⟨4, 1⟩, ⟨7, 1⟩}]

su(10585) → so(10585) → su(2), so(146); su(10585) → su(3), su(145), su(146)

[{⟨1, 1⟩},{⟨10584, 1⟩}],[{⟨1, 1⟩}],[(10584)],[{⟨2, 1⟩}],[(144, 0),(0, 144)], [{⟨1, 2⟩},{⟨144, 2⟩}], [{⟨2, 1⟩},{⟨144, 1⟩}]

su(10608) → sp(5304) → su(2); su(10608) → so(10608) → su(103); su(10608) → su(3)

[{⟨1, 1⟩},{⟨10607, 1⟩}],[{⟨1, 1⟩}],[(10607)],[{⟨1, 1⟩}],[{⟨1, 1⟩, ⟨102, 1⟩}],[(101, 1),(1, 101)]

su(10621) → so(10621) → su(2), so(39)

[{⟨1, 1⟩},{⟨10620, 1⟩}],[{⟨1, 1⟩}],[(10620)],[{⟨1, 3⟩}]

su(10626) → sp(5313) → su(2); su(10626) → so(10626) → so(24); su(10626) → su(3), su(5), su(21), su(24)

[{⟨1, 1⟩},{⟨10625, 1⟩}],[{⟨1, 1⟩}],[(10625)],[{⟨1, 1⟩}],[{⟨4, 1⟩}],[(22, 20),(20, 22)],[(20, 0, 0, 0),(0, 0, 0, 20)],[{⟨1, 4⟩},{⟨20, 4⟩}],[{⟨4, 1⟩},{⟨20, 1⟩}]

su(10640) → sp(5320) → su(2); su(10640) → so(10640) → so(19); su(10640) → su(4)

[{⟨1, 1⟩},{⟨10639, 1⟩}],[{⟨1, 1⟩}],[(10639)],[{⟨1, 1⟩}],[{⟨2, 2⟩}],[(13, 1, 2),(2, 1, 13)]

su(10648) → sp(5324) → su(2); su(10648) → so(10648) → su(3)

[{⟨1, 1⟩},{⟨10647, 1⟩}],[{⟨1, 1⟩}],[(10647)],[{⟨1, 1⟩}],[(21, 21)]

su(10650) → sp(5325) → su(2); su(10650) → so(10650), su(3)

[{⟨1, 1⟩},{⟨10649, 1⟩}],[{⟨1, 1⟩}],[(10649)],[{⟨1, 1⟩}],[(70, 3),(3, 70)]

su(10660) → sp(5330) → su(2); su(10660) → so(10660) → so(5), so(41); su(10660) → su(4), su(39), su(41)

[{⟨1, 1⟩},{⟨10659, 1⟩}],[{⟨1, 1⟩}],[(10659)],[{⟨1, 1⟩}],[(0, 38)], [{⟨3, 1⟩}], [(38, 0, 0),(0, 0, 38)], [{⟨1, 3⟩},{⟨38, 3⟩}],[{⟨3, 1⟩},{⟨38, 1⟩}]

su(10692) → sp(5346) → su(2); su(10692) → so(10692), su(9)

[{⟨1, 1⟩},{⟨10691, 1⟩}],[{⟨1, 1⟩}],[(10691)],[{⟨1, 1⟩}],[{⟨1, 2⟩, ⟨2, 2⟩},{⟨7, 2⟩, ⟨8, 2⟩}]

su(10695) → so(10695) → su(2); su(10695) → su(3)

[{⟨1, 1⟩},{⟨10694, 1⟩}], [{⟨1, 1⟩}], [(10694)], [(30, 14),(14, 30)]

su(10707) → so(10707) → su(2); su(10707) → su(3)

[{⟨1, 1⟩},{⟨10706, 1⟩}], [{⟨1, 1⟩}], [(10706)], [(82, 2),(2, 82)]

su(10710) → sp(5355) → su(2); su(10710) → so(10710), su(3), su(3)

[{⟨1, 1⟩},{⟨10709, 1⟩}],[{⟨1, 1⟩}],[(10709)],[{⟨1, 1⟩}],[(27, 16),(16, 27)],[(62, 4),(4, 62)]

su(10725) → so(10725) → su(2); su(10725) → su(3), su(6), su(11)

[{⟨1, 1⟩},{⟨10724, 1⟩}], [{⟨1, 1⟩}], [(10724)], [(38, 10),(10, 38)],[(9, 0, 0, 0, 1),(1, 0, 0, 0, 9)],[{⟨1, 4⟩, ⟨10, 1⟩},{⟨1, 1⟩, ⟨10, 4⟩}]

su(10730) → sp(5365) → su(2); su(10730) → so(10730) → so(146)

[{⟨1, 1⟩},{⟨10729, 1⟩}],[{⟨1, 1⟩}],[(10729)],[{⟨1, 1⟩}],[{⟨1, 2⟩}]

su(10731) → so(10731) → su(2), so(147), sp(73); su(10731) → su(3), su(146), su(147)

[{⟨1, 1⟩},{⟨10730, 1⟩}],[{⟨1, 1⟩}],[(10730)],[{⟨2, 1⟩}],[{⟨1, 2⟩}], [(145, 0),(0, 145)], [{⟨1, 2⟩},{⟨145, 2⟩}],[{⟨2, 1⟩},{⟨145, 1⟩}]

su(10738) → sp(5369) → su(2); su(10738) → so(10738), su(3)

[{⟨1, 1⟩},{⟨10737, 1⟩}],[{⟨1, 1⟩}],[(10737)],[{⟨1, 1⟩}],[(51, 6),(6, 51)]

su(10752) → sp(5376) → su(2), sp(3), sp(7); su(10752) → so(10752) → so(7), sp(3), so(8); su(10752) → su(3)

[{⟨1, 1⟩},{⟨10751, 1⟩}],[{⟨1, 1⟩}],[(10751)],[(1, 5, 0)], [{⟨1, 1⟩, ⟨4, 1⟩}], [{⟨1, 1⟩}], [(1, 3, 1)], [(5, 1, 1)], [(3, 2, 0, 0),(0, 2, 3, 0),(0, 2, 0, 3)],[(47, 7),(7, 47)]

su(10773) → so(10773) → su(2); su(10773) → su(3)

[{⟨1, 1⟩},{⟨10772, 1⟩}], [{⟨1, 1⟩}], [(10772)], [(56, 5),(5, 56)]

su(2) ⟵ sp(5390)
so(10780)
su(4) ⟵ su(10780)
su(5)
su(8)

[{⟨1, 1⟩},{⟨10779, 1⟩}],[{⟨1, 1⟩}],[(10779)],[{⟨1, 1⟩}],[(3, 6, 2),(2, 6, 3)], [(2, 0, 5, 0),(0, 5, 0, 2)], [{⟨1, 2⟩, ⟨6, 2⟩},{⟨2, 2⟩, ⟨7, 2⟩}]

---

su(2) ⟵ sp(5400)
su(15) ⟵ so(10800) ⟵ su(10800)
su(4)

[{⟨1, 1⟩},{⟨10799, 1⟩}],[{⟨1, 1⟩}],[(10799)],[{⟨1, 1⟩}],[{⟨2, 1⟩, ⟨13, 1⟩}],[(5, 8, 0),(0, 8, 5)]

---

su(2)
so(10815)
su(104) su(10815)
su(3)

[{⟨1, 1⟩},{⟨10814, 1⟩}], [{⟨1, 1⟩}], [(10814)], [{⟨1, 1⟩, ⟨103, 1⟩}],[(102, 1),(1, 102)]

---

su(2)
su(14) ⟵ so(10829) ⟵ su(10829)
$\mathfrak{f}_4$

[{⟨1, 1⟩},{⟨10828, 1⟩}], [{⟨1, 1⟩}], [(10828)], [{⟨1, 2⟩, ⟨13, 2⟩}],[(1, 0, 0, 2)]

---

su(2) ⟵ sp(5415)
so(6) ⟵ so(10830) su(10830)
su(19)

[{⟨1, 1⟩},{⟨10829, 1⟩}],[{⟨1, 1⟩}],[(10829)],[{⟨1, 1⟩}],[(17, 0, 0)],[{⟨2, 2⟩},{⟨17, 2⟩}]

---

su(2) ⟵ sp(5425)
su(10850)
so(5) ⟵ so(10850)

[{⟨1, 1⟩},{⟨10849, 1⟩}],[{⟨1, 1⟩}],[(10849)],[{⟨1, 1⟩}],[(2, 24)]

---

su(2) ⟵ so(10857)
su(10857)
su(3)

[{⟨1, 1⟩},{⟨10856, 1⟩}], [{⟨1, 1⟩}], [(10856)], [(32, 13),(13, 32)]

---

su(2)
so(147) ⟵ so(10877) ⟵ su(10877)
sp(74)

[{⟨1, 1⟩},{⟨10876, 1⟩}],[{⟨1, 1⟩}],[(10876)],[{⟨1, 2⟩}],[{⟨2, 1⟩}]

---

su(2) ⟵ sp(5439)
so(148) ⟵ so(10878)
su(3)
su(3) su(10878)
su(147)
su(148)

[{⟨1, 1⟩},{⟨10877, 1⟩}],[{⟨1, 1⟩}],[(10877)],[{⟨1, 1⟩}],[{⟨2, 1⟩}], [(36, 11),(11, 36)], [(146, 0),(0, 146)], [{⟨1, 2⟩},{⟨146, 2⟩}],[{⟨2, 1⟩},{⟨146, 1⟩}]

---

su(2)
sp(2) ⟵ sp(5440)
sp(16) su(10880)
so(32) ⟵ so(10880)

[{⟨1, 1⟩},{⟨10879, 1⟩}], [{⟨1, 1⟩}], [(10879)], [(29, 1)], [{⟨1, 1⟩, ⟨2, 1⟩}],[{⟨1, 1⟩}],[{⟨1, 1⟩, ⟨2, 1⟩}]

---

su(2) ⟵ sp(5456)
so(10912) su(10912)
su(32)

[{⟨1, 1⟩},{⟨10911, 1⟩}],[{⟨1, 1⟩}],[(10911)],[{⟨1, 1⟩}],[{⟨1, 1⟩, ⟨2, 1⟩},{⟨30, 1⟩, ⟨31, 1⟩}]

---

su(2) ⟵ sp(5460)
so(10920)
su(3) su(10920)
su(3)
su(4)
su(8)

[{⟨1, 1⟩},{⟨10919, 1⟩}],[{⟨1, 1⟩}],[(10919)],[{⟨1, 1⟩}],[(34, 12),(12, 34)], [(41, 9),(9, 41)], [(6, 5, 1),(1, 5, 6)], [{⟨1, 4⟩, ⟨7, 2⟩},{⟨1, 2⟩, ⟨7, 4⟩}]

---

su(2)
so(10935)
so(6)
su(3) su(10935)
su(3)

[{⟨1, 1⟩},{⟨10934, 1⟩}],[{⟨1, 1⟩}],[(10934)],[(2, 5, 5)],[(26, 17),(17, 26)],[(44, 8),(8, 44)]

---

su(2) ⟵ sp(5472)
so(10944) su(10944)
su(3)

[{⟨1, 1⟩},{⟨10943, 1⟩}],[{⟨1, 1⟩}],[(10943)],[{⟨1, 1⟩}],[(71, 3),(3, 71)]

---

su(2) ⟵ sp(5474) su(10948)
so(15) ⟵ so(10948)

[{⟨1, 1⟩},{⟨10947, 1⟩}],[{⟨1, 1⟩}],[(10947)],[{⟨1, 1⟩}],[{⟨1, 5⟩}]

---

su(2) ⟵ sp(5481)
so(10962) su(10962)
su(3)

[{⟨1, 1⟩},{⟨10961, 1⟩}],[{⟨1, 1⟩}],[(10961)],[{⟨1, 1⟩}],[(83, 2),(2, 83)]

---

su(2) ⟵ sp(5488) su(10976)
su(5) ⟵ so(10976)

[{⟨1, 1⟩},{⟨10975, 1⟩}],[{⟨1, 1⟩}],[(10975)],[{⟨1, 1⟩}],[(5, 0, 0, 5)]

---

su(2) ⟵ sp(5500)
so(11000) su(11000)
su(4)

[{⟨1, 1⟩},{⟨10999, 1⟩}],[{⟨1, 1⟩}],[(10999)],[{⟨1, 1⟩}],[(4, 9, 0),(0, 9, 4)]

---

su(2)
so(11011) ⟵ su(11011)
so(12)

[{⟨1, 1⟩},{⟨11010, 1⟩}],[{⟨1, 1⟩}],[(11010)],[{⟨1, 6⟩}]

---

su(2) ⟵ sp(5510) su(11020)
so(5) ⟵ so(11020)

[{⟨1, 1⟩},{⟨11019, 1⟩}],[{⟨1, 1⟩}],[(11019)],[{⟨1, 1⟩}],[(4, 18)]

---

su(2) ⟵ sp(5512)
su(105) ⟵ so(11024) su(11024)
su(3)

[{⟨1, 1⟩},{⟨11023, 1⟩}],[{⟨1, 1⟩}],[(11023)],[{⟨1, 1⟩}],[{⟨1, 1⟩, ⟨104, 1⟩}],[(103, 1),(1, 103)]

---

su(2)
so(11025)
so(148) su(11025)
su(7)

[{⟨1, 1⟩},{⟨11024, 1⟩}],[{⟨1, 1⟩}],[(11024)],[{⟨1, 2⟩}],[{⟨1, 2⟩, ⟨4, 1⟩, ⟨5, 1⟩},{⟨2, 1⟩, ⟨3, 1⟩, ⟨6, 2⟩}]

---

su(2) ⟵ sp(5513)
so(149)
so(11026)
sp(74)
su(3) su(11026)
su(148)
su(149)

[{⟨1, 1⟩},{⟨11025, 1⟩}],[{⟨1, 1⟩}],[(11025)],[{⟨1, 1⟩}],[{⟨2, 1⟩}], [{⟨1, 2⟩}], [(147, 0),(0, 147)], [{⟨1, 2⟩},{⟨147, 2⟩}],[{⟨2, 1⟩},{⟨147, 1⟩}]

---

su(2) ⟵ sp(5520)
so(11040)
su(3) su(11040)
su(3)
su(4)

[{⟨1, 1⟩},{⟨11039, 1⟩}],[{⟨1, 1⟩}],[(11039)],[{⟨1, 1⟩}],[(29, 15),(15, 29)], [(63, 4),(4, 63)], [(19, 2, 0),(0, 2, 19)]

---

su(2)
sp(5544)
sp(6)
so(7)
so(7)
so(11088)
so(12)
so(12)
su(7)
su(8) su(11088)
su(8)
su(9)
su(9)
so(10)

[{⟨1, 1⟩},{⟨11087, 1⟩}], [{⟨1, 1⟩}], [(11087)], [{⟨1, 2⟩, ⟨3, 1⟩}], [{⟨1, 1⟩}], [(1, 0, 7)], [(2, 1, 3)], [{⟨1, 1⟩, ⟨2, 2⟩}], [{⟨1, 3⟩, ⟨2, 1⟩}], [{⟨1, 7⟩, ⟨6, 1⟩},{⟨1, 1⟩, ⟨6, 7⟩}], [{⟨1, 1⟩, ⟨2, 3⟩},{⟨6, 3⟩, ⟨7, 1⟩}], [{⟨1, 2⟩, ⟨3, 1⟩, ⟨7, 1⟩},{⟨1, 1⟩, ⟨5, 1⟩, ⟨7, 2⟩}], [{⟨1, 1⟩, ⟨2, 1⟩, ⟨3, 1⟩},{⟨6, 1⟩, ⟨7, 1⟩, ⟨8, 1⟩}],[{⟨1, 5⟩, ⟨8, 1⟩},{⟨1, 1⟩, ⟨8, 5⟩}],[(1, 0, 0, 2, 1),(1, 0, 0, 1, 2)]

---

su(2) ⟵ so(11115)
su(3) su(11115)
su(4)

[{⟨1, 1⟩},{⟨11114, 1⟩}], [{⟨1, 1⟩}], [(11114)], [(25, 18),(18, 25)],[(12, 4, 0),(0, 4, 12)]

---

su(2) ⟵ sp(5565)
so(11130) su(11130)
su(3)

[{⟨1, 1⟩},{⟨11129, 1⟩}],[{⟨1, 1⟩}],[(11129)],[{⟨1, 1⟩}],[(52, 6),(6, 52)]

---

su(2) ⟵ sp(5568)
so(11136) su(11136)
su(3)

[{⟨1, 1⟩},{⟨11135, 1⟩}],[{⟨1, 1⟩}],[(11135)],[{⟨1, 1⟩}],[(57, 5),(5, 57)]

---

su(2)
so(11165) ⟵ su(11165)
so(5)

[{⟨1, 1⟩},{⟨11164, 1⟩}],[{⟨1, 1⟩}],[(11164)],[(6, 14)]

---

su(2) ⟵ sp(5586)
so(11172) su(11172)
su(3)

[{⟨1, 1⟩},{⟨11171, 1⟩}],[{⟨1, 1⟩}],[(11171)],[{⟨1, 1⟩}],[(48, 7),(7, 48)]

---

su(2) ⟵ sp(5587)
so(149) su(11174)
so(11174)
sp(75)

[{⟨1, 1⟩},{⟨11173, 1⟩}],[{⟨1, 1⟩}],[(11173)],[{⟨1, 1⟩}],[{⟨1, 2⟩}],[{⟨2, 1⟩}]

---

su(2)
so(11175)
so(150)
su(3) su(11175)
su(149)
su(150)

[{⟨1, 1⟩},{⟨11174, 1⟩}],[{⟨1, 1⟩}],[(11174)],[{⟨2, 1⟩}],[(148, 0),(0, 148)], [{⟨1, 2⟩},{⟨148, 2⟩}], [{⟨2, 1⟩},{⟨148, 1⟩}]

---

su(2) ⟵ sp(5600)
so(6) ⟵ so(11200) ⟵ su(11200)
su(4)

[{⟨1, 1⟩},{⟨11199, 1⟩}],[{⟨1, 1⟩}],[(11199)],[{⟨1, 1⟩}],[(5, 3, 3)],[(15, 3, 0),(0, 3, 15)]

---

su(2) ⟵ sp(5610)
so(11220)
su(3) ⟵ su(11220)
su(3)
su(4)
su(4)

[{⟨1, 1⟩},{⟨11219, 1⟩}],[{⟨1, 1⟩}],[(11219)],[{⟨1, 1⟩}],[(39, 10),(10, 39)], [(84, 2),(2, 84)], [(10, 3, 1),(1, 3, 10)],[(16, 0, 3),(3, 0, 16)]

---

su(2) ⟵ sp(5616)
su(11232)
so(12) ⟵ so(11232)

[{⟨1, 1⟩},{⟨11231, 1⟩}],[{⟨1, 1⟩}],[(11231)],[{⟨1, 1⟩}],[{⟨1, 2⟩, ⟨3, 1⟩}]

---

su(2)
so(11235)
su(106)
su(11235)
su(3)

[{⟨1, 1⟩},{⟨11234, 1⟩}], [{⟨1, 1⟩}], [(11234)], [{⟨1, 1⟩, ⟨105, 1⟩}],[(104, 1),(1, 104)]

---

su(2) ⟵ sp(5621)
so(11242) ⟵ su(11242)
su(3)

[{⟨1, 1⟩},{⟨11241, 1⟩}],[{⟨1, 1⟩}],[(11241)],[{⟨1, 1⟩}],[(72, 3),(3, 72)]

---

su(2) ⟵ sp(5625)
so(11250) ⟵ su(11250)
su(3)

[{⟨1, 1⟩},{⟨11249, 1⟩}],[{⟨1, 1⟩}],[(11249)],[{⟨1, 1⟩}],[(24, 19),(19, 24)]

---

su(2) ⟵ sp(5640)
so(11280) ⟵ su(11280)
su(3)

[{⟨1, 1⟩},{⟨11279, 1⟩}],[{⟨1, 1⟩}],[(11279)],[{⟨1, 1⟩}],[(31, 14),(14, 31)]

---

su(2)
so(11305)
sp(9)
su(11305)
su(4)

[{⟨1, 1⟩},{⟨11304, 1⟩}], [{⟨1, 1⟩}], [(11304)], [{⟨1, 1⟩, ⟨3, 1⟩}],[(13, 2, 1),(1, 2, 13)]

---

su(2)
so(11319) ⟵ su(11319)
sp(3)

[{⟨1, 1⟩},{⟨11318, 1⟩}],[{⟨1, 1⟩}],[(11318)],[(3, 2, 1)]

---

su(2) ⟵ sp(5662)
su(11324)
so(150) ⟵ so(11324)

[{⟨1, 1⟩},{⟨11323, 1⟩}],[{⟨1, 1⟩}],[(11323)],[{⟨1, 1⟩}],[{⟨1, 2⟩}]

---

su(2)
so(151) ⟵ so(11325)
sp(75)
su(3)
su(11325)
su(150)
su(151)

[{⟨1, 1⟩},{⟨11324, 1⟩}],[{⟨1, 1⟩}],[(11324)],[{⟨2, 1⟩}],[{⟨1, 2⟩}], [(149, 0),(0, 149)], [{⟨1, 2⟩},{⟨149, 2⟩}],[{⟨2, 1⟩},{⟨149, 1⟩}]

---

su(2)
so(11339)
so(5)
su(11339)
su(3)

[{⟨1, 1⟩},{⟨11338, 1⟩}], [{⟨1, 1⟩}], [(11338)], [(5, 16)],[(28, 16),(16, 28)]

---

su(2)
sp(2) ⟵ sp(5670)
sp(2)
su(6)
so(5)
so(11340)
so(17) ⟵ su(11340)
sp(4)
su(3)
su(4)
su(6)
su(28)

[{⟨1, 1⟩},{⟨11339, 1⟩}], [{⟨1, 1⟩}], [(11339)], [(5, 14)], [(11, 8)], [{⟨1, 1⟩}], [(0, 1, 2, 1, 0)], [(20, 2)], [{⟨1, 2⟩, ⟨2, 1⟩}],[(0, 4, 0, 0)],[(23, 20),(20, 23)],[(26, 0, 1),(1, 0, 26)], [(2, 2, 1, 0, 0),(0, 0, 1, 2, 2)], [{⟨1, 2⟩, ⟨27, 1⟩},{⟨1, 1⟩, ⟨27, 2⟩}]

---

su(2) ⟵ so(11375)
su(3) ⟵ su(11375)
su(5)

[{⟨1, 1⟩},{⟨11374, 1⟩}], [{⟨1, 1⟩}], [(11374)], [(64, 4),(4, 64)],[(9, 2, 0, 0),(0, 0, 2, 9)]

---

su(2) ⟵ so(11385)
su(3) ⟵ su(11385)
su(3)

[{⟨1, 1⟩},{⟨11384, 1⟩}], [{⟨1, 1⟩}], [(11384)], [(22, 21),(21, 22)],[(45, 8),(8, 45)]

---

su(2) ⟵ so(11395)
su(11395)
su(3)

[{⟨1, 1⟩},{⟨11394, 1⟩}], [{⟨1, 1⟩}], [(11394)], [(42, 9),(9, 42)]

---

su(2) ⟵ sp(5700)
so(11400) ⟵ su(11400)
su(3)

[{⟨1, 1⟩},{⟨11399, 1⟩}],[{⟨1, 1⟩}],[(11399)],[{⟨1, 1⟩}],[(37, 11),(11, 37)]

---

su(2) ⟵ sp(5712)
so(11424)
su(3)
su(11424)
su(4)
su(5)
su(17)

[{⟨1, 1⟩},{⟨11423, 1⟩}],[{⟨1, 1⟩}],[(11423)],[{⟨1, 1⟩}],[(33, 13),(13, 33)], [(8, 6, 0),(0, 6, 8)], [(13, 1, 0, 0),(0, 0, 1, 13)],[{⟨1, 1⟩, ⟨14, 1⟩},{⟨3, 1⟩, ⟨16, 1⟩}]

---

su(2)
sp(5719)
sp(21)
su(11438)
so(11438)

[{⟨1, 1⟩},{⟨11437, 1⟩}],[{⟨1, 1⟩}],[(11437)],[{⟨3, 1⟩}],[{⟨1, 1⟩}]

---

su(2)
sp(2)
sp(4) ⟵ sp(5720)
sp(5)
sp(6)
so(5)
so(16) ⟵ so(11440) ⟵ su(11440)
so(40)
su(5)
su(8)
su(10)
su(16)

[{⟨1, 1⟩},{⟨11439, 1⟩}], [{⟨1, 1⟩}], [(11439)], [(21, 3)], [(9, 0, 0, 0)],[(7, 0, 0, 0, 0)],[{⟨1, 1⟩, ⟨2, 2⟩}],[{⟨1, 1⟩}],[(31, 0)],[{⟨7, 1⟩, ⟨8, 1⟩}],[{⟨1, 3⟩}],[(10, 0, 0, 2),(2, 0, 0, 10)],[{⟨1, 9⟩},{⟨7, 9⟩}],[{⟨1, 7⟩},{⟨9, 7⟩}],[{⟨7, 1⟩},{⟨9, 1⟩}]

---

su(2) ⟵ sp(5724)
su(107) ⟵ so(11448) ⟵ su(11448)
su(3)

[{⟨1, 1⟩},{⟨11447, 1⟩}],[{⟨1, 1⟩}],[(11447)],[{⟨1, 1⟩}],[{⟨1, 1⟩, ⟨106, 1⟩}],[(105, 1),(1, 105)]

---

su(2) ⟵ sp(5733)
so(11466)
su(3) ⟵ su(11466)
su(6)
su(7)

[{⟨1, 1⟩},{⟨11465, 1⟩}],[{⟨1, 1⟩}],[(11465)],[{⟨1, 1⟩}],[(35, 12),(12, 35)],[(5, 0, 0, 0, 3),(3, 0, 0, 0, 5)],[{⟨1, 5⟩, ⟨6, 2⟩},{⟨1, 2⟩, ⟨6, 5⟩}]

---

su(2)
so(151)
so(11475) ⟵ su(11475)
sp(76)
so(18)

[{⟨1, 1⟩},{⟨11474, 1⟩}],[{⟨1, 1⟩}],[(11474)],[{⟨1, 2⟩}],[{⟨2, 1⟩}],[{⟨1, 1⟩, ⟨3, 1⟩}]

---

su(2) ⟵ sp(5738)
so(152) ⟵ so(11476)
su(3) ⟵ su(11476)
su(151)
su(152)

[{⟨1, 1⟩},{⟨11475, 1⟩}],[{⟨1, 1⟩}],[(11475)],[{⟨1, 1⟩}],[{⟨2, 1⟩}], [(150, 0),(0, 150)], [{⟨1, 2⟩},{⟨150, 2⟩}],[{⟨2, 1⟩},{⟨150, 1⟩}]

---

su(2)
sp(2) ⟵ sp(5740)
sp(20)
so(42) ⟵ so(11480)
su(11480)
su(4)
su(40)
su(42)

[{⟨1, 1⟩},{⟨11479, 1⟩}], [{⟨1, 1⟩}], [(11479)], [(39, 0)], [{⟨1, 3⟩}], [{⟨1, 1⟩}], [(39, 0, 0),(0, 0, 39)],[{⟨1, 3⟩},{⟨39, 3⟩}],[{⟨3, 1⟩},{⟨39, 1⟩}]

---

su(2) ⟵ so(11481)
su(11481)
su(3)

[{⟨1, 1⟩},{⟨11480, 1⟩}], [{⟨1, 1⟩}], [(11480)], [(85, 2),(2, 85)]

---

su(2) ⟵ so(11505)
su(11505)
su(3)

[{⟨1, 1⟩},{⟨11504, 1⟩}], [{⟨1, 1⟩}], [(11504)], [(58, 5),(5, 58)]

su(2) ← sp(5760)
su(11520)
so(15) ← so(11520)

[{⟨1, 1⟩},{⟨11519, 1⟩}],[{⟨1, 1⟩}],[(11519)],[{⟨1, 1⟩}],[{⟨2, 1⟩, ⟨7, 1⟩}]

---

su(2) ← so(11529)
su(11529)
su(3)

[{⟨1, 1⟩},{⟨11528, 1⟩}], [{⟨1, 1⟩}], [(11528)], [(53, 6),(6, 53)]

---

su(2) ← sp(5772)
so(11544) su(11544)
su(3)

[{⟨1, 1⟩},{⟨11543, 1⟩}],[{⟨1, 1⟩}],[(11543)],[{⟨1, 1⟩}],[(73, 3),(3, 73)]

---

su(2) ← sp(5775)
sp(3) ← so(11550)
su(4)
su(5)
su(5) su(11550)
su(5)
su(6)
su(6)
su(10)

[{⟨1, 1⟩},{⟨11549, 1⟩}],[{⟨1, 1⟩}],[(11549)],[{⟨1, 1⟩}],[(6, 2, 0)],[(20, 0, 2),(2, 0, 20)],[(0, 6, 1, 0),(0, 1, 6, 0)],[(3, 0, 3, 1),(1, 3, 0, 3)],[(5, 0, 3, 0),(0, 3, 0, 5)],[(4, 1, 0, 1, 0),(0, 1, 0, 1, 4)], [(4, 1, 1, 0, 0),(0, 0, 1, 1, 4)], [{⟨1, 3⟩, ⟨9, 2⟩},{⟨1, 2⟩, ⟨9, 3⟩}]

---

su(2)
so(11571) ← su(11571)
g2

[{⟨1, 1⟩},{⟨11570, 1⟩}],[{⟨1, 1⟩}],[(11570)],[(0, 8)]

---

su(2)
so(11583) ← su(11583)
so(11)

[{⟨1, 1⟩},{⟨11582, 1⟩}],[{⟨1, 1⟩}],[(11582)],[(0, 1, 0, 1, 0)]

---

su(2) ← sp(5796)
so(11592) su(11592)
su(3)

[{⟨1, 1⟩},{⟨11591, 1⟩}],[{⟨1, 1⟩}],[(11591)],[{⟨1, 1⟩}],[(27, 17),(17, 27)]

---

su(2) ← sp(5800)
so(11600) su(11600)
su(3)

[{⟨1, 1⟩},{⟨11599, 1⟩}],[{⟨1, 1⟩}],[(11599)],[{⟨1, 1⟩}],[(49, 7),(7, 49)]

---

su(2)
so(11627) ← su(11627)
so(152)

[{⟨1, 1⟩},{⟨11626, 1⟩}],[{⟨1, 1⟩}],[(11626)],[{⟨1, 2⟩}]

---

su(2)
sp(5814)
sp(3)
so(19)
so(153)
so(11628)
sp(3)
sp(76)
su(3)
su(11628)
su(6)
su(15)
su(19)
su(152)
su(17)
su(153)
su(18)

[{⟨1, 1⟩},{⟨11627, 1⟩}], [{⟨1, 1⟩}], [(11627)], [(0, 0, 7)], [{⟨1, 1⟩}], [{⟨5, 1⟩}], [{⟨2, 1⟩}], [(14, 0, 0)], [{⟨1, 2⟩}], [(151, 0),(0, 151)], [(14, 0, 0, 0, 0),(0, 0, 0, 0, 14)], [{⟨1, 5⟩},{⟨14, 5⟩}], [{⟨5, 1⟩},{⟨14, 1⟩}], [{⟨1, 2⟩},{⟨151, 2⟩}], [{⟨2, 1⟩},{⟨151, 1⟩}], [{⟨1, 2⟩, ⟨2, 1⟩},{⟨15, 1⟩, ⟨16, 2⟩}],[{⟨1, 1⟩, ⟨3, 1⟩},{⟨15, 1⟩, ⟨17, 1⟩}]

---

su(2)
sp(3) sp(5824)
sp(6)
su(11648)
so(14)
so(11648)
g2

[{⟨1, 1⟩},{⟨11647, 1⟩}],[{⟨1, 1⟩}],[(11647)],[(9, 1, 0)],[{⟨1, 3⟩, ⟨2, 1⟩}],[{⟨1, 1⟩}],[{⟨1, 1⟩, ⟨4, 1⟩}],[(9, 1)]

---

su(2) ← sp(5828)
so(11656) su(11656)
su(3)

[{⟨1, 1⟩},{⟨11655, 1⟩}],[{⟨1, 1⟩}],[(11655)],[{⟨1, 1⟩}],[(30, 15),(15, 30)]

---

su(2)
so(11663) su(11663)
su(108)
su(3)

[{⟨1, 1⟩},{⟨11662, 1⟩}], [{⟨1, 1⟩}], [(11662)], [{⟨1, 1⟩, ⟨107, 1⟩}],[(106, 1),(1, 106)]

---

su(2)
sp(5850)
sp(2)
so(11700) su(11700)
su(4)

[{⟨1, 1⟩},{⟨11699, 1⟩}], [{⟨1, 1⟩}], [(11699)], [(1, 24)], [{⟨1, 1⟩}],[(2, 9, 1),(1, 9, 2)]

---

su(2) ← sp(5852)
so(7) ← so(11704) su(11704)
su(4)

[{⟨1, 1⟩},{⟨11703, 1⟩}],[{⟨1, 1⟩}],[(11703)],[{⟨1, 1⟩}],[(6, 0, 2)],[(10, 0, 6),(6, 0, 10)]

---

su(2) ← so(11715)
su(11715)
su(3)

[{⟨1, 1⟩},{⟨11714, 1⟩}], [{⟨1, 1⟩}], [(11714)], [(65, 4),(4, 65)]

---

su(2) ← sp(5863)
so(11726) su(11726)
su(3)

[{⟨1, 1⟩},{⟨11725, 1⟩}],[{⟨1, 1⟩}],[(11725)],[{⟨1, 1⟩}],[(40, 10),(10, 40)]

---

su(2) ← so(11745)
su(3)
su(11745)
su(4)
su(29)

[{⟨1, 1⟩},{⟨11744, 1⟩}], [{⟨1, 1⟩}], [(11744)], [(86, 2),(2, 86)], [(26, 1, 0),(0, 1, 26)], [{⟨1, 1⟩, ⟨27, 1⟩},{⟨2, 1⟩, ⟨28, 1⟩}]

---

su(2) ← sp(5880)
so(11760)
su(4) su(11760)
su(6)
su(8)

[{⟨1, 1⟩},{⟨11759, 1⟩}],[{⟨1, 1⟩}],[(11759)],[{⟨1, 1⟩}],[(8, 4, 1),(1, 4, 8)],[(2, 0, 2, 0, 1),(1, 0, 2, 0, 2)],[{⟨1, 1⟩, ⟨4, 2⟩},{⟨4, 2⟩, ⟨7, 1⟩}]

---

su(2) ← sp(5890)
su(11780)
so(153)
so(11780)
sp(77)

[{⟨1, 1⟩},{⟨11779, 1⟩}],[{⟨1, 1⟩}],[(11779)],[{⟨1, 1⟩}],[{⟨1, 2⟩}],[{⟨2, 1⟩}]

---

su(2)
so(11781)
so(154)
su(3)
su(4)
su(4) su(11781)
su(153)
su(154)

[{⟨1, 1⟩},{⟨11780, 1⟩}],[{⟨1, 1⟩}],[(11780)],[{⟨2, 1⟩}],[(152, 0),(0, 152)], [(10, 2, 2),(2, 2, 10)], [(10, 5, 0),(0, 5, 10)],[{⟨1, 2⟩},{⟨152, 2⟩}],[{⟨2, 1⟩},{⟨152, 1⟩}]

---

su(2) ← so(11799)
su(11799)
su(3)

[{⟨1, 1⟩},{⟨11798, 1⟩}], [{⟨1, 1⟩}], [(11798)], [(26, 18),(18, 26)]

---

su(2) ← sp(5922)
so(11844) su(11844)
su(3)

[{⟨1, 1⟩},{⟨11843, 1⟩}],[{⟨1, 1⟩}],[(11843)],[{⟨1, 1⟩}],[(46, 8),(8, 46)]

---

su(2) ← sp(5925)
so(11850) su(11850)
su(3)

[{⟨1, 1⟩},{⟨11849, 1⟩}],[{⟨1, 1⟩}],[(11849)],[{⟨1, 1⟩}],[(74, 3),(3, 74)]

---

su(2) ← sp(5940)
su(109) ← so(11880)
su(3)
su(3)
su(3)
su(3) su(11880)
su(5)
su(8)
su(8)
su(10)

[{⟨1, 1⟩},{⟨11879, 1⟩}],[{⟨1, 1⟩}],[(11879)],[{⟨1, 1⟩}],[{⟨1, 1⟩, ⟨108, 1⟩}],[(32, 14),(14, 32)],[(43, 9),(9, 43)],[(59, 5),(5, 59)],[(107, 1),(1, 107)],[(2, 4, 0, 1),(1, 0, 4, 2)], [{⟨1, 2⟩, ⟨5, 1⟩, ⟨7, 1⟩},{⟨1, 1⟩, ⟨3, 1⟩, ⟨7, 2⟩}], [{⟨1, 4⟩, ⟨3, 1⟩},{⟨5, 1⟩, ⟨7, 4⟩}], [{⟨1, 2⟩, ⟨5, 1⟩},{⟨5, 1⟩, ⟨9, 2⟩}]

---

su(2) ← sp(5950)
so(11900) su(11900)
su(4)

[{⟨1, 1⟩},{⟨11899, 1⟩}],[{⟨1, 1⟩}],[(11899)],[{⟨1, 1⟩}],[(9, 1, 4),(4, 1, 9)]

---

su(2) ← so(11907)
su(6) su(11907)
su(7)

[{⟨1, 1⟩},{⟨11906, 1⟩}],[{⟨1, 1⟩}],[(11906)],[(2, 2, 0, 1, 0),(0, 1, 0, 2, 2)], [{⟨1, 2⟩, ⟨3, 1⟩, ⟨5, 1⟩},{⟨2, 1⟩, ⟨4, 1⟩, ⟨6, 2⟩}]

---

su(2) ← sp(5967)
so(154) ← so(11934) su(11934)
su(3)

[{⟨1, 1⟩},{⟨11933, 1⟩}],[{⟨1, 1⟩}],[(11933)],[{⟨1, 1⟩}],[{⟨1, 2⟩}],[(38, 11),(11, 38)]

su(2) ←
so(5) ←
so(5) ←
so(11935) ←
so(33) ←
su(3) ←
so(155) ←
su(3) ← su(11935)
sp(77) ←
su(154) ←
su(155) ←

[{⟨1, 1⟩},{⟨11934, 1⟩}], [{⟨1, 1⟩}], [(11934)], [(1, 30)], [(9, 10)],[{⟨1, 1⟩, ⟨2, 1⟩}],[{⟨2, 1⟩}],[{⟨1, 2⟩}],[(54, 6), (6, 54)], [(153, 0),(0, 153)], [{⟨1, 2⟩},{⟨153, 2⟩}], [{⟨2, 1⟩},{⟨153, 1⟩}]

---

su(2) ← sp(5980) ←
so(11960) ← su(11960)
su(3) ←

[{⟨1, 1⟩},{⟨11959, 1⟩}],[{⟨1, 1⟩}],[(11959)],[{⟨1, 1⟩}], [(25, 19),(19, 25)]

---

su(2) ← sp(5984) ←
so(11968) ← su(11968)
su(33) ←

[{⟨1, 1⟩},{⟨11967, 1⟩}],[{⟨1, 1⟩}],[(11967)],[{⟨1, 1⟩}], [{⟨1, 1⟩, ⟨2, 1⟩},{⟨31, 1⟩, ⟨32, 1⟩}]

---

su(2) ← so(11985) ←
su(11985)
su(3) ←

[{⟨1, 1⟩},{⟨11984, 1⟩}], [{⟨1, 1⟩}], [(11984)], [(29, 16), (16, 29)]

---

su(2) ← sp(6000) ←
su(12000)
su(5) ← so(12000) ←

[{⟨1, 1⟩},{⟨11999, 1⟩}],[{⟨1, 1⟩}],[(11999)],[{⟨1, 1⟩}], [(1, 2, 2, 1)]

---

su(2) ←
so(12005) ←
so(5) ← su(12005)
su(3) ←

[{⟨1, 1⟩},{⟨12004, 1⟩}], [{⟨1, 1⟩}], [(12004)], [(13, 6)], [(34, 13),(13, 34)]

---

su(2) ← sp(6006) ←
so(9) ←
so(12012) ←
sp(4) ←
su(3) ←
su(12) ← su(12012)
su(12) ←
su(12) ←
su(14) ←

[{⟨1, 1⟩},{⟨12011, 1⟩}],[{⟨1, 1⟩}],[(12011)],[{⟨1, 1⟩}], [(1, 0, 2, 0)], [(0, 0, 2, 1)], [(87, 2),(2, 87)], [{⟨1, 1⟩, ⟨2, 2⟩},{⟨10, 2⟩, ⟨11, 1⟩}], [{⟨1, 2⟩, ⟨3, 1⟩},{⟨9, 1⟩, ⟨11, 2⟩}], [{⟨1, 3⟩, ⟨2, 1⟩},{⟨10, 1⟩, ⟨11, 3⟩}], [{⟨1, 1⟩, ⟨4, 1⟩},{⟨10, 1⟩, ⟨13, 1⟩}]

---

su(2) ← so(12025) ←
su(12025)
su(3) ←

[{⟨1, 1⟩},{⟨12024, 1⟩}], [{⟨1, 1⟩}], [(12024)], [(36, 12), (12, 36)]

---

su(2) ← sp(6018) ←
so(12036) ← su(12036)
su(3) ←

[{⟨1, 1⟩},{⟨12035, 1⟩}],[{⟨1, 1⟩}],[(12035)],[{⟨1, 1⟩}], [(50, 7),(7, 50)]

---

su(2) ← sp(6030) ←
so(12060) ← su(12060)
su(3) ←

[{⟨1, 1⟩},{⟨12059, 1⟩}],[{⟨1, 1⟩}],[(12059)],[{⟨1, 1⟩}], [(66, 4),(4, 66)]

---

su(2) ←
sp(6032) ←
sp(2) ← su(12064)
so(12064) ←

[{⟨1, 1⟩},{⟨12063, 1⟩}], [{⟨1, 1⟩}], [(12063)], [(25, 2)], [{⟨1, 1⟩}]

---

su(2) ← so(12075) ←
su(12075)
su(3) ←

[{⟨1, 1⟩},{⟨12074, 1⟩}], [{⟨1, 1⟩}], [(12074)], [(24, 20), (20, 24)]

---

su(2) ←
so(155) ← so(12089) ← su(12089)
sp(78) ←

[{⟨1, 1⟩},{⟨12088, 1⟩}],[{⟨1, 1⟩}],[(12088)],[{⟨1, 2⟩}], [{⟨2, 1⟩}]

---

su(2) ← sp(6045) ←
so(156) ← so(12090) ←
su(3) ← su(12090)
su(155) ←
su(156) ←

[{⟨1, 1⟩},{⟨12089, 1⟩}],[{⟨1, 1⟩}],[(12089)],[{⟨1, 1⟩}], [{⟨2, 1⟩}], [(154, 0),(0, 154)], [{⟨1, 2⟩},{⟨154, 2⟩}], [{⟨2, 1⟩},{⟨154, 1⟩}]

---

su(2) ←
sp(6048) ←
sp(3) ←
g2 ← so(12096) ← su(12096)
su(4) ←
su(4) ←

[{⟨1, 1⟩},{⟨12095, 1⟩}],[{⟨1, 1⟩}],[(12095)],[(3, 1, 2)], [{⟨1, 1⟩}], [(5, 3)], [(8, 2, 3),(3, 2, 8)], [(11, 1, 3),(3, 1, 11)]

---

su(2) ←
so(12099) ←
su(110) ← su(12099)
su(3) ←

[{⟨1, 1⟩},{⟨12098, 1⟩}], [{⟨1, 1⟩}], [(12098)], [{⟨1, 1⟩, ⟨109, 1⟩}],[(108, 1),(1, 108)]

---

su(2) ← sp(6072) ←
so(12144) ← su(12144)
su(3) ←

[{⟨1, 1⟩},{⟨12143, 1⟩}],[{⟨1, 1⟩}],[(12143)],[{⟨1, 1⟩}], [(23, 21),(21, 23)]

---

su(2) ←
so(12155) ← su(12155)
so(5) ←

[{⟨1, 1⟩},{⟨12154, 1⟩}],[{⟨1, 1⟩}],[(12154)],[(16, 4)]

---

su(2) ← sp(6080) ←
so(12160) ← su(12160)
su(3) ←

[{⟨1, 1⟩},{⟨12159, 1⟩}],[{⟨1, 1⟩}],[(12159)],[{⟨1, 1⟩}], [(75, 3),(3, 75)]

---

su(2) ←
so(12167) ← su(12167)
su(3) ←

[{⟨1, 1⟩},{⟨12166, 1⟩}],[{⟨1, 1⟩}],[(12166)],[(22, 22)]

---

su(2) ←
sp(6118) ←
sp(2) ←
so(12236) ← su(12236)
su(4) ←

[{⟨1, 1⟩},{⟨12235, 1⟩}], [{⟨1, 1⟩}], [(12235)], [(3, 18)], [{⟨1, 1⟩}],[(18, 1, 1),(1, 1, 18)]

---

su(2) ← sp(6120) ←
so(12240) ← su(12240)
su(4) ←

[{⟨1, 1⟩},{⟨12239, 1⟩}],[{⟨1, 1⟩}],[(12239)],[{⟨1, 1⟩}], [(1, 14, 0),(0, 14, 1)]

---

su(2) ← so(12243) ←
su(12243)
su(3) ←

[{⟨1, 1⟩},{⟨12242, 1⟩}], [{⟨1, 1⟩}], [(12242)], [(41, 10), (10, 41)]

---

su(2) ←
so(12245) ← su(12245)
so(156) ←

[{⟨1, 1⟩},{⟨12244, 1⟩}],[{⟨1, 1⟩}],[(12244)],[{⟨1, 2⟩}]

---

su(2) ← sp(6123) ←
so(157) ←
so(12246) ←
sp(78) ←
su(3) ← su(12246)
su(156) ←
su(157) ←

[{⟨1, 1⟩},{⟨12245, 1⟩}],[{⟨1, 1⟩}],[(12245)],[{⟨1, 1⟩}], [{⟨2, 1⟩}], [{⟨1, 2⟩}], [(155, 0),(0, 155)], [{⟨1, 2⟩}, {⟨155, 2⟩}],[{⟨2, 1⟩},{⟨155, 1⟩}]

---

su(2) ← sp(6125) ←
so(12250) ← su(12250)
su(6) ←

[{⟨1, 1⟩},{⟨12249, 1⟩}],[{⟨1, 1⟩}],[(12249)],[{⟨1, 1⟩}], [(2, 1, 1, 0, 1),(1, 0, 1, 1, 2)]

---

su(2) ← so(12261) ←
su(12261)
su(3) ←

[{⟨1, 1⟩},{⟨12260, 1⟩}], [{⟨1, 1⟩}], [(12260)], [(60, 5), (5, 60)]

---

su(2) ← so(12267) ←
su(12267)
su(3) ←

[{⟨1, 1⟩},{⟨12266, 1⟩}], [{⟨1, 1⟩}], [(12266)], [(28, 17), (17, 28)]

---

su(2) ← sp(6141) ←
so(12282) ← su(12282)
su(3) ←

[{⟨1, 1⟩},{⟨12281, 1⟩}],[{⟨1, 1⟩}],[(12281)],[{⟨1, 1⟩}], [(88, 2),(2, 88)]

---

su(2) ←
so(12285) ←
so(13) ←
su(4) ← su(12285)
su(5) ←

[{⟨1, 1⟩},{⟨12284, 1⟩}], [{⟨1, 1⟩}], [(12284)], [{⟨2, 1⟩, ⟨3, 1⟩}],[(5, 6, 1),(1, 6, 5)],[(6, 1, 0, 2),(2, 0, 1, 6)]

---

su(2) ← sp(6144) ←
so(12288) ← su(12288)
su(3) ←

[{⟨1, 1⟩},{⟨12287, 1⟩}],[{⟨1, 1⟩}],[(12287)],[{⟨1, 1⟩}], [(31, 15),(15, 31)]

---

su(2) ← sp(6150) ←
su(12300)
so(41) ← so(12300) ←

[{⟨1, 1⟩},{⟨12299, 1⟩}],[{⟨1, 1⟩}],[(12299)],[{⟨1, 1⟩}], [{⟨1, 3⟩}]

---

su(2) ← sp(6156) ←
so(12312) ← su(12312)
su(3) ←

[{⟨1, 1⟩},{⟨12311, 1⟩}],[{⟨1, 1⟩}],[(12311)],[{⟨1, 1⟩}], [(47, 8),(8, 47)]

su(2) ←
sp(2) ← sp(6160) ←
sp(2) ←
su(111) ←
so(8) ← so(12320) ←
so(8) ←
su(3) ←
su(4) ←
su(5) ← su(12320)
su(5) ←
su(5) ←
su(5) ←
su(7) ←
su(9) ←

[{⟨1, 1⟩},{⟨12319, 1⟩}], [{⟨1, 1⟩}], [(12319)], [(9, 10)], [(13, 7)], [{⟨1, 1⟩}], [{⟨1, 1⟩, ⟨110, 1⟩}], [(3, 0, 2, 1),(3, 0, 1, 2),(2, 0, 3, 1),(2, 0, 1, 3),(1, 0, 3, 2),(1, 0, 2, 3)], [(5, 0, 2, 0),(5, 0, 0, 2),(2, 0, 5, 0),(2, 0, 0, 5),(0, 0, 5, 2),(0, 0, 2, 5)], [(109, 1),(1, 109)], [(6, 3, 3),(3, 3, 6)], [(2, 3, 0, 2),(2, 0, 3, 2)], [(3, 1, 1, 2),(2, 1, 1, 3)],[(3, 3, 1, 0),(0, 1, 3, 3)],[(3, 5, 0, 0),(0, 0, 5, 3)], [{⟨1, 5⟩, ⟨4, 1⟩},{⟨3, 1⟩, ⟨6, 5⟩}], [{⟨1, 3⟩, ⟨6, 1⟩},{⟨3, 1⟩, ⟨8, 3⟩}]

---

su(2) ←
so(5) ← so(12341) ←
so(43) ←
su(4) ← su(12341)
su(41) ←
su(43) ←

[{⟨1, 1⟩},{⟨12340, 1⟩}], [{⟨1, 1⟩}], [(12340)], [(0, 40)], [{⟨3, 1⟩}], [(40, 0, 0),(0, 0, 40)], [{⟨1, 3⟩},{⟨40, 3⟩}], [{⟨3, 1⟩},{⟨40, 1⟩}]

---

su(2) ← sp(6174) ←
so(12348) ← su(12348)
su(3) ←

[{⟨1, 1⟩},{⟨12347, 1⟩}],[{⟨1, 1⟩}],[(12347)],[{⟨1, 1⟩}], [(55, 6),(6, 55)]

---

su(2) ←
su(10) ←
so(9) ← so(12375) ←
sp(3) ←
su(3) ← su(12375)
su(5) ←
su(6) ←

[{⟨1, 1⟩},{⟨12374, 1⟩}], [{⟨1, 1⟩}], [(12374)], [{⟨3, 1⟩, ⟨7, 1⟩}], [(3, 0, 0, 2)], [(4, 3, 0)], [(44, 9),(9, 44)], [(8, 0, 0, 3),(3, 0, 0, 8)],[(4, 0, 2, 0, 0),(0, 0, 2, 0, 4)]

---

su(2) ←
sp(2) ← sp(6188) ←
so(17) ←
sp(6) ← so(12376) ←
f4 ←
su(4) ←
su(5) ← su(12376)
su(7) ←
su(12) ←
su(15) ←
su(17) ←

[{⟨1, 1⟩},{⟨12375, 1⟩}], [{⟨1, 1⟩}], [(12375)], [(7, 12)], [{⟨1, 1⟩}], [{⟨6, 1⟩}], [{⟨1, 6⟩}], [(3, 0, 0, 0)], [(2, 12, 0),(0, 12, 2)], [(12, 0, 1, 0),(0, 1, 0, 12)], [{⟨1, 11⟩},{⟨6, 11⟩}], [{⟨1, 6⟩},{⟨11, 6⟩}], [{⟨1, 2⟩, ⟨13, 1⟩},{⟨2, 1⟩, ⟨14, 2⟩}],[{⟨6, 1⟩},{⟨11, 1⟩}]

---

su(2) ←
so(22) ← so(12397) ← su(12397)

[{⟨1, 1⟩},{⟨12396, 1⟩}],[{⟨1, 1⟩}],[(12396)],[{⟨1, 4⟩}]

---

su(2) ← sp(6201) ←
so(157) ←
sp(79) ← so(12402) ← su(12402)

[{⟨1, 1⟩},{⟨12401, 1⟩}],[{⟨1, 1⟩}],[(12401)],[{⟨1, 1⟩}], [{⟨1, 2⟩}],[{⟨2, 1⟩}]

---

su(2) ←
so(158) ← so(12403) ←
su(3) ← su(12403)
su(157) ←
su(158) ←

[{⟨1, 1⟩},{⟨12402, 1⟩}],[{⟨1, 1⟩}],[(12402)],[{⟨2, 1⟩}], [(156, 0),(0, 156)], [{⟨1, 2⟩},{⟨156, 2⟩}], [{⟨2, 1⟩},{⟨156, 1⟩}]

---

su(2) ← sp(6205) ←
so(12410) ← su(12410)
su(3) ←

[{⟨1, 1⟩},{⟨12409, 1⟩}],[{⟨1, 1⟩}],[(12409)],[{⟨1, 1⟩}], [(67, 4),(4, 67)]

---

su(2) ← sp(6237) ←
so(5) ← so(12474) ←
su(3) ← su(12474)
su(5) ←
su(8) ←

[{⟨1, 1⟩},{⟨12473, 1⟩}],[{⟨1, 1⟩}],[(12473)],[{⟨1, 1⟩}], [(11, 8)], [(76, 3),(3, 76)], [(1, 5, 0, 1),(1, 0, 5, 1)], [{⟨1, 1⟩, ⟨2, 2⟩, ⟨7, 1⟩},{⟨1, 1⟩, ⟨6, 2⟩, ⟨7, 1⟩}]

---

su(2) ← sp(6240) ←
so(12480) ← su(12480)
su(3) ←
su(3) ←

[{⟨1, 1⟩},{⟨12479, 1⟩}],[{⟨1, 1⟩}],[(12479)],[{⟨1, 1⟩}], [(39, 11),(11, 39)],[(51, 7),(7, 51)]

---

su(2) ← so(12495) ← su(12495)
su(3) ←

[{⟨1, 1⟩},{⟨12494, 1⟩}], [{⟨1, 1⟩}], [(12494)], [(33, 14), (14, 33)]

---

su(2) ←
sp(2) ← sp(6250) ←
so(12500) ← su(12500)

[{⟨1, 1⟩},{⟨12499, 1⟩}], [{⟨1, 1⟩}], [(12499)], [(19, 4)], [{⟨1, 1⟩}]

---

su(2) ← sp(6251) ←
so(12502) ← su(12502)
su(3) ←

[{⟨1, 1⟩},{⟨12501, 1⟩}],[{⟨1, 1⟩}],[(12501)],[{⟨1, 1⟩}], [(27, 18),(18, 27)]

---

su(2) ←
so(5) ← so(12529) ← su(12529)

[{⟨1, 1⟩},{⟨12528, 1⟩}],[{⟨1, 1⟩}],[(12528)],[(32, 0)]

---

su(2) ← sp(6270) ←
so(12540) ← su(12540)
su(4) ←

[{⟨1, 1⟩},{⟨12539, 1⟩}],[{⟨1, 1⟩}],[(12539)],[{⟨1, 1⟩}], [(9, 0, 7),(7, 0, 9)]

---

su(2) ←
su(112) ← so(12543) ← su(12543)
su(3) ←

[{⟨1, 1⟩},{⟨12542, 1⟩}], [{⟨1, 1⟩}], [(12542)], [{⟨1, 1⟩, ⟨111, 1⟩}],[(110, 1),(1, 110)]

---

su(2) ← sp(6272) ←
so(6) ← so(12544) ← su(12544)
su(14) ←

[{⟨1, 1⟩},{⟨12543, 1⟩}],[{⟨1, 1⟩}],[(12543)],[{⟨1, 1⟩}], [(11, 1, 1)], [{⟨1, 1⟩, ⟨2, 1⟩, ⟨13, 1⟩},{⟨1, 1⟩, ⟨12, 1⟩, ⟨13, 1⟩}]

---

su(2) ← so(12555) ← su(12555)
su(3) ←

[{⟨1, 1⟩},{⟨12554, 1⟩}], [{⟨1, 1⟩}], [(12554)], [(89, 2), (2, 89)]

---

su(2) ← sp(6280) ← su(12560)
so(158) ← so(12560) ←

[{⟨1, 1⟩},{⟨12559, 1⟩}],[{⟨1, 1⟩}],[(12559)],[{⟨1, 1⟩}], [{⟨1, 2⟩}]

---

su(2) ←
so(159) ← so(12561) ←
sp(79) ←
su(3) ← su(12561)
su(158) ←
su(159) ←

[{⟨1, 1⟩},{⟨12560, 1⟩}],[{⟨1, 1⟩}],[(12560)],[{⟨2, 1⟩}], [{⟨1, 2⟩}], [(157, 0),(0, 157)], [{⟨1, 2⟩},{⟨157, 2⟩}], [{⟨2, 1⟩},{⟨157, 1⟩}]

---

su(2) ← sp(6293) ←
so(12586) ← su(12586)
su(4) ←
su(29) ←

[{⟨1, 1⟩},{⟨12585, 1⟩}],[{⟨1, 1⟩}],[(12585)],[{⟨1, 1⟩}], [(27, 0, 1),(1, 0, 27)], [{⟨1, 2⟩, ⟨28, 1⟩},{⟨1, 1⟩, ⟨28, 2⟩}]

---

su(2) ← so(12597) ← su(12597)
su(3) ←

[{⟨1, 1⟩},{⟨12596, 1⟩}], [{⟨1, 1⟩}], [(12596)], [(37, 12), (12, 37)]

---

su(2) ← sp(6300) ←
so(12600) ←
su(3) ←
su(4) ←
su(4) ← su(12600)
su(4) ←
su(5) ←
su(5) ←
su(6) ←

[{⟨1, 1⟩},{⟨12599, 1⟩}],[{⟨1, 1⟩}],[(12599)],[{⟨1, 1⟩}], [(35, 13),(13, 35)], [(6, 4, 2),(2, 4, 6)], [(14, 0, 4),(4, 0, 14)], [(20, 2, 0),(0, 2, 20)], [(5, 0, 2, 1),(1, 2, 0, 5)], [(8, 0, 1, 1),(1, 1, 0, 8)],[(2, 0, 3, 0, 0),(0, 0, 3, 0, 2)]

---

su(2) ← sp(6324) ←
so(12648) ← su(12648)
su(3) ←
su(3) ←

[{⟨1, 1⟩},{⟨12647, 1⟩}],[{⟨1, 1⟩}],[(12647)],[{⟨1, 1⟩}], [(30, 16),(16, 30)],[(61, 5),(5, 61)]

---

su(2) ← sp(6325) ←
so(25) ←
sp(11) ← so(12650) ←
su(5) ← su(12650)
su(22) ←
su(25) ←

[{⟨1, 1⟩},{⟨12649, 1⟩}],[{⟨1, 1⟩}],[(12649)],[{⟨1, 1⟩}], [{⟨4, 1⟩}], [{⟨1, 4⟩}], [(21, 0, 0, 0),(0, 0, 0, 21)], [{⟨1, 4⟩},{⟨21, 4⟩}],[{⟨4, 1⟩},{⟨21, 1⟩}]

---

su(2) ← sp(6336) ← su(12672)
so(9) ←
so(9) ← so(12672) ←
so(9) ←

[{⟨1, 1⟩},{⟨12671, 1⟩}],[{⟨1, 1⟩}],[(12671)],[{⟨1, 1⟩}],[(0, 1, 0, 3)],[(0, 1, 1, 1)],[(5, 0, 0, 1)]

---

su(2) ← sp(6345)
so(12690) ← su(12690)
su(3)

[{⟨1, 1⟩},{⟨12689, 1⟩}],[{⟨1, 1⟩}],[(12689)],[{⟨1, 1⟩}],[(26, 19),(19, 26)]

---

su(2)
so(159) ← so(12719) ← su(12719)
sp(80)

[{⟨1, 1⟩},{⟨12718, 1⟩}],[{⟨1, 1⟩}],[(12718)],[{⟨1, 2⟩}],[{⟨2, 1⟩}]

---

su(2) ← sp(6360)
so(160) ← so(12720)
su(3) ← su(12720)
su(159)
su(160)

[{⟨1, 1⟩},{⟨12719, 1⟩}],[{⟨1, 1⟩}],[(12719)],[{⟨1, 1⟩}],[{⟨2, 1⟩}], [(158, 0),(0, 158)], [{⟨1, 2⟩},{⟨158, 2⟩}],[{⟨2, 1⟩},{⟨158, 1⟩}]

---

su(2) ← sp(6370)
su(6) ← so(12740) ← su(12740)
su(4)

[{⟨1, 1⟩},{⟨12739, 1⟩}],[{⟨1, 1⟩}],[(12739)],[{⟨1, 1⟩}],[(4, 0, 0, 0, 4)],[(12, 0, 5),(5, 0, 12)]

---

su(2) ← sp(6375)
so(12750) ← su(12750)
su(4)

[{⟨1, 1⟩},{⟨12749, 1⟩}],[{⟨1, 1⟩}],[(12749)],[{⟨1, 1⟩}],[(14, 1, 2),(2, 1, 14)]

---

su(2) ← so(12765)
su(12765)
su(3)

[{⟨1, 1⟩},{⟨12764, 1⟩}], [{⟨1, 1⟩}], [(12764)], [(68, 4),(4, 68)]

---

su(2) ← sp(6384)
su(113) ← so(12768)
su(12768)
su(3)
su(3)

[{⟨1, 1⟩},{⟨12767, 1⟩}],[{⟨1, 1⟩}],[(12767)],[{⟨1, 1⟩}],[{⟨1, 1⟩, ⟨112, 1⟩}],[(56, 6),(6, 56)],[(111, 1),(1, 111)]

---

su(2) ← so(12771)
su(12771)
su(3)

[{⟨1, 1⟩},{⟨12770, 1⟩}], [{⟨1, 1⟩}], [(12770)], [(42, 10),(10, 42)]

---

su(2) ← so(12789)
su(12789)
su(3)

[{⟨1, 1⟩},{⟨12788, 1⟩}], [{⟨1, 1⟩}], [(12788)], [(48, 8),(8, 48)]

---

su(2) ← sp(6396)
so(12792) ← su(12792)
su(3)

[{⟨1, 1⟩},{⟨12791, 1⟩}],[{⟨1, 1⟩}],[(12791)],[{⟨1, 1⟩}],[(77, 3),(3, 77)]

---

su(2)
so(12825) ← su(12825)
so(6)

[{⟨1, 1⟩},{⟨12824, 1⟩}],[{⟨1, 1⟩}],[(12824)],[(0, 8, 8)]

---

su(2) ← so(12831)
su(3) ← su(12831)
su(3)

[{⟨1, 1⟩},{⟨12830, 1⟩}], [{⟨1, 1⟩}], [(12830)], [(25, 20), (20, 25)],[(90, 2),(2, 90)]

---

su(2) ← sp(6417)
su(12834)
so(5) ← so(12834)

[{⟨1, 1⟩},{⟨12833, 1⟩}],[{⟨1, 1⟩}],[(12833)],[{⟨1, 1⟩}],[(3, 22)]

---

su(2)
sp(6426)
sp(3)
su(12852)
so(12852)

[{⟨1, 1⟩},{⟨12851, 1⟩}],[{⟨1, 1⟩}],[(12851)],[(0, 1, 5)],[{⟨1, 1⟩}]

---

su(2) ← sp(6435)
su(16)
so(12870)
so(10)
su(4)
su(12870)
su(9)
su(11)

[{⟨1, 1⟩},{⟨12869, 1⟩}],[{⟨1, 1⟩}],[(12869)],[{⟨1, 1⟩}],[{⟨8, 1⟩}], [(4, 1, 0, 0, 0)], [(3, 8, 1),(1, 8, 3)], [{⟨1, 8⟩},{⟨8, 8⟩}],[{⟨1, 1⟩, ⟨9, 2⟩},{⟨2, 2⟩, ⟨10, 1⟩}]

---

su(2)
so(12879) ← su(12879)
so(160)

[{⟨1, 1⟩},{⟨12878, 1⟩}],[{⟨1, 1⟩}],[(12878)],[{⟨1, 2⟩}]

---

su(2)
sp(6440)
sp(2)
so(161)
so(12880)
sp(80)
su(3) ← su(12880)
su(3)
su(160)
su(161)

[{⟨1, 1⟩},{⟨12879, 1⟩}], [{⟨1, 1⟩}], [(12879)], [(15, 6)], [{⟨1, 1⟩}], [{⟨2, 1⟩}], [{⟨1, 2⟩}], [(45, 9),(9, 45)], [(159, 0),(0, 159)],[{⟨1, 2⟩},{⟨159, 2⟩}],[{⟨2, 1⟩},{⟨159, 1⟩}]

---

su(2) ← sp(6460)
so(12920)
su(12920)
su(5)
su(16)

[{⟨1, 1⟩},{⟨12919, 1⟩}],[{⟨1, 1⟩}],[(12919)],[{⟨1, 1⟩}],[(14, 0, 0, 1),(1, 0, 0, 14)], [{⟨1, 3⟩, ⟨15, 1⟩},{⟨1, 1⟩, ⟨15, 3⟩}]

---

su(2)
so(12925)
so(5)
su(12925)
su(3)

[{⟨1, 1⟩},{⟨12924, 1⟩}], [{⟨1, 1⟩}], [(12924)], [(21, 2)],[(24, 21),(21, 24)]

---

su(2) ← sp(6466)
so(12932) ← su(12932)
su(3)

[{⟨1, 1⟩},{⟨12931, 1⟩}],[{⟨1, 1⟩}],[(12931)],[{⟨1, 1⟩}],[(52, 7),(7, 52)]

---

su(2)
sp(6468)
sp(4)
so(8) ← so(12936)
su(3)
su(6)
su(12936)
su(6)
su(7)
su(7)
su(8)

[{⟨1, 1⟩},{⟨12935, 1⟩}], [{⟨1, 1⟩}], [(12935)], [(3, 2, 0, 0)], [{⟨1, 1⟩}], [(2, 1, 1, 1),(1, 1, 2, 1),(1, 1, 1, 2)], [(32, 15),(15, 32)], [(3, 0, 1, 0, 2),(2, 0, 1, 0, 3)], [(3, 2, 0, 0, 1),(1, 0, 0, 2, 3)], [{⟨1, 2⟩, ⟨2, 3⟩},{⟨5, 3⟩, ⟨6, 2⟩}], [{⟨1, 3⟩, ⟨3, 1⟩, ⟨6, 1⟩},{⟨1, 1⟩, ⟨4, 1⟩, ⟨6, 3⟩}], [{⟨1, 6⟩, ⟨7, 1⟩},{⟨1, 1⟩, ⟨7, 6⟩}]

---

su(2)
sp(6480)
sp(2)
so(12960) ← su(12960)
su(3)

[{⟨1, 1⟩},{⟨12959, 1⟩}], [{⟨1, 1⟩}], [(12959)], [(17, 5)], [{⟨1, 1⟩}],[(29, 17),(17, 29)]

---

su(2) ← sp(6486)
so(12972) ← su(12972)
su(3)

[{⟨1, 1⟩},{⟨12971, 1⟩}],[{⟨1, 1⟩}],[(12971)],[{⟨1, 1⟩}],[(23, 22),(22, 23)]

---

su(2)
so(12995)
su(114)
su(12995)
su(3)

[{⟨1, 1⟩},{⟨12994, 1⟩}], [{⟨1, 1⟩}], [(12994)], [{⟨1, 1⟩, ⟨113, 1⟩}],[(112, 1),(1, 112)]

---

su(2) ← sp(6500)
so(13000) ← su(13000)
su(4)

[{⟨1, 1⟩},{⟨12999, 1⟩}],[{⟨1, 1⟩}],[(12999)],[{⟨1, 1⟩}],[(4, 7, 1),(1, 7, 4)]

---

su(2)
so(13013)
so(7) ← so(8)
su(13013)
su(13)

[{⟨1, 1⟩},{⟨13012, 1⟩}], [{⟨1, 1⟩}], [(13012)], [(10, 0, 0, 0),(0, 0, 10, 0),(0, 0, 0, 10)], [(0, 0, 10)], [{⟨2, 1⟩, ⟨3, 1⟩},{⟨10, 1⟩, ⟨11, 1⟩}]

---

su(2) ← sp(6510)
so(13020)
su(13020)
su(4)
su(30)

[{⟨1, 1⟩},{⟨13019, 1⟩}],[{⟨1, 1⟩}],[(13019)],[{⟨1, 1⟩}],[(27, 1, 0),(0, 1, 27)], [{⟨1, 1⟩, ⟨28, 1⟩},{⟨2, 1⟩, ⟨29, 1⟩}]

---

su(2) ← sp(6519)
so(13038) ← su(13038)
su(3)

[{⟨1, 1⟩},{⟨13037, 1⟩}],[{⟨1, 1⟩}],[(13037)],[{⟨1, 1⟩}],[(40, 11),(11, 40)]

---

su(2) ← sp(6520)
su(13040)
so(161)
so(13040)
sp(81)

[{⟨1, 1⟩},{⟨13039, 1⟩}],[{⟨1, 1⟩}],[(13039)],[{⟨1, 1⟩}],[{⟨1, 2⟩}],[{⟨2, 1⟩}]

---

su(2)
so(13041)
so(162)
su(3)
su(3) ← su(13041)
su(161)
su(162)

[{⟨1, 1⟩},{⟨13040, 1⟩}],[{⟨1, 1⟩}],[(13040)],[{⟨2, 1⟩}],[(62, 5),(5, 62)], [(160, 0),(0, 160)], [{⟨1, 2⟩},{⟨160, 2⟩}],[{⟨2, 1⟩},{⟨160, 1⟩}]

---

su(2)
sp(2) ← sp(6528)
sp(17)
su(13056)
so(34) ← so(13056)
su(4)

[{⟨1, 1⟩},{⟨13055, 1⟩}], [{⟨1, 1⟩}], [(13055)], [(31, 1)], [{⟨1, 1⟩, ⟨2, 1⟩}], [{⟨1, 1⟩}], [{⟨1, 1⟩, ⟨2, 1⟩}], [(7, 7, 0),(0, 7, 7)]

su(2) ← sp(6534) ← su(13068)
so(13068) ← su(13068)
su(11) ← su(13068)

[{⟨1, 1⟩},{⟨13067, 1⟩}],[{⟨1, 1⟩}],[(13067)],[{⟨1, 1⟩}], [{⟨2, 1⟩, ⟨4, 1⟩},{⟨7, 1⟩, ⟨9, 1⟩}]

---

su(2) ← sp(6545) ← su(13090)
so(20), $\mathfrak{g}_2$ ← so(13090) ← su(13090)
su(4) ← su(13090)
su(34) ← su(13090)

[{⟨1, 1⟩},{⟨13089, 1⟩}],[{⟨1, 1⟩}],[(13089)],[{⟨1, 1⟩}], [{⟨2, 2⟩}], [(7, 2)], [(16, 3, 0),(0, 3, 16)], [{⟨1, 1⟩, ⟨2, 1⟩},{⟨32, 1⟩, ⟨33, 1⟩}]

---

su(2), sp(2) ← sp(6552) ← su(13104)
su(8) ← so(13104) ← su(13104)
su(4) ← su(13104)

[{⟨1, 1⟩},{⟨13103, 1⟩}], [{⟨1, 1⟩}], [(13103)], [(1, 25)], [{⟨1, 1⟩}],[{⟨1, 3⟩, ⟨7, 3⟩}],[(8, 3, 2),(2, 3, 8)]

---

su(2) ← sp(6555) ← su(13110)
sp(10) ← so(13110) ← su(13110)
su(3) ← su(13110)
su(4) ← su(13110)

[{⟨1, 1⟩},{⟨13109, 1⟩}],[{⟨1, 1⟩}],[(13109)],[{⟨1, 1⟩}], [{⟨2, 2⟩}],[(91, 2),(2, 91)],[(17, 0, 3),(3, 0, 17)]

---

su(2) ← sp(6557) ← su(13114)
so(13114) ← su(13114)
su(3) ← su(13114)

[{⟨1, 1⟩},{⟨13113, 1⟩}],[{⟨1, 1⟩}],[(13113)],[{⟨1, 1⟩}], [(78, 3),(3, 78)]

---

su(2) ← so(13125) ← su(13125)
su(3) ← su(13125)
su(3) ← su(13125)

[{⟨1, 1⟩},{⟨13124, 1⟩}], [{⟨1, 1⟩}], [(13124)], [(34, 14), (14, 34)],[(69, 4),(4, 69)]

---

su(2) ← sp(6578) ← su(13156)
so(13156) ← su(13156)
su(4) ← su(13156)

[{⟨1, 1⟩},{⟨13155, 1⟩}],[{⟨1, 1⟩}],[(13155)],[{⟨1, 1⟩}], [(21, 0, 2),(2, 0, 21)]

---

su(2) ← sp(6591) ← su(13182)
so(13182) ← su(13182)
su(3) ← su(13182)

[{⟨1, 1⟩},{⟨13181, 1⟩}],[{⟨1, 1⟩}],[(13181)],[{⟨1, 1⟩}], [(38, 12),(12, 38)]

---

su(2) ← so(13195) ← su(13195)
su(3) ← su(13195)

[{⟨1, 1⟩},{⟨13194, 1⟩}], [{⟨1, 1⟩}], [(13194)], [(57, 6), (6, 57)]

---

su(2), sp(22) ← sp(6600) ← su(13200)
so(9) ← so(13200) ← su(13200)
su(5) ← su(13200)

[{⟨1, 1⟩},{⟨13199, 1⟩}],[{⟨1, 1⟩}],[(13199)],[{⟨3, 1⟩}], [{⟨1, 1⟩}],[(0, 0, 2, 1)],[(1, 7, 0, 0),(0, 0, 7, 1)]

---

su(2) ← sp(6601) ← su(13202)
so(42), so(162) ← so(13202) ← su(13202)

[{⟨1, 1⟩},{⟨13201, 1⟩}],[{⟨1, 1⟩}],[(13201)],[{⟨1, 1⟩}], [{⟨1, 3⟩}],[{⟨1, 2⟩}]

---

su(2), so(163), sp(81) ← so(13203) ← su(13203)
su(3) ← su(13203)
su(162) ← su(13203)
su(163) ← su(13203)

[{⟨1, 1⟩},{⟨13202, 1⟩}],[{⟨1, 1⟩}],[(13202)],[{⟨2, 1⟩}], [{⟨1, 2⟩}], [(161, 0),(0, 161)], [{⟨1, 2⟩},{⟨161, 2⟩}], [{⟨2, 1⟩},{⟨161, 1⟩}]

---

su(2) ← so(13209) ← su(13209)
su(3) ← su(13209)

[{⟨1, 1⟩},{⟨13208, 1⟩}], [{⟨1, 1⟩}], [(13208)], [(36, 13), (13, 36)]

---

su(2) ← sp(6612) ← su(13224)
su(115) ← so(13224) ← su(13224)
su(3) ← su(13224)
su(3) ← su(13224)

[{⟨1, 1⟩},{⟨13223, 1⟩}],[{⟨1, 1⟩}],[(13223)],[{⟨1, 1⟩}], [{⟨1, 1⟩, ⟨114, 1⟩}], [(28, 18),(18, 28)], [(113, 1),(1, 113)]

---

su(2), sp(2), sp(21) ← sp(6622) ← su(13244)
so(44) ← so(13244) ← su(13244)
su(4) ← su(13244)
su(42) ← su(13244)
su(44) ← su(13244)

[{⟨1, 1⟩},{⟨13243, 1⟩}], [{⟨1, 1⟩}], [(13243)], [(41, 0)], [{⟨1, 3⟩}], [{⟨1, 1⟩}], [{⟨3, 1⟩}], [(41, 0, 0),(0, 0, 41)], [{⟨1, 3⟩},{⟨41, 3⟩}],[{⟨3, 1⟩},{⟨41, 1⟩}]

---

su(2) ← so(13275) ← su(13275)
su(3) ← su(13275)

[{⟨1, 1⟩},{⟨13274, 1⟩}], [{⟨1, 1⟩}], [(13274)], [(49, 8), (8, 49)]

---

su(2), so(5) ← so(13299) ← su(13299)

[{⟨1, 1⟩},{⟨13298, 1⟩}],[{⟨1, 1⟩}],[(13298)],[(8, 12)]

---

su(2) ← sp(6650) ← su(13300)
so(6) ← so(13300) ← su(13300)
su(4) ← su(13300)
su(20) ← su(13300)

[{⟨1, 1⟩},{⟨13299, 1⟩}],[{⟨1, 1⟩}],[(13299)],[{⟨1, 1⟩}], [(18, 0, 0)],[(13, 4, 0),(0, 4, 13)],[{⟨2, 2⟩},{⟨18, 2⟩}]

---

su(2) ← sp(6655) ← su(13310)
so(13310) ← su(13310)
su(3) ← su(13310)

[{⟨1, 1⟩},{⟨13309, 1⟩}],[{⟨1, 1⟩}],[(13309)],[{⟨1, 1⟩}], [(43, 10),(10, 43)]

---

su(2), so(13) ← sp(6656) ← su(13312)
so(16) ← so(13312) ← su(13312)

[{⟨1, 1⟩},{⟨13311, 1⟩}], [{⟨1, 1⟩}], [(13311)], [{⟨3, 1⟩, ⟨6, 1⟩}],[{⟨1, 1⟩}],[{⟨2, 1⟩, ⟨7, 1⟩},{⟨2, 1⟩, ⟨8, 1⟩}]

---

su(2) ← sp(6664) ← su(13328)
so(13328) ← su(13328)
su(3) ← su(13328)

[{⟨1, 1⟩},{⟨13327, 1⟩}],[{⟨1, 1⟩}],[(13327)],[{⟨1, 1⟩}], [(31, 16),(16, 31)]

---

su(2), so(5), so(163), sp(82) ← so(13365) ← su(13365)
su(5) ← su(13365)

[{⟨1, 1⟩},{⟨13364, 1⟩}], [{⟨1, 1⟩}], [(13364)], [(2, 26)], [{⟨1, 2⟩}],[{⟨2, 1⟩}],[(5, 2, 1, 0),(0, 1, 2, 5)]

---

su(2) ← sp(6683) ← su(13366)
so(164) ← so(13366) ← su(13366)
su(3) ← su(13366)
su(163) ← su(13366)
su(164) ← su(13366)

[{⟨1, 1⟩},{⟨13365, 1⟩}],[{⟨1, 1⟩}],[(13365)],[{⟨1, 1⟩}], [{⟨2, 1⟩}], [(162, 0),(0, 162)], [{⟨1, 2⟩},{⟨162, 2⟩}], [{⟨2, 1⟩},{⟨162, 1⟩}]

---

su(2), sp(2) ← sp(6688) ← su(13376)
so(13376) ← su(13376)

[{⟨1, 1⟩},{⟨13375, 1⟩}], [{⟨1, 1⟩}], [(13375)], [(5, 15)], [{⟨1, 1⟩}]

---

su(2) ← sp(6696) ← su(13392)
so(13392) ← su(13392)
su(3) ← su(13392)
su(3) ← su(13392)

[{⟨1, 1⟩},{⟨13391, 1⟩}],[{⟨1, 1⟩}],[(13391)],[{⟨1, 1⟩}], [(53, 7),(7, 53)],[(92, 2),(2, 92)]

---

su(2) ← so(13395) ← su(13395)
su(3) ← su(13395)

[{⟨1, 1⟩},{⟨13394, 1⟩}], [{⟨1, 1⟩}], [(13394)], [(46, 9), (9, 46)]

---

su(2) ← sp(6720) ← su(13440)
so(15) ← so(13440) ← su(13440)
su(3) ← su(13440)
su(3) ← su(13440)
su(3) ← su(13440)
su(6) ← su(13440)
su(6) ← su(13440)

[{⟨1, 1⟩},{⟨13439, 1⟩}],[{⟨1, 1⟩}],[(13439)],[{⟨1, 1⟩}], [{⟨1, 2⟩, ⟨7, 1⟩}], [(27, 19),(19, 27)], [(63, 5),(5, 63)], [(79, 3),(3, 79)], [(2, 0, 1, 1, 1),(1, 1, 1, 0, 2)], [(5, 0, 0, 1, 1),(1, 1, 0, 0, 5)]

---

su(2), su(116) ← so(13455) ← su(13455)
su(3) ← su(13455)

[{⟨1, 1⟩},{⟨13454, 1⟩}], [{⟨1, 1⟩}], [(13454)], [{⟨1, 1⟩, ⟨115, 1⟩}],[(114, 1),(1, 114)]

---

su(2) ← sp(6732) ← su(13464)
so(13464) ← su(13464)
su(4) ← su(13464)

[{⟨1, 1⟩},{⟨13463, 1⟩}],[{⟨1, 1⟩}],[(13463)],[{⟨1, 1⟩}], [(8, 1, 5),(5, 1, 8)]

---

su(2) ← so(13475) ← su(13475)
su(7) ← su(13475)

[{⟨1, 1⟩},{⟨13474, 1⟩}], [{⟨1, 1⟩}], [(13474)], [{⟨1, 3⟩, ⟨5, 2⟩},{⟨2, 2⟩, ⟨6, 3⟩}]

---

su(2) ← sp(6745) ← su(13490)
so(13490) ← su(13490)
su(3) ← su(13490)

[{⟨1, 1⟩},{⟨13489, 1⟩}],[{⟨1, 1⟩}],[(13489)],[{⟨1, 1⟩}], [(70, 4),(4, 70)]

---

su(2) ← sp(6750) ← su(13500)
so(13500) ← su(13500)
su(4) ← su(13500)
su(4) ← su(13500)

[{⟨1, 1⟩},{⟨13499, 1⟩}],[{⟨1, 1⟩}],[(13499)],[{⟨1, 1⟩}], [(5, 3, 4),(4, 3, 5)],[(14, 2, 1),(1, 2, 14)]

su(2), so(164) ← so(13529) ← su(13529)

[{⟨1, 1⟩},{⟨13528, 1⟩}],[{⟨1, 1⟩}],[(13528)],[{⟨1, 2⟩}]

---

su(2) ← sp(6765); so(165), sp(82) ← so(13530); su(3); su(164); su(165) ← su(13530)

[{⟨1, 1⟩},{⟨13529, 1⟩}],[{⟨1, 1⟩}],[(13529)],[{⟨1, 1⟩}], [{⟨2, 1⟩}], [{⟨1, 2⟩}], [(163, 0),(0, 163)], [{⟨1, 2⟩}, {⟨163, 2⟩}],[{⟨2, 1⟩},{⟨163, 1⟩}]

---

su(2) ← sp(6800); so(13600); su(3) ← su(13600)

[{⟨1, 1⟩},{⟨13599, 1⟩}],[{⟨1, 1⟩}],[(13599)],[{⟨1, 1⟩}], [(33, 15),(15, 33)]

---

su(2) ← sp(6804); so(13608); su(3); su(3) ← su(13608)

[{⟨1, 1⟩},{⟨13607, 1⟩}],[{⟨1, 1⟩}],[(13607)],[{⟨1, 1⟩}], [(26, 20),(20, 26)],[(41, 11),(11, 41)]

---

su(2) ← so(13629); su(3) ← su(13629)

[{⟨1, 1⟩},{⟨13628, 1⟩}], [{⟨1, 1⟩}], [(13628)], [(58, 6), (6, 58)]

---

su(2) ← sp(6825); so(11), sp(6) ← so(13650); su(5); su(5); su(6); su(14) ← su(13650)

[{⟨1, 1⟩},{⟨13649, 1⟩}],[{⟨1, 1⟩}],[(13649)],[{⟨1, 1⟩}], [(0, 3, 0, 0, 0)],[{⟨3, 2⟩}],[(6, 0, 1, 2),(2, 1, 0, 6)],[(8, 0, 2, 0),(0, 2, 0, 8)], [(9, 1, 0, 0, 0),(0, 0, 0, 1, 9)], [{⟨1, 1⟩, ⟨10, 1⟩},{⟨4, 1⟩, ⟨13, 1⟩}]

---

su(2) ← so(13671); su(3) ← su(13671)

[{⟨1, 1⟩},{⟨13670, 1⟩}], [{⟨1, 1⟩}], [(13670)], [(30, 17), (17, 30)]

---

su(2) ← so(13677); su(3) ← su(13677)

[{⟨1, 1⟩},{⟨13676, 1⟩}], [{⟨1, 1⟩}], [(13676)], [(93, 2), (2, 93)]

---

su(2), so(5) ← so(13685) ← su(13685)

[{⟨1, 1⟩},{⟨13684, 1⟩}],[{⟨1, 1⟩}],[(13684)],[(33, 0)]

---

su(2) ← sp(6844); su(117) ← so(13688); su(3) ← su(13688)

[{⟨1, 1⟩},{⟨13687, 1⟩}],[{⟨1, 1⟩}],[(13687)],[{⟨1, 1⟩}], [{⟨1, 1⟩, ⟨116, 1⟩}],[(115, 1),(1, 115)]

---

su(2) ← sp(6847); so(165), sp(83) ← so(13694) ← su(13694)

[{⟨1, 1⟩},{⟨13693, 1⟩}],[{⟨1, 1⟩}],[(13693)],[{⟨1, 1⟩}], [{⟨1, 2⟩}],[{⟨2, 1⟩}]

---

su(2), so(166) ← so(13695); su(3); su(165); su(166) ← su(13695)

[{⟨1, 1⟩},{⟨13694, 1⟩}],[{⟨1, 1⟩}],[(13694)],[{⟨2, 1⟩}], [(164, 0),(0, 164)], [{⟨1, 2⟩},{⟨164, 2⟩}], [{⟨2, 1⟩}, {⟨164, 1⟩}]

---

su(2), sp(4), sp(4), so(12) ← sp(6864); sp(4), so(8) ← so(13728); su(3); su(12) ← su(13728)

[{⟨1, 1⟩},{⟨13727, 1⟩}], [{⟨1, 1⟩}], [(13727)], [(0, 1, 1, 1)], [(2, 1, 1, 0)], [{⟨1, 1⟩, ⟨2, 1⟩, ⟨5, 1⟩},{⟨1, 1⟩, ⟨2, 1⟩, ⟨6, 1⟩}], [{⟨1, 1⟩}], [(2, 0, 0, 2)], [(7, 0, 1, 0),(7, 0, 0, 1), (1, 0, 7, 0),(1, 0, 0, 7),(0, 0, 7, 1),(0, 0, 1, 7)], [(25, 21), (21, 25)],[{⟨2, 1⟩, ⟨9, 1⟩},{⟨3, 1⟩, ⟨10, 1⟩}]

---

su(2) ← sp(6885); so(13770); su(3); su(3); su(3) ← su(13770)

[{⟨1, 1⟩},{⟨13769, 1⟩}],[{⟨1, 1⟩}],[(13769)],[{⟨1, 1⟩}], [(35, 14),(14, 35)],[(50, 8),(8, 50)],[(80, 3),(3, 80)]

---

su(2) ← sp(6890); so(13780); su(3) ← su(13780)

[{⟨1, 1⟩},{⟨13779, 1⟩}],[{⟨1, 1⟩}],[(13779)],[{⟨1, 1⟩}], [(39, 12),(12, 39)]

---

su(2) ← sp(6900); so(13800); su(3) ← su(13800)

[{⟨1, 1⟩},{⟨13799, 1⟩}],[{⟨1, 1⟩}],[(13799)],[{⟨1, 1⟩}], [(24, 22),(22, 24)]

---

su(2) ← sp(6912); su(3), so(7) ← so(13824); su(4); su(8) ← su(13824)

[{⟨1, 1⟩},{⟨13823, 1⟩}],[{⟨1, 1⟩}],[(13823)],[{⟨1, 1⟩}], [(23, 23)], [(5, 1, 1)], [(11, 3, 1),(1, 3, 11)], [{⟨1, 3⟩, ⟨2, 1⟩, ⟨7, 1⟩},{⟨1, 1⟩, ⟨6, 1⟩, ⟨7, 3⟩}]

---

su(2) ← sp(6916); so(13832); su(3) ← su(13832)

[{⟨1, 1⟩},{⟨13831, 1⟩}],[{⟨1, 1⟩}],[(13831)],[{⟨1, 1⟩}], [(37, 13),(13, 37)]

---

su(2) ← so(13845); su(3) ← su(13845)

[{⟨1, 1⟩},{⟨13844, 1⟩}], [{⟨1, 1⟩}], [(13844)], [(64, 5), (5, 64)]

---

su(2) ← sp(6930); so(166) ← so(13860); su(3); su(3); su(3); su(5); su(5); su(6); su(6); su(6); su(7); su(7); su(8); su(10); su(10); su(10) ← su(13860)

[{⟨1, 1⟩},{⟨13859, 1⟩}],[{⟨1, 1⟩}],[(13859)],[{⟨1, 1⟩}], [{⟨1, 2⟩}], [(44, 10),(10, 44)], [(54, 7),(7, 54)], [(71, 4), (4, 71)],[(2, 0, 4, 1),(1, 4, 0, 2)],[(2, 6, 0, 0),(0, 0, 6, 2)], [(0, 6, 0, 0, 0),(0, 0, 0, 6, 0)], [(2, 4, 0, 0, 0),(0, 0, 0, 4, 2)],[(7, 0, 0, 0, 2),(2, 0, 0, 0, 7)],[{⟨1, 3⟩, ⟨4, 1⟩, ⟨6, 1⟩}, {⟨1, 1⟩, ⟨3, 1⟩, ⟨6, 3⟩}], [{⟨1, 4⟩, ⟨2, 2⟩},{⟨5, 2⟩, ⟨6, 4⟩}],[{⟨2, 4⟩},{⟨6, 4⟩}],[{⟨4, 2⟩},{⟨6, 2⟩}],[{⟨3, 1⟩, ⟨4, 1⟩},{⟨6, 1⟩, ⟨7, 1⟩}], [{⟨1, 1⟩, ⟨2, 1⟩, ⟨8, 1⟩},{⟨2, 1⟩, ⟨8, 1⟩, ⟨9, 1⟩}]

---

su(2), so(167), sp(83) ← so(13861); su(3); su(166); su(167) ← su(13861)

[{⟨1, 1⟩},{⟨13860, 1⟩}],[{⟨1, 1⟩}],[(13860)],[{⟨2, 1⟩}], [{⟨1, 2⟩}], [(165, 0),(0, 165)], [{⟨1, 2⟩},{⟨165, 2⟩}], [{⟨2, 1⟩},{⟨165, 1⟩}]

---

su(2) ← sp(6960); so(13920); su(3); su(4); su(30) ← su(13920)

[{⟨1, 1⟩},{⟨13919, 1⟩}],[{⟨1, 1⟩}],[(13919)],[{⟨1, 1⟩}], [(47, 9),(9, 47)],[(28, 0, 1),(1, 0, 28)],[{⟨1, 2⟩, ⟨29, 1⟩}, {⟨1, 1⟩, ⟨29, 2⟩}]

---

su(2), su(118) ← so(13923); su(3) ← su(13923)

[{⟨1, 1⟩},{⟨13922, 1⟩}], [{⟨1, 1⟩}], [(13922)], [{⟨1, 1⟩, ⟨117, 1⟩}],[(116, 1),(1, 116)]

---

su(2) ← so(13965); su(3); su(3) ← su(13965)

[{⟨1, 1⟩},{⟨13964, 1⟩}], [{⟨1, 1⟩}], [(13964)], [(29, 18), (18, 29)],[(94, 2),(2, 94)]

---

su(2) ← sp(7007); so(12) ← so(14014) ← su(14014)

[{⟨1, 1⟩},{⟨14013, 1⟩}],[{⟨1, 1⟩}],[(14013)],[{⟨1, 1⟩}], [{⟨3, 2⟩}]

---

su(2) ← so(14025); su(3) ← su(14025)

[{⟨1, 1⟩},{⟨14024, 1⟩}], [{⟨1, 1⟩}], [(14024)], [(32, 16), (16, 32)]

---

su(2), so(167), sp(84) ← so(14027) ← su(14027)

[{⟨1, 1⟩},{⟨14026, 1⟩}],[{⟨1, 1⟩}],[(14026)],[{⟨1, 2⟩}],[{⟨2, 1⟩}]

su(2) ← sp(7014)
so(168) ← so(14028)
su(3) ← su(14028)
su(167)
su(168)

[{⟨1, 1⟩},{⟨14027, 1⟩}],[{⟨1, 1⟩}],[(14027)],[{⟨1, 1⟩}],[{⟨2, 1⟩}], [(166, 0),(0, 166)], [{⟨1, 2⟩},{⟨166, 2⟩}],[{⟨2, 1⟩},{⟨166, 1⟩}]

---

su(2) ← sp(7035)
so(14070) ← su(14070)
su(3)

[{⟨1, 1⟩},{⟨14069, 1⟩}],[{⟨1, 1⟩}],[(14069)],[{⟨1, 1⟩}],[(59, 6),(6, 59)]

---

su(2)
sp(2) ← sp(7040)
sp(2) ← so(14080)
su(4) ← su(14080)
su(4)

[{⟨1, 1⟩},{⟨14079, 1⟩}], [{⟨1, 1⟩}], [(14079)], [(3, 19)], [(11, 9)], [{⟨1, 1⟩}], [(7, 2, 4),(4, 2, 7)], [(19, 1, 1),(1, 1, 19)]

---

su(2) ← sp(7052)
so(14104) ← su(14104)
su(3)

[{⟨1, 1⟩},{⟨14103, 1⟩}],[{⟨1, 1⟩}],[(14103)],[{⟨1, 1⟩}],[(81, 3),(3, 81)]

---

su(2)
so(14105) ← su(14105)
so(5)

[{⟨1, 1⟩},{⟨14104, 1⟩}],[{⟨1, 1⟩}],[(14104)],[(4, 20)]

---

su(2)
sp(7056)
su(6)
so(14112) ← su(14112)
su(8)

[{⟨1, 1⟩},{⟨14111, 1⟩}],[{⟨1, 1⟩}],[(14111)],[(0, 0, 5, 0, 0)],[{⟨1, 1⟩}],[{⟨3, 3⟩},{⟨5, 3⟩}]

---

su(2) ← sp(7072)
su(16) ← so(14144) ← su(14144)
su(4)

[{⟨1, 1⟩},{⟨14143, 1⟩}],[{⟨1, 1⟩}],[(14143)],[{⟨1, 1⟩}],[{⟨2, 1⟩, ⟨14, 1⟩}],[(3, 11, 0),(0, 11, 3)]

---

su(2)
so(14145) ← su(14145)
so(5)

[{⟨1, 1⟩},{⟨14144, 1⟩}],[{⟨1, 1⟩}],[(14144)],[(17, 4)]

---

su(2)
so(14147) ← su(14147)
so(43)

[{⟨1, 1⟩},{⟨14146, 1⟩}],[{⟨1, 1⟩}],[(14146)],[{⟨1, 3⟩}]

---

su(2) ← sp(7080)
su(119) ← so(14160) ← su(14160)
su(3)

[{⟨1, 1⟩},{⟨14159, 1⟩}],[{⟨1, 1⟩}],[(14159)],[{⟨1, 1⟩}],[{⟨1, 1⟩, ⟨118, 1⟩}],[(117, 1),(1, 117)]

---

su(2)
so(14175)
su(15) ← su(14175)
su(6)

[{⟨1, 1⟩},{⟨14174, 1⟩}], [{⟨1, 1⟩}], [(14174)], [{⟨1, 2⟩, ⟨14, 2⟩}],[(2, 1, 0, 2, 0),(0, 2, 0, 1, 2)]

---

su(2) ← sp(7095)
so(5)
so(14190)
so(45)
su(3) ← su(14190)
su(4)
su(43)
su(45)

[{⟨1, 1⟩},{⟨14189, 1⟩}],[{⟨1, 1⟩}],[(14189)],[{⟨1, 1⟩}],[(0, 42)], [{⟨3, 1⟩}], [(42, 11),(11, 42)], [(42, 0, 0),(0, 0, 42)],[{⟨1, 3⟩},{⟨42, 3⟩}],[{⟨3, 1⟩},{⟨42, 1⟩}]

---

su(2)
so(14195) ← su(14195)
so(168)

[{⟨1, 1⟩},{⟨14194, 1⟩}],[{⟨1, 1⟩}],[(14194)],[{⟨1, 2⟩}]

---

su(2) ← sp(7098)
so(169)
so(14196)
sp(84)
su(3) ← su(14196)
su(168)
su(169)

[{⟨1, 1⟩},{⟨14195, 1⟩}],[{⟨1, 1⟩}],[(14195)],[{⟨1, 1⟩}],[{⟨2, 1⟩}], [{⟨1, 2⟩}], [(167, 0),(0, 167)], [{⟨1, 2⟩},{⟨167, 2⟩}],[{⟨2, 1⟩},{⟨167, 1⟩}]

---

su(2) ← sp(7105)
so(14210) ← su(14210)
su(3)

[{⟨1, 1⟩},{⟨14209, 1⟩}],[{⟨1, 1⟩}],[(14209)],[{⟨1, 1⟩}],[(28, 19),(19, 28)]

---

su(2) ← sp(7106)
su(14212)
so(18) ← so(14212)

[{⟨1, 1⟩},{⟨14211, 1⟩}],[{⟨1, 1⟩}],[(14211)],[{⟨1, 1⟩}],[{⟨1, 2⟩, ⟨2, 1⟩}]

---

su(2) ← so(14235)
su(14235)
su(3)

[{⟨1, 1⟩},{⟨14234, 1⟩}], [{⟨1, 1⟩}], [(14234)], [(72, 4),(4, 72)]

---

su(2)
so(5)
so(14245) ← su(14245)
so(5)
so(35)

[{⟨1, 1⟩},{⟨14244, 1⟩}], [{⟨1, 1⟩}], [(14244)], [(1, 32)], [(14, 6)],[{⟨1, 1⟩, ⟨2, 1⟩}]

---

su(2) ← sp(7128)
so(14256)
su(14256)
su(3)
su(3)

[{⟨1, 1⟩},{⟨14255, 1⟩}],[{⟨1, 1⟩}],[(14255)],[{⟨1, 1⟩}],[(65, 5),(5, 65)],[(95, 2),(2, 95)]

---

su(2) ← sp(7130)
su(14260)
so(5) ← so(14260)

[{⟨1, 1⟩},{⟨14259, 1⟩}],[{⟨1, 1⟩}],[(14259)],[{⟨1, 1⟩}],[(7, 14)]

---

su(2) ← sp(7137)
so(14274) ← su(14274)
su(3)

[{⟨1, 1⟩},{⟨14273, 1⟩}],[{⟨1, 1⟩}],[(14273)],[{⟨1, 1⟩}],[(51, 8),(8, 51)]

---

su(2) ← sp(7140)
so(14280)
su(3)
su(4) ← su(14280)
su(4)
su(4)
su(35)

[{⟨1, 1⟩},{⟨14279, 1⟩}],[{⟨1, 1⟩}],[(14279)],[{⟨1, 1⟩}],[(34, 15),(15, 34)], [(6, 8, 0),(0, 8, 6)], [(7, 1, 6),(6, 1, 7)], [(9, 6, 0),(0, 6, 9)], [{⟨1, 1⟩, ⟨2, 1⟩},{⟨33, 1⟩, ⟨34, 1⟩}]

---

su(2) ← sp(7150)
so(13)
sp(3) su(14300)
so(14300)
sp(4)
su(4)
sp(5)
su(10)

[{⟨1, 1⟩},{⟨14299, 1⟩}],[{⟨1, 1⟩}],[(14299)],[{⟨1, 1⟩}],[{⟨1, 1⟩, ⟨5, 1⟩}],[(9, 0, 1)],[(2, 1, 0, 1)],[(4, 1, 0, 0, 0)],[(21, 2, 0),(0, 2, 21)], [{⟨1, 2⟩, ⟨2, 1⟩, ⟨9, 1⟩},{⟨1, 1⟩, ⟨8, 1⟩, ⟨9, 2⟩}]

---

su(2)
sp(7168)
sp(2)
so(14336)
su(3) ← su(14336)
su(4)
su(7)

[{⟨1, 1⟩},{⟨14335, 1⟩}], [{⟨1, 1⟩}], [(14335)], [(23, 3)], [{⟨1, 1⟩}], [(55, 7),(7, 55)], [(7, 5, 1),(1, 5, 7)], [{⟨1, 1⟩, ⟨2, 1⟩, ⟨3, 1⟩, ⟨6, 1⟩},{⟨1, 1⟩, ⟨4, 1⟩, ⟨5, 1⟩, ⟨6, 1⟩}]

---

su(2)
sp(7182)
sp(10)
so(19)
su(14364)
so(169)
so(14364)
sp(9)
su(4)
sp(85)

[{⟨1, 1⟩},{⟨14363, 1⟩}],[{⟨1, 1⟩}],[(14363)],[{⟨5, 1⟩}],[{⟨1, 1⟩}],[{⟨1, 1⟩, ⟨3, 1⟩}],[{⟨1, 2⟩}],[{⟨1, 2⟩, ⟨2, 1⟩}],[{⟨2, 1⟩}],[(11, 5, 0),(0, 5, 11)]

---

su(2)
so(14365)
so(170)
su(3)
su(14365)
su(169)
su(170)

[{⟨1, 1⟩},{⟨14364, 1⟩}],[{⟨1, 1⟩}],[(14364)],[{⟨2, 1⟩}],[(168, 0),(0, 168)], [{⟨1, 2⟩},{⟨168, 2⟩}], [{⟨2, 1⟩},{⟨168, 1⟩}]

---

su(2) ← sp(7192)
so(14384)
su(14384)
su(4)
su(31)

[{⟨1, 1⟩},{⟨14383, 1⟩}],[{⟨1, 1⟩}],[(14383)],[{⟨1, 1⟩}],[(28, 1, 0),(0, 1, 28)], [{⟨1, 1⟩, ⟨29, 1⟩},{⟨2, 1⟩, ⟨30, 1⟩}]

---

su(2) ← so(14391)
su(14391)
su(3)

[{⟨1, 1⟩},{⟨14390, 1⟩}], [{⟨1, 1⟩}], [(14390)], [(40, 12),(12, 40)]

---

su(2)
so(14399)
su(120)
su(14399)
su(3)

[{⟨1, 1⟩},{⟨14398, 1⟩}], [{⟨1, 1⟩}], [(14398)], [{⟨1, 1⟩, ⟨119, 1⟩}],[(118, 1),(1, 118)]

su(2) ← sp(7200)
so(14400)
su(3)
su(8)
su(14400)

[{⟨1, 1⟩},{⟨14399, 1⟩}],[{⟨1, 1⟩}],[(14399)],[{⟨1, 1⟩}], [(31, 17),(17, 31)],[{⟨2, 2⟩, ⟨5, 1⟩},{⟨3, 1⟩, ⟨6, 2⟩}]

---

su(2) ← sp(7203)
so(14406)
su(3)
su(14406)

[{⟨1, 1⟩},{⟨14405, 1⟩}],[{⟨1, 1⟩}],[(14405)],[{⟨1, 1⟩}], [(27, 20),(20, 27)]

---

su(2) ← so(14421)
su(3)
su(14421)

[{⟨1, 1⟩},{⟨14420, 1⟩}], [{⟨1, 1⟩}], [(14420)], [(45, 10), (10, 45)]

---

su(2) ← sp(7215)
so(14430)
su(3)
su(14430)

[{⟨1, 1⟩},{⟨14429, 1⟩}],[{⟨1, 1⟩}],[(14429)],[{⟨1, 1⟩}], [(36, 14),(14, 36)]

---

su(2) ← sp(7221)
so(14442)
su(3)
su(14442)

[{⟨1, 1⟩},{⟨14441, 1⟩}],[{⟨1, 1⟩}],[(14441)],[{⟨1, 1⟩}], [(82, 3),(3, 82)]

---

su(2) ← so(14455)
su(3)
su(14455)

[{⟨1, 1⟩},{⟨14454, 1⟩}], [{⟨1, 1⟩}], [(14454)], [(48, 9), (9, 48)]

---

su(2) ← so(14469)
su(3)
su(14469)

[{⟨1, 1⟩},{⟨14468, 1⟩}], [{⟨1, 1⟩}], [(14468)], [(38, 13), (13, 38)]

---

su(2) ← sp(7259)
so(14518)
su(3)
su(14518)

[{⟨1, 1⟩},{⟨14517, 1⟩}],[{⟨1, 1⟩}],[(14517)],[{⟨1, 1⟩}], [(60, 6),(6, 60)]

---

su(2) ← sp(7267)
so(170) ← so(14534)
su(14534)

[{⟨1, 1⟩},{⟨14533, 1⟩}],[{⟨1, 1⟩}],[(14533)],[{⟨1, 1⟩}], [{⟨1, 2⟩}]

---

su(2)
so(171) ← so(14535)
sp(85)
su(3)
su(5)
su(18)
su(170)
su(18)
su(19) ← su(171)
su(14535)

[{⟨1, 1⟩},{⟨14534, 1⟩}],[{⟨1, 1⟩}],[(14534)],[{⟨2, 1⟩}], [{⟨1, 2⟩}],[(169, 0),(0, 169)],[(14, 1, 0, 0),(0, 0, 1, 14)], [{⟨1, 1⟩, ⟨15, 1⟩},{⟨3, 1⟩, ⟨17, 1⟩}], [{⟨1, 2⟩}, {⟨169, 2⟩}], [{⟨2, 1⟩},{⟨169, 1⟩}], [{⟨1, 2⟩, ⟨2, 1⟩}, {⟨16, 1⟩, ⟨17, 2⟩}],[{⟨1, 1⟩, ⟨3, 1⟩},{⟨16, 1⟩, ⟨18, 1⟩}]

---

su(2) ← sp(7275)
so(14550)
su(3)
su(14550)

[{⟨1, 1⟩},{⟨14549, 1⟩}],[{⟨1, 1⟩}],[(14549)],[{⟨1, 1⟩}], [(96, 2),(2, 96)]

---

su(2) ← so(14553)
su(3)
su(14553)

[{⟨1, 1⟩},{⟨14552, 1⟩}], [{⟨1, 1⟩}], [(14552)], [(26, 21), (21, 26)]

---

su(2) ← sp(7280)
so(14560)
su(4)
su(5)
su(14560)

[{⟨1, 1⟩},{⟨14559, 1⟩}],[{⟨1, 1⟩}],[(14559)],[{⟨1, 1⟩}], [(11, 0, 6),(6, 0, 11)],[(7, 3, 0, 0),(0, 0, 3, 7)]

---

su(2) ← sp(7290)
so(6) ← so(14580)
su(4)
su(4)
su(14580)

[{⟨1, 1⟩},{⟨14579, 1⟩}],[{⟨1, 1⟩}],[(14579)],[{⟨1, 1⟩}], [(8, 2, 2)],[(5, 5, 2),(2, 5, 5)],[(11, 2, 2),(2, 2, 11)]

---

su(2) ← so(14615)
su(3)
su(14615)

[{⟨1, 1⟩},{⟨14614, 1⟩}], [{⟨1, 1⟩}], [(14614)], [(73, 4), (4, 73)]

---

su(2)
sp(2)
sp(7308)
so(14616)
su(14616)

[{⟨1, 1⟩},{⟨14615, 1⟩}], [{⟨1, 1⟩}], [(14615)], [(1, 26)], [{⟨1, 1⟩}]

---

su(2)
sp(13)
so(14625)
su(5)
su(14625)

[{⟨1, 1⟩},{⟨14624, 1⟩}],[{⟨1, 1⟩}],[(14624)],[{⟨4, 1⟩}], [(9, 1, 0, 1),(1, 0, 1, 9)]

---

su(2) ← sp(7320)
su(121) ← so(14640)
su(3)
su(14640)

[{⟨1, 1⟩},{⟨14639, 1⟩}],[{⟨1, 1⟩}],[(14639)],[{⟨1, 1⟩}], [{⟨1, 1⟩, ⟨120, 1⟩}],[(119, 1),(1, 119)]

---

su(2)
so(5)
so(14641) ← su(14641)

[{⟨1, 1⟩},{⟨14640, 1⟩}],[{⟨1, 1⟩}],[(14640)],[(10, 10)]

---

su(2)
so(5)
so(14651)
su(3)
su(14651)

[{⟨1, 1⟩},{⟨14650, 1⟩}], [{⟨1, 1⟩}], [(14650)], [(22, 2)], [(25, 22),(22, 25)]

---

su(2) ← so(14673)
su(3)
su(14673)

[{⟨1, 1⟩},{⟨14672, 1⟩}], [{⟨1, 1⟩}], [(14672)], [(66, 5), (5, 66)]

---

su(2) ← sp(7337)
so(23) ← so(14674)
su(14674)

[{⟨1, 1⟩},{⟨14673, 1⟩}],[{⟨1, 1⟩}],[(14673)],[{⟨1, 1⟩}], [{⟨1, 4⟩}]

---

su(2) ← sp(7344)
so(16) ← so(14688)
su(14688)

[{⟨1, 1⟩},{⟨14687, 1⟩}],[{⟨1, 1⟩}],[(14687)],[{⟨1, 1⟩}], [{⟨1, 5⟩}]

---

su(2) ← sp(7350)
so(14700)
su(3)
su(7)
su(7)
su(7)
su(8)
su(14700)

[{⟨1, 1⟩},{⟨14699, 1⟩}],[{⟨1, 1⟩}],[(14699)],[{⟨1, 1⟩}], [(24, 23),(23, 24)], [{⟨1, 1⟩, ⟨2, 2⟩, ⟨5, 1⟩},{⟨2, 1⟩, ⟨5, 2⟩, ⟨6, 1⟩}], [{⟨1, 1⟩, ⟨2, 2⟩, ⟨3, 1⟩},{⟨4, 1⟩, ⟨5, 2⟩, ⟨6, 1⟩}],[{⟨1, 4⟩, ⟨2, 1⟩, ⟨6, 1⟩},{⟨1, 1⟩, ⟨5, 1⟩, ⟨6, 4⟩}], [{⟨1, 1⟩, ⟨3, 1⟩, ⟨4, 1⟩},{⟨4, 1⟩, ⟨5, 1⟩, ⟨7, 1⟩}]

---

su(2)
so(171) ← so(14705) ← su(14705)
sp(86)

[{⟨1, 1⟩},{⟨14704, 1⟩}],[{⟨1, 1⟩}],[(14704)],[{⟨1, 2⟩}], [{⟨2, 1⟩}]

---

su(2) ← sp(7353)
so(172) ← so(14706)
su(3)
su(171)
su(172)
su(14706)

[{⟨1, 1⟩},{⟨14705, 1⟩}],[{⟨1, 1⟩}],[(14705)],[{⟨1, 1⟩}], [{⟨2, 1⟩}], [(170, 0),(0, 170)], [{⟨1, 2⟩},{⟨170, 2⟩}], [{⟨2, 1⟩},{⟨170, 1⟩}]

---

su(2)
so(5)
so(14725)
su(3)
su(14725)

[{⟨1, 1⟩},{⟨14724, 1⟩}], [{⟨1, 1⟩}], [(14724)], [(5, 18)], [(30, 18),(18, 30)]

---

su(2) ← so(14739)
su(3)
su(14739)

[{⟨1, 1⟩},{⟨14738, 1⟩}], [{⟨1, 1⟩}], [(14738)], [(33, 16), (16, 33)]

---

su(2)
sp(2)
sp(7378)
so(5)
g2 ← so(7)
so(14756)
su(14756)

[{⟨1, 1⟩},{⟨14755, 1⟩}], [{⟨1, 1⟩}], [(14755)], [(27, 2)], [{⟨1, 1⟩}],[(6, 16)],[(13, 0, 0)],[(13, 0)]

---

su(2)
sp(2)
sp(7392)
so(10) ← so(14784)
su(3)
su(3)
su(8)
su(8)
su(14784)

[{⟨1, 1⟩},{⟨14783, 1⟩}], [{⟨1, 1⟩}], [(14783)], [(7, 13)], [{⟨1, 1⟩}],[(3, 0, 1, 0, 0)],[(43, 11),(11, 43)],[(83, 3),(3, 83)], [{⟨1, 2⟩, ⟨4, 1⟩, ⟨7, 1⟩},{⟨1, 1⟩, ⟨4, 1⟩, ⟨7, 2⟩}], [{⟨1, 3⟩, ⟨2, 2⟩},{⟨6, 2⟩, ⟨7, 3⟩}]

---

su(2) ← so(14787)
su(3)
su(14787)

[{⟨1, 1⟩},{⟨14786, 1⟩}], [{⟨1, 1⟩}], [(14786)], [(52, 8), (8, 52)]

---

su(2) ← sp(7410)
so(14820)
su(3)
su(4)
su(14820)

[{⟨1, 1⟩},{⟨14819, 1⟩}],[{⟨1, 1⟩}],[(14819)],[{⟨1, 1⟩}], [(56, 7),(7, 56)],[(12, 1, 3),(3, 1, 12)]

---

su(2) ← so(14847)
su(3)
su(14847)

[{⟨1, 1⟩},{⟨14846, 1⟩}], [{⟨1, 1⟩}], [(14846)], [(97, 2), (2, 97)]

---

su(2) ← sp(7425)
so(14850)
su(4)
su(14850)

[{⟨1, 1⟩},{⟨14849, 1⟩}],[{⟨1, 1⟩}],[(14849)],[{⟨1, 1⟩}], [(5, 4, 3),(3, 4, 5)]

su(2) ← so(14875) ← su(14875)
su(4) ← su(14875)

[{⟨1, 1⟩},{⟨14874, 1⟩}], [{⟨1, 1⟩}], [(14874)], [(9, 4, 1), (1, 4, 9)]

---

su(2), so(172) ← so(14877) ← su(14877)

[{⟨1, 1⟩},{⟨14876, 1⟩}],[{⟨1, 1⟩}],[(14876)],[{⟨1, 2⟩}]

---

su(2) ← sp(7439) ← su(14878)
so(173), sp(86) ← so(14878) ← su(14878)
su(3) ← su(14878)
su(172) ← su(14878)
su(173) ← su(14878)

[{⟨1, 1⟩},{⟨14877, 1⟩}],[{⟨1, 1⟩}],[(14877)],[{⟨1, 1⟩}], [{⟨2, 1⟩}], [{⟨1, 2⟩}], [(171, 0),(0, 171)], [{⟨1, 2⟩}, {⟨171, 2⟩}],[{⟨2, 1⟩},{⟨171, 1⟩}]

---

su(2), su(122) ← so(14883) ← su(14883)
su(3) ← su(14883)

[{⟨1, 1⟩},{⟨14882, 1⟩}], [{⟨1, 1⟩}], [(14882)], [{⟨1, 1⟩, ⟨121, 1⟩}],[(120, 1),(1, 120)]

---

su(2) ← sp(7452) ← su(14904)
so(14904) ← su(14904)
su(4) ← su(14904)

[{⟨1, 1⟩},{⟨14903, 1⟩}],[{⟨1, 1⟩}],[(14903)],[{⟨1, 1⟩}], [(22, 0, 2),(2, 0, 22)]

---

su(2) ← sp(7455) ← su(14910)
so(5) ← so(14910) ← su(14910)

[{⟨1, 1⟩},{⟨14909, 1⟩}],[{⟨1, 1⟩}],[(14909)],[{⟨1, 1⟩}], [(34, 0)]

---

su(2) ← sp(7475) ← su(14950)
so(26) ← so(14950) ← su(14950)
su(5) ← su(14950)
su(23) ← su(14950)
su(26) ← su(14950)

[{⟨1, 1⟩},{⟨14949, 1⟩}],[{⟨1, 1⟩}],[(14949)],[{⟨1, 1⟩}], [{⟨4, 1⟩}], [(22, 0, 0, 0),(0, 0, 0, 22)], [{⟨1, 4⟩}, {⟨22, 4⟩}],[{⟨4, 1⟩},{⟨22, 1⟩}]

---

su(2), sp(2) ← sp(7480) ← su(14960)
so(14960) ← su(14960)
su(4) ← su(14960)
su(4) ← su(14960)
su(4) ← su(14960)

[{⟨1, 1⟩},{⟨14959, 1⟩}], [{⟨1, 1⟩}], [(14959)], [(9, 11)], [{⟨1, 1⟩}],[(4, 10, 0),(0, 10, 4)],[(5, 9, 0),(0, 9, 5)],[(15, 0, 4),(4, 0, 15)]

---

su(2) ← so(14973) ← su(14973)
su(3) ← su(14973)

[{⟨1, 1⟩},{⟨14972, 1⟩}], [{⟨1, 1⟩}], [(14972)], [(61, 6), (6, 61)]

---

su(2) ← sp(7488) ← su(14976)
so(14976) ← su(14976)
su(3) ← su(14976)

[{⟨1, 1⟩},{⟨14975, 1⟩}],[{⟨1, 1⟩}],[(14975)],[{⟨1, 1⟩}], [(35, 15),(15, 35)]

---

su(2) ← so(14993) ← su(14993)
su(3) ← su(14993)

[{⟨1, 1⟩},{⟨14992, 1⟩}], [{⟨1, 1⟩}], [(14992)], [(46, 10), (10, 46)]

---

su(2) ← sp(7500) ← su(15000)
so(15000) ← su(15000)
su(3) ← su(15000)
su(3) ← su(15000)
su(3) ← su(15000)

[{⟨1, 1⟩},{⟨14999, 1⟩}],[{⟨1, 1⟩}],[(14999)],[{⟨1, 1⟩}], [(29, 19),(19, 29)],[(49, 9),(9, 49)],[(74, 4),(4, 74)]

---

su(2), so(5), sp(5), so(8) ← so(15015) ← su(15015)
su(3) ← su(15015)
su(4) ← su(15015)
su(5) ← su(15015)
su(5) ← su(15015)
su(5) ← su(15015)
su(6) ← su(15015)
su(6) ← su(15015)
su(10) ← su(15015)
su(11) ← su(15015)
su(13) ← su(15015)

[{⟨1, 1⟩},{⟨15014, 1⟩}], [{⟨1, 1⟩}], [(15014)], [(12, 8)], [(3, 0, 1, 0, 0)], [(6, 1, 0, 0),(0, 1, 6, 0),(0, 1, 0, 6)], [(41, 12),(12, 41)], [(10, 1, 4),(4, 1, 10)], [(5, 4, 0, 0),(0, 0, 4, 5)], [(6, 2, 0, 1),(1, 0, 2, 6)], [(8, 1, 1, 0),(0, 1, 1, 8)], [(6, 2, 0, 0, 0),(0, 0, 0, 2, 6)], [(8, 0, 0, 1, 0),(0, 1, 0, 0, 8)], [{⟨1, 4⟩, ⟨2, 1⟩},{⟨8, 1⟩, ⟨9, 4⟩}], [{⟨1, 3⟩, ⟨9, 1⟩}, {⟨2, 1⟩, ⟨10, 3⟩}],[{⟨1, 1⟩, ⟨5, 1⟩},{⟨8, 1⟩, ⟨12, 1⟩}]

---

su(2) ← sp(7525) ← su(15050)
so(173), sp(87) ← so(15050) ← su(15050)

[{⟨1, 1⟩},{⟨15049, 1⟩}],[{⟨1, 1⟩}],[(15049)],[{⟨1, 1⟩}], [{⟨1, 2⟩}],[{⟨2, 1⟩}]

---

su(2), so(174) ← so(15051) ← su(15051)
su(3) ← su(15051)
su(173) ← su(15051)
su(174) ← su(15051)

[{⟨1, 1⟩},{⟨15050, 1⟩}],[{⟨1, 1⟩}],[(15050)],[{⟨2, 1⟩}], [(172, 0),(0, 172)], [{⟨1, 2⟩},{⟨172, 2⟩}], [{⟨2, 1⟩}, {⟨172, 1⟩}]

---

su(2) ← sp(7546) ← su(15092)
sp(3), so(8) ← so(15092) ← su(15092)

[{⟨1, 1⟩},{⟨15091, 1⟩}],[{⟨1, 1⟩}],[(15091)],[{⟨1, 1⟩}], [(6, 0, 2)],[(2, 0, 2, 2)]

---

su(2) ← sp(7548) ← su(15096)
so(15096) ← su(15096)
su(3) ← su(15096)

[{⟨1, 1⟩},{⟨15095, 1⟩}],[{⟨1, 1⟩}],[(15095)],[{⟨1, 1⟩}], [(67, 5),(5, 67)]

---

su(2) ← so(15105) ← su(15105)
su(3) ← su(15105)

[{⟨1, 1⟩},{⟨15104, 1⟩}], [{⟨1, 1⟩}], [(15104)], [(37, 14), (14, 37)]

---

su(2) ← sp(7560) ← su(15120)
so(15120) ← su(15120)
su(3) ← su(15120)
su(4) ← su(15120)
su(4) ← su(15120)
su(5) ← su(15120)
su(6) ← su(15120)
su(7) ← su(15120)
su(8) ← su(15120)
su(8) ← su(15120)
so(10) ← su(15120)

[{⟨1, 1⟩},{⟨15119, 1⟩}],[{⟨1, 1⟩}],[(15119)],[{⟨1, 1⟩}], [(39, 13),(13, 39)], [(6, 2, 5),(5, 2, 6)], [(15, 1, 2),(2, 1, 15)], [(4, 2, 0, 2),(2, 0, 2, 4)], [(0, 4, 1, 0, 0),(0, 0, 1, 4, 0)], [{⟨1, 2⟩, ⟨3, 1⟩, ⟨4, 1⟩},{⟨3, 1⟩, ⟨4, 1⟩, ⟨6, 2⟩}], [{⟨2, 2⟩, ⟨4, 1⟩},{⟨4, 1⟩, ⟨6, 2⟩}], [{⟨1, 1⟩, ⟨3, 1⟩, ⟨5, 1⟩},{⟨3, 1⟩, ⟨5, 1⟩, ⟨7, 1⟩}], [(2, 1, 0, 1, 0),(2, 1, 0, 0, 1)]

---

su(2) ← sp(7564) ← su(15128)
su(123) ← so(15128) ← su(15128)
su(3) ← su(15128)

[{⟨1, 1⟩},{⟨15127, 1⟩}],[{⟨1, 1⟩}],[(15127)],[{⟨1, 1⟩}], [{⟨1, 1⟩, ⟨122, 1⟩}],[(121, 1),(1, 121)]

---

su(2) ← sp(7565) ← su(15130)
so(15130) ← su(15130)
su(3) ← su(15130)

[{⟨1, 1⟩},{⟨15129, 1⟩}],[{⟨1, 1⟩}],[(15129)],[{⟨1, 1⟩}], [(84, 3),(3, 84)]

---

su(2), sp(23) ← sp(7567) ← su(15134)
so(15134) ← su(15134)

[{⟨1, 1⟩},{⟨15133, 1⟩}],[{⟨1, 1⟩}],[(15133)],[{⟨3, 1⟩}], [{⟨1, 1⟩}]

---

su(2) ← sp(7568) ← su(15136)
so(44) ← so(15136) ← su(15136)

[{⟨1, 1⟩},{⟨15135, 1⟩}],[{⟨1, 1⟩}],[(15135)],[{⟨1, 1⟩}], [{⟨1, 3⟩}]

---

su(2) ← so(15147) ← su(15147)
su(3) ← su(15147)
su(3) ← su(15147)

[{⟨1, 1⟩},{⟨15146, 1⟩}], [{⟨1, 1⟩}], [(15146)], [(32, 17), (17, 32)],[(98, 2),(2, 98)]

---

su(2), sp(2), sp(22) ← sp(7590) ← su(15180)
so(46) ← so(15180) ← su(15180)
su(4) ← su(15180)
su(4) ← su(15180)
su(44) ← su(15180)
su(46) ← su(15180)

[{⟨1, 1⟩},{⟨15179, 1⟩}], [{⟨1, 1⟩}], [(15179)], [(43, 0)], [{⟨1, 3⟩}], [{⟨1, 1⟩}], [{⟨3, 1⟩}], [(17, 3, 0),(0, 3, 17)], [(43, 0, 0),(0, 0, 43)], [{⟨1, 3⟩},{⟨43, 3⟩}], [{⟨3, 1⟩}, {⟨43, 1⟩}]

---

su(2) ← sp(7600) ← su(15200)
so(15200) ← su(15200)
su(4) ← su(15200)

[{⟨1, 1⟩},{⟨15199, 1⟩}],[{⟨1, 1⟩}],[(15199)],[{⟨1, 1⟩}], [(18, 0, 3),(3, 0, 18)]

---

su(2) ← sp(7612) ← su(15224)
so(174) ← so(15224) ← su(15224)

[{⟨1, 1⟩},{⟨15223, 1⟩}],[{⟨1, 1⟩}],[(15223)],[{⟨1, 1⟩}], [{⟨1, 2⟩}]

su(2)
so(175) so(15225)
sp(87)
su(3)
su(3) su(15225)
su(174)
su(175)

[{⟨1, 1⟩},{⟨15224, 1⟩}],[{⟨1, 1⟩}],[(15224)],[{⟨2, 1⟩}],[{⟨1, 2⟩}], [(28, 20),(20, 28)], [(173, 0),(0, 173)], [{⟨1, 2⟩},{⟨173, 2⟩}],[{⟨2, 1⟩},{⟨173, 1⟩}]

---

su(2) sp(7644)
so(15288) su(15288)
su(7)

[{⟨1, 1⟩},{⟨15287, 1⟩}],[{⟨1, 1⟩}],[(15287)],[{⟨1, 1⟩}], [{⟨1, 4⟩, ⟨6, 3⟩},{⟨1, 3⟩, ⟨6, 4⟩}]

---

su(2) so(15309)
su(15309)
su(3)

[{⟨1, 1⟩},{⟨15308, 1⟩}], [{⟨1, 1⟩}], [(15308)], [(53, 8), (8, 53)]

---

su(2) sp(7656)
so(15312) su(15312)
su(3)

[{⟨1, 1⟩},{⟨15311, 1⟩}],[{⟨1, 1⟩}],[(15311)],[{⟨1, 1⟩}], [(57, 7),(7, 57)]

---

su(2) so(15345)
su(4) su(15345)
su(31)

[{⟨1, 1⟩},{⟨15344, 1⟩}],[{⟨1, 1⟩}],[(15344)],[(29, 0, 1), (1, 0, 29)],[{⟨1, 2⟩, ⟨30, 1⟩},{⟨1, 1⟩, ⟨30, 2⟩}]

---

su(2) sp(7680)
so(16) so(15360) su(15360)
su(5)

[{⟨1, 1⟩},{⟨15359, 1⟩}],[{⟨1, 1⟩}],[(15359)],[{⟨1, 1⟩}], [{⟨1, 2⟩, ⟨7, 1⟩},{⟨1, 2⟩, ⟨8, 1⟩}], [(5, 1, 1, 1),(1, 1, 1, 5)]

---

su(2)
so(15375)
su(124) su(15375)
su(3)

[{⟨1, 1⟩},{⟨15374, 1⟩}], [{⟨1, 1⟩}], [(15374)], [{⟨1, 1⟩, ⟨123, 1⟩}],[(122, 1),(1, 122)]

---

su(2) sp(7695)
so(15390)
su(3) su(15390)
su(3)

[{⟨1, 1⟩},{⟨15389, 1⟩}],[{⟨1, 1⟩}],[(15389)],[{⟨1, 1⟩}], [(44, 11),(11, 44)],[(75, 4),(4, 75)]

---

su(2)
so(175) so(15399) su(15399)
sp(88)

[{⟨1, 1⟩},{⟨15398, 1⟩}],[{⟨1, 1⟩}],[(15398)],[{⟨1, 2⟩}], [{⟨2, 1⟩}]

---

su(2) sp(7700)
so(11)
so(8) so(15400)
so(176)
su(3)
su(3)
su(5)
su(5) su(15400)
su(5)
su(8)
su(8)
su(175)
su(176)

[{⟨1, 1⟩},{⟨15399, 1⟩}],[{⟨1, 1⟩}],[(15399)],[{⟨1, 1⟩}], [(2, 0, 0, 1, 0)], [(4, 0, 3, 0),(4, 0, 0, 3),(3, 0, 4, 0),(3, 0, 0, 4),(0, 0, 4, 3),(0, 0, 3, 4)], [{⟨2, 1⟩}], [(27, 21),(21, 27)], [(174, 0),(0, 174)], [(2, 4, 1, 0),(0, 1, 4, 2)], [(3, 1, 3, 0),(0, 3, 1, 3)], [(10, 2, 0, 0),(0, 0, 2, 10)], [{⟨1, 2⟩, ⟨2, 1⟩, ⟨6, 1⟩},{⟨2, 1⟩, ⟨6, 1⟩, ⟨7, 2⟩}], [{⟨1, 4⟩, ⟨5, 1⟩},{⟨3, 1⟩, ⟨7, 4⟩}], [{⟨1, 2⟩},{⟨174, 2⟩}], [{⟨2, 1⟩},{⟨174, 1⟩}]

---

su(2) so(15435)
su(3) su(15435)
su(4)

[{⟨1, 1⟩},{⟨15434, 1⟩}], [{⟨1, 1⟩}], [(15434)], [(62, 6), (6, 62)],[(13, 0, 5),(5, 0, 13)]

---

su(2) sp(7722)
su(15444)
so(9)
so(15444)
so(9)

[{⟨1, 1⟩},{⟨15443, 1⟩}],[{⟨1, 1⟩}],[(15443)],[{⟨1, 1⟩}], [(0, 2, 1, 0)],[(1, 1, 0, 2)]

---

su(2) sp(7725)
so(15450) su(15450)
su(3)

[{⟨1, 1⟩},{⟨15449, 1⟩}],[{⟨1, 1⟩}],[(15449)],[{⟨1, 1⟩}], [(99, 2),(2, 99)]

---

su(2)
sp(7728)
sp(2) su(15456)
so(15456)

[{⟨1, 1⟩},{⟨15455, 1⟩}], [{⟨1, 1⟩}], [(15455)], [(13, 8)], [{⟨1, 1⟩}]

---

su(2) sp(7735)
so(15470)
su(3) su(15470)
su(4)
su(5)

[{⟨1, 1⟩},{⟨15469, 1⟩}],[{⟨1, 1⟩}],[(15469)],[{⟨1, 1⟩}], [(34, 16),(16, 34)], [(9, 2, 3),(3, 2, 9)], [(11, 0, 0, 2),(2, 0, 0, 11)]

---

su(2) sp(7740)
so(15480) su(15480)
su(3)

[{⟨1, 1⟩},{⟨15479, 1⟩}],[{⟨1, 1⟩}],[(15479)],[{⟨1, 1⟩}], [(85, 3),(3, 85)]

---

su(2)
sp(2)
sp(3) sp(7752)
sp(8)
sp(18)
sp(9)
so(20) so(15504) su(15504)
so(36) su(3)
su(4)
su(6)
su(16)
su(20)

[{⟨1, 1⟩},{⟨15503, 1⟩}], [{⟨1, 1⟩}], [(15503)], [(33, 1)], [(15, 0, 0)], [{⟨1, 5⟩}], [{⟨1, 1⟩, ⟨2, 1⟩}], [{⟨1, 1⟩}], [{⟨6, 1⟩}], [{⟨5, 1⟩}], [{⟨1, 1⟩, ⟨2, 1⟩}], [(31, 18),(18, 31)], [(1, 15, 0),(0, 15, 1)], [(15, 0, 0, 0, 0),(0, 0, 0, 0, 15)],[{⟨1, 5⟩},{⟨15, 5⟩}],[{⟨5, 1⟩},{⟨15, 1⟩}]

---

su(2) so(15525)
su(3) su(15525)
su(3)

[{⟨1, 1⟩},{⟨15524, 1⟩}], [{⟨1, 1⟩}], [(15524)], [(26, 22), (22, 26)],[(68, 5),(5, 68)]

---

su(2) sp(7770)
so(15540) su(15540)
su(36)

[{⟨1, 1⟩},{⟨15539, 1⟩}],[{⟨1, 1⟩}],[(15539)],[{⟨1, 1⟩}], [{⟨1, 1⟩, ⟨2, 1⟩},{⟨34, 1⟩, ⟨35, 1⟩}]

---

su(2) so(15555)
su(15555)
su(3)

[{⟨1, 1⟩},{⟨15554, 1⟩}], [{⟨1, 1⟩}], [(15554)], [(50, 9), (9, 50)]

---

su(2)
so(15561) su(15561)
so(7)

[{⟨1, 1⟩},{⟨15560, 1⟩}],[{⟨1, 1⟩}],[(15560)],[(5, 2, 0)]

---

su(2)
so(15575) su(15575)
so(176)

[{⟨1, 1⟩},{⟨15574, 1⟩}],[{⟨1, 1⟩}],[(15574)],[{⟨1, 2⟩}]

---

su(2) sp(7788)
so(177)
so(15576)
sp(88)
su(3)
su(3) su(15576)
su(176)
su(177)

[{⟨1, 1⟩},{⟨15575, 1⟩}],[{⟨1, 1⟩}],[(15575)],[{⟨1, 1⟩}], [{⟨2, 1⟩}], [{⟨1, 2⟩}], [(47, 10),(10, 47)], [(175, 0),(0, 175)],[{⟨1, 2⟩},{⟨175, 2⟩}],[{⟨2, 1⟩},{⟨175, 1⟩}]

---

su(2) sp(7800)
so(15600) su(15600)
su(3)

[{⟨1, 1⟩},{⟨15599, 1⟩}],[{⟨1, 1⟩}],[(15599)],[{⟨1, 1⟩}], [(25, 23),(23, 25)]

---

su(2) sp(7812)
su(125) so(15624) su(15624)
su(3)

[{⟨1, 1⟩},{⟨15623, 1⟩}],[{⟨1, 1⟩}],[(15623)],[{⟨1, 1⟩}], [{⟨1, 1⟩, ⟨124, 1⟩}],[(123, 1),(1, 123)]

---

su(2)
su(3)
so(15625) su(15625)
so(6)
$\mathfrak{g}_2$

[{⟨1, 1⟩},{⟨15624, 1⟩}],[{⟨1, 1⟩}],[(15624)],[(24, 24)],[(4, 4, 4)],[(4, 4)]

---

su(2)
sp(2) ⟶ sp(7820)
so(15640) ⟶ su(15640)

[{⟨1, 1⟩},{⟨15639, 1⟩}], [{⟨1, 1⟩}], [(15639)], [(5, 16)], [{⟨1, 1⟩}]

---

su(2) ⟵ sp(7826)
so(15652) ⟵ su(15652)
su(3)

[{⟨1, 1⟩},{⟨15651, 1⟩}],[{⟨1, 1⟩}],[(15651)],[{⟨1, 1⟩}],[(42, 12),(12, 42)]

---

su(2) ⟵ sp(7840)
so(15680) ⟵ su(15680)
su(7)

[{⟨1, 1⟩},{⟨15679, 1⟩}],[{⟨1, 1⟩}],[(15679)],[{⟨1, 1⟩}],[{⟨1, 1⟩, ⟨3, 2⟩, ⟨6, 1⟩},{⟨1, 1⟩, ⟨4, 2⟩, ⟨6, 1⟩}]

---

su(2) ⟵ sp(7844)
so(15688) ⟵ su(15688)
su(3)

[{⟨1, 1⟩},{⟨15687, 1⟩}],[{⟨1, 1⟩}],[(15687)],[{⟨1, 1⟩}],[(36, 15),(15, 36)]

---

su(2)
sp(3) ⟶ sp(7854)
so(15708) ⟶ su(15708)

[{⟨1, 1⟩},{⟨15707, 1⟩}],[{⟨1, 1⟩}],[(15707)],[(0, 5, 1)],[{⟨1, 1⟩}]

---

su(2) ⟵ sp(7865)
so(15730)
su(5)
su(11) ⟵ su(15730)
su(11)
su(12)

[{⟨1, 1⟩},{⟨15729, 1⟩}],[{⟨1, 1⟩}],[(15729)],[{⟨1, 1⟩}],[(0, 9, 0, 0),(0, 0, 9, 0)], [{⟨2, 3⟩},{⟨9, 3⟩}], [{⟨1, 1⟩, ⟨3, 1⟩, ⟨10, 1⟩},{⟨1, 1⟩, ⟨8, 1⟩, ⟨10, 1⟩}], [{⟨3, 2⟩},{⟨9, 2⟩}]

---

su(2)
sp(3) ⟶ sp(7875)
so(15750)
su(4)
su(4) ⟵ su(15750)
su(5)
su(5)
su(6)

[{⟨1, 1⟩},{⟨15749, 1⟩}],[{⟨1, 1⟩}],[(15749)],[(4, 0, 3)],[{⟨1, 1⟩}], [(4, 6, 2),(2, 6, 4)], [(14, 4, 0),(0, 4, 14)], [(4, 3, 0, 1),(1, 0, 3, 4)], [(7, 0, 0, 4),(4, 0, 0, 7)], [(2, 1, 2, 0, 0),(0, 0, 2, 1, 2)]

---

su(2) ⟵ sp(7876)
so(177)
sp(89) ⟶ so(15752) ⟶ su(15752)

[{⟨1, 1⟩},{⟨15751, 1⟩}],[{⟨1, 1⟩}],[(15751)],[{⟨1, 1⟩}],[{⟨1, 2⟩}],[{⟨2, 1⟩}]

---

su(2)
so(178) ⟶ so(15753)
su(3) ⟵ su(15753)
su(177)
su(178)

[{⟨1, 1⟩},{⟨15752, 1⟩}],[{⟨1, 1⟩}],[(15752)],[{⟨2, 1⟩}],[(176, 0),(0, 176)], [{⟨1, 2⟩},{⟨176, 2⟩}], [{⟨2, 1⟩},{⟨176, 1⟩}]

---

su(2) ⟵ sp(7878)
so(15756) ⟵ su(15756)
su(3)

[{⟨1, 1⟩},{⟨15755, 1⟩}],[{⟨1, 1⟩}],[(15755)],[{⟨1, 1⟩}],[(100, 2),(2, 100)]

---

su(2) ⟵ so(15785)
su(3) ⟵ su(15785)
su(3)

[{⟨1, 1⟩},{⟨15784, 1⟩}], [{⟨1, 1⟩}], [(15784)], [(40, 13),(13, 40)],[(76, 4),(4, 76)]

---

su(2) ⟵ so(15795)
su(3) ⟵ su(15795)

[{⟨1, 1⟩},{⟨15794, 1⟩}], [{⟨1, 1⟩}], [(15794)], [(38, 14),(14, 38)]

---

su(2) ⟵ sp(7905)
so(15810) ⟵ su(15810)
su(3)

[{⟨1, 1⟩},{⟨15809, 1⟩}],[{⟨1, 1⟩}],[(15809)],[{⟨1, 1⟩}],[(30, 19),(19, 30)]

---

su(2) ⟵ sp(7906)
so(15812) ⟵ su(15812)
su(3)

[{⟨1, 1⟩},{⟨15811, 1⟩}],[{⟨1, 1⟩}],[(15811)],[{⟨1, 1⟩}],[(58, 7),(7, 58)]

---

su(2) ⟵ sp(7917)
so(15834) ⟵ su(15834)
su(3)

[{⟨1, 1⟩},{⟨15833, 1⟩}],[{⟨1, 1⟩}],[(15833)],[{⟨1, 1⟩}],[(86, 3),(3, 86)]

---

su(2)
sp(2) ⟶ sp(7920)
so(15840)
su(3)
su(4)
su(4)
su(4) ⟵ su(15840)
su(5)
su(5)
su(9)
su(9)
su(32)

[{⟨1, 1⟩},{⟨15839, 1⟩}], [{⟨1, 1⟩}], [(15839)], [(21, 4)], [{⟨1, 1⟩}], [(54, 8),(8, 54)], [(3, 7, 2),(2, 7, 3)], [(10, 0, 7),(7, 0, 10)], [(29, 1, 0),(0, 1, 29)], [(1, 5, 1, 0),(0, 1, 5, 1)], [(5, 1, 2, 0),(0, 2, 1, 5)], [{⟨1, 1⟩, ⟨6, 1⟩, ⟨7, 1⟩},{⟨2, 1⟩, ⟨3, 1⟩, ⟨8, 1⟩}], [{⟨1, 3⟩, ⟨4, 1⟩},{⟨5, 1⟩, ⟨8, 3⟩}],[{⟨1, 1⟩, ⟨30, 1⟩},{⟨2, 1⟩, ⟨31, 1⟩}]

---

su(2)
su(126) ⟶ so(15875) ⟵ su(15875)
su(3)

[{⟨1, 1⟩},{⟨15874, 1⟩}], [{⟨1, 1⟩}], [(15874)], [{⟨1, 1⟩, ⟨125, 1⟩}],[(124, 1),(1, 124)]

---

su(2) ⟵ sp(7938)
so(15876) ⟵ su(15876)
su(8)

[{⟨1, 1⟩},{⟨15875, 1⟩}],[{⟨1, 1⟩}],[(15875)],[{⟨1, 1⟩}],[{⟨2, 1⟩, ⟨3, 2⟩},{⟨5, 2⟩, ⟨6, 1⟩}]

---

su(2) ⟵ sp(7952)
so(15904) ⟵ su(15904)
su(3)

[{⟨1, 1⟩},{⟨15903, 1⟩}],[{⟨1, 1⟩}],[(15903)],[{⟨1, 1⟩}],[(63, 6),(6, 63)]

---

su(2) ⟵ sp(7956)
so(7) ⟵ so(15912) ⟵ su(15912)
su(3)

[{⟨1, 1⟩},{⟨15911, 1⟩}],[{⟨1, 1⟩}],[(15911)],[{⟨1, 1⟩}],[(3, 3, 0)],[(33, 17),(17, 33)]

---

su(2) ⟵ sp(7965)
so(178) ⟵ so(15930) ⟶ su(15930)

[{⟨1, 1⟩},{⟨15929, 1⟩}],[{⟨1, 1⟩}],[(15929)],[{⟨1, 1⟩}],[{⟨1, 2⟩}]

---

su(2)
so(179) ⟶ so(15931)
sp(89)
su(3)
su(178) ⟵ su(15931)
su(179)

[{⟨1, 1⟩},{⟨15930, 1⟩}],[{⟨1, 1⟩}],[(15930)],[{⟨2, 1⟩}],[{⟨1, 2⟩}], [(177, 0),(0, 177)], [{⟨1, 2⟩},{⟨177, 2⟩}],[{⟨2, 1⟩},{⟨177, 1⟩}]

---

su(2)
so(7) ⟶ so(15939) ⟵ su(15939)
so(21)

[{⟨1, 1⟩},{⟨15938, 1⟩}],[{⟨1, 1⟩}],[(15938)],[(8, 1, 0)],[{⟨2, 2⟩}]

---

su(2) ⟵ sp(7975)
so(5) ⟵ so(15950) ⟶ su(15950)

[{⟨1, 1⟩},{⟨15949, 1⟩}],[{⟨1, 1⟩}],[(15949)],[{⟨1, 1⟩}],[(3, 24)]

---

su(2) ⟵ sp(7980)
so(15960)
su(3) ⟵ su(15960)
su(4)

[{⟨1, 1⟩},{⟨15959, 1⟩}],[{⟨1, 1⟩}],[(15959)],[{⟨1, 1⟩}],[(69, 5),(5, 69)],[(15, 2, 1),(1, 2, 15)]

---

su(2) ⟵ sp(8004)
so(16008) ⟵ su(16008)
su(3)

[{⟨1, 1⟩},{⟨16007, 1⟩}],[{⟨1, 1⟩}],[(16007)],[{⟨1, 1⟩}],[(45, 11),(11, 45)]

---

su(2) ⟵ sp(8008)
so(7)
so(7) ⟶ so(16016)
su(4)
su(6) ⟵ su(16016)
su(7)
su(12)
su(13)

[{⟨1, 1⟩},{⟨16015, 1⟩}],[{⟨1, 1⟩}],[(16015)],[{⟨1, 1⟩}],[(0, 1, 7)], [(9, 0, 1)], [(2, 10, 1),(1, 10, 2)], [(10, 0, 0, 1),(1, 0, 0, 0, 10)], [{⟨1, 7⟩, ⟨2, 1⟩},{⟨5, 1⟩, ⟨6, 7⟩}], [{⟨1, 4⟩, ⟨11, 1⟩},{⟨1, 1⟩, ⟨11, 4⟩}], [{⟨1, 1⟩, ⟨8, 1⟩},{⟨5, 1⟩, ⟨12, 1⟩}]

---

su(2) ⟵ so(16065)
su(3)
su(3) ⟵ su(16065)
su(4)
su(5)
su(16)

[{⟨1, 1⟩},{⟨16064, 1⟩}], [{⟨1, 1⟩}], [(16064)], [(29, 20),(20, 29)], [(101, 2),(2, 101)], [(2, 13, 0),(0, 13, 2)], [(13, 0, 1, 0),(0, 1, 0, 13)],[{⟨1, 2⟩, ⟨14, 1⟩},{⟨2, 1⟩, ⟨15, 2⟩}]

su(2), sp(2) ← sp(8050); sp(8050), so(16100), su(4) ← su(16100)

[{⟨1, 1⟩},{⟨16099, 1⟩}], [{⟨1, 1⟩}], [(16099)], [(3, 20)], [{⟨1, 1⟩}],[(20, 1, 1),(1, 1, 20)]

---

su(2), so(179), sp(90) ← so(16109) ← su(16109)

[{⟨1, 1⟩},{⟨16108, 1⟩}],[{⟨1, 1⟩}],[(16108)],[{⟨1, 2⟩}], [{⟨2, 1⟩}]

---

su(2) ← sp(8055); so(180) ← so(16110); sp(8055), so(16110), su(3), su(179), su(180) ← su(16110)

[{⟨1, 1⟩},{⟨16109, 1⟩}],[{⟨1, 1⟩}],[(16109)],[{⟨1, 1⟩}], [{⟨2, 1⟩}], [(178, 0),(0, 178)], [{⟨1, 2⟩},{⟨178, 2⟩}], [{⟨2, 1⟩},{⟨178, 1⟩}]

---

su(2) ← sp(8060); sp(8060), so(16120), su(3) ← su(16120)

[{⟨1, 1⟩},{⟨16119, 1⟩}],[{⟨1, 1⟩}],[(16119)],[{⟨1, 1⟩}], [(51, 9),(9, 51)]

---

su(2) ← sp(8064); su(127), so(7) ← so(16128); sp(8064), so(16128), su(3), su(6), su(8) ← su(16128)

[{⟨1, 1⟩},{⟨16127, 1⟩}],[{⟨1, 1⟩}],[(16127)],[{⟨1, 1⟩}], [{⟨1, 1⟩, ⟨126, 1⟩}], [(3, 2, 1)], [(125, 1),(1, 125)], [(1, 3, 1, 0, 0),(0, 0, 1, 3, 1)], [{⟨1, 1⟩, ⟨4, 1⟩, ⟨5, 1⟩},{⟨3, 1⟩, ⟨4, 1⟩, ⟨7, 1⟩}]

---

su(2) ← sp(8073); sp(8073), so(16146), su(4) ← su(16146)

[{⟨1, 1⟩},{⟨16145, 1⟩}],[{⟨1, 1⟩}],[(16145)],[{⟨1, 1⟩}], [(22, 2, 0),(0, 2, 22)]

---

su(2) ← sp(8085); so(45), so(6) ← so(16170); sp(8085), so(16170), su(3), su(5), su(5), su(21) ← su(16170)

[{⟨1, 1⟩},{⟨16169, 1⟩}],[{⟨1, 1⟩}],[(16169)],[{⟨1, 1⟩}], [{⟨1, 3⟩}],[(19, 0, 0)],[(48, 10),(10, 48)],[(3, 2, 1, 1),(1, 1, 2, 3)],[(3, 2, 2, 0),(0, 2, 2, 3)],[{⟨2, 2⟩},{⟨19, 2⟩}]

---

su(2) ← so(16185); so(16185), su(3) ← su(16185)

[{⟨1, 1⟩},{⟨16184, 1⟩}], [{⟨1, 1⟩}], [(16184)], [(77, 4), (4, 77)]

---

su(2) ← sp(8096); sp(8096), so(16192), su(3) ← su(16192)

[{⟨1, 1⟩},{⟨16191, 1⟩}],[{⟨1, 1⟩}],[(16191)],[{⟨1, 1⟩}], [(87, 3),(3, 87)]

---

su(2) ← sp(8103); so(5) ← so(16206); sp(8103), so(16206) ← su(16206)

[{⟨1, 1⟩},{⟨16205, 1⟩}],[{⟨1, 1⟩}],[(16205)],[{⟨1, 1⟩}], [(35, 0)]

---

su(2), so(5), so(47) ← so(16215); so(16215), su(4), su(45), su(47) ← su(16215)

[{⟨1, 1⟩},{⟨16214, 1⟩}], [{⟨1, 1⟩}], [(16214)], [(0, 44)], [{⟨3, 1⟩}], [(44, 0, 0),(0, 0, 44)], [{⟨1, 3⟩},{⟨44, 3⟩}], [{⟨3, 1⟩},{⟨44, 1⟩}]

---

su(2) ← sp(8109); sp(8109), so(16218), su(3) ← su(16218)

[{⟨1, 1⟩},{⟨16217, 1⟩}],[{⟨1, 1⟩}],[(16217)],[{⟨1, 1⟩}], [(35, 16),(16, 35)]

---

su(2), sp(2) ← sp(8120); so(5) ← so(16240); sp(8120), so(16240) ← su(16240)

[{⟨1, 1⟩},{⟨16239, 1⟩}], [{⟨1, 1⟩}], [(16239)], [(1, 27)], [{⟨1, 1⟩}],[(2, 28)]

---

su(2) ← so(16269); so(16269), su(3) ← su(16269)

[{⟨1, 1⟩},{⟨16268, 1⟩}], [{⟨1, 1⟩}], [(16268)], [(28, 21), (21, 28)]

---

su(2), so(180) ← so(16289) ← su(16289)

[{⟨1, 1⟩},{⟨16288, 1⟩}],[{⟨1, 1⟩}],[(16288)],[{⟨1, 2⟩}]

---

su(2) ← sp(8145); so(181), sp(90) ← so(16290); sp(8145), so(16290), su(3), su(180), su(181) ← su(16290)

[{⟨1, 1⟩},{⟨16289, 1⟩}],[{⟨1, 1⟩}],[(16289)],[{⟨1, 1⟩}], [{⟨2, 1⟩}], [{⟨1, 2⟩}], [(179, 0),(0, 179)], [{⟨1, 2⟩}, {⟨179, 2⟩}],[{⟨2, 1⟩},{⟨179, 1⟩}]

---

su(2) ← sp(8151); so(9), so(13), $\mathfrak{f}_4$ ← so(16302); sp(8151), so(16302), su(3), su(3) ← su(16302)

[{⟨1, 1⟩},{⟨16301, 1⟩}],[{⟨1, 1⟩}],[(16301)],[{⟨1, 1⟩}], [(5, 1, 0, 0)], [{⟨1, 3⟩, ⟨2, 1⟩}], [(0, 0, 0, 4)], [(32, 18), (18, 32)],[(43, 12),(12, 43)]

---

su(2) ← sp(8160); sp(8160), so(16320), su(3), su(5), su(17) ← su(16320)

[{⟨1, 1⟩},{⟨16319, 1⟩}],[{⟨1, 1⟩}],[(16319)],[{⟨1, 1⟩}], [(59, 7),(7, 59)], [(15, 0, 0, 1),(1, 0, 0, 15)], [{⟨1, 3⟩, ⟨16, 1⟩},{⟨1, 1⟩, ⟨16, 3⟩}]

---

su(2) ← so(16335); so(16335), su(11) ← su(16335)

[{⟨1, 1⟩},{⟨16334, 1⟩}], [{⟨1, 1⟩}], [(16334)], [{⟨2, 1⟩, ⟨7, 1⟩},{⟨4, 1⟩, ⟨9, 1⟩}]

---

su(2) ← sp(8170); so(5) ← so(16340); sp(8170), so(16340) ← su(16340)

[{⟨1, 1⟩},{⟨16339, 1⟩}],[{⟨1, 1⟩}],[(16339)],[{⟨1, 1⟩}], [(18, 4)]

---

su(2) ← so(16377); so(16377), su(3) ← su(16377)

[{⟨1, 1⟩},{⟨16376, 1⟩}], [{⟨1, 1⟩}], [(16376)], [(102, 2), (2, 102)]

---

su(2) ← sp(8190); so(10) ← so(16380); sp(8190), so(16380), su(3), su(3), su(5), su(6), su(7), su(9), su(12) ← su(16380)

[{⟨1, 1⟩},{⟨16379, 1⟩}],[{⟨1, 1⟩}],[(16379)],[{⟨1, 1⟩}], [(2, 2, 0, 0, 0)], [(55, 8),(8, 55)], [(64, 6),(6, 64)], [(5, 1, 0, 3),(3, 0, 1, 5)], [(8, 0, 1, 0, 0),(0, 0, 1, 0, 8)], [{⟨1, 6⟩, ⟨5, 1⟩},{⟨2, 1⟩, ⟨6, 6⟩}], [{⟨1, 4⟩, ⟨7, 1⟩},{⟨2, 1⟩, ⟨8, 4⟩}],[{⟨1, 2⟩, ⟨9, 1⟩},{⟨3, 1⟩, ⟨11, 2⟩}]

---

su(2), su(128) ← so(16383); so(16383), su(3) ← su(16383)

[{⟨1, 1⟩},{⟨16382, 1⟩}], [{⟨1, 1⟩}], [(16382)], [{⟨1, 1⟩, ⟨127, 1⟩}],[(126, 1),(1, 126)]

---

su(2), so(29), sp(2) ← sp(8192); sp(8192), so(16384), su(4), so(30) ← su(16384)

[{⟨1, 1⟩},{⟨16383, 1⟩}], [{⟨1, 1⟩}], [(16383)], [{⟨14, 1⟩}], [(15, 7)], [{⟨1, 1⟩}], [(7, 3, 3),(3, 3, 7)], [{⟨14, 1⟩},{⟨15, 1⟩}]

---

su(2) ← so(16401); so(16401), su(3) ← su(16401)

[{⟨1, 1⟩},{⟨16400, 1⟩}], [{⟨1, 1⟩}], [(16400)], [(70, 5), (5, 70)]

---

su(2) ← sp(8208); sp(8208), so(16416), su(3) ← su(16416)

[{⟨1, 1⟩},{⟨16415, 1⟩}],[{⟨1, 1⟩}],[(16415)],[{⟨1, 1⟩}], [(37, 15),(15, 37)]

---

su(2) ← sp(8211); sp(8211), so(16422), su(3) ← su(16422)

[{⟨1, 1⟩},{⟨16421, 1⟩}],[{⟨1, 1⟩}],[(16421)],[{⟨1, 1⟩}], [(27, 22),(22, 27)]

---

su(2), so(5), so(11) ← so(16445) ← su(16445)

[{⟨1, 1⟩},{⟨16444, 1⟩}], [{⟨1, 1⟩}], [(16444)], [(9, 12)], [(7, 0, 0, 0, 0)]

---

su(2) ← sp(8232); sp(8232), so(16464), su(3), su(4) ← su(16464)

[{⟨1, 1⟩},{⟨16463, 1⟩}],[{⟨1, 1⟩}],[(16463)],[{⟨1, 1⟩}], [(41, 13),(13, 41)],[(6, 6, 1),(1, 6, 6)]

---

su(2) ← sp(8235); so(181), sp(91) ← so(16470); sp(8235), so(16470) ← su(16470)

[{⟨1, 1⟩},{⟨16469, 1⟩}],[{⟨1, 1⟩}],[(16469)],[{⟨1, 1⟩}], [{⟨1, 2⟩}],[{⟨2, 1⟩}]

su(2), so(182) → so(16471); su(3), su(181), su(182) → su(16471)

[{⟨1, 1⟩},{⟨16470, 1⟩}],[{⟨1, 1⟩}],[(16470)],[{⟨2, 1⟩}],[(180, 0),(0, 180)], [{⟨1, 2⟩},{⟨180, 2⟩}], [{⟨2, 1⟩},{⟨180, 1⟩}]

---

su(2) ← sp(8250); so(16500); su(3); su(4); su(4); su(6) → su(16500)

[{⟨1, 1⟩},{⟨16499, 1⟩}],[{⟨1, 1⟩}],[(16499)],[{⟨1, 1⟩}],[(39, 14),(14, 39)], [(4, 5, 3),(3, 5, 4)], [(9, 0, 8),(8, 0, 9)],[(4, 0, 1, 1, 0),(0, 1, 1, 0, 4)]

---

su(2) ← sp(8262); so(5) ← so(16524); su(3); su(4) → su(16524)

[{⟨1, 1⟩},{⟨16523, 1⟩}],[{⟨1, 1⟩}],[(16523)],[{⟨1, 1⟩}],[(23, 2)],[(26, 23),(23, 26)],[(8, 7, 0),(0, 7, 8)]

---

su(2) ← sp(8277); so(16554); su(3) → su(16554)

[{⟨1, 1⟩},{⟨16553, 1⟩}],[{⟨1, 1⟩}],[(16553)],[{⟨1, 1⟩}],[(88, 3),(3, 88)]

---

su(2), so(13), so(6) → so(16575); su(3); su(15) → su(16575)

[{⟨1, 1⟩},{⟨16574, 1⟩}], [{⟨1, 1⟩}], [(16574)], [{⟨1, 1⟩, ⟨2, 2⟩}], [(12, 1, 1)], [(25, 24),(24, 25)], [{⟨1, 1⟩, ⟨2, 1⟩, ⟨14, 1⟩},{⟨1, 1⟩, ⟨13, 1⟩, ⟨14, 1⟩}]

---

su(2) ← sp(8295); so(16590); su(3) → su(16590)

[{⟨1, 1⟩},{⟨16589, 1⟩}],[{⟨1, 1⟩}],[(16589)],[{⟨1, 1⟩}],[(78, 4),(4, 78)]

---

su(2), sp(3) → sp(8316); so(7), so(7) → so(16632); su(6); su(7); su(9) → su(16632)

[{⟨1, 1⟩},{⟨16631, 1⟩}],[{⟨1, 1⟩}],[(16631)],[(2, 3, 1)],[{⟨1, 1⟩}],[(2, 0, 6)],[(5, 0, 3)],[(1, 5, 0, 0, 0),(0, 0, 0, 5, 1)], [{⟨1, 2⟩, ⟨2, 2⟩, ⟨6, 1⟩},{⟨1, 1⟩, ⟨5, 2⟩, ⟨6, 2⟩}], [{⟨1, 1⟩, ⟨3, 2⟩},{⟨6, 2⟩, ⟨8, 1⟩}]

---

su(2) ← sp(8319); so(16638); su(3) → su(16638)

[{⟨1, 1⟩},{⟨16637, 1⟩}],[{⟨1, 1⟩}],[(16637)],[{⟨1, 1⟩}],[(46, 11),(11, 46)]

---

su(2), sp(2) → sp(8320); su(129) ← so(16640); su(3); su(3); su(4) → su(16640)

[{⟨1, 1⟩},{⟨16639, 1⟩}], [{⟨1, 1⟩}], [(16639)], [(19, 5)], [{⟨1, 1⟩}],[{⟨1, 1⟩, ⟨128, 1⟩}],[(31, 19),(19, 31)],[(127, 1),(1, 127)],[(7, 4, 2),(2, 4, 7)]

---

su(2) ← sp(8326); so(182) ← so(16652) → su(16652)

[{⟨1, 1⟩},{⟨16651, 1⟩}],[{⟨1, 1⟩}],[(16651)],[{⟨1, 1⟩}],[{⟨1, 2⟩}]

---

su(2), so(183), sp(91) → so(16653); su(3); su(182); su(183) → su(16653)

[{⟨1, 1⟩},{⟨16652, 1⟩}],[{⟨1, 1⟩}],[(16652)],[{⟨2, 1⟩}],[{⟨1, 2⟩}], [(181, 0),(0, 181)], [{⟨1, 2⟩},{⟨181, 2⟩}],[{⟨2, 1⟩},{⟨181, 1⟩}]

---

su(2) ← sp(8330); so(16660); su(4) → su(16660)

[{⟨1, 1⟩},{⟨16659, 1⟩}],[{⟨1, 1⟩}],[(16659)],[{⟨1, 1⟩}],[(9, 3, 2),(2, 3, 9)]

---

su(2) ← sp(8346); so(16692); su(3) → su(16692)

[{⟨1, 1⟩},{⟨16691, 1⟩}],[{⟨1, 1⟩}],[(16691)],[{⟨1, 1⟩}],[(103, 2),(2, 103)]

---

su(2) ← so(16695); su(3); su(3) → su(16695)

[{⟨1, 1⟩},{⟨16694, 1⟩}], [{⟨1, 1⟩}], [(16694)], [(34, 17),(17, 34)],[(52, 9),(9, 52)]

---

su(2) ← sp(8372); so(5), so(13) → so(16744) → su(16744)

[{⟨1, 1⟩},{⟨16743, 1⟩}],[{⟨1, 1⟩}],[(16743)],[{⟨1, 1⟩}],[(15, 6)],[{⟨1, 6⟩}]

---

su(2) ← so(16775); su(3) → su(16775)

[{⟨1, 1⟩},{⟨16774, 1⟩}], [{⟨1, 1⟩}], [(16774)], [(49, 10),(10, 49)]

---

su(2), sp(9) → sp(8398); so(16796); su(4) → su(16796)

[{⟨1, 1⟩},{⟨16795, 1⟩}],[{⟨1, 1⟩}],[(16795)],[{⟨9, 1⟩}],[{⟨1, 1⟩}],[(12, 3, 1),(1, 3, 12)]

---

su(2), sp(2) → sp(8400); so(8) ← so(16800); su(4); su(7); su(7) → su(16800)

[{⟨1, 1⟩},{⟨16799, 1⟩}], [{⟨1, 1⟩}], [(16799)], [(17, 6)], [{⟨1, 1⟩}],[(4, 1, 1, 0),(4, 1, 0, 1),(1, 1, 4, 0),(1, 1, 0, 4),(0, 1, 4, 1),(0, 1, 1, 4)], [(23, 0, 2),(2, 0, 23)], [{⟨1, 1⟩, ⟨2, 1⟩, ⟨5, 2⟩},{⟨2, 2⟩, ⟨5, 1⟩, ⟨6, 1⟩}], [{⟨1, 1⟩, ⟨2, 1⟩, ⟨4, 1⟩, ⟨6, 1⟩},{⟨1, 1⟩, ⟨3, 1⟩, ⟨5, 1⟩, ⟨6, 1⟩}]

---

su(2), so(5), so(37), so(183), sp(92) → so(16835) ← su(16835)

[{⟨1, 1⟩},{⟨16834, 1⟩}], [{⟨1, 1⟩}], [(16834)], [(1, 34)], [{⟨1, 1⟩, ⟨2, 1⟩}],[{⟨1, 2⟩}],[{⟨2, 1⟩}]

---

su(2) ← sp(8418); so(184) ← so(16836); su(3); su(3); su(183); su(184) → su(16836)

[{⟨1, 1⟩},{⟨16835, 1⟩}],[{⟨1, 1⟩}],[(16835)],[{⟨1, 1⟩}],[{⟨2, 1⟩}],[(60, 7),(7, 60)],[(182, 0),(0, 182)],[{⟨1, 2⟩},{⟨182, 2⟩}],[{⟨2, 1⟩},{⟨182, 1⟩}]

---

su(2) ← sp(8424); sp(4) ← so(16848); su(3) → su(16848)

[{⟨1, 1⟩},{⟨16847, 1⟩}],[{⟨1, 1⟩}],[(16847)],[{⟨1, 1⟩}],[(2, 0, 2, 0)],[(71, 5),(5, 71)]

---

su(2) ← so(16863); su(3) → su(16863)

[{⟨1, 1⟩},{⟨16862, 1⟩}], [{⟨1, 1⟩}], [(16862)], [(65, 6),(6, 65)]

---

su(2) ← sp(8432); so(16864); su(4); su(32) → su(16864)

[{⟨1, 1⟩},{⟨16863, 1⟩}],[{⟨1, 1⟩}],[(16863)],[{⟨1, 1⟩}],[(30, 0, 1),(1, 0, 30)], [{⟨1, 2⟩, ⟨31, 1⟩},{⟨1, 1⟩, ⟨31, 2⟩}]

---

su(2) ← sp(8436); so(16872); su(37) → su(16872)

[{⟨1, 1⟩},{⟨16871, 1⟩}],[{⟨1, 1⟩}],[(16871)],[{⟨1, 1⟩}],[{⟨1, 1⟩, ⟨2, 1⟩},{⟨35, 1⟩, ⟨36, 1⟩}]

---

su(2) ← sp(8448); so(9) ← so(16896) → su(16896)

[{⟨1, 1⟩},{⟨16895, 1⟩}],[{⟨1, 1⟩}],[(16895)],[{⟨1, 1⟩}],[(0, 0, 1, 3)]

---

su(2), su(130) → so(16899); su(3) → su(16899)

[{⟨1, 1⟩},{⟨16898, 1⟩}], [{⟨1, 1⟩}], [(16898)], [{⟨1, 1⟩, ⟨129, 1⟩}],[(128, 1),(1, 128)]

---

su(2) ← sp(8460); so(16920); su(3) → su(16920)

[{⟨1, 1⟩},{⟨16919, 1⟩}],[{⟨1, 1⟩}],[(16919)],[{⟨1, 1⟩}],[(89, 3),(3, 89)]

---

su(2) ← sp(8463); so(16926); su(3) → su(16926)

[{⟨1, 1⟩},{⟨16925, 1⟩}],[{⟨1, 1⟩}],[(16925)],[{⟨1, 1⟩}],[(30, 20),(20, 30)]

---

su(2) ← so(16929); su(3) → su(16929)

[{⟨1, 1⟩},{⟨16928, 1⟩}], [{⟨1, 1⟩}], [(16928)], [(56, 8),(8, 56)]

---

su(2) ← sp(8470); so(6) ← so(16940) → su(16940)

[{⟨1, 1⟩},{⟨16939, 1⟩}],[{⟨1, 1⟩}],[(16939)],[{⟨1, 1⟩}],[(6, 3, 3)]

---

su(2) ← so(16965); su(3) → su(16965)

[{⟨1, 1⟩},{⟨16964, 1⟩}], [{⟨1, 1⟩}], [(16964)], [(44, 12),

(12, 44)]

---

su(2) ← so(16983)
su(3)
← su(16983)

[{⟨1, 1⟩},{⟨16982, 1⟩}], [{⟨1, 1⟩}], [(16982)], [(36, 16), (16, 36)]

---

su(2) ← sp(8500)
so(17000)
su(3)
← su(17000)

[{⟨1, 1⟩},{⟨16999, 1⟩}],[{⟨1, 1⟩}],[(16999)],[{⟨1, 1⟩}], [(79, 4),(4, 79)]

---

su(2) ← sp(8505)
so(17010)
su(3)
su(5)
su(6)
su(6)
su(6)
← su(17010)

[{⟨1, 1⟩},{⟨17009, 1⟩}],[{⟨1, 1⟩}],[(17009)],[{⟨1, 1⟩}], [(104, 2),(2, 104)], [(4, 0, 2, 2),(2, 2, 0, 4)], [(0, 4, 0, 1, 0),(0, 1, 0, 4, 0)], [(2, 0, 1, 2, 0),(0, 2, 1, 0, 2)], [(5, 0, 1, 0, 1),(1, 0, 1, 0, 5)]

---

su(2)
so(13)
so(15)
sp(3)
g2
← so(17017) ← su(17017)

[{⟨1, 1⟩},{⟨17016, 1⟩}], [{⟨1, 1⟩}], [(17016)], [{⟨1, 2⟩, ⟨3, 1⟩}],[{⟨1, 1⟩, ⟨4, 1⟩}],[(10, 1, 0)],[(10, 1)]

---

su(2)
so(184)
← so(17019) ← su(17019)

[{⟨1, 1⟩},{⟨17018, 1⟩}],[{⟨1, 1⟩}],[(17018)],[{⟨1, 2⟩}]

---

su(2) ← sp(8510)
so(185), sp(92) ← so(17020)
su(3)
su(184)
su(185)
← su(17020)

[{⟨1, 1⟩},{⟨17019, 1⟩}],[{⟨1, 1⟩}],[(17019)],[{⟨1, 1⟩}], [{⟨2, 1⟩}], [{⟨1, 2⟩}], [(183, 0),(0, 183)], [{⟨1, 2⟩},{⟨183, 2⟩}],[{⟨2, 1⟩},{⟨183, 1⟩}]

---

su(2) ← so(17119)
su(3)
← su(17119)

[{⟨1, 1⟩},{⟨17118, 1⟩}], [{⟨1, 1⟩}], [(17118)], [(33, 18), (18, 33)]

---

su(2) ← so(17157)
su(3)
← su(17157)

[{⟨1, 1⟩},{⟨17156, 1⟩}], [{⟨1, 1⟩}], [(17156)], [(42, 13), (13, 42)]

---

su(2) ← sp(8580)
su(131), so(11) ← so(17160)
su(3)
su(3)
su(3)
su(10)
su(10)
su(11)
← su(17160)

[{⟨1, 1⟩},{⟨17159, 1⟩}],[{⟨1, 1⟩}],[(17159)],[{⟨1, 1⟩}], [{⟨1, 1⟩, ⟨130, 1⟩}], [(0, 1, 0, 0, 2)], [(29, 21),(21, 29)], [(38, 15),(15, 38)], [(129, 1),(1, 129)], [{⟨1, 2⟩, ⟨8, 1⟩, ⟨9, 1⟩},{⟨1, 1⟩, ⟨2, 1⟩, ⟨9, 2⟩}], [{⟨1, 3⟩, ⟨3, 1⟩},{⟨7, 1⟩, ⟨9, 3⟩}],[{⟨1, 2⟩, ⟨4, 1⟩},{⟨7, 1⟩, ⟨10, 2⟩}]

---

su(2) ← so(17199)
su(5)
← su(17199)

[{⟨1, 1⟩},{⟨17198, 1⟩}], [{⟨1, 1⟩}], [(17198)], [(5, 0, 1, 3),(3, 1, 0, 5)]

---

su(2), sp(2) ← sp(8602)
so(185), sp(93) ← so(17204)
← su(17204)

[{⟨1, 1⟩},{⟨17203, 1⟩}],[{⟨1, 1⟩}],[(17203)],[(11, 10)], [{⟨1, 1⟩}],[{⟨1, 2⟩}],[{⟨2, 1⟩}]

---

su(2), so(186) ← so(17205)
su(3)
su(185)
su(186)
← su(17205)

[{⟨1, 1⟩},{⟨17204, 1⟩}],[{⟨1, 1⟩}],[(17204)],[{⟨2, 1⟩}], [(184, 0),(0, 184)], [{⟨1, 2⟩},{⟨184, 2⟩}], [{⟨2, 1⟩},{⟨184, 1⟩}]

---

su(2) ← sp(8610)
so(17220)
su(3)
← su(17220)

[{⟨1, 1⟩},{⟨17219, 1⟩}],[{⟨1, 1⟩}],[(17219)],[{⟨1, 1⟩}], [(40, 14),(14, 40)]

---

su(2), sp(24) ← sp(8624)
so(17248)
su(7)
su(7)
← su(17248)

[{⟨1, 1⟩},{⟨17247, 1⟩}],[{⟨1, 1⟩}],[(17247)],[{⟨3, 1⟩}], [{⟨1, 1⟩}], [{⟨1, 2⟩, ⟨3, 1⟩, ⟨6, 2⟩},{⟨1, 2⟩, ⟨4, 1⟩, ⟨6, 2⟩}],[{⟨1, 3⟩, ⟨2, 1⟩, ⟨5, 1⟩},{⟨2, 1⟩, ⟨5, 1⟩, ⟨6, 3⟩}]

---

su(2) ← sp(8625)
so(24), so(46) ← so(17250)
← su(17250)

[{⟨1, 1⟩},{⟨17249, 1⟩}],[{⟨1, 1⟩}],[(17249)],[{⟨1, 1⟩}], [{⟨1, 4⟩}],[{⟨1, 3⟩}]

---

su(2) ← sp(8640)
so(17280)
su(3)
su(3)
su(4)
su(10)
so(10)
← su(17280)

[{⟨1, 1⟩},{⟨17279, 1⟩}],[{⟨1, 1⟩}],[(17279)],[{⟨1, 1⟩}], [(47, 11),(11, 47)], [(53, 9),(9, 53)], [(9, 1, 5),(5, 1, 9)], [{⟨1, 1⟩, ⟨4, 1⟩, ⟨9, 1⟩},{⟨1, 1⟩, ⟨6, 1⟩, ⟨9, 1⟩}], [(0, 1, 0, 3, 0),(0, 1, 0, 0, 3)]

---

su(2) ← sp(8645)
so(17290)
su(3)
su(4)
← su(17290)

[{⟨1, 1⟩},{⟨17289, 1⟩}],[{⟨1, 1⟩}],[(17289)],[{⟨1, 1⟩}], [(90, 3),(3, 90)],[(12, 5, 0),(0, 5, 12)]

---

su(2), sp(2), sp(23) ← sp(8648)
so(48) ← so(17296)
su(4)
su(46)
su(48)
← su(17296)

[{⟨1, 1⟩},{⟨17295, 1⟩}], [{⟨1, 1⟩}], [(17295)], [(45, 0)], [{⟨1, 3⟩}], [{⟨1, 1⟩}], [{⟨3, 1⟩}], [(45, 0, 0),(0, 0, 45)], [{⟨1, 3⟩},{⟨45, 3⟩}],[{⟨3, 1⟩},{⟨45, 1⟩}]

---

su(2) ← so(17301)
su(3)
← su(17301)

[{⟨1, 1⟩},{⟨17300, 1⟩}], [{⟨1, 1⟩}], [(17300)], [(72, 5), (5, 72)]

---

su(2) ← so(17325)
su(5)
su(5)
su(5)
su(6)
su(6)
su(8)
su(9)
su(9)
su(9)
so(10)
← su(17325)

[{⟨1, 1⟩},{⟨17324, 1⟩}], [{⟨1, 1⟩}], [(17324)], [(0, 5, 2, 0),(0, 2, 5, 0)],[(3, 1, 2, 1),(1, 2, 1, 3)],[(4, 0, 4, 0),(0, 4, 0, 4)], [(3, 0, 0, 2, 1),(1, 2, 0, 0, 3)], [(4, 3, 0, 0, 0),(0, 0, 0, 3, 4)], [{⟨1, 4⟩, ⟨4, 1⟩},{⟨4, 1⟩, ⟨7, 4⟩}], [{⟨2, 2⟩, ⟨7, 1⟩},{⟨2, 1⟩, ⟨7, 2⟩}], [{⟨1, 1⟩, ⟨2, 1⟩, ⟨6, 1⟩},{⟨3, 1⟩, ⟨7, 1⟩, ⟨8, 1⟩}], [{⟨1, 3⟩, ⟨5, 1⟩},{⟨4, 1⟩, ⟨8, 3⟩}], [(3, 0, 0, 2, 0),(3, 0, 0, 0, 2)]

---

su(2) ← so(17331)
su(3)
← su(17331)

[{⟨1, 1⟩},{⟨17330, 1⟩}], [{⟨1, 1⟩}], [(17330)], [(105, 2), (2, 105)]

---

su(2) ← sp(8671)
so(17342)
su(3)
← su(17342)

[{⟨1, 1⟩},{⟨17341, 1⟩}],[{⟨1, 1⟩}],[(17341)],[{⟨1, 1⟩}], [(28, 22),(22, 28)]

---

su(2) ← so(17353)
su(3)
← su(17353)

[{⟨1, 1⟩},{⟨17352, 1⟩}], [{⟨1, 1⟩}], [(17352)], [(66, 6), (6, 66)]

---

su(2) ← sp(8680)
so(17360)
su(3)
← su(17360)

[{⟨1, 1⟩},{⟨17359, 1⟩}],[{⟨1, 1⟩}],[(17359)],[{⟨1, 1⟩}], [(61, 7),(7, 61)]

---

su(2) ← sp(8695)
so(186) ← so(17390)
← su(17390)

[{⟨1, 1⟩},{⟨17389, 1⟩}],[{⟨1, 1⟩}],[(17389)],[{⟨1, 1⟩}], [{⟨1, 2⟩}]

---

su(2), so(187), sp(93) ← so(17391)
su(3)
su(3)
su(4)
su(33)
su(186)
su(187)
← su(17391)

[{⟨1, 1⟩},{⟨17390, 1⟩}],[{⟨1, 1⟩}],[(17390)],[{⟨2, 1⟩}], [{⟨1, 2⟩}],[(50, 10),(10, 50)],[(185, 0),(0, 185)],[(30, 1, 0),(0, 1, 30)], [{⟨1, 1⟩, ⟨31, 1⟩},{⟨2, 1⟩, ⟨32, 1⟩}], [{⟨1, 2⟩},{⟨185, 2⟩}],[{⟨2, 1⟩},{⟨185, 1⟩}]

---

su(2) ← so(17415)
su(3)
← su(17415)

[{⟨1, 1⟩},{⟨17414, 1⟩}], [{⟨1, 1⟩}], [(17414)], [(80, 4), (4, 80)]

su(2)
su(132) so(17423)
su(3) su(17423)

[{⟨1, 1⟩},{⟨17422, 1⟩}], [{⟨1, 1⟩}], [(17422)], [{⟨1, 1⟩, ⟨131, 1⟩}],[(130, 1),(1, 130)]

---

su(2) ← sp(8736)
so(7)
so(17472)
g2
su(3) su(17472)
su(13)
su(15)
so(14)

[{⟨1, 1⟩},{⟨17471, 1⟩}],[{⟨1, 1⟩}],[(17471)],[{⟨1, 1⟩}], [(0, 3, 3)], [(1, 7)], [(27, 23),(23, 27)], [{⟨1, 3⟩, ⟨2, 1⟩}, {⟨11, 1⟩, ⟨12, 3⟩}], [{⟨1, 1⟩, ⟨4, 1⟩},{⟨11, 1⟩, ⟨14, 1⟩}], [{⟨3, 1⟩, ⟨6, 1⟩},{⟨3, 1⟩, ⟨7, 1⟩}]

---

su(2)
sp(8740)
sp(2)
so(17480) su(17480)
su(4)

[{⟨1, 1⟩},{⟨17479, 1⟩}], [{⟨1, 1⟩}], [(17479)], [(7, 14)], [{⟨1, 1⟩}],[(18, 3, 0),(0, 3, 18)]

---

su(2) ← so(17487)
su(3) su(17487)

[{⟨1, 1⟩},{⟨17486, 1⟩}], [{⟨1, 1⟩}], [(17486)], [(57, 8), (8, 57)]

---

su(2) ← sp(8745)
so(17490) su(17490)
su(3)

[{⟨1, 1⟩},{⟨17489, 1⟩}],[{⟨1, 1⟩}],[(17489)],[{⟨1, 1⟩}], [(32, 19),(19, 32)]

---

su(2) ← sp(8748)
so(17496) su(17496)
su(3)

[{⟨1, 1⟩},{⟨17495, 1⟩}],[{⟨1, 1⟩}],[(17495)],[{⟨1, 1⟩}], [(35, 17),(17, 35)]

---

su(2) ← sp(8750)
so(17500) su(17500)
su(4)

[{⟨1, 1⟩},{⟨17499, 1⟩}],[{⟨1, 1⟩}],[(17499)],[{⟨1, 1⟩}], [(19, 0, 3),(3, 0, 19)]

---

su(2)
sp(8775)
sp(3)
so(27)
so(17550)
sp(12)
su(3) su(17550)
su(5)
su(24)
e6 ← su(27)

[{⟨1, 1⟩},{⟨17549, 1⟩}],[{⟨1, 1⟩}],[(17549)],[(2, 1, 3)], [{⟨1, 1⟩}],[{⟨4, 1⟩}],[{⟨1, 4⟩}],[(26, 24),(24, 26)],[(23, 0, 0, 0),(0, 0, 0, 23)], [{⟨1, 4⟩},{⟨23, 4⟩}], [{⟨4, 1⟩}, {⟨23, 1⟩}],[{⟨2, 1⟩, ⟨3, 1⟩},{⟨2, 1⟩, ⟨5, 1⟩}]

---

su(2) ← sp(8778)
sp(10) ← so(17556) su(17556)
su(4)

[{⟨1, 1⟩},{⟨17555, 1⟩}],[{⟨1, 1⟩}],[(17555)],[{⟨1, 1⟩}], [{⟨1, 1⟩, ⟨3, 1⟩}],[(10, 6, 0),(0, 6, 10)]

---

su(2)
so(17575) ← su(17575)
so(5)

[{⟨1, 1⟩},{⟨17574, 1⟩}],[{⟨1, 1⟩}],[(17574)],[(36, 0)]

---

su(2) ← sp(8788)
su(17576)
su(3) ← so(17576)

[{⟨1, 1⟩},{⟨17575, 1⟩}],[{⟨1, 1⟩}],[(17575)],[{⟨1, 1⟩}], [(25, 25)]

---

su(2)
so(187) so(17577) ← su(17577)
sp(94)

[{⟨1, 1⟩},{⟨17576, 1⟩}],[{⟨1, 1⟩}],[(17576)],[{⟨1, 2⟩}], [{⟨2, 1⟩}]

---

su(2) ← sp(8789)
so(188) ← so(17578)
su(3) su(17578)
su(187)
su(188)

[{⟨1, 1⟩},{⟨17577, 1⟩}],[{⟨1, 1⟩}],[(17577)],[{⟨1, 1⟩}], [{⟨2, 1⟩}], [(186, 0),(0, 186)], [{⟨1, 2⟩},{⟨186, 2⟩}], [{⟨2, 1⟩},{⟨186, 1⟩}]

---

su(2)
so(17595)
so(19)
su(4) su(17595)

[{⟨1, 1⟩},{⟨17594, 1⟩}], [{⟨1, 1⟩}], [(17594)], [{⟨1, 2⟩, ⟨2, 1⟩}],[(16, 0, 4),(4, 0, 16)]

---

su(2) ← sp(8800)
so(17600) su(17600)
su(5)

[{⟨1, 1⟩},{⟨17599, 1⟩}],[{⟨1, 1⟩}],[(17599)],[{⟨1, 1⟩}], [(9, 0, 0, 3),(3, 0, 0, 9)]

---

su(2) ← sp(8820)
so(7) ← so(17640)
su(5)
su(6) su(17640)
su(6)
su(6)
su(7)

[{⟨1, 1⟩},{⟨17639, 1⟩}],[{⟨1, 1⟩}],[(17639)],[{⟨1, 1⟩}], [(1, 2, 3)],[(6, 0, 0, 5),(5, 0, 0, 6)],[(1, 0, 4, 0, 0),(0, 0, 4, 0, 1)], [(1, 3, 0, 1, 0),(0, 1, 0, 3, 1)], [(4, 1, 0, 0, 2),(2, 0, 0, 1, 4)],[{⟨2, 3⟩, ⟨3, 1⟩},{⟨4, 1⟩, ⟨5, 3⟩}]

---

su(2) ← so(17641)
su(17641)
su(3)

[{⟨1, 1⟩},{⟨17640, 1⟩}], [{⟨1, 1⟩}], [(17640)], [(45, 12), (12, 45)]

---

su(2) ← so(17655)
su(17655)
su(3)

[{⟨1, 1⟩},{⟨17654, 1⟩}], [{⟨1, 1⟩}], [(17654)], [(106, 2), (2, 106)]

---

su(2) ← sp(8832)
so(17664) su(17664)
su(3)

[{⟨1, 1⟩},{⟨17663, 1⟩}],[{⟨1, 1⟩}],[(17663)],[{⟨1, 1⟩}], [(91, 3),(3, 91)]

---

su(2)
sp(8840)
sp(2) su(17680)
so(17680)

[{⟨1, 1⟩},{⟨17679, 1⟩}], [{⟨1, 1⟩}], [(17679)], [(25, 3)], [{⟨1, 1⟩}]

---

su(2) ← sp(8844)
su(133) ← so(17688) su(17688)
su(3)

[{⟨1, 1⟩},{⟨17687, 1⟩}],[{⟨1, 1⟩}],[(17687)],[{⟨1, 1⟩}], [{⟨1, 1⟩, ⟨132, 1⟩}],[(131, 1),(1, 131)]

---

su(2) ← sp(8855)
so(5) su(17710)
so(17710)
so(5)

[{⟨1, 1⟩},{⟨17709, 1⟩}],[{⟨1, 1⟩}],[(17709)],[{⟨1, 1⟩}], [(4, 22)],[(11, 10)]

---

su(2) ← so(17745)
su(17745)
su(13)

[{⟨1, 1⟩},{⟨17744, 1⟩}], [{⟨1, 1⟩}], [(17744)], [{⟨1, 1⟩, ⟨2, 2⟩},{⟨11, 2⟩, ⟨12, 1⟩}]

---

su(2) ← sp(8880)
so(17760) su(17760)
su(3)

[{⟨1, 1⟩},{⟨17759, 1⟩}],[{⟨1, 1⟩}],[(17759)],[{⟨1, 1⟩}], [(73, 5),(5, 73)]

---

su(2)
so(20) so(17765)
so(188) su(3) su(17765)
su(4)

[{⟨1, 1⟩},{⟨17764, 1⟩}], [{⟨1, 1⟩}], [(17764)], [{⟨1, 1⟩, ⟨3, 1⟩}], [{⟨1, 2⟩}], [(37, 16),(16, 37)], [(16, 1, 2),(2, 1, 16)]

---

su(2) ← sp(8883)
so(189)
so(17766)
sp(94)
su(3) su(17766)
su(188)
su(189)

[{⟨1, 1⟩},{⟨17765, 1⟩}],[{⟨1, 1⟩}],[(17765)],[{⟨1, 1⟩}], [{⟨2, 1⟩}], [{⟨1, 2⟩}], [(187, 0),(0, 187)], [{⟨1, 2⟩}, {⟨187, 2⟩}],[{⟨2, 1⟩},{⟨187, 1⟩}]

---

su(2) ← sp(8892)
so(17784) su(17784)
su(4)

[{⟨1, 1⟩},{⟨17783, 1⟩}],[{⟨1, 1⟩}],[(17783)],[{⟨1, 1⟩}], [(12, 2, 2),(2, 2, 12)]

---

su(2) ← sp(8904)
so(17808) su(17808)
su(3)

[{⟨1, 1⟩},{⟨17807, 1⟩}],[{⟨1, 1⟩}],[(17807)],[{⟨1, 1⟩}], [(31, 20),(20, 31)]

---

su(2)
sp(8910)
sp(2)
so(5) su(17820)
so(17820)
sp(5)
su(5)

[{⟨1, 1⟩},{⟨17819, 1⟩}], [{⟨1, 1⟩}], [(17819)], [(29, 2)], [{⟨1, 1⟩}], [(8, 14)], [(2, 2, 0, 0, 0)], [(1, 0, 7, 0),(0, 7, 0, 1)]

---

su(2) ← so(17835)
su(17835)
su(3)

[{⟨1, 1⟩},{⟨17834, 1⟩}], [{⟨1, 1⟩}], [(17834)], [(81, 4), (4, 81)]

---

su(2) ← sp(8918)
so(17836) su(17836)
su(4)

[{⟨1, 1⟩},{⟨17835, 1⟩}],[{⟨1, 1⟩}],[(17835)],[{⟨1, 1⟩}], [(12, 0, 6),(6, 0, 12)]

---

su(2)
sp(8925)
sp(7)
so(17850) su(17850)
su(3)

[{⟨1, 1⟩},{⟨17849, 1⟩}], [{⟨1, 1⟩}], [(17849)], [{⟨2, 1⟩, ⟨3, 1⟩}],[{⟨1, 1⟩}],[(67, 6),(6, 67)]

su(2) ← sp(8932)
so(17864) ← su(17864)
su(3)

[{⟨1, 1⟩},{⟨17863, 1⟩}],[{⟨1, 1⟩}],[(17863)],[{⟨1, 1⟩}], [(43, 13),(13, 43)]

---

su(2)
so(17871) ← su(17871)
so(5)

[{⟨1, 1⟩},{⟨17870, 1⟩}],[{⟨1, 1⟩}],[(17870)],[(13, 8)]

---

su(2)
so(17875)
so(9)
su(3) ← su(17875)
su(5)

[{⟨1, 1⟩},{⟨17874, 1⟩}], [{⟨1, 1⟩}], [(17874)], [(9, 0, 0, 0)],[(54, 9),(9, 54)],[(9, 0, 1, 1),(1, 1, 0, 9)]

---

su(2) ← sp(8946)
so(17892) ← su(17892)
su(3)

[{⟨1, 1⟩},{⟨17891, 1⟩}],[{⟨1, 1⟩}],[(17891)],[{⟨1, 1⟩}], [(62, 7),(7, 62)]

---

su(2)
so(17901) ← su(17901)
f4

[{⟨1, 1⟩},{⟨17900, 1⟩}], [{⟨1, 1⟩}], [(17900)], [(2, 0, 0, 1)]

---

su(2) ← sp(8960)
so(7)
sp(5) ← so(17920)
so(10)
su(3)
su(4) ← su(17920)
su(4)
su(4)
su(5)
su(8)

[{⟨1, 1⟩},{⟨17919, 1⟩}],[{⟨1, 1⟩}],[(17919)],[{⟨1, 1⟩}], [(1, 1, 5)], [(1, 1, 1, 0, 0)], [(1, 1, 1, 0, 0)], [(39, 15),(15, 39)], [(3, 9, 1),(1, 9, 3)], [(5, 7, 1),(1, 7, 5)], [(13, 1, 3),(3, 1, 13)], [(3, 2, 0, 3),(3, 0, 2, 3)], [{⟨1, 3⟩, ⟨6, 1⟩, ⟨7, 1⟩},{⟨1, 1⟩, ⟨2, 1⟩, ⟨7, 3⟩}]

---

su(2) ← sp(8967)
so(17934) ← su(17934)
su(3)

[{⟨1, 1⟩},{⟨17933, 1⟩}],[{⟨1, 1⟩}],[(17933)],[{⟨1, 1⟩}], [(48, 11),(11, 48)]

---

su(2)
sp(8970)
sp(2) ← su(17940)
so(17940)

[{⟨1, 1⟩},{⟨17939, 1⟩}], [{⟨1, 1⟩}], [(17939)], [(9, 12)], [{⟨1, 1⟩}]

---

su(2) ← sp(8977)
so(189) ← su(17954)
so(17954)
sp(95)

[{⟨1, 1⟩},{⟨17953, 1⟩}],[{⟨1, 1⟩}],[(17953)],[{⟨1, 1⟩}], [{⟨1, 2⟩}],[{⟨2, 1⟩}]

---

su(2)
su(134) ← so(17955)
so(190)
su(3)
su(3)
su(3) ← su(17955)
su(3)
su(189)
su(19)
su(190)
su(20)

[{⟨1, 1⟩},{⟨17954, 1⟩}], [{⟨1, 1⟩}], [(17954)], [{⟨1, 1⟩, ⟨133, 1⟩}], [{⟨2, 1⟩}], [(34, 18),(18, 34)], [(41, 14),(14, 41)], [(132, 1),(1, 132)], [(188, 0),(0, 188)], [{⟨1, 2⟩},{⟨188, 2⟩}], [{⟨2, 1⟩},{⟨188, 1⟩}], [{⟨1, 2⟩, ⟨2, 1⟩},{⟨17, 1⟩, ⟨18, 2⟩}],[{⟨1, 1⟩, ⟨3, 1⟩},{⟨17, 1⟩, ⟨19, 1⟩}]

---

su(2)
sp(8990)
sp(2) ← su(17980)
so(17980)

[{⟨1, 1⟩},{⟨17979, 1⟩}], [{⟨1, 1⟩}], [(17979)], [(1, 28)], [{⟨1, 1⟩}]

---

su(2) ← sp(8991)
so(17982) ← su(17982)
su(3)

[{⟨1, 1⟩},{⟨17981, 1⟩}],[{⟨1, 1⟩}],[(17981)],[{⟨1, 1⟩}], [(107, 2),(2, 107)]

---

su(2)
sp(9009)
sp(3)
so(9)
so(9) ← so(18018)
sp(7) ← su(18018)
su(3)
su(6)
su(13)

[{⟨1, 1⟩},{⟨18017, 1⟩}],[{⟨1, 1⟩}],[(18017)],[(6, 1, 1)], [{⟨1, 1⟩}], [(1, 0, 0, 4)], [(1, 3, 0, 0)], [{⟨1, 1⟩, ⟨7, 1⟩}], [(51, 10),(10, 51)],[(6, 1, 0, 0, 1),(1, 0, 0, 1, 6)],[{⟨1, 2⟩, ⟨3, 1⟩},{⟨10, 1⟩, ⟨12, 2⟩}]

---

su(2) ← sp(9021)
so(18042) ← su(18042)
su(3)

[{⟨1, 1⟩},{⟨18041, 1⟩}],[{⟨1, 1⟩}],[(18041)],[{⟨1, 1⟩}], [(92, 3),(3, 92)]

---

su(2) ← sp(9027)
so(18054) ← su(18054)
su(3)

[{⟨1, 1⟩},{⟨18053, 1⟩}],[{⟨1, 1⟩}],[(18053)],[{⟨1, 1⟩}], [(58, 8),(8, 58)]

---

su(2) ← so(18073)
su(18073)
su(3)

[{⟨1, 1⟩},{⟨18072, 1⟩}], [{⟨1, 1⟩}], [(18072)], [(30, 21), (21, 30)]

---

su(2)
sp(9072)
sp(2)
so(8) ← su(18144)
so(18144)
so(190)
su(4)

[{⟨1, 1⟩},{⟨18143, 1⟩}], [{⟨1, 1⟩}], [(18143)], [(5, 17)], [{⟨1, 1⟩}], [(2, 2, 1, 0),(2, 2, 0, 1),(1, 2, 2, 0),(1, 2, 0, 2), (0, 2, 2, 1),(0, 2, 1, 2)],[{⟨1, 2⟩}],[(23, 2, 0),(0, 2, 23)]

---

su(2)
so(191) ← so(18145)
sp(95)
su(3)
su(190) ← su(18145)
su(191)

[{⟨1, 1⟩},{⟨18144, 1⟩}],[{⟨1, 1⟩}],[(18144)],[{⟨2, 1⟩}], [{⟨1, 2⟩}], [(189, 0),(0, 189)], [{⟨1, 2⟩},{⟨189, 2⟩}], [{⟨2, 1⟩},{⟨189, 1⟩}]

---

su(2) ← sp(9075)
so(18150) ← su(18150)
su(11)

[{⟨1, 1⟩},{⟨18149, 1⟩}],[{⟨1, 1⟩}],[(18149)],[{⟨1, 1⟩}], [{⟨1, 3⟩, ⟨10, 2⟩},{⟨1, 2⟩, ⟨10, 3⟩}]

---

su(2) ← sp(9100)
so(14) ← so(18200)
su(18200)
su(5)
su(5)

[{⟨1, 1⟩},{⟨18199, 1⟩}],[{⟨1, 1⟩}],[(18199)],[{⟨1, 1⟩}], [{⟨2, 1⟩, ⟨3, 1⟩}],[(4, 1, 0, 4),(4, 0, 1, 4)],[(6, 0, 3, 0),(0, 3, 0, 6)]

---

su(2)
so(18207) ← su(18207)
su(17)

[{⟨1, 1⟩},{⟨18206, 1⟩}], [{⟨1, 1⟩}], [(18206)], [{⟨2, 1⟩, ⟨15, 1⟩}]

---

su(2) ← sp(9112)
su(135) ← so(18224) ← su(18224)
su(3)

[{⟨1, 1⟩},{⟨18223, 1⟩}],[{⟨1, 1⟩}],[(18223)],[{⟨1, 1⟩}], [{⟨1, 1⟩, ⟨134, 1⟩}],[(133, 1),(1, 133)]

---

su(2) ← so(18225)
su(18225)
su(3)

[{⟨1, 1⟩},{⟨18224, 1⟩}], [{⟨1, 1⟩}], [(18224)], [(74, 5), (5, 74)]

---

su(2)
sp(2) ← sp(9120)
sp(19)
su(16) ← su(18240)
so(18240)
so(38)
su(5)
su(19)

[{⟨1, 1⟩},{⟨18239, 1⟩}], [{⟨1, 1⟩}], [(18239)], [(35, 1)], [{⟨1, 1⟩, ⟨2, 1⟩}], [{⟨1, 1⟩}], [{⟨1, 2⟩, ⟨15, 2⟩}], [{⟨1, 1⟩, ⟨2, 1⟩}], [(15, 1, 0, 0),(0, 0, 1, 15)], [{⟨1, 1⟩, ⟨16, 1⟩},{⟨3, 1⟩, ⟨18, 1⟩}]

---

su(2) ← sp(9130)
so(18260) ← su(18260)
su(3)

[{⟨1, 1⟩},{⟨18259, 1⟩}],[{⟨1, 1⟩}],[(18259)],[{⟨1, 1⟩}], [(82, 4),(4, 82)]

---

su(2) ← sp(9139)
so(18278) ← su(18278)
su(38)

[{⟨1, 1⟩},{⟨18277, 1⟩}],[{⟨1, 1⟩}],[(18277)],[{⟨1, 1⟩}], [{⟨1, 1⟩, ⟨2, 1⟩},{⟨36, 1⟩, ⟨37, 1⟩}]

---

su(2) ← so(18285)
su(18285)
su(3)

[{⟨1, 1⟩},{⟨18284, 1⟩}], [{⟨1, 1⟩}], [(18284)], [(29, 22), (22, 29)]

---

su(2)
sp(2) ← sp(9152)
sp(3) ← su(18304)
g2 ← so(18304)
su(4)

[{⟨1, 1⟩},{⟨18303, 1⟩}], [{⟨1, 1⟩}], [(18303)], [(3, 21)], [(7, 2, 0)],[{⟨1, 1⟩}],[(3, 5)],[(21, 1, 1),(1, 1, 21)]

---

su(2) ← sp(9156)
so(18312) ← su(18312)
su(3)

[{⟨1, 1⟩},{⟨18311, 1⟩}],[{⟨1, 1⟩}],[(18311)],[{⟨1, 1⟩}], [(108, 2),(2, 108)]

---

su(2) ← so(18315)
su(18315)
su(3)

[{⟨1, 1⟩},{⟨18314, 1⟩}], [{⟨1, 1⟩}], [(18314)], [(36, 17), (17, 36)]

su(2) ← sp(9165) ←
so(18330) ← su(18330)
su(3) ←

[{⟨1, 1⟩},{⟨18329, 1⟩}],[{⟨1, 1⟩}],[(18329)],[{⟨1, 1⟩}], [(46, 12),(12, 46)]

---

su(2) ←
so(191) ← so(18335) ← su(18335)
sp(96) ←

[{⟨1, 1⟩},{⟨18334, 1⟩}],[{⟨1, 1⟩}],[(18334)],[{⟨1, 2⟩}], [{⟨2, 1⟩}]

---

su(2) ← sp(9168) ←
so(192) ← so(18336) ←
su(3) ← su(18336)
su(191) ←
su(192) ←

[{⟨1, 1⟩},{⟨18335, 1⟩}],[{⟨1, 1⟩}],[(18335)],[{⟨1, 1⟩}], [{⟨2, 1⟩}], [(190, 0),(0, 190)], [{⟨1, 2⟩},{⟨190, 2⟩}], [{⟨2, 1⟩},{⟨190, 1⟩}]

---

su(2) ← sp(9177) ←
so(18354) ← su(18354)
su(3) ←

[{⟨1, 1⟩},{⟨18353, 1⟩}],[{⟨1, 1⟩}],[(18353)],[{⟨1, 1⟩}], [(68, 6),(6, 68)]

---

su(2) ← sp(9180) ←
so(18360) ←
su(3) ←
su(4) ← su(18360)
su(4) ←
su(4) ←

[{⟨1, 1⟩},{⟨18359, 1⟩}],[{⟨1, 1⟩}],[(18359)],[{⟨1, 1⟩}], [(33, 19),(19, 33)], [(7, 8, 0),(0, 8, 7)], [(8, 2, 4),(4, 2, 8)],[(8, 5, 1),(1, 5, 8)]

---

su(2) ←
so(18377) ← su(18377)
so(47) ←

[{⟨1, 1⟩},{⟨18376, 1⟩}],[{⟨1, 1⟩}],[(18376)],[{⟨1, 3⟩}]

---

su(2) ← sp(9212) ←
so(5) ←
so(18424) ←
so(49) ←
su(3) ← su(18424)
su(4) ←
su(47) ←
su(49) ←

[{⟨1, 1⟩},{⟨18423, 1⟩}],[{⟨1, 1⟩}],[(18423)],[{⟨1, 1⟩}], [(0, 46)], [{⟨3, 1⟩}], [(93, 3),(3, 93)], [(46, 0, 0),(0, 0, 46)],[{⟨1, 3⟩},{⟨46, 3⟩}],[{⟨3, 1⟩},{⟨46, 1⟩}]

---

su(2) ← sp(9216) ←
so(18432) ← su(18432)
su(3) ←

[{⟨1, 1⟩},{⟨18431, 1⟩}],[{⟨1, 1⟩}],[(18431)],[{⟨1, 1⟩}], [(63, 7),(7, 63)]

---

su(2) ← sp(9222) ←
so(18444) ← su(18444)
su(3) ←

[{⟨1, 1⟩},{⟨18443, 1⟩}],[{⟨1, 1⟩}],[(18443)],[{⟨1, 1⟩}], [(28, 23),(23, 28)]

---

su(2) ←
sp(9240) ←
sp(3) ←
so(9) ← so(18480) ←
su(3) ←
su(4) ←
su(4) ←
su(4) ←
su(4) ←
su(4) ←
su(4) ← su(18480)
su(5) ←
su(5) ←
su(6) ←
su(6) ←
su(7) ←
su(8) ←
su(8) ←
su(33) ←

[{⟨1, 1⟩},{⟨18479, 1⟩}],[{⟨1, 1⟩}],[(18479)],[(3, 4, 0)], [{⟨1, 1⟩}], [(2, 0, 0, 3)], [(55, 9),(9, 55)], [(4, 8, 1),(1, 8, 4)], [(6, 3, 4),(4, 3, 6)], [(10, 4, 1),(1, 4, 10)], [(14, 0, 5),(5, 0, 14)], [(15, 4, 0),(0, 4, 15)], [(31, 0, 1),(1, 0, 31)], [(1, 1, 5, 0),(0, 5, 1, 1)],[(7, 1, 0, 2),(2, 0, 1, 7)],[(2, 2, 0, 0, 2),(2, 0, 0, 2, 2)], [(5, 0, 0, 2, 0),(0, 2, 0, 0, 5)], [{⟨1, 3⟩, ⟨2, 1⟩, ⟨3, 1⟩},{⟨4, 1⟩, ⟨5, 1⟩, ⟨6, 3⟩}], [{⟨1, 1⟩, ⟨6, 3⟩},{⟨2, 3⟩, ⟨7, 1⟩}], [{⟨1, 2⟩, ⟨2, 1⟩, ⟨3, 1⟩},{⟨5, 1⟩, ⟨6, 1⟩, ⟨7, 2⟩}],[{⟨1, 2⟩, ⟨32, 1⟩},{⟨1, 1⟩, ⟨32, 2⟩}]

---

su(2) ←
so(18495) ←
su(136) ←
su(3) ← su(18495)

[{⟨1, 1⟩},{⟨18494, 1⟩}], [{⟨1, 1⟩}], [(18494)], [{⟨1, 1⟩, ⟨135, 1⟩}],[(134, 1),(1, 134)]

---

su(2) ←
so(18527) ← su(18527)
so(192) ←

[{⟨1, 1⟩},{⟨18526, 1⟩}],[{⟨1, 1⟩}],[(18526)],[{⟨1, 2⟩}]

---

su(2) ← sp(9264) ←
so(193) ←
so(18528) ←
sp(96) ←
su(3) ← su(18528)
su(192) ←
su(193) ←

[{⟨1, 1⟩},{⟨18527, 1⟩}],[{⟨1, 1⟩}],[(18527)],[{⟨1, 1⟩}], [{⟨2, 1⟩}], [{⟨1, 2⟩}], [(191, 0),(0, 191)], [{⟨1, 2⟩},{⟨191, 2⟩}],[{⟨2, 1⟩},{⟨191, 1⟩}]

---

su(2) ← sp(9275) ←
so(5) ← so(18550) ← su(18550)
su(3) ←

[{⟨1, 1⟩},{⟨18549, 1⟩}],[{⟨1, 1⟩}],[(18549)],[{⟨1, 1⟩}], [(24, 2)],[(27, 24),(24, 27)]

---

su(2) ← sp(9282) ←
sp(3) ←
so(18564) ←
so(18) ←
su(3) ←
su(4) ← su(18564)
su(7) ←
su(13) ←
su(18) ←

[{⟨1, 1⟩},{⟨18563, 1⟩}],[{⟨1, 1⟩}],[(18563)],[{⟨1, 1⟩}], [(0, 2, 4)], [{⟨6, 1⟩}], [(38, 16),(16, 38)], [(3, 12, 0),(0, 12, 3)], [{⟨1, 12⟩},{⟨6, 12⟩}], [{⟨1, 6⟩},{⟨12, 6⟩}], [{⟨6, 1⟩},{⟨12, 1⟩}]

---

su(2) ← so(18585) ←
su(18585)
su(3) ←

[{⟨1, 1⟩},{⟨18584, 1⟩}], [{⟨1, 1⟩}], [(18584)], [(44, 13), (13, 44)]

---

su(2) ← sp(9300) ←
so(18600) ← su(18600)
su(3) ←

[{⟨1, 1⟩},{⟨18599, 1⟩}],[{⟨1, 1⟩}],[(18599)],[{⟨1, 1⟩}], [(49, 11),(11, 49)]

---

su(2) ← so(18603) ←
su(18603)
su(3) ←

[{⟨1, 1⟩},{⟨18602, 1⟩}], [{⟨1, 1⟩}], [(18602)], [(26, 25), (25, 26)]

---

su(2) ← sp(9310) ←
so(18620) ← su(18620)
su(4) ←

[{⟨1, 1⟩},{⟨18619, 1⟩}],[{⟨1, 1⟩}],[(18619)],[{⟨1, 1⟩}], [(11, 1, 4),(4, 1, 11)]

---

su(2) ← sp(9315) ←
so(18630) ← su(18630)
su(3) ←

[{⟨1, 1⟩},{⟨18629, 1⟩}],[{⟨1, 1⟩}],[(18629)],[{⟨1, 1⟩}], [(59, 8),(8, 59)]

---

su(2) ← so(18645) ←
su(18645)
su(3) ←

[{⟨1, 1⟩},{⟨18644, 1⟩}], [{⟨1, 1⟩}], [(18644)], [(109, 2), (2, 109)]

---

su(2) ← sp(9328) ←
so(18656) ← su(18656)
su(3) ←

[{⟨1, 1⟩},{⟨18655, 1⟩}],[{⟨1, 1⟩}],[(18655)],[{⟨1, 1⟩}], [(52, 10),(10, 52)]

---

su(2) ← sp(9345) ←
so(18690) ← su(18690)
su(3) ←

[{⟨1, 1⟩},{⟨18689, 1⟩}],[{⟨1, 1⟩}],[(18689)],[{⟨1, 1⟩}], [(83, 4),(4, 83)]

---

su(2) ← sp(9348) ←
so(18696) ←
su(3) ← su(18696)
su(3) ←

[{⟨1, 1⟩},{⟨18695, 1⟩}],[{⟨1, 1⟩}],[(18695)],[{⟨1, 1⟩}], [(40, 15),(15, 40)],[(75, 5),(5, 75)]

---

su(2) ← sp(9350) ←
so(5) ← so(18700) ← su(18700)
su(4) ←

[{⟨1, 1⟩},{⟨18699, 1⟩}],[{⟨1, 1⟩}],[(18699)],[{⟨1, 1⟩}], [(7, 16)],[(16, 2, 1),(1, 2, 16)]

---

su(2) ← so(18705) ←
su(18705)
su(3) ←

[{⟨1, 1⟩},{⟨18704, 1⟩}], [{⟨1, 1⟩}], [(18704)], [(42, 14), (14, 42)]

---

su(2) ←
so(5) ← so(18711) ←
so(8) ←
su(3) ← su(18711)
su(4) ←

[{⟨1, 1⟩},{⟨18710, 1⟩}], [{⟨1, 1⟩}], [(18710)], [(5, 20)], [(5, 0, 1, 1),(1, 0, 5, 1),(1, 0, 1, 5)], [(32, 20),(20, 32)], [(8, 1, 6),(6, 1, 8)]

---

su(2) ← sp(9360) ←
su(18720)
so(193) ←
so(18720) ←
sp(97) ←

[{⟨1, 1⟩},{⟨18719, 1⟩}],[{⟨1, 1⟩}],[(18719)],[{⟨1, 1⟩}], [{⟨1, 2⟩}],[{⟨2, 1⟩}]

su(2), so(194) ← so(18721)
so(18721), su(3), su(193), su(194) ← su(18721)

[{⟨1, 1⟩},{⟨18720, 1⟩}],[{⟨1, 1⟩}],[(18720)],[{⟨2, 1⟩}], [(192, 0),(0, 192)], [{⟨1, 2⟩},{⟨192, 2⟩}], [{⟨2, 1⟩}, {⟨192, 1⟩}]

su(2) ← sp(9375); so(5) ← so(18750)
sp(9375), so(18750) ← su(18750)

[{⟨1, 1⟩},{⟨18749, 1⟩}],[{⟨1, 1⟩}],[(18749)],[{⟨1, 1⟩}], [(19, 4)]

su(2) ← sp(9384); su(137) ← so(18768)
sp(9384), so(18768), su(3) ← su(18768)

[{⟨1, 1⟩},{⟨18767, 1⟩}],[{⟨1, 1⟩}],[(18767)],[{⟨1, 1⟩}], [{⟨1, 1⟩, ⟨136, 1⟩}],[(135, 1),(1, 135)]

su(2) ← sp(9405); sp(3) ← so(18810)
sp(9405), so(18810), su(3), su(3) ← su(18810)

[{⟨1, 1⟩},{⟨18809, 1⟩}],[{⟨1, 1⟩}],[(18809)],[{⟨1, 1⟩}], [(0, 7, 0)],[(35, 18),(18, 35)],[(94, 3),(3, 94)]

su(2), sp(3) ← sp(9408)
sp(9408), so(18816) ← su(18816)

[{⟨1, 1⟩},{⟨18815, 1⟩}], [{⟨1, 1⟩}], [(18815)], [(1, 1, 4)], [{⟨1, 1⟩}]

su(2) ← sp(9425)
sp(9425), so(18850), su(4) ← su(18850)

[{⟨1, 1⟩},{⟨18849, 1⟩}],[{⟨1, 1⟩}],[(18849)],[{⟨1, 1⟩}], [(24, 0, 2),(2, 0, 24)]

su(2) ← so(18865)
so(18865), su(3) ← su(18865)

[{⟨1, 1⟩},{⟨18864, 1⟩}], [{⟨1, 1⟩}], [(18864)], [(69, 6), (6, 69)]

su(2) ← sp(9450)
sp(9450), so(18900), su(7) ← su(18900)

[{⟨1, 1⟩},{⟨18899, 1⟩}],[{⟨1, 1⟩}],[(18899)],[{⟨1, 1⟩}], [{⟨2, 3⟩, ⟨5, 1⟩},{⟨2, 1⟩, ⟨5, 3⟩}]

su(2) ← sp(9457); so(194) ← so(18914)
sp(9457), so(18914) ← su(18914)

[{⟨1, 1⟩},{⟨18913, 1⟩}],[{⟨1, 1⟩}],[(18913)],[{⟨1, 1⟩}], [{⟨1, 2⟩}]

su(2), so(195), sp(97) ← so(18915)
so(18915), su(3), su(194), su(195) ← su(18915)

[{⟨1, 1⟩},{⟨18914, 1⟩}],[{⟨1, 1⟩}],[(18914)],[{⟨2, 1⟩}], [{⟨1, 2⟩}], [(193, 0),(0, 193)], [{⟨1, 2⟩},{⟨193, 2⟩}], [{⟨2, 1⟩},{⟨193, 1⟩}]

su(2) ← sp(9477); sp(6) ← so(18954)
sp(9477), so(18954) ← su(18954)

[{⟨1, 1⟩},{⟨18953, 1⟩}],[{⟨1, 1⟩}],[(18953)],[{⟨1, 1⟩}], [{⟨2, 1⟩, ⟨4, 1⟩}]

su(2) ← sp(9490)
sp(9490), so(18980), su(3) ← su(18980)

[{⟨1, 1⟩},{⟨18979, 1⟩}],[{⟨1, 1⟩}],[(18979)],[{⟨1, 1⟩}], [(64, 7),(7, 64)]

su(2) ← so(18981)
so(18981), su(3) ← su(18981)

[{⟨1, 1⟩},{⟨18980, 1⟩}], [{⟨1, 1⟩}], [(18980)], [(110, 2), (2, 110)]

su(2) ← sp(9504)
sp(9504), so(19008), su(3) ← su(19008)

[{⟨1, 1⟩},{⟨19007, 1⟩}],[{⟨1, 1⟩}],[(19007)],[{⟨1, 1⟩}], [(31, 21),(21, 31)]

su(2), so(5), so(5), g2 ← so(19019) ← su(19019)

[{⟨1, 1⟩},{⟨19018, 1⟩}], [{⟨1, 1⟩}], [(19018)], [(6, 18)], [(37, 0)],[(6, 3)]

su(2) ← sp(9516)
sp(9516), so(19032), su(3) ← su(19032)

[{⟨1, 1⟩},{⟨19031, 1⟩}],[{⟨1, 1⟩}],[(19031)],[{⟨1, 1⟩}], [(47, 12),(12, 47)]

su(2), sp(2) ← sp(9520)
sp(9520), so(19040), su(4), su(34) ← su(19040)

[{⟨1, 1⟩},{⟨19039, 1⟩}], [{⟨1, 1⟩}], [(19039)], [(13, 9)], [{⟨1, 1⟩}], [(31, 1, 0),(0, 1, 31)], [{⟨1, 1⟩, ⟨32, 1⟩}, {⟨2, 1⟩, ⟨33, 1⟩}]

su(2), su(138) ← so(19043)
so(19043), su(3) ← su(19043)

[{⟨1, 1⟩},{⟨19042, 1⟩}], [{⟨1, 1⟩}], [(19042)], [{⟨1, 1⟩, ⟨137, 1⟩}],[(136, 1),(1, 136)]

su(2) ← so(19095)
so(19095), su(3) ← su(19095)

[{⟨1, 1⟩},{⟨19094, 1⟩}], [{⟨1, 1⟩}], [(19094)], [(56, 9), (9, 56)]

su(2) ← sp(9548); g2 ← so(19096)
sp(9548), so(19096) ← su(19096)

[{⟨1, 1⟩},{⟨19095, 1⟩}],[{⟨1, 1⟩}],[(19095)],[{⟨1, 1⟩}], [(0, 9)]

su(2), so(195), sp(98) ← so(19109) ← su(19109)

[{⟨1, 1⟩},{⟨19108, 1⟩}],[{⟨1, 1⟩}],[(19108)],[{⟨1, 2⟩}], [{⟨2, 1⟩}]

su(2) ← sp(9555); so(196) ← so(19110)
sp(9555), so(19110), su(3), su(14), su(195), su(196) ← su(19110)

[{⟨1, 1⟩},{⟨19109, 1⟩}],[{⟨1, 1⟩}],[(19109)],[{⟨1, 1⟩}], [{⟨2, 1⟩}], [(194, 0),(0, 194)], [{⟨2, 1⟩, ⟨3, 1⟩},{⟨11, 1⟩, ⟨12, 1⟩}],[{⟨1, 2⟩},{⟨194, 2⟩}],[{⟨2, 1⟩},{⟨194, 1⟩}]

su(2) ← so(19125)
so(19125), su(3) ← su(19125)

[{⟨1, 1⟩},{⟨19124, 1⟩}], [{⟨1, 1⟩}], [(19124)], [(84, 4), (4, 84)]

su(2) ← sp(9576)
sp(9576), so(19152), su(3) ← su(19152)

[{⟨1, 1⟩},{⟨19151, 1⟩}],[{⟨1, 1⟩}],[(19151)],[{⟨1, 1⟩}], [(37, 17),(17, 37)]

su(2) ← so(19173)
so(19173), su(3) ← su(19173)

[{⟨1, 1⟩},{⟨19172, 1⟩}], [{⟨1, 1⟩}], [(19172)], [(76, 5), (5, 76)]

su(2) ← sp(9600); so(6), so(6) ← so(19200)
sp(9600), so(19200), su(3), su(6) ← su(19200)

[{⟨1, 1⟩},{⟨19199, 1⟩}],[{⟨1, 1⟩}],[(19199)],[{⟨1, 1⟩}], [(1, 7, 7)], [(3, 5, 5)], [(95, 3),(3, 95)], [(1, 2, 0, 1, 1),(1, 1, 0, 2, 1)]

su(2) ← so(19215)
so(19215), su(3) ← su(19215)

[{⟨1, 1⟩},{⟨19214, 1⟩}], [{⟨1, 1⟩}], [(19214)], [(60, 8), (8, 60)]

su(2) ← sp(9614); so(22) ← so(19228)
sp(9614), so(19228) ← su(19228)

[{⟨1, 1⟩},{⟨19227, 1⟩}],[{⟨1, 1⟩}],[(19227)],[{⟨1, 1⟩}], [{⟨2, 2⟩}]

su(2) ← sp(9625); sp(11) ← so(19250)
sp(9625), so(19250), su(3), su(5), su(5), su(6) ← su(19250)

[{⟨1, 1⟩},{⟨19249, 1⟩}],[{⟨1, 1⟩}],[(19249)],[{⟨1, 1⟩}], [{⟨2, 2⟩}], [(34, 19),(19, 34)], [(2, 1, 4, 0),(0, 4, 1, 2)], [(9, 0, 2, 0),(0, 2, 0, 9)],[(3, 0, 0, 3, 0),(0, 3, 0, 0, 3)]

su(2) ← so(19251)
so(19251), su(3) ← su(19251)

[{⟨1, 1⟩},{⟨19250, 1⟩}], [{⟨1, 1⟩}], [(19250)], [(30, 22), (22, 30)]

su(2) ← sp(9639); f4, g2 ← so(19278)
sp(9639), so(19278), su(3) ← su(19278)

[{⟨1, 1⟩},{⟨19277, 1⟩}],[{⟨1, 1⟩}],[(19277)],[{⟨1, 1⟩}], [(0, 1, 0, 1)],[(2, 6)],[(50, 11),(11, 50)]

su(2), so(7), so(13), sp(4), so(10), so(196) ← so(19305)
so(19305), su(3), su(7), su(10), su(10), e6, e6 ← su(19305)

[{⟨1, 1⟩},{⟨19304, 1⟩}],[{⟨1, 1⟩}],[(19304)],[(1, 0, 8)], [{⟨1, 1⟩, ⟨6, 2⟩}],[(6, 1, 0, 0)],[(8, 0, 0, 0, 0)],[{⟨1, 2⟩}], [(53, 10),(10, 53)], [{⟨1, 8⟩, ⟨6, 1⟩},{⟨1, 1⟩, ⟨6, 8⟩}], [{⟨1, 2⟩, ⟨2, 2⟩},{⟨8, 2⟩, ⟨9, 2⟩}], [{⟨1, 5⟩, ⟨9, 1⟩}, {⟨1, 1⟩, ⟨9, 5⟩}], [{⟨1, 2⟩, ⟨2, 1⟩},{⟨2, 1⟩, ⟨6, 2⟩}], [{⟨1, 4⟩},{⟨6, 4⟩}]

su(2) ⟵ sp(9653)
so(197), sp(98) ⟵ so(19306)
su(3)
su(196)
su(197)
⟵ su(19306)

[{⟨1, 1⟩},{⟨19305, 1⟩}],[{⟨1, 1⟩}],[(19305)],[{⟨1, 1⟩}],[{⟨2, 1⟩}], [{⟨1, 2⟩}], [(195, 0),(0, 195)], [{⟨1, 2⟩},{⟨195, 2⟩}],[{⟨2, 1⟩},{⟨195, 1⟩}]

---

su(2) ⟵ sp(9660)
su(139) ⟵ so(19320)
su(3)
su(3)
su(3)
⟵ su(19320)

[{⟨1, 1⟩},{⟨19319, 1⟩}],[{⟨1, 1⟩}],[(19319)],[{⟨1, 1⟩}],[{⟨1, 1⟩, ⟨138, 1⟩}], [(45, 13),(13, 45)], [(111, 2),(2, 111)],[(137, 1),(1, 137)]

---

su(2) ⟵ sp(9690)
so(17) ⟵ so(19380)
su(3)
su(4)
⟵ su(19380)

[{⟨1, 1⟩},{⟨19379, 1⟩}],[{⟨1, 1⟩}],[(19379)],[{⟨1, 1⟩}],[{⟨1, 5⟩}],[(39, 16),(16, 39)],[(1, 16, 0),(0, 16, 1)]

---

su(2) ⟵ so(19383)
su(3)
⟵ su(19383)

[{⟨1, 1⟩},{⟨19382, 1⟩}], [{⟨1, 1⟩}], [(19382)], [(70, 6),(6, 70)]

---

su(2) ⟵ sp(9702)
su(10), sp(3) ⟵ so(19404)
su(4)
su(7)
su(7)
⟵ su(19404)

[{⟨1, 1⟩},{⟨19403, 1⟩}],[{⟨1, 1⟩}],[(19403)],[{⟨1, 1⟩}],[{⟨5, 2⟩}], [(1, 4, 1)], [(10, 2, 3),(3, 2, 10)], [{⟨2, 5⟩},{⟨5, 5⟩}],[{⟨1, 1⟩, ⟨2, 4⟩},{⟨5, 4⟩, ⟨6, 1⟩}]

---

su(2) ⟵ sp(9720)
so(19440)
su(3)
⟵ su(19440)

[{⟨1, 1⟩},{⟨19439, 1⟩}],[{⟨1, 1⟩}],[(19439)],[{⟨1, 1⟩}],[(29, 23),(23, 29)]

---

su(2) ⟵ sp(9724)
so(17), sp(4) ⟵ so(19448), f4
su(8)
su(11)
su(17)
⟵ su(19448)

[{⟨1, 1⟩},{⟨19447, 1⟩}],[{⟨1, 1⟩}],[(19447)],[{⟨1, 1⟩}],[{⟨7, 1⟩}], [(10, 0, 0, 0)], [(0, 0, 2, 0)], [{⟨1, 10⟩},{⟨7, 10⟩}],[{⟨1, 7⟩},{⟨10, 7⟩}],[{⟨7, 1⟩},{⟨10, 1⟩}]

---

su(2) ⟵ sp(9735)
so(19470)
su(3)
⟵ su(19470)

[{⟨1, 1⟩},{⟨19469, 1⟩}],[{⟨1, 1⟩}],[(19469)],[{⟨1, 1⟩}],[(43, 14),(14, 43)]

---

su(2), so(6) ⟵ so(19481)
su(22)
⟵ su(19481)

[{⟨1, 1⟩},{⟨19480, 1⟩}], [{⟨1, 1⟩}], [(19480)], [(20, 0, 0)],[{⟨2, 2⟩},{⟨20, 2⟩}]

---

su(2) ⟵ sp(9744)
so(19488)
su(3)
⟵ su(19488)

[{⟨1, 1⟩},{⟨19487, 1⟩}],[{⟨1, 1⟩}],[(19487)],[{⟨1, 1⟩}],[(41, 15),(15, 41)]

---

su(2), so(5) ⟵ so(19499) ⟵ su(19499)

[{⟨1, 1⟩},{⟨19498, 1⟩}],[{⟨1, 1⟩}],[(19498)],[(2, 30)]

---

su(2) ⟵ sp(9751)
so(197), sp(99) ⟵ so(19502)
⟵ su(19502)

[{⟨1, 1⟩},{⟨19501, 1⟩}],[{⟨1, 1⟩}],[(19501)],[{⟨1, 1⟩}],[{⟨1, 2⟩}],[{⟨2, 1⟩}]

---

su(2), so(198) ⟵ so(19503)
su(3)
su(197)
su(198)
⟵ su(19503)

[{⟨1, 1⟩},{⟨19502, 1⟩}],[{⟨1, 1⟩}],[(19502)],[{⟨2, 1⟩}],[(196, 0),(0, 196)], [{⟨1, 2⟩},{⟨196, 2⟩}], [{⟨2, 1⟩},{⟨196, 1⟩}]

---

su(2) ⟵ sp(9758)
so(5) ⟵ so(19516)
⟵ su(19516)

[{⟨1, 1⟩},{⟨19515, 1⟩}],[{⟨1, 1⟩}],[(19515)],[{⟨1, 1⟩}],[(16, 6)]

---

su(2) ⟵ sp(9765)
so(5) ⟵ so(19530)
⟵ su(19530)

[{⟨1, 1⟩},{⟨19529, 1⟩}],[{⟨1, 1⟩}],[(19529)],[{⟨1, 1⟩}],[(3, 26)]

---

su(2) ⟵ sp(9768)
so(19536)
su(3)
⟵ su(19536)

[{⟨1, 1⟩},{⟨19535, 1⟩}],[{⟨1, 1⟩}],[(19535)],[{⟨1, 1⟩}],[(65, 7),(7, 65)]

---

su(2), sp(25) ⟵ sp(9775)
so(19550)
⟵ su(19550)

[{⟨1, 1⟩},{⟨19549, 1⟩}],[{⟨1, 1⟩}],[(19549)],[{⟨3, 1⟩}],[{⟨1, 1⟩}]

---

su(2) ⟵ sp(9776)
so(48) ⟵ so(19552)
⟵ su(19552)

[{⟨1, 1⟩},{⟨19551, 1⟩}],[{⟨1, 1⟩}],[(19551)],[{⟨1, 1⟩}],[{⟨1, 3⟩}]

---

su(2) ⟵ so(19565)
su(3)
⟵ su(19565)

[{⟨1, 1⟩},{⟨19564, 1⟩}], [{⟨1, 1⟩}], [(19564)], [(85, 4),(4, 85)]

---

su(2) ⟵ so(19575)
su(3)
⟵ su(19575)

[{⟨1, 1⟩},{⟨19574, 1⟩}], [{⟨1, 1⟩}], [(19574)], [(28, 24),(24, 28)]

---

su(2) ⟵ sp(9797)
so(19594)
su(3)
⟵ su(19594)

[{⟨1, 1⟩},{⟨19593, 1⟩}],[{⟨1, 1⟩}],[(19593)],[{⟨1, 1⟩}],[(96, 3),(3, 96)]

---

su(2), su(140) ⟵ so(19599)
su(3)
⟵ su(19599)

[{⟨1, 1⟩},{⟨19598, 1⟩}], [{⟨1, 1⟩}], [(19598)], [{⟨1, 1⟩, ⟨139, 1⟩}],[(138, 1),(1, 138)]

---

su(2), su(6), sp(2), sp(24) ⟵ sp(9800)
so(50) ⟵ so(19600)
su(4)
su(7)
su(48)
su(50)
⟵ su(19600)

[{⟨1, 1⟩},{⟨19599, 1⟩}],[{⟨1, 1⟩}],[(19599)],[(1, 0, 3, 0, 1)], [(47, 0)], [{⟨1, 3⟩}], [{⟨1, 1⟩}], [{⟨3, 1⟩}], [(47, 0, 0),(0, 0, 47)], [{⟨1, 4⟩, ⟨5, 1⟩, ⟨6, 1⟩},{⟨1, 1⟩, ⟨2, 1⟩, ⟨6, 4⟩}],[{⟨1, 3⟩},{⟨47, 3⟩}],[{⟨3, 1⟩},{⟨47, 1⟩}]

---

su(2), so(7) ⟵ so(19635)
su(3)
su(4)
⟵ su(19635)

[{⟨1, 1⟩},{⟨19634, 1⟩}],[{⟨1, 1⟩}],[(19634)],[(4, 0, 4)],[(33, 20),(20, 33)],[(6, 9, 0),(0, 9, 6)]

---

su(2) ⟵ sp(9828)
so(7), so(7) ⟵ so(19656)
su(3)
su(3)
su(4)
su(4)
su(8)
⟵ su(19656)

[{⟨1, 1⟩},{⟨19655, 1⟩}],[{⟨1, 1⟩}],[(19655)],[{⟨1, 1⟩}],[(0, 2, 5)],[(7, 0, 2)],[(27, 25),(25, 27)],[(77, 5),(5, 77)],[(6, 5, 2),(2, 5, 6)], [(11, 0, 7),(7, 0, 11)], [{⟨1, 5⟩, ⟨6, 1⟩},{⟨2, 1⟩, ⟨7, 5⟩}]

---

su(2) ⟵ sp(9831)
so(19662)
su(3)
⟵ su(19662)

[{⟨1, 1⟩},{⟨19661, 1⟩}],[{⟨1, 1⟩}],[(19661)],[{⟨1, 1⟩}],[(112, 2),(2, 112)]

---

su(2), su(3), so(7), sp(3), g2 ⟵ so(19683) ⟵ su(19683)

[{⟨1, 1⟩},{⟨19682, 1⟩}],[{⟨1, 1⟩}],[(19682)],[(26, 26)],[(2, 2, 2)],[(2, 2, 2)],[(8, 2)]

---

su(2) ⟵ sp(9842)
so(19684)
su(3)
⟵ su(19684)

[{⟨1, 1⟩},{⟨19683, 1⟩}],[{⟨1, 1⟩}],[(19683)],[{⟨1, 1⟩}],[(36, 18),(18, 36)]

---

su(2) ⟵ sp(9850)
so(198) ⟵ so(19700)
⟵ su(19700)

[{⟨1, 1⟩},{⟨19699, 1⟩}],[{⟨1, 1⟩}],[(19699)],[{⟨1, 1⟩}],[{⟨1, 2⟩}]

---

su(2), so(199), sp(99) ⟵ so(19701)
su(3)
su(198)
su(199)
⟵ su(19701)

[{⟨1, 1⟩},{⟨19700, 1⟩}],[{⟨1, 1⟩}],[(19700)],[{⟨2, 1⟩}],[{⟨1, 2⟩}], [(197, 0),(0, 197)], [{⟨1, 2⟩},{⟨197, 2⟩}],[{⟨2, 1⟩},{⟨197, 1⟩}]

su(2) ⟵ sp(9856) ⟵ su(19712)
so(7), so(9) ⟵ so(19712) ⟵ su(19712)

[{⟨1, 1⟩},{⟨19711, 1⟩}],[{⟨1, 1⟩}],[(19711)],[{⟨1, 1⟩}],[(3, 0, 5)],[(2, 0, 1, 1)]

---

su(2), sp(2) ⟵ sp(9860) ⟵ su(19720)
so(19720) ⟵ su(19720)
su(3) ⟵ su(19720)

[{⟨1, 1⟩},{⟨19719, 1⟩}], [{⟨1, 1⟩}], [(19719)], [(23, 4)], [{⟨1, 1⟩}],[(57, 9),(9, 57)]

---

su(2), so(5), so(39) ⟵ so(19721) ⟵ su(19721)

[{⟨1, 1⟩},{⟨19720, 1⟩}], [{⟨1, 1⟩}], [(19720)], [(1, 36)], [{⟨1, 1⟩, ⟨2, 1⟩}]

---

su(2) ⟵ so(19747) ⟵ su(19747)
su(3) ⟵ su(19747)

[{⟨1, 1⟩},{⟨19746, 1⟩}], [{⟨1, 1⟩}], [(19746)], [(48, 12), (12, 48)]

---

su(2) ⟵ sp(9880) ⟵ su(19760)
so(19760) ⟵ su(19760)
su(39) ⟵ su(19760)

[{⟨1, 1⟩},{⟨19759, 1⟩}],[{⟨1, 1⟩}],[(19759)],[{⟨1, 1⟩}],[{⟨1, 1⟩, ⟨2, 1⟩},{⟨37, 1⟩, ⟨38, 1⟩}]

---

su(2) ⟵ sp(9900) ⟵ su(19800)
so(19800) ⟵ su(19800)
su(5) ⟵ su(19800)
su(9) ⟵ su(19800)
su(10) ⟵ su(19800)

[{⟨1, 1⟩},{⟨19799, 1⟩}],[{⟨1, 1⟩}],[(19799)],[{⟨1, 1⟩}],[(2, 2, 1, 2),(2, 1, 2, 2)], [{⟨1, 1⟩, ⟨3, 1⟩, ⟨7, 1⟩},{⟨2, 1⟩, ⟨6, 1⟩, ⟨8, 1⟩}],[{⟨3, 1⟩, ⟨6, 1⟩},{⟨4, 1⟩, ⟨7, 1⟩}]

---

su(2) ⟵ so(19809) ⟵ su(19809)
su(3) ⟵ su(19809)

[{⟨1, 1⟩},{⟨19808, 1⟩}], [{⟨1, 1⟩}], [(19808)], [(61, 8), (8, 61)]

---

su(2), sp(2) ⟵ sp(9920) ⟵ su(19840)
so(19840) ⟵ su(19840)

[{⟨1, 1⟩},{⟨19839, 1⟩}], [{⟨1, 1⟩}], [(19839)], [(1, 29)], [{⟨1, 1⟩}]

---

su(2) ⟵ so(19845) ⟵ su(19845)
su(6) ⟵ su(19845)
su(6) ⟵ su(19845)

[{⟨1, 1⟩},{⟨19844, 1⟩}],[{⟨1, 1⟩}],[(19844)],[(2, 0, 2, 1, 0),(0, 1, 2, 0, 2)],[(4, 0, 0, 1, 2),(2, 1, 0, 0, 4)]

---

su(2) ⟵ sp(9940) ⟵ su(19880)
su(141) ⟵ so(19880) ⟵ su(19880)
su(3) ⟵ su(19880)

[{⟨1, 1⟩},{⟨19879, 1⟩}],[{⟨1, 1⟩}],[(19879)],[{⟨1, 1⟩}],[{⟨1, 1⟩, ⟨140, 1⟩}],[(139, 1),(1, 139)]

---

su(2) ⟵ sp(9945) ⟵ su(19890)
so(19890) ⟵ su(19890)
su(4) ⟵ su(19890)

[{⟨1, 1⟩},{⟨19889, 1⟩}],[{⟨1, 1⟩}],[(19889)],[{⟨1, 1⟩}],[(4, 11, 0),(0, 11, 4)]

---

su(2), so(199), sp(100) ⟵ so(19899) ⟵ su(19899)

[{⟨1, 1⟩},{⟨19898, 1⟩}],[{⟨1, 1⟩}],[(19898)],[{⟨1, 2⟩}],[{⟨2, 1⟩}]

---

su(2) ⟵ sp(9950) ⟵ su(19900)
so(200) ⟵ so(19900) ⟵ su(19900)
su(3) ⟵ su(19900)
su(199) ⟵ su(19900)
su(200) ⟵ su(19900)

[{⟨1, 1⟩},{⟨19899, 1⟩}],[{⟨1, 1⟩}],[(19899)],[{⟨1, 1⟩}],[{⟨2, 1⟩}], [(198, 0),(0, 198)], [{⟨1, 2⟩},{⟨198, 2⟩}],[{⟨2, 1⟩},{⟨198, 1⟩}]

---

su(2) ⟵ sp(9954) ⟵ su(19908)
so(19908) ⟵ su(19908)
su(3) ⟵ su(19908)

[{⟨1, 1⟩},{⟨19907, 1⟩}],[{⟨1, 1⟩}],[(19907)],[{⟨1, 1⟩}],[(71, 6),(6, 71)]

---

su(2) ⟵ so(19965) ⟵ su(19965)
su(3) ⟵ su(19965)
su(3) ⟵ su(19965)

[{⟨1, 1⟩},{⟨19964, 1⟩}], [{⟨1, 1⟩}], [(19964)], [(32, 21), (21, 32)],[(54, 10),(10, 54)]

---

su(2) ⟵ sp(9984) ⟵ su(19968)
so(19968) ⟵ su(19968)
su(3) ⟵ su(19968)

[{⟨1, 1⟩},{⟨19967, 1⟩}],[{⟨1, 1⟩}],[(19967)],[{⟨1, 1⟩}],[(51, 11),(11, 51)]

---

su(2) ⟵ sp(9996) ⟵ su(19992)
so(19992) ⟵ su(19992)
su(3) ⟵ su(19992)

[{⟨1, 1⟩},{⟨19991, 1⟩}],[{⟨1, 1⟩}],[(19991)],[{⟨1, 1⟩}],[(97, 3),(3, 97)]

---

su(2) ⟵ sp(10000) ⟵ su(20000)
so(20000) ⟵ su(20000)
su(4) ⟵ su(20000)

[{⟨1, 1⟩},{⟨19999, 1⟩}],[{⟨1, 1⟩}],[(19999)],[{⟨1, 1⟩}],[(19, 3, 0),(0, 3, 19)]

---

su(2) ⟵ so(20007) ⟵ su(20007)
su(3) ⟵ su(20007)
su(3) ⟵ su(20007)

[{⟨1, 1⟩},{⟨20006, 1⟩}], [{⟨1, 1⟩}], [(20006)], [(38, 17), (17, 38)],[(113, 2),(2, 113)]

---

su(2) ⟵ sp(10005) ⟵ su(20010)
so(20010) ⟵ su(20010)
su(3) ⟵ su(20010)

[{⟨1, 1⟩},{⟨20009, 1⟩}],[{⟨1, 1⟩}],[(20009)],[{⟨1, 1⟩}],[(86, 4),(4, 86)]

---

su(2) ⟵ sp(10010) ⟵ su(20020)
so(5), sp(7) ⟵ so(20020) ⟵ su(20020)
su(4) ⟵ su(20020)
su(5) ⟵ su(20020)
su(5) ⟵ su(20020)
su(5) ⟵ su(20020)
su(6) ⟵ su(20020)
su(7) ⟵ su(20020)
su(11) ⟵ su(20020)
su(12) ⟵ su(20020)
su(15) ⟵ su(20020)

[{⟨1, 1⟩},{⟨20019, 1⟩}],[{⟨1, 1⟩}],[(20019)],[{⟨1, 1⟩}],[(10, 12)],[{⟨1, 1⟩, ⟨5, 1⟩}],[(20, 0, 3),(3, 0, 20)],[(4, 5, 0, 0),(0, 0, 5, 4)], [(6, 0, 2, 1),(1, 2, 0, 6)], [(10, 1, 0, 1),(1, 0, 1, 10)], [(10, 1, 0, 0, 0),(0, 0, 0, 1, 10)], [{⟨1, 6⟩, ⟨3, 1⟩},{⟨4, 1⟩, ⟨6, 6⟩}], [{⟨1, 2⟩, ⟨7, 1⟩},{⟨4, 1⟩, ⟨10, 2⟩}], [{⟨1, 1⟩, ⟨10, 2⟩},{⟨2, 2⟩, ⟨11, 1⟩}], [{⟨1, 1⟩, ⟨11, 1⟩},{⟨4, 1⟩, ⟨14, 1⟩}]

---

su(2) ⟵ so(20069) ⟵ su(20069)
su(3) ⟵ su(20069)

[{⟨1, 1⟩},{⟨20068, 1⟩}], [{⟨1, 1⟩}], [(20068)], [(46, 13), (13, 46)]

---

su(2), sp(14) ⟵ so(20097) ⟵ su(20097)

[{⟨1, 1⟩},{⟨20096, 1⟩}],[{⟨1, 1⟩}],[(20096)],[{⟨4, 1⟩}]

---

su(2), so(200) ⟵ so(20099) ⟵ su(20099)

[{⟨1, 1⟩},{⟨20098, 1⟩}],[{⟨1, 1⟩}],[(20098)],[{⟨1, 2⟩}]

---

su(2) ⟵ sp(10050) ⟵ su(20100)
so(201), sp(100) ⟵ so(20100) ⟵ su(20100)
su(3) ⟵ su(20100)
su(3) ⟵ su(20100)
su(200) ⟵ su(20100)
su(201) ⟵ su(20100)

[{⟨1, 1⟩},{⟨20099, 1⟩}],[{⟨1, 1⟩}],[(20099)],[{⟨1, 1⟩}],[{⟨2, 1⟩}], [{⟨1, 2⟩}], [(66, 7),(7, 66)], [(199, 0),(0, 199)],[{⟨1, 2⟩},{⟨199, 2⟩}],[{⟨2, 1⟩},{⟨199, 1⟩}]

---

su(2) ⟵ so(20145) ⟵ su(20145)
su(3) ⟵ su(20145)

[{⟨1, 1⟩},{⟨20144, 1⟩}], [{⟨1, 1⟩}], [(20144)], [(78, 5), (5, 78)]

---

su(2) ⟵ sp(10075) ⟵ su(20150)
so(25) ⟵ so(20150) ⟵ su(20150)

[{⟨1, 1⟩},{⟨20149, 1⟩}],[{⟨1, 1⟩}],[(20149)],[{⟨1, 1⟩}],[{⟨1, 4⟩}]

---

su(2) ⟵ sp(10080) ⟵ su(20160)
so(20160) ⟵ su(20160)
su(3) ⟵ su(20160)
su(4) ⟵ su(20160)
su(4) ⟵ su(20160)
su(7) ⟵ su(20160)

[{⟨1, 1⟩},{⟨20159, 1⟩}],[{⟨1, 1⟩}],[(20159)],[{⟨1, 1⟩}],[(35, 19),(19, 35)], [(6, 4, 3),(3, 4, 6)], [(13, 3, 1),(1, 3, 13)],[{⟨1, 1⟩, ⟨2, 2⟩, ⟨4, 1⟩},{⟨3, 1⟩, ⟨5, 2⟩, ⟨6, 1⟩}]

---

su(2), su(142) ⟵ so(20163) ⟵ su(20163)
su(3) ⟵ su(20163)

[{⟨1, 1⟩},{⟨20162, 1⟩}], [{⟨1, 1⟩}], [(20162)], [{⟨1, 1⟩, ⟨141, 1⟩}],[(140, 1),(1, 140)]

---

su(2) ⟵ sp(10098) ⟵ su(20196)
$\mathfrak{g}_2$ ⟵ so(7), so(9), sp(3) ⟵ so(20196) ⟵ su(20196)
su(4) ⟵ su(20196)
su(4) ⟵ su(20196)
su(4) ⟵ su(20196)
su(34) ⟵ su(20196)

[{⟨1, 1⟩},{⟨20195, 1⟩}],[{⟨1, 1⟩}],[(20195)],[{⟨1, 1⟩}],[(14, 0, 0)], [(14, 0)], [(4, 0, 1, 0)], [(0, 4, 2)], [(5, 10, 0),(0, 10, 5)], [(7, 2, 5),(5, 2, 7)], [(32, 0, 1),(1, 0, 32)], [{⟨1, 2⟩, ⟨33, 1⟩},{⟨1, 1⟩, ⟨33, 2⟩}]

---

su(2) ⟵ so(20213) ⟵ su(20213)
su(3) ⟵ su(20213)

[{⟨1, 1⟩},{⟨20212, 1⟩}], [{⟨1, 1⟩}], [(20212)], [(40, 16), (16, 40)]

---

su(2) ⟵ sp(10120) ⟵ su(20240)
so(20240) ⟵ su(20240)
su(3) ⟵ su(20240)

[{⟨1, 1⟩},{⟨20239, 1⟩}],[{⟨1, 1⟩}],[(20239)],[{⟨1, 1⟩}], [(31, 22),(22, 31)]

---

su(2) ⟵ sp(10125)
so(20250) ⟵ su(20250)
su(3)

[{⟨1, 1⟩},{⟨20249, 1⟩}],[{⟨1, 1⟩}],[(20249)],[{⟨1, 1⟩}], [(44, 14),(14, 44)]

---

su(2) ⟵ sp(10140)
so(6) ⟵ so(20280)
su(20280)

[{⟨1, 1⟩},{⟨20279, 1⟩}],[{⟨1, 1⟩}],[(20279)],[{⟨1, 1⟩}], [(9, 2, 2)]

---

su(2) ⟵ sp(10148)
so(20296) ⟵ su(20296)
su(3)

[{⟨1, 1⟩},{⟨20295, 1⟩}],[{⟨1, 1⟩}],[(20295)],[{⟨1, 1⟩}], [(42, 15),(15, 42)]

---

su(2) ⟵ sp(10150)
so(201), sp(101) ⟵ so(20300) ⟵ su(20300)
su(4)

[{⟨1, 1⟩},{⟨20299, 1⟩}],[{⟨1, 1⟩}],[(20299)],[{⟨1, 1⟩}], [{⟨1, 2⟩}],[{⟨2, 1⟩}],[(24, 2, 0),(0, 2, 24)]

---

su(2), so(202) ⟵ so(20301)
su(3)
su(201) ⟵ su(20301)
su(202)

[{⟨1, 1⟩},{⟨20300, 1⟩}],[{⟨1, 1⟩}],[(20300)],[{⟨2, 1⟩}], [(200, 0),(0, 200)], [{⟨1, 2⟩},{⟨200, 2⟩}], [{⟨2, 1⟩}, {⟨200, 1⟩}]

---

su(2) ⟵ sp(10164)
so(20328) ⟵ su(20328)
su(11)

[{⟨1, 1⟩},{⟨20327, 1⟩}],[{⟨1, 1⟩}],[(20327)],[{⟨1, 1⟩}], [{⟨2, 1⟩, ⟨5, 1⟩},{⟨6, 1⟩, ⟨9, 1⟩}]

---

su(2), so(21), sp(3) ⟵ so(20349)
su(5)
su(6)
su(17) ⟵ su(20349)
su(18)
su(21)

[{⟨1, 1⟩},{⟨20348, 1⟩}],[{⟨1, 1⟩}],[(20348)],[{⟨5, 1⟩}], [(16, 0, 0)], [(16, 0, 0, 1),(1, 0, 0, 16)], [(16, 0, 0, 0, 0), (0, 0, 0, 0, 16)], [{⟨1, 5⟩},{⟨16, 5⟩}], [{⟨1, 3⟩, ⟨17, 1⟩}, {⟨1, 1⟩, ⟨17, 3⟩}],[{⟨5, 1⟩},{⟨16, 1⟩}]

---

su(2) ⟵ so(20355)
su(3) ⟵ su(20355)
su(3)

[{⟨1, 1⟩},{⟨20354, 1⟩}], [{⟨1, 1⟩}], [(20354)], [(58, 9), (9, 58)],[(114, 2),(2, 114)]

---

su(2), sp(4) ⟵ sp(10192)
so(7) ⟵ so(8) ⟵ so(20384)
su(20384)

[{⟨1, 1⟩},{⟨20383, 1⟩}], [{⟨1, 1⟩}], [(20383)], [(5, 0, 0, 1)], [{⟨1, 1⟩}], [(11, 0, 0, 0),(0, 0, 11, 0),(0, 0, 0, 11)], [(0, 0, 11)]

---

su(2) ⟵ sp(10197)
so(20394) ⟵ su(20394)
su(3)

[{⟨1, 1⟩},{⟨20393, 1⟩}],[{⟨1, 1⟩}],[(20393)],[{⟨1, 1⟩}], [(98, 3),(3, 98)]

---

su(2), sp(2) ⟵ sp(10200)
so(20400) ⟵ su(20400)
su(5)

[{⟨1, 1⟩},{⟨20399, 1⟩}], [{⟨1, 1⟩}], [(20399)], [(15, 8)], [{⟨1, 1⟩}],[(11, 2, 0, 0),(0, 0, 2, 11)]

---

su(2) ⟵ sp(10206)
so(20412)
su(3) ⟵ su(20412)
su(8)

[{⟨1, 1⟩},{⟨20411, 1⟩}],[{⟨1, 1⟩}],[(20411)],[{⟨1, 1⟩}], [(62, 8),(8, 62)], [{⟨1, 2⟩, ⟨2, 1⟩, ⟨7, 2⟩},{⟨1, 2⟩, ⟨6, 1⟩, ⟨7, 2⟩}]

---

su(2) ⟵ sp(10220)
so(20440) ⟵ su(20440)
su(3)

[{⟨1, 1⟩},{⟨20439, 1⟩}],[{⟨1, 1⟩}],[(20439)],[{⟨1, 1⟩}], [(72, 6),(6, 72)]

---

su(2) ⟵ sp(10224)
su(143) ⟵ so(20448) ⟵ su(20448)
su(3)

[{⟨1, 1⟩},{⟨20447, 1⟩}],[{⟨1, 1⟩}],[(20447)],[{⟨1, 1⟩}], [{⟨1, 1⟩, ⟨142, 1⟩}],[(141, 1),(1, 141)]

---

su(2) ⟵ sp(10230)
so(20460)
su(3) ⟵ su(20460)
su(3)

[{⟨1, 1⟩},{⟨20459, 1⟩}],[{⟨1, 1⟩}],[(20459)],[{⟨1, 1⟩}], [(30, 23),(23, 30)],[(87, 4),(4, 87)]

---

su(2), so(28) ⟵ so(20475)
su(3)
su(5)
su(5)
su(5) ⟵ su(20475)
su(5)
su(25)
su(28)

[{⟨1, 1⟩},{⟨20474, 1⟩}],[{⟨1, 1⟩}],[(20474)],[{⟨4, 1⟩}], [(49, 12),(12, 49)], [(6, 2, 1, 0),(0, 1, 2, 6)], [(8, 3, 0, 0), (0, 0, 3, 8)], [(12, 0, 0, 2),(2, 0, 0, 12)], [(24, 0, 0, 0),(0, 0, 0, 24)],[{⟨1, 4⟩},{⟨24, 4⟩}],[{⟨4, 1⟩},{⟨24, 1⟩}]

---

su(2), so(21), sp(2) ⟵ sp(10240)
so(20480) ⟵ su(20480)

[{⟨1, 1⟩},{⟨20479, 1⟩}], [{⟨1, 1⟩}], [(20479)], [{⟨1, 1⟩, ⟨10, 1⟩}],[(7, 15)],[{⟨1, 1⟩}]

---

su(2) ⟵ sp(10251)
so(202) ⟵ so(20502)
su(20502)

[{⟨1, 1⟩},{⟨20501, 1⟩}],[{⟨1, 1⟩}],[(20501)],[{⟨1, 1⟩}], [{⟨1, 2⟩}]

---

su(2), so(203), sp(101) ⟵ so(20503)
su(3)
su(202) ⟵ su(20503)
su(203)

[{⟨1, 1⟩},{⟨20502, 1⟩}],[{⟨1, 1⟩}],[(20502)],[{⟨2, 1⟩}], [{⟨1, 2⟩}], [(201, 0),(0, 201)], [{⟨1, 2⟩},{⟨201, 2⟩}], [{⟨2, 1⟩},{⟨201, 1⟩}]

---

su(2) ⟵ sp(10260)
so(20520)
su(4)
su(4) ⟵ su(20520)
su(4)
su(5)
su(17)

[{⟨1, 1⟩},{⟨20519, 1⟩}],[{⟨1, 1⟩}],[(20519)],[{⟨1, 1⟩}], [(2, 14, 0),(0, 14, 2)], [(9, 7, 0),(0, 7, 9)], [(17, 0, 4),(4, 0, 17)], [(14, 0, 1, 0),(0, 1, 0, 14)], [{⟨1, 2⟩, ⟨15, 1⟩}, {⟨2, 1⟩, ⟨16, 2⟩}]

---

su(2) ⟵ sp(10270)
so(5) ⟵ so(20540)
su(20540)

[{⟨1, 1⟩},{⟨20539, 1⟩}],[{⟨1, 1⟩}],[(20539)],[{⟨1, 1⟩}], [(38, 0)]

---

su(2) ⟵ so(20577)
su(3) ⟵ su(20577)

[{⟨1, 1⟩},{⟨20576, 1⟩}], [{⟨1, 1⟩}], [(20576)], [(37, 18), (18, 37)]

---

su(2) ⟵ sp(10290)
so(20580)
su(3)
su(4) ⟵ su(20580)
su(6)
su(7)

[{⟨1, 1⟩},{⟨20579, 1⟩}],[{⟨1, 1⟩}],[(20579)],[{⟨1, 1⟩}], [(34, 20),(20, 34)], [(13, 5, 0),(0, 5, 13)], [(6, 0, 0, 0, 3), (3, 0, 0, 0, 6)],[{⟨1, 1⟩, ⟨3, 3⟩},{⟨4, 3⟩, ⟨6, 1⟩}]

---

su(2) ⟵ sp(10296)
so(20592)
su(9) ⟵ su(20592)
su(13)
so(10)

[{⟨1, 1⟩},{⟨20591, 1⟩}],[{⟨1, 1⟩}],[(20591)],[{⟨1, 1⟩}], [{⟨1, 5⟩, ⟨2, 1⟩},{⟨7, 1⟩, ⟨8, 5⟩}], [{⟨1, 1⟩, ⟨6, 1⟩}, {⟨7, 1⟩, ⟨12, 1⟩}],[(5, 0, 0, 1, 0),(5, 0, 0, 0, 1)]

---

su(2) ⟵ so(20625)
su(3) ⟵ su(20625)
su(5)

[{⟨1, 1⟩},{⟨20624, 1⟩}], [{⟨1, 1⟩}], [(20624)], [(29, 24), (24, 29)],[(0, 4, 3, 0),(0, 3, 4, 0)]

---

su(2) ⟵ sp(10318)
so(20636) ⟵ su(20636)
su(3)

[{⟨1, 1⟩},{⟨20635, 1⟩}],[{⟨1, 1⟩}],[(20635)],[{⟨1, 1⟩}], [(55, 10),(10, 55)]

---

su(2) ⟵ sp(10320)
so(20640) ⟵ su(20640)
su(3)

[{⟨1, 1⟩},{⟨20639, 1⟩}],[{⟨1, 1⟩}],[(20639)],[{⟨1, 1⟩}], [(79, 5),(5, 79)]

---

su(2) ⟵ sp(10335)
so(20670) ⟵ su(20670)
su(3)

[{⟨1, 1⟩},{⟨20669, 1⟩}],[{⟨1, 1⟩}],[(20669)],[{⟨1, 1⟩}], [(52, 11),(11, 52)]

---

su(2) ⟵ sp(10336)
so(20672) ⟵ su(20672)
su(3)

[{⟨1, 1⟩},{⟨20671, 1⟩}],[{⟨1, 1⟩}],[(20671)],[{⟨1, 1⟩}], [(67, 7),(7, 67)]

su(2), sp(2) ← sp(10350)
sp(10350), so(20700), su(4), su(4) ← su(20700)

[{⟨1, 1⟩},{⟨20699, 1⟩}], [{⟨1, 1⟩}], [(20699)], [(3, 22)], [{⟨1, 1⟩}],[(17, 1, 2),(2, 1, 17)],[(22, 1, 1),(1, 1, 22)]

---

su(2), so(203), sp(102) ← so(20705) ← su(20705)

[{⟨1, 1⟩},{⟨20704, 1⟩}],[{⟨1, 1⟩}],[(20704)],[{⟨1, 2⟩}], [{⟨2, 1⟩}]

---

su(2) ← sp(10353)
so(204) ← so(20706)
sp(10353), so(20706), su(3), su(3), su(203), su(204) ← su(20706)

[{⟨1, 1⟩},{⟨20705, 1⟩}],[{⟨1, 1⟩}],[(20705)],[{⟨1, 1⟩}], [{⟨2, 1⟩}], [(115, 2),(2, 115)], [(202, 0),(0, 202)], [{⟨1, 2⟩},{⟨202, 2⟩}],[{⟨2, 1⟩},{⟨202, 1⟩}]

---

su(2), su(144), so(5) ← so(20735)
so(20735), su(3), su(3) ← su(20735)

[{⟨1, 1⟩},{⟨20734, 1⟩}], [{⟨1, 1⟩}], [(20734)], [{⟨1, 1⟩, ⟨143, 1⟩}], [(25, 2)], [(28, 25),(25, 28)], [(142, 1),(1, 142)]

---

su(2), sp(2) ← sp(10368)
sp(10368), so(20736) ← su(20736)

[{⟨1, 1⟩},{⟨20735, 1⟩}],[{⟨1, 1⟩}],[(20735)],[(11, 11)], [{⟨1, 1⟩}]

---

su(2) ← sp(10388)
so(49) ← so(20776)
sp(10388), so(20776) ← su(20776)

[{⟨1, 1⟩},{⟨20775, 1⟩}],[{⟨1, 1⟩}],[(20775)],[{⟨1, 1⟩}], [{⟨1, 3⟩}]

---

su(2) ← sp(10395)
sp(10395), so(20790), su(3), su(4), su(4), su(4), su(5), su(5), su(7), su(9), su(9), su(9), su(9), su(10), su(35), so(10) ← su(20790)

[{⟨1, 1⟩},{⟨20789, 1⟩}],[{⟨1, 1⟩}],[(20789)],[{⟨1, 1⟩}], [(27, 26),(26, 27)], [(10, 0, 8),(8, 0, 10)], [(10, 3, 2),(2, 3, 10)], [(32, 1, 0),(0, 1, 32)], [(4, 3, 1, 0),(0, 1, 3, 4)], [(7, 0, 1, 2),(2, 1, 0, 7)], [{⟨1, 2⟩, ⟨5, 2⟩, ⟨6, 1⟩},{⟨1, 1⟩, ⟨2, 2⟩, ⟨6, 2⟩}], [{⟨2, 2⟩, ⟨3, 1⟩},{⟨6, 1⟩, ⟨7, 2⟩}], [{⟨1, 1⟩, ⟨6, 2⟩},{⟨3, 2⟩, ⟨8, 1⟩}], [{⟨1, 1⟩, ⟨2, 1⟩, ⟨4, 1⟩},{⟨5, 1⟩, ⟨7, 1⟩, ⟨8, 1⟩}], [{⟨1, 4⟩, ⟨8, 2⟩},{⟨1, 2⟩, ⟨8, 4⟩}], [{⟨3, 1⟩, ⟨5, 1⟩},{⟨5, 1⟩, ⟨7, 1⟩}], [{⟨1, 1⟩, ⟨33, 1⟩},{⟨2, 1⟩, ⟨34, 1⟩}],[(1, 0, 0, 4, 0),(1, 0, 0, 0, 4)]

---

su(2) ← sp(10400)
sp(10400), so(20800), su(3) ← su(20800)

[{⟨1, 1⟩},{⟨20799, 1⟩}],[{⟨1, 1⟩}],[(20799)],[{⟨1, 1⟩}], [(99, 3),(3, 99)]

---

su(2), so(5), so(7), so(51), so(6) ← so(20825)
so(20825), su(4), su(49), su(51) ← su(20825)

[{⟨1, 1⟩},{⟨20824, 1⟩}], [{⟨1, 1⟩}], [(20824)], [(0, 48)], [(4, 1, 2)], [{⟨3, 1⟩}], [(2, 6, 6)], [(48, 0, 0),(0, 0, 48)], [{⟨1, 3⟩},{⟨48, 3⟩}],[{⟨3, 1⟩},{⟨48, 1⟩}]

---

su(2) ← sp(10416)
sp(10416), so(20832), su(3) ← su(20832)

[{⟨1, 1⟩},{⟨20831, 1⟩}],[{⟨1, 1⟩}],[(20831)],[{⟨1, 1⟩}], [(47, 13),(13, 47)]

---

su(2) ← sp(10440)
sp(10440), so(20880), su(3) ← su(20880)

[{⟨1, 1⟩},{⟨20879, 1⟩}],[{⟨1, 1⟩}],[(20879)],[{⟨1, 1⟩}], [(39, 17),(17, 39)]

---

su(2), sp(2) ← sp(10450)
sp(10450), so(20900) ← su(20900)

[{⟨1, 1⟩},{⟨20899, 1⟩}], [{⟨1, 1⟩}], [(20899)], [(5, 18)], [{⟨1, 1⟩}]

---

su(2), so(204) ← so(20909) ← su(20909)

[{⟨1, 1⟩},{⟨20908, 1⟩}],[{⟨1, 1⟩}],[(20908)],[{⟨1, 2⟩}]

---

su(2) ← sp(10455)
so(205), sp(102) ← so(20910)
sp(10455), so(20910), su(3), su(204), su(205) ← su(20910)

[{⟨1, 1⟩},{⟨20909, 1⟩}],[{⟨1, 1⟩}],[(20909)],[{⟨1, 1⟩}], [{⟨2, 1⟩}], [{⟨1, 2⟩}], [(203, 0),(0, 203)], [{⟨1, 2⟩}, {⟨203, 2⟩}],[{⟨2, 1⟩},{⟨203, 1⟩}]

---

su(2) ← so(20915)
so(20915), su(3) ← su(20915)

[{⟨1, 1⟩},{⟨20914, 1⟩}], [{⟨1, 1⟩}], [(20914)], [(88, 4), (4, 88)]

---

su(2), sp(2), sp(3) ← sp(10472)
sp(10472), so(20944), su(3) ← su(20944)

[{⟨1, 1⟩},{⟨20943, 1⟩}], [{⟨1, 1⟩}], [(20943)], [(21, 5)], [(10, 0, 1)],[{⟨1, 1⟩}],[(33, 21),(21, 33)]

---

su(2) ← so(20979)
so(20979), su(3) ← su(20979)

[{⟨1, 1⟩},{⟨20978, 1⟩}], [{⟨1, 1⟩}], [(20978)], [(73, 6), (6, 73)]

---

su(2), su(10), sp(3) ← sp(10500)
sp(10500), so(21000), su(3), su(5), su(5), su(6), su(6) ← su(21000)

[{⟨1, 1⟩},{⟨20999, 1⟩}], [{⟨1, 1⟩}], [(20999)], [{⟨1, 1⟩, ⟨5, 1⟩, ⟨9, 1⟩}], [(4, 2, 1)], [{⟨1, 1⟩}], [(59, 9),(9, 59)], [(4, 0, 3, 1),(1, 3, 0, 4)],[(9, 1, 1, 0),(0, 1, 1, 9)],[(1, 1, 0, 3, 0),(0, 3, 0, 1, 1)],[(1, 2, 1, 0, 1),(1, 0, 1, 2, 1)]

---

su(2), sp(4), sp(5), so(12) ← so(21021)
so(21021), su(8), su(13), so(14) ← su(21021)

[{⟨1, 1⟩},{⟨21020, 1⟩}], [{⟨1, 1⟩}], [(21020)], [(5, 0, 1, 0)], [(3, 0, 0, 0, 1)], [{⟨2, 1⟩, ⟨4, 1⟩}], [{⟨1, 6⟩, ⟨2, 1⟩}, {⟨6, 1⟩, ⟨7, 6⟩}], [{⟨1, 1⟩, ⟨7, 1⟩},{⟨6, 1⟩, ⟨12, 1⟩}], [{⟨1, 1⟩, ⟨6, 2⟩},{⟨1, 1⟩, ⟨7, 2⟩}]

---

su(2) ← sp(10512)
su(145) ← so(21024)
sp(10512), so(21024), su(3), su(3) ← su(21024)

[{⟨1, 1⟩},{⟨21023, 1⟩}],[{⟨1, 1⟩}],[(21023)],[{⟨1, 1⟩}], [{⟨1, 1⟩, ⟨144, 1⟩}],[(63, 8),(8, 63)],[(143, 1),(1, 143)]

---

su(2) ← so(21045)
so(21045), su(3) ← su(21045)

[{⟨1, 1⟩},{⟨21044, 1⟩}], [{⟨1, 1⟩}], [(21044)], [(45, 14), (14, 45)]

---

su(2) ← sp(10530)
so(5) ← so(21060)
sp(10530), so(21060), su(3), su(4) ← su(21060)

[{⟨1, 1⟩},{⟨21059, 1⟩}],[{⟨1, 1⟩}],[(21059)],[{⟨1, 1⟩}], [(14, 8)],[(116, 2),(2, 116)],[(25, 0, 2),(2, 0, 25)]

---

su(2) ← so(21063)
so(21063), su(3) ← su(21063)

[{⟨1, 1⟩},{⟨21062, 1⟩}], [{⟨1, 1⟩}], [(21062)], [(41, 16), (16, 41)]

---

su(2) ← sp(10545)
sp(10545), so(21090), su(3) ← su(21090)

[{⟨1, 1⟩},{⟨21089, 1⟩}],[{⟨1, 1⟩}],[(21089)],[{⟨1, 1⟩}], [(36, 19),(19, 36)]

---

su(2) ← sp(10557)
so(205), sp(103) ← so(21114)
sp(10557), so(21114) ← su(21114)

[{⟨1, 1⟩},{⟨21113, 1⟩}],[{⟨1, 1⟩}],[(21113)],[{⟨1, 1⟩}], [{⟨1, 2⟩}],[{⟨2, 1⟩}]

---

su(2), so(206) ← so(21115)
so(21115), su(3), su(205), su(206) ← su(21115)

[{⟨1, 1⟩},{⟨21114, 1⟩}],[{⟨1, 1⟩}],[(21114)],[{⟨2, 1⟩}], [(204, 0),(0, 204)], [{⟨1, 2⟩},{⟨204, 2⟩}], [{⟨2, 1⟩}, {⟨204, 1⟩}]

su(2), sp(3) → sp(10560); sp(10560), so(21120), su(3), su(6), su(10) ← su(21120)

[{⟨1, 1⟩},{⟨21119, 1⟩}], [{⟨1, 1⟩}], [(21119)], [(5, 3, 0)], [{⟨1, 1⟩}], [(43, 15),(15, 43)], [(5, 1, 1, 0, 0),(0, 0, 1, 1, 5)],[{⟨1, 1⟩, ⟨2, 1⟩, ⟨3, 1⟩},{⟨7, 1⟩, ⟨8, 1⟩, ⟨9, 1⟩}]

---

su(2) ← so(21141); so(21141), su(3) ← su(21141)

[{⟨1, 1⟩},{⟨21140, 1⟩}], [{⟨1, 1⟩}], [(21140)], [(80, 5), (5, 80)]

---

su(2) ← sp(10582); so(5) ← so(21164); sp(10582), so(21164) ← su(21164)

[{⟨1, 1⟩},{⟨21163, 1⟩}],[{⟨1, 1⟩}],[(21163)],[{⟨1, 1⟩}], [(12, 10)]

---

su(2) ← sp(10584); sp(10584), so(21168), su(7) ← su(21168)

[{⟨1, 1⟩},{⟨21167, 1⟩}],[{⟨1, 1⟩}],[(21167)],[{⟨1, 1⟩}], [{⟨1, 1⟩, ⟨4, 1⟩, ⟨5, 2⟩},{⟨2, 2⟩, ⟨3, 1⟩, ⟨6, 1⟩}]

---

su(2), so(6) ← so(21175) ← su(21175)

[{⟨1, 1⟩},{⟨21174, 1⟩}],[{⟨1, 1⟩}],[(21174)],[(0, 9, 9)]

---

su(2) ← sp(10605); sp(10605), so(21210), su(3) ← su(21210)

[{⟨1, 1⟩},{⟨21209, 1⟩}],[{⟨1, 1⟩}],[(21209)],[{⟨1, 1⟩}], [(100, 3),(3, 100)]

---

su(2), sp(2), sp(3) ← sp(10608); sp(10608), so(21216), su(3), su(4) ← su(21216)

[{⟨1, 1⟩},{⟨21215, 1⟩}], [{⟨1, 1⟩}], [(21215)], [(17, 7)], [(0, 3, 3)], [{⟨1, 1⟩}], [(50, 12),(12, 50)], [(8, 3, 3),(3, 3, 8)]

---

su(2) ← sp(10626); sp(10626), so(21252), su(3), su(3) ← su(21252)

[{⟨1, 1⟩},{⟨21251, 1⟩}],[{⟨1, 1⟩}],[(21251)],[{⟨1, 1⟩}], [(32, 22),(22, 32)],[(68, 7),(7, 68)]

---

su(2), sp(2), sp(2), sp(2), sp(20) ← sp(10640); so(40) ← so(21280); sp(10640), so(21280), su(4) ← su(21280)

[{⟨1, 1⟩},{⟨21279, 1⟩}], [{⟨1, 1⟩}], [(21279)], [(9, 13)], [(31, 2)], [(37, 1)], [{⟨1, 1⟩, ⟨2, 1⟩}], [{⟨1, 1⟩}], [{⟨1, 1⟩, ⟨2, 1⟩}],[(11, 6, 0),(0, 6, 11)]

---

su(2) ← sp(10647); sp(10647), so(21294), su(13) ← su(21294)

[{⟨1, 1⟩},{⟨21293, 1⟩}],[{⟨1, 1⟩}],[(21293)],[{⟨1, 1⟩}], [{⟨2, 1⟩, ⟨10, 1⟩},{⟨3, 1⟩, ⟨11, 1⟩}]

---

su(2), so(146) ← so(21315); so(21315), su(3) ← su(21315)

[{⟨1, 1⟩},{⟨21314, 1⟩}], [{⟨1, 1⟩}], [(21314)], [{⟨1, 1⟩, ⟨145, 1⟩}],[(144, 1),(1, 144)]

---

su(2) ← sp(10659); sp(10659), so(21318), su(3) ← su(21318)

[{⟨1, 1⟩},{⟨21317, 1⟩}],[{⟨1, 1⟩}],[(21317)],[{⟨1, 1⟩}], [(56, 10),(10, 56)]

---

su(2) ← sp(10660); so(206) ← so(21320); sp(10660), so(21320), su(40) ← su(21320)

[{⟨1, 1⟩},{⟨21319, 1⟩}],[{⟨1, 1⟩}],[(21319)],[{⟨1, 1⟩}], [{⟨1, 2⟩}],[{⟨1, 1⟩, ⟨2, 1⟩},{⟨38, 1⟩, ⟨39, 1⟩}]

---

su(2), so(207), sp(103) ← so(21321); so(21321), su(3), su(206), su(207) ← su(21321)

[{⟨1, 1⟩},{⟨21320, 1⟩}],[{⟨1, 1⟩}],[(21320)],[{⟨2, 1⟩}], [{⟨1, 2⟩}], [(205, 0),(0, 205)], [{⟨1, 2⟩},{⟨205, 2⟩}], [{⟨2, 1⟩},{⟨205, 1⟩}]

---

su(2) ← so(21375); so(21375), su(3) ← su(21375)

[{⟨1, 1⟩},{⟨21374, 1⟩}], [{⟨1, 1⟩}], [(21374)], [(89, 4), (4, 89)]

---

su(2) ← sp(10692); sp(10692), so(21384), su(3), su(6) ← su(21384)

[{⟨1, 1⟩},{⟨21383, 1⟩}],[{⟨1, 1⟩}],[(21383)],[{⟨1, 1⟩}], [(53, 11),(11, 53)],[(5, 1, 0, 1, 0),(0, 1, 0, 1, 5)]

---

su(2), so(5) ← so(21385) ← su(21385)

[{⟨1, 1⟩},{⟨21384, 1⟩}],[{⟨1, 1⟩}],[(21384)],[(20, 4)]

---

su(2) ← so(21417); so(21417), su(3) ← su(21417)

[{⟨1, 1⟩},{⟨21416, 1⟩}], [{⟨1, 1⟩}], [(21416)], [(117, 2), (2, 117)]

---

su(2), sp(2), sp(3) ← sp(10710); sp(10710), so(21420), su(4), su(4), su(4), su(4), su(4) ← su(21420)

[{⟨1, 1⟩},{⟨21419, 1⟩}], [{⟨1, 1⟩}], [(21419)], [(19, 6)], [(1, 0, 6)], [{⟨1, 1⟩}], [(2, 11, 1),(1, 11, 2)], [(7, 6, 1),(1, 6, 7)], [(8, 4, 2),(2, 4, 8)], [(13, 2, 2),(2, 2, 13)], [(14, 1, 3),(3, 1, 14)]

---

su(2) ← sp(10725); sp(6), so(12) ← so(21450); sp(10725), so(21450) ← su(21450)

[{⟨1, 1⟩},{⟨21449, 1⟩}],[{⟨1, 1⟩}],[(21449)],[{⟨1, 1⟩}], [{⟨2, 1⟩, ⟨6, 1⟩}],[{⟨2, 1⟩, ⟨5, 2⟩},{⟨2, 1⟩, ⟨6, 2⟩}]

---

su(2) ← so(21489); so(21489), su(3) ← su(21489)

[{⟨1, 1⟩},{⟨21488, 1⟩}], [{⟨1, 1⟩}], [(21488)], [(38, 18), (18, 38)]

---

su(2), sp(2) ← sp(10752); so(6) ← so(21504); sp(10752), so(21504), su(3), su(6), su(16), so(22) ← su(21504)

[{⟨1, 1⟩},{⟨21503, 1⟩}], [{⟨1, 1⟩}], [(21503)], [(27, 3)], [{⟨1, 1⟩}], [(13, 1, 1)], [(31, 23),(23, 31)], [(3, 1, 0, 0, 3), (3, 0, 0, 1, 3)], [{⟨1, 1⟩, ⟨2, 1⟩, ⟨15, 1⟩},{⟨1, 1⟩, ⟨14, 1⟩, ⟨15, 1⟩}],[{⟨1, 1⟩, ⟨10, 1⟩},{⟨1, 1⟩, ⟨11, 1⟩}]

---

su(2) ← so(21505); so(21505), su(4) ← su(21505)

[{⟨1, 1⟩},{⟨21504, 1⟩}],[{⟨1, 1⟩}],[(21504)],[(16, 4, 0), (0, 4, 16)]

---

su(2) ← so(21525); so(21525), su(3) ← su(21525)

[{⟨1, 1⟩},{⟨21524, 1⟩}], [{⟨1, 1⟩}], [(21524)], [(74, 6), (6, 74)]

---

su(2), so(207), sp(104) ← so(21527) ← su(21527)

[{⟨1, 1⟩},{⟨21526, 1⟩}],[{⟨1, 1⟩}],[(21526)],[{⟨1, 2⟩}], [{⟨2, 1⟩}]

---

su(2) ← sp(10764); so(208) ← so(21528); sp(10764), so(21528), su(3), su(207), su(208) ← su(21528)

[{⟨1, 1⟩},{⟨21527, 1⟩}],[{⟨1, 1⟩}],[(21527)],[{⟨1, 1⟩}], [{⟨2, 1⟩}], [(206, 0),(0, 206)], [{⟨1, 2⟩},{⟨206, 2⟩}], [{⟨2, 1⟩},{⟨206, 1⟩}]

---

su(2) ← sp(10773); so(20) ← so(21546); sp(10773), so(21546), su(3) ← su(21546)

[{⟨1, 1⟩},{⟨21545, 1⟩}],[{⟨1, 1⟩}],[(21545)],[{⟨1, 1⟩}], [{⟨1, 2⟩, ⟨2, 1⟩}],[(35, 20),(20, 35)]

---

su(2) ← sp(10780); sp(10780), so(21560), su(4), su(5), su(5) ← su(21560)

[{⟨1, 1⟩},{⟨21559, 1⟩}],[{⟨1, 1⟩}],[(21559)],[{⟨1, 1⟩}], [(13, 0, 6),(6, 0, 13)], [(2, 3, 2, 0),(0, 2, 3, 2)], [(3, 0, 5, 0),(0, 5, 0, 3)]

---

su(2) ← sp(10800); sp(10800), so(21600), su(5) ← su(21600)

[{⟨1, 1⟩},{⟨21599, 1⟩}],[{⟨1, 1⟩}],[(21599)],[{⟨1, 1⟩}], [(3, 4, 0, 1),(1, 0, 4, 3)]

---

su(2) ← sp(10804); su(147) ← so(21608); sp(10804), so(21608), su(3) ← su(21608)

[{⟨1, 1⟩},{⟨21607, 1⟩}],[{⟨1, 1⟩}],[(21607)],[{⟨1, 1⟩}], [{⟨1, 1⟩, ⟨146, 1⟩}],[(145, 1),(1, 145)]

---

su(2) ← so(21609); so(21609), su(3) ← su(21609)

[{⟨1, 1⟩},{⟨21608, 1⟩}], [{⟨1, 1⟩}], [(21608)], [(48, 13), (13, 48)]

su(2) ← sp(10812); so(21624) ← su(21624); su(3) ← su(21624)

[{⟨1, 1⟩},{⟨21623, 1⟩}],[{⟨1, 1⟩}],[(21623)],[{⟨1, 1⟩}], [(101, 3),(3, 101)]

---

su(2) ← so(21645) ← su(21645); su(3) ← su(21645)

[{⟨1, 1⟩},{⟨21644, 1⟩}], [{⟨1, 1⟩}], [(21644)], [(64, 8), (8, 64)]

---

su(2) ← sp(10824); so(21648) ← su(21648); su(3) ← su(21648)

[{⟨1, 1⟩},{⟨21647, 1⟩}],[{⟨1, 1⟩}],[(21647)],[{⟨1, 1⟩}], [(81, 5),(5, 81)]

---

su(2) ← so(21655) ← su(21655); su(3) ← su(21655)

[{⟨1, 1⟩},{⟨21654, 1⟩}], [{⟨1, 1⟩}], [(21654)], [(60, 9), (9, 60)]

---

su(2) ← sp(10850); so(21700) ← su(21700); su(3) ← su(21700)

[{⟨1, 1⟩},{⟨21699, 1⟩}],[{⟨1, 1⟩}],[(21699)],[{⟨1, 1⟩}], [(30, 24),(24, 30)]

---

su(2), so(21), sp(10), so(208) ← so(21735) ← su(21735); su(4) ← su(21735)

[{⟨1, 1⟩},{⟨21734, 1⟩}], [{⟨1, 1⟩}], [(21734)], [{⟨1, 1⟩, ⟨3, 1⟩}], [{⟨1, 2⟩, ⟨2, 1⟩}], [{⟨1, 2⟩}], [(17, 2, 1),(1, 2, 17)]

---

su(2) ← sp(10868); so(209), sp(104) ← so(21736); su(3); su(4); su(208); su(209) ← su(21736)

[{⟨1, 1⟩},{⟨21735, 1⟩}],[{⟨1, 1⟩}],[(21735)],[{⟨1, 1⟩}], [{⟨2, 1⟩}],[{⟨1, 2⟩}],[(207, 0),(0, 207)],[(10, 1, 5),(5, 1, 10)],[{⟨1, 2⟩},{⟨207, 2⟩}],[{⟨2, 1⟩},{⟨207, 1⟩}]

---

su(2) ← so(21771) ← su(21771); su(3) ← su(21771)

[{⟨1, 1⟩},{⟨21770, 1⟩}], [{⟨1, 1⟩}], [(21770)], [(40, 17), (17, 40)]

---

su(2) ← so(21777) ← su(21777); su(3) ← su(21777)

[{⟨1, 1⟩},{⟨21776, 1⟩}], [{⟨1, 1⟩}], [(21776)], [(118, 2), (2, 118)]

---

su(2) ← sp(10890); so(21780); su(5); su(11) ← su(21780)

[{⟨1, 1⟩},{⟨21779, 1⟩}],[{⟨1, 1⟩}],[(21779)],[{⟨1, 1⟩}], [(0, 7, 1, 0),(0, 1, 7, 0)], [{⟨2, 1⟩, ⟨6, 1⟩},{⟨5, 1⟩, ⟨9, 1⟩}]

---

su(2), sp(2) ← sp(10912); so(21824) ← su(21824)

[{⟨1, 1⟩},{⟨21823, 1⟩}], [{⟨1, 1⟩}], [(21823)], [(1, 30)], [{⟨1, 1⟩}]

---

su(2) ← sp(10920); so(8) ← so(21840); su(3); su(3); su(3); su(4) ← su(21840)

[{⟨1, 1⟩},{⟨21839, 1⟩}],[{⟨1, 1⟩}],[(21839)],[{⟨1, 1⟩}], [(2, 3, 0, 0),(0, 3, 2, 0),(0, 3, 0, 2)], [(29, 25),(25, 29)], [(69, 7),(7, 69)],[(90, 4),(4, 90)],[(5, 6, 2),(2, 6, 5)]

---

su(2) ← so(21855) ← su(21855); su(3) ← su(21855)

[{⟨1, 1⟩},{⟨21854, 1⟩}], [{⟨1, 1⟩}], [(21854)], [(46, 14), (14, 46)]

---

su(2), so(5), so(5) ← so(21875) ← su(21875)

[{⟨1, 1⟩},{⟨21874, 1⟩}], [{⟨1, 1⟩}], [(21874)], [(4, 24)], [(9, 14)]

---

su(2) ← sp(10948); so(21896) ← su(21896); su(4) ← su(21896)

[{⟨1, 1⟩},{⟨21895, 1⟩}],[{⟨1, 1⟩}],[(21895)],[{⟨1, 1⟩}], [(15, 0, 5),(5, 0, 15)]

---

su(2), su(148) ← so(21903); su(3) ← su(21903)

[{⟨1, 1⟩},{⟨21902, 1⟩}], [{⟨1, 1⟩}], [(21902)], [{⟨1, 1⟩, ⟨147, 1⟩}],[(146, 1),(1, 146)]

---

su(2) ← sp(10962); so(21924) ← su(21924); su(3) ← su(21924)

[{⟨1, 1⟩},{⟨21923, 1⟩}],[{⟨1, 1⟩}],[(21923)],[{⟨1, 1⟩}], [(28, 26),(26, 28)]

---

su(2) ← sp(10965); so(21930) ← su(21930); su(3) ← su(21930)

[{⟨1, 1⟩},{⟨21929, 1⟩}],[{⟨1, 1⟩}],[(21929)],[{⟨1, 1⟩}], [(42, 16),(16, 42)]

---

su(2) ← sp(10972); so(209), sp(105) ← so(21944) ← su(21944)

[{⟨1, 1⟩},{⟨21943, 1⟩}],[{⟨1, 1⟩}],[(21943)],[{⟨1, 1⟩}], [{⟨1, 2⟩}],[{⟨2, 1⟩}]

---

su(2), so(11), sp(3), so(210) ← so(21945); su(3); su(3); su(209); su(20), su(21) ← su(210) ← su(21945)

[{⟨1, 1⟩},{⟨21944, 1⟩}],[{⟨1, 1⟩}],[(21944)],[(4, 1, 0, 0)],[(0, 0, 8)],[{⟨2, 1⟩}],[(34, 21),(21, 34)],[(208, 0),(0, 208)], [{⟨1, 2⟩},{⟨208, 2⟩}], [{⟨2, 1⟩},{⟨208, 1⟩}], [{⟨1, 2⟩, ⟨2, 1⟩},{⟨18, 1⟩, ⟨19, 2⟩}], [{⟨1, 1⟩, ⟨3, 1⟩}, {⟨18, 1⟩, ⟨20, 1⟩}]

---

su(2) ← sp(10976); su(3) ← so(21952) ← su(21952)

[{⟨1, 1⟩},{⟨21951, 1⟩}],[{⟨1, 1⟩}],[(21951)],[{⟨1, 1⟩}], [(27, 27)]

---

su(2) ← sp(10980); so(21960) ← su(21960); su(3) ← su(21960)

[{⟨1, 1⟩},{⟨21959, 1⟩}],[{⟨1, 1⟩}],[(21959)],[{⟨1, 1⟩}], [(44, 15),(15, 44)]

---

su(2) ← sp(10985); so(21970) ← su(21970); su(3) ← su(21970)

[{⟨1, 1⟩},{⟨21969, 1⟩}],[{⟨1, 1⟩}],[(21969)],[{⟨1, 1⟩}], [(51, 12),(12, 51)]

---

su(2), sp(3) ← sp(11000); so(22000) ← su(22000); su(4) ← su(22000)

[{⟨1, 1⟩},{⟨21999, 1⟩}],[{⟨1, 1⟩}],[(21999)],[(3, 0, 4)], [{⟨1, 1⟩}],[(5, 4, 4),(4, 4, 5)]

---

su(2) ← so(22011) ← su(22011); su(3) ← su(22011)

[{⟨1, 1⟩},{⟨22010, 1⟩}], [{⟨1, 1⟩}], [(22010)], [(57, 10), (10, 57)]

---

su(2) ← so(22015); su(4); su(35) ← su(22015)

[{⟨1, 1⟩},{⟨22014, 1⟩}],[{⟨1, 1⟩}],[(22014)],[(33, 0, 1), (1, 0, 33)],[{⟨1, 2⟩, ⟨34, 1⟩},{⟨1, 1⟩, ⟨34, 2⟩}]

---

su(2) ← sp(11020); so(22040) ← su(22040); su(3) ← su(22040)

[{⟨1, 1⟩},{⟨22039, 1⟩}],[{⟨1, 1⟩}],[(22039)],[{⟨1, 1⟩}], [(37, 19),(19, 37)]

---

su(2) ← sp(11021); so(22042) ← su(22042); su(3) ← su(22042)

[{⟨1, 1⟩},{⟨22041, 1⟩}],[{⟨1, 1⟩}],[(22041)],[{⟨1, 1⟩}], [(102, 3),(3, 102)]

---

su(2), sp(26) ← sp(11024); so(22048) ← su(22048)

[{⟨1, 1⟩},{⟨22047, 1⟩}],[{⟨1, 1⟩}],[(22047)],[{⟨3, 1⟩}], [{⟨1, 1⟩}]

---

su(2) ← sp(11025); so(50) ← so(22050); su(5); su(6); su(6) ← su(22050)

[{⟨1, 1⟩},{⟨22049, 1⟩}],[{⟨1, 1⟩}],[(22049)],[{⟨1, 1⟩}], [{⟨1, 3⟩}], [(4, 1, 1, 2),(2, 1, 1, 4)], [(1, 0, 1, 3, 0),(0, 3, 1, 0, 1)],[(2, 1, 1, 1, 0),(0, 1, 1, 1, 2)]

---

su(2) ← sp(11039); so(22078) ← su(22078); su(3) ← su(22078)

[{⟨1, 1⟩},{⟨22077, 1⟩}],[{⟨1, 1⟩}],[(22077)],[{⟨1, 1⟩}], [(75, 6),(6, 75)]

---

su(2), sp(2), sp(25) ← sp(11050); so(52) ← so(22100); su(4); su(50); su(52) ← su(22100)

[{⟨1, 1⟩},{⟨22099, 1⟩}], [{⟨1, 1⟩}], [(22099)], [(49, 0)], [{⟨1, 3⟩}], [{⟨1, 1⟩}], [{⟨3, 1⟩}], [(49, 0, 0),(0, 0, 49)], [{⟨1, 3⟩},{⟨49, 3⟩}],[{⟨3, 1⟩},{⟨49, 1⟩}]

su(2) ⟵ sp(11055) ⟵
so(22110) ⟵ su(22110)
su(3) ⟵

[{⟨1, 1⟩},{⟨22109, 1⟩}],[{⟨1, 1⟩}],[(22109)],[{⟨1, 1⟩}],[(54, 11),(11, 54)]

---

su(2) ⟵ sp(11070) ⟵
so(5) ⟵ so(22140) ⟵ su(22140)
su(3) ⟵

[{⟨1, 1⟩},{⟨22139, 1⟩}],[{⟨1, 1⟩}],[(22139)],[{⟨1, 1⟩}],[(39, 0)],[(119, 2),(2, 119)]

---

su(2) ⟵ sp(11077) ⟵ su(22154)
so(210) ⟵ so(22154) ⟵

[{⟨1, 1⟩},{⟨22153, 1⟩}],[{⟨1, 1⟩}],[(22153)],[{⟨1, 1⟩}],[{⟨1, 2⟩}]

---

su(2) ⟵
so(211) ⟵ so(22155) ⟵
sp(105) ⟵
su(3) ⟵ su(22155)
su(210) ⟵
su(211) ⟵

[{⟨1, 1⟩},{⟨22154, 1⟩}],[{⟨1, 1⟩}],[(22154)],[{⟨2, 1⟩}],[{⟨1, 2⟩}], [(209, 0),(0, 209)], [{⟨1, 2⟩},{⟨209, 2⟩}],[{⟨2, 1⟩},{⟨209, 1⟩}]

---

su(2) ⟵ so(22161) ⟵ su(22161)
su(3) ⟵

[{⟨1, 1⟩},{⟨22160, 1⟩}], [{⟨1, 1⟩}], [(22160)], [(82, 5),(5, 82)]

---

su(2) ⟵ sp(11088) ⟵
so(22176) ⟵
su(5) ⟵
su(5) ⟵ su(22176)
su(5) ⟵
su(6) ⟵
su(9) ⟵

[{⟨1, 1⟩},{⟨22175, 1⟩}],[{⟨1, 1⟩}],[(22175)],[{⟨1, 1⟩}],[(2, 0, 6, 0),(0, 6, 0, 2)],[(2, 3, 1, 1),(1, 1, 3, 2)],[(7, 2, 0, 1),(1, 0, 2, 7)], [(2, 3, 0, 0, 1),(1, 0, 0, 3, 2)], [{⟨1, 2⟩, ⟨7, 2⟩},{⟨2, 2⟩, ⟨8, 2⟩}]

---

su(2) ⟵ sp(11100) ⟵
su(149) ⟵ so(22200) ⟵ su(22200)
su(3) ⟵

[{⟨1, 1⟩},{⟨22199, 1⟩}],[{⟨1, 1⟩}],[(22199)],[{⟨1, 1⟩}],[{⟨1, 1⟩, ⟨148, 1⟩}],[(147, 1),(1, 147)]

---

su(2) ⟵
so(11) ⟵ so(22275) ⟵
su(3) ⟵ su(22275)
su(6) ⟵

[{⟨1, 1⟩},{⟨22274, 1⟩}],[{⟨1, 1⟩}],[(22274)],[(2, 0, 0, 0, 2)],[(65, 8),(8, 65)],[(8, 0, 0, 0, 2),(2, 0, 0, 0, 8)]

---

su(2) ⟵ so(22287) ⟵ su(22287)
su(3) ⟵

[{⟨1, 1⟩},{⟨22286, 1⟩}], [{⟨1, 1⟩}], [(22286)], [(33, 22),(22, 33)]

---

su(2) ⟵ so(22295) ⟵ su(22295)
su(5) ⟵

[{⟨1, 1⟩},{⟨22294, 1⟩}], [{⟨1, 1⟩}], [(22294)], [(6, 4, 0, 0),(0, 0, 4, 6)]

---

su(2) ⟵ sp(11155) ⟵
so(22310) ⟵ su(22310)
su(3) ⟵

[{⟨1, 1⟩},{⟨22309, 1⟩}],[{⟨1, 1⟩}],[(22309)],[{⟨1, 1⟩}],[(91, 4),(4, 91)]

---

su(2) ⟵ sp(11160) ⟵
so(22320) ⟵ su(22320)
su(3) ⟵

[{⟨1, 1⟩},{⟨22319, 1⟩}],[{⟨1, 1⟩}],[(22319)],[{⟨1, 1⟩}],[(61, 9),(9, 61)]

---

su(2) ⟵
so(211) ⟵ so(22365) ⟵ su(22365)
sp(106) ⟵

[{⟨1, 1⟩},{⟨22364, 1⟩}],[{⟨1, 1⟩}],[(22364)],[{⟨1, 2⟩}],[{⟨2, 1⟩}]

---

su(2) ⟵ sp(11183) ⟵
so(212) ⟵ so(22366) ⟵
su(3) ⟵ su(22366)
su(211) ⟵
su(212) ⟵

[{⟨1, 1⟩},{⟨22365, 1⟩}],[{⟨1, 1⟩}],[(22365)],[{⟨1, 1⟩}],[{⟨2, 1⟩}], [(210, 0),(0, 210)], [{⟨1, 2⟩},{⟨210, 2⟩}],[{⟨2, 1⟩},{⟨210, 1⟩}]

---

su(2) ⟵ sp(11200) ⟵
so(22400) ⟵ su(22400)
su(3) ⟵

[{⟨1, 1⟩},{⟨22399, 1⟩}],[{⟨1, 1⟩}],[(22399)],[{⟨1, 1⟩}],[(49, 13),(13, 49)]

---

su(2) ⟵ sp(11210) ⟵
so(22420) ⟵ su(22420)
su(3) ⟵

[{⟨1, 1⟩},{⟨22419, 1⟩}],[{⟨1, 1⟩}],[(22419)],[{⟨1, 1⟩}],[(39, 18),(18, 39)]

---

su(2) ⟵ sp(11218) ⟵
so(22436) ⟵ su(22436)
su(3) ⟵

[{⟨1, 1⟩},{⟨22435, 1⟩}],[{⟨1, 1⟩}],[(22435)],[{⟨1, 1⟩}],[(70, 7),(7, 70)]

---

su(2) ⟵
sp(4) ⟵ sp(11232) ⟵
so(22464) ⟵ su(22464)
su(3) ⟵
su(4) ⟵

[{⟨1, 1⟩},{⟨22463, 1⟩}], [{⟨1, 1⟩}], [(22463)], [(2, 0, 1, 1)],[{⟨1, 1⟩}],[(103, 3),(3, 103)],[(3, 8, 2),(2, 8, 3)]

---

su(2) ⟵
su(150) ⟵ so(22499) ⟵ su(22499)
su(3) ⟵

[{⟨1, 1⟩},{⟨22498, 1⟩}], [{⟨1, 1⟩}], [(22498)], [{⟨1, 1⟩, ⟨149, 1⟩}],[(148, 1),(1, 148)]

---

su(2) ⟵ sp(11253) ⟵
so(22506) ⟵ su(22506)
su(3) ⟵

[{⟨1, 1⟩},{⟨22505, 1⟩}],[{⟨1, 1⟩}],[(22505)],[{⟨1, 1⟩}],[(120, 2),(2, 120)]

---

su(2) ⟵ so(22533) ⟵ su(22533)
su(3) ⟵

[{⟨1, 1⟩},{⟨22532, 1⟩}], [{⟨1, 1⟩}], [(22532)], [(36, 20),(20, 36)]

---

su(2) ⟵ sp(11286) ⟵
so(22572) ⟵ su(22572)
su(3) ⟵

[{⟨1, 1⟩},{⟨22571, 1⟩}],[{⟨1, 1⟩}],[(22571)],[{⟨1, 1⟩}],[(32, 23),(23, 32)]

---

su(2) ⟵
so(5) ⟵ so(22575) ⟵ su(22575)

[{⟨1, 1⟩},{⟨22574, 1⟩}],[{⟨1, 1⟩}],[(22574)],[(17, 6)]

---

su(2) ⟵
so(212) ⟵ so(22577) ⟵ su(22577)

[{⟨1, 1⟩},{⟨22576, 1⟩}],[{⟨1, 1⟩}],[(22576)],[{⟨1, 2⟩}]

---

su(2) ⟵ sp(11289) ⟵
so(213) ⟵
sp(106) ⟵ so(22578) ⟵
su(3) ⟵ su(22578)
su(212) ⟵
su(213) ⟵

[{⟨1, 1⟩},{⟨22577, 1⟩}],[{⟨1, 1⟩}],[(22577)],[{⟨1, 1⟩}],[{⟨2, 1⟩}], [{⟨1, 2⟩}], [(211, 0),(0, 211)], [{⟨1, 2⟩},{⟨211, 2⟩}],[{⟨2, 1⟩},{⟨211, 1⟩}]

---

su(2) ⟵ sp(11305) ⟵
so(22610) ⟵
su(4) ⟵ su(22610)
su(5) ⟵
su(20) ⟵

[{⟨1, 1⟩},{⟨22609, 1⟩}],[{⟨1, 1⟩}],[(22609)],[{⟨1, 1⟩}],[(11, 4, 1),(1, 4, 11)],[(16, 1, 0, 0),(0, 0, 1, 16)],[{⟨1, 1⟩, ⟨17, 1⟩},{⟨3, 1⟩, ⟨19, 1⟩}]

---

su(2) ⟵ sp(11310) ⟵
so(22620) ⟵ su(22620)
su(4) ⟵

[{⟨1, 1⟩},{⟨22619, 1⟩}],[{⟨1, 1⟩}],[(22619)],[{⟨1, 1⟩}],[(25, 2, 0),(0, 2, 25)]

---

su(2) ⟵ sp(11319) ⟵
so(22638) ⟵ su(22638)
su(3) ⟵
su(7) ⟵

[{⟨1, 1⟩},{⟨22637, 1⟩}],[{⟨1, 1⟩}],[(22637)],[{⟨1, 1⟩}],[(76, 6),(6, 76)],[{⟨1, 6⟩, ⟨6, 2⟩},{⟨1, 2⟩, ⟨6, 6⟩}]

---

su(2) ⟵ sp(11322) ⟵
so(22644) ⟵ su(22644)
su(4) ⟵
su(36) ⟵

[{⟨1, 1⟩},{⟨22643, 1⟩}],[{⟨1, 1⟩}],[(22643)],[{⟨1, 1⟩}],[(33, 1, 0),(0, 1, 33)], [{⟨1, 1⟩, ⟨34, 1⟩},{⟨2, 1⟩, ⟨35, 1⟩}]

---

su(2) ⟵ sp(11340) ⟵
so(8) ⟵ so(22680) ⟵
su(3) ⟵ su(22680)
su(3) ⟵
su(3) ⟵
su(8) ⟵

[{⟨1, 1⟩},{⟨22679, 1⟩}], [{⟨1, 1⟩}], [(22679)], [{⟨1, 1⟩}], [(3, 1, 2, 0),(3, 1, 0, 2),(2, 1, 3, 0),(2, 1, 0, 3),(0, 1, 3, 2),(0, 1, 2, 3)],[(41, 17),(17, 41)],[(47, 14),(14, 47)], [(83, 5),(5, 83)], [{⟨2, 1⟩, ⟨3, 1⟩, ⟨6, 1⟩},{⟨2, 1⟩, ⟨5, 1⟩, ⟨6, 1⟩}]

---

su(2) ⟵ so(22715) ⟵ su(22715)
su(3) ⟵

[{⟨1, 1⟩},{⟨22714, 1⟩}], [{⟨1, 1⟩}], [(22714)], [(58, 10),(10, 58)]

---

su(2) ⟵ so(22737) ⟵ su(22737)
su(3) ⟵

[{⟨1, 1⟩},{⟨22736, 1⟩}], [{⟨1, 1⟩}], [(22736)], [(52, 12),(12, 52)]

---

su(2) ⟵ sp(11375) ⟵
sp(3) ⟵ so(22750) ⟵ su(22750)
su(4) ⟵
su(4) ⟵

[{⟨1, 1⟩},{⟨22749, 1⟩}],[{⟨1, 1⟩}],[(22749)],[{⟨1, 1⟩}],[(4, 1, 2)],[(12, 1, 4),(4, 1, 12)],[(20, 3, 0),(0, 3, 20)]

---

su(2) ← sp(11385)
so(22770) ← su(22770)
su(4)

[{⟨1, 1⟩},{⟨22769, 1⟩}],[{⟨1, 1⟩}],[(22769)],[{⟨1, 1⟩}],[(21, 0, 3),(3, 0, 21)]

---

su(2) ← so(22785)
su(3)
su(22785)

[{⟨1, 1⟩},{⟨22784, 1⟩}], [{⟨1, 1⟩}], [(22784)], [(92, 4),(4, 92)]

---

su(2) ← sp(11395)
so(213), sp(107) → so(22790)
su(22790)

[{⟨1, 1⟩},{⟨22789, 1⟩}],[{⟨1, 1⟩}],[(22789)],[{⟨1, 1⟩}],[{⟨1, 2⟩}],[{⟨2, 1⟩}]

---

su(2), so(214) → so(22791)
su(3)
su(213)
su(214)
su(22791)

[{⟨1, 1⟩},{⟨22790, 1⟩}],[{⟨1, 1⟩}],[(22790)],[{⟨2, 1⟩}],[(212, 0),(0, 212)], [{⟨1, 2⟩},{⟨212, 2⟩}], [{⟨2, 1⟩},{⟨212, 1⟩}]

---

su(2) ← sp(11400)
su(151) ← so(22800)
su(3)
su(3)
su(22800)

[{⟨1, 1⟩},{⟨22799, 1⟩}],[{⟨1, 1⟩}],[(22799)],[{⟨1, 1⟩}],[{⟨1, 1⟩, ⟨150, 1⟩}], [(31, 24),(24, 31)], [(149, 1),(1, 149)]

---

su(2) ← sp(11407)
so(22814) ← su(22814)
su(3)

[{⟨1, 1⟩},{⟨22813, 1⟩}],[{⟨1, 1⟩}],[(22813)],[{⟨1, 1⟩}],[(43, 16),(16, 43)]

---

su(2) ← sp(11408)
so(22816) ← su(22816)
su(3)

[{⟨1, 1⟩},{⟨22815, 1⟩}],[{⟨1, 1⟩}],[(22815)],[{⟨1, 1⟩}],[(45, 15),(15, 45)]

---

su(2), sp(8) → sp(11424)
so(7) ← so(22848)
su(3)
su(22848)

[{⟨1, 1⟩},{⟨22847, 1⟩}], [{⟨1, 1⟩}], [(22847)], [{⟨1, 1⟩, ⟨4, 1⟩}],[{⟨1, 1⟩}],[(0, 6, 0)],[(55, 11),(11, 55)]

---

su(2) ← so(22869)
su(11)
su(22869)

[{⟨1, 1⟩},{⟨22868, 1⟩}], [{⟨1, 1⟩}], [(22868)], [{⟨1, 2⟩, ⟨2, 1⟩, ⟨10, 1⟩},{⟨1, 1⟩, ⟨9, 1⟩, ⟨10, 2⟩}]

---

su(2) ← so(22875)
su(3)
su(22875)

[{⟨1, 1⟩},{⟨22874, 1⟩}], [{⟨1, 1⟩}], [(22874)], [(121, 2),(2, 121)]

---

su(2), so(11) → sp(11440)
so(22880)
su(4)
su(11)
su(22880)

[{⟨1, 1⟩},{⟨22879, 1⟩}],[{⟨1, 1⟩}],[(22879)],[(4, 0, 0, 0, 1)], [{⟨1, 1⟩}], [(4, 7, 2),(2, 7, 4)], [{⟨1, 1⟩, ⟨2, 1⟩, ⟨9, 1⟩},{⟨2, 1⟩, ⟨9, 1⟩, ⟨10, 1⟩}]

---

su(2) ← sp(11445)
so(22890) ← su(22890)
su(3)

[{⟨1, 1⟩},{⟨22889, 1⟩}],[{⟨1, 1⟩}],[(22889)],[{⟨1, 1⟩}],[(104, 3),(3, 104)]

---

su(2) ← sp(11457)
so(22914) ← su(22914)
su(3)

[{⟨1, 1⟩},{⟨22913, 1⟩}],[{⟨1, 1⟩}],[(22913)],[{⟨1, 1⟩}],[(66, 8),(8, 66)]

---

su(2)
so(5) ← so(22919) ← su(22919)
so(41)

[{⟨1, 1⟩},{⟨22918, 1⟩}], [{⟨1, 1⟩}], [(22918)], [(1, 38)], [{⟨1, 1⟩, ⟨2, 1⟩}]

---

su(2) ← sp(11466)
so(9) ← so(22932)
su(22932)

[{⟨1, 1⟩},{⟨22931, 1⟩}],[{⟨1, 1⟩}],[(22931)],[{⟨1, 1⟩}],[(0, 4, 0, 0)]

---

su(2) ← sp(11480)
so(22960) ← su(22960)
su(41)

[{⟨1, 1⟩},{⟨22959, 1⟩}],[{⟨1, 1⟩}],[(22959)],[{⟨1, 1⟩}],[{⟨1, 1⟩, ⟨2, 1⟩},{⟨39, 1⟩, ⟨40, 1⟩}]

---

su(2) ← sp(11484)
so(22968) ← su(22968)
su(3)

[{⟨1, 1⟩},{⟨22967, 1⟩}],[{⟨1, 1⟩}],[(22967)],[{⟨1, 1⟩}],[(35, 21),(21, 35)]

---

su(2) ← so(22971)
su(3)
su(22971)

[{⟨1, 1⟩},{⟨22970, 1⟩}], [{⟨1, 1⟩}], [(22970)], [(30, 25),(25, 30)]

---

su(2) ← so(22995)
su(3)
su(22995)

[{⟨1, 1⟩},{⟨22994, 1⟩}], [{⟨1, 1⟩}], [(22994)], [(62, 9),(9, 62)]

---

su(2) ← sp(11500)
so(23) ← so(23000)
su(23000)

[{⟨1, 1⟩},{⟨22999, 1⟩}],[{⟨1, 1⟩}],[(22999)],[{⟨1, 1⟩}],[{⟨2, 2⟩}]

---

su(2) ← sp(11502)
so(214) ← so(23004)
su(23004)

[{⟨1, 1⟩},{⟨23003, 1⟩}],[{⟨1, 1⟩}],[(23003)],[{⟨1, 1⟩}],[{⟨1, 2⟩}]

---

su(2), so(215), sp(107) → so(23005)
su(3)
su(214)
su(215)
su(23005)

[{⟨1, 1⟩},{⟨23004, 1⟩}],[{⟨1, 1⟩}],[(23004)],[{⟨2, 1⟩}],[{⟨1, 2⟩}], [(213, 0),(0, 213)], [{⟨1, 2⟩},{⟨213, 2⟩}],[{⟨2, 1⟩},{⟨213, 1⟩}]

---

su(2) ← sp(11505)
so(23010) ← su(23010)
su(3)

[{⟨1, 1⟩},{⟨23009, 1⟩}],[{⟨1, 1⟩}],[(23009)],[{⟨1, 1⟩}],[(38, 19),(19, 38)]

---

su(2) ← sp(11520)
so(23040)
su(3)
su(4) ← su(23040)
su(4)
su(5)
so(10)

[{⟨1, 1⟩},{⟨23039, 1⟩}],[{⟨1, 1⟩}],[(23039)],[{⟨1, 1⟩}],[(71, 7),(7, 71)], [(5, 5, 3),(3, 5, 5)], [(9, 5, 1),(1, 5, 9)],[(3, 3, 0, 2),(2, 0, 3, 3)],[(1, 1, 0, 2, 0),(1, 1, 0, 0, 2)]

---

su(2)
su(18) ← so(23085)
so(5)
su(3) ← su(23085)
su(4)

[{⟨1, 1⟩},{⟨23084, 1⟩}], [{⟨1, 1⟩}], [(23084)], [{⟨2, 1⟩, ⟨16, 1⟩}],[(26, 2)],[(29, 26),(26, 29)],[(8, 8, 0),(0, 8, 8)]

---

su(2), sp(2) → sp(11550)
so(12) ← so(23100)
su(5)
su(5)
su(5) ← su(23100)
su(6)
su(6)
su(7)
su(12)

[{⟨1, 1⟩},{⟨23099, 1⟩}],[{⟨1, 1⟩}],[(23099)],[(13, 10)],[{⟨1, 1⟩}], [{⟨2, 3⟩}], [(1, 4, 2, 0),(0, 2, 4, 1)], [(2, 2, 3, 0),(0, 3, 2, 2)],[(8, 0, 0, 4),(4, 0, 0, 8)],[(5, 0, 2, 0, 0),(0, 0, 2, 0, 5)], [(9, 0, 0, 1, 0),(0, 1, 0, 0, 9)], [{⟨1, 3⟩, ⟨3, 2⟩},{⟨4, 2⟩, ⟨6, 3⟩}], [{⟨1, 3⟩, ⟨10, 1⟩},{⟨2, 1⟩, ⟨11, 3⟩}]

---

su(2), su(152) → so(23103)
su(3)
su(23103)

[{⟨1, 1⟩},{⟨23102, 1⟩}], [{⟨1, 1⟩}], [(23102)], [{⟨1, 1⟩, ⟨151, 1⟩}],[(150, 1),(1, 150)]

---

su(2) ← sp(11560)
su(17) ← so(23120)
su(23120)

[{⟨1, 1⟩},{⟨23119, 1⟩}],[{⟨1, 1⟩}],[(23119)],[{⟨1, 1⟩}],[{⟨1, 2⟩, ⟨16, 2⟩}]

---

su(2) ← sp(11571)
so(23142) ← su(23142)
su(3)

[{⟨1, 1⟩},{⟨23141, 1⟩}],[{⟨1, 1⟩}],[(23141)],[{⟨1, 1⟩}],[(28, 27),(27, 28)]

---

su(2) ← sp(11583)
so(5) ← so(23166) ← su(23166)
su(12)

[{⟨1, 1⟩},{⟨23165, 1⟩}],[{⟨1, 1⟩}],[(23165)],[{⟨1, 1⟩}],[(2, 32)],[{⟨2, 1⟩, ⟨4, 1⟩},{⟨8, 1⟩, ⟨10, 1⟩}]

---

su(2), so(5) → so(23205)
su(3)
su(3)
su(3) ← su(23205)
su(6)
su(13)

[{⟨1, 1⟩},{⟨23204, 1⟩}], [{⟨1, 1⟩}], [(23204)], [(8, 16)], [(50, 13),(13, 50)], [(77, 6),(6, 77)], [(84, 5),(5, 84)], [(11, 0, 0, 0, 1),(1, 0, 0, 0, 11)], [{⟨1, 4⟩, ⟨12, 1⟩},{⟨1, 1⟩, ⟨12, 4⟩}]

su(2), so(215), sp(108) ← so(23219) ← su(23219)

[{⟨1, 1⟩},{⟨23218, 1⟩}],[{⟨1, 1⟩}],[(23218)],[{⟨1, 2⟩}],[{⟨2, 1⟩}]

---

su(2) ← sp(11610)
so(216) ← so(23220)
sp(11610), so(23220), su(3), su(215), su(216) ← su(23220)

[{⟨1, 1⟩},{⟨23219, 1⟩}],[{⟨1, 1⟩}],[(23219)],[{⟨1, 1⟩}],[{⟨2, 1⟩}], [(214, 0),(0, 214)], [{⟨1, 2⟩},{⟨214, 2⟩}],[{⟨2, 1⟩},{⟨214, 1⟩}]

---

su(2) ← so(23247)
so(23247), su(3) ← su(23247)

[{⟨1, 1⟩},{⟨23246, 1⟩}], [{⟨1, 1⟩}], [(23246)], [(122, 2),(2, 122)]

---

su(2), sp(9) ← sp(11628)
sp(11628), so(23256) ← su(23256)

[{⟨1, 1⟩},{⟨23255, 1⟩}],[{⟨1, 1⟩}],[(23255)],[{⟨7, 1⟩}],[{⟨1, 1⟩}]

---

su(2) ← so(23265)
so(23265), su(3) ← su(23265)

[{⟨1, 1⟩},{⟨23264, 1⟩}], [{⟨1, 1⟩}], [(23264)], [(93, 4),(4, 93)]

---

su(2) ← sp(11638)
so(6) ← so(23276)
sp(11638), so(23276), su(23) ← su(23276)

[{⟨1, 1⟩},{⟨23275, 1⟩}],[{⟨1, 1⟩}],[(23275)],[{⟨1, 1⟩}],[(21, 0, 0)],[{⟨2, 2⟩},{⟨21, 2⟩}]

---

su(2), so(13), sp(2) ← sp(11648)
so(14) ← so(23296)
sp(11648), so(23296), su(4) ← su(23296)

[{⟨1, 1⟩},{⟨23295, 1⟩}], [{⟨1, 1⟩}], [(23295)], [{⟨1, 3⟩, ⟨6, 1⟩}],[(3, 23)],[{⟨1, 1⟩}],[{⟨1, 3⟩, ⟨2, 1⟩}],[(23, 1, 1),(1, 1, 23)]

---

su(2) ← sp(11660)
sp(11660), so(23320), su(3) ← su(23320)

[{⟨1, 1⟩},{⟨23319, 1⟩}],[{⟨1, 1⟩}],[(23319)],[{⟨1, 1⟩}],[(105, 3),(3, 105)]

---

su(2) ← sp(11664)
sp(11664), so(23328), su(9) ← su(23328)

[{⟨1, 1⟩},{⟨23327, 1⟩}],[{⟨1, 1⟩}],[(23327)],[{⟨1, 1⟩}],[{⟨1, 2⟩, ⟨3, 1⟩, ⟨8, 1⟩},{⟨1, 1⟩, ⟨6, 1⟩, ⟨8, 2⟩}]

---

su(2), so(5) ← so(23345)
so(23345), su(3) ← su(23345)

[{⟨1, 1⟩},{⟨23344, 1⟩}], [{⟨1, 1⟩}], [(23344)], [(5, 22)], [(34, 22),(22, 34)]

---

su(2) ← sp(11685)
sp(11685), so(23370), su(3) ← su(23370)

[{⟨1, 1⟩},{⟨23369, 1⟩}],[{⟨1, 1⟩}],[(23369)],[{⟨1, 1⟩}],[(40, 18),(18, 40)]

---

su(2), so(51) ← so(23375) ← su(23375)

[{⟨1, 1⟩},{⟨23374, 1⟩}],[{⟨1, 1⟩}],[(23374)],[{⟨1, 3⟩}]

---

su(2) ← sp(11700)
so(8), so(26) ← so(23400)
sp(11700), so(23400), su(4) ← su(23400)

[{⟨1, 1⟩},{⟨23399, 1⟩}],[{⟨1, 1⟩}],[(23399)],[{⟨1, 1⟩}],[(4, 2, 0, 0),(0, 2, 4, 0),(0, 2, 0, 4)], [{⟨1, 4⟩}], [(9, 2, 4),(4, 2, 9)]

---

su(2) ← sp(11704)
su(153) ← so(23408)
sp(11704), so(23408), su(3) ← su(23408)

[{⟨1, 1⟩},{⟨23407, 1⟩}],[{⟨1, 1⟩}],[(23407)],[{⟨1, 1⟩}],[{⟨1, 1⟩, ⟨152, 1⟩}],[(151, 1),(1, 151)]

---

su(2) ← sp(11713)
so(5), so(53) ← so(23426)
sp(11713), so(23426), su(4), su(51), su(53) ← su(23426)

[{⟨1, 1⟩},{⟨23425, 1⟩}],[{⟨1, 1⟩}],[(23425)],[{⟨1, 1⟩}],[(0, 50)], [{⟨3, 1⟩}], [(50, 0, 0),(0, 0, 50)], [{⟨1, 3⟩},{⟨50, 3⟩}],[{⟨3, 1⟩},{⟨50, 1⟩}]

---

su(2) ← sp(11715)
sp(11715), so(23430), su(3) ← su(23430)

[{⟨1, 1⟩},{⟨23429, 1⟩}],[{⟨1, 1⟩}],[(23429)],[{⟨1, 1⟩}],[(59, 10),(10, 59)]

---

su(2), so(216) ← so(23435) ← su(23435)

[{⟨1, 1⟩},{⟨23434, 1⟩}],[{⟨1, 1⟩}],[(23434)],[{⟨1, 2⟩}]

---

su(2) ← sp(11718)
so(217), sp(108) ← so(23436)
sp(11718), so(23436), su(3), su(4), su(216), su(217) ← su(23436)

[{⟨1, 1⟩},{⟨23435, 1⟩}],[{⟨1, 1⟩}],[(23435)],[{⟨1, 1⟩}],[{⟨2, 1⟩}],[{⟨1, 2⟩}],[(215, 0),(0, 215)],[(26, 0, 2),(2, 0, 26)],[{⟨1, 2⟩},{⟨215, 2⟩}],[{⟨2, 1⟩},{⟨215, 1⟩}]

---

su(2) ← so(23517)
so(23517), su(3) ← su(23517)

[{⟨1, 1⟩},{⟨23516, 1⟩}], [{⟨1, 1⟩}], [(23516)], [(53, 12),(12, 53)]

---

su(2) ← sp(11760)
sp(11760), so(23520), su(3), su(7), su(7) ← su(23520)

[{⟨1, 1⟩},{⟨23519, 1⟩}],[{⟨1, 1⟩}],[(23519)],[{⟨1, 1⟩}],[(48, 14),(14, 48)], [{⟨1, 1⟩, ⟨4, 3⟩},{⟨3, 3⟩, ⟨6, 1⟩}],[{⟨1, 1⟩, ⟨2, 1⟩, ⟨3, 2⟩},{⟨4, 2⟩, ⟨5, 1⟩, ⟨6, 1⟩}]

---

su(2) ← so(23541)
so(23541), su(3) ← su(23541)

[{⟨1, 1⟩},{⟨23540, 1⟩}], [{⟨1, 1⟩}], [(23540)], [(37, 20),(20, 37)]

---

su(2) ← sp(11781)
so(7), sp(3) ← so(23562)
sp(11781), so(23562), su(3) ← su(23562)

[{⟨1, 1⟩},{⟨23561, 1⟩}],[{⟨1, 1⟩}],[(23561)],[{⟨1, 1⟩}],[(2, 4, 0)],[(2, 5, 0)],[(67, 8),(8, 67)]

---

su(2), so(9), so(11), so(11) ← so(23595)
so(23595), su(5) ← su(23595)

[{⟨1, 1⟩},{⟨23594, 1⟩}], [{⟨1, 1⟩}], [(23594)], [(0, 0, 3, 0)], [(0, 0, 0, 2, 0)], [(0, 0, 1, 1, 0)], [(1, 8, 0, 0),(0, 0, 8, 1)]

---

su(2) ← sp(11799)
sp(11799), so(23598), su(3) ← su(23598)

[{⟨1, 1⟩},{⟨23597, 1⟩}],[{⟨1, 1⟩}],[(23597)],[{⟨1, 1⟩}],[(56, 11),(11, 56)]

---

su(2) ← sp(11803)
so(5) ← so(23606)
sp(11803), so(23606) ← su(23606)

[{⟨1, 1⟩},{⟨23605, 1⟩}],[{⟨1, 1⟩}],[(23605)],[{⟨1, 1⟩}],[(3, 28)]

---

su(2) ← so(23607)
so(23607), su(3) ← su(23607)

[{⟨1, 1⟩},{⟨23606, 1⟩}], [{⟨1, 1⟩}], [(23606)], [(42, 17),(17, 42)]

---

su(2) ← sp(11811)
sp(11811), so(23622), su(3) ← su(23622)

[{⟨1, 1⟩},{⟨23621, 1⟩}],[{⟨1, 1⟩}],[(23621)],[{⟨1, 1⟩}],[(123, 2),(2, 123)]

---

su(2), so(7) ← so(23625) ← su(23625)

[{⟨1, 1⟩},{⟨23624, 1⟩}],[{⟨1, 1⟩}],[(23624)],[(2, 1, 4)]

---

su(2) ← sp(11826)
so(217), sp(109) ← so(23652)
sp(11826), so(23652), su(3) ← su(23652)

[{⟨1, 1⟩},{⟨23651, 1⟩}],[{⟨1, 1⟩}],[(23651)],[{⟨1, 1⟩}],[{⟨1, 2⟩}],[{⟨2, 1⟩}],[(72, 7),(7, 72)]

---

su(2), so(218) ← so(23653)
so(23653), su(3), su(217), su(218) ← su(23653)

[{⟨1, 1⟩},{⟨23652, 1⟩}],[{⟨1, 1⟩}],[(23652)],[{⟨2, 1⟩}],[(216, 0),(0, 216)], [{⟨1, 2⟩},{⟨216, 2⟩}], [{⟨2, 1⟩},{⟨216, 1⟩}]

---

su(2) ← sp(11830)
so(13) ← so(23660)
sp(11830), so(23660) ← su(23660)

[{⟨1, 1⟩},{⟨23659, 1⟩}],[{⟨1, 1⟩}],[(23659)],[{⟨1, 1⟩}],[{⟨3, 2⟩}]

---

su(2) ← sp(11832)
sp(11832), so(23664), su(3) ← su(23664)

[{⟨1, 1⟩},{⟨23663, 1⟩}],[{⟨1, 1⟩}],[(23663)],[{⟨1, 1⟩}],[(33, 23),(23, 33)]

---

su(2) ← sp(11840)
sp(11840), so(23680), su(3) ← su(23680)

[{⟨1, 1⟩},{⟨23679, 1⟩}],[{⟨1, 1⟩}],[(23679)],[{⟨1, 1⟩}],[(63, 9),(9, 63)]

---

su(2) ← sp(11844)
sp(11844), so(23688), su(3) ← su(23688)

[{⟨1, 1⟩},{⟨23687, 1⟩}],[{⟨1, 1⟩}],[(23687)],[{⟨1, 1⟩}],[(46, 15),(15, 46)]

su(2)
su(154)
so(23715)
su(3)
su(3)
su(23715)

[{⟨1, 1⟩},{⟨23714, 1⟩}], [{⟨1, 1⟩}], [(23714)], [{⟨1, 1⟩, ⟨153, 1⟩}],[(44, 16),(16, 44)],[(152, 1),(1, 152)]

---

su(2) ← sp(11868)
so(23736)
su(3)
su(23736)

[{⟨1, 1⟩},{⟨23735, 1⟩}],[{⟨1, 1⟩}],[(23735)],[{⟨1, 1⟩}], [(85, 5),(5, 85)]

---

su(2) ← sp(11875)
so(23750)
su(3)
su(4)
su(23750)

[{⟨1, 1⟩},{⟨23749, 1⟩}],[{⟨1, 1⟩}],[(23749)],[{⟨1, 1⟩}], [(94, 4),(4, 94)],[(18, 0, 4),(4, 0, 18)]

---

su(2)
so(29)
sp(13)
so(23751)
su(5)
su(26)
su(29)
su(23751)

[{⟨1, 1⟩},{⟨23750, 1⟩}],[{⟨1, 1⟩}],[(23750)],[{⟨4, 1⟩}], [{⟨1, 4⟩}], [(25, 0, 0, 0),(0, 0, 0, 25)], [{⟨1, 4⟩}, {⟨25, 4⟩}],[{⟨4, 1⟩},{⟨25, 1⟩}]

---

su(2) ← sp(11877)
so(23754)
su(3)
su(23754)

[{⟨1, 1⟩},{⟨23753, 1⟩}],[{⟨1, 1⟩}],[(23753)],[{⟨1, 1⟩}], [(106, 3),(3, 106)]

---

su(2) ← sp(11880)
so(23760)
su(5)
su(9)
su(9)
so(10)
su(23760)

[{⟨1, 1⟩},{⟨23759, 1⟩}],[{⟨1, 1⟩}],[(23759)],[{⟨1, 1⟩}], [(2, 1, 3, 1),(1, 3, 1, 2)], [{⟨1, 1⟩, ⟨2, 1⟩, ⟨5, 1⟩},{⟨4, 1⟩, ⟨7, 1⟩, ⟨8, 1⟩}], [{⟨1, 1⟩, ⟨2, 3⟩},{⟨7, 3⟩, ⟨8, 1⟩}], [(2, 0, 0, 3, 0),(2, 0, 0, 0, 3)]

---

su(2) ← so(23779)
su(3)
su(23779)

[{⟨1, 1⟩},{⟨23778, 1⟩}], [{⟨1, 1⟩}], [(23778)], [(78, 6), (6, 78)]

---

su(2)
sp(2)
sp(11900)
so(23800)
su(4)
su(23800)

[{⟨1, 1⟩},{⟨23799, 1⟩}], [{⟨1, 1⟩}], [(23799)], [(7, 16)], [{⟨1, 1⟩}],[(6, 7, 1),(1, 7, 6)]

---

su(2)
so(5)
so(23821) ← su(23821)

[{⟨1, 1⟩},{⟨23820, 1⟩}],[{⟨1, 1⟩}],[(23820)],[(40, 0)]

---

su(2) ← sp(11934)
so(9) ← so(23868)
su(23868)

[{⟨1, 1⟩},{⟨23867, 1⟩}],[{⟨1, 1⟩}],[(23867)],[{⟨1, 1⟩}], [(3, 2, 0, 0)]

---

su(2) ← sp(11935)
so(218) ← so(23870)
su(23870)

[{⟨1, 1⟩},{⟨23869, 1⟩}],[{⟨1, 1⟩}],[(23869)],[{⟨1, 1⟩}], [{⟨1, 2⟩}]

---

su(2)
so(219)
sp(109)
so(23871)
su(3)
su(218)
su(219)
su(23871)

[{⟨1, 1⟩},{⟨23870, 1⟩}],[{⟨1, 1⟩}],[(23870)],[{⟨2, 1⟩}], [{⟨1, 2⟩}], [(217, 0),(0, 217)], [{⟨1, 2⟩},{⟨217, 2⟩}], [{⟨2, 1⟩},{⟨217, 1⟩}]

---

su(2)
sp(2)
sp(11960)
so(23920)
su(23920)

[{⟨1, 1⟩},{⟨23919, 1⟩}], [{⟨1, 1⟩}], [(23919)], [(5, 19)], [{⟨1, 1⟩}]

---

su(2) ← so(23925)
su(3)
su(23925)

[{⟨1, 1⟩},{⟨23924, 1⟩}], [{⟨1, 1⟩}], [(23924)], [(32, 24), (24, 32)]

---

su(2)
sp(2)
sp(11968)
so(23936)
su(23936)

[{⟨1, 1⟩},{⟨23935, 1⟩}], [{⟨1, 1⟩}], [(23935)], [(1, 31)], [{⟨1, 1⟩}]

---

su(2) ← sp(11970)
so(5) ← so(23940)
su(4)
su(4)
su(4)
su(4)
su(4)
su(4)
su(4)
su(36)
su(23940)

[{⟨1, 1⟩},{⟨23939, 1⟩}],[{⟨1, 1⟩}],[(23939)],[{⟨1, 1⟩}], [(7, 18)],[(1, 17, 0),(0, 17, 1)],[(3, 13, 0),(0, 13, 3)],[(9, 1, 6),(6, 1, 9)], [(11, 2, 3),(3, 2, 11)], [(14, 3, 1),(1, 3, 14)],[(18, 1, 2),(2, 1, 18)],[(34, 0, 1),(1, 0, 34)],[{⟨1, 2⟩, ⟨35, 1⟩},{⟨1, 1⟩, ⟨35, 2⟩}]

---

su(2) ← sp(12000)
so(24000)
su(3)
su(3)
su(24000)

[{⟨1, 1⟩},{⟨23999, 1⟩}],[{⟨1, 1⟩}],[(23999)],[{⟨1, 1⟩}], [(39, 19),(19, 39)],[(124, 2),(2, 124)]

---

su(2) ← sp(12005)
so(5) ← so(24010)
su(24010)

[{⟨1, 1⟩},{⟨24009, 1⟩}],[{⟨1, 1⟩}],[(24009)],[{⟨1, 1⟩}], [(6, 20)]

---

su(2) ← so(24013)
su(3)
su(24013)

[{⟨1, 1⟩},{⟨24012, 1⟩}], [{⟨1, 1⟩}], [(24012)], [(36, 21), (21, 36)]

---

su(2) ← sp(12012)
su(155)
so(7)
so(7)
sp(3)
so(8)
so(8)
so(14)
so(14)
so(24024)
su(3)
su(3)
su(4)
su(5)
su(5)
su(6)
su(6)
su(7)
su(10)
su(24024)

[{⟨1, 1⟩},{⟨24023, 1⟩}],[{⟨1, 1⟩}],[(24023)],[{⟨1, 1⟩}], [{⟨1, 1⟩, ⟨154, 1⟩}], [(6, 1, 1)], [(10, 0, 1)], [(1, 2, 3)], [(6, 0, 2, 0),(6, 0, 0, 2),(2, 0, 6, 0),(2, 0, 0, 6),(0, 0, 6, 2),(0, 0, 2, 6)], [(8, 0, 1, 0),(8, 0, 0, 1),(1, 0, 8, 0),(1, 0, 0, 8),(0, 0, 8, 1),(0, 0, 1, 8)], [{⟨1, 1⟩, ⟨5, 1⟩}], [{⟨1, 1⟩, ⟨2, 2⟩}],[(51, 13),(13, 51)],[(153, 1),(1, 153)], [(12, 0, 7),(7, 0, 12)], [(3, 6, 0, 0),(0, 0, 6, 3)], [(6, 1, 1, 1),(1, 1, 1, 6)], [(6, 0, 0, 1, 1),(1, 1, 0, 0, 6)], [(7, 2, 0, 0, 0),(0, 0, 0, 2, 7)], [{⟨1, 6⟩, ⟨4, 1⟩},{⟨3, 1⟩, ⟨6, 6⟩}], [{⟨1, 3⟩, ⟨7, 1⟩},{⟨3, 1⟩, ⟨9, 3⟩}]

---

su(2) ← sp(12025)
so(5) ← so(24050)
su(24050)

[{⟨1, 1⟩},{⟨24049, 1⟩}],[{⟨1, 1⟩}],[(24049)],[{⟨1, 1⟩}], [(11, 12)]

---

su(2)
so(219)
sp(110)
so(24089) ← su(24089)

[{⟨1, 1⟩},{⟨24088, 1⟩}],[{⟨1, 1⟩}],[(24088)],[{⟨1, 2⟩}], [{⟨2, 1⟩}]

---

su(2) ← sp(12045)
so(220) ← so(24090)
su(3)
su(219)
su(220)
su(24090)

[{⟨1, 1⟩},{⟨24089, 1⟩}],[{⟨1, 1⟩}],[(24089)],[{⟨1, 1⟩}], [{⟨2, 1⟩}], [(218, 0),(0, 218)], [{⟨1, 2⟩},{⟨218, 2⟩}], [{⟨2, 1⟩},{⟨218, 1⟩}]

---

su(2) ← sp(12064)
so(24128)
su(3)
su(24128)

[{⟨1, 1⟩},{⟨24127, 1⟩}],[{⟨1, 1⟩}],[(24127)],[{⟨1, 1⟩}], [(31, 25),(25, 31)]

---

su(2) ← sp(12078)
so(24156)
su(3)
su(24156)

[{⟨1, 1⟩},{⟨24155, 1⟩}],[{⟨1, 1⟩}],[(24155)],[{⟨1, 1⟩}], [(60, 10),(10, 60)]

---

su(2)
sp(2)
sp(12090)
so(24180)
su(24180)

[{⟨1, 1⟩},{⟨24179, 1⟩}], [{⟨1, 1⟩}], [(24179)], [(25, 4)], [{⟨1, 1⟩}]

---

su(2) ←, sp(3) ←, sp(3) ← sp(12096), sp(3) ←, sp(7) ←; so(9) ←, so(16) ← so(24192), g2 ←; su(3) ←, su(7) ← — su(24192)

[{⟨1, 1⟩},{⟨24191, 1⟩}],[{⟨1, 1⟩}],[(24191)],[(1, 3, 2)],[(7, 0, 2)],[(11, 1, 0)],[{⟨1, 3⟩, ⟨2, 1⟩}],[{⟨1, 1⟩}],[(1, 2, 0, 1)], [{⟨1, 1⟩, ⟨4, 1⟩}], [(11, 1)], [(107, 3),(3, 107)], [{⟨1, 3⟩, ⟨2, 1⟩, ⟨6, 2⟩},{⟨1, 2⟩, ⟨5, 1⟩, ⟨6, 3⟩}]

---

su(2) ← sp(12100); su(11), so(6) ← so(24200) — su(24200)

[{⟨1, 1⟩},{⟨24199, 1⟩}],[{⟨1, 1⟩}],[(24199)],[{⟨1, 1⟩}],[{⟨3, 1⟩, ⟨8, 1⟩}],[(5, 4, 4)]

---

su(2) ← so(24219); su(3) ← — su(24219)

[{⟨1, 1⟩},{⟨24218, 1⟩}], [{⟨1, 1⟩}], [(24218)], [(68, 8),(8, 68)]

---

su(2) ← sp(12120); so(24240) ←; su(3) ← — su(24240)

[{⟨1, 1⟩},{⟨24239, 1⟩}],[{⟨1, 1⟩}],[(24239)],[{⟨1, 1⟩}],[(95, 4),(4, 95)]

---

su(2), su(8), so(5) ← so(24255); su(4) ←, su(5) ←, su(6) ←, su(6) ←, su(7) ← — su(24255)

[{⟨1, 1⟩},{⟨24254, 1⟩}], [{⟨1, 1⟩}], [(24254)], [{⟨1, 1⟩, ⟨2, 1⟩, ⟨6, 1⟩, ⟨7, 1⟩}], [(21, 4)], [(14, 5, 0),(0, 5, 14)], [(1, 4, 1, 1),(1, 1, 4, 1)],[(3, 1, 0, 1, 1),(1, 1, 0, 1, 3)],[(3, 2, 1, 0, 0),(0, 0, 1, 2, 3)],[{⟨1, 3⟩, ⟨2, 1⟩, ⟨4, 1⟩},{⟨3, 1⟩, ⟨5, 1⟩, ⟨6, 3⟩}]

---

su(2) ← sp(12136); so(24272) ←; su(3) ← — su(24272)

[{⟨1, 1⟩},{⟨24271, 1⟩}],[{⟨1, 1⟩}],[(24271)],[{⟨1, 1⟩}],[(73, 7),(7, 73)]

---

su(2) ← so(24273); su(3) ←, su(3) ← — su(24273)

[{⟨1, 1⟩},{⟨24272, 1⟩}], [{⟨1, 1⟩}], [(24272)], [(30, 26),(26, 30)],[(86, 5),(5, 86)]

---

su(2), so(220) ← so(24309) ← su(24309)

[{⟨1, 1⟩},{⟨24308, 1⟩}],[{⟨1, 1⟩}],[(24308)],[{⟨1, 2⟩}]

---

su(2) ← sp(12155); so(17), so(221), sp(5), sp(6), sp(110) ← so(24310); su(3) ←, su(3) ←, su(4) ←, su(5) ←, su(9) ←, su(10) ←, su(17) ←, su(220) ←, su(221) ←, so(18) ← — su(24310)

[{⟨1, 1⟩},{⟨24309, 1⟩}],[{⟨1, 1⟩}],[(24309)],[{⟨1, 1⟩}],[{⟨8, 2⟩}], [{⟨2, 1⟩}], [(8, 0, 0, 0, 0)], [{⟨2, 3⟩}],[{⟨1, 2⟩}],[(54, 12),(12, 54)],[(219, 0),(0, 219)],[(3, 10, 1),(1, 10, 3)], [(10, 0, 0, 3),(3, 0, 0, 10)], [{⟨1, 9⟩},{⟨8, 9⟩}], [{⟨1, 8⟩},{⟨9, 8⟩}], [{⟨8, 1⟩},{⟨9, 1⟩}], [{⟨1, 2⟩},{⟨219, 2⟩}], [{⟨2, 1⟩},{⟨219, 1⟩}], [{⟨8, 2⟩},{⟨9, 2⟩}]

---

su(2), $\mathfrak{c}_7$ ← sp(12160); so(24320) — su(24320)

[{⟨1, 1⟩},{⟨24319, 1⟩}],[{⟨1, 1⟩}],[(24319)],[{⟨7, 3⟩}],[{⟨1, 1⟩}]

---

su(2), su(156) ← so(24335); su(3) ← — su(24335)

[{⟨1, 1⟩},{⟨24334, 1⟩}], [{⟨1, 1⟩}], [(24334)], [{⟨1, 1⟩, ⟨155, 1⟩}],[(154, 1),(1, 154)]

---

su(2) ← so(24339); su(3) ← — su(24339)

[{⟨1, 1⟩},{⟨24338, 1⟩}], [{⟨1, 1⟩}], [(24338)], [(41, 18),(18, 41)]

---

su(2) ← sp(12180); so(24360) ←; su(3) ←, su(3) ←, su(3) ← — su(24360)

[{⟨1, 1⟩},{⟨24359, 1⟩}],[{⟨1, 1⟩}],[(24359)],[{⟨1, 1⟩}],[(29, 27),(27, 29)],[(57, 11),(11, 57)],[(79, 6),(6, 79)]

---

su(2), so(7) ← so(24375); su(3) ←, su(3) ← — su(24375)

[{⟨1, 1⟩},{⟨24374, 1⟩}],[{⟨1, 1⟩}],[(24374)],[(9, 1, 0)],[(49, 14),(14, 49)],[(64, 9),(9, 64)]

---

su(2) ← so(24381); su(3) ← — su(24381)

[{⟨1, 1⟩},{⟨24380, 1⟩}], [{⟨1, 1⟩}], [(24380)], [(125, 2),(2, 125)]

---

su(2), su(3) ← so(24389) ← su(24389)

[{⟨1, 1⟩},{⟨24388, 1⟩}],[{⟨1, 1⟩}],[(24388)],[(28, 28)]

---

su(2) ← sp(12213); so(24426) ←; su(3) ← — su(24426)

[{⟨1, 1⟩},{⟨24425, 1⟩}],[{⟨1, 1⟩}],[(24425)],[{⟨1, 1⟩}],[(35, 22),(22, 35)]

---

su(2) ← sp(12240); so(24480) ←; su(4) ← — su(24480)

[{⟨1, 1⟩},{⟨24479, 1⟩}],[{⟨1, 1⟩}],[(24479)],[{⟨1, 1⟩}],[(7, 3, 4),(4, 3, 7)]

---

su(2) ← sp(12250); su(7) ← so(24500) — su(24500)

[{⟨1, 1⟩},{⟨24499, 1⟩}],[{⟨1, 1⟩}],[(24499)],[{⟨1, 1⟩}],[{⟨1, 1⟩, ⟨3, 1⟩, ⟨4, 1⟩, ⟨6, 1⟩}]

---

su(2) ← sp(12265); so(221), sp(111) ← so(24530) — su(24530)

[{⟨1, 1⟩},{⟨24529, 1⟩}],[{⟨1, 1⟩}],[(24529)],[{⟨1, 1⟩}],[{⟨1, 2⟩}],[{⟨2, 1⟩}]

---

su(2), so(222) ← so(24531); su(3) ←, su(221) ←, su(222) ← — su(24531)

[{⟨1, 1⟩},{⟨24530, 1⟩}],[{⟨1, 1⟩}],[(24530)],[{⟨2, 1⟩}],[(220, 0),(0, 220)], [{⟨1, 2⟩},{⟨220, 2⟩}], [{⟨2, 1⟩},{⟨220, 1⟩}]

---

su(2) ← sp(12276); so(24552) ←; su(3) ← — su(24552)

[{⟨1, 1⟩},{⟨24551, 1⟩}],[{⟨1, 1⟩}],[(24551)],[{⟨1, 1⟩}],[(43, 17),(17, 43)]

---

su(2), sp(7) ← sp(12285); so(7) ← so(24570); su(3) ←, su(5) ←, su(5) ← — su(24570)

[{⟨1, 1⟩},{⟨24569, 1⟩}], [{⟨1, 1⟩}], [(24569)], [{⟨1, 1⟩, ⟨2, 2⟩}], [{⟨1, 1⟩}], [(0, 4, 2)], [(38, 20),(20, 38)], [(5, 2, 0, 2),(2, 0, 2, 5)],[(6, 1, 2, 0),(0, 2, 1, 6)]

---

su(2) ← sp(12288); su(5), so(7), so(6) ← so(24576); su(3) ← — su(24576)

[{⟨1, 1⟩},{⟨24575, 1⟩}],[{⟨1, 1⟩}],[(24575)],[{⟨1, 1⟩}],[(3, 1, 1, 3)],[(3, 1, 3)],[(7, 3, 3)],[(47, 15),(15, 47)]

---

su(2) ← sp(12300); so(5) ← so(24600) — su(24600)

[{⟨1, 1⟩},{⟨24599, 1⟩}],[{⟨1, 1⟩}],[(24599)],[{⟨1, 1⟩}],[(15, 8)]

---

su(2) ← so(24605); su(4) ←, su(37) ← — su(24605)

[{⟨1, 1⟩},{⟨24604, 1⟩}],[{⟨1, 1⟩}],[(24604)],[(34, 1, 0),(0, 1, 34)],[{⟨1, 1⟩, ⟨35, 1⟩},{⟨2, 1⟩, ⟨36, 1⟩}]

---

su(2) ← so(24633); su(3) ← — su(24633)

[{⟨1, 1⟩},{⟨24632, 1⟩}], [{⟨1, 1⟩}], [(24632)], [(45, 16),(16, 45)]

---

su(2) ← sp(12317); so(24634) ←; su(3) ← — su(24634)

[{⟨1, 1⟩},{⟨24633, 1⟩}],[{⟨1, 1⟩}],[(24633)],[{⟨1, 1⟩}],[(108, 3),(3, 108)]

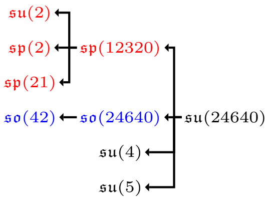


[{⟨1, 1⟩},{⟨24639, 1⟩}], [{⟨1, 1⟩}], [(24639)], [(39, 1)], [{⟨1, 1⟩, ⟨2, 1⟩}], [{⟨1, 1⟩}], [{⟨1, 1⟩, ⟨2, 1⟩}], [(4, 6, 3), (3, 6, 4)],[(10, 0, 1, 1),(1, 1, 0, 10)]

---

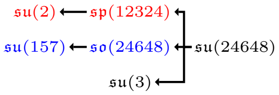


[{⟨1, 1⟩},{⟨24647, 1⟩}],[{⟨1, 1⟩}],[(24647)],[{⟨1, 1⟩}], [{⟨1, 1⟩, ⟨156, 1⟩}],[(155, 1),(1, 155)]

---

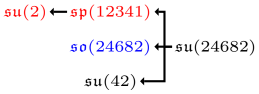


[{⟨1, 1⟩},{⟨24681, 1⟩}],[{⟨1, 1⟩}],[(24681)],[{⟨1, 1⟩}], [{⟨1, 1⟩, ⟨2, 1⟩},{⟨40, 1⟩, ⟨41, 1⟩}]

---

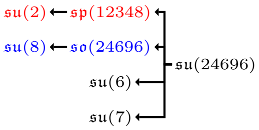


[{⟨1, 1⟩},{⟨24695, 1⟩}],[{⟨1, 1⟩}],[(24695)],[{⟨1, 1⟩}], [{⟨4, 3⟩}], [(5, 0, 0, 0, 4),(4, 0, 0, 0, 5)], [{⟨3, 4⟩},{⟨4, 4⟩}]

---

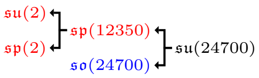


[{⟨1, 1⟩},{⟨24699, 1⟩}],[{⟨1, 1⟩}],[(24699)],[(11, 12)], [{⟨1, 1⟩}]

---

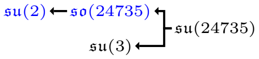


[{⟨1, 1⟩},{⟨24734, 1⟩}], [{⟨1, 1⟩}], [(24734)], [(96, 4), (4, 96)]

---

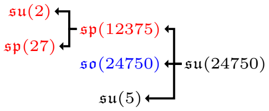


[{⟨1, 1⟩},{⟨24749, 1⟩}],[{⟨1, 1⟩}],[(24749)],[{⟨3, 1⟩}], [{⟨1, 1⟩}],[(1, 2, 4, 0),(0, 4, 2, 1)]

---

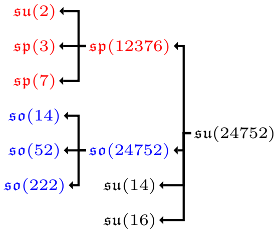


[{⟨1, 1⟩},{⟨24751, 1⟩}],[{⟨1, 1⟩}],[(24751)],[(2, 0, 5)], [{⟨1, 2⟩, ⟨3, 1⟩}], [{⟨1, 1⟩}], [{⟨1, 6⟩}], [{⟨1, 3⟩}], [{⟨1, 2⟩}], [{⟨1, 3⟩, ⟨2, 1⟩},{⟨12, 1⟩, ⟨13, 3⟩}], [{⟨1, 1⟩, ⟨4, 1⟩},{⟨12, 1⟩, ⟨15, 1⟩}]

---

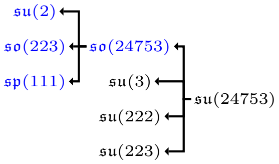


[{⟨1, 1⟩},{⟨24752, 1⟩}],[{⟨1, 1⟩}],[(24752)],[{⟨2, 1⟩}], [{⟨1, 2⟩}], [(221, 0),(0, 221)], [{⟨1, 2⟩},{⟨221, 2⟩}], [{⟨2, 1⟩},{⟨221, 1⟩}]

---

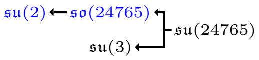


[{⟨1, 1⟩},{⟨24764, 1⟩}], [{⟨1, 1⟩}], [(24764)], [(126, 2), (2, 126)]

---

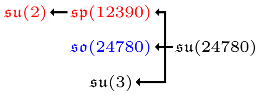


[{⟨1, 1⟩},{⟨24779, 1⟩}],[{⟨1, 1⟩}],[(24779)],[{⟨1, 1⟩}], [(34, 23),(23, 34)]

---

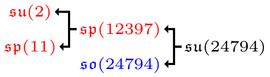


[{⟨1, 1⟩},{⟨24793, 1⟩}],[{⟨1, 1⟩}],[(24793)],[{⟨5, 1⟩}], [{⟨1, 1⟩}]

---

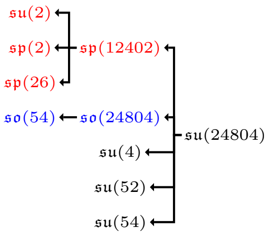


[{⟨1, 1⟩},{⟨24803, 1⟩}], [{⟨1, 1⟩}], [(24803)], [(51, 0)], [{⟨1, 3⟩}], [{⟨1, 1⟩}], [{⟨3, 1⟩}], [(51, 0, 0),(0, 0, 51)], [{⟨1, 3⟩},{⟨51, 3⟩}],[{⟨3, 1⟩},{⟨51, 1⟩}]

---

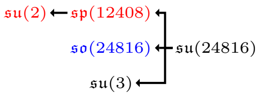


[{⟨1, 1⟩},{⟨24815, 1⟩}],[{⟨1, 1⟩}],[(24815)],[{⟨1, 1⟩}], [(87, 5),(5, 87)]

---

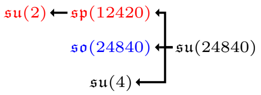


[{⟨1, 1⟩},{⟨24839, 1⟩}],[{⟨1, 1⟩}],[(24839)],[{⟨1, 1⟩}], [(17, 4, 0),(0, 4, 17)]

---

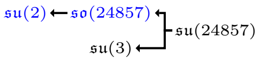


[{⟨1, 1⟩},{⟨24856, 1⟩}], [{⟨1, 1⟩}], [(24856)], [(52, 13), (13, 52)]

---

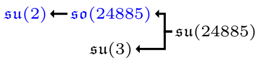


[{⟨1, 1⟩},{⟨24884, 1⟩}], [{⟨1, 1⟩}], [(24884)], [(69, 8), (8, 69)]

---

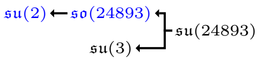


[{⟨1, 1⟩},{⟨24892, 1⟩}], [{⟨1, 1⟩}], [(24892)], [(61, 10), (10, 61)]

---

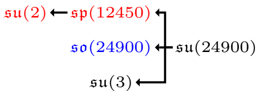


[{⟨1, 1⟩},{⟨24899, 1⟩}],[{⟨1, 1⟩}],[(24899)],[{⟨1, 1⟩}], [(74, 7),(7, 74)]

---

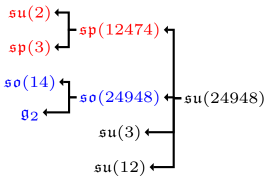


[{⟨1, 1⟩},{⟨24947, 1⟩}],[{⟨1, 1⟩}],[(24947)],[(1, 6, 0)], [{⟨1, 1⟩}], [{⟨1, 2⟩, ⟨3, 1⟩}], [(5, 4)], [(80, 6),(6, 80)], [{⟨1, 1⟩, ⟨3, 1⟩, ⟨11, 1⟩},{⟨1, 1⟩, ⟨9, 1⟩, ⟨11, 1⟩}]

---

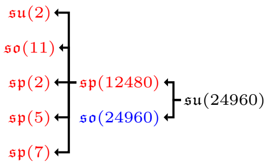


[{⟨1, 1⟩},{⟨24959, 1⟩}],[{⟨1, 1⟩}],[(24959)],[(0, 2, 0, 0, 1)],[(15, 9)],[(3, 0, 0, 1, 0)],[{⟨1, 1⟩, ⟨6, 1⟩}],[{⟨1, 1⟩}]

---

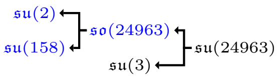


[{⟨1, 1⟩},{⟨24962, 1⟩}], [{⟨1, 1⟩}], [(24962)], [{⟨1, 1⟩, ⟨157, 1⟩}],[(156, 1),(1, 156)]

---

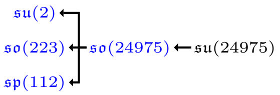


[{⟨1, 1⟩},{⟨24974, 1⟩}],[{⟨1, 1⟩}],[(24974)],[{⟨1, 2⟩}], [{⟨2, 1⟩}]

---

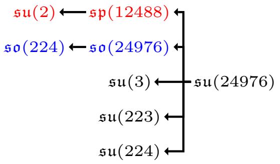


[{⟨1, 1⟩},{⟨24975, 1⟩}],[{⟨1, 1⟩}],[(24975)],[{⟨1, 1⟩}], [{⟨2, 1⟩}], [(222, 0),(0, 222)], [{⟨1, 2⟩},{⟨222, 2⟩}], [{⟨2, 1⟩},{⟨222, 1⟩}]

---

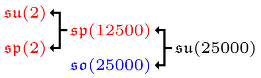


[{⟨1, 1⟩},{⟨24999, 1⟩}], [{⟨1, 1⟩}], [(24999)], [(9, 14)], [{⟨1, 1⟩}]

---

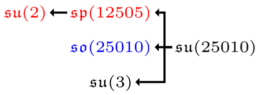


[{⟨1, 1⟩},{⟨25009, 1⟩}],[{⟨1, 1⟩}],[(25009)],[{⟨1, 1⟩}], [(40, 19),(19, 40)]

---

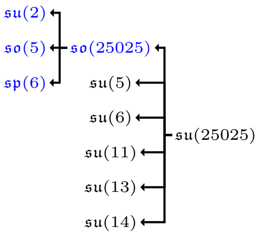


[{⟨1, 1⟩},{⟨25024, 1⟩}],[{⟨1, 1⟩}],[(25024)],[(13, 10)], [{⟨1, 2⟩, ⟨4, 1⟩}], [(5, 3, 0, 1),(1, 0, 3, 5)], [(9, 0, 1, 0, 0), (0, 0, 1, 0, 9)], [{⟨1, 4⟩, ⟨2, 1⟩},{⟨9, 1⟩, ⟨10, 4⟩}], [{⟨1, 2⟩, ⟨10, 1⟩},{⟨3, 1⟩, ⟨12, 2⟩}], [{⟨1, 1⟩, ⟨5, 1⟩}, {⟨9, 1⟩, ⟨13, 1⟩}]

---

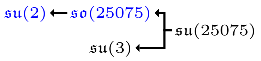


[{⟨1, 1⟩},{⟨25074, 1⟩}], [{⟨1, 1⟩}], [(25074)], [(33, 24), (24, 33)]

su(2) ⟵ sp(12540)
so(25080)
su(3)
su(3)
su(3)
su(4) — su(25080)
su(4)
su(4)
su(4)
su(5)
su(19)

[{⟨1, 1⟩},{⟨25079, 1⟩}],[{⟨1, 1⟩}],[(25079)],[{⟨1, 1⟩}], [(37, 21),(21, 37)], [(65, 9),(9, 65)], [(109, 3),(3, 109)], [(7, 9, 0),(0, 9, 7)], [(8, 1, 7),(7, 1, 8)], [(10, 7, 0),(0, 7, 10)], [(18, 2, 1),(1, 2, 18)], [(17, 0, 0, 1),(1, 0, 0, 17)], [{⟨1, 3⟩, ⟨18, 1⟩},{⟨1, 1⟩, ⟨18, 3⟩}]

---

su(2) ⟵ sp(12555)
so(25110) ⟵ su(25110)
su(4)

[{⟨1, 1⟩},{⟨25109, 1⟩}],[{⟨1, 1⟩}],[(25109)],[{⟨1, 1⟩}], [(26, 2, 0),(0, 2, 26)]

---

su(2) ⟵ sp(12558)
so(25116) ⟵ su(25116)
su(3)

[{⟨1, 1⟩},{⟨25115, 1⟩}],[{⟨1, 1⟩}],[(25115)],[{⟨1, 1⟩}], [(55, 12),(12, 55)]

---

su(2) ⟵ sp(12567)
so(25134) ⟵ su(25134)
su(3)

[{⟨1, 1⟩},{⟨25133, 1⟩}],[{⟨1, 1⟩}],[(25133)],[{⟨1, 1⟩}], [(58, 11),(11, 58)]

---

su(2) ⟵ sp(12576)
so(25152) ⟵ su(25152)
su(3)

[{⟨1, 1⟩},{⟨25151, 1⟩}],[{⟨1, 1⟩}],[(25151)],[{⟨1, 1⟩}], [(127, 2),(2, 127)]

---

su(2)
sp(2) — sp(12580) — su(25160)
so(25160)

[{⟨1, 1⟩},{⟨25159, 1⟩}], [{⟨1, 1⟩}], [(25159)], [(33, 2)], [{⟨1, 1⟩}]

---

su(2) ⟵ sp(12597) — su(25194)
sp(9)
so(18) — so(25194)

[{⟨1, 1⟩},{⟨25193, 1⟩}],[{⟨1, 1⟩}],[(25193)],[{⟨1, 1⟩}], [{⟨8, 1⟩}],[{⟨1, 5⟩}]

---

su(2)
so(224) — so(25199) ⟵ su(25199)

[{⟨1, 1⟩},{⟨25198, 1⟩}],[{⟨1, 1⟩}],[(25198)],[{⟨1, 2⟩}]

---

su(2) ⟵ sp(12600)
su(9)
so(225) ⟵ so(25200)
sp(112)
su(3)
su(5)
su(5)
su(6)
su(6) — su(25200)
su(6)
su(6)
su(7)
su(8)
su(9)
su(224)
su(225)
so(10)

[{⟨1, 1⟩},{⟨25199, 1⟩}],[{⟨1, 1⟩}],[(25199)],[{⟨1, 1⟩}], [{⟨1, 3⟩, ⟨8, 3⟩}], [{⟨2, 1⟩}], [{⟨1, 2⟩}], [(223, 0),(0, 223)], [(1, 6, 0, 1),(1, 0, 6, 1)], [(3, 0, 3, 2),(2, 3, 0, 3)], [(0, 3, 2, 0),(0, 0, 2, 3, 0)], [(1, 2, 0, 2, 0),(0, 2, 0, 2, 1)], [(1, 2, 2, 0, 0),(0, 0, 2, 2, 1)], [(4, 2, 0, 0, 1),(1, 0, 0, 2, 4)],[{⟨2, 3⟩, ⟨4, 1⟩},{⟨3, 1⟩, ⟨5, 3⟩}],[{⟨2, 1⟩, ⟨5, 2⟩}, {⟨3, 2⟩, ⟨6, 1⟩}], [{⟨1, 1⟩, ⟨2, 2⟩, ⟨8, 1⟩},{⟨1, 1⟩, ⟨7, 2⟩, ⟨8, 1⟩}],[{⟨1, 2⟩},{⟨223, 2⟩}],[{⟨2, 1⟩},{⟨223, 1⟩}],[(0, 1, 1, 1, 0),(0, 1, 1, 0, 1)]

---

su(2) ⟵ so(25235) — su(25235)
su(3)

[{⟨1, 1⟩},{⟨25234, 1⟩}], [{⟨1, 1⟩}], [(25234)], [(97, 4), (4, 97)]

---

su(2) ⟵ so(25245)
su(3) — su(25245)
su(4)

[{⟨1, 1⟩},{⟨25244, 1⟩}], [{⟨1, 1⟩}], [(25244)], [(50, 14), (14, 50)],[(5, 8, 1),(1, 8, 5)]

---

su(2) ⟵ sp(12640)
su(159) ⟵ so(25280) — su(25280)
su(3)

[{⟨1, 1⟩},{⟨25279, 1⟩}],[{⟨1, 1⟩}],[(25279)],[{⟨1, 1⟩}], [{⟨1, 1⟩, ⟨158, 1⟩}],[(157, 1),(1, 157)]

---

su(2) ⟵ so(25311) — su(25311)
su(3)

[{⟨1, 1⟩},{⟨25310, 1⟩}], [{⟨1, 1⟩}], [(25310)], [(32, 25), (25, 32)]

---

su(2) ⟵ so(25327) — su(25327)
su(3)

[{⟨1, 1⟩},{⟨25326, 1⟩}], [{⟨1, 1⟩}], [(25326)], [(42, 18), (18, 42)]

---

su(2) ⟵ sp(12672)
so(25344) ⟵ su(25344)
su(4)

[{⟨1, 1⟩},{⟨25343, 1⟩}],[{⟨1, 1⟩}],[(25343)],[{⟨1, 1⟩}], [(15, 1, 3),(3, 1, 15)]

---

su(2) ⟵ so(25365) — su(25365)
su(3)

[{⟨1, 1⟩},{⟨25364, 1⟩}], [{⟨1, 1⟩}], [(25364)], [(88, 5), (5, 88)]

---

su(2) ⟵ sp(12712) — su(25424)
so(225)
sp(113) — so(25424)

[{⟨1, 1⟩},{⟨25423, 1⟩}],[{⟨1, 1⟩}],[(25423)],[{⟨1, 1⟩}], [{⟨1, 2⟩}],[{⟨2, 1⟩}]

---

su(2)
so(226) — so(25425)
su(3) — su(25425)
su(225)
su(226)

[{⟨1, 1⟩},{⟨25424, 1⟩}],[{⟨1, 1⟩}],[(25424)],[{⟨2, 1⟩}], [(224, 0),(0, 224)], [{⟨1, 2⟩},{⟨224, 2⟩}], [{⟨2, 1⟩}, {⟨224, 1⟩}]

---

su(2) ⟵ sp(12740)
so(25480)
su(3) — su(25480)
su(4)
su(14)

[{⟨1, 1⟩},{⟨25479, 1⟩}],[{⟨1, 1⟩}],[(25479)],[{⟨1, 1⟩}], [(48, 15),(15, 48)], [(12, 6, 0),(0, 6, 12)], [{⟨1, 1⟩, ⟨2, 2⟩},{⟨12, 2⟩, ⟨13, 1⟩}]

---

su(2) ⟵ sp(12744)
so(25488) ⟵ su(25488)
su(3)

[{⟨1, 1⟩},{⟨25487, 1⟩}],[{⟨1, 1⟩}],[(25487)],[{⟨1, 1⟩}], [(31, 26),(26, 31)]

---

su(2) ⟵ sp(12750)
so(25500) ⟵ su(25500)
su(4)

[{⟨1, 1⟩},{⟨25499, 1⟩}],[{⟨1, 1⟩}],[(25499)],[{⟨1, 1⟩}], [(4, 9, 1),(1, 9, 4)]

---

su(2) ⟵ so(25515)
su(3)
su(4) — su(25515)
su(5)
su(9)

[{⟨1, 1⟩},{⟨25514, 1⟩}], [{⟨1, 1⟩}], [(25514)], [(44, 17), (17, 44)], [(14, 2, 2),(2, 2, 14)], [(2, 5, 0, 1),(1, 0, 5, 2)], [{⟨1, 2⟩, ⟨6, 1⟩, ⟨8, 1⟩},{⟨1, 1⟩, ⟨3, 1⟩, ⟨8, 2⟩}]

---

su(2) ⟵ sp(12765)
so(25530) — su(25530)
su(3)
su(3)

[{⟨1, 1⟩},{⟨25529, 1⟩}],[{⟨1, 1⟩}],[(25529)],[{⟨1, 1⟩}], [(36, 22),(22, 36)],[(110, 3),(3, 110)]

---

su(2) ⟵ sp(12768)
so(25536) — su(25536)
su(3)
su(4)

[{⟨1, 1⟩},{⟨25535, 1⟩}],[{⟨1, 1⟩}],[(25535)],[{⟨1, 1⟩}], [(75, 7),(7, 75)],[(11, 3, 2),(2, 3, 11)]

---

su(2) ⟵ sp(12771)
so(25542) ⟵ su(25542)
su(3)

[{⟨1, 1⟩},{⟨25541, 1⟩}],[{⟨1, 1⟩}],[(25541)],[{⟨1, 1⟩}], [(128, 2),(2, 128)]

---

su(2) ⟵ so(25543) — su(25543)
su(3)

[{⟨1, 1⟩},{⟨25542, 1⟩}], [{⟨1, 1⟩}], [(25542)], [(81, 6), (6, 81)]

---

su(2) ⟵ sp(12780)
so(25560) ⟵ su(25560)
su(3)

[{⟨1, 1⟩},{⟨25559, 1⟩}],[{⟨1, 1⟩}],[(25559)],[{⟨1, 1⟩}], [(70, 8),(8, 70)]

su(2) ← sp(12784) ←
so(25568) ← su(25568)
su(3) ←

[{⟨1, 1⟩},{⟨25567, 1⟩}],[{⟨1, 1⟩}],[(25567)],[{⟨1, 1⟩}],[(46, 16),(16, 46)]

---

su(2) ←
so(5) ← so(25585) ← su(25585)

[{⟨1, 1⟩},{⟨25584, 1⟩}],[{⟨1, 1⟩}],[(25584)],[(41, 0)]

---

su(2) ←
su(160) ← so(25599) ←
su(3) ← su(25599)

[{⟨1, 1⟩},{⟨25598, 1⟩}], [{⟨1, 1⟩}], [(25598)], [{⟨1, 1⟩, ⟨159, 1⟩}],[(158, 1),(1, 158)]

---

su(2) ← sp(12803) ←
so(5) ← so(25606) ← su(25606)
su(3) ←

[{⟨1, 1⟩},{⟨25605, 1⟩}],[{⟨1, 1⟩}],[(25605)],[{⟨1, 1⟩}],[(27, 2)],[(30, 27),(27, 30)]

---

su(2) ← sp(12810) ←
so(25620) ← su(25620)
su(3) ←

[{⟨1, 1⟩},{⟨25619, 1⟩}],[{⟨1, 1⟩}],[(25619)],[{⟨1, 1⟩}],[(39, 20),(20, 39)]

---

su(2) ← so(25641) ←
su(3) ← su(25641)

[{⟨1, 1⟩},{⟨25640, 1⟩}], [{⟨1, 1⟩}], [(25640)], [(62, 10),(10, 62)]

---

su(2) ← sp(12825) ←
so(226) ← so(25650) ← su(25650)

[{⟨1, 1⟩},{⟨25649, 1⟩}],[{⟨1, 1⟩}],[(25649)],[{⟨1, 1⟩}],[{⟨1, 2⟩}]

---

su(2) ←
so(227) ← so(25651) ←
sp(113) ←
su(3) ← su(25651)
su(226) ←
su(227) ←

[{⟨1, 1⟩},{⟨25650, 1⟩}],[{⟨1, 1⟩}],[(25650)],[{⟨2, 1⟩}],[{⟨1, 2⟩}], [(225, 0),(0, 225)], [{⟨1, 2⟩},{⟨225, 2⟩}],[{⟨2, 1⟩},{⟨225, 1⟩}]

---

su(2) ← so(25665) ←
su(3) ← su(25665)

[{⟨1, 1⟩},{⟨25664, 1⟩}], [{⟨1, 1⟩}], [(25664)], [(29, 28),(28, 29)]

---

su(2) ← sp(12852) ←
so(25704) ←
su(3) ← su(25704)
su(4) ←
su(4) ←

[{⟨1, 1⟩},{⟨25703, 1⟩}],[{⟨1, 1⟩}],[(25703)],[{⟨1, 1⟩}],[(53, 13),(13, 53)], [(7, 5, 2),(2, 5, 7)], [(16, 0, 5),(5, 0, 16)]

---

su(2) ←
so(8) ← so(25725) ←
su(5) ← su(25725)

[{⟨1, 1⟩},{⟨25724, 1⟩}], [{⟨1, 1⟩}], [(25724)], [(1, 2, 1, 1)],[(6, 1, 0, 3),(3, 0, 1, 6)]

---

su(2) ← sp(12870) ←
so(9) ← so(25740) ←
su(3) ←
su(4) ←
su(4) ←
su(5) ← su(25740)
su(8) ←
su(9) ←
su(9) ←
su(11) ←

[{⟨1, 1⟩},{⟨25739, 1⟩}],[{⟨1, 1⟩}],[(25739)],[{⟨1, 1⟩}],[(1, 0, 1, 2)],[(98, 4),(4, 98)],[(11, 0, 8),(8, 0, 11)],[(21, 3, 0),(0, 3, 21)], [(2, 7, 0, 0),(0, 0, 7, 2)], [{⟨1, 7⟩, ⟨7, 1⟩},{⟨1, 1⟩, ⟨7, 7⟩}], [{⟨1, 4⟩, ⟨3, 1⟩},{⟨6, 1⟩, ⟨8, 4⟩}], [{⟨1, 6⟩, ⟨8, 1⟩},{⟨1, 1⟩, ⟨8, 6⟩}], [{⟨1, 2⟩, ⟨5, 1⟩},{⟨6, 1⟩, ⟨10, 2⟩}]

---

su(2) ← sp(12880) ←
so(25760) ← su(25760)
su(4) ←
su(4) ←

[{⟨1, 1⟩},{⟨25759, 1⟩}],[{⟨1, 1⟩}],[(25759)],[{⟨1, 1⟩}],[(14, 0, 6),(6, 0, 14)],[(22, 0, 3),(3, 0, 22)]

---

su(2) ← so(25795) ←
su(3) ← su(25795)

[{⟨1, 1⟩},{⟨25794, 1⟩}], [{⟨1, 1⟩}], [(25794)], [(66, 9),(9, 66)]

---

su(2) ←
sp(2) ← sp(12920) ←
so(25840) ←
su(4) ← su(25840)
su(5) ←
su(18) ←

[{⟨1, 1⟩},{⟨25839, 1⟩}], [{⟨1, 1⟩}], [(25839)], [(29, 3)], [{⟨1, 1⟩}], [(2, 15, 0),(0, 15, 2)], [(15, 0, 1, 0),(0, 1, 0, 15)],[{⟨1, 2⟩, ⟨16, 1⟩},{⟨2, 1⟩, ⟨17, 2⟩}]

---

su(2) ← sp(12936) ←
so(25872) ←
su(6) ←
su(6) ← su(25872)
su(8) ←
su(8) ←

[{⟨1, 1⟩},{⟨25871, 1⟩}],[{⟨1, 1⟩}],[(25871)],[{⟨1, 1⟩}],[(1, 0, 0, 5, 0),(0, 5, 0, 0, 1)], [(3, 2, 0, 1, 0),(0, 1, 0, 2, 3)], [{⟨1, 2⟩, ⟨3, 2⟩},{⟨5, 2⟩, ⟨7, 2⟩}], [{⟨1, 5⟩, ⟨7, 2⟩},{⟨1, 2⟩, ⟨7, 5⟩}]

---

su(2) ←
so(227) ← so(25877) ← su(25877)
sp(114) ←

[{⟨1, 1⟩},{⟨25876, 1⟩}],[{⟨1, 1⟩}],[(25876)],[{⟨1, 2⟩}],[{⟨2, 1⟩}]

---

su(2) ← sp(12939) ←
so(228) ← so(25878) ←
su(3) ← su(25878)
su(227) ←
su(228) ←

[{⟨1, 1⟩},{⟨25877, 1⟩}],[{⟨1, 1⟩}],[(25877)],[{⟨1, 1⟩}],[{⟨2, 1⟩}], [(226, 0),(0, 226)], [{⟨1, 2⟩},{⟨226, 2⟩}],[{⟨2, 1⟩},{⟨226, 1⟩}]

---

su(2) ←
sp(2) ← sp(12960) ←
su(161) ← so(25920) ←
su(3) ← su(25920)
su(3) ←
su(3) ←
su(3) ←

[{⟨1, 1⟩},{⟨25919, 1⟩}], [{⟨1, 1⟩}], [(25919)], [(23, 5)], [{⟨1, 1⟩}], [{⟨1, 1⟩, ⟨160, 1⟩}], [(35, 23),(23, 35)], [(59, 11),(11, 59)],[(89, 5),(5, 89)],[(159, 1),(1, 159)]

---

su(2) ←
so(5) ← so(25935) ←
su(3) ← su(25935)
su(3) ←
su(4) ←

[{⟨1, 1⟩},{⟨25934, 1⟩}], [{⟨1, 1⟩}], [(25934)], [(18, 6)], [(56, 12),(12, 56)], [(129, 2),(2, 129)], [(4, 12, 0),(0, 12, 4)]

---

su(2) ← sp(12987) ←
so(25974) ← su(25974)
su(4) ←
su(37) ←

[{⟨1, 1⟩},{⟨25973, 1⟩}],[{⟨1, 1⟩}],[(25973)],[{⟨1, 1⟩}],[(35, 0, 1),(1, 0, 35)], [{⟨1, 2⟩, ⟨36, 1⟩},{⟨1, 1⟩, ⟨36, 2⟩}]

---

su(2) ← sp(12992) ←
so(25984) ← su(25984)
su(3) ←
su(4) ←

[{⟨1, 1⟩},{⟨25983, 1⟩}],[{⟨1, 1⟩}],[(25983)],[{⟨1, 1⟩}],[(111, 3),(3, 111)],[(27, 0, 2),(2, 0, 27)]

---

su(2) ← sp(13013) ←
sp(4) ← so(26026) ←
su(5) ← su(26026)
su(12) ←
su(13) ←

[{⟨1, 1⟩},{⟨26025, 1⟩}],[{⟨1, 1⟩}],[(26025)],[{⟨1, 1⟩}],[(0, 0, 0, 4)], [(0, 10, 0, 0),(0, 0, 10, 0)], [{⟨2, 3⟩},{⟨10, 3⟩}],[{⟨3, 2⟩},{⟨10, 2⟩}]

---

su(2) ← sp(13020) ←
so(26040) ← su(26040)
su(3) ←

[{⟨1, 1⟩},{⟨26039, 1⟩}],[{⟨1, 1⟩}],[(26039)],[{⟨1, 1⟩}],[(41, 19),(19, 41)]

---

su(2) ← sp(13041) ←
sp(11) ← so(26082) ← su(26082)

[{⟨1, 1⟩},{⟨26081, 1⟩}],[{⟨1, 1⟩}],[(26081)],[{⟨1, 1⟩}],[{⟨1, 1⟩, ⟨3, 1⟩}]

---

su(2) ←
sp(2) ← sp(13050) ←
so(26100) ← su(26100)
su(4) ←

[{⟨1, 1⟩},{⟨26099, 1⟩}], [{⟨1, 1⟩}], [(26099)], [(3, 24)], [{⟨1, 1⟩}],[(24, 1, 1),(1, 1, 24)]

---

su(2) ←
so(228) ← so(26105) ← su(26105)

[{⟨1, 1⟩},{⟨26104, 1⟩}],[{⟨1, 1⟩}],[(26104)],[{⟨1, 2⟩}]

su(2) ← sp(13053); so(229), sp(114) → so(26106); su(3); su(228); su(229) ← su(26106)

[{⟨1, 1⟩},{⟨26105, 1⟩}],[{⟨1, 1⟩}],[(26105)],[{⟨1, 1⟩}],[{⟨2, 1⟩}], [{⟨1, 2⟩}], [(227, 0),(0, 227)], [{⟨1, 2⟩},{⟨227, 2⟩}],[{⟨2, 1⟩},{⟨227, 1⟩}]

---

su(2), so(21) ← so(26125) ← su(26125)

[{⟨1, 1⟩},{⟨26124, 1⟩}], [{⟨1, 1⟩}], [(26124)], [{⟨1, 2⟩, ⟨2, 1⟩}]

---

su(2) ← sp(13065); so(26130); su(3) ← su(26130)

[{⟨1, 1⟩},{⟨26129, 1⟩}],[{⟨1, 1⟩}],[(26129)],[{⟨1, 1⟩}], [(51, 14),(14, 51)]

---

su(2) ← so(26145); su(3) ← su(26145)

[{⟨1, 1⟩},{⟨26144, 1⟩}], [{⟨1, 1⟩}], [(26144)], [(82, 6), (6, 82)]

---

su(2) ← so(26169); su(3) ← su(26169)

[{⟨1, 1⟩},{⟨26168, 1⟩}], [{⟨1, 1⟩}], [(26168)], [(38, 21), (21, 38)]

---

su(2), sp(2) → sp(13090); so(15) ← so(26180); su(3); su(4) ← su(26180)

[{⟨1, 1⟩},{⟨26179, 1⟩}], [{⟨1, 1⟩}], [(26179)], [(1, 32)], [{⟨1, 1⟩}], [{⟨2, 1⟩, ⟨3, 1⟩}], [(76, 7),(7, 76)], [(6, 3, 5), (5, 3, 6)]

---

su(2) ← sp(13091); so(53) ← so(26182) ← su(26182)

[{⟨1, 1⟩},{⟨26181, 1⟩}],[{⟨1, 1⟩}],[(26181)],[{⟨1, 1⟩}], [{⟨1, 3⟩}]

---

su(2) ← sp(13104); so(7) ← so(26208); su(14) ← su(26208)

[{⟨1, 1⟩},{⟨26207, 1⟩}],[{⟨1, 1⟩}],[(26207)],[{⟨1, 1⟩}], [(2, 3, 1)],[{⟨1, 2⟩, ⟨3, 1⟩},{⟨11, 1⟩, ⟨13, 2⟩}]

---

su(2), so(5), so(55) → so(26235); su(4); su(53); su(55) ← su(26235)

[{⟨1, 1⟩},{⟨26234, 1⟩}], [{⟨1, 1⟩}], [(26234)], [(0, 52)], [{⟨3, 1⟩}], [(52, 0, 0),(0, 0, 52)], [{⟨1, 3⟩},{⟨52, 3⟩}], [{⟨3, 1⟩},{⟨52, 1⟩}]

---

su(2), su(162) → so(26243); su(3) ← su(26243)

[{⟨1, 1⟩},{⟨26242, 1⟩}], [{⟨1, 1⟩}], [(26242)], [{⟨1, 1⟩, ⟨161, 1⟩}],[(160, 1),(1, 160)]

---

su(2), sp(2) → sp(13122); so(26244); su(3); su(4) ← su(26244)

[{⟨1, 1⟩},{⟨26243, 1⟩}], [{⟨1, 1⟩}], [(26243)], [(17, 8)], [{⟨1, 1⟩}],[(71, 8),(8, 71)],[(8, 2, 5),(5, 2, 8)]

---

su(2) ← sp(13125); so(26250); su(3); su(3) ← su(26250)

[{⟨1, 1⟩},{⟨26249, 1⟩}],[{⟨1, 1⟩}],[(26249)],[{⟨1, 1⟩}], [(34, 24),(24, 34)],[(99, 4),(4, 99)]

---

su(2) ← so(26331); su(3) ← su(26331)

[{⟨1, 1⟩},{⟨26330, 1⟩}], [{⟨1, 1⟩}], [(26330)], [(130, 2), (2, 130)]

---

su(2), sp(3), sp(9) → sp(13167); so(229), sp(115), so(22), so(22) → so(26334); su(3); su(4); su(6); su(18); su(22) ← su(26334)

[{⟨1, 1⟩},{⟨26333, 1⟩}], [{⟨1, 1⟩}], [(26333)], [(17, 0, 0)],[{⟨1, 5⟩}],[{⟨1, 1⟩}],[{⟨1, 2⟩}],[{⟨2, 1⟩}],[{⟨5, 1⟩}], [{⟨1, 1⟩, ⟨3, 1⟩}], [(43, 18),(18, 43)], [(6, 10, 0),(0, 10, 6)],[(17, 0, 0, 0, 0),(0, 0, 0, 0, 17)],[{⟨1, 5⟩},{⟨17, 5⟩}], [{⟨5, 1⟩},{⟨17, 1⟩}]

---

su(2), so(230) → so(26335); su(3); su(229); su(230) ← su(26335)

[{⟨1, 1⟩},{⟨26334, 1⟩}],[{⟨1, 1⟩}],[(26334)],[{⟨2, 1⟩}], [(228, 0),(0, 228)], [{⟨1, 2⟩},{⟨228, 2⟩}], [{⟨2, 1⟩}, {⟨228, 1⟩}]

---

su(2) ← sp(13200); so(26400); su(3); su(3); su(5); su(5); so(10) ← su(26400)

[{⟨1, 1⟩},{⟨26399, 1⟩}],[{⟨1, 1⟩}],[(26399)],[{⟨1, 1⟩}], [(49, 15),(15, 49)], [(63, 10),(10, 63)], [(1, 3, 3, 0),(0, 3, 3, 1)], [(10, 0, 2, 0),(0, 2, 0, 10)], [(0, 0, 0, 4, 1),(0, 0, 0, 1, 4)]

---

su(2), so(7) → so(26411) ← su(26411)

[{⟨1, 1⟩},{⟨26410, 1⟩}],[{⟨1, 1⟩}],[(26410)],[(6, 2, 0)]

---

su(2) ← sp(13221); so(26442); su(3) ← su(26442)

[{⟨1, 1⟩},{⟨26441, 1⟩}],[{⟨1, 1⟩}],[(26441)],[{⟨1, 1⟩}], [(112, 3),(3, 112)]

---

su(2), so(5), so(43) → so(26445) ← su(26445)

[{⟨1, 1⟩},{⟨26444, 1⟩}], [{⟨1, 1⟩}], [(26444)], [(1, 40)], [{⟨1, 1⟩, ⟨2, 1⟩}]

---

su(2), so(5) → so(26455) ← su(26455)

[{⟨1, 1⟩},{⟨26454, 1⟩}],[{⟨1, 1⟩}],[(26454)],[(10, 14)]

---

su(2) ← sp(13230); so(26460); su(6); su(7); su(7) ← su(26460)

[{⟨1, 1⟩},{⟨26459, 1⟩}],[{⟨1, 1⟩}],[(26459)],[{⟨1, 1⟩}], [(0, 1, 4, 0, 0),(0, 0, 4, 1, 0)], [{⟨1, 1⟩, ⟨3, 1⟩, ⟨5, 2⟩}, {⟨2, 2⟩, ⟨4, 1⟩, ⟨6, 1⟩}], [{⟨1, 3⟩, ⟨5, 1⟩, ⟨6, 2⟩},{⟨1, 2⟩, ⟨2, 1⟩, ⟨6, 3⟩}]

---

su(2) ← so(26481); su(3) ← su(26481)

[{⟨1, 1⟩},{⟨26480, 1⟩}], [{⟨1, 1⟩}], [(26480)], [(90, 5), (5, 90)]

---

su(2) ← sp(13244); so(26488); su(43) ← su(26488)

[{⟨1, 1⟩},{⟨26487, 1⟩}],[{⟨1, 1⟩}],[(26487)],[{⟨1, 1⟩}], [{⟨1, 1⟩, ⟨2, 1⟩},{⟨41, 1⟩, ⟨42, 1⟩}]

---

su(2) ← sp(13248); so(26496); su(3) ← su(26496)

[{⟨1, 1⟩},{⟨26495, 1⟩}],[{⟨1, 1⟩}],[(26495)],[{⟨1, 1⟩}], [(45, 17),(17, 45)]

---

su(2) ← sp(13260); so(11) ← so(26520); su(3); su(3); su(3); su(4); su(5) ← su(26520)

[{⟨1, 1⟩},{⟨26519, 1⟩}],[{⟨1, 1⟩}],[(26519)],[{⟨1, 1⟩}], [(3, 0, 1, 0, 0)], [(33, 25),(25, 33)], [(47, 16),(16, 47)], [(67, 9),(9, 67)], [(7, 4, 3),(3, 4, 7)], [(12, 2, 0, 0),(0, 0, 2, 12)]

---

su(2) ← sp(13282); so(230) ← so(26564) ← su(26564)

[{⟨1, 1⟩},{⟨26563, 1⟩}],[{⟨1, 1⟩}],[(26563)],[{⟨1, 1⟩}], [{⟨1, 2⟩}]

---

su(2), so(231), sp(115) → so(26565); su(3); su(3); su(230); su(21), su(22) → su(231) ← su(26565)

[{⟨1, 1⟩},{⟨26564, 1⟩}],[{⟨1, 1⟩}],[(26564)],[{⟨2, 1⟩}], [{⟨1, 2⟩}], [(54, 13),(13, 54)], [(229, 0),(0, 229)], [{⟨1, 2⟩},{⟨229, 2⟩}], [{⟨2, 1⟩},{⟨229, 1⟩}], [{⟨1, 2⟩, ⟨2, 1⟩},{⟨19, 1⟩, ⟨20, 2⟩}], [{⟨1, 1⟩, ⟨3, 1⟩},{⟨19, 1⟩, ⟨21, 1⟩}]

---

su(2) ← sp(13284); su(163) ← so(26568); su(3) ← su(26568)

[{⟨1, 1⟩},{⟨26567, 1⟩}],[{⟨1, 1⟩}],[(26567)],[{⟨1, 1⟩}], [{⟨1, 1⟩, ⟨162, 1⟩}],[(161, 1),(1, 161)]

---

su(2) ← sp(13300); so(26600); su(5) ← su(26600)

[{⟨1, 1⟩},{⟨26599, 1⟩}],[{⟨1, 1⟩}],[(26599)],[{⟨1, 1⟩}], [(13, 0, 0, 2),(2, 0, 0, 13)]

su(26620) → sp(13310) → su(2); so(26620); su(4)

[{⟨1, 1⟩},{⟨26619, 1⟩}],[{⟨1, 1⟩}],[(26619)],[{⟨1, 1⟩}], [(10, 0, 9),(9, 0, 10)]

---

su(26640) → sp(13320) → su(2); so(26640) → so(5)

[{⟨1, 1⟩},{⟨26639, 1⟩}],[{⟨1, 1⟩}],[(26639)],[{⟨1, 1⟩}], [(4, 26)]

---

su(26657) → so(26657) → su(2); su(3)

[{⟨1, 1⟩},{⟨26656, 1⟩}], [{⟨1, 1⟩}], [(26656)], [(37, 22), (22, 37)]

---

su(26676) → sp(13338) → su(2); so(26676); su(4); su(4); su(38)

[{⟨1, 1⟩},{⟨26675, 1⟩}],[{⟨1, 1⟩}],[(26675)],[{⟨1, 1⟩}], [(5, 11, 0),(0, 11, 5)], [(35, 1, 0),(0, 1, 35)], [{⟨1, 1⟩, ⟨36, 1⟩},{⟨2, 1⟩, ⟨37, 1⟩}]

---

su(26691) → so(26691) → su(2); su(3)

[{⟨1, 1⟩},{⟨26690, 1⟩}], [{⟨1, 1⟩}], [(26690)], [(40, 20), (20, 40)]

---

su(26718) → sp(13359) → su(2); so(26718); su(3)

[{⟨1, 1⟩},{⟨26717, 1⟩}],[{⟨1, 1⟩}],[(26717)],[{⟨1, 1⟩}], [(60, 11),(11, 60)]

---

su(26730) → sp(13365) → su(2); so(26730); su(3); su(3); su(5); su(5)

[{⟨1, 1⟩},{⟨26729, 1⟩}],[{⟨1, 1⟩}],[(26729)],[{⟨1, 1⟩}], [(32, 26),(26, 32)], [(131, 2),(2, 131)], [(2, 2, 2, 1),(1, 2, 2, 2)],[(8, 1, 0, 2),(2, 0, 1, 8)]

---

su(26754) → sp(13377) → su(2); so(26754); su(3)

[{⟨1, 1⟩},{⟨26753, 1⟩}],[{⟨1, 1⟩}],[(26753)],[{⟨1, 1⟩}], [(83, 6),(6, 83)]

---

su(26765) → so(26765) → su(2); su(3)

[{⟨1, 1⟩},{⟨26764, 1⟩}], [{⟨1, 1⟩}], [(26764)], [(100, 4), (4, 100)]

---

su(26767) → so(26767) → su(2); su(3)

[{⟨1, 1⟩},{⟨26766, 1⟩}], [{⟨1, 1⟩}], [(26766)], [(57, 12), (12, 57)]

---

su(26775) → so(26775) → su(2); su(5)

[{⟨1, 1⟩},{⟨26774, 1⟩}], [{⟨1, 1⟩}], [(26774)], [(11, 1, 0, 1),(1, 0, 1, 11)]

---

su(26795) → so(26795) → su(2), so(231), sp(116)

[{⟨1, 1⟩},{⟨26794, 1⟩}],[{⟨1, 1⟩}],[(26794)],[{⟨1, 2⟩}], [{⟨2, 1⟩}]

---

su(26796) → sp(13398) → su(2), sp(2); so(26796) → so(232); su(3); su(231); su(232)

[{⟨1, 1⟩},{⟨26795, 1⟩}], [{⟨1, 1⟩}], [(26795)], [(21, 6)], [{⟨1, 1⟩}], [{⟨2, 1⟩}], [(230, 0),(0, 230)], [{⟨1, 2⟩},{⟨230, 2⟩}],[{⟨2, 1⟩},{⟨230, 1⟩}]

---

su(26832) → sp(13416) → su(2); so(26832); su(3)

[{⟨1, 1⟩},{⟨26831, 1⟩}],[{⟨1, 1⟩}],[(26831)],[{⟨1, 1⟩}], [(77, 7),(7, 77)]

---

su(26880) → sp(13440) → su(2), sp(2); so(26880); su(3); su(4); su(4); su(5); su(6); su(6)

[{⟨1, 1⟩},{⟨26879, 1⟩}], [{⟨1, 1⟩}], [(26879)], [(19, 7)], [{⟨1, 1⟩}],[(31, 27),(27, 31)],[(9, 3, 3),(3, 3, 9)],[(11, 1, 5),(5, 1, 11)], [(7, 0, 0, 5),(5, 0, 0, 7)], [(1, 1, 2, 0, 1),(1, 0, 2, 1, 1)],[(1, 1, 3, 0, 0),(0, 0, 3, 1, 1)]

---

su(26895) → so(26895) → su(2), su(164); su(3)

[{⟨1, 1⟩},{⟨26894, 1⟩}], [{⟨1, 1⟩}], [(26894)], [{⟨1, 1⟩, ⟨163, 1⟩}],[(162, 1),(1, 162)]

---

su(26904) → sp(13452) → su(2); so(26904); su(3)

[{⟨1, 1⟩},{⟨26903, 1⟩}],[{⟨1, 1⟩}],[(26903)],[{⟨1, 1⟩}], [(113, 3),(3, 113)]

---

su(26937) → so(26937) → su(2); su(3)

[{⟨1, 1⟩},{⟨26936, 1⟩}], [{⟨1, 1⟩}], [(26936)], [(72, 8), (8, 72)]

---

su(26950) → sp(13475) → su(2); so(26950); su(5); su(6); su(7)

[{⟨1, 1⟩},{⟨26949, 1⟩}],[{⟨1, 1⟩}],[(26949)],[{⟨1, 1⟩}], [(4, 1, 3, 0),(0, 3, 1, 4)], [(2, 0, 0, 4, 0),(0, 4, 0, 0, 2)], [{⟨1, 2⟩, ⟨5, 3⟩},{⟨2, 3⟩, ⟨6, 2⟩}]

---

su(26970) → sp(13485) → su(2); so(26970) → sp(15); su(3)

[{⟨1, 1⟩},{⟨26969, 1⟩}],[{⟨1, 1⟩}],[(26969)],[{⟨1, 1⟩}], [{⟨4, 1⟩}],[(30, 28),(28, 30)]

---

su(27000) → sp(13500) → su(2); so(27000) → su(3), su(7), e8; su(4); su(6)

[{⟨1, 1⟩},{⟨26999, 1⟩}],[{⟨1, 1⟩}],[(26999)],[{⟨1, 1⟩}], [(29, 29)], [{⟨2, 2⟩, ⟨5, 2⟩}], [{⟨8, 2⟩}], [(9, 4, 2),(2, 4, 9)],[(0, 3, 0, 2, 0),(0, 2, 0, 3, 0)]

---

su(27027) → so(27027) → su(2), so(7), so(7), so(9), so(27), sp(6), so(12), so(232); su(7); su(7); su(8); su(9); su(11); su(14)

[{⟨1, 1⟩},{⟨27026, 1⟩}], [{⟨1, 1⟩}], [(27026)], [(0, 1, 8)], [(1, 3, 2)], [(0, 1, 2, 0)], [{⟨1, 4⟩}], [{⟨1, 2⟩, ⟨6, 1⟩}], [{⟨1, 2⟩, ⟨5, 2⟩},{⟨1, 2⟩, ⟨6, 2⟩}], [{⟨1, 2⟩}], [{⟨1, 5⟩, ⟨2, 2⟩},{⟨5, 2⟩, ⟨6, 5⟩}], [{⟨1, 8⟩, ⟨2, 1⟩},{⟨5, 1⟩, ⟨6, 8⟩}], [{⟨1, 5⟩, ⟨3, 1⟩},{⟨5, 1⟩, ⟨7, 5⟩}], [{⟨1, 3⟩, ⟨2, 1⟩, ⟨8, 1⟩},{⟨1, 1⟩, ⟨7, 1⟩, ⟨8, 3⟩}], [{⟨1, 2⟩, ⟨6, 1⟩},{⟨5, 1⟩, ⟨10, 2⟩}],[{⟨1, 1⟩, ⟨9, 1⟩},{⟨5, 1⟩, ⟨13, 1⟩}]

---

su(27028) → sp(13514) → su(2); so(27028) → so(233), sp(116); su(3); su(232); su(233)

[{⟨1, 1⟩},{⟨27027, 1⟩}],[{⟨1, 1⟩}],[(27027)],[{⟨1, 1⟩}], [{⟨2, 1⟩}], [{⟨1, 2⟩}], [(231, 0),(0, 231)], [{⟨1, 2⟩},{⟨231, 2⟩}],[{⟨2, 1⟩},{⟨231, 1⟩}]

---

su(27030) → sp(13515) → su(2); so(27030); su(3)

[{⟨1, 1⟩},{⟨27029, 1⟩}],[{⟨1, 1⟩}],[(27029)],[{⟨1, 1⟩}], [(52, 14),(14, 52)]

---

su(27048) → sp(13524) → su(2); so(27048); su(3)

[{⟨1, 1⟩},{⟨27047, 1⟩}],[{⟨1, 1⟩}],[(27047)],[{⟨1, 1⟩}], [(91, 5),(5, 91)]

---

su(27084) → sp(13542) → su(2); so(27084); su(3)

[{⟨1, 1⟩},{⟨27083, 1⟩}],[{⟨1, 1⟩}],[(27083)],[{⟨1, 1⟩}], [(36, 23),(23, 36)]

---

su(27090) → sp(13545) → su(2); so(27090); su(3)

[{⟨1, 1⟩},{⟨27089, 1⟩}],[{⟨1, 1⟩}],[(27089)],[{⟨1, 1⟩}], [(42, 19),(19, 42)]

---

su(27104) → sp(13552) → su(2); so(27104) → so(8)

[{⟨1, 1⟩},{⟨27103, 1⟩}],[{⟨1, 1⟩}],[(27103)],[{⟨1, 1⟩}], [(7, 1, 0, 0),(0, 1, 7, 0),(0, 1, 0, 7)]

---

su(27132) → sp(13566) → su(2); so(27132) → so(7) → g2, so(19), sp(3), sp(7); su(3); su(7); su(14); su(19)

[{⟨1, 1⟩},{⟨27131, 1⟩}],[{⟨1, 1⟩}],[(27131)],[{⟨1, 1⟩}], [(15, 0, 0)], [(15, 0)], [{⟨6, 1⟩}], [(0, 1, 6)], [{⟨1, 6⟩}], [(132, 2),(2, 132)], [{⟨1, 13⟩},{⟨6, 13⟩}], [{⟨1, 6⟩},{⟨13, 6⟩}],[{⟨6, 1⟩},{⟨13, 1⟩}]

su(27170) → sp(13585), so(27170), su(3); sp(13585) → su(2)

[{⟨1, 1⟩},{⟨27169, 1⟩}],[{⟨1, 1⟩}],[(27169)],[{⟨1, 1⟩}], [(64, 10),(10, 64)]

---

su(27216) → sp(13608), so(27216), su(4), su(6); sp(13608) → su(2), sp(2)

[{⟨1, 1⟩},{⟨27215, 1⟩}], [{⟨1, 1⟩}], [(27215)], [(5, 20)], [{⟨1, 1⟩}], [(8, 6, 1),(1, 6, 8)], [(4, 0, 1, 0, 2),(2, 0, 1, 0, 4)]

---

su(27224) → sp(13612), so(27224), su(3); sp(13612) → su(2); so(27224) → su(165)

[{⟨1, 1⟩},{⟨27223, 1⟩}],[{⟨1, 1⟩}],[(27223)],[{⟨1, 1⟩}], [{⟨1, 1⟩, ⟨164, 1⟩}],[(163, 1),(1, 163)]

---

su(27255) → so(27255), su(3); so(27255) → su(2)

[{⟨1, 1⟩},{⟨27254, 1⟩}], [{⟨1, 1⟩}], [(27254)], [(68, 9), (9, 68)]

---

su(27260) → sp(13630), so(27260); sp(13630) → su(2); so(27260) → so(233), sp(117)

[{⟨1, 1⟩},{⟨27259, 1⟩}],[{⟨1, 1⟩}],[(27259)],[{⟨1, 1⟩}], [{⟨1, 2⟩}],[{⟨2, 1⟩}]

---

su(27261) → so(27261), su(3), su(233), su(234); so(27261) → su(2), so(234)

[{⟨1, 1⟩},{⟨27260, 1⟩}],[{⟨1, 1⟩}],[(27260)],[{⟨2, 1⟩}], [(232, 0),(0, 232)], [{⟨1, 2⟩},{⟨232, 2⟩}], [{⟨2, 1⟩}, {⟨232, 1⟩}]

---

su(27265) → so(27265); so(27265) → su(2), so(5)

[{⟨1, 1⟩},{⟨27264, 1⟩}],[{⟨1, 1⟩}],[(27264)],[(2, 34)]

---

su(27280) → sp(13640), so(27280), su(3); sp(13640) → su(2)

[{⟨1, 1⟩},{⟨27279, 1⟩}],[{⟨1, 1⟩}],[(27279)],[{⟨1, 1⟩}], [(39, 21),(21, 39)]

---

su(27285) → so(27285), su(3); so(27285) → su(2)

[{⟨1, 1⟩},{⟨27284, 1⟩}], [{⟨1, 1⟩}], [(27284)], [(101, 4), (4, 101)]

---

su(27300) → sp(13650), so(27300), su(4), su(4), su(5), su(15); sp(13650) → su(2); so(27300) → so(24)

[{⟨1, 1⟩},{⟨27299, 1⟩}],[{⟨1, 1⟩}],[(27299)],[{⟨1, 1⟩}], [{⟨2, 2⟩}], [(12, 4, 1),(1, 4, 12)], [(19, 0, 4),(4, 0, 19)], [(7, 0, 3, 0),(0, 3, 0, 7)], [{⟨2, 1⟩, ⟨3, 1⟩},{⟨12, 1⟩, ⟨13, 1⟩}]

---

su(27324) → sp(13662), so(27324); sp(13662) → su(2); so(27324) → sp(12)

[{⟨1, 1⟩},{⟨27323, 1⟩}],[{⟨1, 1⟩}],[(27323)],[{⟨1, 1⟩}], [{⟨2, 2⟩}]

---

su(27336) → sp(13668), so(27336), su(3); sp(13668) → su(2)

[{⟨1, 1⟩},{⟨27335, 1⟩}],[{⟨1, 1⟩}],[(27335)],[{⟨1, 1⟩}], [(50, 15),(15, 50)]

---

su(27360) → sp(13680), so(27360), su(3); sp(13680) → su(2)

[{⟨1, 1⟩},{⟨27359, 1⟩}],[{⟨1, 1⟩}],[(27359)],[{⟨1, 1⟩}], [(44, 18),(18, 44)]

---

su(27370) → sp(13685), so(27370), su(3), su(3); sp(13685) → su(2); so(27370) → so(5)

[{⟨1, 1⟩},{⟨27369, 1⟩}],[{⟨1, 1⟩}],[(27369)],[{⟨1, 1⟩}], [(22, 4)],[(84, 6),(6, 84)],[(114, 3),(3, 114)]

---

su(27405) → so(27405), su(5), su(27), su(30); so(27405) → su(2), so(30)

[{⟨1, 1⟩},{⟨27404, 1⟩}],[{⟨1, 1⟩}],[(27404)],[{⟨4, 1⟩}], [(26, 0, 0, 0),(0, 0, 0, 26)], [{⟨1, 4⟩},{⟨26, 4⟩}], [{⟨4, 1⟩},{⟨26, 1⟩}]

---

su(27434) → sp(13717), so(27434); sp(13717) → su(2); so(27434) → so(5)

[{⟨1, 1⟩},{⟨27433, 1⟩}],[{⟨1, 1⟩}],[(27433)],[{⟨1, 1⟩}], [(42, 0)]

---

su(27440) → sp(13720), so(27440), su(3), su(4), su(5); sp(13720) → su(2)

[{⟨1, 1⟩},{⟨27439, 1⟩}],[{⟨1, 1⟩}],[(27439)],[{⟨1, 1⟩}], [(55, 13),(13, 55)], [(13, 1, 4),(4, 1, 13)], [(6, 0, 1, 3),(3, 1, 0, 6)]

---

su(27450) → sp(13725), so(27450), su(3); sp(13725) → su(2)

[{⟨1, 1⟩},{⟨27449, 1⟩}],[{⟨1, 1⟩}],[(27449)],[{⟨1, 1⟩}], [(35, 24),(24, 35)]

---

su(27455) → so(27455), su(17); so(27455) → su(2), so(6)

[{⟨1, 1⟩},{⟨27454, 1⟩}], [{⟨1, 1⟩}], [(27454)], [(14, 1, 1)],[{⟨1, 1⟩, ⟨2, 1⟩, ⟨16, 1⟩},{⟨1, 1⟩, ⟨15, 1⟩, ⟨16, 1⟩}]

---

su(27456) → sp(13728), so(27456), su(12), so(14); sp(13728) → su(2), so(13), so(13), sp(2), sp(4), sp(6); so(27456) → so(9), so(9), so(12), so(12)

[{⟨1, 1⟩},{⟨27455, 1⟩}],[{⟨1, 1⟩}],[(27455)],[{⟨6, 3⟩}], [{⟨4, 1⟩, ⟨6, 1⟩}], [(7, 17)], [(1, 0, 0, 3)], [{⟨2, 1⟩, ⟨5, 1⟩}], [{⟨1, 1⟩}], [(0, 2, 0, 2)], [(6, 0, 0, 1)], [{⟨1, 2⟩, ⟨4, 1⟩}], [{⟨1, 7⟩}], [{⟨1, 3⟩, ⟨11, 2⟩},{⟨1, 2⟩, ⟨11, 3⟩}], [{⟨6, 3⟩},{⟨7, 3⟩}]

---

su(27489) → so(27489), su(3); so(27489) → su(2), so(6)

[{⟨1, 1⟩},{⟨27488, 1⟩}], [{⟨1, 1⟩}], [(27488)], [(10, 2, 2)],[(48, 16),(16, 48)]

---

su(27492) → sp(13746), so(27492), su(3); sp(13746) → su(2)

[{⟨1, 1⟩},{⟨27491, 1⟩}],[{⟨1, 1⟩}],[(27491)],[{⟨1, 1⟩}], [(78, 7),(7, 78)]

---

su(27494) → sp(13747), so(27494); sp(13747) → su(2); so(27494) → so(234)

[{⟨1, 1⟩},{⟨27493, 1⟩}],[{⟨1, 1⟩}],[(27493)],[{⟨1, 1⟩}], [{⟨1, 2⟩}]

---

su(27495) → so(27495), su(3), su(3), su(234), su(235); so(27495) → su(2), so(235), sp(117)

[{⟨1, 1⟩},{⟨27494, 1⟩}],[{⟨1, 1⟩}],[(27494)],[{⟨2, 1⟩}], [{⟨1, 2⟩}], [(46, 17),(17, 46)], [(233, 0),(0, 233)], [{⟨1, 2⟩},{⟨233, 2⟩}],[{⟨2, 1⟩},{⟨233, 1⟩}]

---

su(27500) → sp(13750), so(27500), su(4); sp(13750) → su(2)

[{⟨1, 1⟩},{⟨27499, 1⟩}],[{⟨1, 1⟩}],[(27499)],[{⟨1, 1⟩}], [(19, 1, 2),(2, 1, 19)]

---

su(27528) → sp(13764), so(27528), su(3); sp(13764) → su(2)

[{⟨1, 1⟩},{⟨27527, 1⟩}],[{⟨1, 1⟩}],[(27527)],[{⟨1, 1⟩}], [(61, 11),(11, 61)]

---

su(27537) → so(27537), su(3); so(27537) → su(2)

[{⟨1, 1⟩},{⟨27536, 1⟩}], [{⟨1, 1⟩}], [(27536)], [(133, 2), (2, 133)]

---

su(27555) → so(27555), su(3); so(27555) → su(2), su(166)

[{⟨1, 1⟩},{⟨27554, 1⟩}], [{⟨1, 1⟩}], [(27554)], [{⟨1, 1⟩, ⟨165, 1⟩}],[(164, 1),(1, 164)]

---

su(27600) → sp(13800), so(27600), su(24); sp(13800) → su(2); so(27600) → so(6)

[{⟨1, 1⟩},{⟨27599, 1⟩}],[{⟨1, 1⟩}],[(27599)],[{⟨1, 1⟩}], [(22, 0, 0)],[{⟨2, 2⟩},{⟨22, 2⟩}]

---

su(27612) → sp(13806), so(27612), su(3); sp(13806) → su(2)

[{⟨1, 1⟩},{⟨27611, 1⟩}],[{⟨1, 1⟩}],[(27611)],[{⟨1, 1⟩}], [(58, 12),(12, 58)]

---

su(27621) → so(27621), su(3); so(27621) → su(2)

[{⟨1, 1⟩},{⟨27620, 1⟩}], [{⟨1, 1⟩}], [(27620)], [(92, 5), (5, 92)]

---

su(27639) → so(27639), su(3); so(27639) → su(2)

[{⟨1, 1⟩},{⟨27638, 1⟩}], [{⟨1, 1⟩}], [(27638)], [(73, 8), (8, 73)]

---

su(27648) → sp(13824), so(27648); sp(13824) → su(2); so(27648) → so(9)

[{⟨1, 1⟩},{⟨27647, 1⟩}],[{⟨1, 1⟩}],[(27647)],[{⟨1, 1⟩}], [(3, 1, 0, 1)]

su(2)
sp(2) ← sp(13832)
c7 ← sp(28)   so(27664)   su(27664)

[{⟨1, 1⟩},{⟨27663, 1⟩}],[{⟨1, 1⟩}],[(27663)],[(13, 11)], [{⟨3, 1⟩}],[{⟨5, 1⟩}],[{⟨1, 1⟩}]

---

su(2) ← sp(13833)
so(54) ← so(27666)   su(27666)

[{⟨1, 1⟩},{⟨27665, 1⟩}],[{⟨1, 1⟩}],[(27665)],[{⟨1, 1⟩}], [{⟨1, 3⟩}]

---

su(2)
sp(2) ← sp(13860)
sp(27)
sp(3)
sp(4)
so(10) ← so(27720)
so(56)
su(4)
su(4)
su(5)
su(5)
su(5)
su(6)
su(6)   su(27720)
su(6)
su(6)
su(8)
su(9)
su(10)
su(11)
su(21)
su(54)
su(56)

[{⟨1, 1⟩},{⟨27719, 1⟩}], [{⟨1, 1⟩}], [(27719)], [(53, 0)], [{⟨1, 3⟩}], [{⟨1, 1⟩}], [(5, 0, 3)], [(2, 3, 0, 0)], [(1, 0, 2, 0, 0)], [{⟨3, 1⟩}], [(7, 2, 6),(6, 2, 7)], [(53, 0, 0),(0, 0, 53)], [(3, 4, 1, 0),(0, 1, 4, 3)], [(4, 2, 2, 0),(0, 2, 2, 4)], [(17, 1, 0, 0),(0, 0, 1, 17)],[(2, 0, 0, 3, 1),(1, 3, 0, 0, 2)],[(3, 0, 2, 0, 1),(1, 0, 2, 0, 3)], [(3, 1, 1, 0, 1),(1, 0, 1, 1, 3)], [(3, 4, 0, 0, 0),(0, 0, 0, 4, 3)], [{⟨1, 2⟩, ⟨2, 1⟩, ⟨5, 1⟩},{⟨3, 1⟩, ⟨6, 1⟩, ⟨7, 2⟩}], [{⟨1, 1⟩, ⟨5, 1⟩, ⟨7, 1⟩},{⟨2, 1⟩, ⟨4, 1⟩, ⟨8, 1⟩}], [{⟨4, 1⟩, ⟨5, 1⟩},{⟨5, 1⟩, ⟨6, 1⟩}], [{⟨1, 2⟩, ⟨9, 1⟩, ⟨10, 1⟩},{⟨1, 1⟩, ⟨2, 1⟩, ⟨10, 2⟩}], [{⟨1, 1⟩, ⟨18, 1⟩},{⟨3, 1⟩, ⟨20, 1⟩}], [{⟨1, 3⟩},{⟨53, 3⟩}], [{⟨3, 1⟩},{⟨53, 1⟩}]

---

su(2)
so(235) ← so(27729) ← su(27729)
sp(118)

[{⟨1, 1⟩},{⟨27728, 1⟩}],[{⟨1, 1⟩}],[(27728)],[{⟨1, 2⟩}], [{⟨2, 1⟩}]

---

su(2) ← sp(13865)
so(236) ← so(27730)
su(3)   su(27730)
su(235)
su(236)

[{⟨1, 1⟩},{⟨27729, 1⟩}],[{⟨1, 1⟩}],[(27729)],[{⟨1, 1⟩}], [{⟨2, 1⟩}], [(234, 0),(0, 234)], [{⟨1, 2⟩},{⟨234, 2⟩}], [{⟨2, 1⟩},{⟨234, 1⟩}]

---

su(2) ← so(27755)   su(27755)
su(3)

[{⟨1, 1⟩},{⟨27754, 1⟩}], [{⟨1, 1⟩}], [(27754)], [(34, 25), (25, 34)]

---

su(2) ← sp(13888)
so(27776)   su(27776)
su(4)

[{⟨1, 1⟩},{⟨27775, 1⟩}],[{⟨1, 1⟩}],[(27775)],[{⟨1, 1⟩}], [(27, 2, 0),(0, 2, 27)]

---

su(2) ← so(27783)   su(27783)
su(3)

[{⟨1, 1⟩},{⟨27782, 1⟩}], [{⟨1, 1⟩}], [(27782)], [(41, 20), (20, 41)]

---

su(2) ← so(27807)   su(27807)
su(3)

[{⟨1, 1⟩},{⟨27806, 1⟩}], [{⟨1, 1⟩}], [(27806)], [(38, 22), (22, 38)]

---

su(2) ← sp(13905)
so(27810)   su(27810)
su(3)

[{⟨1, 1⟩},{⟨27809, 1⟩}],[{⟨1, 1⟩}],[(27809)],[{⟨1, 1⟩}], [(102, 4),(4, 102)]

---

su(2) ← sp(13920)
so(27840)   su(27840)
su(3)

[{⟨1, 1⟩},{⟨27839, 1⟩}],[{⟨1, 1⟩}],[(27839)],[{⟨1, 1⟩}], [(115, 3),(3, 115)]

---

su(2) ← sp(13923)   su(27846)
so(7)
sp(3)   so(27846)

[{⟨1, 1⟩},{⟨27845, 1⟩}],[{⟨1, 1⟩}],[(27845)],[{⟨1, 1⟩}], [(1, 5, 0)],[(8, 2, 0)]

---

su(2) ← sp(13944)
su(167) ← so(27888)   su(27888)
su(3)

[{⟨1, 1⟩},{⟨27887, 1⟩}],[{⟨1, 1⟩}],[(27887)],[{⟨1, 1⟩}], [{⟨1, 1⟩, ⟨166, 1⟩}],[(165, 1),(1, 165)]

---

su(2) ← so(27945)
su(3)   su(27945)
su(3)

[{⟨1, 1⟩},{⟨27944, 1⟩}], [{⟨1, 1⟩}], [(27944)], [(53, 14), (14, 53)],[(134, 2),(2, 134)]

---

su(2) ← so(27951)   su(27951)
su(3)

[{⟨1, 1⟩},{⟨27950, 1⟩}], [{⟨1, 1⟩}], [(27950)], [(65, 10), (10, 65)]

---

su(2)
so(236)   so(27965) ← su(27965)

[{⟨1, 1⟩},{⟨27964, 1⟩}],[{⟨1, 1⟩}],[(27964)],[{⟨1, 2⟩}]

---

su(2) ← sp(13983)
so(237)
sp(118)   so(27966)
su(3)   su(27966)
su(236)
su(237)

[{⟨1, 1⟩},{⟨27965, 1⟩}],[{⟨1, 1⟩}],[(27965)],[{⟨1, 1⟩}], [{⟨2, 1⟩}], [{⟨1, 2⟩}], [(235, 0),(0, 235)], [{⟨1, 2⟩}, {⟨235, 2⟩}],[{⟨2, 1⟩},{⟨235, 1⟩}]

---

su(2) ← so(27993)   su(27993)
su(3)

[{⟨1, 1⟩},{⟨27992, 1⟩}], [{⟨1, 1⟩}], [(27992)], [(85, 6), (6, 85)]

---

su(2) ← so(27999)   su(27999)
su(3)

[{⟨1, 1⟩},{⟨27998, 1⟩}], [{⟨1, 1⟩}], [(27998)], [(33, 26), (26, 33)]

---

su(2) ← sp(14000)
so(28000)
su(3)   su(28000)
su(5)
su(5)
su(5)

[{⟨1, 1⟩},{⟨27999, 1⟩}],[{⟨1, 1⟩}],[(27999)],[{⟨1, 1⟩}], [(69, 9),(9, 69)], [(3, 0, 4, 1),(1, 4, 0, 3)], [(4, 2, 1, 1),(1, 1, 2, 4)],[(9, 3, 0, 0),(0, 0, 3, 9)]

---

su(2)
sp(5)   sp(14014)   su(28028)
so(28028)

[{⟨1, 1⟩},{⟨28027, 1⟩}],[{⟨1, 1⟩}],[(28027)],[(1, 0, 2, 0, 0)],[{⟨1, 1⟩}]

---

su(2) ← sp(14040)
so(28080)   su(28080)
su(4)

[{⟨1, 1⟩},{⟨28079, 1⟩}],[{⟨1, 1⟩}],[(28079)],[{⟨1, 1⟩}], [(2, 12, 1),(1, 12, 2)]

---

su(2) ← sp(14060)
so(28120)
su(4)   su(28120)
su(38)

[{⟨1, 1⟩},{⟨28119, 1⟩}],[{⟨1, 1⟩}],[(28119)],[{⟨1, 1⟩}], [(36, 0, 1),(1, 0, 36)], [{⟨1, 2⟩, ⟨37, 1⟩},{⟨1, 1⟩, ⟨37, 2⟩}]

---

su(2) ← sp(14080)
sp(5)
so(10)   so(28160)
su(3)   su(28160)
su(3)
su(4)

[{⟨1, 1⟩},{⟨28159, 1⟩}],[{⟨1, 1⟩}],[(28159)],[{⟨1, 1⟩}], [(1, 1, 0, 0, 1)], [(3, 0, 0, 1, 1)], [(43, 19),(19, 43)], [(79, 7),(7, 79)],[(15, 3, 1),(1, 3, 15)]

---

su(2) ← sp(14091)
so(28182)   su(28182)
su(3)

[{⟨1, 1⟩},{⟨28181, 1⟩}],[{⟨1, 1⟩}],[(28181)],[{⟨1, 1⟩}], [(32, 27),(27, 32)]

---

su(2) ← sp(14100)
so(28200)   su(28200)
su(3)

[{⟨1, 1⟩},{⟨28199, 1⟩}],[{⟨1, 1⟩}],[(28199)],[{⟨1, 1⟩}], [(93, 5),(5, 93)]

---

su(2) ← sp(14101)   su(28202)
so(237)
sp(119)   so(28202)

[{⟨1, 1⟩},{⟨28201, 1⟩}],[{⟨1, 1⟩}],[(28201)],[{⟨1, 1⟩}], [{⟨1, 2⟩}],[{⟨2, 1⟩}]

---

su(2)
so(238)   so(28203)
su(3)   su(28203)
su(237)
su(238)

[{⟨1, 1⟩},{⟨28202, 1⟩}],[{⟨1, 1⟩}],[(28202)],[{⟨2, 1⟩}], [(236, 0),(0, 236)], [{⟨1, 2⟩},{⟨236, 2⟩}], [{⟨2, 1⟩}, {⟨236, 1⟩}]

---

su(2) ← sp(14105)   su(28210)
so(5) ← so(28210)

[{⟨1, 1⟩},{⟨28209, 1⟩}],[{⟨1, 1⟩}],[(28209)],[{⟨1, 1⟩}],

[⟨3, 30⟩]

---

su(2), su(168) ← so(28223)
so(28223), su(3) ← su(28223)

[{⟨1, 1⟩},{⟨28222, 1⟩}], [{⟨1, 1⟩}], [(28222)], [{⟨1, 1⟩, ⟨167, 1⟩}],[(166, 1),(1, 166)]

---

su(2) ← sp(14112)
su(5), so(7) ← so(28224)
sp(14112), so(28224) ← su(28224)

[{⟨1, 1⟩},{⟨28223, 1⟩}],[{⟨1, 1⟩}],[(28223)],[{⟨1, 1⟩}], [(6, 0, 0, 6)],[(0, 5, 1)]

---

su(2) ← sp(14136)
sp(14136), so(28272), su(3) ← su(28272)

[{⟨1, 1⟩},{⟨28271, 1⟩}],[{⟨1, 1⟩}],[(28271)],[{⟨1, 1⟩}], [(37, 23),(23, 37)]

---

su(2) ← sp(14144)
sp(14144), so(28288), su(3) ← su(28288)

[{⟨1, 1⟩},{⟨28287, 1⟩}],[{⟨1, 1⟩}],[(28287)],[{⟨1, 1⟩}], [(51, 15),(15, 51)]

---

su(2) ← sp(14152)
so(5) ← so(28304)
sp(14152), so(28304), su(3) ← su(28304)

[{⟨1, 1⟩},{⟨28303, 1⟩}],[{⟨1, 1⟩}],[(28303)],[{⟨1, 1⟩}], [(28, 2)],[(31, 28),(28, 31)]

---

su(2), so(5) ← so(28305) ← su(28305)

[{⟨1, 1⟩},{⟨28304, 1⟩}],[{⟨1, 1⟩}],[(28304)],[(9, 16)]

---

su(2) ← sp(14157)
so(9), so(12) ← so(28314)
so(11) ← so(12)
sp(14157), so(28314), su(3), so(10) ← su(28314)

[{⟨1, 1⟩},{⟨28313, 1⟩}],[{⟨1, 1⟩}],[(28313)],[{⟨1, 1⟩}], [(0, 0, 0, 6)], [{⟨5, 4⟩},{⟨6, 4⟩}], [(0, 0, 0, 0, 4)], [(116, 3),(3, 116)],[(0, 0, 0, 6, 0),(0, 0, 0, 0, 6)]

---

su(2) ← so(28329)
so(28329), su(3) ← su(28329)

[{⟨1, 1⟩},{⟨28328, 1⟩}], [{⟨1, 1⟩}], [(28328)], [(56, 13), (13, 56)]

---

su(2), sp(2), sp(22) ← sp(14168)
so(44) ← so(28336)
sp(14168), so(28336), su(4) ← su(28336)

[{⟨1, 1⟩},{⟨28335, 1⟩}], [{⟨1, 1⟩}], [(28335)], [(41, 1)], [{⟨1, 1⟩, ⟨2, 1⟩}],[{⟨1, 1⟩}],[{⟨1, 1⟩, ⟨2, 1⟩}],[(15, 5, 0), (0, 5, 15)]

---

su(2) ← sp(14170)
sp(14170), so(28340), su(3) ← su(28340)

[{⟨1, 1⟩},{⟨28339, 1⟩}],[{⟨1, 1⟩}],[(28339)],[{⟨1, 1⟩}], [(103, 4),(4, 103)]

---

su(2) ← sp(14175)
sp(14175), so(28350), su(3), su(3) ← su(28350)

[{⟨1, 1⟩},{⟨28349, 1⟩}],[{⟨1, 1⟩}],[(28349)],[{⟨1, 1⟩}], [(62, 11),(11, 62)],[(74, 8),(8, 74)]

---

su(2) ← sp(14178)
sp(14178), so(28356), su(3) ← su(28356)

[{⟨1, 1⟩},{⟨28355, 1⟩}],[{⟨1, 1⟩}],[(28355)],[{⟨1, 1⟩}], [(135, 2),(2, 135)]

---

su(2) ← so(28365)
so(28365), su(3) ← su(28365)

[{⟨1, 1⟩},{⟨28364, 1⟩}], [{⟨1, 1⟩}], [(28364)], [(30, 29), (29, 30)]

---

su(2) ← sp(14190)
sp(14190), so(28380), su(44) ← su(28380)

[{⟨1, 1⟩},{⟨28379, 1⟩}],[{⟨1, 1⟩}],[(28379)],[{⟨1, 1⟩}], [{⟨1, 1⟩, ⟨2, 1⟩},{⟨42, 1⟩, ⟨43, 1⟩}]

---

su(2) ← so(28405)
so(28405), su(3) ← su(28405)

[{⟨1, 1⟩},{⟨28404, 1⟩}], [{⟨1, 1⟩}], [(28404)], [(45, 18), (18, 45)]

---

su(2) ← so(28413)
so(28413), su(3) ← su(28413)

[{⟨1, 1⟩},{⟨28412, 1⟩}], [{⟨1, 1⟩}], [(28412)], [(40, 21), (21, 40)]

---

su(2) ← sp(14212)
sp(14212), so(28424), su(4) ← su(28424)

[{⟨1, 1⟩},{⟨28423, 1⟩}],[{⟨1, 1⟩}],[(28423)],[{⟨1, 1⟩}], [(10, 5, 1),(1, 5, 10)]

---

su(2) ← sp(14220)
so(238) ← so(28440)
sp(14220), so(28440) ← su(28440)

[{⟨1, 1⟩},{⟨28439, 1⟩}],[{⟨1, 1⟩}],[(28439)],[{⟨1, 1⟩}], [{⟨1, 2⟩}]

---

su(2), so(239), sp(119) ← so(28441)
so(28441), su(3), su(238), su(239) ← su(28441)

[{⟨1, 1⟩},{⟨28440, 1⟩}],[{⟨1, 1⟩}],[(28440)],[{⟨2, 1⟩}], [{⟨1, 2⟩}], [(237, 0),(0, 237)], [{⟨1, 2⟩},{⟨237, 2⟩}], [{⟨2, 1⟩},{⟨237, 1⟩}]

---

su(2) ← sp(14235)
sp(14235), so(28470), su(3) ← su(28470)

[{⟨1, 1⟩},{⟨28469, 1⟩}],[{⟨1, 1⟩}],[(28469)],[{⟨1, 1⟩}], [(59, 12),(12, 59)]

---

su(2) ← so(28475)
so(28475), su(3) ← su(28475)

[{⟨1, 1⟩},{⟨28474, 1⟩}], [{⟨1, 1⟩}], [(28474)], [(49, 16), (16, 49)]

---

su(2) ← sp(14250)
sp(14250), so(28500), su(4), su(4) ← su(28500)

[{⟨1, 1⟩},{⟨28499, 1⟩}],[{⟨1, 1⟩}],[(28499)],[{⟨1, 1⟩}], [(9, 8, 0),(0, 8, 9)],[(18, 4, 0),(0, 4, 18)]

---

su(2), so(5) ← so(28509) ← su(28509)

[{⟨1, 1⟩},{⟨28508, 1⟩}],[{⟨1, 1⟩}],[(28508)],[(16, 8)]

---

su(2), so(11) ← sp(14256)
so(8) ← so(28512)
sp(14256), so(28512), su(3) ← su(28512)

[{⟨1, 1⟩},{⟨28511, 1⟩}],[{⟨1, 1⟩}],[(28511)],[(1, 0, 1, 0, 1)], [{⟨1, 1⟩}], [(4, 0, 2, 1),(4, 0, 1, 2),(2, 0, 4, 1),(2, 0, 1, 4),(1, 0, 4, 2),(1, 0, 2, 4)],[(47, 17),(17, 47)]

---

su(2), sp(2) ← sp(14280)
su(169) ← so(28560)
sp(14280), so(28560), su(3), su(6), su(16) ← su(28560)

[{⟨1, 1⟩},{⟨28559, 1⟩}], [{⟨1, 1⟩}], [(28559)], [(1, 33)], [{⟨1, 1⟩}], [{⟨1, 1⟩, ⟨168, 1⟩}], [(167, 1),(1, 167)], [(11, 1, 0, 0, 0),(0, 0, 0, 1, 11)], [{⟨1, 1⟩, ⟨12, 1⟩},{⟨4, 1⟩, ⟨15, 1⟩}]

---

su(2), so(5) ← so(28561) ← su(28561)

[{⟨1, 1⟩},{⟨28560, 1⟩}],[{⟨1, 1⟩}],[(28560)],[(12, 12)]

---

su(2) ← sp(14300)
sp(14300), so(28600), su(5) ← su(28600)

[{⟨1, 1⟩},{⟨28599, 1⟩}],[{⟨1, 1⟩}],[(28599)],[{⟨1, 1⟩}], [(10, 1, 1, 0),(0, 1, 1, 10)]

---

su(2) ← so(28623)
so(28623), su(3) ← su(28623)

[{⟨1, 1⟩},{⟨28622, 1⟩}], [{⟨1, 1⟩}], [(28622)], [(86, 6), (6, 86)]

---

su(2) ← sp(14326)
g2 ← so(28652)
sp(14326), so(28652) ← su(28652)

[{⟨1, 1⟩},{⟨28651, 1⟩}],[{⟨1, 1⟩}],[(28651)],[{⟨1, 1⟩}], [(9, 2)]

---

su(2) ← so(28665)
so(28665), su(5), su(5) ← su(28665)

[{⟨1, 1⟩},{⟨28664, 1⟩}], [{⟨1, 1⟩}], [(28664)], [(5, 0, 2, 2),(2, 2, 0, 5)],[(5, 0, 4, 0),(0, 4, 0, 5)]

---

su(2) ← sp(14336)
sp(3), g2 ← so(28672)
sp(14336), so(28672) ← su(28672)

[{⟨1, 1⟩},{⟨28671, 1⟩}],[{⟨1, 1⟩}],[(28671)],[{⟨1, 1⟩}], [(7, 1, 1)],[(7, 3)]

---

su(2), so(5) ← so(28675)
so(28675), su(3) ← su(28675)

[{⟨1, 1⟩},{⟨28674, 1⟩}], [{⟨1, 1⟩}], [(28674)], [(5, 24)], [(36, 24),(24, 36)]

---

su(2), so(239), sp(120) ← so(28679) ← su(28679)

[{⟨1, 1⟩},{⟨28678, 1⟩}],[{⟨1, 1⟩}],[(28678)],[{⟨1, 2⟩}], [{⟨2, 1⟩}]

---

su(2) ← sp(14340)
so(240) ← so(28680)
sp(14340), so(28680), su(3), su(239), su(240) ← su(28680)

[{⟨1, 1⟩},{⟨28679, 1⟩}],[{⟨1, 1⟩}],[(28679)],[{⟨1, 1⟩}], [{⟨2, 1⟩}], [(238, 0),(0, 238)], [{⟨1, 2⟩},{⟨238, 2⟩}], [{⟨2, 1⟩},{⟨238, 1⟩}]

---

su(2) ← sp(14355)
sp(14355), so(28710), su(4) ← su(28710)

[{⟨1, 1⟩},{⟨28709, 1⟩}],[{⟨1, 1⟩}],[(28709)],[{⟨1, 1⟩}], [(28, 0, 2),(2, 0, 28)]

su(2) ⟵ so(28743) ⟵ su(28743)
su(3) ⟵ su(28743)

[{⟨1, 1⟩},{⟨28742, 1⟩}], [{⟨1, 1⟩}], [(28742)], [(66, 10), (10, 66)]

su(2) ⟵ sp(14375) ⟵ su(28750)
so(28750) ⟵ su(28750)
su(4) ⟵ su(28750)

[{⟨1, 1⟩},{⟨28749, 1⟩}],[{⟨1, 1⟩}],[(28749)],[{⟨1, 1⟩}], [(19, 2, 1),(1, 2, 19)]

su(2) ⟵ so(28755) ⟵ su(28755)
su(3) ⟵ su(28755)

[{⟨1, 1⟩},{⟨28754, 1⟩}], [{⟨1, 1⟩}], [(28754)], [(70, 9), (9, 70)]

su(2) ⟵ sp(14385) ⟵ su(28770)
so(28770) ⟵ su(28770)
su(3) ⟵ su(28770)

[{⟨1, 1⟩},{⟨28769, 1⟩}],[{⟨1, 1⟩}],[(28769)],[{⟨1, 1⟩}], [(136, 2),(2, 136)]

su(2) ⟵ so(28785) ⟵ su(28785)
su(3) ⟵ su(28785)

[{⟨1, 1⟩},{⟨28784, 1⟩}], [{⟨1, 1⟩}], [(28784)], [(94, 5), (5, 94)]

su(2) ⟵ sp(14396) ⟵ su(28792)
so(28792) ⟵ su(28792)
su(3) ⟵ su(28792)

[{⟨1, 1⟩},{⟨28791, 1⟩}],[{⟨1, 1⟩}],[(28791)],[{⟨1, 1⟩}], [(117, 3),(3, 117)]

su(2) ⟵ sp(14399) ⟵ su(28798)
so(11) ⟵ so(28798) ⟵ su(28798)

[{⟨1, 1⟩},{⟨28797, 1⟩}],[{⟨1, 1⟩}],[(28797)],[{⟨1, 1⟩}], [(2, 2, 0, 0, 0)]

su(2) ⟵ sp(14418) ⟵ su(28836)
so(28836) ⟵ su(28836)
su(3) ⟵ su(28836)

[{⟨1, 1⟩},{⟨28835, 1⟩}],[{⟨1, 1⟩}],[(28835)],[{⟨1, 1⟩}], [(80, 7),(7, 80)]

su(2) ⟵ sp(14430) ⟵ su(28860)
so(28860) ⟵ su(28860)
su(4) ⟵ su(28860)
su(39) ⟵ su(28860)

[{⟨1, 1⟩},{⟨28859, 1⟩}],[{⟨1, 1⟩}],[(28859)],[{⟨1, 1⟩}], [(36, 1, 0),(0, 1, 36)], [{⟨1, 1⟩, ⟨37, 1⟩},{⟨2, 1⟩, ⟨38, 1⟩}]

su(2) ⟵ so(28875) ⟵ su(28875)
su(3) ⟵ su(28875)
su(3) ⟵ su(28875)
su(6) ⟵ su(28875)
su(7) ⟵ su(28875)

[{⟨1, 1⟩},{⟨28874, 1⟩}], [{⟨1, 1⟩}], [(28874)], [(54, 14), (14, 54)], [(104, 4),(4, 104)], [(3, 0, 3, 0, 0),(0, 0, 3, 0, 3)],[{⟨1, 3⟩, ⟨4, 2⟩},{⟨3, 2⟩, ⟨6, 3⟩}]

su(2) ⟵ sp(14440) ⟵ su(28880)
su(19) ⟵ so(28880) ⟵ su(28880)

[{⟨1, 1⟩},{⟨28879, 1⟩}],[{⟨1, 1⟩}],[(28879)],[{⟨1, 1⟩}], [{⟨2, 1⟩, ⟨17, 1⟩}]

su(2) ⟵ sp(14448) ⟵ su(28896)
so(28896) ⟵ su(28896)
su(3) ⟵ su(28896)

[{⟨1, 1⟩},{⟨28895, 1⟩}],[{⟨1, 1⟩}],[(28895)],[{⟨1, 1⟩}], [(42, 20),(20, 42)]

su(2) ⟵ so(28899) ⟵ su(28899)
su(170) ⟵ so(28899)
su(3) ⟵ su(28899)

[{⟨1, 1⟩},{⟨28898, 1⟩}], [{⟨1, 1⟩}], [(28898)], [{⟨1, 1⟩, ⟨169, 1⟩}],[(168, 1),(1, 168)]

su(2) ⟵ so(28917) ⟵ su(28917)
su(18) ⟵ so(28917)

[{⟨1, 1⟩},{⟨28916, 1⟩}], [{⟨1, 1⟩}], [(28916)], [{⟨1, 2⟩, ⟨17, 2⟩}]

su(2) ⟵ so(28919) ⟵ su(28919)
so(240) ⟵ so(28919)

[{⟨1, 1⟩},{⟨28918, 1⟩}],[{⟨1, 1⟩}],[(28918)],[{⟨1, 2⟩}]

su(2) ⟵ sp(14460) ⟵ su(28920)
so(241) ⟵ so(28920) ⟵ su(28920)
sp(120) ⟵ so(28920)
su(3) ⟵ su(28920)
su(240) ⟵ su(28920)
su(241) ⟵ su(28920)

[{⟨1, 1⟩},{⟨28919, 1⟩}],[{⟨1, 1⟩}],[(28919)],[{⟨1, 1⟩}], [{⟨2, 1⟩}], [{⟨1, 2⟩}], [(239, 0),(0, 239)], [{⟨1, 2⟩}, {⟨239, 2⟩}],[{⟨2, 1⟩},{⟨239, 1⟩}]

su(2) ⟵ sp(14490) ⟵ su(28980)
so(28980) ⟵ su(28980)
su(3) ⟵ su(28980)
su(4) ⟵ su(28980)
su(4) ⟵ su(28980)

[{⟨1, 1⟩},{⟨28979, 1⟩}],[{⟨1, 1⟩}],[(28979)],[{⟨1, 1⟩}], [(39, 22),(22, 39)], [(13, 0, 7),(7, 0, 13)], [(22, 3, 0),(0, 3, 22)]

su(2) ⟵ sp(14500) ⟵ su(29000)
so(29000) ⟵ su(29000)
su(4) ⟵ su(29000)

[{⟨1, 1⟩},{⟨28999, 1⟩}],[{⟨1, 1⟩}],[(28999)],[{⟨1, 1⟩}], [(23, 0, 3),(3, 0, 23)]

su(2) ⟵ sp(14508) ⟵ su(29016)
so(29016) ⟵ su(29016)
su(3) ⟵ su(29016)

[{⟨1, 1⟩},{⟨29015, 1⟩}],[{⟨1, 1⟩}],[(29015)],[{⟨1, 1⟩}], [(35, 25),(25, 35)]

su(2) ⟵ sp(14520) ⟵ su(29040)
so(29040) ⟵ su(29040)
su(11) ⟵ su(29040)

[{⟨1, 1⟩},{⟨29039, 1⟩}],[{⟨1, 1⟩}],[(29039)],[{⟨1, 1⟩}], [{⟨3, 1⟩, ⟨4, 1⟩},{⟨7, 1⟩, ⟨8, 1⟩}]

su(2) ⟵ sp(14535) ⟵ su(29070)
so(29070) ⟵ su(29070)
su(3) ⟵ su(29070)

[{⟨1, 1⟩},{⟨29069, 1⟩}],[{⟨1, 1⟩}],[(29069)],[{⟨1, 1⟩}], [(75, 8),(8, 75)]

su(2) ⟵ sp(14553) ⟵ su(29106)
sp(4) ⟵ so(29106) ⟵ su(29106)
su(6) ⟵ su(29106)
su(7) ⟵ su(29106)

[{⟨1, 1⟩},{⟨29105, 1⟩}],[{⟨1, 1⟩}],[(29105)],[{⟨1, 1⟩}], [(1, 2, 1, 0)], [(1, 4, 0, 0, 1),(1, 0, 0, 4, 1)], [{⟨1, 1⟩, ⟨2, 3⟩, ⟨6, 1⟩},{⟨1, 1⟩, ⟨5, 3⟩, ⟨6, 1⟩}]

su(2) ⟵ sp(14560) ⟵ su(29120)
sp(2) ⟵ sp(14560)
sp(2) ⟵ sp(14560)
sp(2) ⟵ sp(14560)
so(7) ⟵ so(29120) ⟵ su(29120)
su(4) ⟵ su(29120)
su(4) ⟵ su(29120)
so(14) ⟵ su(29120)

[{⟨1, 1⟩},{⟨29119, 1⟩}], [{⟨1, 1⟩}], [(29119)], [(3, 25)], [(9, 15)],[(11, 13)],[{⟨1, 1⟩}],[(6, 0, 3)],[(12, 2, 3),(3, 2, 12)], [(25, 1, 1),(1, 1, 25)], [{⟨1, 3⟩, ⟨6, 1⟩},{⟨1, 3⟩, ⟨7, 1⟩}]

su(2) ⟵ so(29155) ⟵ su(29155)
su(4) ⟵ su(29155)

[{⟨1, 1⟩},{⟨29154, 1⟩}], [{⟨1, 1⟩}], [(29154)], [(6, 6, 2), (2, 6, 6)]

su(2) ⟵ sp(14580) ⟵ su(29160)
so(241) ⟵ so(29160) ⟵ su(29160)
sp(121) ⟵ so(29160)
su(5) ⟵ su(29160)

[{⟨1, 1⟩},{⟨29159, 1⟩}],[{⟨1, 1⟩}],[(29159)],[{⟨1, 1⟩}], [{⟨1, 2⟩}],[{⟨2, 1⟩}],[(2, 4, 0, 2),(2, 0, 4, 2)]

su(2) ⟵ so(29161) ⟵ su(29161)
so(242) ⟵ so(29161)
su(3) ⟵ su(29161)
su(241) ⟵ su(29161)
su(242) ⟵ su(29161)

[{⟨1, 1⟩},{⟨29160, 1⟩}],[{⟨1, 1⟩}],[(29160)],[{⟨2, 1⟩}], [(240, 0),(0, 240)], [{⟨1, 2⟩},{⟨240, 2⟩}], [{⟨2, 1⟩}, {⟨240, 1⟩}]

su(2) ⟵ sp(14586) ⟵ su(29172)
$\mathfrak{f}_4$ ⟵ so(29172) ⟵ su(29172)

[{⟨1, 1⟩},{⟨29171, 1⟩}],[{⟨1, 1⟩}],[(29171)],[{⟨1, 1⟩}], [(1, 1, 0, 0)]

su(2) ⟵ sp(14592) ⟵ su(29184)
so(29184) ⟵ su(29184)
su(3) ⟵ su(29184)

[{⟨1, 1⟩},{⟨29183, 1⟩}],[{⟨1, 1⟩}],[(29183)],[{⟨1, 1⟩}], [(63, 11),(11, 63)]

su(2) ⟵ so(29187) ⟵ su(29187)
su(3) ⟵ su(29187)

[{⟨1, 1⟩},{⟨29186, 1⟩}], [{⟨1, 1⟩}], [(29186)], [(137, 2), (2, 137)]

su(2) ⟵ so(29205) ⟵ su(29205)
so(55) ⟵ so(29205)

[{⟨1, 1⟩},{⟨29204, 1⟩}],[{⟨1, 1⟩}],[(29204)],[{⟨1, 3⟩}]

su(2) ⟵ sp(14616) ⟵ su(29232)
so(29232) ⟵ su(29232)
su(3) ⟵ su(29232)

[{⟨1, 1⟩},{⟨29231, 1⟩}],[{⟨1, 1⟩}],[(29231)],[{⟨1, 1⟩}], [(57, 13),(13, 57)]

su(2) ⟵ sp(14620) ⟵ su(29240)
su(171) ⟵ so(29240) ⟵ su(29240)
su(3) ⟵ su(29240)

[{⟨1, 1⟩},{⟨29239, 1⟩}],[{⟨1, 1⟩}],[(29239)],[{⟨1, 1⟩}], [{⟨1, 1⟩, ⟨170, 1⟩}],[(169, 1),(1, 169)]

su(2) ⟵ sp(14625) ⟵ su(29250)
so(29250) ⟵ su(29250)
su(3) ⟵ su(29250)

[{⟨1, 1⟩},{⟨29249, 1⟩}],[{⟨1, 1⟩}],[(29249)],[{⟨1, 1⟩}], [(44, 19),(19, 44)]

su(2) ← sp(14628)
so(29256) ← su(29256)
su(3)

[{⟨1, 1⟩},{⟨29255, 1⟩}],[{⟨1, 1⟩}],[(29255)],[{⟨1, 1⟩}],[(52, 15),(15, 52)]

---

su(2), sp(2) ← sp(14630)
so(5), so(57) ← so(29260)
su(3), su(4), su(4), su(4), su(55), su(57) ← su(29260)

[{⟨1, 1⟩},{⟨29259, 1⟩}], [{⟨1, 1⟩}], [(29259)], [(27, 4)], [{⟨1, 1⟩}], [(0, 54)], [{⟨3, 1⟩}], [(87, 6),(6, 87)], [(1, 18, 0),(0, 18, 1)], [(10, 2, 4),(4, 2, 10)], [(54, 0, 0),(0, 0, 54)],[{⟨1, 3⟩},{⟨54, 3⟩}],[{⟨3, 1⟩},{⟨54, 1⟩}]

---

su(2) ← sp(14637)
so(29274) ← su(29274)
su(3)

[{⟨1, 1⟩},{⟨29273, 1⟩}],[{⟨1, 1⟩}],[(29273)],[{⟨1, 1⟩}],[(118, 3),(3, 118)]

---

su(2) ← so(29295)
su(3) ← su(29295)

[{⟨1, 1⟩},{⟨29294, 1⟩}], [{⟨1, 1⟩}], [(29294)], [(34, 26),(26, 34)]

---

su(2), so(5) ← so(29315) ← su(29315)

[{⟨1, 1⟩},{⟨29314, 1⟩}],[{⟨1, 1⟩}],[(29314)],[(14, 10)]

---

su(2) ← so(29341)
su(3) ← su(29341)

[{⟨1, 1⟩},{⟨29340, 1⟩}], [{⟨1, 1⟩}], [(29340)], [(60, 12),(12, 60)]

---

su(2) ← sp(14685)
so(5) ← so(29370)
← su(29370)

[{⟨1, 1⟩},{⟨29369, 1⟩}],[{⟨1, 1⟩}],[(29369)],[{⟨1, 1⟩}],[(43, 0)]

---

su(2) ← sp(14688)
so(29376) ← su(29376)
su(3)

[{⟨1, 1⟩},{⟨29375, 1⟩}],[{⟨1, 1⟩}],[(29375)],[{⟨1, 1⟩}],[(95, 5),(5, 95)]

---

su(2) ← sp(14701)
so(242) ← so(29402)
← su(29402)

[{⟨1, 1⟩},{⟨29401, 1⟩}],[{⟨1, 1⟩}],[(29401)],[{⟨1, 1⟩}],[{⟨1, 2⟩}]

---

su(2), so(243), sp(121) ← so(29403)
su(3), su(242), su(243) ← su(29403)

[{⟨1, 1⟩},{⟨29402, 1⟩}],[{⟨1, 1⟩}],[(29402)],[{⟨2, 1⟩}],[{⟨1, 2⟩}], [(241, 0),(0, 241)], [{⟨1, 2⟩},{⟨241, 2⟩}],[{⟨2, 1⟩},{⟨241, 1⟩}]

---

su(2) ← so(29415)
su(3) ← su(29415)

[{⟨1, 1⟩},{⟨29414, 1⟩}], [{⟨1, 1⟩}], [(29414)], [(105, 4),(4, 105)]

---

su(2) ← so(29469)
su(3) ← su(29469)

[{⟨1, 1⟩},{⟨29468, 1⟩}], [{⟨1, 1⟩}], [(29468)], [(46, 18),(18, 46)]

---

su(2) ← sp(14739)
so(29478) ← su(29478)
su(3)

[{⟨1, 1⟩},{⟨29477, 1⟩}],[{⟨1, 1⟩}],[(29477)],[{⟨1, 1⟩}],[(50, 16),(16, 50)]

---

su(2), sp(2) ← sp(14742)
so(29484) ← su(29484)
su(3)

[{⟨1, 1⟩},{⟨29483, 1⟩}], [{⟨1, 1⟩}], [(29483)], [(35, 2)], [{⟨1, 1⟩}],[(38, 23),(23, 38)]

---

su(2) ← sp(14756)
so(29512) ← su(29512)
su(3)

[{⟨1, 1⟩},{⟨29511, 1⟩}],[{⟨1, 1⟩}],[(29511)],[{⟨1, 1⟩}],[(33, 27),(27, 33)]

---

su(2) ← sp(14760)
so(29520)
su(3)
su(3)
← su(29520)

[{⟨1, 1⟩},{⟨29519, 1⟩}],[{⟨1, 1⟩}],[(29519)],[{⟨1, 1⟩}],[(71, 9),(9, 71)],[(81, 7),(7, 81)]

---

su(2) ← sp(14763)
so(5) ← so(29526)
← su(29526)

[{⟨1, 1⟩},{⟨29525, 1⟩}],[{⟨1, 1⟩}],[(29525)],[{⟨1, 1⟩}],[(8, 18)]

---

su(2) ← sp(14773)
so(29546) ← su(29546)
su(3)

[{⟨1, 1⟩},{⟨29545, 1⟩}],[{⟨1, 1⟩}],[(29545)],[{⟨1, 1⟩}],[(67, 10),(10, 67)]

---

su(2) ← so(29547)
su(3) ← su(29547)

[{⟨1, 1⟩},{⟨29546, 1⟩}], [{⟨1, 1⟩}], [(29546)], [(48, 17),(17, 48)]

---

su(2) ← sp(14784)
so(29568)
su(3)
su(6) ← su(29568)
su(7)
su(9)
so(10)

[{⟨1, 1⟩},{⟨29567, 1⟩}],[{⟨1, 1⟩}],[(29567)],[{⟨1, 1⟩}],[(41, 21),(21, 41)],[(7, 1, 0, 0, 1),(1, 0, 0, 1, 7)],[{⟨1, 3⟩, ⟨2, 3⟩},{⟨5, 3⟩, ⟨6, 3⟩}], [{⟨1, 1⟩, ⟨4, 1⟩, ⟨7, 1⟩},{⟨2, 1⟩, ⟨5, 1⟩, ⟨8, 1⟩}],[(0, 0, 1, 3, 0),(0, 0, 1, 0, 3)]

---

su(2), su(172) ← so(29583)
su(3) ← su(29583)

[{⟨1, 1⟩},{⟨29582, 1⟩}], [{⟨1, 1⟩}], [(29582)], [{⟨1, 1⟩, ⟨171, 1⟩}],[(170, 1),(1, 170)]

---

su(2) ← so(29607)
su(3) ← su(29607)

[{⟨1, 1⟩},{⟨29606, 1⟩}], [{⟨1, 1⟩}], [(29606)], [(138, 2),(2, 138)]

---

su(2) ← sp(14805)
so(5) ← so(29610)
← su(29610)

[{⟨1, 1⟩},{⟨29609, 1⟩}],[{⟨1, 1⟩}],[(29609)],[{⟨1, 1⟩}],[(19, 6)]

---

su(2), so(243), sp(122) ← so(29645) ← su(29645)

[{⟨1, 1⟩},{⟨29644, 1⟩}],[{⟨1, 1⟩}],[(29644)],[{⟨1, 2⟩}],[{⟨2, 1⟩}]

---

su(2) ← sp(14823)
so(244) ← so(29646)
su(3) ← su(29646)
su(243)
su(244)

[{⟨1, 1⟩},{⟨29645, 1⟩}],[{⟨1, 1⟩}],[(29645)],[{⟨1, 1⟩}],[{⟨2, 1⟩}], [(242, 0),(0, 242)], [{⟨1, 2⟩},{⟨242, 2⟩}],[{⟨2, 1⟩},{⟨242, 1⟩}]

---

su(2), $\mathfrak{g}_2$ ← so(29667)
su(3) ← su(29667)

[{⟨1, 1⟩},{⟨29666, 1⟩}], [{⟨1, 1⟩}], [(29666)], [(1, 8)],[(32, 28),(28, 32)]

---

su(2) ← sp(14850)
su(6), su(10), sp(4) ← so(29700)
su(8)
← su(29700)

[{⟨1, 1⟩},{⟨29699, 1⟩}],[{⟨1, 1⟩}],[(29699)],[{⟨1, 1⟩}],[(2, 1, 0, 1, 2)], [{⟨4, 1⟩, ⟨6, 1⟩}], [(4, 2, 0, 0)], [{⟨1, 2⟩, ⟨2, 1⟩, ⟨4, 1⟩},{⟨4, 1⟩, ⟨6, 1⟩, ⟨7, 2⟩}]

---

su(2) ← sp(14858)
so(29716) ← su(29716)
su(4)

[{⟨1, 1⟩},{⟨29715, 1⟩}],[{⟨1, 1⟩}],[(29715)],[{⟨1, 1⟩}],[(16, 1, 3),(3, 1, 16)]

---

su(2) ← sp(14875)
so(29750) ← su(29750)
su(4)

[{⟨1, 1⟩},{⟨29749, 1⟩}],[{⟨1, 1⟩}],[(29749)],[{⟨1, 1⟩}],[(6, 4, 4),(4, 4, 6)]

---

su(2) ← sp(14880)
so(29760)
su(3)
su(3)
← su(29760)

[{⟨1, 1⟩},{⟨29759, 1⟩}],[{⟨1, 1⟩}],[(29759)],[{⟨1, 1⟩}],[(31, 29),(29, 31)],[(119, 3),(3, 119)]

---

su(2), so(5) ← so(29785) ← su(29785)

[{⟨1, 1⟩},{⟨29784, 1⟩}],[{⟨1, 1⟩}],[(29784)],[(6, 22)]

---

su(2), su(3) ← so(29791) ← su(29791)

[{⟨1, 1⟩},{⟨29790, 1⟩}],[{⟨1, 1⟩}],[(29790)],[(30, 30)]

---

su(2) ← so(29799)
su(3) ← su(29799)

[{⟨1, 1⟩},{⟨29798, 1⟩}], [{⟨1, 1⟩}], [(29798)], [(76, 8),(8, 76)]

---

su(2) ← sp(14910)
so(29820) ← su(29820)
su(3)

[{⟨1, 1⟩},{⟨29819, 1⟩}],[{⟨1, 1⟩}],[(29819)],[{⟨1, 1⟩}],[(55, 14),(14, 55)]

---

su(2), sp(3) ← so(29835) ← su(29835)

[{⟨1, 1⟩},{⟨29834, 1⟩}],[{⟨1, 1⟩}],[(29834)],[(11, 0, 1)]

---

su(2), so(244) ← so(29889) ← su(29889)

[{⟨1, 1⟩},{⟨29888, 1⟩}],[{⟨1, 1⟩}],[(29888)],[{⟨1, 2⟩}]

su(2) ← sp(14945)
so(245), sp(122) → so(29890)
su(3), su(244), su(245)
su(29890)

[{⟨1, 1⟩},{⟨29889, 1⟩}],[{⟨1, 1⟩}],[(29889)],[{⟨1, 1⟩}],[{⟨2, 1⟩}], [{⟨1, 2⟩}], [(243, 0),(0, 243)], [{⟨1, 2⟩},{⟨243, 2⟩}],[{⟨2, 1⟩},{⟨243, 1⟩}]

su(2) ← sp(14952)
so(29904) — su(29904)
su(3)

[{⟨1, 1⟩},{⟨29903, 1⟩}],[{⟨1, 1⟩}],[(29903)],[{⟨1, 1⟩}],[(88, 6),(6, 88)]

su(2), so(7) → so(29925)
su(3) — su(29925)
su(4)

[{⟨1, 1⟩},{⟨29924, 1⟩}],[{⟨1, 1⟩}],[(29924)],[(4, 3, 0)],[(37, 24),(24, 37)],[(17, 0, 5),(5, 0, 17)]

su(2) ← sp(14964)
su(173) ← so(29928) — su(29928)
su(3)

[{⟨1, 1⟩},{⟨29927, 1⟩}],[{⟨1, 1⟩}],[(29927)],[{⟨1, 1⟩}],[{⟨1, 1⟩, ⟨172, 1⟩}],[(171, 1),(1, 171)]

su(2) ← sp(14976)
so(7) ← so(29952)
su(29952)

[{⟨1, 1⟩},{⟨29951, 1⟩}],[{⟨1, 1⟩}],[(29951)],[{⟨1, 1⟩}],[(2, 0, 7)]

su(2) ← sp(14980)
so(29960) — su(29960)
su(3)

[{⟨1, 1⟩},{⟨29959, 1⟩}],[{⟨1, 1⟩}],[(29959)],[{⟨1, 1⟩}],[(106, 4),(4, 106)]

su(2) ← so(29973)
su(3)
su(29973)

[{⟨1, 1⟩},{⟨29972, 1⟩}], [{⟨1, 1⟩}], [(29972)], [(96, 5),(5, 96)]

su(2) ← sp(15015)
so(30030)
su(3), su(3), su(3), su(4), su(5), su(6), su(6), su(7), su(7), su(10), su(11), su(12), su(12), su(13)
su(30030)

[{⟨1, 1⟩},{⟨30029, 1⟩}],[{⟨1, 1⟩}],[(30029)],[{⟨1, 1⟩}],[(43, 20),(20, 43)], [(64, 11),(11, 64)], [(139, 2),(2, 139)], [(10, 1, 6),(6, 1, 10)], [(7, 2, 1, 0),(0, 1, 2, 7)], [(5, 3, 0, 0, 0),(0, 0, 0, 3, 5)], [(6, 0, 1, 0, 1),(1, 0, 1, 0, 6)], [{⟨1, 5⟩, ⟨2, 1⟩, ⟨6, 1⟩},{⟨1, 1⟩, ⟨5, 1⟩, ⟨6, 5⟩}], [{⟨1, 7⟩, ⟨5, 1⟩},{⟨2, 1⟩, ⟨6, 7⟩}], [{⟨1, 4⟩, ⟨8, 1⟩},{⟨2, 1⟩, ⟨9, 4⟩}], [{⟨1, 3⟩, ⟨3, 1⟩},{⟨8, 1⟩, ⟨10, 3⟩}], [{⟨2, 1⟩, ⟨8, 1⟩},{⟨4, 1⟩, ⟨10, 1⟩}], [{⟨1, 2⟩, ⟨4, 1⟩},{⟨8, 1⟩, ⟨11, 2⟩}],[{⟨1, 1⟩, ⟨11, 2⟩},{⟨2, 2⟩, ⟨12, 1⟩}]

su(2) ← sp(15022)
so(5) ← so(30044)
su(30044)

[{⟨1, 1⟩},{⟨30043, 1⟩}],[{⟨1, 1⟩}],[(30043)],[{⟨1, 1⟩}],[(7, 20)]

su(2), sp(2) → sp(15048)
so(30096) — su(30096)
su(4)

[{⟨1, 1⟩},{⟨30095, 1⟩}],[{⟨1, 1⟩}],[(30095)],[(15, 10)],[{⟨1, 1⟩}],[(15, 2, 2),(2, 2, 15)]

su(2), $\mathfrak{g}_2$, $\mathfrak{g}_2$ → so(30107) ← su(30107)

[{⟨1, 1⟩},{⟨30106, 1⟩}], [{⟨1, 1⟩}], [(30106)], [(0, 10)], [(4, 5)]

su(2) ← sp(15067)
so(245), sp(123) → so(30134)
su(30134)

[{⟨1, 1⟩},{⟨30133, 1⟩}],[{⟨1, 1⟩}],[(30133)],[{⟨1, 1⟩}],[{⟨1, 2⟩}],[{⟨2, 1⟩}]

su(2), so(246) → so(30135)
su(3), su(245), su(246)
su(30135)

[{⟨1, 1⟩},{⟨30134, 1⟩}],[{⟨1, 1⟩}],[(30134)],[{⟨2, 1⟩}],[(244, 0),(0, 244)], [{⟨1, 2⟩},{⟨244, 2⟩}], [{⟨2, 1⟩},{⟨244, 1⟩}]

su(2) ← so(30149)
su(3)
su(30149)

[{⟨1, 1⟩},{⟨30148, 1⟩}], [{⟨1, 1⟩}], [(30148)], [(58, 13),(13, 58)]

su(2) ← sp(15088)
so(30176) — su(30176)
su(3)

[{⟨1, 1⟩},{⟨30175, 1⟩}],[{⟨1, 1⟩}],[(30175)],[{⟨1, 1⟩}],[(40, 22),(22, 40)]

su(2) ← sp(15092)
so(30184) — su(30184)
su(4)

[{⟨1, 1⟩},{⟨30183, 1⟩}],[{⟨1, 1⟩}],[(30183)],[{⟨1, 1⟩}],[(13, 6, 0),(0, 6, 13)]

su(2) ← sp(15106)
so(30212) — su(30212)
su(3)

[{⟨1, 1⟩},{⟨30211, 1⟩}],[{⟨1, 1⟩}],[(30211)],[{⟨1, 1⟩}],[(82, 7),(7, 82)]

su(2) ← so(30225)
su(3)
su(30225)

[{⟨1, 1⟩},{⟨30224, 1⟩}], [{⟨1, 1⟩}], [(30224)], [(61, 12),(12, 61)]

su(2) ← sp(15120)
so(30240)
su(3), su(4), su(5), su(5), su(5), su(6), su(7)
su(30240)

[{⟨1, 1⟩},{⟨30239, 1⟩}],[{⟨1, 1⟩}],[(30239)],[{⟨1, 1⟩}],[(53, 15),(15, 53)], [(11, 7, 0),(0, 7, 11)], [(2, 0, 5, 1),(1, 5, 0, 2)],[(5, 1, 0, 4),(4, 0, 1, 5)],[(7, 0, 2, 1),(1, 2, 0, 7)],[(0, 2, 3, 0, 0),(0, 0, 3, 2, 0)], [{⟨1, 4⟩, ⟨3, 1⟩, ⟨6, 1⟩},{⟨1, 1⟩, ⟨4, 1⟩, ⟨6, 4⟩}]

su(2) ← sp(15125)
so(30250) — su(30250)
su(3)

[{⟨1, 1⟩},{⟨30249, 1⟩}],[{⟨1, 1⟩}],[(30249)],[{⟨1, 1⟩}],[(120, 3),(3, 120)]

su(2), su(174) → so(30275)
su(3)
su(30275)

[{⟨1, 1⟩},{⟨30274, 1⟩}], [{⟨1, 1⟩}], [(30274)], [{⟨1, 1⟩, ⟨173, 1⟩}],[(172, 1),(1, 172)]

su(2) ← so(30295)
su(3)
su(30295)

[{⟨1, 1⟩},{⟨30294, 1⟩}], [{⟨1, 1⟩}], [(30294)], [(72, 9),(9, 72)]

su(2) ← so(30303)
su(3)
su(30303)

[{⟨1, 1⟩},{⟨30302, 1⟩}], [{⟨1, 1⟩}], [(30302)], [(36, 25),(25, 36)]

su(2), so(5), so(45) → so(30315) ← su(30315)

[{⟨1, 1⟩},{⟨30314, 1⟩}], [{⟨1, 1⟩}], [(30314)], [(1, 42)], [{⟨1, 1⟩, ⟨2, 1⟩}]

su(2) ← sp(15180)
so(30360)
su(3), su(3), su(45)
su(30360)

[{⟨1, 1⟩},{⟨30359, 1⟩}],[{⟨1, 1⟩}],[(30359)],[{⟨1, 1⟩}],[(45, 19),(19, 45)], [(68, 10),(10, 68)], [{⟨1, 1⟩, ⟨2, 1⟩},{⟨43, 1⟩, ⟨44, 1⟩}]

su(2) ← so(30375)
su(5)
su(30375)

[{⟨1, 1⟩},{⟨30374, 1⟩}], [{⟨1, 1⟩}], [(30374)], [(8, 0, 1, 2),(2, 1, 0, 8)]

su(2) ← sp(15190)
so(246), $\mathfrak{e}_8$ → so(30380)
su(30380)

[{⟨1, 1⟩},{⟨30379, 1⟩}],[{⟨1, 1⟩}],[(30379)],[{⟨1, 1⟩}],[{⟨1, 2⟩}],[{⟨7, 1⟩}]

su(2), so(247), sp(123) → so(30381)
su(3), su(4), su(39), su(246), su(247)
su(30381)

[{⟨1, 1⟩},{⟨30380, 1⟩}],[{⟨1, 1⟩}],[(30380)],[{⟨2, 1⟩}],[{⟨1, 2⟩}], [(245, 0),(0, 245)], [(37, 0, 1),(1, 0, 37)], [{⟨1, 2⟩, ⟨38, 1⟩},{⟨1, 1⟩, ⟨38, 2⟩}], [{⟨1, 2⟩},{⟨245, 2⟩}],[{⟨2, 1⟩},{⟨245, 1⟩}]

su(2) ← sp(15200)
so(30400) — su(30400)
su(4)

[{⟨1, 1⟩},{⟨30399, 1⟩}],[{⟨1, 1⟩}],[(30399)],[{⟨1, 1⟩}],[(3, 14, 0),(0, 14, 3)]

- su(2) ← sp(15228) ← su(30456)
- so(30456) ← su(30456)
- su(3) ← su(30456)

[{⟨1, 1⟩},{⟨30455, 1⟩}],[{⟨1, 1⟩}],[(30455)],[{⟨1, 1⟩}], [(140, 2),(2, 140)]

---

- su(2) ← sp(15232) ← su(30464)
- so(17) ← so(30464) ← su(30464)
- su(4) ← su(30464)

[{⟨1, 1⟩},{⟨30463, 1⟩}],[{⟨1, 1⟩}],[(30463)],[{⟨1, 1⟩}], [{⟨2, 1⟩, ⟨8, 1⟩}],[(15, 0, 6),(6, 0, 15)]

---

- su(2) ← sp(15249) ← su(30498)
- so(30498) ← su(30498)
- su(3) ← su(30498)

[{⟨1, 1⟩},{⟨30497, 1⟩}],[{⟨1, 1⟩}],[(30497)],[{⟨1, 1⟩}], [(51, 16),(16, 51)]

---

- su(2) ← sp(15255) ← su(30510)
- so(30510) ← su(30510)
- su(3) ← su(30510)

[{⟨1, 1⟩},{⟨30509, 1⟩}],[{⟨1, 1⟩}],[(30509)],[{⟨1, 1⟩}], [(107, 4),(4, 107)]

---

- su(2) ← so(30537) ← su(30537)
- su(3) ← su(30537)

[{⟨1, 1⟩},{⟨30536, 1⟩}], [{⟨1, 1⟩}], [(30536)], [(77, 8), (8, 77)]

---

- su(2) ← sp(15276) ← su(30552)
- so(30552) ← su(30552)
- su(3) ← su(30552)

[{⟨1, 1⟩},{⟨30551, 1⟩}],[{⟨1, 1⟩}],[(30551)],[{⟨1, 1⟩}], [(47, 18),(18, 47)]

---

- su(2) ← so(30555) ← su(30555)
- su(3) ← su(30555)

[{⟨1, 1⟩},{⟨30554, 1⟩}], [{⟨1, 1⟩}], [(30554)], [(89, 6), (6, 89)]

---

- su(2) ← sp(15288) ← su(30576)
- so(8) ← so(30576) ← su(30576)
- su(3) ← su(30576)
- su(5) ← su(30576)

[{⟨1, 1⟩},{⟨30575, 1⟩}],[{⟨1, 1⟩}],[(30575)],[{⟨1, 1⟩}], [(1, 3, 1, 0),(1, 3, 0, 1),(0, 3, 1, 1)], [(97, 5),(5, 97)], [(5, 5, 0, 0),(0, 0, 5, 5)]

---

- su(2) ← sp(15295) ← su(30590)
- so(30590) ← su(30590)
- su(5) ← su(30590)
- su(20) ← su(30590)

[{⟨1, 1⟩},{⟨30589, 1⟩}],[{⟨1, 1⟩}],[(30589)],[{⟨1, 1⟩}], [(18, 0, 0, 1),(1, 0, 0, 18)], [{⟨1, 3⟩, ⟨19, 1⟩},{⟨1, 1⟩, ⟨19, 3⟩}]

---

- su(2) ← sp(15300) ← su(30600)
- so(30600) ← su(30600)
- su(3) ← su(30600)

[{⟨1, 1⟩},{⟨30599, 1⟩}],[{⟨1, 1⟩}],[(30599)],[{⟨1, 1⟩}], [(49, 17),(17, 49)]

---

- su(2) ← sp(15309) ← su(30618)
- su(8) ← so(30618) ← su(30618)
- su(3) ← su(30618)

[{⟨1, 1⟩},{⟨30617, 1⟩}],[{⟨1, 1⟩}],[(30617)],[{⟨1, 1⟩}], [{⟨2, 1⟩, ⟨4, 1⟩, ⟨6, 1⟩}],[(35, 26),(26, 35)]

---

- su(2) ← sp(15312) ← su(30624)
- su(175) ← so(30624) ← su(30624)
- su(3) ← su(30624)
- su(4) ← su(30624)

[{⟨1, 1⟩},{⟨30623, 1⟩}],[{⟨1, 1⟩}],[(30623)],[{⟨1, 1⟩}], [{⟨1, 1⟩, ⟨174, 1⟩}], [(173, 1),(1, 173)], [(28, 2, 0),(0, 2, 28)]

---

- su(2) ← so(30625) ← su(30625)
- su(5) ← su(30625)

[{⟨1, 1⟩},{⟨30624, 1⟩}], [{⟨1, 1⟩}], [(30624)], [(4, 1, 2, 1),(1, 2, 1, 4)]

---

- su(2) ← so(30627) ← su(30627)
- so(247) ← so(30627) ← su(30627)
- sp(124) ← so(30627) ← su(30627)

[{⟨1, 1⟩},{⟨30626, 1⟩}],[{⟨1, 1⟩}],[(30626)],[{⟨1, 2⟩}], [{⟨2, 1⟩}]

---

- su(2) ← sp(15314) ← su(30628)
- so(248) ← so(30628) ← su(30628)
- su(3) ← su(30628)
- su(247) ← su(30628)
- su(248) ← su(30628)

[{⟨1, 1⟩},{⟨30627, 1⟩}],[{⟨1, 1⟩}],[(30627)],[{⟨1, 1⟩}], [{⟨2, 1⟩}], [(246, 0),(0, 246)], [{⟨1, 2⟩},{⟨246, 2⟩}], [{⟨2, 1⟩},{⟨246, 1⟩}]

---

- su(2) ← sp(15360) ← su(30720)
- sp(2) ← sp(15360) ← su(30720)
- so(30720) ← su(30720)
- su(3) ← su(30720)
- su(4) ← su(30720)

[{⟨1, 1⟩},{⟨30719, 1⟩}], [{⟨1, 1⟩}], [(30719)], [(31, 3)], [{⟨1, 1⟩}],[(39, 23),(23, 39)],[(7, 7, 1),(1, 7, 7)]

---

- su(2) ← sp(15370) ← su(30740)
- so(5) ← so(30740) ← su(30740)

[{⟨1, 1⟩},{⟨30739, 1⟩}],[{⟨1, 1⟩}],[(30739)],[{⟨1, 1⟩}], [(23, 4)]

---

- su(2) ← sp(15372) ← su(30744)
- so(30744) ← su(30744)
- su(3) ← su(30744)

[{⟨1, 1⟩},{⟨30743, 1⟩}],[{⟨1, 1⟩}],[(30743)],[{⟨1, 1⟩}], [(121, 3),(3, 121)]

---

- su(2) ← so(30745) ← su(30745)
- su(3) ← su(30745)

[{⟨1, 1⟩},{⟨30744, 1⟩}], [{⟨1, 1⟩}], [(30744)], [(42, 21), (21, 42)]

---

- su(2) ← sp(15390) ← su(30780)
- so(30780) ← su(30780)
- su(3) ← su(30780)

[{⟨1, 1⟩},{⟨30779, 1⟩}],[{⟨1, 1⟩}],[(30779)],[{⟨1, 1⟩}], [(56, 14),(14, 56)]

---

- su(2) ← sp(15399) ← su(30798)
- sp(29) ← sp(15399) ← su(30798)
- so(30798) ← su(30798)

[{⟨1, 1⟩},{⟨30797, 1⟩}],[{⟨1, 1⟩}],[(30797)],[{⟨3, 1⟩}], [{⟨1, 1⟩}]

---

- su(2) ← sp(15400) ← su(30800)
- sp(2) ← sp(15400) ← su(30800)
- so(56) ← so(30800) ← su(30800)
- su(7) ← su(30800)
- su(8) ← su(30800)
- so(10) ← su(30800)

[{⟨1, 1⟩},{⟨30799, 1⟩}], [{⟨1, 1⟩}], [(30799)], [(5, 21)], [{⟨1, 1⟩}], [{⟨1, 3⟩}], [{⟨1, 3⟩, ⟨4, 1⟩, ⟨5, 1⟩},{⟨2, 1⟩, ⟨3, 1⟩, ⟨6, 3⟩}], [{⟨1, 2⟩, ⟨5, 1⟩, ⟨6, 1⟩},{⟨2, 1⟩, ⟨3, 1⟩, ⟨7, 2⟩}],[(0, 0, 2, 1, 0),(0, 0, 2, 0, 1)]

---

- su(2) ← so(30855) ← su(30855)
- so(6) ← so(30855) ← su(30855)

[{⟨1, 1⟩},{⟨30854, 1⟩}],[{⟨1, 1⟩}],[(30854)],[(4, 5, 5)]

---

- su(2) ← sp(15428) ← su(30856)
- sp(2) ← sp(15428) ← su(30856)
- sp(28) ← sp(15428) ← su(30856)
- so(58) ← so(30856) ← su(30856)
- su(4) ← su(30856)
- su(56) ← su(30856)
- su(58) ← su(30856)

[{⟨1, 1⟩},{⟨30855, 1⟩}], [{⟨1, 1⟩}], [(30855)], [(55, 0)], [{⟨1, 3⟩}], [{⟨1, 1⟩}], [{⟨3, 1⟩}], [(55, 0, 0),(0, 0, 55)], [{⟨1, 3⟩},{⟨55, 3⟩}],[{⟨3, 1⟩},{⟨55, 1⟩}]

---

- su(2) ← sp(15435) ← su(30870)
- so(30870) ← su(30870)
- su(3) ← su(30870)
- su(5) ← su(30870)
- su(6) ← su(30870)
- su(7) ← su(30870)

[{⟨1, 1⟩},{⟨30869, 1⟩}],[{⟨1, 1⟩}],[(30869)],[{⟨1, 1⟩}], [(34, 27),(27, 34)], [(5, 0, 1, 4),(4, 1, 0, 5)], [(1, 0, 3, 1, 0),(0, 1, 3, 0, 1)], [{⟨1, 1⟩, ⟨4, 2⟩, ⟨5, 1⟩},{⟨2, 1⟩, ⟨3, 2⟩, ⟨6, 1⟩}]

---

- su(2) ← so(30875) ← su(30875)
- so(248) ← so(30875) ← su(30875)

[{⟨1, 1⟩},{⟨30874, 1⟩}],[{⟨1, 1⟩}],[(30874)],[{⟨1, 2⟩}]

---

- su(2) ← sp(15438) ← su(30876)
- so(249) ← so(30876) ← su(30876)
- sp(124) ← so(30876) ← su(30876)
- su(3) ← su(30876)
- su(248) ← su(30876)
- su(249) ← su(30876)

[{⟨1, 1⟩},{⟨30875, 1⟩}],[{⟨1, 1⟩}],[(30875)],[{⟨1, 1⟩}], [{⟨2, 1⟩}], [{⟨1, 2⟩}], [(247, 0),(0, 247)], [{⟨1, 2⟩},{⟨247, 2⟩}],[{⟨2, 1⟩},{⟨247, 1⟩}]

---

- su(2) ← so(30885) ← su(30885)
- su(3) ← su(30885)

[{⟨1, 1⟩},{⟨30884, 1⟩}], [{⟨1, 1⟩}], [(30884)], [(141, 2), (2, 141)]

---

- su(2) ← sp(15444) ← su(30888)
- so(9) ← so(30888) ← su(30888)
- su(3) ← su(30888)
- su(9) ← su(30888)

[{⟨1, 1⟩},{⟨30887, 1⟩}],[{⟨1, 1⟩}],[(30887)],[{⟨1, 1⟩}], [(10, 0, 0, 0)], [(65, 11),(11, 65)], [{⟨1, 3⟩, ⟨2, 2⟩},{⟨7, 2⟩, ⟨8, 3⟩}]

---

- su(2) ← sp(15456) ← su(30912)
- so(30912) ← su(30912)
- su(3) ← su(30912)

[{⟨1, 1⟩},{⟨30911, 1⟩}],[{⟨1, 1⟩}],[(30911)],[{⟨1, 1⟩}], [(83, 7),(7, 83)]

---

- su(2) ← sp(15470) ← su(30940)
- so(7) ← so(8) ← so(30940) ← su(30940)
- su(4) ← su(30940)
- su(4) ← su(30940)
- su(4) ← su(30940)

[{⟨1, 1⟩},{⟨30939, 1⟩}],[{⟨1, 1⟩}],[(30939)],[{⟨1, 1⟩}], [(12, 0, 0, 0),(0, 0, 12, 0),(0, 0, 0, 12)], [(0, 0, 12)], [(3, 9, 2),(2, 9, 3)],[(6, 5, 3),(3, 5, 6)],[(12, 3, 2),(2, 3, 12)]

---

- su(2) ← so(30975) ← su(30975)
- su(176) ← so(30975) ← su(30975)
- su(3) ← su(30975)

[{⟨1, 1⟩},{⟨30974, 1⟩}], [{⟨1, 1⟩}], [(30974)], [{⟨1, 1⟩, ⟨175, 1⟩}],[(174, 1),(1, 174)]

su(2), so(28) ← so(31059)
so(31059), su(3) ← su(31059)

[{⟨1, 1⟩},{⟨31058, 1⟩}], [{⟨1, 1⟩}], [(31058)], [{⟨1, 4⟩}], [(33, 28),(28, 33)]

su(2) ← so(31065)
so(31065), su(3) ← su(31065)

[{⟨1, 1⟩},{⟨31064, 1⟩}], [{⟨1, 1⟩}], [(31064)], [(108, 4), (4, 108)]

su(2), sp(2) ← sp(15540)
sp(15540), so(31080), su(3), su(3) ← su(31080)

[{⟨1, 1⟩},{⟨31079, 1⟩}], [{⟨1, 1⟩}], [(31079)], [(1, 34)], [{⟨1, 1⟩}], [(59, 13),(13, 59)], [(73, 9),(9, 73)]

su(2) ← sp(15561)
sp(15561), so(31122), su(3) ← su(31122)

[{⟨1, 1⟩},{⟨31121, 1⟩}], [{⟨1, 1⟩}], [(31121)], [{⟨1, 1⟩}], [(62, 12),(12, 62)]

su(2) ← sp(15562)
so(249), sp(125) ← so(31124)
sp(15562), so(31124) ← su(31124)

[{⟨1, 1⟩},{⟨31123, 1⟩}], [{⟨1, 1⟩}], [(31123)], [{⟨1, 1⟩}], [{⟨1, 2⟩}], [{⟨2, 1⟩}]

su(2), so(250) ← so(31125)
so(31125), su(3), su(249), su(250) ← su(31125)

[{⟨1, 1⟩},{⟨31124, 1⟩}], [{⟨1, 1⟩}], [(31124)], [{⟨2, 1⟩}], [(248, 0),(0, 248)], [{⟨1, 2⟩},{⟨248, 2⟩}], [{⟨2, 1⟩}, {⟨248, 1⟩}]

su(2) ← sp(15580)
sp(15580), so(31160), su(4), su(40) ← su(31160)

[{⟨1, 1⟩},{⟨31159, 1⟩}], [{⟨1, 1⟩}], [(31159)], [{⟨1, 1⟩}], [(37, 1, 0),(0, 1, 37)], [{⟨1, 1⟩, ⟨38, 1⟩},{⟨2, 1⟩, ⟨39, 1⟩}]

su(2), so(5) ← so(31185)
so(31185), su(3), su(3), su(3), su(3), su(4), su(5), su(5), su(6), su(10) ← su(31185)

[{⟨1, 1⟩},{⟨31184, 1⟩}], [{⟨1, 1⟩}], [(31184)], [(29, 2)], [(32, 29),(29, 32)], [(44, 20),(20, 44)], [(69, 10),(10, 69)], [(98, 5),(5, 98)], [(20, 0, 4),(4, 0, 20)], [(1, 3, 2, 1),(1, 2, 3, 1)], [(1, 6, 1, 0),(0, 1, 6, 1)], [(5, 0, 1, 1, 0),(0, 1, 1, 0, 5)], [{⟨1, 1⟩, ⟨7, 1⟩, ⟨8, 1⟩},{⟨2, 1⟩, ⟨3, 1⟩, ⟨9, 1⟩}]

su(2) ← sp(15600)
so(7) ← so(31200)
sp(15600), so(31200), su(3), su(5) ← su(31200)

[{⟨1, 1⟩},{⟨31199, 1⟩}], [{⟨1, 1⟩}], [(31199)], [{⟨1, 1⟩}], [(4, 2, 1)], [(38, 24),(24, 38)], [(4, 2, 0, 3),(3, 0, 2, 4)]

su(2) ← so(31213)
so(31213), su(3) ← su(31213)

[{⟨1, 1⟩},{⟨31212, 1⟩}], [{⟨1, 1⟩}], [(31212)], [(90, 6), (6, 90)]

su(2) ← sp(15620)
sp(15620), so(31240), su(3) ← su(31240)

[{⟨1, 1⟩},{⟨31239, 1⟩}], [{⟨1, 1⟩}], [(31239)], [{⟨1, 1⟩}], [(54, 15),(15, 54)]

su(2) ← sp(15621)
sp(15621), so(31242), su(3) ← su(31242)

[{⟨1, 1⟩},{⟨31241, 1⟩}], [{⟨1, 1⟩}], [(31241)], [{⟨1, 1⟩}], [(122, 3),(3, 122)]

su(2) ← sp(15624)
sp(15624), so(31248), su(3) ← su(31248)

[{⟨1, 1⟩},{⟨31247, 1⟩}], [{⟨1, 1⟩}], [(31247)], [{⟨1, 1⟩}], [(31, 30),(30, 31)]

su(2) ← sp(15642)
sp(15642), so(31284), su(3) ← su(31284)

[{⟨1, 1⟩},{⟨31283, 1⟩}], [{⟨1, 1⟩}], [(31283)], [{⟨1, 1⟩}], [(78, 8),(8, 78)]

su(2) ← so(31317)
so(31317), su(3) ← su(31317)

[{⟨1, 1⟩},{⟨31316, 1⟩}], [{⟨1, 1⟩}], [(31316)], [(142, 2), (2, 142)]

su(2) ← sp(15664)
su(177) ← so(31328)
sp(15664), so(31328), su(3) ← su(31328)

[{⟨1, 1⟩},{⟨31327, 1⟩}], [{⟨1, 1⟩}], [(31327)], [{⟨1, 1⟩}], [{⟨1, 1⟩, ⟨176, 1⟩}], [(175, 1),(1, 175)]

su(2) ← sp(15675)
sp(15675), so(31350), su(4) ← su(31350)

[{⟨1, 1⟩},{⟨31349, 1⟩}], [{⟨1, 1⟩}], [(31349)], [{⟨1, 1⟩}], [(8, 9, 0),(0, 9, 8)]

su(2), su(6) ← sp(15680)
sp(15680), so(31360) ← su(31360)

[{⟨1, 1⟩},{⟨31359, 1⟩}], [{⟨1, 1⟩}], [(31359)], [(3, 0, 1, 0, 3)], [{⟨1, 1⟩}]

su(2) ← sp(15687)
so(250) ← so(31374)
sp(15687), so(31374) ← su(31374)

[{⟨1, 1⟩},{⟨31373, 1⟩}], [{⟨1, 1⟩}], [(31373)], [{⟨1, 1⟩}], [{⟨1, 2⟩}]

su(2), so(251), sp(125) ← so(31375)
so(31375), su(3), su(250), su(251) ← su(31375)

[{⟨1, 1⟩},{⟨31374, 1⟩}], [{⟨1, 1⟩}], [(31374)], [{⟨2, 1⟩}], [{⟨1, 2⟩}], [(249, 0),(0, 249)], [{⟨1, 2⟩},{⟨249, 2⟩}], [{⟨2, 1⟩},{⟨249, 1⟩}]

su(2), so(5), so(7), so(22) ← so(31395)
so(31395), su(3), su(4), su(4) ← su(31395)

[{⟨1, 1⟩},{⟨31394, 1⟩}], [{⟨1, 1⟩}], [(31394)], [(44, 0)], [(8, 0, 2)], [{⟨1, 2⟩, ⟨2, 1⟩}], [(41, 22),(22, 41)], [(12, 0, 8),(8, 0, 12)], [(20, 1, 2),(2, 1, 20)]

su(2) ← sp(15708)
sp(15708), so(31416), su(4) ← su(31416)

[{⟨1, 1⟩},{⟨31415, 1⟩}], [{⟨1, 1⟩}], [(31415)], [{⟨1, 1⟩}], [(5, 7, 2),(2, 7, 5)]

su(2), sp(2) ← sp(15732)
sp(15732), so(31464) ← su(31464)

[{⟨1, 1⟩},{⟨31463, 1⟩}], [{⟨1, 1⟩}], [(31463)], [(7, 18)], [{⟨1, 1⟩}]

su(2), so(31), sp(14) ← so(31465)
so(31465), su(5), su(28), su(31) ← su(31465)

[{⟨1, 1⟩},{⟨31464, 1⟩}], [{⟨1, 1⟩}], [(31464)], [{⟨4, 1⟩}], [{⟨1, 4⟩}], [(27, 0, 0, 0),(0, 0, 0, 27)], [{⟨1, 4⟩}, {⟨27, 4⟩}], [{⟨4, 1⟩},{⟨27, 1⟩}]

su(2) ← sp(15745)
sp(15745), so(31490), su(3) ← su(31490)

[{⟨1, 1⟩},{⟨31489, 1⟩}], [{⟨1, 1⟩}], [(31489)], [{⟨1, 1⟩}], [(46, 19),(19, 46)]

su(2) ← sp(15750)
so(9) ← so(31500)
sp(15750), so(31500) ← su(31500)

[{⟨1, 1⟩},{⟨31499, 1⟩}], [{⟨1, 1⟩}], [(31499)], [{⟨1, 1⟩}], [(2, 1, 1, 0)]

su(2) ← so(31535)
so(31535), su(3) ← su(31535)

[{⟨1, 1⟩},{⟨31534, 1⟩}], [{⟨1, 1⟩}], [(31534)], [(52, 16), (16, 52)]

su(2) ← sp(15795)
so(5) ← so(31590)
sp(15795), so(31590), su(4), su(5) ← su(31590)

[{⟨1, 1⟩},{⟨31589, 1⟩}], [{⟨1, 1⟩}], [(31589)], [{⟨1, 1⟩}], [(11, 14)], [(8, 3, 4),(4, 3, 8)], [(8, 2, 0, 1),(1, 0, 2, 8)]

su(2), sp(2) ← sp(15808)
sp(15808), so(31616), su(3) ← su(31616)

[{⟨1, 1⟩},{⟨31615, 1⟩}], [{⟨1, 1⟩}], [(31615)], [(25, 5)], [{⟨1, 1⟩}], [(37, 25),(25, 37)]

su(2) ← sp(15810)
sp(15810), so(31620), su(3), su(4) ← su(31620)

[{⟨1, 1⟩},{⟨31619, 1⟩}], [{⟨1, 1⟩}], [(31619)], [{⟨1, 1⟩}], [(84, 7),(7, 84)], [(29, 0, 2),(2, 0, 29)]

su(2) ←
so(23) ←
so(251) ← so(31625) ← su(31625)
sp(11) ← su(3) ←
sp(126) ←

[{⟨1, 1⟩},{⟨31624, 1⟩}], [{⟨1, 1⟩}], [(31624)], [{⟨1, 1⟩, ⟨3, 1⟩}], [{⟨1, 2⟩}], [{⟨1, 2⟩, ⟨2, 1⟩}], [{⟨2, 1⟩}], [(109, 4),(4, 109)]

---

su(2) ← sp(15813) ←
so(252) ← so(31626) ←
su(3) ← su(31626)
su(251) ←
su(252) ←

[{⟨1, 1⟩},{⟨31625, 1⟩}],[{⟨1, 1⟩}],[(31625)],[{⟨1, 1⟩}], [{⟨2, 1⟩}], [(250, 0),(0, 250)], [{⟨1, 2⟩},{⟨250, 2⟩}], [{⟨2, 1⟩},{⟨250, 1⟩}]

---

su(2) ← sp(15827) ←
so(31654) ← su(31654)
su(3) ←

[{⟨1, 1⟩},{⟨31653, 1⟩}],[{⟨1, 1⟩}],[(31653)],[{⟨1, 1⟩}], [(48, 18),(18, 48)]

---

su(2) ← so(31671) ← su(31671)
su(3) ←

[{⟨1, 1⟩},{⟨31670, 1⟩}], [{⟨1, 1⟩}], [(31670)], [(50, 17), (17, 50)]

---

su(2) ← sp(15840) ←
sp(4) ← su(31680)
so(10) ← so(31680) ←

[{⟨1, 1⟩},{⟨31679, 1⟩}], [{⟨1, 1⟩}], [(31679)], [(1, 2, 0, 1)],[{⟨1, 1⟩}],[(5, 1, 0, 0, 0)]

---

su(2) ← so(31683) ← su(31683)
su(178) ←
su(3) ←

[{⟨1, 1⟩},{⟨31682, 1⟩}], [{⟨1, 1⟩}], [(31682)], [{⟨1, 1⟩, ⟨177, 1⟩}],[(176, 1),(1, 176)]

---

su(2) ← sp(15872) ←
so(31744) ← su(31744)
su(3) ←

[{⟨1, 1⟩},{⟨31743, 1⟩}],[{⟨1, 1⟩}],[(31743)],[{⟨1, 1⟩}], [(123, 3),(3, 123)]

---

su(2) ← sp(15876) ←
so(31752) ←
su(3) ← su(31752)
su(6) ←
su(7) ←
su(8) ←

[{⟨1, 1⟩},{⟨31751, 1⟩}],[{⟨1, 1⟩}],[(31751)],[{⟨1, 1⟩}], [(143, 2),(2, 143)],[(1, 0, 2, 2, 0),(0, 2, 2, 0, 1)],[{⟨2, 2⟩, ⟨3, 2⟩},{⟨4, 2⟩, ⟨5, 2⟩}], [{⟨2, 1⟩, ⟨4, 2⟩},{⟨4, 2⟩, ⟨6, 1⟩}]

---

su(2) ← so(31755) ← su(31755)
su(3) ←

[{⟨1, 1⟩},{⟨31754, 1⟩}], [{⟨1, 1⟩}], [(31754)], [(57, 14), (14, 57)]

---

su(2) ← sp(15879) ←
so(31758) ← su(31758)
su(3) ←

[{⟨1, 1⟩},{⟨31757, 1⟩}],[{⟨1, 1⟩}],[(31757)],[{⟨1, 1⟩}], [(66, 11),(11, 66)]

---

su(2) ← sp(15900) ←
so(31800) ← su(31800)
su(3) ←

[{⟨1, 1⟩},{⟨31799, 1⟩}],[{⟨1, 1⟩}],[(31799)],[{⟨1, 1⟩}], [(99, 5),(5, 99)]

---

su(2) ← sp(15910) ← su(31820)
so(5) ← so(31820) ←

[{⟨1, 1⟩},{⟨31819, 1⟩}],[{⟨1, 1⟩}],[(31819)],[{⟨1, 1⟩}], [(2, 36)]

---

su(2) ←
sp(4) ← sp(15912) ←
sp(6) ←
so(18) ← so(31824) ← su(31824)
su(8) ←
su(12) ←
su(18) ←

[{⟨1, 1⟩},{⟨31823, 1⟩}], [{⟨1, 1⟩}], [(31823)], [(11, 0, 0, 0)], [{⟨1, 7⟩}], [{⟨1, 1⟩}], [{⟨7, 1⟩}], [{⟨1, 11⟩},{⟨7, 11⟩}],[{⟨1, 7⟩},{⟨11, 7⟩}],[{⟨7, 1⟩},{⟨11, 1⟩}]

---

su(2) ← sp(15925) ←
so(31850) ← su(31850)
su(5) ←
su(14) ←

[{⟨1, 1⟩},{⟨31849, 1⟩}],[{⟨1, 1⟩}],[(31849)],[{⟨1, 1⟩}], [(7, 4, 0, 0),(0, 0, 4, 7)], [{⟨2, 1⟩, ⟨11, 1⟩},{⟨3, 1⟩, ⟨12, 1⟩}]

---

su(2) ← so(31875) ← su(31875)
su(3) ←

[{⟨1, 1⟩},{⟨31874, 1⟩}], [{⟨1, 1⟩}], [(31874)], [(74, 9), (9, 74)]

---

su(2) ← so(31877) ← su(31877)
so(252) ←

[{⟨1, 1⟩},{⟨31876, 1⟩}],[{⟨1, 1⟩}],[(31876)],[{⟨1, 2⟩}]

---

su(2) ← sp(15939) ←
so(253) ← so(31878) ←
sp(126) ←
su(3) ← su(31878)
su(3) ←
su(252) ←
su(22) ← su(253) ←
su(23) ←

[{⟨1, 1⟩},{⟨31877, 1⟩}],[{⟨1, 1⟩}],[(31877)],[{⟨1, 1⟩}], [{⟨2, 1⟩}], [{⟨1, 2⟩}], [(91, 6),(6, 91)], [(251, 0),(0, 251)], [{⟨1, 2⟩},{⟨251, 2⟩}], [{⟨2, 1⟩},{⟨251, 1⟩}], [{⟨1, 2⟩, ⟨2, 1⟩},{⟨20, 1⟩, ⟨21, 2⟩}], [{⟨1, 1⟩, ⟨3, 1⟩},{⟨20, 1⟩, ⟨22, 1⟩}]

---

su(2) ← sp(15960) ← su(31920)
sp(2) ←
so(31920) ←

[{⟨1, 1⟩},{⟨31919, 1⟩}], [{⟨1, 1⟩}], [(31919)], [(17, 9)], [{⟨1, 1⟩}]

---

su(2) ← sp(15972) ←
so(31944) ← su(31944)
su(3) ←

[{⟨1, 1⟩},{⟨31943, 1⟩}],[{⟨1, 1⟩}],[(31943)],[{⟨1, 1⟩}], [(43, 21),(21, 43)]

---

su(2) ← sp(15984) ←
so(31968) ← su(31968)
su(3) ←

[{⟨1, 1⟩},{⟨31967, 1⟩}],[{⟨1, 1⟩}],[(31967)],[{⟨1, 1⟩}], [(36, 26),(26, 36)]

---

su(2) ← sp(15990) ←
so(31980) ← su(31980)
su(3) ←

[{⟨1, 1⟩},{⟨31979, 1⟩}],[{⟨1, 1⟩}],[(31979)],[{⟨1, 1⟩}], [(40, 23),(23, 40)]

---

su(2) ← sp(16000) ←
so(32000) ← su(32000)
su(4) ←

[{⟨1, 1⟩},{⟨31999, 1⟩}],[{⟨1, 1⟩}],[(31999)],[{⟨1, 1⟩}], [(9, 1, 7),(7, 1, 9)]

---

su(2) ← so(32021) ← su(32021)
su(3) ←

[{⟨1, 1⟩},{⟨32020, 1⟩}], [{⟨1, 1⟩}], [(32020)], [(70, 10), (10, 70)]

---

su(2) ← so(32025) ← su(32025)
su(3) ←

[{⟨1, 1⟩},{⟨32024, 1⟩}], [{⟨1, 1⟩}], [(32024)], [(60, 13), (13, 60)]

---

su(2) ← sp(16016) ←
so(12) ←
so(7) ← so(32032) ←
so(8) ← su(32032)
su(3) ←
su(7) ←
su(11) ←

[{⟨1, 1⟩},{⟨32031, 1⟩}], [{⟨1, 1⟩}], [(32031)], [{⟨1, 4⟩, ⟨5, 1⟩},{⟨1, 4⟩, ⟨6, 1⟩}], [{⟨1, 1⟩}], [(1, 0, 9)], [(5, 0, 3, 0),(5, 0, 0, 3),(3, 0, 5, 0),(3, 0, 0, 5),(0, 0, 5, 3),(0, 0, 3, 5)], [(63, 12),(12, 63)], [{⟨1, 9⟩, ⟨6, 1⟩},{⟨1, 1⟩, ⟨6, 9⟩}],[{⟨1, 5⟩, ⟨10, 1⟩},{⟨1, 1⟩, ⟨10, 5⟩}]

---

su(2) ← sp(16020) ←
su(179) ← so(32040) ← su(32040)
su(3) ←
su(3) ←

[{⟨1, 1⟩},{⟨32039, 1⟩}],[{⟨1, 1⟩}],[(32039)],[{⟨1, 1⟩}], [{⟨1, 1⟩, ⟨178, 1⟩}],[(79, 8),(8, 79)],[(177, 1),(1, 177)]

---

su(2) ← so(32045) ← su(32045)
so(5) ←

[{⟨1, 1⟩},{⟨32044, 1⟩}],[{⟨1, 1⟩}],[(32044)],[(4, 28)]

---

su(2) ← sp(16038) ←
so(32076) ← su(32076)
su(5) ←
su(9) ←

[{⟨1, 1⟩},{⟨32075, 1⟩}],[{⟨1, 1⟩}],[(32075)],[{⟨1, 1⟩}], [(2, 5, 1, 0),(0, 1, 5, 2)], [{⟨1, 2⟩, ⟨2, 1⟩, ⟨7, 1⟩},{⟨2, 1⟩, ⟨7, 1⟩, ⟨8, 2⟩}]

---

su(2) ← sp(16065) ←
so(253) ← so(32130) ←
sp(127) ←
su(4) ← su(32130)
su(4) ←
su(5) ←
su(19) ←

[{⟨1, 1⟩},{⟨32129, 1⟩}],[{⟨1, 1⟩}],[(32129)],[{⟨1, 1⟩}], [{⟨1, 2⟩}], [{⟨2, 1⟩}], [(2, 16, 0),(0, 16, 2)], [(4, 8, 2),(2, 8, 4)], [(16, 0, 1, 0),(0, 1, 0, 16)], [{⟨1, 2⟩, ⟨17, 1⟩}, {⟨2, 1⟩, ⟨18, 2⟩}]

---

su(2) ← so(32131) ←
so(254) ←
su(3) ← su(32131)
su(253) ←
su(254) ←

[{⟨1, 1⟩},{⟨32130, 1⟩}],[{⟨1, 1⟩}],[(32130)],[{⟨2, 1⟩}], [(252, 0),(0, 252)], [{⟨1, 2⟩},{⟨252, 2⟩}], [{⟨2, 1⟩}, {⟨252, 1⟩}]

---

su(2) ← so(32175) ← su(32175)
so(25) ←
su(5) ←

[{⟨1, 1⟩},{⟨32174, 1⟩}],[{⟨1, 1⟩}],[(32174)],[{⟨2, 2⟩}], [(1, 0, 8, 0),(0, 8, 0, 1)]

---

su(2) ← sp(16095)
so(32190)
su(3)
su(3)
su(32190)

[{⟨1, 1⟩},{⟨32189, 1⟩}],[{⟨1, 1⟩}],[(32189)],[{⟨1, 1⟩}], [(110, 4),(4, 110)],[(144, 2),(2, 144)]

---

su(2) ← sp(16125)
so(32250)
su(3)
su(32250)

[{⟨1, 1⟩},{⟨32249, 1⟩}],[{⟨1, 1⟩}],[(32249)],[{⟨1, 1⟩}], [(124, 3),(3, 124)]

---

su(2) ← sp(16128)
so(32256)
su(3)
su(3)
su(4)
su(32256)

[{⟨1, 1⟩},{⟨32255, 1⟩}],[{⟨1, 1⟩}],[(32255)],[{⟨1, 1⟩}], [(35, 27),(27, 35)], [(55, 15),(15, 55)], [(3, 11, 1),(1, 11, 3)]

---

su(2)
so(19)
so(32319) ← su(32319)

[{⟨1, 1⟩},{⟨32318, 1⟩}],[{⟨1, 1⟩}],[(32318)],[{⟨1, 5⟩}]

---

su(2) ← sp(16168)
so(32336)
su(3)
su(32336)

[{⟨1, 1⟩},{⟨32335, 1⟩}],[{⟨1, 1⟩}],[(32335)],[{⟨1, 1⟩}], [(85, 7),(7, 85)]

---

su(2)
sp(5)
sp(16170)
so(8) ← so(32340)
su(6)
su(6)
su(7)
su(7)
su(7)
su(32340)

[{⟨1, 1⟩},{⟨32339, 1⟩}],[{⟨1, 1⟩}],[(32339)],[(1, 1, 0, 1, 0)], [{⟨1, 1⟩}], [(3, 0, 3, 1),(3, 0, 1, 3),(1, 0, 3, 3)], [(3, 0, 1, 1, 1),(1, 1, 1, 0, 3)], [(3, 1, 0, 2, 0),(0, 2, 0, 1, 3)], [{⟨1, 1⟩, ⟨5, 4⟩},{⟨2, 4⟩, ⟨6, 1⟩}], [{⟨1, 3⟩, ⟨3, 1⟩, ⟨5, 1⟩},{⟨2, 1⟩, ⟨4, 1⟩, ⟨6, 3⟩}], [{⟨1, 4⟩, ⟨5, 2⟩},{⟨2, 2⟩, ⟨6, 4⟩}]

---

su(2) ← so(32361)
su(3)
su(32361)

[{⟨1, 1⟩},{⟨32360, 1⟩}], [{⟨1, 1⟩}], [(32360)], [(45, 20), (20, 45)]

---

su(2)
sp(2)
sp(16182)
so(32364)
su(4)
su(32364)

[{⟨1, 1⟩},{⟨32363, 1⟩}], [{⟨1, 1⟩}], [(32363)], [(3, 26)], [{⟨1, 1⟩}],[(26, 1, 1),(1, 1, 26)]

---

su(2)
sp(2)
sp(23)
sp(16192)
so(46)
so(254)
so(32384)
su(32384)

[{⟨1, 1⟩},{⟨32383, 1⟩}], [{⟨1, 1⟩}], [(32383)], [(43, 1)], [{⟨1, 1⟩, ⟨2, 1⟩}],[{⟨1, 1⟩}],[{⟨1, 1⟩, ⟨2, 1⟩}],[{⟨1, 2⟩}]

---

su(2)
so(255)
sp(127)
so(32385)
su(3)
su(254)
su(255)
su(32385)

[{⟨1, 1⟩},{⟨32384, 1⟩}],[{⟨1, 1⟩}],[(32384)],[{⟨2, 1⟩}], [{⟨1, 2⟩}], [(253, 0),(0, 253)], [{⟨1, 2⟩},{⟨253, 2⟩}], [{⟨2, 1⟩},{⟨253, 1⟩}]

---

su(2)
su(180)
so(32399)
su(3)
su(32399)

[{⟨1, 1⟩},{⟨32398, 1⟩}], [{⟨1, 1⟩}], [(32398)], [{⟨1, 1⟩, ⟨179, 1⟩}],[(178, 1),(1, 178)]

---

su(2) ← so(32421)
su(3)
su(32421)

[{⟨1, 1⟩},{⟨32420, 1⟩}], [{⟨1, 1⟩}], [(32420)], [(100, 5), (5, 100)]

---

su(2) ← sp(16215)
so(32430)
su(46)
su(32430)

[{⟨1, 1⟩},{⟨32429, 1⟩}],[{⟨1, 1⟩}],[(32429)],[{⟨1, 1⟩}], [{⟨1, 1⟩, ⟨2, 1⟩},{⟨44, 1⟩, ⟨45, 1⟩}]

---

su(2) ← sp(16226)
so(57) ← so(32452)
su(32452)

[{⟨1, 1⟩},{⟨32451, 1⟩}],[{⟨1, 1⟩}],[(32451)],[{⟨1, 1⟩}], [{⟨1, 3⟩}]

---

su(2) ← sp(16240)
so(32480)
su(3)
su(4)
su(32480)

[{⟨1, 1⟩},{⟨32479, 1⟩}],[{⟨1, 1⟩}],[(32479)],[{⟨1, 1⟩}], [(34, 28),(28, 34)],[(23, 3, 0),(0, 3, 23)]

---

su(2)
so(15)
so(32487) ← su(32487)

[{⟨1, 1⟩},{⟨32486, 1⟩}], [{⟨1, 1⟩}], [(32486)], [{⟨1, 3⟩, ⟨2, 1⟩}]

---

su(2) ← sp(16250)
so(6) ← so(32500)
su(3)
su(4)
su(4)
su(25)
su(32500)

[{⟨1, 1⟩},{⟨32499, 1⟩}],[{⟨1, 1⟩}],[(32499)],[{⟨1, 1⟩}], [(23, 0, 0)], [(39, 24),(24, 39)], [(19, 4, 0),(0, 4, 19)], [(24, 0, 3),(3, 0, 24)],[{⟨2, 2⟩},{⟨23, 2⟩}]

---

su(2)
so(5)
so(59)
so(32509)
su(4)
su(57)
su(59)
su(32509)

[{⟨1, 1⟩},{⟨32508, 1⟩}], [{⟨1, 1⟩}], [(32508)], [(0, 56)], [{⟨3, 1⟩}], [(56, 0, 0),(0, 0, 56)], [{⟨1, 3⟩},{⟨56, 3⟩}], [{⟨3, 1⟩},{⟨56, 1⟩}]

---

su(2) ← sp(16275)
so(32550)
su(3)
su(32550)

[{⟨1, 1⟩},{⟨32549, 1⟩}],[{⟨1, 1⟩}],[(32549)],[{⟨1, 1⟩}], [(92, 6),(6, 92)]

---

su(2) ← so(32585)
su(4)
su(32585)

[{⟨1, 1⟩},{⟨32584, 1⟩}],[{⟨1, 1⟩}],[(32584)],[(13, 4, 1), (1, 4, 13)]

---

su(2) ← so(32589)
su(3)
su(32589)

[{⟨1, 1⟩},{⟨32588, 1⟩}], [{⟨1, 1⟩}], [(32588)], [(53, 16), (16, 53)]

---

su(2) ← so(32631)
su(3)
su(32631)

[{⟨1, 1⟩},{⟨32630, 1⟩}], [{⟨1, 1⟩}], [(32630)], [(145, 2), (2, 145)]

---

su(2) ← so(32637)
su(3)
su(32637)

[{⟨1, 1⟩},{⟨32636, 1⟩}], [{⟨1, 1⟩}], [(32636)], [(42, 22), (22, 42)]

---

su(2)
so(255)
sp(128)
so(32639) ← su(32639)

[{⟨1, 1⟩},{⟨32638, 1⟩}],[{⟨1, 1⟩}],[(32638)],[{⟨1, 2⟩}], [{⟨2, 1⟩}]

---

su(2) ← sp(16320)
so(256) ← so(32640)
su(3)
su(3)
su(3)
su(3)
su(255)
su(256)
su(32640)

[{⟨1, 1⟩},{⟨32639, 1⟩}],[{⟨1, 1⟩}],[(32639)],[{⟨1, 1⟩}], [{⟨2, 1⟩}], [(33, 29),(29, 33)], [(47, 19),(19, 47)], [(67, 11),(11, 67)], [(254, 0),(0, 254)], [{⟨1, 2⟩},{⟨254, 2⟩}], [{⟨2, 1⟩},{⟨254, 1⟩}]

---

su(2) ← sp(16335)
so(6) ← so(32670)
su(6)
su(9)
su(11)
su(32670)

[{⟨1, 1⟩},{⟨32669, 1⟩}],[{⟨1, 1⟩}],[(32669)],[{⟨1, 1⟩}], [(1, 8, 8)], [(0, 7, 0, 0, 0),(0, 0, 0, 7, 0)], [{⟨2, 4⟩},{⟨7, 4⟩}],[{⟨4, 2⟩},{⟨7, 2⟩}]

---

su(2) ← sp(16340)
so(32680)
su(3)
su(32680)

[{⟨1, 1⟩},{⟨32679, 1⟩}],[{⟨1, 1⟩}],[(32679)],[{⟨1, 1⟩}], [(75, 9),(9, 75)]

---

su(2)
so(9)
sp(3)
so(32725)
su(4)
su(5)
su(32725)

[{⟨1, 1⟩},{⟨32724, 1⟩}], [{⟨1, 1⟩}], [(32724)], [(4, 0, 0, 2)], [(4, 4, 0)], [(14, 1, 4),(4, 1, 14)], [(9, 0, 0, 4),(4, 0, 0, 9)]

---

su(2) ← sp(16368)
so(32736)
su(3)
su(32736)

[{⟨1, 1⟩},{⟨32735, 1⟩}],[{⟨1, 1⟩}],[(32735)],[{⟨1, 1⟩}], [(32, 30),(30, 32)]

---

su(2) ← so(32745)
su(3)
su(32745)

[{⟨1, 1⟩},{⟨32744, 1⟩}], [{⟨1, 1⟩}], [(32744)], [(58, 14), (14, 58)]

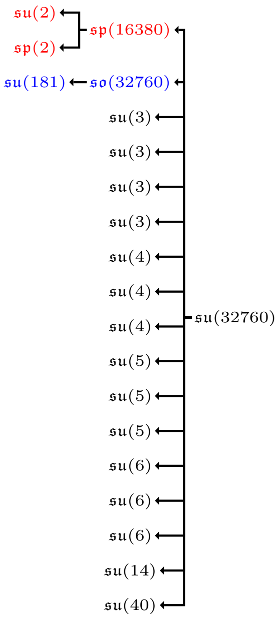


[{⟨1, 1⟩},{⟨32759, 1⟩}], [{⟨1, 1⟩}], [(32759)], [(13, 12)], [{⟨1, 1⟩}], [{⟨1, 1⟩, ⟨180, 1⟩}], [(51, 17),(17, 51)], [(111, 4),(4, 111)], [(125, 3),(3, 125)], [(179, 1),(1, 179)], [(12, 1, 5),(5, 1, 12)], [(20, 2, 1),(1, 2, 20)], [(38, 0, 1),(1, 0, 38)], [(4, 0, 2, 3),(3, 2, 0, 4)], [(5, 3, 1, 0),(0, 1, 3, 5)], [(11, 0, 0, 3),(3, 0, 0, 11)], [(5, 1, 0, 0, 2),(2, 0, 0, 1, 5)], [(6, 0, 0, 2, 0),(0, 2, 0, 0, 6)], [(12, 0, 0, 0, 1),(1, 0, 0, 0, 12)], [{⟨1, 4⟩, ⟨13, 1⟩},{⟨1, 1⟩, ⟨13, 4⟩}], [{⟨1, 2⟩, ⟨39, 1⟩},{⟨1, 1⟩, ⟨39, 2⟩}]

---

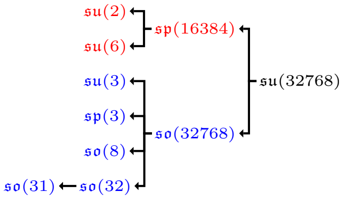


[{⟨1, 1⟩},{⟨32767, 1⟩}], [{⟨1, 1⟩}], [(32767)], [(1, 1, 1, 1, 1)], [{⟨1, 1⟩}], [(31, 31)], [(3, 3, 1)], [(3, 1, 1, 1),(1, 1, 3, 1),(1, 1, 1, 3)], [{⟨15, 1⟩},{⟨16, 1⟩}], [{⟨15, 1⟩}]
